# Supplementary material for: The $b_1$ resonance in coupled $\pi\omega$, $\pi\phi$ scattering from lattice QCD
Source: arXiv:1904.04136 ancillary file (2019-04-08)
Supplement: Supplementary file 1 [file supplemental_material.pdf]

# **Supplemental Material**

## **$J^P = 1^+$ Amplitudes**



For coupled  $\pi\omega\{^3S_1\}$ ,  $\pi\omega\{^3D_1\}$  and  $\pi\phi\{^3S_1\}$  amplitudes, in the following we present additional figures for the phase-shifts, mixing-angles, amplitude squared magnitudes and poles. In addition, we give the scattering parameters along with the statistical uncertainties and correlations followed by the pole singularities found across the Riemann sheets and give the momenta, couplings and branching fractions.

All amplitudes are of the form,

$$K_{\ell J_a, \ell' J_b} = \frac{(g_{\ell J_a}^{(0)} + g_{\ell J_a}^{(1)} s)(g_{\ell' J_b}^{(0)} + g_{\ell' J_b}^{(1)} s)}{m^2 - s} + \gamma_{\ell J_a, \ell' J_b}^{(0)} + \gamma_{\ell J_a, \ell' J_b}^{(1)} s + \gamma_{\ell J_a, \ell' J_b}^{(2)} s^2. \quad (0.1)$$

Amplitudes have names encoding the  $K$ -matrix parameterization as follows:

- **coupled\_po\_pp.3s1\_3d1.pole+** – all begin with this which denotes that these parameterizations are, in general, coupled  $\pi\omega\{^3S_1\}$ ,  $\pi\omega\{^3D_1\}$  and  $\pi\phi\{^3S_1\}$  and all contain a pole term as shown in Eq. 0.1.
- **G0\_** – this lists non-zero elements  $\gamma_{\ell J_a, \ell' J_b}^{(0)}$ .
- **G1\_** – this lists non-zero elements  $\gamma_{\ell J_a, \ell' J_b}^{(1)}$ .
- **G2\_** – this lists non-zero elements  $\gamma_{\ell J_a, \ell' J_b}^{(2)}$ .
- **gorder0\_** – this lists non-zero elements  $g_{\ell J_a}^{(0)}$ .
- **gorder1\_** – this lists non-zero elements  $g_{\ell J_a}^{(1)}$ .

The key for the specific elements are:

- **3s1** =  $\gamma_{\pi\omega\{^3S_1\}, \pi\omega\{^3S_1\}}$  or  $g_{\pi\omega\{^3S_1\}}$  as appropriate
- **3d1** =  $\gamma_{\pi\omega\{^3D_1\}, \pi\omega\{^3D_1\}}$  or  $g_{\pi\omega\{^3S_1\}}$  as appropriate
- **3S1** =  $\gamma_{\pi\phi\{^3S_1\}, \pi\phi\{^3S_1\}}$  or  $g_{\pi\phi\{^3S_1\}}$  as appropriate
- **3sd1** =  $\gamma_{\pi\omega\{^3S_1\}, \pi\omega\{^3D_1\}}$
- **3sS1** =  $\gamma_{\pi\omega\{^3S_1\}, \pi\phi\{^3S_1\}}$
- **3dS1** =  $\gamma_{\pi\omega\{^3D_1\}, \pi\phi\{^3S_1\}}$

Regarding the phase space, we use three different prescriptions,

- **pole0\_sub** – this denotes the Chew-Mandelstam phase space with  $\text{Re}\{I_a(s = m^2) = 0\}$
- **threshold\_sub** – this denotes the Chew-Mandelstam phase space with  $\text{Re}\{I_a(s = s_a^{\text{thr}}) = 0\}$
- **irho** – this denotes  $I_a(s) = -i\rho_a(s)$



As an illustrative example, we take the parameterization,

**coupled\_po\_pp.3s1\_3d1.pole+G0\_3s1\_3S1+G1\_3s1.gorder0\_3s1\_3d1\_3S1.pole0\_sub.**

The explicit  $K$ -matrix encoded in this name is,

$$\begin{aligned} \mathbf{K}(s) = \frac{1}{m^2 - s} & \begin{pmatrix} g_{\pi\omega\{^3S_1\}}^2 & g_{\pi\omega\{^3S_1\}} g_{\pi\omega\{^3D_1\}} & g_{\pi\omega\{^3S_1\}} g_{\pi\phi\{^3S_1\}} \\ g_{\pi\omega\{^3S_1\}} g_{\pi\omega\{^3D_1\}} & g_{\pi\omega\{^3D_1\}}^2 & g_{\pi\omega\{^3D_1\}} g_{\pi\phi\{^3S_1\}} \\ g_{\pi\omega\{^3S_1\}} g_{\pi\phi\{^3S_1\}} & g_{\pi\omega\{^3D_1\}} g_{\pi\phi\{^3S_1\}} & g_{\pi\phi\{^3S_1\}}^2 \end{pmatrix} + \begin{pmatrix} \gamma_{\pi\omega\{^3S_1\},\pi\omega\{^3S_1\}}^{(0)} & 0 & 0 \\ 0 & 0 & 0 \\ 0 & 0 & \gamma_{\pi\phi\{^3S_1\},\pi\phi\{^3S_1\}}^{(0)} \end{pmatrix} \\ & + \begin{pmatrix} \gamma_{\pi\omega\{^3S_1\},\pi\omega\{^3S_1\}}^{(1)} & 0 & 0 \\ 0 & 0 & 0 \\ 0 & 0 & 0 \end{pmatrix} s \end{aligned} \quad (0.2)$$

with the Chew-Mandelstam prescription where  $\text{Re}\{I_a(s = m^2) = 0\}$ .

In Section 1 we provide the amplitudes for the successful parameterizations in Table XVI, transcribed in Table 0.1 for convenience, and in Section 2 we provide the amplitudes for the parameterizations given in Table 0.2 that had unphysical poles, i.e. poles off the real axis on the physical sheet, as discussed in the paper.

Displayed for each parameterization are first the phase-shifts and mixing-angles (left), see Figure 9 in the paper, and magnitude squared amplitudes (right), see Figure 10 in the paper. Dashed curves reflect the statistical uncertainties on the scattering parameters. The next figure shows the pole singularities in a region of the complex plane relevant for the study. For successful parameterizations given in Section 1, only sheet II and III poles appeared in this region of the complex plane and these are indistinguishable in the figures. For unphysical parameterization given in Section 2, we find sheet I poles as well as indistinguishable sheet II and III poles. After the figures, the scattering parameters, statistical uncertainties and correlations between the parameters are given. Then, we present the results of the pole analysis and show the pole location, couplings to each channel and the corresponding branching fractions using the definition given in Eq. 29 in the paper.



| Parameterization                                                                                                                                                                                                 | Further Restrictions                                                                           | Phase-space                                   | $N_{\text{pars}}$ | $\chi^2/N_{\text{dof}}$ |
|------------------------------------------------------------------------------------------------------------------------------------------------------------------------------------------------------------------|------------------------------------------------------------------------------------------------|-----------------------------------------------|-------------------|-------------------------|
| $K_{\ell J_a, \ell' J_b} = \frac{(g_{\ell J_a}^{(0)} + g_{\ell J_a}^{(1)} s)(g_{\ell' J_b}^{(0)} + g_{\ell' J_b}^{(1)} s)}{m^2 - s} + \gamma_{\ell J_a, \ell' J_b}^{(0)} + \gamma_{\ell J_a, \ell' J_b}^{(1)} s$ | $g_{\pi\phi\{^3S_1\}}^{(0)} = g_{\pi\omega\{^3S_1\}}^{(1)} = 0$                                | $I_a(s) = -i\rho_a(s)$                        |                   | 1.18                    |
|                                                                                                                                                                                                                  | $\gamma_{\pi\omega\{^3S_1\}, \pi\omega\{^3D_1\}}^{(0)} = 0$                                    | <b>CM Re<math>\{I_a(s = m^2) = 0\}</math></b> | <b>5</b>          | <b>1.19</b>             |
|                                                                                                                                                                                                                  | $\gamma_{\pi\omega\{^3S_1\}, \pi\phi\{^3S_1\}}^{(0)} = 0$                                      | CM Re $\{I_a(s = s_a^{\text{thr}}) = 0\}$     |                   | 1.19                    |
|                                                                                                                                                                                                                  | $\gamma_{\pi\omega\{^3S_1\}, \pi\omega\{^3S_1\}}^{(1)} = 0$                                    |                                               |                   |                         |
| where $\gamma_{\pi\omega\{^3D_1\}, \pi\omega\{^3D_1\}}^{(0,1)} = 0$ ,                                                                                                                                            |                                                                                                |                                               |                   |                         |
| $\gamma_{\pi\phi\{^3S_1\}, \pi\phi\{^3S_1\}}^{(1)} = 0$ ,                                                                                                                                                        | $g_{\pi\phi\{^3S_1\}}^{(0)} = g_{\pi\omega\{^3S_1\}}^{(1)} = 0$                                | $I_a(s) = -i\rho_a(s)$                        |                   | 1.22                    |
| $\gamma_{\pi\omega\{^3S_1\}, \pi\omega\{^3D_1\}}^{(1)} = 0$ ,                                                                                                                                                    | $\gamma_{\pi\omega\{^3S_1\}, \pi\phi\{^3S_1\}}^{(0)} = 0$                                      | CM Re $\{I_a(s = m^2) = 0\}$                  | 6                 | 1.22                    |
| $\gamma_{\pi\omega\{^3S_1\}, \pi\phi\{^3S_1\}}^{(1)} = 0$ ,                                                                                                                                                      | $\gamma_{\pi\omega\{^3S_1\}, \pi\omega\{^3S_1\}}^{(1)} = 0$                                    | CM Re $\{I_a(s = s_a^{\text{thr}}) = 0\}$     |                   | 1.22                    |
| $\gamma_{\pi\omega\{^3D_1\}, \pi\phi\{^3S_1\}}^{(0,1)} = 0$ ,                                                                                                                                                    |                                                                                                |                                               |                   |                         |
| $g_{\pi\omega\{^3D_1\}}^{(1)} = 0$ ,                                                                                                                                                                             | $g_{\pi\omega\{^3S_1\}}^{(1)} = 0$                                                             | $I_a(s) = -i\rho_a(s)$                        |                   | 1.27                    |
| $g_{\pi\phi\{^3S_1\}}^{(1)} = 0$ ,                                                                                                                                                                               | $\gamma_{\pi\omega\{^3S_1\}, \pi\phi\{^3S_1\}}^{(0)} = 0$                                      | CM Re $\{I_a(s = m^2) = 0\}$                  | 7                 | 1.27                    |
|                                                                                                                                                                                                                  | $\gamma_{\pi\omega\{^3S_1\}, \pi\omega\{^3S_1\}}^{(1)} = 0$                                    | CM Re $\{I_a(s = s_a^{\text{thr}}) = 0\}$     |                   | 1.27                    |
| hence $19 - 9 = 10$ free real-parameters.                                                                                                                                                                        |                                                                                                |                                               |                   |                         |
|                                                                                                                                                                                                                  | $g_{\pi\omega\{^3S_1\}}^{(1)} = 0$                                                             | CM Re $\{I_a(s = m^2) = 0\}$                  | 7                 | 1.24                    |
|                                                                                                                                                                                                                  | $\gamma_{\pi\omega\{^3S_1\}, \pi\phi\{^3S_1\}}^{(0)} = 0$                                      | CM Re $\{I_a(s = s_a^{\text{thr}}) = 0\}$     |                   | 1.24                    |
|                                                                                                                                                                                                                  | $\gamma_{\pi\omega\{^3S_1\}, \pi\omega\{^3D_1\}}^{(0)} = 0$                                    |                                               |                   |                         |
|                                                                                                                                                                                                                  | $g_{\pi\phi\{^3S_1\}}^{(0)} = g_{\pi\omega\{^3S_1\}}^{(1)} = 0$                                | CM Re $\{I_a(s = m^2) = 0\}$                  | 6                 | 1.20                    |
|                                                                                                                                                                                                                  | $\gamma_{\pi\omega\{^3S_1\}, \pi\phi\{^3S_1\}}^{(0)} = 0$                                      | CM Re $\{I_a(s = s_a^{\text{thr}}) = 0\}$     |                   | 1.20                    |
|                                                                                                                                                                                                                  | $\gamma_{\pi\omega\{^3S_1\}, \pi\omega\{^3D_1\}}^{(0)} = 0$                                    |                                               |                   |                         |
|                                                                                                                                                                                                                  | $g_{\pi\omega\{^3D_1\}}^{(0)} = g_{\pi\phi\{^3S_1\}}^{(0)} = g_{\pi\omega\{^3S_1\}}^{(1)} = 0$ | $I_a(s) = -i\rho_a(s)$                        |                   | 1.35                    |
|                                                                                                                                                                                                                  | $\gamma_{\pi\omega\{^3S_1\}, \pi\omega\{^3S_1\}}^{(1)} = 0$                                    | CM Re $\{I_a(s = m^2) = 0\}$                  | 6                 | 1.35                    |
|                                                                                                                                                                                                                  |                                                                                                | CM Re $\{I_a(s = s_a^{\text{thr}}) = 0\}$     |                   | 1.32                    |
|                                                                                                                                                                                                                  | $g_{\pi\omega\{^3D_1\}}^{(0)} = g_{\pi\phi\{^3S_1\}}^{(0)} = 0$                                | $I_a(s) = -i\rho_a(s)$                        | 6                 | 1.35                    |
|                                                                                                                                                                                                                  | $\gamma_{\pi\omega\{^3S_1\}, \pi\phi\{^3S_1\}}^{(0)} = 0$                                      | CM Re $\{I_a(s = m^2) = 0\}$                  |                   | 1.35                    |
|                                                                                                                                                                                                                  | $\gamma_{\pi\omega\{^3S_1\}, \pi\omega\{^3S_1\}}^{(1)} = 0$                                    |                                               |                   |                         |
|                                                                                                                                                                                                                  | $g_{\pi\omega\{^3D_1\}}^{(0)} = g_{\pi\phi\{^3S_1\}}^{(0)} = g_{\pi\omega\{^3S_1\}}^{(1)} = 0$ | $I_a(s) = -i\rho_a(s)$                        |                   | 1.31                    |
|                                                                                                                                                                                                                  | $\gamma_{\pi\omega\{^3S_1\}, \pi\omega\{^3S_1\}}^{(1)} = 0$                                    | CM Re $\{I_a(s = m^2) = 0\}$                  | 5                 | 1.31                    |
|                                                                                                                                                                                                                  | $\gamma_{\pi\omega\{^3S_1\}, \pi\phi\{^3S_1\}}^{(0)} = 0$                                      | CM Re $\{I_a(s = s_a^{\text{thr}}) = 0\}$     |                   | 1.28                    |

Table 0.1: Transcribed from Table XVI in the paper. Parameterizations of coupled  $\pi\omega\{^3S_1\}$ ,  $\pi\omega\{^3D_1\}$  and  $\pi\phi\{^3S_1\}$  scattering amplitudes. Fits used 36 energy levels below  $\pi\pi\pi\pi$  threshold as described in the paper. Displayed in bold is the reference amplitude of Eq. 22. ‘CM’ denotes that the Chew-Mandelstam prescription was employed with subtraction at energy  $m$  or at threshold  $s_a^{\text{thr}}$  where  $s_a^{\text{thr}} = (m_1^{(a)} + m_2^{(a)})^2$ . Otherwise, we set  $I_a(s) = -i\rho_a(s)$ .



| Parameterization                                                                                                                                                                                                                                                                                                                                                                                                       | Further Restrictions                                                                           | Phase-space                                     | $N_{\text{pars}}$ | $\chi^2/N_{\text{dof}}$ |
|------------------------------------------------------------------------------------------------------------------------------------------------------------------------------------------------------------------------------------------------------------------------------------------------------------------------------------------------------------------------------------------------------------------------|------------------------------------------------------------------------------------------------|-------------------------------------------------|-------------------|-------------------------|
| $K_{\ell J_a, \ell' J_b} = \frac{(g_{\ell J_a}^{(0)} + g_{\ell J_a}^{(1)} s)(g_{\ell' J_b}^{(0)} + g_{\ell' J_b}^{(1)} s)}{m^2 - s}$ $+ \gamma_{\ell J_a, \ell' J_b}^{(0)} + \gamma_{\ell J_a, \ell' J_b}^{(1)} s + \gamma_{\ell J_a, \ell' J_b}^{(2)} s^2$                                                                                                                                                            | $g_{\pi\omega\{^3D_1\}}^{(0)} = g_{\pi\phi\{^3S_1\}}^{(0)} = g_{\pi\omega\{^3S_1\}}^{(1)} = 0$ | $I_a(s) = -i\rho_a(s)$                          |                   | 1.11                    |
|                                                                                                                                                                                                                                                                                                                                                                                                                        | $\gamma_{\pi\omega\{^3S_1\}, \pi\omega\{^3S_1\}}^{(2)} = 0$                                    | CM $\text{Re}\{I_a(s = m^2) = 0\}$              | 6                 | 1.11                    |
|                                                                                                                                                                                                                                                                                                                                                                                                                        |                                                                                                | CM $\text{Re}\{I_a(s = s_a^{\text{thr}}) = 0\}$ |                   | 1.11                    |
| where $\gamma_{\pi\omega\{^3S_1\}, \pi\phi\{^3S_1\}}^{(0,1,2)} = 0,$<br>$\gamma_{\pi\omega\{^3D_1\}, \pi\phi\{^3S_1\}}^{(0,1,2)} = 0,$<br>$\gamma_{\pi\omega\{^3D_1\}, \pi\omega\{^3D_1\}}^{(0,1,2)} = 0,$<br>$\gamma_{\pi\omega\{^3S_1\}, \pi\omega\{^3D_1\}}^{(1,2)} = 0,$<br>$\gamma_{\pi\phi\{^3S_1\}, \pi\phi\{^3S_1\}}^{(1,2)} = 0,$<br>$g_{\pi\omega\{^3D_1\}}^{(1)} = 0,$<br>$g_{\pi\phi\{^3S_1\}}^{(1)} = 0,$ | $g_{\pi\omega\{^3D_1\}}^{(0)} = g_{\pi\omega\{^3S_1\}}^{(1)} = 0$                              | $I_a(s) = -i\rho_a(s)$                          |                   | 1.15                    |
|                                                                                                                                                                                                                                                                                                                                                                                                                        | $\gamma_{\pi\omega\{^3S_1\}, \pi\omega\{^3S_1\}}^{(2)} = 0$                                    | CM $\text{Re}\{I_a(s = m^2) = 0\}$              | 7                 | 1.15                    |
|                                                                                                                                                                                                                                                                                                                                                                                                                        |                                                                                                | CM $\text{Re}\{I_a(s = s_a^{\text{thr}}) = 0\}$ |                   | 1.15                    |
|                                                                                                                                                                                                                                                                                                                                                                                                                        | $g_{\pi\phi\{^3S_1\}}^{(0)} = 0$                                                               | $I_a(s) = -i\rho_a(s)$                          |                   | 1.18                    |
|                                                                                                                                                                                                                                                                                                                                                                                                                        | $\gamma_{\pi\omega\{^3S_1\}, \pi\omega\{^3S_1\}}^{(2)} = 0$                                    | CM $\text{Re}\{I_a(s = m^2) = 0\}$              | 8                 | 1.17                    |
|                                                                                                                                                                                                                                                                                                                                                                                                                        |                                                                                                | CM $\text{Re}\{I_a(s = s_a^{\text{thr}}) = 0\}$ |                   | 1.13                    |
| hence $25 - 15 = 10$ free real-parameters.                                                                                                                                                                                                                                                                                                                                                                             | $g_{\pi\omega\{^3S_1\}}^{(1)} = 0$                                                             | $I_a(s) = -i\rho_a(s)$                          |                   | 1.18                    |
|                                                                                                                                                                                                                                                                                                                                                                                                                        | $\gamma_{\pi\omega\{^3S_1\}, \pi\omega\{^3S_1\}}^{(2)} = 0$                                    | CM $\text{Re}\{I_a(s = m^2) = 0\}$              | 8                 | 1.17                    |
|                                                                                                                                                                                                                                                                                                                                                                                                                        |                                                                                                | CM $\text{Re}\{I_a(s = s_a^{\text{thr}}) = 0\}$ |                   | 1.13                    |
|                                                                                                                                                                                                                                                                                                                                                                                                                        | $g_{\pi\omega\{^3D_1\}}^{(0)} = g_{\pi\phi\{^3S_1\}}^{(0)} = g_{\pi\omega\{^3S_1\}}^{(1)} = 0$ | $I_a(s) = -i\rho_a(s)$                          |                   | 1.15                    |
|                                                                                                                                                                                                                                                                                                                                                                                                                        |                                                                                                | CM $\text{Re}\{I_a(s = m^2) = 0\}$              | 7                 | 1.15                    |
|                                                                                                                                                                                                                                                                                                                                                                                                                        |                                                                                                | CM $\text{Re}\{I_a(s = s_a^{\text{thr}}) = 0\}$ |                   | 1.15                    |
|                                                                                                                                                                                                                                                                                                                                                                                                                        | $g_{\pi\omega\{^3D_1\}}^{(0)} = g_{\pi\phi\{^3S_1\}}^{(0)} = 0$                                | CM $\text{Re}\{I_a(s = s_a^{\text{thr}}) = 0\}$ | 6                 | 1.11                    |
|                                                                                                                                                                                                                                                                                                                                                                                                                        | $\gamma_{\pi\omega\{^3S_1\}, \pi\omega\{^3S_1\}}^{(1)} = 0$                                    |                                                 |                   |                         |
|                                                                                                                                                                                                                                                                                                                                                                                                                        | $\gamma_{\pi\omega\{^3S_1\}, \pi\omega\{^3S_1\}}^{(2)} = 0$                                    |                                                 |                   |                         |
|                                                                                                                                                                                                                                                                                                                                                                                                                        | $g_{\pi\phi\{^3S_1\}}^{(0)} = g_{\pi\omega\{^3S_1\}}^{(1)} = 0$                                | $I_a(s) = -i\rho_a(s)$                          | 6                 | 1.20                    |
|                                                                                                                                                                                                                                                                                                                                                                                                                        | $\gamma_{\pi\omega\{^3S_1\}, \pi\omega\{^3D_1\}}^{(0)} = 0$                                    |                                                 |                   |                         |
|                                                                                                                                                                                                                                                                                                                                                                                                                        | $\gamma_{\pi\omega\{^3S_1\}, \pi\omega\{^3S_1\}}^{(2)} = 0$                                    |                                                 |                   |                         |
|                                                                                                                                                                                                                                                                                                                                                                                                                        | $g_{\pi\omega\{^3S_1\}}^{(1)} = 0$                                                             | $I_a(s) = -i\rho_a(s)$                          | 7                 | 1.24                    |
|                                                                                                                                                                                                                                                                                                                                                                                                                        | $\gamma_{\pi\omega\{^3S_1\}, \pi\omega\{^3D_1\}}^{(0)} = 0$                                    |                                                 |                   |                         |
|                                                                                                                                                                                                                                                                                                                                                                                                                        | $\gamma_{\pi\omega\{^3S_1\}, \pi\omega\{^3S_1\}}^{(2)} = 0$                                    |                                                 |                   |                         |

Table 0.2: As Table 0.1 but for amplitudes that resulted in poles on the physical sheet off the real axis and were subsequently rejected as discussed in the paper.



# 1 Successful Parameterizations



## 1.1 coupled\_po\_pp.3s1\_3d1.pole+G0\_3s1\_3S1+G1\_3s1.gorder0\_3s1\_3d1\_3S1.pole0\_sub

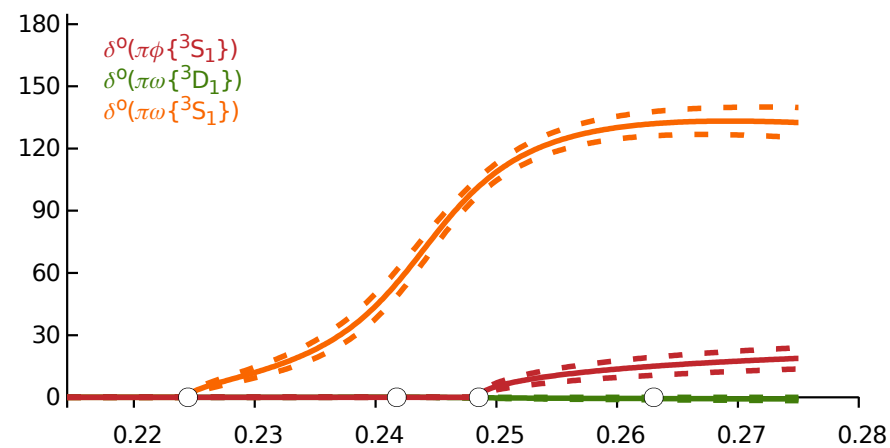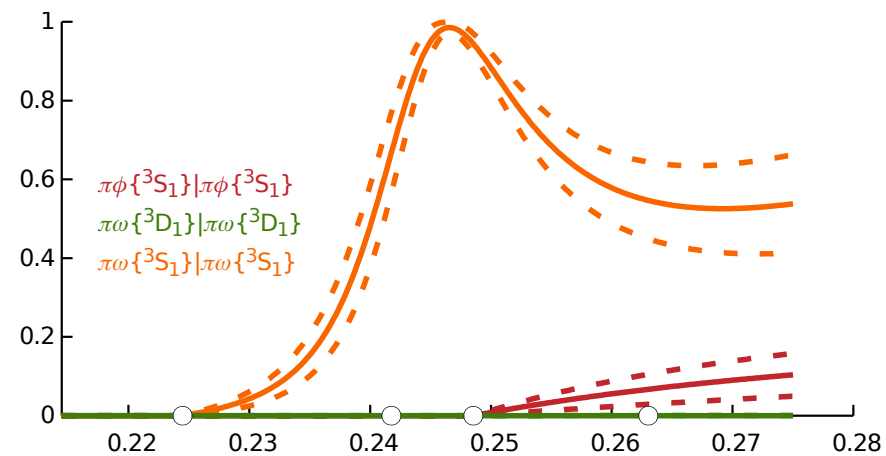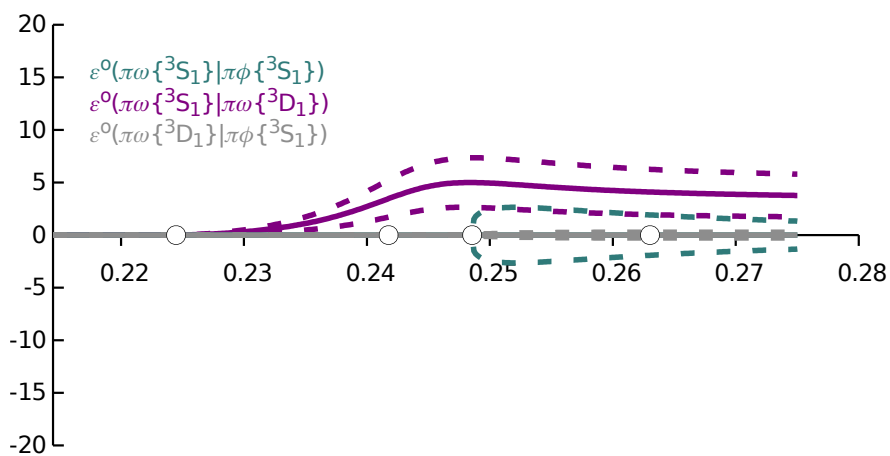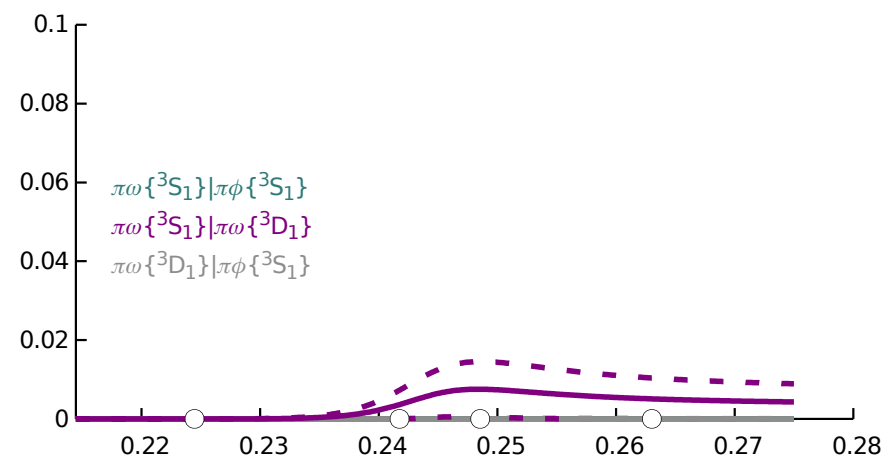



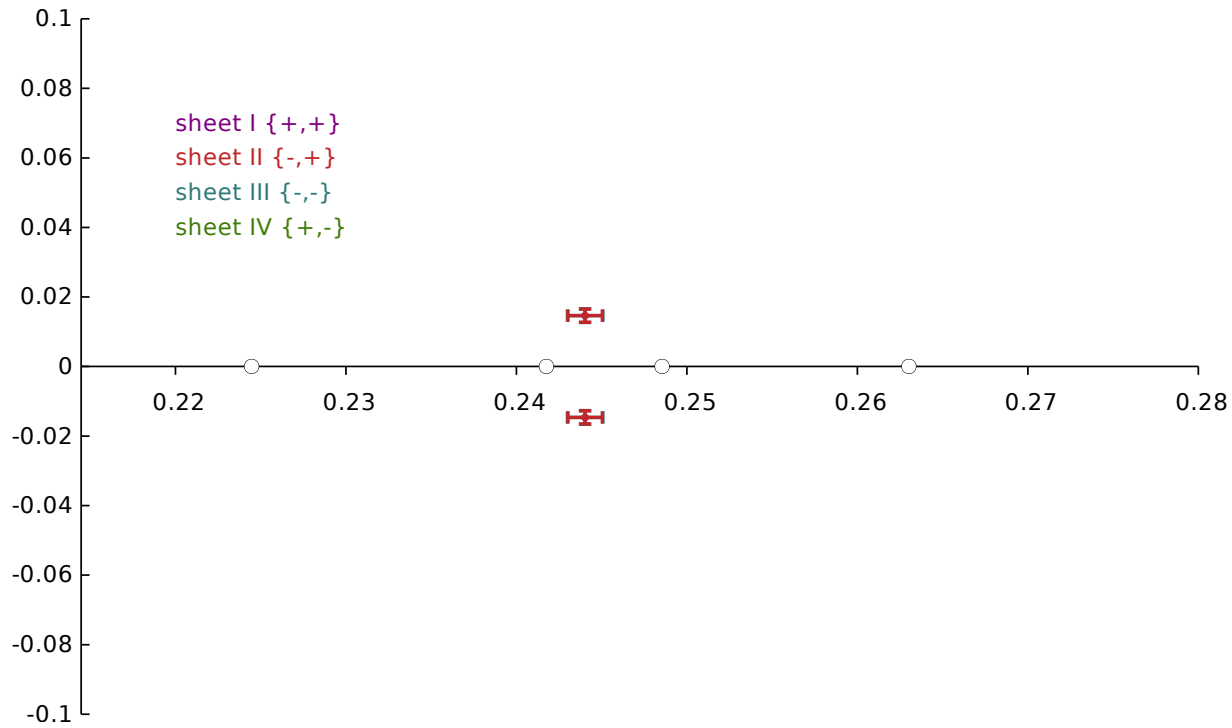

### parameter values

minimised with  $\text{chisq}/\text{nDoF} = 36.05 / (36 - 7) = 1.24$

|                                               |  |                           |  |      |      |       |       |       |       |       |
|-----------------------------------------------|--|---------------------------|--|------|------|-------|-------|-------|-------|-------|
| JP1+_g_pi:omega/3^D_1_pole0                   |  | 0.93996 +/- 0.49168       |  | 1.00 | 0.73 | -0.01 | -0.16 | 0.02  | -0.06 | 0.05  |
| JP1+_g_pi:omega/3^S_1_pole0                   |  | 0.10010 +/- 0.0074569     |  |      | 1.00 | -0.02 | -0.34 | 0.15  | -0.05 | -0.02 |
| JP1+_g_pi:phi/3^S_1_pole0                     |  | -3.0312e-06 +/- 0.0093502 |  |      |      | 1.00  | 0.01  | -0.01 | -0.02 | -0.05 |
| JP1+_gamma_pi:omega/3^S_1 pi:omega/3^S_1_orde |  | 1.2164 +/- 0.54645        |  |      |      |       | 1.00  | -0.94 | 0.01  | 0.00  |
| JP1+_gamma_pi:omega/3^S_1 pi:omega/3^S_1_orde |  | -28.554 +/- 9.9992        |  |      |      |       |       | 1.00  | 0.08  | -0.02 |
| JP1+_gamma_pi:phi/3^S_1 pi:phi/3^S_1_order0   |  | 0.86558 +/- 0.24054       |  |      |      |       |       |       | 1.00  | -0.23 |
| JP1+_m_pole0                                  |  | 0.24658 +/- 0.00066388    |  |      |      |       |       |       |       | 1.00  |

### pole singularities

pi:omega[-] pi:phi[+] upper half-plane

$\text{sqrt}(s)_{\text{pole}} = (0.24403 \pm 0.0010114)$   
 $+ (i/2) * (0.014632 \pm 0.0018828) [-0.45]$

$s_{\text{pole}} = (0.059496 \pm 0.00049994)$   
 $+ i * (0.0035707 \pm 0.00045298) [-0.45]$

|                          |  |                         |  |
|--------------------------|--|-------------------------|--|
| pi:omega                 |  | pi:phi                  |  |
| =====                    |  | =====                   |  |
| k_re= -0.0454 +/- 0.0011 |  | k_re= 0.0138 +/- 0.0012 |  |
| k_im= -0.0088 +/- 0.0012 |  | k_im= 0.0256 +/- 0.0019 |  |



# 1 Successful Parameterizations

```

corr= [-0.45] | corr= [ 0.15] |

===== pi:omega/3^S_1(*) | pi:phi/3^S_1 | pi:omega/3^D_1 |
=====
|g|= 0.0924 +/- 0.0061 | |g|= 0.0003 +/- 0.0053 | |g|= 0.0081 +/- 0.0040 |
arg(g)/pi= 0.0781 +/- 0.0209 | arg(g)/pi= -0.4343 +/- 11.1606 | arg(g)/pi= 0.1446 +/- 0.0215 |
-----
g_re= 0.0896 +/- 0.0062 | g_re= -0.0000 +/- 0.0086 | g_re= 0.0073 +/- 0.0034 |
g_im= 0.0224 +/- 0.0060 | g_im= -0.0000 +/- 0.0012 | g_im= 0.0036 +/- 0.0021 |
corr= [-0.04] | corr= [ 1.00] | corr= [ 0.97] |
-----
Br = 0.8775 +/- 0.0284 | Br = 0.0000 +/- 0.0000 | Br = 0.0068 +/- 0.0062 |

--
pi:omega[-] pi:phi[+] lower half-plane

sqrt(s)_pole = (0.24403 +/- 0.0010114)
+ (i/2)*(-0.014632 +/- 0.0018828) [ 0.45]

s_pole = (0.059496 +/- 0.00049994)
+ i*(-0.0035707 +/- 0.00045298) [ 0.45]

===== pi:omega | pi:phi |
=====
k_re= 0.0454 +/- 0.0011 | k_re= -0.0138 +/- 0.0012 |
k_im= -0.0088 +/- 0.0012 | k_im= 0.0256 +/- 0.0019 |
corr= [ 0.45] | corr= [-0.15] |

===== pi:omega/3^S_1(*) | pi:phi/3^S_1 | pi:omega/3^D_1 |
=====
|g|= 0.0924 +/- 0.0061 | |g|= 0.0003 +/- 0.0053 | |g|= 0.0081 +/- 0.0040 |
arg(g)/pi= -0.0781 +/- 0.0209 | arg(g)/pi= 0.4343 +/- 11.1606 | arg(g)/pi= -0.1446 +/- 0.0215 |
-----
g_re= 0.0896 +/- 0.0062 | g_re= -0.0000 +/- 0.0086 | g_re= 0.0073 +/- 0.0034 |
g_im= -0.0224 +/- 0.0060 | g_im= 0.0000 +/- 0.0012 | g_im= -0.0036 +/- 0.0021 |
corr= [ 0.04] | corr= [-1.00] | corr= [-0.97] |
-----
Br = 0.8775 +/- 0.0284 | Br = 0.0000 +/- 0.0000 | Br = 0.0068 +/- 0.0062 |

--
pi:omega[-] pi:phi[-] upper half-plane

sqrt(s)_pole = (0.24403 +/- 0.0010398)
+ (i/2)*(+0.014632 +/- 0.001965) [-0.46]

s_pole = (0.059495 +/- 0.00051426)
+ i*(+0.0035706 +/- 0.00047269) [-0.46]

===== pi:omega | pi:phi |
=====
k_re= -0.0454 +/- 0.0011 | k_re= -0.0138 +/- 0.0013 |
k_im= -0.0088 +/- 0.0012 | k_im= -0.0256 +/- 0.0020 |
corr= [-0.46] | corr= [ 0.17] |

===== pi:omega/3^S_1(*) | pi:phi/3^S_1 | pi:omega/3^D_1 |
=====
|g|= 0.0924 +/- 0.0064 | |g|= 0.0005 +/- 0.0078 | |g|= 0.0081 +/- 0.0041 |
arg(g)/pi= 0.0781 +/- 0.0212 | arg(g)/pi= 0.4562 +/- 11.1675 | arg(g)/pi= 0.1446 +/- 0.0224 |
-----
g_re= 0.0896 +/- 0.0065 | g_re= -0.0000 +/- 0.0130 | g_re= 0.0073 +/- 0.0035 |
g_im= 0.0224 +/- 0.0061 | g_im= 0.0000 +/- 0.0014 | g_im= 0.0036 +/- 0.0022 |
corr= [-0.03] | corr= [-1.00] | corr= [ 0.97] |

```



# 1 Successful Parameterizations

```

-----|-----|-----|
      Br =  0.8775 +/- 0.0286 |      Br =  0.0000 +/- 0.0000 |      Br =  0.0068 +/- 0.0063 |

--
pi:omega[-] pi:phi[-]  lower half-plane

sqrt(s)_pole = (0.24403 +/- 0.0010398)
               + (i/2)*(-0.014632 +/- 0.001965) [ 0.46]

s_pole = (0.059495 +/- 0.00051426)
         + i*(-0.0035706 +/- 0.00047269) [ 0.46]

=====|=====|
      pi:omega |      pi:phi |
=====|=====|
      k_re=  0.0454 +/- 0.0011 |      k_re=  0.0138 +/- 0.0013 |
      k_im= -0.0088 +/- 0.0012 |      k_im= -0.0256 +/- 0.0020 |
      corr= [ 0.46]           |      corr= [-0.17]           |

=====|=====|=====|
      pi:omega/3^S_1(*) |      pi:phi/3^S_1 |      pi:omega/3^D_1 |
=====|=====|=====|
      |g|=  0.0924 +/- 0.0064 |      |g|=  0.0005 +/- 0.0078 |      |g|=  0.0081 +/- 0.0041 |
arg(g)/pi= -0.0781 +/- 0.0212 | arg(g)/pi= -0.4560 +/- 11.1715 | arg(g)/pi= -0.1446 +/- 0.0224 |
-----|-----|-----|
      g_re=  0.0896 +/- 0.0065 |      g_re= -0.0000 +/- 0.0130 |      g_re=  0.0073 +/- 0.0035 |
      g_im= -0.0224 +/- 0.0061 |      g_im= -0.0000 +/- 0.0014 |      g_im= -0.0036 +/- 0.0022 |
      corr= [ 0.03]           |      corr= [ 1.00]           |      corr= [-0.97]           |
-----|-----|-----|
      Br =  0.8775 +/- 0.0286 |      Br =  0.0000 +/- 0.0000 |      Br =  0.0068 +/- 0.0063 |

```



## 1.2 coupled\_po\_pp.3s1\_3d1.pole+G0\_3s1\_3S1+G1\_3s1.gorder0\_3s1\_3d1\_3S1.threshold\_sub

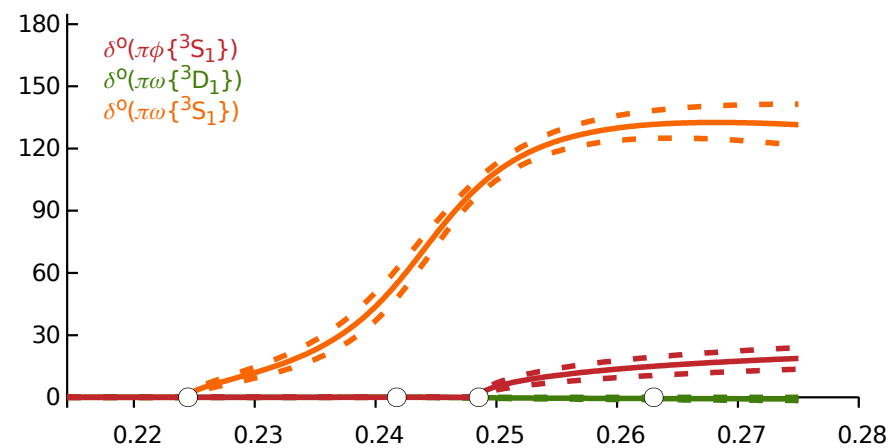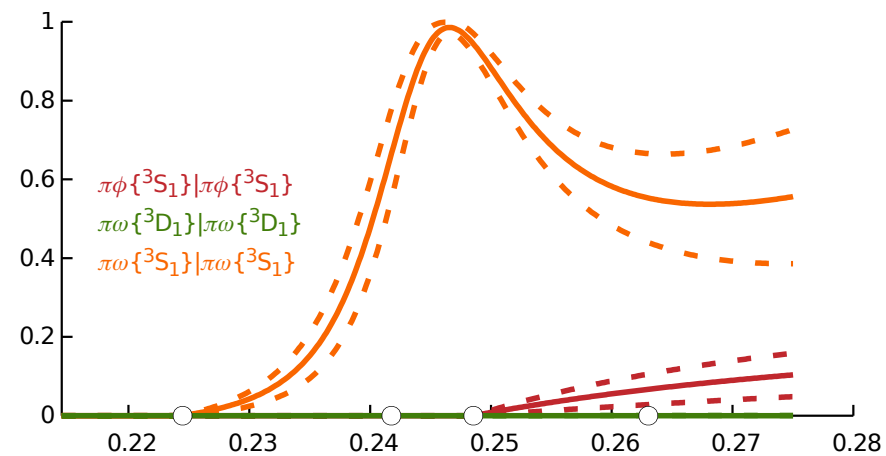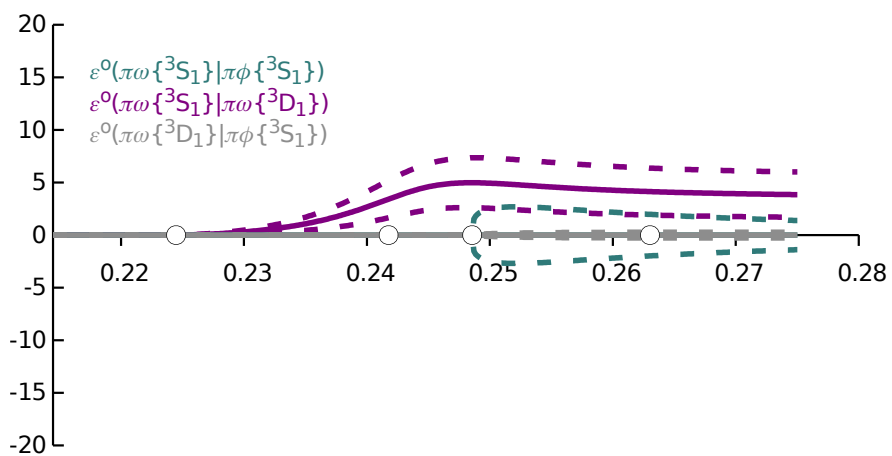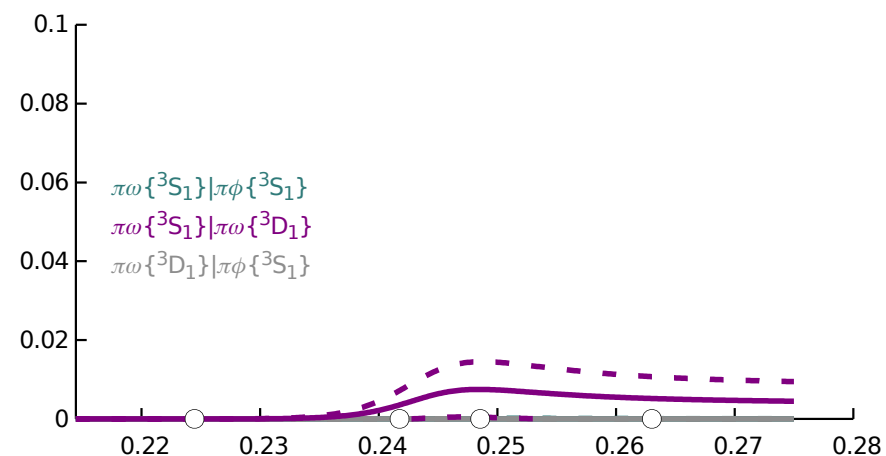



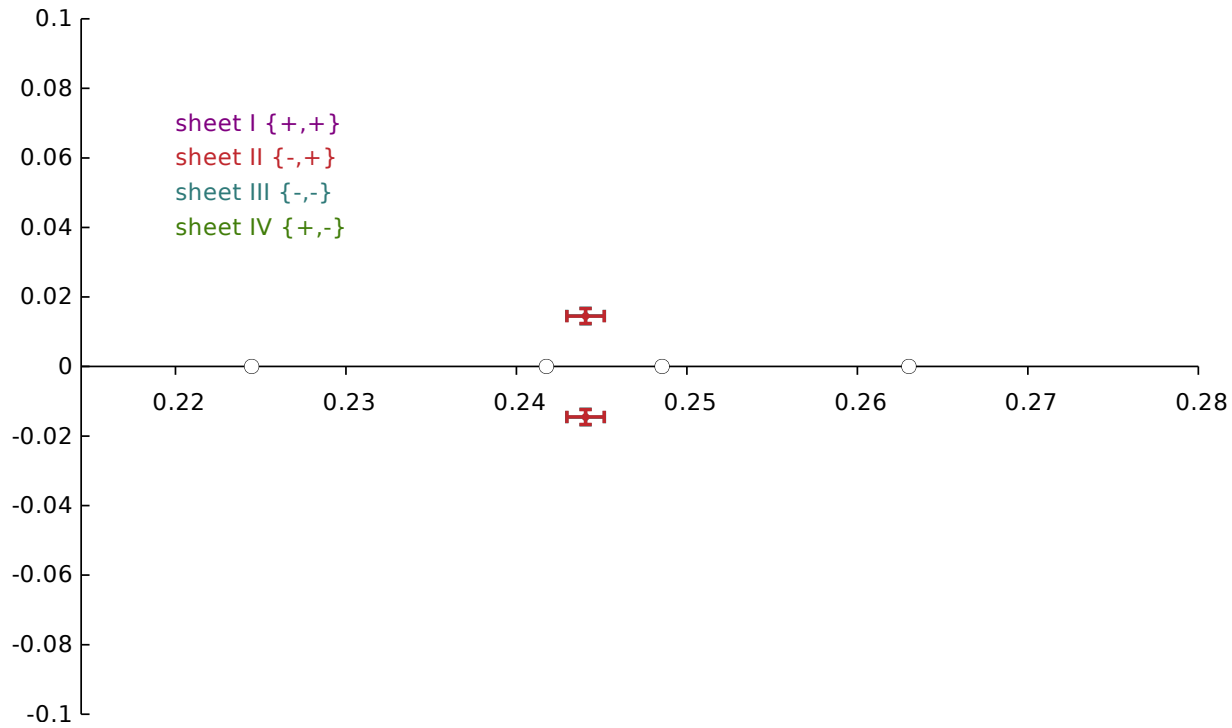

### parameter values

minimised with  $\text{chisq}/\text{nDoF} = 36.02 / (36 - 7) = 1.24$

|                                               |  |                          |  |      |      |       |       |       |       |       |
|-----------------------------------------------|--|--------------------------|--|------|------|-------|-------|-------|-------|-------|
| JP1+_g_pi:omega/3^D_1_pole0                   |  | 0.93053 +/- 0.49566      |  | 1.00 | 0.67 | -0.00 | -0.20 | 0.12  | -0.02 | -0.36 |
| JP1+_g_pi:omega/3^S_1_pole0                   |  | 0.095180 +/- 0.007314    |  |      | 1.00 | -0.01 | -0.55 | 0.51  | 0.08  | -0.58 |
| JP1+_g_pi:phi/3^S_1_pole0                     |  | -1.7589e-05 +/- 0.010383 |  |      |      | 1.00  | 0.00  | -0.00 | 0.00  | -0.02 |
| JP1+_gamma_pi:omega/3^S_1 pi:omega/3^S_1_orde |  | 1.2269 +/- 0.90034       |  |      |      |       | 1.00  | -0.98 | -0.05 | 0.28  |
| JP1+_gamma_pi:omega/3^S_1 pi:omega/3^S_1_orde |  | -27.519 +/- 15.828       |  |      |      |       |       | 1.00  | 0.09  | -0.25 |
| JP1+_gamma_pi:phi/3^S_1 pi:phi/3^S_1_order0   |  | 0.95117 +/- 0.29844      |  |      |      |       |       |       | 1.00  | -0.28 |
| JP1+_m_pole0                                  |  | 0.24464 +/- 0.00074184   |  |      |      |       |       |       |       | 1.00  |

### pole singularities

pi:omega[-] pi:phi[+] upper half-plane

$\text{sqrt}(s)_{\text{pole}} = (0.24406 \pm 0.0010928)$   
 $+ (i/2) * (+0.014521 \pm 0.0021623) [-0.50]$

$s_{\text{pole}} = (0.059513 \pm 0.00054139)$   
 $+ i * (+0.0035441 \pm 0.00052002) [-0.49]$

|                          |                         |
|--------------------------|-------------------------|
| pi:omega                 | pi:phi                  |
| ===== =====              | ===== =====             |
| k_re= -0.0455 +/- 0.0012 | k_re= 0.0137 +/- 0.0013 |
| k_im= -0.0087 +/- 0.0014 | k_im= 0.0255 +/- 0.0022 |



# 1 Successful Parameterizations

```

corr= [-0.48] | corr= [ 0.24] |

===== pi:omega/3^S_1(*) | pi:phi/3^S_1 | pi:omega/3^D_1 |
=====
|g|= 0.0919 +/- 0.0079 | |g|= 0.0003 +/- 0.0053 | |g|= 0.0080 +/- 0.0040 |
arg(g)/pi= 0.0776 +/- 0.0215 | arg(g)/pi= -0.4356 +/- 11.1637 | arg(g)/pi= 0.1463 +/- 0.0250 |
-----
g_re= 0.0892 +/- 0.0079 | g_re= -0.0000 +/- 0.0085 | g_re= 0.0072 +/- 0.0034 |
g_im= 0.0222 +/- 0.0061 | g_im= -0.0000 +/- 0.0013 | g_im= 0.0036 +/- 0.0022 |
corr= [ 0.02] | corr= [ 1.00] | corr= [ 0.96] |
-----
Br = 0.8755 +/- 0.0409 | Br = 0.0000 +/- 0.0000 | Br = 0.0067 +/- 0.0061 |

--
pi:omega[-] pi:phi[+] lower half-plane

sqrt(s)_pole = (0.24406 +/- 0.0010928)
+ (i/2)*(-0.014521 +/- 0.0021623) [ 0.50]

s_pole = (0.059513 +/- 0.00054139)
+ i*(-0.0035441 +/- 0.00052002) [ 0.49]

===== pi:omega | pi:phi |
=====
k_re= 0.0455 +/- 0.0012 | k_re= -0.0137 +/- 0.0013 |
k_im= -0.0087 +/- 0.0014 | k_im= 0.0255 +/- 0.0022 |
corr= [ 0.48] | corr= [-0.24] |

===== pi:omega/3^S_1(*) | pi:phi/3^S_1 | pi:omega/3^D_1 |
=====
|g|= 0.0919 +/- 0.0079 | |g|= 0.0003 +/- 0.0053 | |g|= 0.0080 +/- 0.0040 |
arg(g)/pi= -0.0776 +/- 0.0215 | arg(g)/pi= 0.4356 +/- 11.1637 | arg(g)/pi= -0.1463 +/- 0.0250 |
-----
g_re= 0.0892 +/- 0.0079 | g_re= -0.0000 +/- 0.0085 | g_re= 0.0072 +/- 0.0034 |
g_im= -0.0222 +/- 0.0061 | g_im= 0.0000 +/- 0.0013 | g_im= -0.0036 +/- 0.0022 |
corr= [-0.02] | corr= [-1.00] | corr= [-0.96] |
-----
Br = 0.8755 +/- 0.0409 | Br = 0.0000 +/- 0.0000 | Br = 0.0067 +/- 0.0061 |

--
pi:omega[-] pi:phi[-] upper half-plane

sqrt(s)_pole = (0.24406 +/- 0.0011037)
+ (i/2)*(+0.014522 +/- 0.0022478) [-0.49]

s_pole = (0.059511 +/- 0.00054696)
+ i*(+0.0035442 +/- 0.00054088) [-0.49]

===== pi:omega | pi:phi |
=====
k_re= -0.0454 +/- 0.0012 | k_re= -0.0137 +/- 0.0014 |
k_im= -0.0087 +/- 0.0014 | k_im= -0.0255 +/- 0.0022 |
corr= [-0.47] | corr= [ 0.26] |

===== pi:omega/3^S_1(*) | pi:phi/3^S_1 | pi:omega/3^D_1 |
=====
|g|= 0.0919 +/- 0.0082 | |g|= 0.0005 +/- 0.0079 | |g|= 0.0080 +/- 0.0041 |
arg(g)/pi= 0.0777 +/- 0.0221 | arg(g)/pi= 0.4673 +/- 11.1697 | arg(g)/pi= 0.1463 +/- 0.0259 |
-----
g_re= 0.0892 +/- 0.0083 | g_re= -0.0000 +/- 0.0130 | g_re= 0.0072 +/- 0.0035 |
g_im= 0.0222 +/- 0.0063 | g_im= 0.0000 +/- 0.0013 | g_im= 0.0036 +/- 0.0022 |
corr= [ 0.02] | corr= [-1.00] | corr= [ 0.97] |

```



## 1 Successful Parameterizations

```

-----|-----|-----|
      Br =  0.8754 +/- 0.0415 |      Br =  0.0000 +/- 0.0000 |      Br =  0.0067 +/- 0.0062 |

--
pi:omega[-] pi:phi[-] lower half-plane

sqrt(s)_pole = (0.24406 +/- 0.0011037)
               + (i/2)*(-0.014522 +/- 0.0022478) [ 0.49]

s_pole = (0.059511 +/- 0.00054696)
         + i*(-0.0035442 +/- 0.00054088) [ 0.49]

=====|=====|
      pi:omega |      pi:phi |
=====|=====|
      k_re=  0.0454 +/- 0.0012 |      k_re=  0.0137 +/- 0.0014 |
      k_im= -0.0087 +/- 0.0014 |      k_im= -0.0255 +/- 0.0022 |
      corr= [ 0.47]           |      corr= [-0.26]           |

=====|=====|=====|
      pi:omega/3^S_1(*) |      pi:phi/3^S_1 |      pi:omega/3^D_1 |
=====|=====|=====|
      |g|=  0.0919 +/- 0.0082 |      |g|=  0.0005 +/- 0.0079 |      |g|=  0.0080 +/- 0.0041 |
arg(g)/pi= -0.0777 +/- 0.0221 | arg(g)/pi= -0.4673 +/- 11.1697 | arg(g)/pi= -0.1463 +/- 0.0259 |
-----|-----|-----|
      g_re=  0.0892 +/- 0.0083 |      g_re= -0.0000 +/- 0.0130 |      g_re=  0.0072 +/- 0.0035 |
      g_im= -0.0222 +/- 0.0063 |      g_im= -0.0000 +/- 0.0013 |      g_im= -0.0036 +/- 0.0022 |
      corr= [-0.02]           |      corr= [ 1.00]           |      corr= [-0.97]           |
-----|-----|-----|
      Br =  0.8754 +/- 0.0415 |      Br =  0.0000 +/- 0.0000 |      Br =  0.0067 +/- 0.0062 |

```



## 1.3 coupled\_po\_pp.3s1\_3d1.pole+G0\_3s1\_3S1+G1\_3s1.gorder0\_3s1\_3d1.pole0\_sub

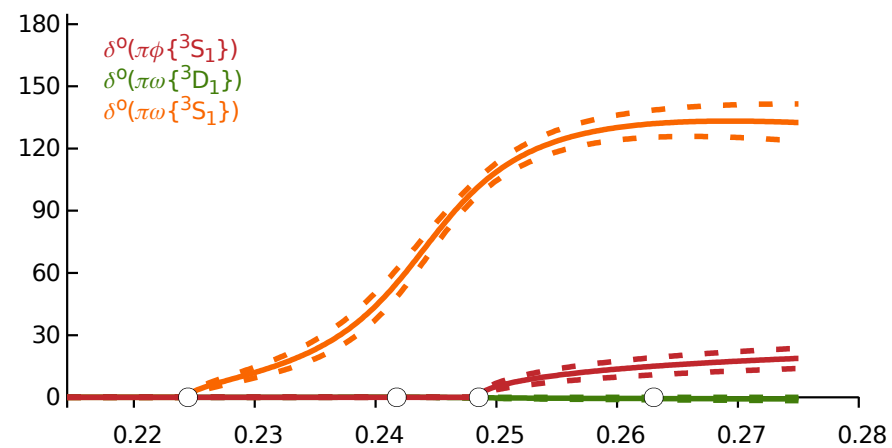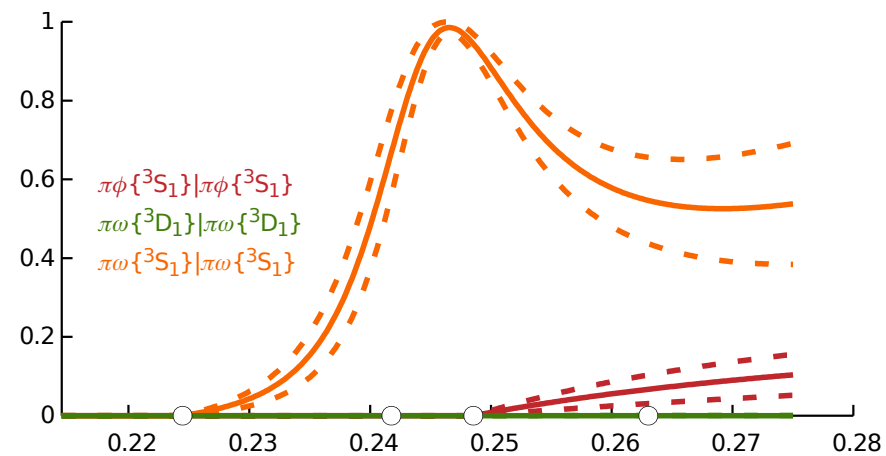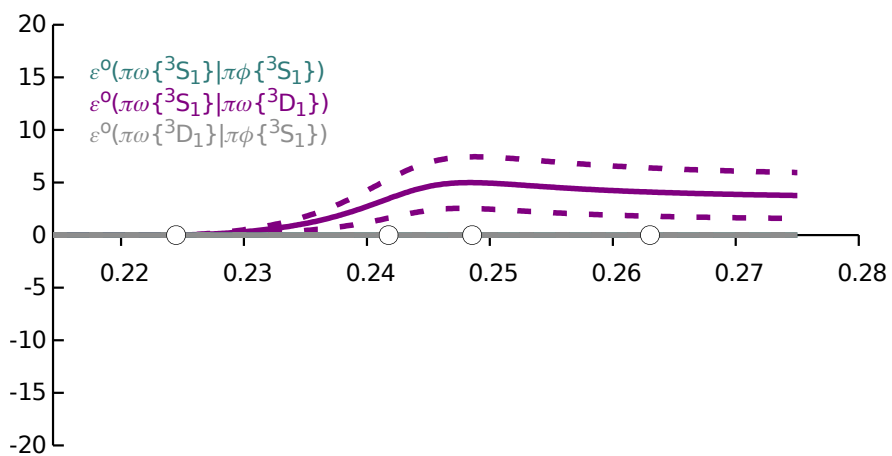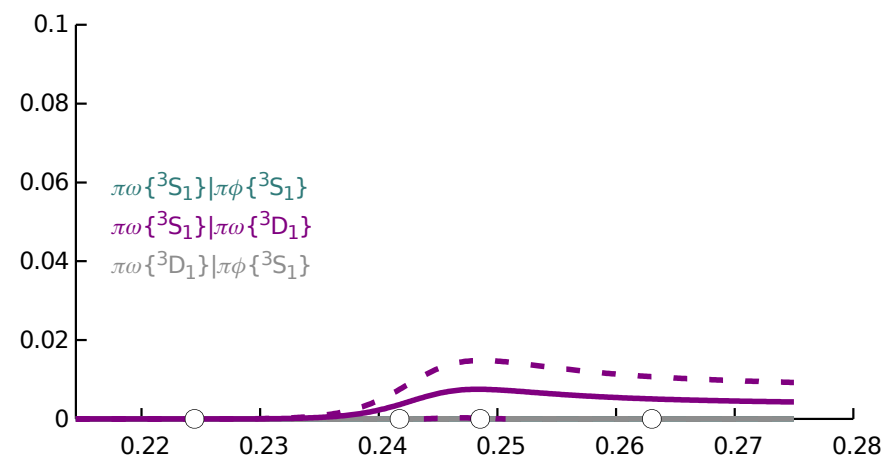



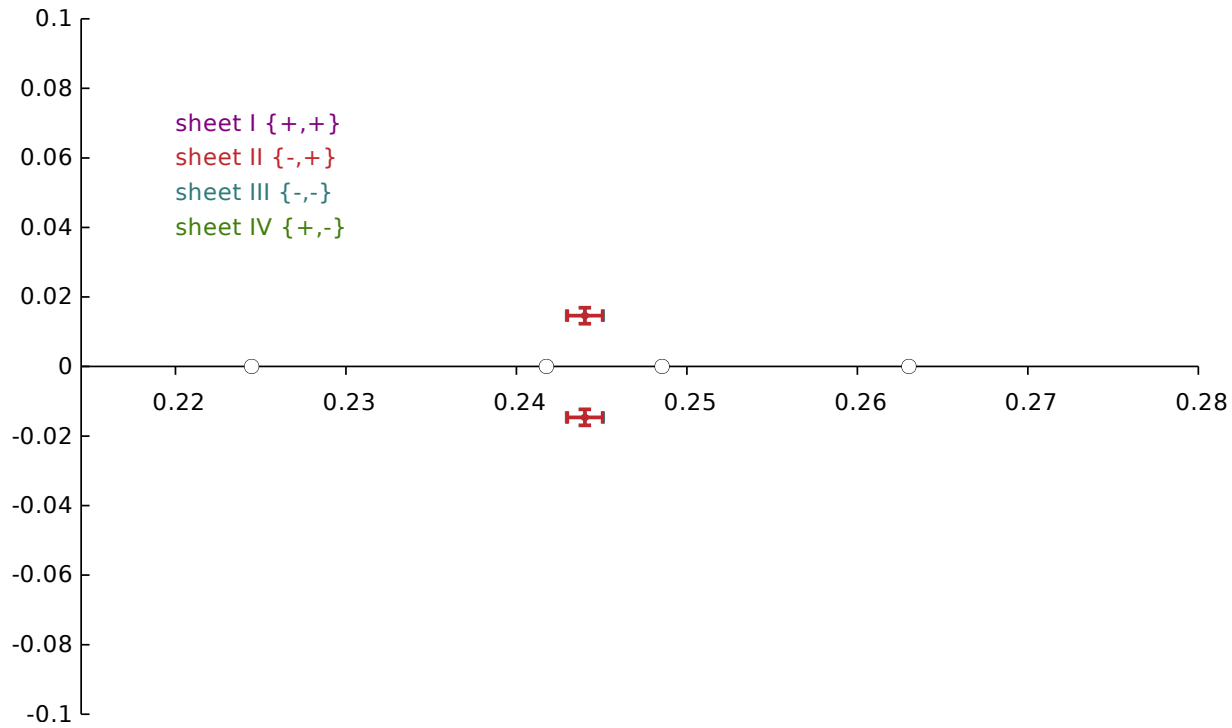

### parameter values

minimised with  $\text{chisq}/\text{nDoF} = 36.05 / (36 - 6) = 1.20$

|                                               |  |                        |  |      |      |       |       |       |       |
|-----------------------------------------------|--|------------------------|--|------|------|-------|-------|-------|-------|
| JP1+_g_pi:omega/3^D_1_pole0                   |  | 0.93910 +/- 0.49929    |  | 1.00 | 0.74 | -0.19 | 0.08  | -0.06 | 0.04  |
| JP1+_g_pi:omega/3^S_1_pole0                   |  | 0.10010 +/- 0.0078404  |  |      | 1.00 | -0.42 | 0.29  | -0.05 | -0.03 |
| JP1+_gamma_pi:omega/3^S_1 pi:omega/3^S_1_orde |  | 1.2152 +/- 0.79759     |  |      |      | 1.00  | -0.97 | -0.02 | 0.01  |
| JP1+_gamma_pi:omega/3^S_1 pi:omega/3^S_1_orde |  | -28.539 +/- 14.557     |  |      |      |       | 1.00  | 0.08  | -0.02 |
| JP1+_gamma_pi:phi/3^S_1 pi:phi/3^S_1_order0   |  | 0.86503 +/- 0.24108    |  |      |      |       |       | 1.00  | -0.24 |
| JP1+_m_pole0                                  |  | 0.24658 +/- 0.00066445 |  |      |      |       |       |       | 1.00  |

### pole singularities

pi:omega[-] pi:phi[+] upper half-plane

\*\*\* not found on > 5% cfs \*\*\*

sqrt(s)\_pole = (0.24402 +/- 0.0010312)  
+ (i/2)\*(+0.01462 +/- 0.0022835) [-0.51]

s\_pole = (0.059493 +/- 0.00051191)  
+ i\*(+0.0035677 +/- 0.00054974) [-0.51]

|                          |                         |
|--------------------------|-------------------------|
| pi:omega                 | pi:phi                  |
| ===== =====              |                         |
| k_re= -0.0454 +/- 0.0011 | k_re= 0.0137 +/- 0.0014 |
| k_im= -0.0088 +/- 0.0014 | k_im= 0.0256 +/- 0.0021 |
| corr= [-0.47]            | corr= [ 0.34]           |



| pi:omega/3^S_1(*)                                                   | pi:phi/3^S_1                                                        | pi:omega/3^D_1                                                      |
|---------------------------------------------------------------------|---------------------------------------------------------------------|---------------------------------------------------------------------|
| g = 0.0923 +/- 0.0080<br>arg(g)/pi= 0.0782 +/- 0.0225               | g = 0.0000 +/- 0.0000<br>arg(g)/pi= 0.4218 +/- 0.0225               | g = 0.0081 +/- 0.0042<br>arg(g)/pi= 0.1445 +/- 0.0263               |
| g_re= 0.0896 +/- 0.0081<br>g_im= 0.0225 +/- 0.0064<br>corr= [-0.01] | g_re= 0.0000 +/- 0.0000<br>g_im= 0.0000 +/- 0.0000<br>corr= [ 0.20] | g_re= 0.0073 +/- 0.0036<br>g_im= 0.0036 +/- 0.0023<br>corr= [ 0.97] |
| Br = 0.8767 +/- 0.0365                                              | Br = 0.0000 +/- 0.0000                                              | Br = 0.0067 +/- 0.0063                                              |

```
--
pi:omega[-] pi:phi[+] lower half-plane
*** not found on > 5% cfigs ***
sqrt(s)_pole = (0.24402 +/- 0.0010312)
+ (i/2)*(-0.01462 +/- 0.0022835) [ 0.51]

s_pole = (0.059493 +/- 0.00051191)
+ i*(-0.0035677 +/- 0.00054974) [ 0.51]
```

| pi:omega                                                             | pi:phi                                                               |
|----------------------------------------------------------------------|----------------------------------------------------------------------|
| k_re= 0.0454 +/- 0.0011<br>k_im= -0.0088 +/- 0.0014<br>corr= [ 0.47] | k_re= -0.0137 +/- 0.0014<br>k_im= 0.0256 +/- 0.0021<br>corr= [-0.34] |

| pi:omega/3^S_1(*)                                                    | pi:phi/3^S_1                                                         | pi:omega/3^D_1                                                       |
|----------------------------------------------------------------------|----------------------------------------------------------------------|----------------------------------------------------------------------|
| g = 0.0923 +/- 0.0080<br>arg(g)/pi= -0.0782 +/- 0.0225               | g = 0.0000 +/- 0.0000<br>arg(g)/pi= 0.5782 +/- 0.0225                | g = 0.0081 +/- 0.0042<br>arg(g)/pi= -0.1445 +/- 0.0263               |
| g_re= 0.0896 +/- 0.0081<br>g_im= -0.0225 +/- 0.0064<br>corr= [ 0.01] | g_re= -0.0000 +/- 0.0000<br>g_im= 0.0000 +/- 0.0000<br>corr= [-0.20] | g_re= 0.0073 +/- 0.0036<br>g_im= -0.0036 +/- 0.0023<br>corr= [-0.97] |
| Br = 0.8767 +/- 0.0365                                               | Br = 0.0000 +/- 0.0000                                               | Br = 0.0067 +/- 0.0063                                               |

```
--
pi:omega[-] pi:phi[-] upper half-plane

sqrt(s)_pole = (0.24402 +/- 0.0010745)
+ (i/2)*(+0.014628 +/- 0.00231) [-0.52]

s_pole = (0.059492 +/- 0.00053335)
+ i*(+0.0035696 +/- 0.00055571) [-0.52]
```

| pi:omega                                                              | pi:phi                                                                |
|-----------------------------------------------------------------------|-----------------------------------------------------------------------|
| k_re= -0.0454 +/- 0.0012<br>k_im= -0.0088 +/- 0.0015<br>corr= [-0.48] | k_re= -0.0137 +/- 0.0014<br>k_im= -0.0256 +/- 0.0022<br>corr= [ 0.33] |

| pi:omega/3^S_1(*)                                                   | pi:phi/3^S_1                                                        | pi:omega/3^D_1                                                      |
|---------------------------------------------------------------------|---------------------------------------------------------------------|---------------------------------------------------------------------|
| g = 0.0924 +/- 0.0081<br>arg(g)/pi= 0.0782 +/- 0.0222               | g = 0.0000 +/- 0.0000<br>arg(g)/pi= 0.4218 +/- 0.0222               | g = 0.0081 +/- 0.0043<br>arg(g)/pi= 0.1446 +/- 0.0268               |
| g_re= 0.0896 +/- 0.0081<br>g_im= 0.0225 +/- 0.0065<br>corr= [ 0.06] | g_re= 0.0000 +/- 0.0000<br>g_im= 0.0000 +/- 0.0000<br>corr= [ 0.15] | g_re= 0.0073 +/- 0.0037<br>g_im= 0.0036 +/- 0.0023<br>corr= [ 0.97] |



# 1 Successful Parameterizations

```

Br = 0.8768 +/- 0.0372 | Br = 0.0000 +/- 0.0000 | Br = 0.0067 +/- 0.0065 |

--
pi:omega[-] pi:phi[-] lower half-plane

sqrt(s)_pole = (0.24402 +/- 0.0010745)
               + (i/2)*(-0.014628 +/- 0.00231) [ 0.52]

s_pole = (0.059492 +/- 0.00053335)
          + i*(-0.0035696 +/- 0.00055571) [ 0.52]

=====
pi:omega | pi:phi |
=====
k_re= 0.0454 +/- 0.0012 | k_re= 0.0137 +/- 0.0014 |
k_im= -0.0088 +/- 0.0015 | k_im= -0.0256 +/- 0.0022 |
corr= [ 0.48] | corr= [-0.33] |

=====
pi:omega/3^S_1(*) | pi:phi/3^S_1 | pi:omega/3^D_1 |
=====
|g|= 0.0924 +/- 0.0081 | |g|= 0.0000 +/- 0.0000 | |g|= 0.0081 +/- 0.0043 |
arg(g)/pi= -0.0782 +/- 0.0222 | arg(g)/pi= 0.5782 +/- 0.0222 | arg(g)/pi= -0.1446 +/- 0.0268 |
-----
g_re= 0.0896 +/- 0.0081 | g_re= -0.0000 +/- 0.0000 | g_re= 0.0073 +/- 0.0037 |
g_im= -0.0225 +/- 0.0065 | g_im= 0.0000 +/- 0.0000 | g_im= -0.0036 +/- 0.0023 |
corr= [-0.06] | corr= [-0.15] | corr= [-0.97] |
-----
Br = 0.8768 +/- 0.0372 | Br = 0.0000 +/- 0.0000 | Br = 0.0067 +/- 0.0065 |

```



## 1.4 coupled\_po\_pp.3s1\_3d1.pole+G0\_3s1\_3S1+G1\_3s1.gorder0\_3s1\_3d1.threshold\_sub

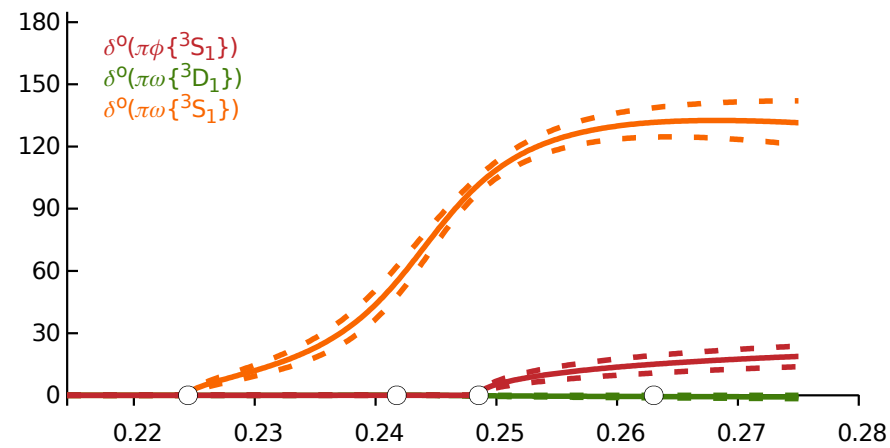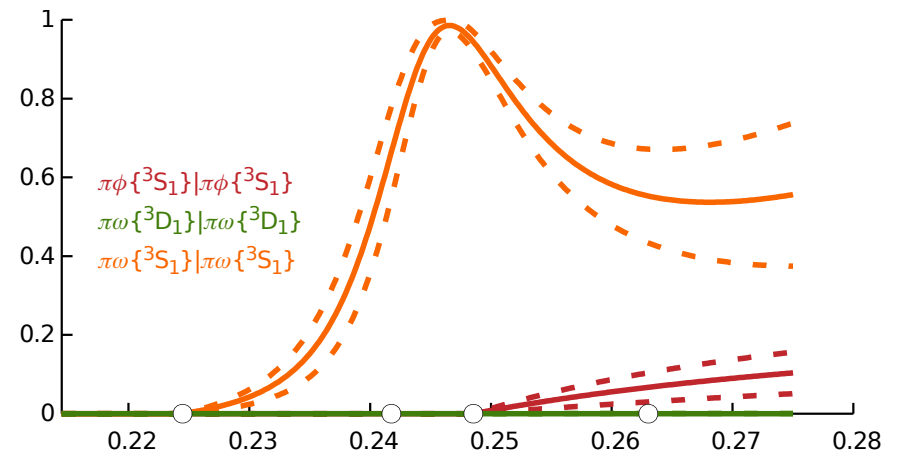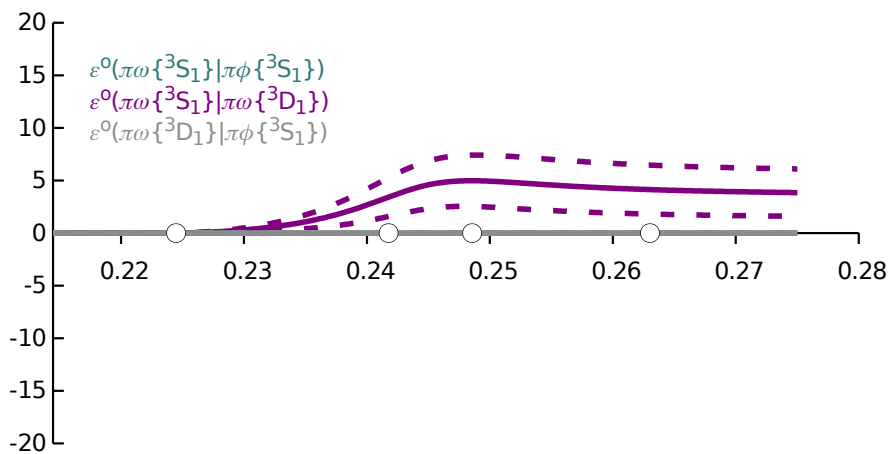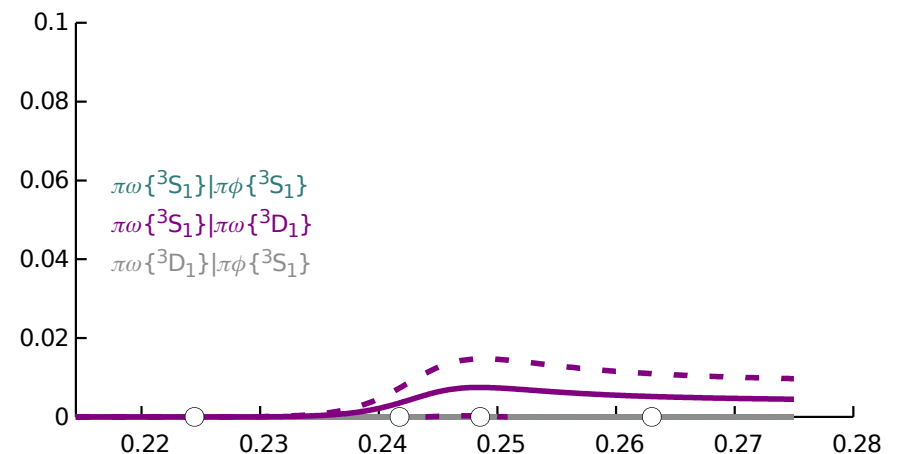



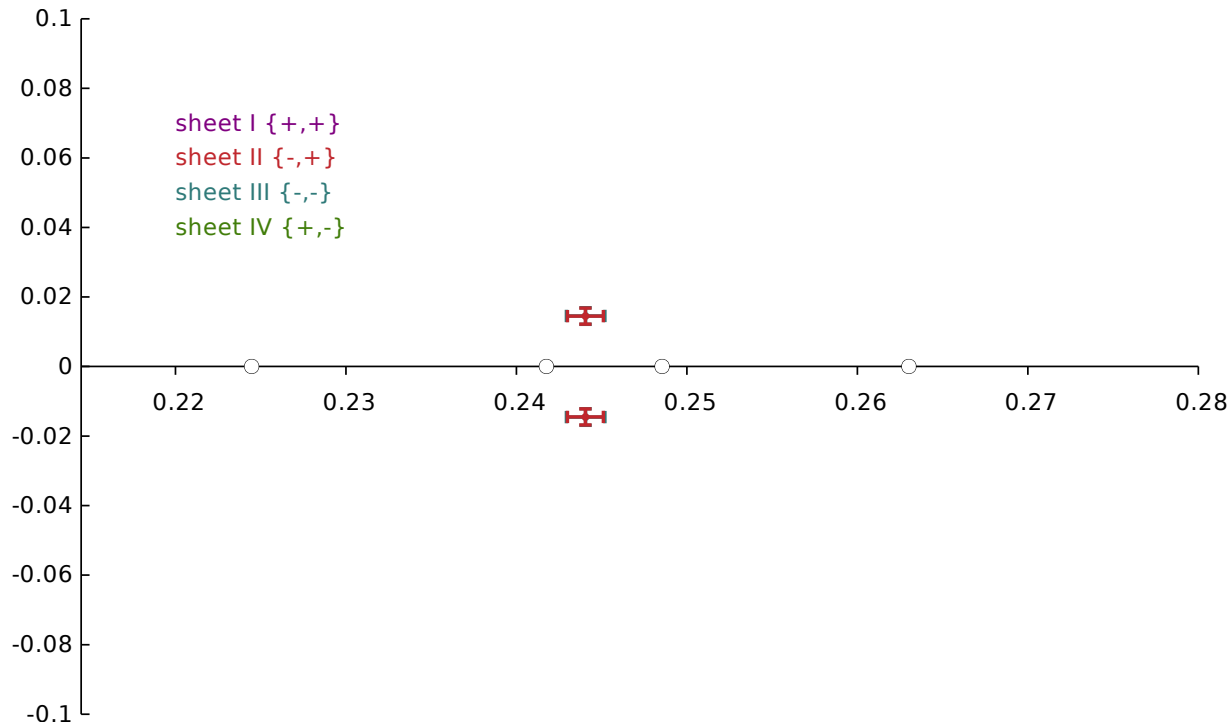

### parameter values

minimised with  $\text{chisq}/\text{nDoF} = 36.02 / (36 - 6) = 1.20$

|                                               |  |                        |  |      |      |       |       |       |       |
|-----------------------------------------------|--|------------------------|--|------|------|-------|-------|-------|-------|
| JP1+_g_pi:omega/3^D_1_pole0                   |  | 0.93062 +/- 0.49566    |  | 1.00 | 0.67 | -0.20 | 0.12  | -0.02 | -0.36 |
| JP1+_g_pi:omega/3^S_1_pole0                   |  | 0.095182 +/- 0.0073138 |  |      | 1.00 | -0.55 | 0.51  | 0.08  | -0.58 |
| JP1+_gamma_pi:omega/3^S_1 pi:omega/3^S_1_orde |  | 1.2267 +/- 0.90033     |  |      |      | 1.00  | -0.98 | -0.05 | 0.28  |
| JP1+_gamma_pi:omega/3^S_1 pi:omega/3^S_1_orde |  | -27.515 +/- 15.828     |  |      |      |       | 1.00  | 0.09  | -0.25 |
| JP1+_gamma_pi:phi/3^S_1 pi:phi/3^S_1_order0   |  | 0.95120 +/- 0.29845    |  |      |      |       |       | 1.00  | -0.28 |
| JP1+_m_pole0                                  |  | 0.24464 +/- 0.00074165 |  |      |      |       |       |       | 1.00  |

### pole singularities

pi:omega[-] pi:phi[+] upper half-plane  
 \*\*\* not found on > 5% cfs \*\*\*  
 sqrt(s)\_pole = (0.24405 +/- 0.001056)  
 + (i/2)\*(+0.014516 +/- 0.0023185) [-0.52]

s\_pole = (0.059509 +/- 0.00052444)  
 + i\*(+0.0035426 +/- 0.00055797) [-0.53]

|                          |                         |
|--------------------------|-------------------------|
| pi:omega                 | pi:phi                  |
| ===== =====              |                         |
| k_re= -0.0454 +/- 0.0011 | k_re= 0.0137 +/- 0.0014 |
| k_im= -0.0087 +/- 0.0015 | k_im= 0.0255 +/- 0.0022 |
| corr= [-0.49]            | corr= [ 0.35]           |



| pi:omega/3^S_1(*)                                                   | pi:phi/3^S_1                                                        | pi:omega/3^D_1                                                      |
|---------------------------------------------------------------------|---------------------------------------------------------------------|---------------------------------------------------------------------|
| g = 0.0919 +/- 0.0086<br>arg(g)/pi= 0.0778 +/- 0.0227               | g = 0.0000 +/- 0.0000<br>arg(g)/pi= 0.4222 +/- 0.0227               | g = 0.0080 +/- 0.0041<br>arg(g)/pi= 0.1462 +/- 0.0266               |
| g_re= 0.0891 +/- 0.0087<br>g_im= 0.0222 +/- 0.0063<br>corr= [-0.02] | g_re= 0.0000 +/- 0.0000<br>g_im= 0.0000 +/- 0.0000<br>corr= [ 0.27] | g_re= 0.0072 +/- 0.0035<br>g_im= 0.0036 +/- 0.0023<br>corr= [ 0.97] |
| Br = 0.8740 +/- 0.0424                                              | Br = 0.0000 +/- 0.0000                                              | Br = 0.0066 +/- 0.0061                                              |

```
--
pi:omega[-] pi:phi[+] lower half-plane
*** not found on > 5% cfigs ***
sqrt(s)_pole = (0.24405 +/- 0.001056)
+ (i/2)*(-0.014516 +/- 0.0023185) [ 0.52]

s_pole = (0.059509 +/- 0.00052444)
+ i*(-0.0035426 +/- 0.00055797) [ 0.53]
```

| pi:omega                                                             | pi:phi                                                               |
|----------------------------------------------------------------------|----------------------------------------------------------------------|
| k_re= 0.0454 +/- 0.0011<br>k_im= -0.0087 +/- 0.0015<br>corr= [ 0.49] | k_re= -0.0137 +/- 0.0014<br>k_im= 0.0255 +/- 0.0022<br>corr= [-0.35] |

| pi:omega/3^S_1(*)                                                    | pi:phi/3^S_1                                                         | pi:omega/3^D_1                                                       |
|----------------------------------------------------------------------|----------------------------------------------------------------------|----------------------------------------------------------------------|
| g = 0.0919 +/- 0.0086<br>arg(g)/pi= -0.0778 +/- 0.0227               | g = 0.0000 +/- 0.0000<br>arg(g)/pi= 0.5778 +/- 0.0227                | g = 0.0080 +/- 0.0041<br>arg(g)/pi= -0.1462 +/- 0.0266               |
| g_re= 0.0891 +/- 0.0087<br>g_im= -0.0222 +/- 0.0063<br>corr= [ 0.02] | g_re= -0.0000 +/- 0.0000<br>g_im= 0.0000 +/- 0.0000<br>corr= [-0.27] | g_re= 0.0072 +/- 0.0035<br>g_im= -0.0036 +/- 0.0023<br>corr= [-0.97] |
| Br = 0.8740 +/- 0.0424                                               | Br = 0.0000 +/- 0.0000                                               | Br = 0.0066 +/- 0.0061                                               |

```
--
pi:omega[-] pi:phi[-] upper half-plane

sqrt(s)_pole = (0.24406 +/- 0.0011281)
+ (i/2)*(+0.014523 +/- 0.0024019) [-0.54]

s_pole = (0.059511 +/- 0.00056028)
+ i*(+0.0035443 +/- 0.00057749) [-0.54]
```

| pi:omega                                                              | pi:phi                                                                |
|-----------------------------------------------------------------------|-----------------------------------------------------------------------|
| k_re= -0.0454 +/- 0.0012<br>k_im= -0.0087 +/- 0.0015<br>corr= [-0.51] | k_re= -0.0137 +/- 0.0014<br>k_im= -0.0255 +/- 0.0023<br>corr= [ 0.33] |

| pi:omega/3^S_1(*)                                                   | pi:phi/3^S_1                                                        | pi:omega/3^D_1                                                      |
|---------------------------------------------------------------------|---------------------------------------------------------------------|---------------------------------------------------------------------|
| g = 0.0919 +/- 0.0088<br>arg(g)/pi= 0.0777 +/- 0.0224               | g = 0.0000 +/- 0.0000<br>arg(g)/pi= 0.4223 +/- 0.0224               | g = 0.0080 +/- 0.0042<br>arg(g)/pi= 0.1463 +/- 0.0278               |
| g_re= 0.0892 +/- 0.0088<br>g_im= 0.0222 +/- 0.0064<br>corr= [ 0.06] | g_re= 0.0000 +/- 0.0000<br>g_im= 0.0000 +/- 0.0000<br>corr= [ 0.23] | g_re= 0.0072 +/- 0.0036<br>g_im= 0.0036 +/- 0.0024<br>corr= [ 0.97] |



# 1 Successful Parameterizations

```

Br = 0.8742 +/- 0.0434 | Br = 0.0000 +/- 0.0000 | Br = 0.0067 +/- 0.0064 |

--
pi:omega[-] pi:phi[-] lower half-plane

sqrt(s)_pole = (0.24406 +/- 0.0011281)
               + (i/2)*(-0.014523 +/- 0.0024019) [ 0.54]

s_pole = (0.059511 +/- 0.00056028)
          + i*(-0.0035443 +/- 0.00057749) [ 0.54]

=====
pi:omega | pi:phi |
=====
k_re= 0.0454 +/- 0.0012 | k_re= 0.0137 +/- 0.0014 |
k_im= -0.0087 +/- 0.0015 | k_im= -0.0255 +/- 0.0023 |
corr= [ 0.51] | corr= [-0.33] |

=====
pi:omega/3^S_1(*) | pi:phi/3^S_1 | pi:omega/3^D_1 |
=====
|g|= 0.0919 +/- 0.0088 | |g|= 0.0000 +/- 0.0000 | |g|= 0.0080 +/- 0.0042 |
arg(g)/pi= -0.0777 +/- 0.0224 | arg(g)/pi= 0.5777 +/- 0.0224 | arg(g)/pi= -0.1463 +/- 0.0278 |
-----
g_re= 0.0892 +/- 0.0088 | g_re= -0.0000 +/- 0.0000 | g_re= 0.0072 +/- 0.0036 |
g_im= -0.0222 +/- 0.0064 | g_im= 0.0000 +/- 0.0000 | g_im= -0.0036 +/- 0.0024 |
corr= [-0.06] | corr= [-0.23] | corr= [-0.97] |
-----
Br = 0.8742 +/- 0.0434 | Br = 0.0000 +/- 0.0000 | Br = 0.0067 +/- 0.0064 |

```



## 1.5 coupled\_po\_pp.3s1\_3d1.pole+G0\_3s1\_3S1.gorder0\_3s1\_3d1.irho

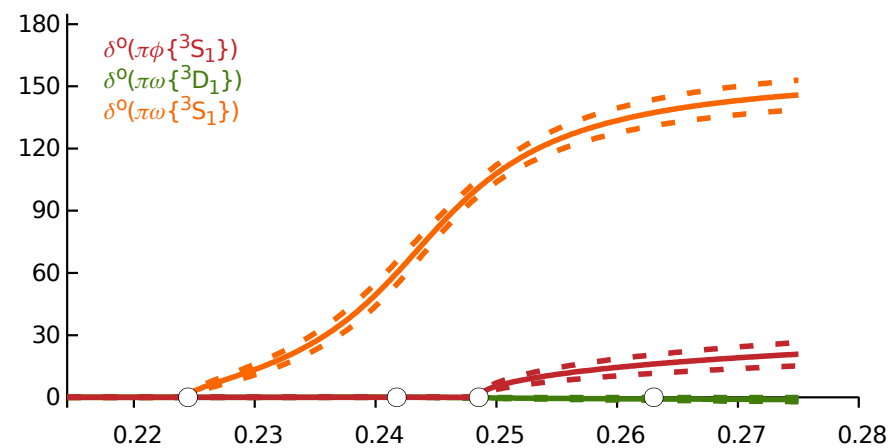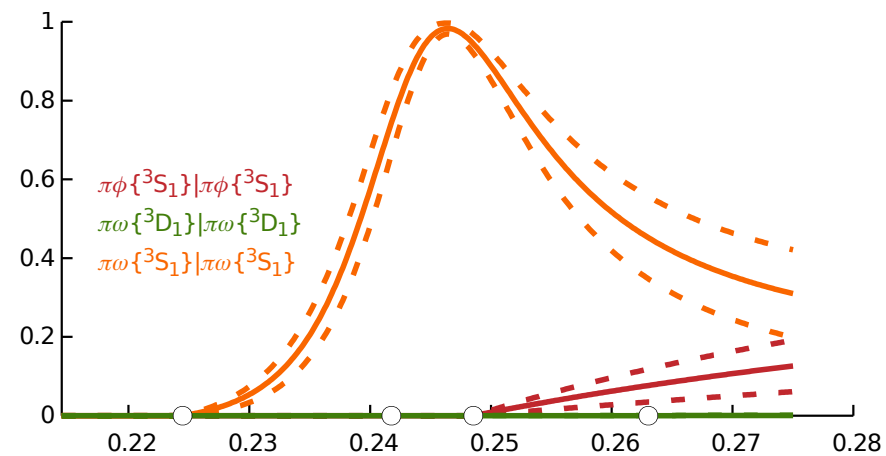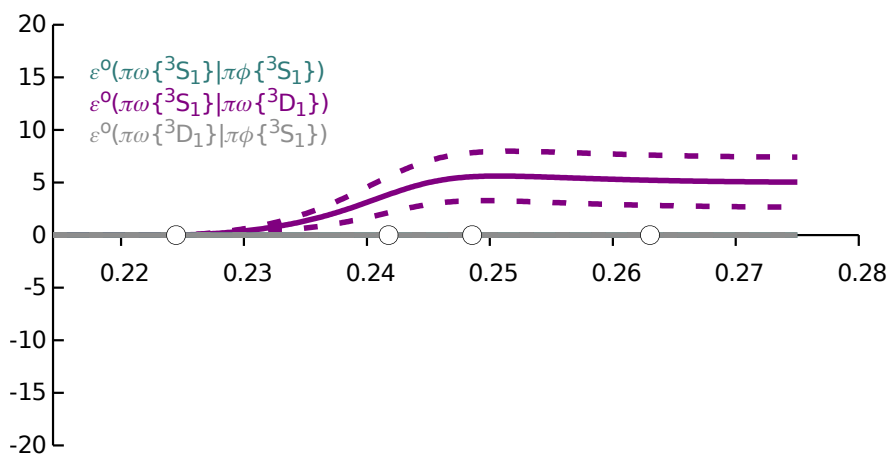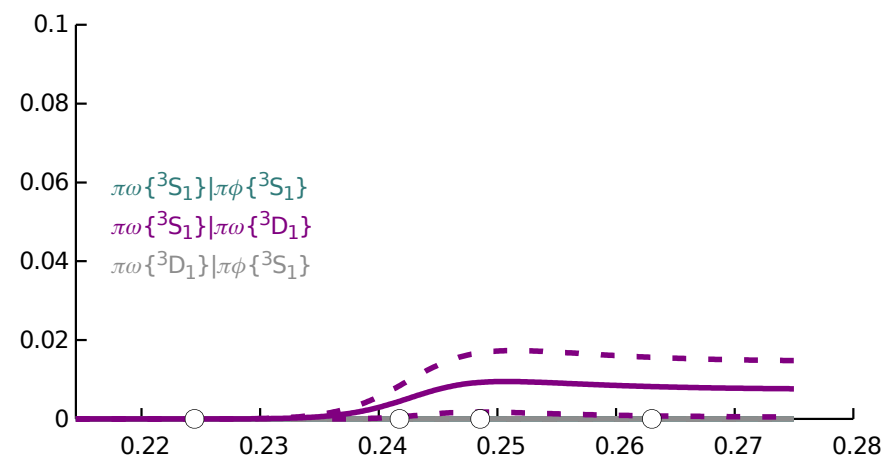



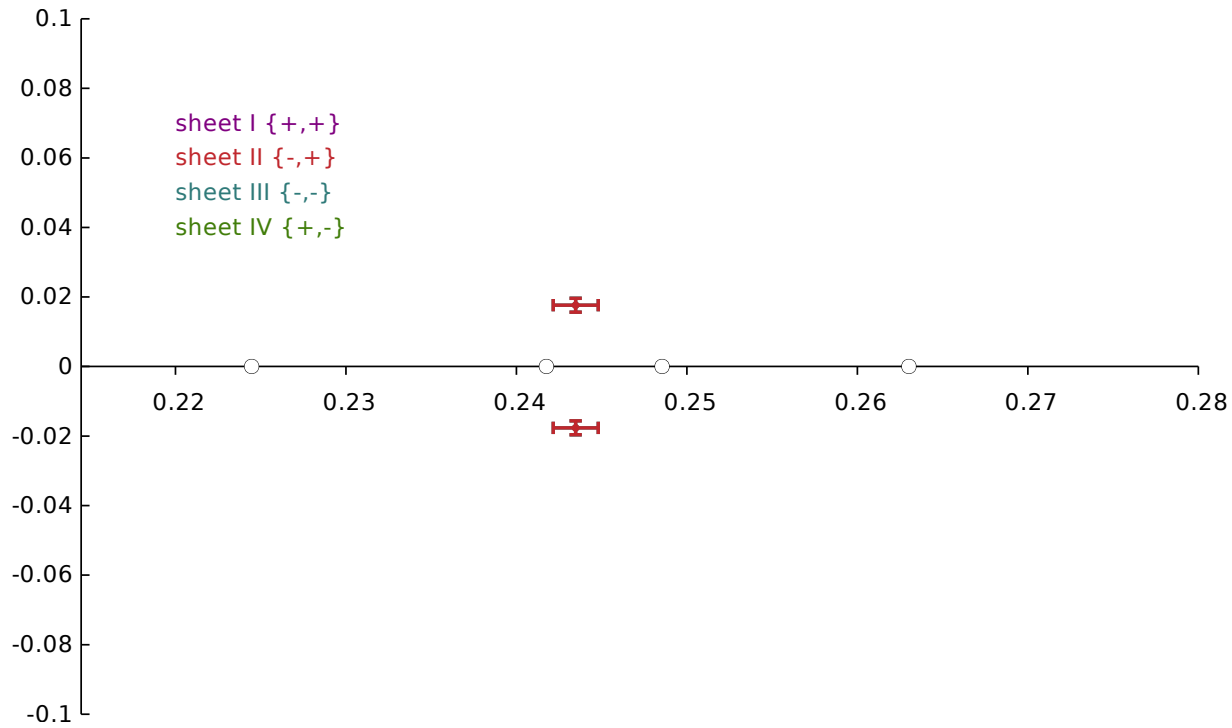

### parameter values

```

minimised with chisq/nDoF = 36.73 / (36 - 5) = 1.18
=====
JP1+_g_pi:omega/3^D_1_pole0_order0 | 1.1391 +/- 0.50529 | 1.00 0.71 -0.41 -0.06 0.05
JP1+_g_pi:omega/3^S_1_pole0_order0 | 0.11142 +/- 0.0081806 | 1.00 -0.57 -0.05 -0.05
JP1+_gamma_pi:omega/3^S_1|pi:omega/3^S_1_orde | -0.40171 +/- 0.22802 | 1.00 0.21 -0.01
JP1+_gamma_pi:phi/3^S_1|pi:phi/3^S_1_order0 | 0.97026 +/- 0.28629 | 1.00 -0.31
JP1+_m_pole0 | 0.24647 +/- 0.00070097 | 1.00
=====

```

### pole singularities

pi:omega[-] pi:phi[+] upper half-plane

```

sqrt(s)_pole = (0.24348 +/- 0.0013168)
               + (i/2)*(+0.017627 +/- 0.0020049) [-0.50]

```

```

s_pole = (0.059203 +/- 0.0006502)
          + i*(+0.0042917 +/- 0.00047698) [-0.48]

```

```

=====
pi:omega | pi:phi |
=====
k_re= -0.0451 +/- 0.0014 | k_re= 0.0153 +/- 0.0012 |
k_im= -0.0106 +/- 0.0013 | k_im= 0.0276 +/- 0.0022 |
corr= [-0.55] | corr= [-0.06] |
=====

```



# 1 Successful Parameterizations

| pi:omega/3^S_1(*)            | pi:phi/3^S_1                 | pi:omega/3^D_1               |
|------------------------------|------------------------------|------------------------------|
| g = 0.1060 +/- 0.0062        | g = 0.0000 +/- 0.0000        | g = 0.0097 +/- 0.0042        |
| arg(g)/pi= 0.0775 +/- 0.0268 | arg(g)/pi= 0.4225 +/- 0.0268 | arg(g)/pi= 0.1790 +/- 0.0251 |
| g_re= 0.1029 +/- 0.0061      | g_re= 0.0000 +/- 0.0000      | g_re= 0.0082 +/- 0.0033      |
| g_im= 0.0256 +/- 0.0090      | g_im= 0.0000 +/- 0.0000      | g_im= 0.0052 +/- 0.0028      |
| corr= [-0.07]                | corr= [-0.28]                | corr= [ 0.97]                |
| Br = 0.9502 +/- 0.0231       | Br = 0.0000 +/- 0.0000       | Br = 0.0079 +/- 0.0064       |

--  
pi:omega[-] pi:phi[+] lower half-plane

sqrts)\_pole = (0.24348 +/- 0.0013168)  
+ (i/2)\*(-0.017627 +/- 0.0020049) [ 0.50]

s\_pole = (0.059203 +/- 0.0006502)  
+ i\*(-0.0042917 +/- 0.00047698) [ 0.48]

| pi:omega                 | pi:phi                   |
|--------------------------|--------------------------|
| k_re= 0.0451 +/- 0.0014  | k_re= -0.0153 +/- 0.0012 |
| k_im= -0.0106 +/- 0.0013 | k_im= 0.0276 +/- 0.0022  |
| corr= [ 0.55]            | corr= [ 0.06]            |

| pi:omega/3^S_1(*)             | pi:phi/3^S_1                 | pi:omega/3^D_1                |
|-------------------------------|------------------------------|-------------------------------|
| g = 0.1060 +/- 0.0062         | g = 0.0000 +/- 0.0000        | g = 0.0097 +/- 0.0042         |
| arg(g)/pi= -0.0775 +/- 0.0268 | arg(g)/pi= 0.5775 +/- 0.0268 | arg(g)/pi= -0.1790 +/- 0.0251 |
| g_re= 0.1029 +/- 0.0061       | g_re= -0.0000 +/- 0.0000     | g_re= 0.0082 +/- 0.0033       |
| g_im= -0.0256 +/- 0.0090      | g_im= 0.0000 +/- 0.0000      | g_im= -0.0052 +/- 0.0028      |
| corr= [ 0.07]                 | corr= [ 0.28]                | corr= [-0.97]                 |
| Br = 0.9502 +/- 0.0231        | Br = 0.0000 +/- 0.0000       | Br = 0.0079 +/- 0.0064        |

--  
pi:omega[-] pi:phi[-] upper half-plane

sqrts)\_pole = (0.24348 +/- 0.00132)  
+ (i/2)\*(+0.017627 +/- 0.0020158) [-0.50]

s\_pole = (0.059203 +/- 0.00065185)  
+ i\*(+0.0042918 +/- 0.0004796) [-0.48]

| pi:omega                 | pi:phi                   |
|--------------------------|--------------------------|
| k_re= -0.0451 +/- 0.0014 | k_re= -0.0153 +/- 0.0012 |
| k_im= -0.0106 +/- 0.0013 | k_im= -0.0276 +/- 0.0022 |
| corr= [-0.55]            | corr= [-0.06]            |

| pi:omega/3^S_1(*)            | pi:phi/3^S_1                 | pi:omega/3^D_1               |
|------------------------------|------------------------------|------------------------------|
| g = 0.1061 +/- 0.0062        | g = 0.0000 +/- 0.0000        | g = 0.0097 +/- 0.0043        |
| arg(g)/pi= 0.0775 +/- 0.0269 | arg(g)/pi= 0.4225 +/- 0.0269 | arg(g)/pi= 0.1791 +/- 0.0252 |
| g_re= 0.1029 +/- 0.0061      | g_re= 0.0000 +/- 0.0000      | g_re= 0.0082 +/- 0.0033      |
| g_im= 0.0256 +/- 0.0090      | g_im= 0.0000 +/- 0.0000      | g_im= 0.0052 +/- 0.0028      |
| corr= [-0.08]                | corr= [-0.27]                | corr= [ 0.97]                |
| Br = 0.9502 +/- 0.0232       | Br = 0.0000 +/- 0.0000       | Br = 0.0079 +/- 0.0064       |



```
--
pi:omega[-] pi:phi[-] lower half-plane

sqrt(s)_pole = (0.24348 +/- 0.00132)
               + (i/2)*(-0.017627 +/- 0.0020158) [ 0.50]

s_pole = (0.059203 +/- 0.00065185)
         + i*(-0.0042918 +/- 0.0004796) [ 0.48]

=====
pi:omega | pi:phi |
=====
k_re= 0.0451 +/- 0.0014 | k_re= 0.0153 +/- 0.0012 |
k_im= -0.0106 +/- 0.0013 | k_im= -0.0276 +/- 0.0022 |
corr= [ 0.55] | corr= [ 0.06] |

=====
pi:omega/3^S_1(*) | pi:phi/3^S_1 | pi:omega/3^D_1 |
=====
|g|= 0.1061 +/- 0.0062 | |g|= 0.0000 +/- 0.0000 | |g|= 0.0097 +/- 0.0043 |
arg(g)/pi= -0.0775 +/- 0.0269 | arg(g)/pi= 0.5775 +/- 0.0269 | arg(g)/pi= -0.1791 +/- 0.0252 |
-----
g_re= 0.1029 +/- 0.0061 | g_re= -0.0000 +/- 0.0000 | g_re= 0.0082 +/- 0.0033 |
g_im= -0.0256 +/- 0.0090 | g_im= 0.0000 +/- 0.0000 | g_im= -0.0052 +/- 0.0028 |
corr= [ 0.08] | corr= [ 0.27] | corr= [-0.97] |
-----
Br = 0.9502 +/- 0.0232 | Br = 0.0000 +/- 0.0000 | Br = 0.0079 +/- 0.0064 |
```



## 1.6 coupled\_po\_pp.3s1\_3d1.pole+G0\_3s1\_3S1.gorder0\_3s1\_3d1.pole0\_sub

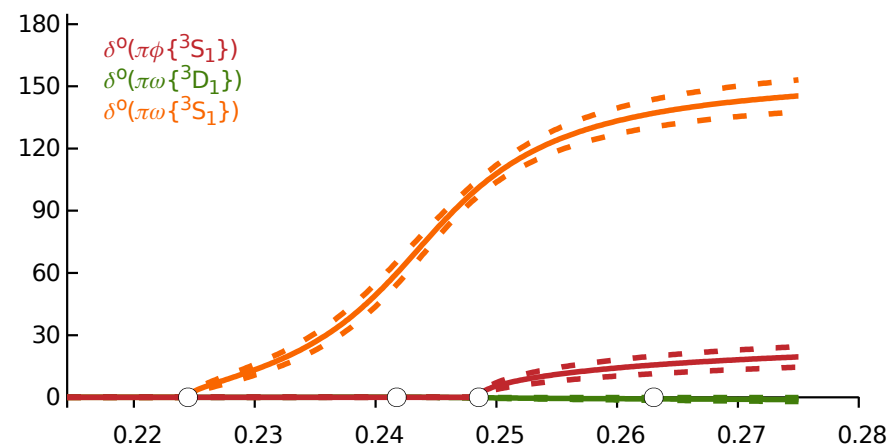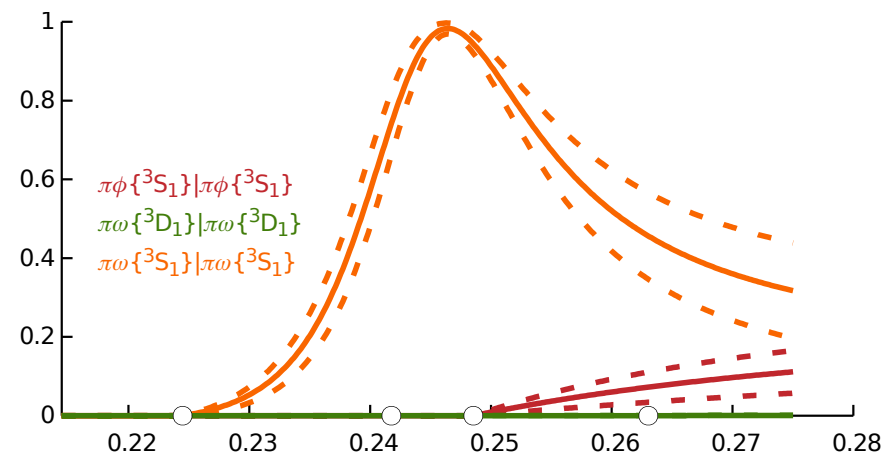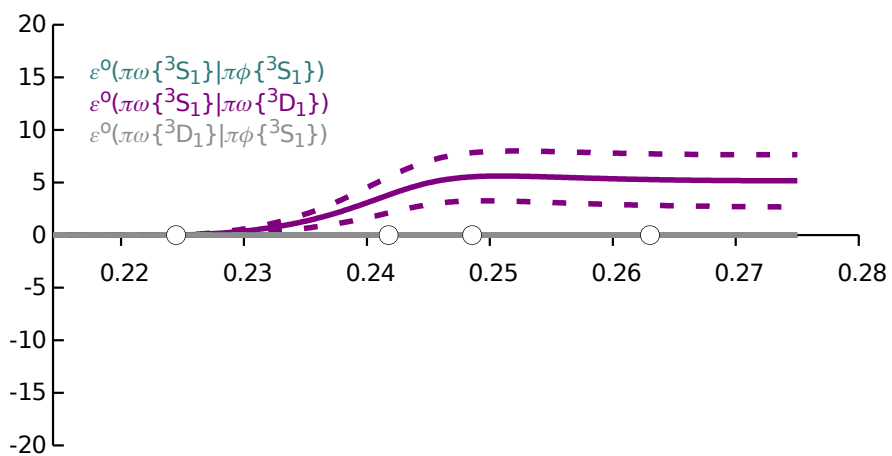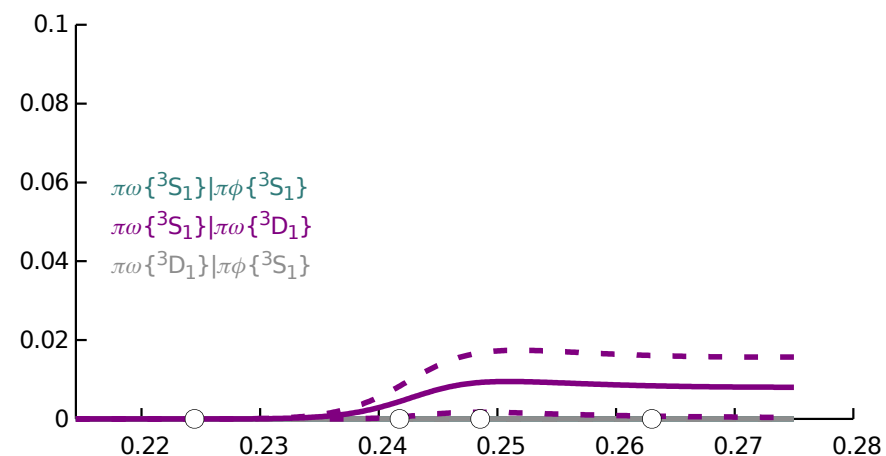



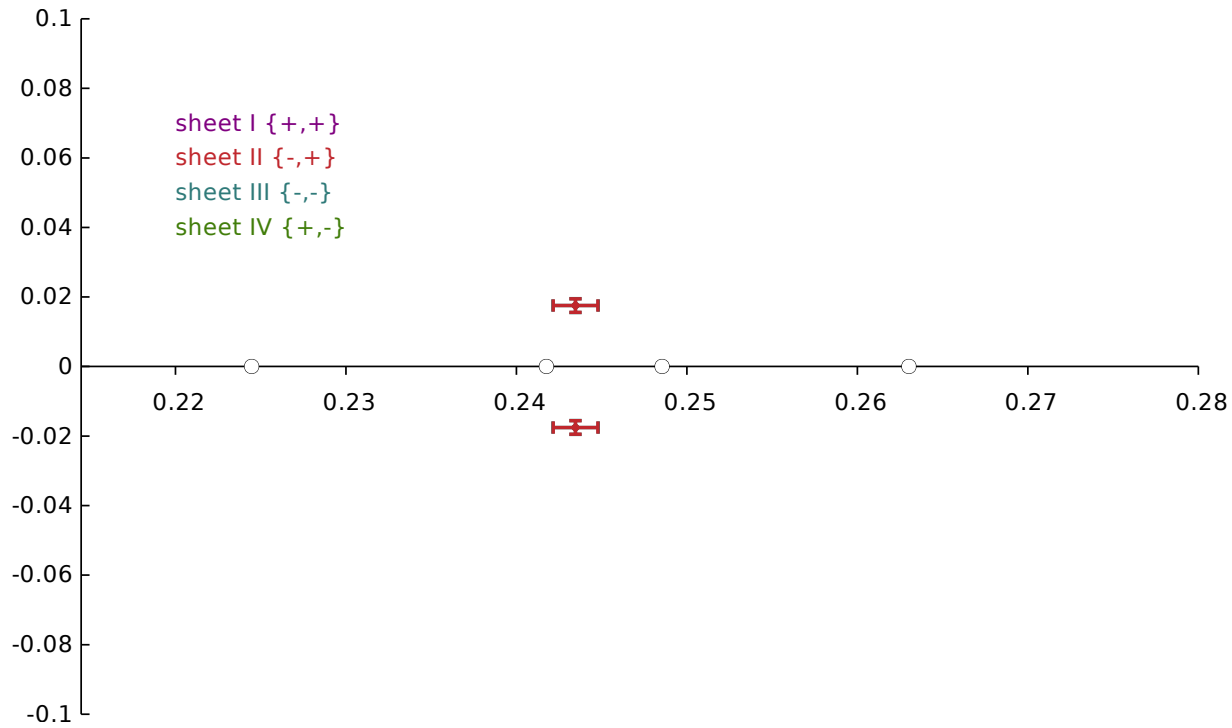

### parameter values

```

minimised with chisq/nDoF = 36.76 / (36 - 5) = 1.19
=====
JP1+_g_pi:omega/3^D_1_pole0_order0 | 1.0778 +/- 0.47432 | 1.00 0.70 -0.39 -0.06 0.05
JP1+_g_pi:omega/3^S_1_pole0_order0 | 0.10573 +/- 0.0070454 | 1.00 -0.54 -0.06 -0.05
JP1+_gamma_pi:omega/3^S_1|pi:omega/3^S_1_orde | -0.34601 +/- 0.19317 | 1.00 0.22 -0.01
JP1+_gamma_pi:phi/3^S_1|pi:phi/3^S_1_order0 | 0.89837 +/- 0.24036 | 1.00 -0.23
JP1+_m_pole0 | 0.24647 +/- 0.00069632 | 1.00
=====

```

### pole singularities

pi:omega[-] pi:phi[+] upper half-plane

```

sqrt(s)_pole = (0.24347 +/- 0.0013132)
               + (i/2)*(+0.017524 +/- 0.0019625) [-0.48]

```

```

s_pole = (0.059202 +/- 0.0006479)
         + i*(+0.0042666 +/- 0.00046717) [-0.46]

```

```

=====
pi:omega | pi:phi |
=====
k_re= -0.0451 +/- 0.0014 | k_re= 0.0152 +/- 0.0012 |
k_im= -0.0106 +/- 0.0013 | k_im= 0.0276 +/- 0.0022 |
corr= [-0.53] | corr= [-0.09] |
=====

```



# 1 Successful Parameterizations

| pi:omega/3^S_1(*)            | pi:phi/3^S_1                 | pi:omega/3^D_1               |
|------------------------------|------------------------------|------------------------------|
| g = 0.1056 +/- 0.0061        | g = 0.0000 +/- 0.0000        | g = 0.0096 +/- 0.0042        |
| arg(g)/pi= 0.0782 +/- 0.0272 | arg(g)/pi= 0.4218 +/- 0.0272 | arg(g)/pi= 0.1813 +/- 0.0257 |
| g_re= 0.1024 +/- 0.0062      | g_re= 0.0000 +/- 0.0000      | g_re= 0.0081 +/- 0.0032      |
| g_im= 0.0257 +/- 0.0089      | g_im= 0.0000 +/- 0.0000      | g_im= 0.0052 +/- 0.0027      |
| corr= [-0.15]                | corr= [-0.23]                | corr= [ 0.97]                |
| Br = 0.9469 +/- 0.0243       | Br = 0.0000 +/- 0.0000       | Br = 0.0078 +/- 0.0062       |

--  
pi:omega[-] pi:phi[+] lower half-plane

sqrt(s)\_pole = (0.24347 +/- 0.0013132)  
+ (i/2)\*(-0.017524 +/- 0.0019625) [ 0.48]

s\_pole = (0.059202 +/- 0.0006479)  
+ i\*(-0.0042666 +/- 0.00046717) [ 0.46]

| pi:omega                 | pi:phi                   |
|--------------------------|--------------------------|
| k_re= 0.0451 +/- 0.0014  | k_re= -0.0152 +/- 0.0012 |
| k_im= -0.0106 +/- 0.0013 | k_im= 0.0276 +/- 0.0022  |
| corr= [ 0.53]            | corr= [ 0.09]            |

| pi:omega/3^S_1(*)             | pi:phi/3^S_1                 | pi:omega/3^D_1                |
|-------------------------------|------------------------------|-------------------------------|
| g = 0.1056 +/- 0.0061         | g = 0.0000 +/- 0.0000        | g = 0.0096 +/- 0.0042         |
| arg(g)/pi= -0.0782 +/- 0.0272 | arg(g)/pi= 0.5782 +/- 0.0272 | arg(g)/pi= -0.1813 +/- 0.0257 |
| g_re= 0.1024 +/- 0.0062       | g_re= -0.0000 +/- 0.0000     | g_re= 0.0081 +/- 0.0032       |
| g_im= -0.0257 +/- 0.0089      | g_im= 0.0000 +/- 0.0000      | g_im= -0.0052 +/- 0.0027      |
| corr= [ 0.15]                 | corr= [ 0.23]                | corr= [-0.97]                 |
| Br = 0.9469 +/- 0.0243        | Br = 0.0000 +/- 0.0000       | Br = 0.0078 +/- 0.0062        |

--  
pi:omega[-] pi:phi[-] upper half-plane

sqrt(s)\_pole = (0.24347 +/- 0.0013258)  
+ (i/2)\*(+0.017524 +/- 0.0019962) [-0.48]

s\_pole = (0.059201 +/- 0.00065408)  
+ i\*(+0.0042665 +/- 0.00047541) [-0.46]

| pi:omega                 | pi:phi                   |
|--------------------------|--------------------------|
| k_re= -0.0451 +/- 0.0014 | k_re= -0.0152 +/- 0.0012 |
| k_im= -0.0106 +/- 0.0013 | k_im= -0.0276 +/- 0.0022 |
| corr= [-0.53]            | corr= [-0.08]            |

| pi:omega/3^S_1(*)            | pi:phi/3^S_1                 | pi:omega/3^D_1               |
|------------------------------|------------------------------|------------------------------|
| g = 0.1056 +/- 0.0062        | g = 0.0000 +/- 0.0000        | g = 0.0096 +/- 0.0042        |
| arg(g)/pi= 0.0782 +/- 0.0275 | arg(g)/pi= 0.4218 +/- 0.0275 | arg(g)/pi= 0.1813 +/- 0.0260 |
| g_re= 0.1024 +/- 0.0063      | g_re= 0.0000 +/- 0.0000      | g_re= 0.0081 +/- 0.0033      |
| g_im= 0.0257 +/- 0.0090      | g_im= 0.0000 +/- 0.0000      | g_im= 0.0052 +/- 0.0028      |
| corr= [-0.15]                | corr= [-0.23]                | corr= [ 0.97]                |
| Br = 0.9469 +/- 0.0244       | Br = 0.0000 +/- 0.0000       | Br = 0.0078 +/- 0.0063       |



```
--
```

```
pi:omega[-] pi:phi[-] lower half-plane
```

```
sqrt(s)_pole = (0.24347 +/- 0.0013258)
               + (i/2)*(-0.017524 +/- 0.0019962) [ 0.48]
```

```
s_pole = (0.059201 +/- 0.00065408)
          + i*(-0.0042665 +/- 0.00047541) [ 0.46]
```

| pi:omega                 |  | pi:phi                   |  |
|--------------------------|--|--------------------------|--|
| =====                    |  | =====                    |  |
| k_re= 0.0451 +/- 0.0014  |  | k_re= 0.0152 +/- 0.0012  |  |
| k_im= -0.0106 +/- 0.0013 |  | k_im= -0.0276 +/- 0.0022 |  |
| corr= [ 0.53]            |  | corr= [ 0.08]            |  |

| pi:omega/3^S_1(*)             |  | pi:phi/3^S_1                 |  | pi:omega/3^D_1                |  |
|-------------------------------|--|------------------------------|--|-------------------------------|--|
| =====                         |  | =====                        |  | =====                         |  |
| g = 0.1056 +/- 0.0062         |  | g = 0.0000 +/- 0.0000        |  | g = 0.0096 +/- 0.0042         |  |
| arg(g)/pi= -0.0782 +/- 0.0275 |  | arg(g)/pi= 0.5782 +/- 0.0275 |  | arg(g)/pi= -0.1813 +/- 0.0260 |  |
| -----                         |  | -----                        |  | -----                         |  |
| g_re= 0.1024 +/- 0.0063       |  | g_re= -0.0000 +/- 0.0000     |  | g_re= 0.0081 +/- 0.0033       |  |
| g_im= -0.0257 +/- 0.0090      |  | g_im= 0.0000 +/- 0.0000      |  | g_im= -0.0052 +/- 0.0028      |  |
| corr= [ 0.15]                 |  | corr= [ 0.23]                |  | corr= [-0.97]                 |  |
| -----                         |  | -----                        |  | -----                         |  |
| Br = 0.9469 +/- 0.0244        |  | Br = 0.0000 +/- 0.0000       |  | Br = 0.0078 +/- 0.0063        |  |



## 1.7 coupled\_po\_pp.3s1\_3d1.pole+G0\_3s1\_3S1.gorder0\_3s1\_3d1.threshold\_sub

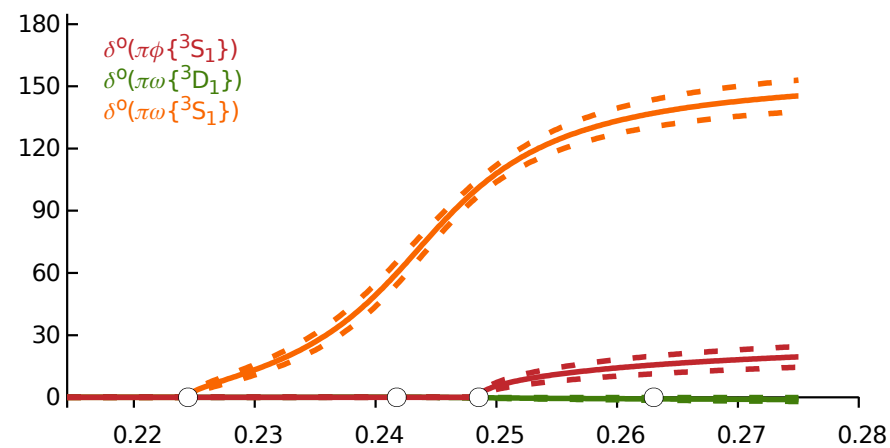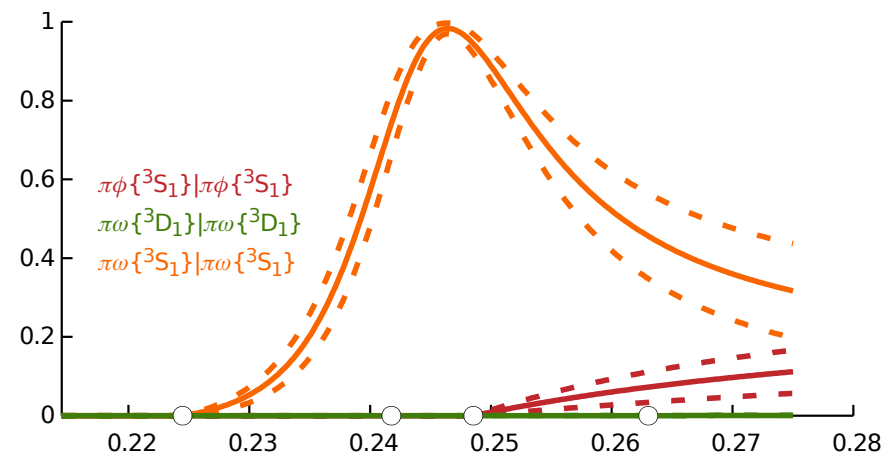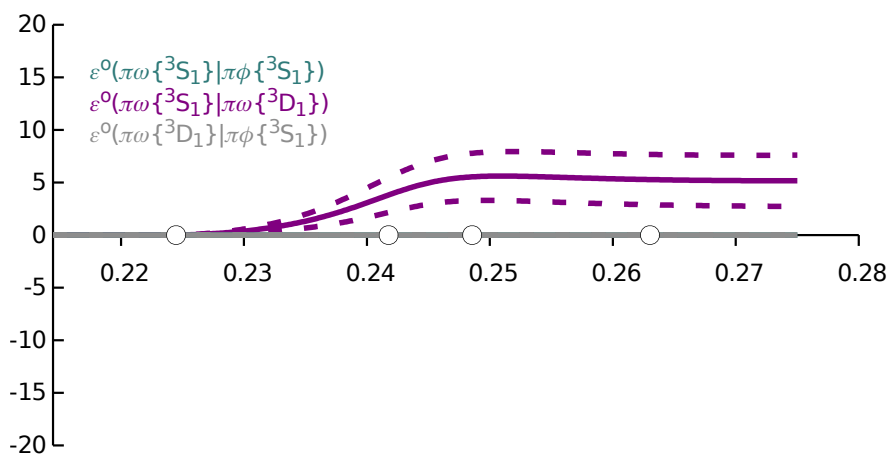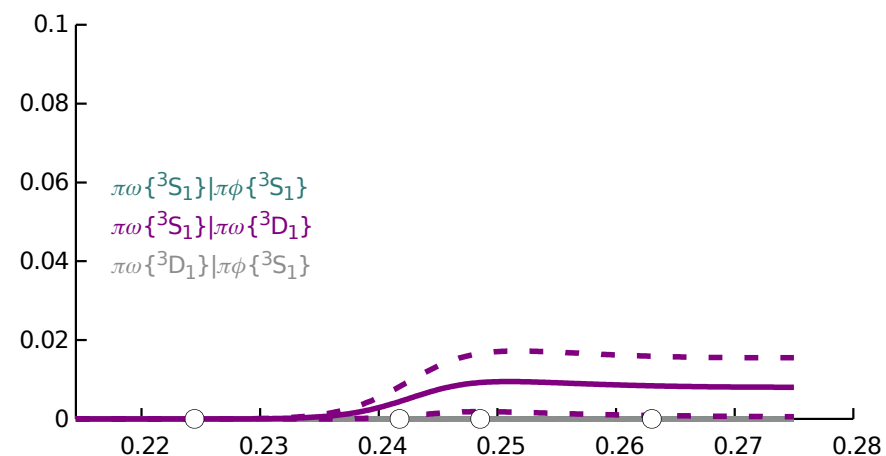



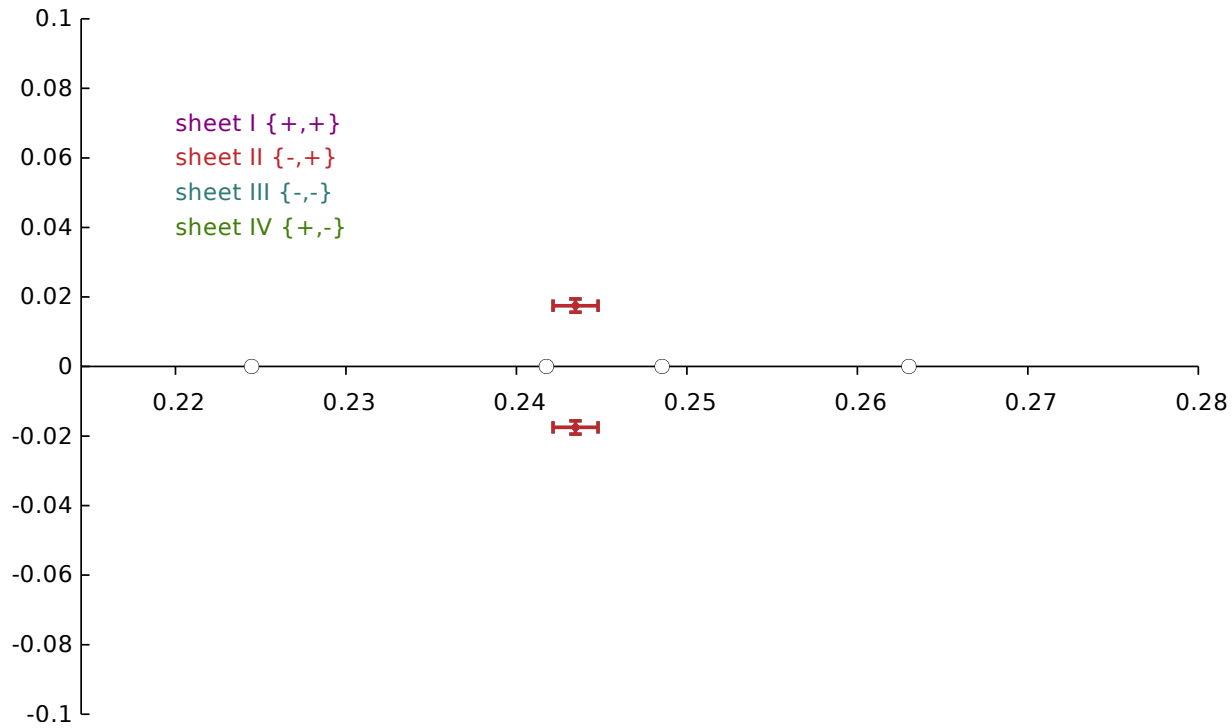

### parameter values

minimised with  $\text{chisq}/\text{nDoF} = 36.76 / (36 - 5) = 1.19$

|                                               |  |                       |  |      |      |       |       |       |
|-----------------------------------------------|--|-----------------------|--|------|------|-------|-------|-------|
| JP1+_g_pi:omega/3^D_1_pole0_order0            |  | 1.0754 +/- 0.46101    |  | 1.00 | 0.65 | -0.36 | -0.05 | -0.24 |
| JP1+_g_pi:omega/3^S_1_pole0_order0            |  | 0.10211 +/- 0.0057448 |  |      | 1.00 | -0.27 | 0.03  | -0.47 |
| JP1+_gamma_pi:omega/3^S_1 pi:omega/3^S_1_orde |  | -0.33282 +/- 0.18006  |  |      |      | 1.00  | 0.21  | 0.16  |
| JP1+_gamma_pi:phi/3^S_1 pi:phi/3^S_1_order0   |  | 0.99592 +/- 0.30191   |  |      |      |       | 1.00  | -0.27 |
| JP1+_m_pole0                                  |  | 0.24427 +/- 0.0007151 |  |      |      |       |       | 1.00  |

### pole singularities

pi:omega[-] pi:phi[+] upper half-plane

$\text{sqrt}(s)_{\text{pole}} = (0.24347 \pm 0.0013163)$   
 $+ (i/2)(+0.017521 \pm 0.001914) [-0.46]$

$s_{\text{pole}} = (0.059203 \pm 0.00064875)$   
 $+ i(+0.004266 \pm 0.00045596) [-0.44]$

|                          |                         |
|--------------------------|-------------------------|
| pi:omega                 | pi:phi                  |
| ===== =====              | =====                   |
| k_re= -0.0451 +/- 0.0014 | k_re= 0.0152 +/- 0.0012 |
| k_im= -0.0106 +/- 0.0013 | k_im= 0.0275 +/- 0.0022 |
| corr= [-0.52]            | corr= [-0.13]           |



# 1 Successful Parameterizations

| pi:omega/3^S_1(*)            | pi:phi/3^S_1                 | pi:omega/3^D_1               |
|------------------------------|------------------------------|------------------------------|
| g = 0.1056 +/- 0.0059        | g = 0.0000 +/- 0.0000        | g = 0.0096 +/- 0.0041        |
| arg(g)/pi= 0.0781 +/- 0.0271 | arg(g)/pi= 0.4219 +/- 0.0271 | arg(g)/pi= 0.1814 +/- 0.0252 |
| g_re= 0.1024 +/- 0.0061      | g_re= 0.0000 +/- 0.0000      | g_re= 0.0081 +/- 0.0032      |
| g_im= 0.0256 +/- 0.0089      | g_im= 0.0000 +/- 0.0000      | g_im= 0.0052 +/- 0.0027      |
| corr= [-0.17]                | corr= [-0.22]                | corr= [ 0.96]                |
| Br = 0.9471 +/- 0.0243       | Br = 0.0000 +/- 0.0000       | Br = 0.0078 +/- 0.0062       |

--

pi:omega[-] pi:phi[+] lower half-plane

sqrt(s)\_pole = (0.24347 +/- 0.0013163)  
+ (i/2)\*(-0.017521 +/- 0.001914) [ 0.46]

s\_pole = (0.059203 +/- 0.00064875)  
+ i\*(-0.004266 +/- 0.00045596) [ 0.44]

| pi:omega                 | pi:phi                   |
|--------------------------|--------------------------|
| k_re= 0.0451 +/- 0.0014  | k_re= -0.0152 +/- 0.0012 |
| k_im= -0.0106 +/- 0.0013 | k_im= 0.0275 +/- 0.0022  |
| corr= [ 0.52]            | corr= [ 0.13]            |

| pi:omega/3^S_1(*)             | pi:phi/3^S_1                 | pi:omega/3^D_1                |
|-------------------------------|------------------------------|-------------------------------|
| g = 0.1056 +/- 0.0059         | g = 0.0000 +/- 0.0000        | g = 0.0096 +/- 0.0041         |
| arg(g)/pi= -0.0781 +/- 0.0271 | arg(g)/pi= 0.5781 +/- 0.0271 | arg(g)/pi= -0.1814 +/- 0.0252 |
| g_re= 0.1024 +/- 0.0061       | g_re= -0.0000 +/- 0.0000     | g_re= 0.0081 +/- 0.0032       |
| g_im= -0.0256 +/- 0.0089      | g_im= 0.0000 +/- 0.0000      | g_im= -0.0052 +/- 0.0027      |
| corr= [ 0.17]                 | corr= [ 0.22]                | corr= [-0.96]                 |
| Br = 0.9471 +/- 0.0243        | Br = 0.0000 +/- 0.0000       | Br = 0.0078 +/- 0.0062        |

--

pi:omega[-] pi:phi[-] upper half-plane

sqrt(s)\_pole = (0.24347 +/- 0.001325)  
+ (i/2)\*(+0.017521 +/- 0.0019257) [-0.46]

s\_pole = (0.059203 +/- 0.00065316)  
+ i\*(+0.004266 +/- 0.0004586) [-0.44]

| pi:omega                 | pi:phi                   |
|--------------------------|--------------------------|
| k_re= -0.0451 +/- 0.0015 | k_re= -0.0152 +/- 0.0012 |
| k_im= -0.0106 +/- 0.0013 | k_im= -0.0275 +/- 0.0022 |
| corr= [-0.53]            | corr= [-0.13]            |

| pi:omega/3^S_1(*)            | pi:phi/3^S_1                 | pi:omega/3^D_1               |
|------------------------------|------------------------------|------------------------------|
| g = 0.1056 +/- 0.0060        | g = 0.0000 +/- 0.0000        | g = 0.0096 +/- 0.0041        |
| arg(g)/pi= 0.0781 +/- 0.0272 | arg(g)/pi= 0.4219 +/- 0.0272 | arg(g)/pi= 0.1814 +/- 0.0254 |
| g_re= 0.1024 +/- 0.0061      | g_re= 0.0000 +/- 0.0000      | g_re= 0.0081 +/- 0.0032      |
| g_im= 0.0256 +/- 0.0089      | g_im= 0.0000 +/- 0.0000      | g_im= 0.0052 +/- 0.0027      |
| corr= [-0.17]                | corr= [-0.23]                | corr= [ 0.96]                |
| Br = 0.9471 +/- 0.0243       | Br = 0.0000 +/- 0.0000       | Br = 0.0078 +/- 0.0062       |



# 1 Successful Parameterizations

```
--
pi:omega[-] pi:phi[-] lower half-plane

sqrt(s)_pole = (0.24347 +/- 0.001325)
               + (i/2)*(-0.017521 +/- 0.0019257) [ 0.46]

s_pole = (0.059203 +/- 0.00065316)
         + i*(-0.004266 +/- 0.0004586) [ 0.44]

=====
pi:omega | pi:phi |
=====
k_re= 0.0451 +/- 0.0015 | k_re= 0.0152 +/- 0.0012 |
k_im= -0.0106 +/- 0.0013 | k_im= -0.0275 +/- 0.0022 |
corr= [ 0.53] | corr= [ 0.13] |

=====
pi:omega/3^S_1(*) | pi:phi/3^S_1 | pi:omega/3^D_1 |
=====
|g|= 0.1056 +/- 0.0060 | |g|= 0.0000 +/- 0.0000 | |g|= 0.0096 +/- 0.0041 |
arg(g)/pi= -0.0781 +/- 0.0272 | arg(g)/pi= 0.5781 +/- 0.0272 | arg(g)/pi= -0.1814 +/- 0.0254 |
-----
g_re= 0.1024 +/- 0.0061 | g_re= -0.0000 +/- 0.0000 | g_re= 0.0081 +/- 0.0032 |
g_im= -0.0256 +/- 0.0089 | g_im= 0.0000 +/- 0.0000 | g_im= -0.0052 +/- 0.0027 |
corr= [ 0.17] | corr= [ 0.23] | corr= [-0.96] |
-----
Br = 0.9471 +/- 0.0243 | Br = 0.0000 +/- 0.0000 | Br = 0.0078 +/- 0.0062 |
```



## 1.8 coupled\_po\_pp.3s1\_3d1.pole+G0\_3s1\_3sd1\_3S1\_3sS1.gorder0\_3s1.irho

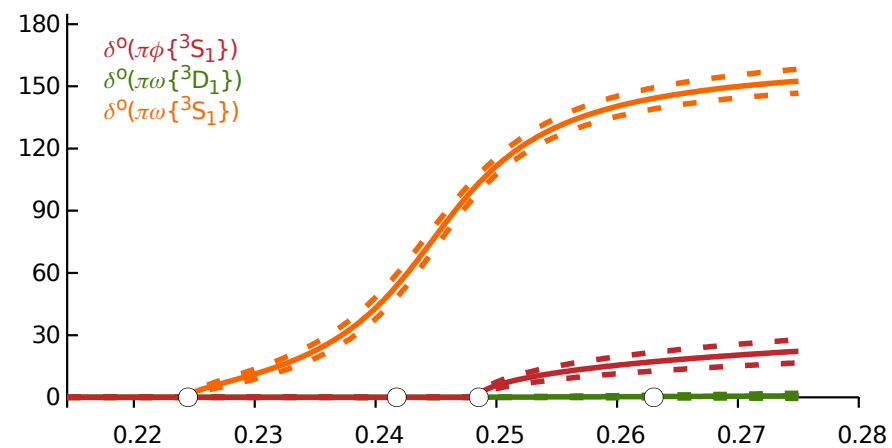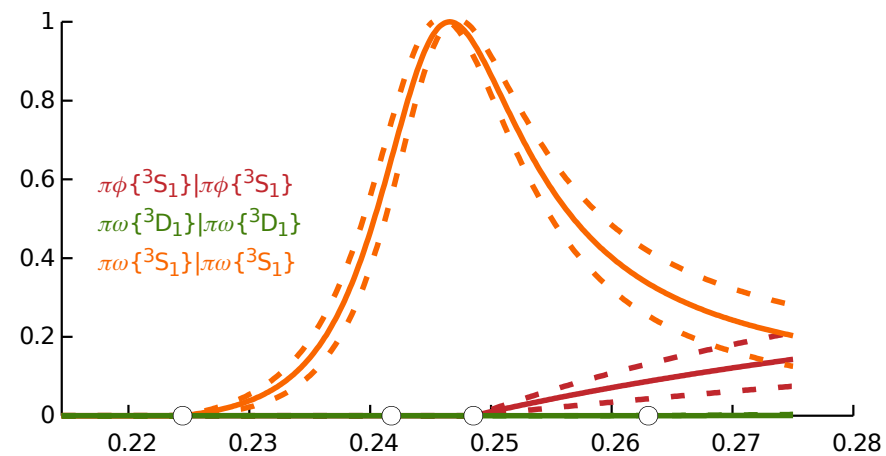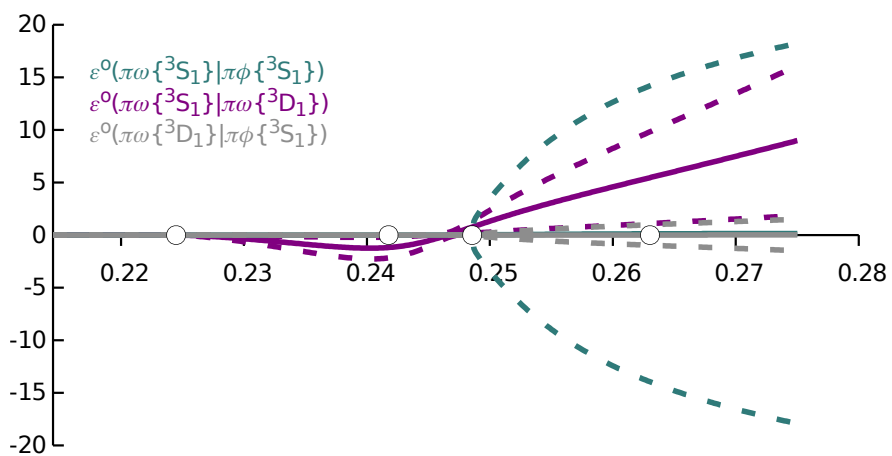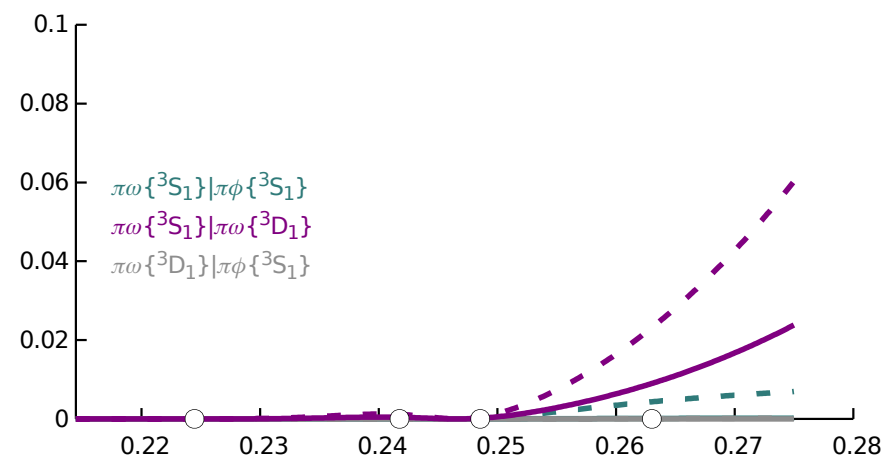



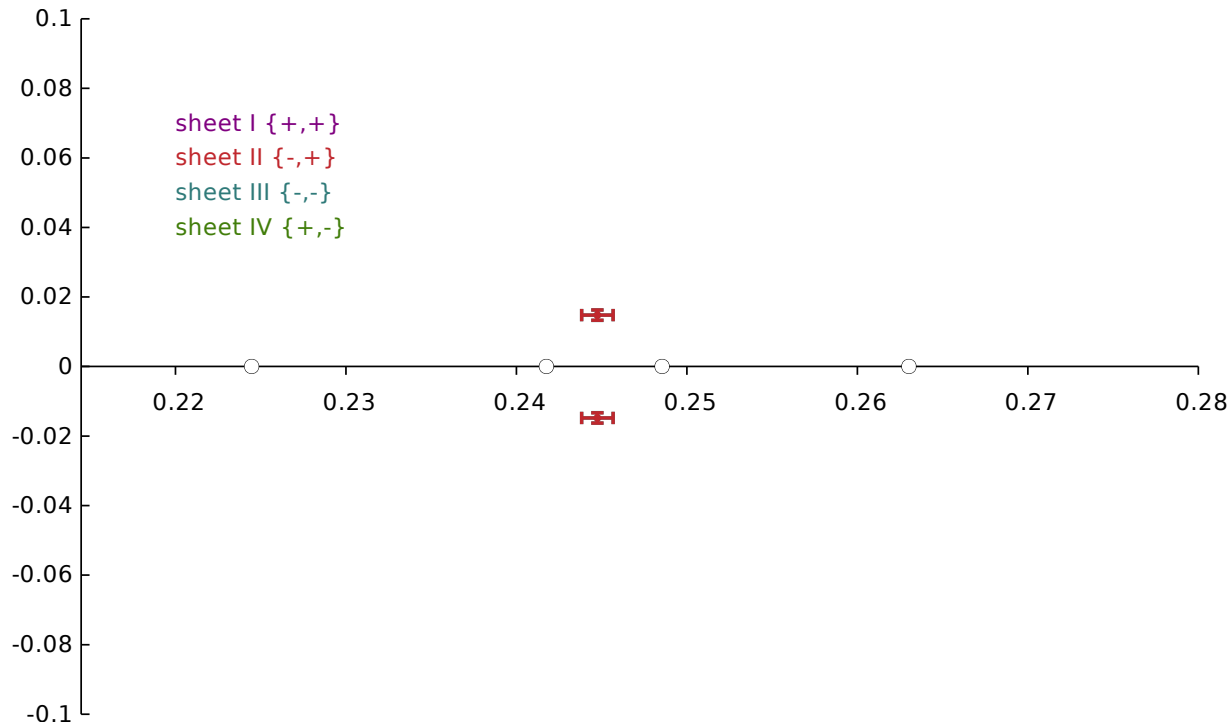

### parameter values

minimised with  $\text{chisq}/\text{nDoF} = 40.51 / (36 - 6) = 1.35$

|                                               |  |                        |  |      |       |       |       |       |       |
|-----------------------------------------------|--|------------------------|--|------|-------|-------|-------|-------|-------|
| JP1+_g_pi:omega/3^S_1_pole0_order0            |  | 0.099752 +/- 0.0055513 |  | 1.00 | -0.15 | -0.37 | -0.09 | 0.05  | -0.16 |
| JP1+_gamma_pi:omega/3^S_1 pi:omega/3^D_1_orde |  | -14.286 +/- 11.774     |  |      | 1.00  | 0.22  | 0.08  | -0.15 | -0.19 |
| JP1+_gamma_pi:omega/3^S_1 pi:omega/3^S_1_orde |  | -0.27643 +/- 0.19795   |  |      |       | 1.00  | 0.34  | 0.13  | -0.05 |
| JP1+_gamma_pi:omega/3^S_1 pi:phi/3^S_1_order0 |  | -0.0071941 +/- 0.82977 |  |      |       |       | 1.00  | -0.07 | 0.01  |
| JP1+_gamma_pi:phi/3^S_1 pi:phi/3^S_1_order0   |  | 1.0420 +/- 0.29662     |  |      |       |       |       | 1.00  | -0.28 |
| JP1+_m_pole0                                  |  | 0.24658 +/- 0.00066362 |  |      |       |       |       |       | 1.00  |

### pole singularities

pi:omega[-] pi:phi[+] upper half-plane

$\text{sqrt}(s)_{\text{pole}} = (0.24475 \pm 0.00092308)$   
 $+ (i/2)*(+0.014784 \pm 0.0014851) [-0.37]$

$s_{\text{pole}} = (0.059849 \pm 0.00045604)$   
 $+ i*(+0.0036184 \pm 0.00035865) [-0.36]$

|                          |                         |
|--------------------------|-------------------------|
| pi:omega                 | pi:phi                  |
| ===== =====              |                         |
| k_re= -0.0463 +/- 0.0010 | k_re= 0.0145 +/- 0.0011 |
| k_im= -0.0088 +/- 0.0009 | k_im= 0.0246 +/- 0.0017 |
| corr= [-0.41]            | corr= [-0.07]           |



| pi:omega/3^S_1(*)                                                   | pi:phi/3^S_1                                                         | pi:omega/3^D_1                                                       |
|---------------------------------------------------------------------|----------------------------------------------------------------------|----------------------------------------------------------------------|
| g = 0.0975 +/- 0.0053<br>arg(g)/pi= 0.0568 +/- 0.0224               | g = 0.0009 +/- 0.0165<br>arg(g)/pi= 0.2208 +/- 11.0295               | g = 0.0048 +/- 0.0039<br>arg(g)/pi= 0.7257 +/- 0.0332                |
| g_re= 0.0959 +/- 0.0054<br>g_im= 0.0173 +/- 0.0068<br>corr= [-0.14] | g_re= -0.0001 +/- 0.0110<br>g_im= 0.0002 +/- 0.0231<br>corr= [-1.00] | g_re= -0.0031 +/- 0.0026<br>g_im= 0.0036 +/- 0.0030<br>corr= [-0.97] |
| Br = 0.9795 +/- 0.0211                                              | Br = 0.0000 +/- 0.0000                                               | Br = 0.0023 +/- 0.0038                                               |

--

pi:omega[-] pi:phi[+] lower half-plane

$$\text{sqrt}(s)_{\text{pole}} = (0.24475 \pm 0.00092308) + (i/2)*(-0.014784 \pm 0.0014851) [0.37]$$

$$s_{\text{pole}} = (0.059849 \pm 0.00045604) + i*(-0.0036184 \pm 0.00035865) [0.36]$$

| pi:omega                                                            | pi:phi                                                              |
|---------------------------------------------------------------------|---------------------------------------------------------------------|
| k_re= 0.0463 +/- 0.0010<br>k_im= -0.0088 +/- 0.0009<br>corr= [0.41] | k_re= -0.0145 +/- 0.0011<br>k_im= 0.0246 +/- 0.0017<br>corr= [0.07] |

| pi:omega/3^S_1(*)                                                   | pi:phi/3^S_1                                                         | pi:omega/3^D_1                                                       |
|---------------------------------------------------------------------|----------------------------------------------------------------------|----------------------------------------------------------------------|
| g = 0.0975 +/- 0.0053<br>arg(g)/pi= -0.0568 +/- 0.0224              | g = 0.0009 +/- 0.0165<br>arg(g)/pi= -0.2208 +/- 11.0295              | g = 0.0048 +/- 0.0039<br>arg(g)/pi= -0.7257 +/- 0.0332               |
| g_re= 0.0959 +/- 0.0054<br>g_im= -0.0173 +/- 0.0068<br>corr= [0.14] | g_re= -0.0001 +/- 0.0110<br>g_im= -0.0002 +/- 0.0231<br>corr= [1.00] | g_re= -0.0031 +/- 0.0026<br>g_im= -0.0036 +/- 0.0030<br>corr= [0.97] |
| Br = 0.9795 +/- 0.0211                                              | Br = 0.0000 +/- 0.0000                                               | Br = 0.0023 +/- 0.0038                                               |

--

pi:omega[-] pi:phi[-] upper half-plane

$$\text{sqrt}(s)_{\text{pole}} = (0.24475 \pm 0.0009231) + (i/2)*(+0.014785 \pm 0.0014946) [-0.37]$$

$$s_{\text{pole}} = (0.05985 \pm 0.00045611) + i*(+0.0036186 \pm 0.00036092) [-0.36]$$

| pi:omega                                                              | pi:phi                                                                |
|-----------------------------------------------------------------------|-----------------------------------------------------------------------|
| k_re= -0.0463 +/- 0.0010<br>k_im= -0.0088 +/- 0.0009<br>corr= [-0.41] | k_re= -0.0145 +/- 0.0011<br>k_im= -0.0246 +/- 0.0017<br>corr= [-0.06] |

| pi:omega/3^S_1(*)                                                   | pi:phi/3^S_1                                                         | pi:omega/3^D_1                                                       |
|---------------------------------------------------------------------|----------------------------------------------------------------------|----------------------------------------------------------------------|
| g = 0.0975 +/- 0.0053<br>arg(g)/pi= 0.0567 +/- 0.0221               | g = 0.0014 +/- 0.0248<br>arg(g)/pi= 0.1330 +/- 11.0344               | g = 0.0048 +/- 0.0039<br>arg(g)/pi= 0.7256 +/- 0.0330                |
| g_re= 0.0959 +/- 0.0054<br>g_im= 0.0173 +/- 0.0067<br>corr= [-0.13] | g_re= -0.0001 +/- 0.0066<br>g_im= 0.0003 +/- 0.0381<br>corr= [-1.00] | g_re= -0.0031 +/- 0.0026<br>g_im= 0.0036 +/- 0.0030<br>corr= [-0.97] |



# 1 Successful Parameterizations

```

Br = 0.9795 +/- 0.0223 | Br = 0.0000 +/- 0.0000 | Br = 0.0023 +/- 0.0038 |

--
pi:omega[-] pi:phi[-] lower half-plane

sqrt(s)_pole = (0.24475 +/- 0.0009231)
               + (i/2)*(-0.014785 +/- 0.0014946) [ 0.37]

s_pole = (0.05985 +/- 0.00045611)
         + i*(-0.0036186 +/- 0.00036092) [ 0.36]

=====
pi:omega | pi:phi |
=====
k_re= 0.0463 +/- 0.0010 | k_re= 0.0145 +/- 0.0011 |
k_im= -0.0088 +/- 0.0009 | k_im= -0.0246 +/- 0.0017 |
corr= [ 0.41] | corr= [ 0.06] |

=====
pi:omega/3^S_1(*) | pi:phi/3^S_1 | pi:omega/3^D_1 |
=====
|g|= 0.0975 +/- 0.0053 | |g|= 0.0014 +/- 0.0248 | |g|= 0.0048 +/- 0.0039 |
arg(g)/pi= -0.0567 +/- 0.0221 | arg(g)/pi= -0.1330 +/- 11.0344 | arg(g)/pi= -0.7256 +/- 0.0330 |
-----
g_re= 0.0959 +/- 0.0054 | g_re= -0.0001 +/- 0.0066 | g_re= -0.0031 +/- 0.0026 |
g_im= -0.0173 +/- 0.0067 | g_im= -0.0003 +/- 0.0381 | g_im= -0.0036 +/- 0.0030 |
corr= [ 0.13] | corr= [ 1.00] | corr= [ 0.97] |
-----
Br = 0.9795 +/- 0.0223 | Br = 0.0000 +/- 0.0000 | Br = 0.0023 +/- 0.0038 |

```



## 1.9 coupled\_po\_pp.3s1\_3d1.pole+G0\_3s1\_3sd1\_3S1\_3sS1.gorder0\_3s1.pole0\_sub

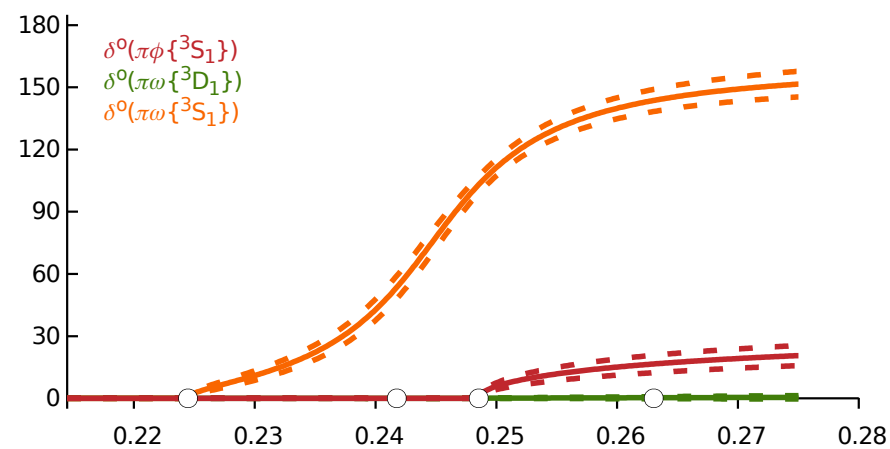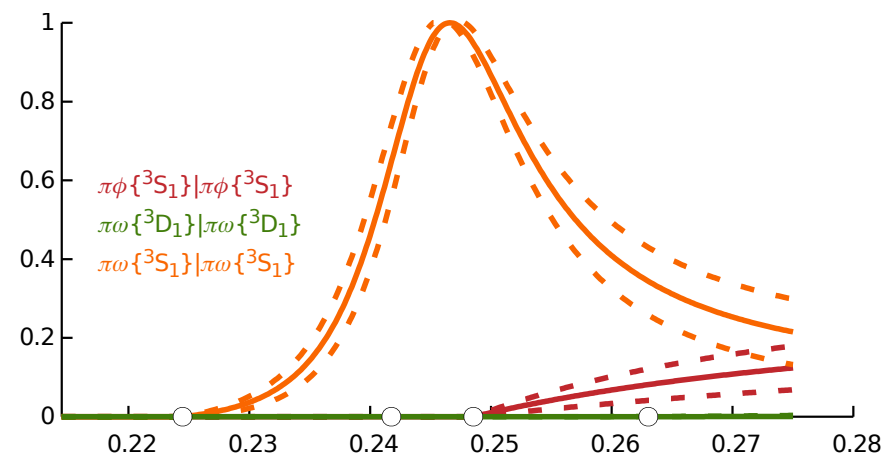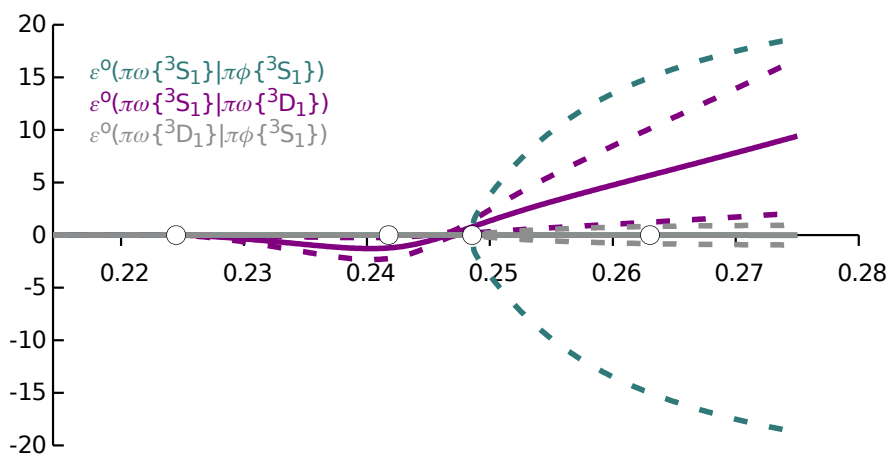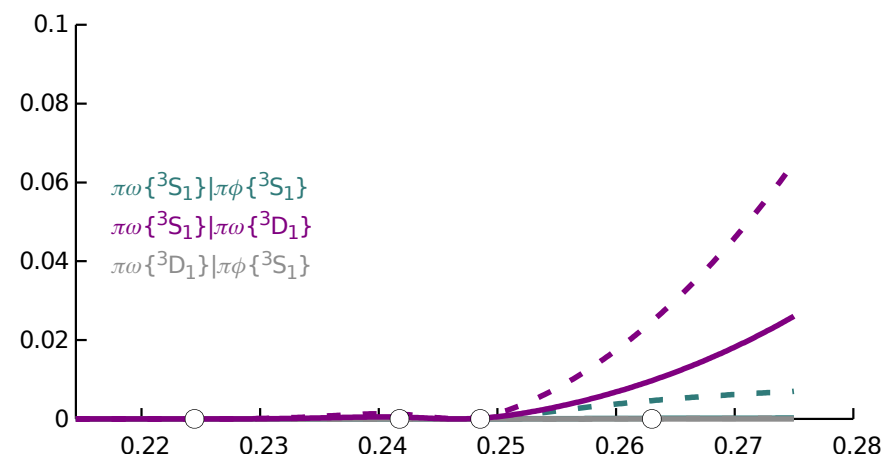



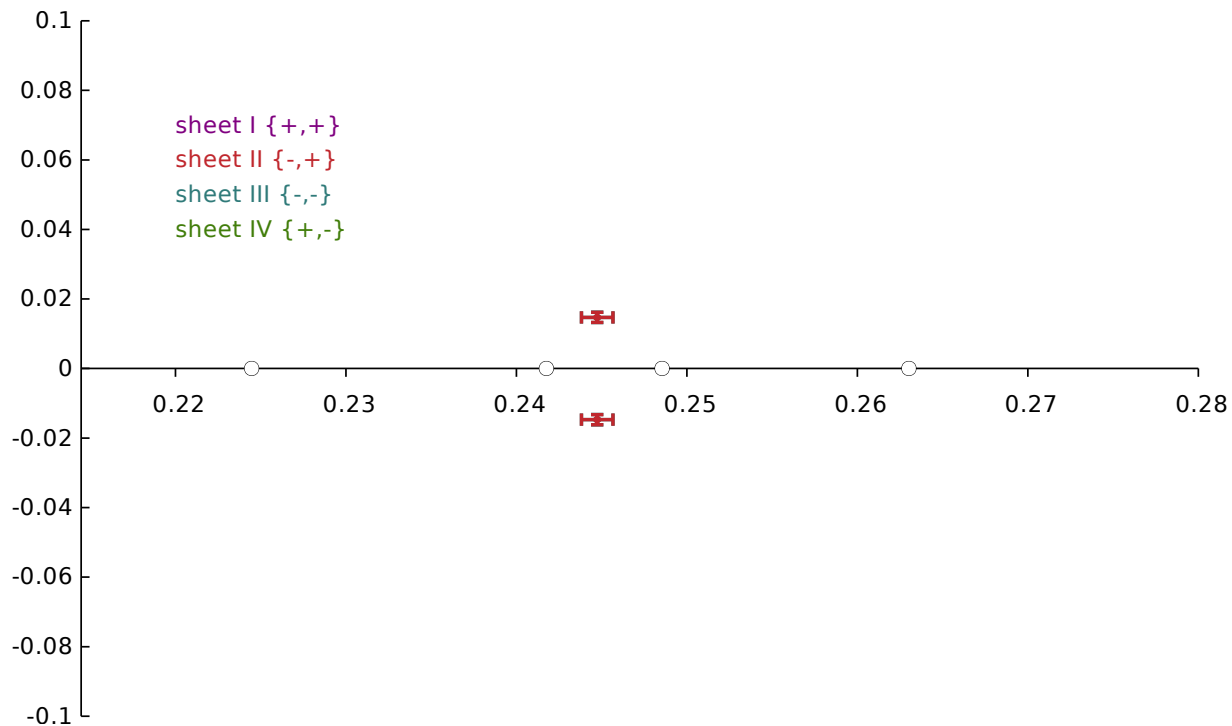

### parameter values

minimised with  $\text{chisq}/\text{nDoF} = 40.52 / (36 - 6) = 1.35$

|                                               |  |                        |  |      |       |       |       |       |       |
|-----------------------------------------------|--|------------------------|--|------|-------|-------|-------|-------|-------|
| JP1+_g_pi:omega/3^S_1_pole0_order0            |  | 0.095708 +/- 0.0049913 |  | 1.00 | -0.15 | -0.40 | -0.17 | 0.03  | -0.15 |
| JP1+_gamma_pi:omega/3^S_1 pi:omega/3^D_1_orde |  | -13.591 +/- 11.01      |  |      | 1.00  | 0.23  | 0.09  | -0.17 | -0.19 |
| JP1+_gamma_pi:omega/3^S_1 pi:omega/3^S_1_orde |  | -0.25813 +/- 0.17079   |  |      |       | 1.00  | 0.27  | 0.14  | -0.05 |
| JP1+_gamma_pi:omega/3^S_1 pi:phi/3^S_1_order0 |  | 0.00043758 +/- 0.76398 |  |      |       |       | 1.00  | -0.09 | 0.04  |
| JP1+_gamma_pi:phi/3^S_1 pi:phi/3^S_1_order0   |  | 0.95708 +/- 0.24737    |  |      |       |       |       | 1.00  | -0.18 |
| JP1+_m_pole0                                  |  | 0.24661 +/- 0.00064102 |  |      |       |       |       |       | 1.00  |

### pole singularities

pi:omega[+] pi:phi[-] upper half-plane

$\text{sqrt}(s)_{\text{pole}} = (0.19004 \pm 0.023799)$   
 $+ (i/2)*(+2.9847e-16 \pm 2.1628e-13) [0.00]$

$s_{\text{pole}} = (0.036115 \pm 0.0090388)$   
 $+ i*(+5.706e-17 \pm 4.1045e-14) [0.00]$

| pi:omega                | pi:phi                   |
|-------------------------|--------------------------|
| ===== =====             |                          |
| k_re= 0.0000 +/- 0.0000 | k_re= -0.0000 +/- 0.0000 |
| k_im= 0.0532 +/- 0.0151 | k_im= -0.0652 +/- 0.0073 |
| corr= [ 0.00]           | corr= [ 0.00]            |



# 1 Successful Parameterizations

| pi:omega/3^S_1                | pi:phi/3^S_1(*)              | pi:omega/3^D_1                 |
|-------------------------------|------------------------------|--------------------------------|
| =====                         | =====                        | =====                          |
| g = 0.0050 +/- 0.0893         | g = 0.1837 +/- 0.0024        | g = 0.0002 +/- 0.0039          |
| arg(g)/pi= 0.0180 +/- 11.1612 | arg(g)/pi= 0.5000 +/- 0.0000 | arg(g)/pi= -0.0182 +/- 11.1468 |
| -----                         | -----                        | -----                          |
| g_re= 0.0000 +/- 0.0000       | g_re= 0.0000 +/- 0.0000      | g_re= 0.0000 +/- 0.0000        |
| g_im= 0.0001 +/- 0.1437       | g_im= 0.1837 +/- 0.0024      | g_im= -0.0000 +/- 0.0062       |
| corr= [-1.00]                 | corr= [-1.00]                | corr= [-0.77]                  |
| -----                         | -----                        | -----                          |
| Br = 0.0000 +/- 0.0000        | Br = 0.0000 +/- 0.0000       | Br = 0.0000 +/- 0.0000         |

--

pi:omega[-] pi:phi[+] upper half-plane

sqrt(s)\_pole = (0.24474 +/- 0.00091894)  
+ (i/2)\*(+0.014717 +/- 0.0014624) [-0.39]

s\_pole = (0.059842 +/- 0.00045409)  
+ i\*(+0.0036017 +/- 0.00035286) [-0.38]

| pi:omega                 | pi:phi                  |
|--------------------------|-------------------------|
| =====                    | =====                   |
| k_re= -0.0463 +/- 0.0010 | k_re= 0.0145 +/- 0.0011 |
| k_im= -0.0087 +/- 0.0009 | k_im= 0.0246 +/- 0.0017 |
| corr= [-0.43]            | corr= [-0.07]           |

| pi:omega/3^S_1(*)            | pi:phi/3^S_1                  | pi:omega/3^D_1               |
|------------------------------|-------------------------------|------------------------------|
| =====                        | =====                         | =====                        |
| g = 0.0971 +/- 0.0052        | g = 0.0010 +/- 0.0180         | g = 0.0049 +/- 0.0040        |
| arg(g)/pi= 0.0587 +/- 0.0224 | arg(g)/pi= 0.1229 +/- 11.1696 | arg(g)/pi= 0.7288 +/- 0.0349 |
| -----                        | -----                         | -----                        |
| g_re= 0.0955 +/- 0.0053      | g_re= 0.0000 +/- 0.0121       | g_re= -0.0032 +/- 0.0027     |
| g_im= 0.0178 +/- 0.0067      | g_im= -0.0000 +/- 0.0263      | g_im= 0.0037 +/- 0.0030      |
| corr= [-0.14]                | corr= [-1.00]                 | corr= [-0.96]                |
| -----                        | -----                         | -----                        |
| Br = 0.9768 +/- 0.0210       | Br = 0.0000 +/- 0.0000        | Br = 0.0025 +/- 0.0040       |

--

pi:omega[-] pi:phi[+] lower half-plane

sqrt(s)\_pole = (0.24474 +/- 0.00091894)  
+ (i/2)\*(-0.014717 +/- 0.0014624) [ 0.39]

s\_pole = (0.059842 +/- 0.00045409)  
+ i\*(-0.0036017 +/- 0.00035286) [ 0.38]

| pi:omega                 | pi:phi                   |
|--------------------------|--------------------------|
| =====                    | =====                    |
| k_re= 0.0463 +/- 0.0010  | k_re= -0.0145 +/- 0.0011 |
| k_im= -0.0087 +/- 0.0009 | k_im= 0.0246 +/- 0.0017  |
| corr= [ 0.43]            | corr= [ 0.07]            |

| pi:omega/3^S_1(*)             | pi:phi/3^S_1                   | pi:omega/3^D_1                |
|-------------------------------|--------------------------------|-------------------------------|
| =====                         | =====                          | =====                         |
| g = 0.0971 +/- 0.0052         | g = 0.0010 +/- 0.0180          | g = 0.0049 +/- 0.0040         |
| arg(g)/pi= -0.0587 +/- 0.0224 | arg(g)/pi= -0.1229 +/- 11.1696 | arg(g)/pi= -0.7288 +/- 0.0349 |
| -----                         | -----                          | -----                         |
| g_re= 0.0955 +/- 0.0053       | g_re= 0.0000 +/- 0.0121        | g_re= -0.0032 +/- 0.0027      |
| g_im= -0.0178 +/- 0.0067      | g_im= 0.0000 +/- 0.0263        | g_im= -0.0037 +/- 0.0030      |
| corr= [ 0.14]                 | corr= [ 1.00]                  | corr= [ 0.96]                 |
| -----                         | -----                          | -----                         |



## 1 Successful Parameterizations

```

Br = 0.9768 +/- 0.0210 | Br = 0.0000 +/- 0.0000 | Br = 0.0025 +/- 0.0040 |

--
pi:omega[-] pi:phi[-] lower half-plane

sqrt(s)_pole = (0.19018 +/- 0.023947)
+ (i/2)*(-8.0609e-16 +/- 5.8586e-13) [ 0.00]

s_pole = (0.036168 +/- 0.0091031)
+ i*(-1.542e-16 +/- 1.1178e-13) [ 0.00]

=====
pi:omega | pi:phi |
=====
k_re= 0.0000 +/- 0.0000 | k_re= 0.0000 +/- 0.0000 |
k_im= -0.0531 +/- 0.0152 | k_im= -0.0651 +/- 0.0074 |
corr= [ 0.00] | corr= [ 0.00] |

=====
pi:omega/3^S_1 | pi:phi/3^S_1(*) | pi:omega/3^D_1 |
=====
|g|= 0.0058 +/- 0.1022 | |g|= 0.1835 +/- 0.0058 | |g|= 0.0007 +/- 0.0130 |
arg(g)/pi= 0.0180 +/- 11.1613 | arg(g)/pi= 0.5000 +/- 0.0000 | arg(g)/pi= 0.0181 +/- 11.1573 |
-----
g_re= 0.0000 +/- 0.0000 | g_re= 0.0000 +/- 0.0000 | g_re= 0.0000 +/- 0.0000 |
g_im= 0.0001 +/- 0.1651 | g_im= 0.1835 +/- 0.0058 | g_im= 0.0000 +/- 0.0211 |
corr= [-1.00] | corr= [-1.00] | corr= [-0.88] |
-----
Br = 0.0000 +/- 0.0000 | Br = 0.0000 +/- 0.0000 | Br = 0.0000 +/- 0.0000 |

--
pi:omega[-] pi:phi[-] upper half-plane

sqrt(s)_pole = (0.24474 +/- 0.00092395)
+ (i/2)*(+0.014717 +/- 0.0014822) [-0.39]

s_pole = (0.059843 +/- 0.00045663)
+ i*(+0.0036019 +/- 0.00035765) [-0.38]

=====
pi:omega | pi:phi |
=====
k_re= -0.0463 +/- 0.0010 | k_re= -0.0145 +/- 0.0011 |
k_im= -0.0087 +/- 0.0009 | k_im= -0.0246 +/- 0.0017 |
corr= [-0.43] | corr= [-0.06] |

=====
pi:omega/3^S_1(*) | pi:phi/3^S_1 | pi:omega/3^D_1 |
=====
|g|= 0.0971 +/- 0.0053 | |g|= 0.0015 +/- 0.0272 | |g|= 0.0049 +/- 0.0040 |
arg(g)/pi= 0.0586 +/- 0.0224 | arg(g)/pi= 0.0257 +/- 11.1631 | arg(g)/pi= 0.7287 +/- 0.0351 |
-----
g_re= 0.0955 +/- 0.0054 | g_re= 0.0000 +/- 0.0060 | g_re= -0.0032 +/- 0.0027 |
g_im= 0.0178 +/- 0.0068 | g_im= -0.0000 +/- 0.0433 | g_im= 0.0037 +/- 0.0030 |
corr= [-0.12] | corr= [-1.00] | corr= [-0.96] |
-----
Br = 0.9766 +/- 0.0230 | Br = 0.0000 +/- 0.0000 | Br = 0.0025 +/- 0.0040 |

--
pi:omega[-] pi:phi[-] lower half-plane

sqrt(s)_pole = (0.24474 +/- 0.00092395)
+ (i/2)*(-0.014717 +/- 0.0014822) [ 0.39]

s_pole = (0.059843 +/- 0.00045663)
+ i*(-0.0036019 +/- 0.00035765) [ 0.38]

```



# 1 Successful Parameterizations

| pi:omega |                    | pi:phi |                    |
|----------|--------------------|--------|--------------------|
| =====    |                    | =====  |                    |
| k_re=    | 0.0463 +/- 0.0010  | k_re=  | 0.0145 +/- 0.0011  |
| k_im=    | -0.0087 +/- 0.0009 | k_im=  | -0.0246 +/- 0.0017 |
| corr=    | [ 0.43]            | corr=  | [ 0.06]            |

  

| pi:omega/3^S_1(*) |                    | pi:phi/3^S_1 |                     | pi:omega/3^D_1 |                    |
|-------------------|--------------------|--------------|---------------------|----------------|--------------------|
| =====             |                    | =====        |                     | =====          |                    |
| g =               | 0.0971 +/- 0.0053  | g =          | 0.0015 +/- 0.0272   | g =            | 0.0049 +/- 0.0040  |
| arg(g)/pi=        | -0.0586 +/- 0.0224 | arg(g)/pi=   | -0.0257 +/- 11.1631 | arg(g)/pi=     | -0.7287 +/- 0.0351 |
| -----             |                    | -----        |                     | -----          |                    |
| g_re=             | 0.0955 +/- 0.0054  | g_re=        | 0.0000 +/- 0.0060   | g_re=          | -0.0032 +/- 0.0027 |
| g_im=             | -0.0178 +/- 0.0068 | g_im=        | 0.0000 +/- 0.0433   | g_im=          | -0.0037 +/- 0.0030 |
| corr=             | [ 0.12]            | corr=        | [ 1.00]             | corr=          | [ 0.96]            |
| -----             |                    | -----        |                     | -----          |                    |
| Br =              | 0.9766 +/- 0.0230  | Br =         | 0.0000 +/- 0.0000   | Br =           | 0.0025 +/- 0.0040  |



## 1.10 coupled\_po\_pp.3s1\_3d1.pole+G0\_3s1\_3sd1\_3S1\_3sS1.gorder0\_3s1.threshold\_sub

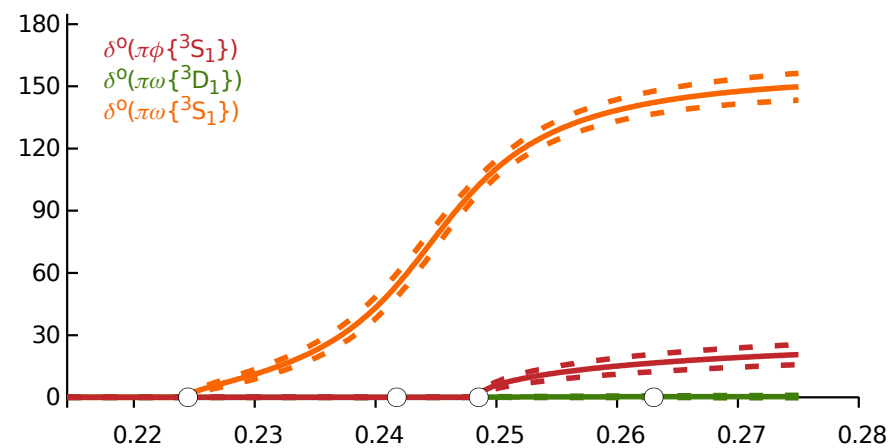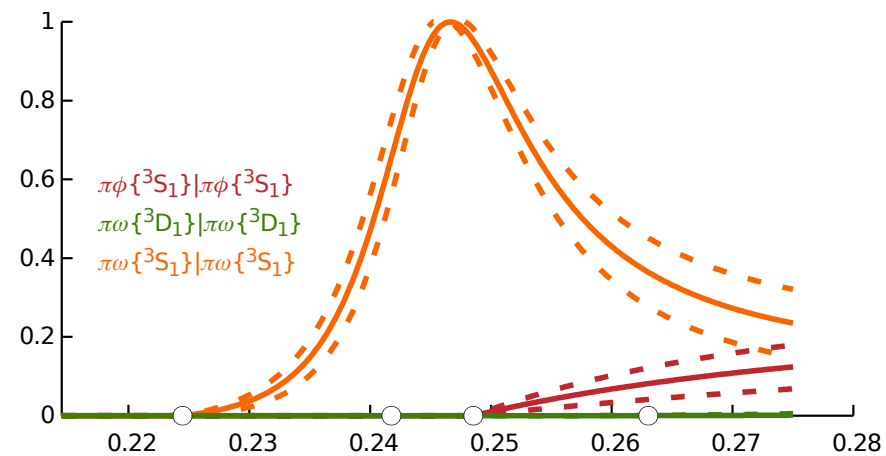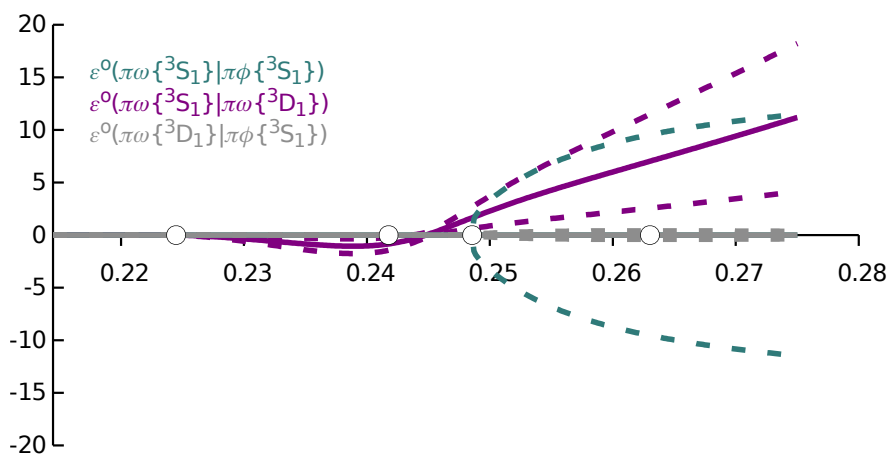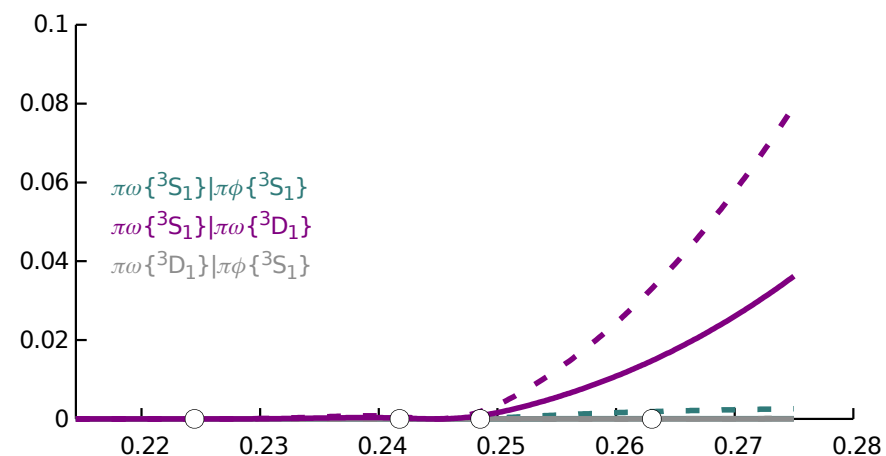



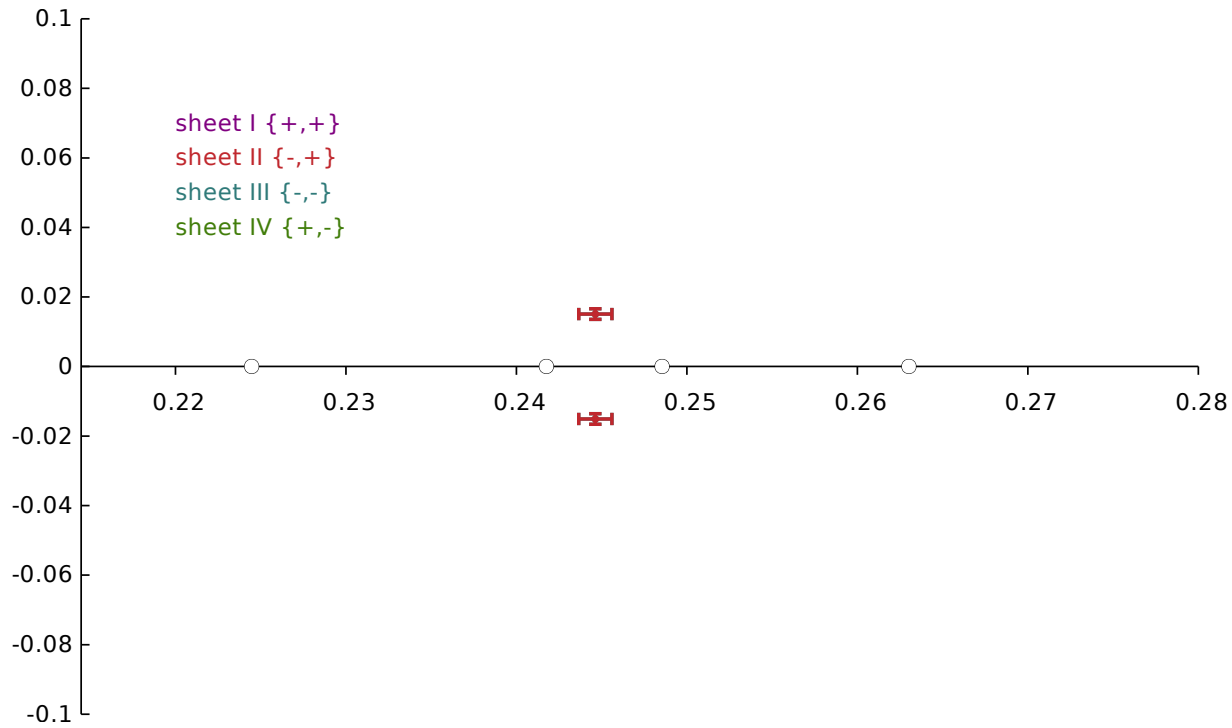

### parameter values

minimised with  $\text{chisq}/\text{nDoF} = 39.62 / (36 - 6) = 1.32$

|                                               |  |                         |  |      |       |       |       |       |       |
|-----------------------------------------------|--|-------------------------|--|------|-------|-------|-------|-------|-------|
| JP1+_g_pi:omega/3^S_1_pole0_order0            |  | 0.094523 +/- 0.0046975  |  | 1.00 | -0.19 | -0.15 | -0.03 | 0.11  | -0.47 |
| JP1+_gamma_pi:omega/3^S_1 pi:omega/3^D_1_orde |  | -14.947 +/- 9.8736      |  |      | 1.00  | 0.22  | 0.01  | -0.11 | -0.14 |
| JP1+_gamma_pi:omega/3^S_1 pi:omega/3^S_1_orde |  | -0.27063 +/- 0.16241    |  |      |       | 1.00  | 0.05  | 0.16  | 0.07  |
| JP1+_gamma_pi:omega/3^S_1 pi:phi/3^S_1_order0 |  | -3.5328e-05 +/- 0.47439 |  |      |       |       | 1.00  | -0.01 | 0.00  |
| JP1+_gamma_pi:phi/3^S_1 pi:phi/3^S_1_order0   |  | 1.0637 +/- 0.31053      |  |      |       |       |       | 1.00  | -0.27 |
| JP1+_m_pole0                                  |  | 0.24478 +/- 0.00068266  |  |      |       |       |       |       | 1.00  |

### pole singularities

pi:omega[+] pi:phi[-] upper half-plane

$\sqrt{s}_{\text{pole}} = (0.19007 \pm 0.023828)$   
 $+ (i/2)(+5.3742e-14 \pm 2.7234e-11) [0.00]$

$s_{\text{pole}} = (0.036127 \pm 0.0090517)$   
 $+ i*(+1.0235e-14 \pm 5.186e-12) [0.00]$

| pi:omega                | pi:phi                   |
|-------------------------|--------------------------|
| ===== =====             |                          |
| k_re= 0.0000 +/- 0.0000 | k_re= -0.0000 +/- 0.0000 |
| k_im= 0.0532 +/- 0.0151 | k_im= -0.0652 +/- 0.0073 |
| corr= [ 0.00]           | corr= [ 0.00]            |



# 1 Successful Parameterizations

| pi:omega/3^S_1                 | pi:phi/3^S_1(*)              | pi:omega/3^D_1                |
|--------------------------------|------------------------------|-------------------------------|
| =====                          | =====                        | =====                         |
| g = 0.0028 +/- 0.0499          | g = 0.1837 +/- 0.0019        | g = 0.0002 +/- 0.0032         |
| arg(g)/pi= -0.0180 +/- 11.1615 | arg(g)/pi= 0.5000 +/- 0.0000 | arg(g)/pi= 0.0180 +/- 11.1557 |
| -----                          | -----                        | -----                         |
| g_re= 0.0000 +/- 0.0000        | g_re= 0.0000 +/- 0.0000      | g_re= 0.0000 +/- 0.0000       |
| g_im= -0.0000 +/- 0.0806       | g_im= 0.1837 +/- 0.0019      | g_im= 0.0000 +/- 0.0052       |
| corr= [-1.00]                  | corr= [-1.00]                | corr= [-0.80]                 |
| -----                          | -----                        | -----                         |
| Br = 0.0000 +/- 0.0000         | Br = 0.0000 +/- 0.0000       | Br = 0.0000 +/- 0.0000        |

--

pi:omega[-] pi:phi[+] upper half-plane

sqrt(s)\_pole = (0.27244 +/- 0.016733)  
+ (i/2)\*(+0.21136 +/- 0.085173) [ 0.90]

s\_pole = (0.06305 +/- 0.0040042)  
+ i\*(+0.057584 +/- 0.026449) [-0.14]

| pi:omega                 | pi:phi                  |
|--------------------------|-------------------------|
| =====                    | =====                   |
| k_re= -0.0892 +/- 0.0170 | k_re= 0.0770 +/- 0.0190 |
| k_im= -0.0765 +/- 0.0227 | k_im= 0.0838 +/- 0.0222 |
| corr= [ 0.95]            | corr= [ 0.95]           |

| pi:omega/3^S_1(*)             | pi:phi/3^S_1                   | pi:omega/3^D_1               |
|-------------------------------|--------------------------------|------------------------------|
| =====                         | =====                          | =====                        |
| g = 0.1434 +/- 0.0184         | g = 0.0017 +/- 0.0305          | g = 0.1340 +/- 0.0184        |
| arg(g)/pi= -0.4370 +/- 0.0479 | arg(g)/pi= -0.3588 +/- 11.1614 | arg(g)/pi= 0.5051 +/- 0.0435 |
| -----                         | -----                          | -----                        |
| g_re= 0.0282 +/- 0.0244       | g_re= 0.0000 +/- 0.0456        | g_re= -0.0021 +/- 0.0186     |
| g_im= -0.1406 +/- 0.0145      | g_im= 0.0000 +/- 0.0186        | g_im= 0.1340 +/- 0.0182      |
| corr= [-0.82]                 | corr= [ 1.00]                  | corr= [-0.92]                |
| -----                         | -----                          | -----                        |
| Br = 0.1915 +/- 0.0513        | Br = 0.0000 +/- 0.0010         | Br = 0.1672 +/- 0.0407       |

--

pi:omega[-] pi:phi[+] upper half-plane

sqrt(s)\_pole = (0.24463 +/- 0.00096969)  
+ (i/2)\*(+0.015075 +/- 0.0015205) [-0.41]

s\_pole = (0.059789 +/- 0.00047927)  
+ i\*(+0.0036878 +/- 0.0003662) [-0.40]

| pi:omega                 | pi:phi                  |
|--------------------------|-------------------------|
| =====                    | =====                   |
| k_re= -0.0462 +/- 0.0011 | k_re= 0.0146 +/- 0.0011 |
| k_im= -0.0089 +/- 0.0010 | k_im= 0.0249 +/- 0.0018 |
| corr= [-0.45]            | corr= [-0.08]           |

| pi:omega/3^S_1(*)            | pi:phi/3^S_1                  | pi:omega/3^D_1               |
|------------------------------|-------------------------------|------------------------------|
| =====                        | =====                         | =====                        |
| g = 0.0981 +/- 0.0053        | g = 0.0006 +/- 0.0101         | g = 0.0054 +/- 0.0036        |
| arg(g)/pi= 0.0619 +/- 0.0223 | arg(g)/pi= 0.0848 +/- 11.1608 | arg(g)/pi= 0.6598 +/- 0.0359 |
| -----                        | -----                         | -----                        |
| g_re= 0.0963 +/- 0.0054      | g_re= -0.0000 +/- 0.0033      | g_re= -0.0026 +/- 0.0018     |
| g_im= 0.0190 +/- 0.0068      | g_im= 0.0000 +/- 0.0160       | g_im= 0.0047 +/- 0.0031      |
| corr= [-0.12]                | corr= [-1.00]                 | corr= [-0.93]                |
| -----                        | -----                         | -----                        |



## 1 Successful Parameterizations

```
Br = 0.9719 +/- 0.0221 | Br = 0.0000 +/- 0.0000 | Br = 0.0029 +/- 0.0038 |

--
pi:omega[-] pi:phi[+] lower half-plane

sqrt(s)_pole = (0.27244 +/- 0.016733)
+ (i/2)*(-0.21136 +/- 0.085173) [-0.90]

s_pole = (0.06305 +/- 0.0040042)
+ i*(-0.057584 +/- 0.026449) [ 0.14]

=====
pi:omega | pi:phi |
=====
k_re= 0.0892 +/- 0.0170 | k_re= -0.0770 +/- 0.0190 |
k_im= -0.0765 +/- 0.0227 | k_im= 0.0838 +/- 0.0222 |
corr= [-0.95] | corr= [-0.95] |

=====
pi:omega/3^S_1(*) | pi:phi/3^S_1 | pi:omega/3^D_1 |
=====
|g|= 0.1434 +/- 0.0184 | |g|= 0.0017 +/- 0.0305 | |g|= 0.1340 +/- 0.0184 |
arg(g)/pi= 0.4370 +/- 0.0479 | arg(g)/pi= 0.3588 +/- 11.1614 | arg(g)/pi= -0.5051 +/- 0.0435 |
-----
g_re= 0.0282 +/- 0.0244 | g_re= 0.0000 +/- 0.0456 | g_re= -0.0021 +/- 0.0186 |
g_im= 0.1406 +/- 0.0145 | g_im= -0.0000 +/- 0.0186 | g_im= -0.1340 +/- 0.0182 |
corr= [ 0.82] | corr= [-1.00] | corr= [ 0.92] |
-----
Br = 0.1915 +/- 0.0513 | Br = 0.0000 +/- 0.0010 | Br = 0.1672 +/- 0.0407 |

--
pi:omega[-] pi:phi[+] lower half-plane

sqrt(s)_pole = (0.24463 +/- 0.00096969)
+ (i/2)*(-0.015075 +/- 0.0015205) [ 0.41]

s_pole = (0.059789 +/- 0.00047927)
+ i*(-0.0036878 +/- 0.0003662) [ 0.40]

=====
pi:omega | pi:phi |
=====
k_re= 0.0462 +/- 0.0011 | k_re= -0.0146 +/- 0.0011 |
k_im= -0.0089 +/- 0.0010 | k_im= 0.0249 +/- 0.0018 |
corr= [ 0.45] | corr= [ 0.08] |

=====
pi:omega/3^S_1(*) | pi:phi/3^S_1 | pi:omega/3^D_1 |
=====
|g|= 0.0981 +/- 0.0053 | |g|= 0.0006 +/- 0.0101 | |g|= 0.0054 +/- 0.0036 |
arg(g)/pi= -0.0619 +/- 0.0223 | arg(g)/pi= -0.0848 +/- 11.1608 | arg(g)/pi= -0.6598 +/- 0.0359 |
-----
g_re= 0.0963 +/- 0.0054 | g_re= -0.0000 +/- 0.0033 | g_re= -0.0026 +/- 0.0018 |
g_im= -0.0190 +/- 0.0068 | g_im= -0.0000 +/- 0.0160 | g_im= -0.0047 +/- 0.0031 |
corr= [ 0.12] | corr= [ 1.00] | corr= [ 0.93] |
-----
Br = 0.9719 +/- 0.0221 | Br = 0.0000 +/- 0.0000 | Br = 0.0029 +/- 0.0038 |

--
pi:omega[-] pi:phi[-] upper half-plane

sqrt(s)_pole = (0.27244 +/- 0.01674)
+ (i/2)*(+0.21138 +/- 0.085165) [ 0.90]

s_pole = (0.06305 +/- 0.0040012)
+ i*(+0.057592 +/- 0.02645) [-0.14]
```



```

pi:omega | pi:phi |
=====|=====|
k_re= -0.0893 +/- 0.0170 | k_re= -0.0770 +/- 0.0190 |
k_im= -0.0765 +/- 0.0227 | k_im= -0.0838 +/- 0.0222 |
corr= [ 0.95] | corr= [ 0.96] |

pi:omega/3^S_1(*) | pi:phi/3^S_1 | pi:omega/3^D_1 |
=====|=====|=====|
|g|= 0.1434 +/- 0.0184 | |g|= 0.0020 +/- 0.0344 | |g|= 0.1340 +/- 0.0184 |
arg(g)/pi= -0.4370 +/- 0.0479 | arg(g)/pi= 0.2343 +/- 11.1645 | arg(g)/pi= 0.5051 +/- 0.0435 |
-----|-----|-----|
g_re= 0.0282 +/- 0.0244 | g_re= 0.0000 +/- 0.0396 | g_re= -0.0021 +/- 0.0186 |
g_im= -0.1406 +/- 0.0145 | g_im= -0.0000 +/- 0.0390 | g_im= 0.1340 +/- 0.0182 |
corr= [-0.82] | corr= [-1.00] | corr= [-0.92] |
-----|-----|-----|
Br = 0.1915 +/- 0.0513 | Br = 0.0000 +/- 0.0013 | Br = 0.1673 +/- 0.0407 |

--
pi:omega[-] pi:phi[-] upper half-plane

sqrt(s)_pole = (0.19011 +/- 0.023803)
+ (i/2)*(+1.7468e-16 +/- 2.5299e-13) [ 0.00]

s_pole = (0.036143 +/- 0.0090446)
+ i*(+3.3768e-17 +/- 4.8027e-14) [ 0.00]

pi:omega | pi:phi |
=====|=====|
k_re= -0.0000 +/- 0.0000 | k_re= -0.0000 +/- 0.0000 |
k_im= -0.0532 +/- 0.0151 | k_im= -0.0652 +/- 0.0073 |
corr= [ 0.00] | corr= [ 0.00] |

pi:omega/3^S_1 | pi:phi/3^S_1(*) | pi:omega/3^D_1 |
=====|=====|=====|
|g|= 0.0032 +/- 0.0567 | |g|= 0.1836 +/- 0.0025 | |g|= 0.0004 +/- 0.0071 |
arg(g)/pi= -0.0180 +/- 11.1616 | arg(g)/pi= 0.5000 +/- 0.0000 | arg(g)/pi= -0.0180 +/- 11.1591 |
-----|-----|-----|
g_re= 0.0000 +/- 0.0000 | g_re= 0.0000 +/- 0.0000 | g_re= 0.0000 +/- 0.0000 |
g_im= -0.0000 +/- 0.0917 | g_im= 0.1836 +/- 0.0025 | g_im= -0.0000 +/- 0.0114 |
corr= [-1.00] | corr= [-1.00] | corr= [-0.92] |
-----|-----|-----|
Br = 0.0000 +/- 0.0000 | Br = 0.0000 +/- 0.0000 | Br = 0.0000 +/- 0.0000 |

--
pi:omega[-] pi:phi[-] lower half-plane

sqrt(s)_pole = (0.27244 +/- 0.01674)
+ (i/2)*(-0.21138 +/- 0.085165) [-0.90]

s_pole = (0.06305 +/- 0.0040012)
+ i*(-0.057592 +/- 0.02645) [ 0.14]

pi:omega | pi:phi |
=====|=====|
k_re= 0.0893 +/- 0.0170 | k_re= 0.0770 +/- 0.0190 |
k_im= -0.0765 +/- 0.0227 | k_im= -0.0838 +/- 0.0222 |
corr= [-0.95] | corr= [-0.96] |

pi:omega/3^S_1(*) | pi:phi/3^S_1 | pi:omega/3^D_1 |
=====|=====|=====|
|g|= 0.1434 +/- 0.0184 | |g|= 0.0020 +/- 0.0344 | |g|= 0.1340 +/- 0.0184 |
arg(g)/pi= 0.4370 +/- 0.0479 | arg(g)/pi= -0.2343 +/- 11.1645 | arg(g)/pi= -0.5051 +/- 0.0435 |

```



# 1 Successful Parameterizations

```

-----|-----|-----|
g_re= 0.0282 +/- 0.0244 | g_re= 0.0000 +/- 0.0396 | g_re= -0.0021 +/- 0.0186 |
g_im= 0.1406 +/- 0.0145 | g_im= 0.0000 +/- 0.0390 | g_im= -0.1340 +/- 0.0182 |
corr= [ 0.82] | corr= [ 1.00] | corr= [ 0.92] |
-----|-----|-----|
Br = 0.1915 +/- 0.0513 | Br = 0.0000 +/- 0.0013 | Br = 0.1673 +/- 0.0407 |

--
pi:omega[-] pi:phi[-] upper half-plane

sqrt(s)_pole = (0.24463 +/- 0.00097259)
+ (i/2)*(+0.015074 +/- 0.0015329) [-0.41]

s_pole = (0.059789 +/- 0.00048068)
+ i*(+0.0036876 +/- 0.00036926) [-0.39]

=====|=====|
pi:omega | pi:phi |
=====|=====|
k_re= -0.0462 +/- 0.0011 | k_re= -0.0146 +/- 0.0011 |
k_im= -0.0089 +/- 0.0010 | k_im= -0.0249 +/- 0.0018 |
corr= [-0.45] | corr= [-0.08] |

=====|=====|
pi:omega/3^S_1(*) | pi:phi/3^S_1 | pi:omega/3^D_1 |
=====|=====|
|g|= 0.0981 +/- 0.0054 | |g|= 0.0009 +/- 0.0154 | |g|= 0.0054 +/- 0.0036 |
arg(g)/pi= 0.0619 +/- 0.0224 | arg(g)/pi= -0.0117 +/- 11.1609 | arg(g)/pi= 0.6597 +/- 0.0360 |
-----|-----|-----|
g_re= 0.0963 +/- 0.0055 | g_re= 0.0000 +/- 0.0023 | g_re= -0.0026 +/- 0.0019 |
g_im= 0.0190 +/- 0.0068 | g_im= 0.0000 +/- 0.0247 | g_im= 0.0047 +/- 0.0031 |
corr= [-0.13] | corr= [ 1.00] | corr= [-0.93] |
-----|-----|-----|
Br = 0.9719 +/- 0.0225 | Br = 0.0000 +/- 0.0000 | Br = 0.0029 +/- 0.0038 |

--
pi:omega[-] pi:phi[-] lower half-plane

sqrt(s)_pole = (0.24463 +/- 0.00097259)
+ (i/2)*(-0.015074 +/- 0.0015329) [ 0.41]

s_pole = (0.059789 +/- 0.00048068)
+ i*(-0.0036876 +/- 0.00036926) [ 0.39]

=====|=====|
pi:omega | pi:phi |
=====|=====|
k_re= 0.0462 +/- 0.0011 | k_re= 0.0146 +/- 0.0011 |
k_im= -0.0089 +/- 0.0010 | k_im= -0.0249 +/- 0.0018 |
corr= [ 0.45] | corr= [ 0.08] |

=====|=====|
pi:omega/3^S_1(*) | pi:phi/3^S_1 | pi:omega/3^D_1 |
=====|=====|
|g|= 0.0981 +/- 0.0054 | |g|= 0.0009 +/- 0.0154 | |g|= 0.0054 +/- 0.0036 |
arg(g)/pi= -0.0619 +/- 0.0224 | arg(g)/pi= 0.0117 +/- 11.1609 | arg(g)/pi= -0.6597 +/- 0.0360 |
-----|-----|-----|
g_re= 0.0963 +/- 0.0055 | g_re= 0.0000 +/- 0.0023 | g_re= -0.0026 +/- 0.0019 |
g_im= -0.0190 +/- 0.0068 | g_im= -0.0000 +/- 0.0247 | g_im= -0.0047 +/- 0.0031 |
corr= [ 0.13] | corr= [-1.00] | corr= [ 0.93] |
-----|-----|-----|
Br = 0.9719 +/- 0.0225 | Br = 0.0000 +/- 0.0000 | Br = 0.0029 +/- 0.0038 |

```



## 1.11 coupled\_po\_pp.3s1\_3d1.pole+G0\_3s1\_3sd1\_3S1.gorder0\_3s1\_3d1\_3S1.irho

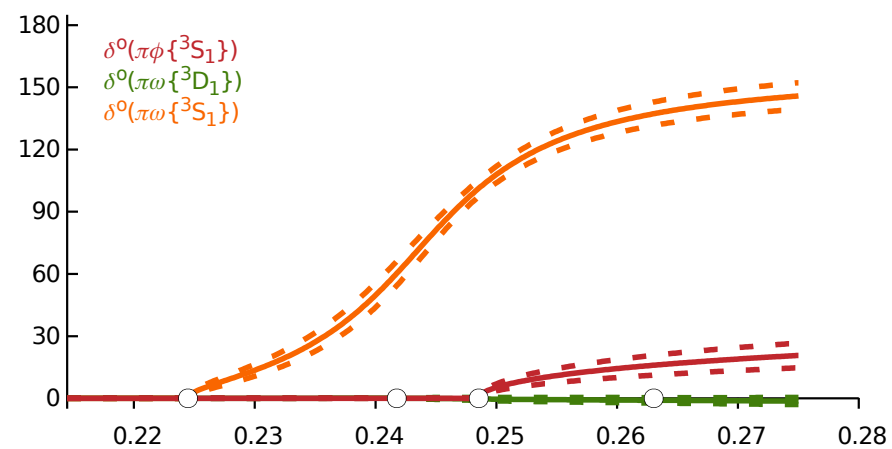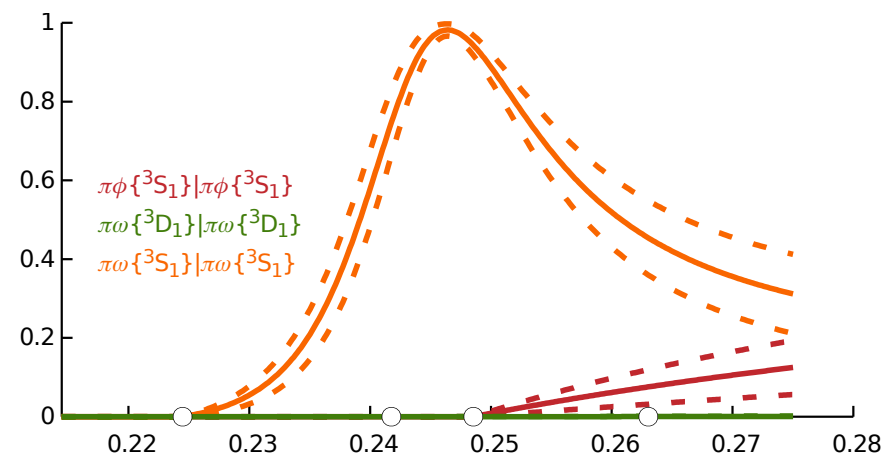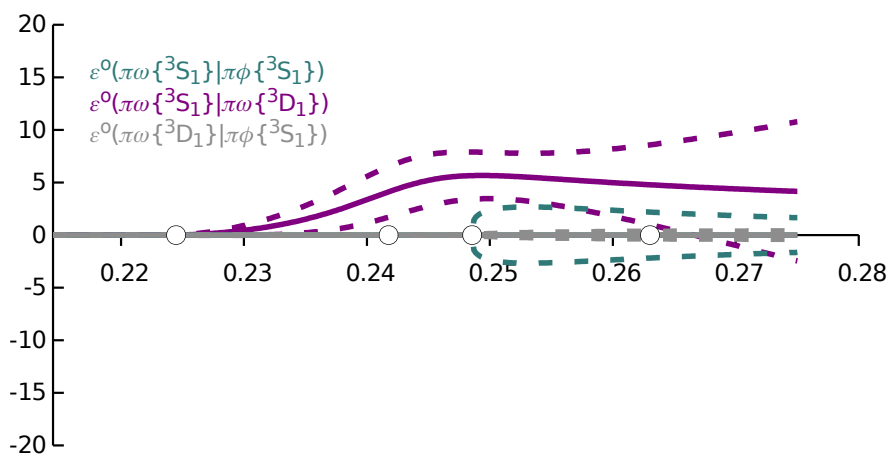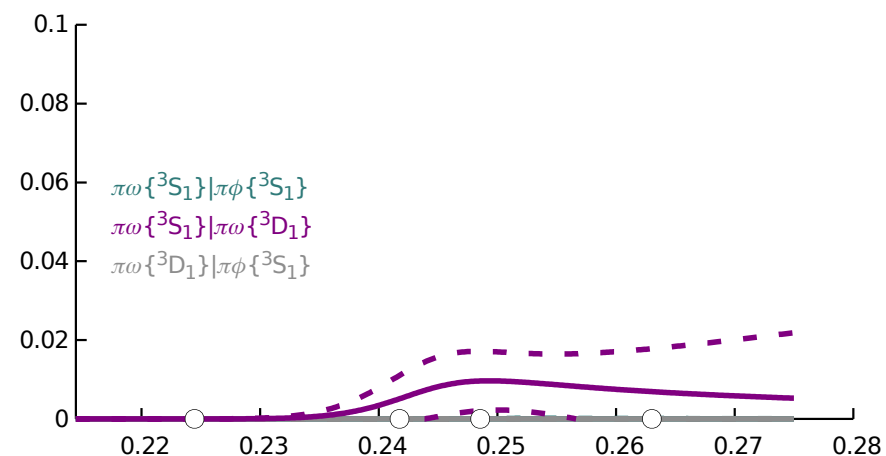



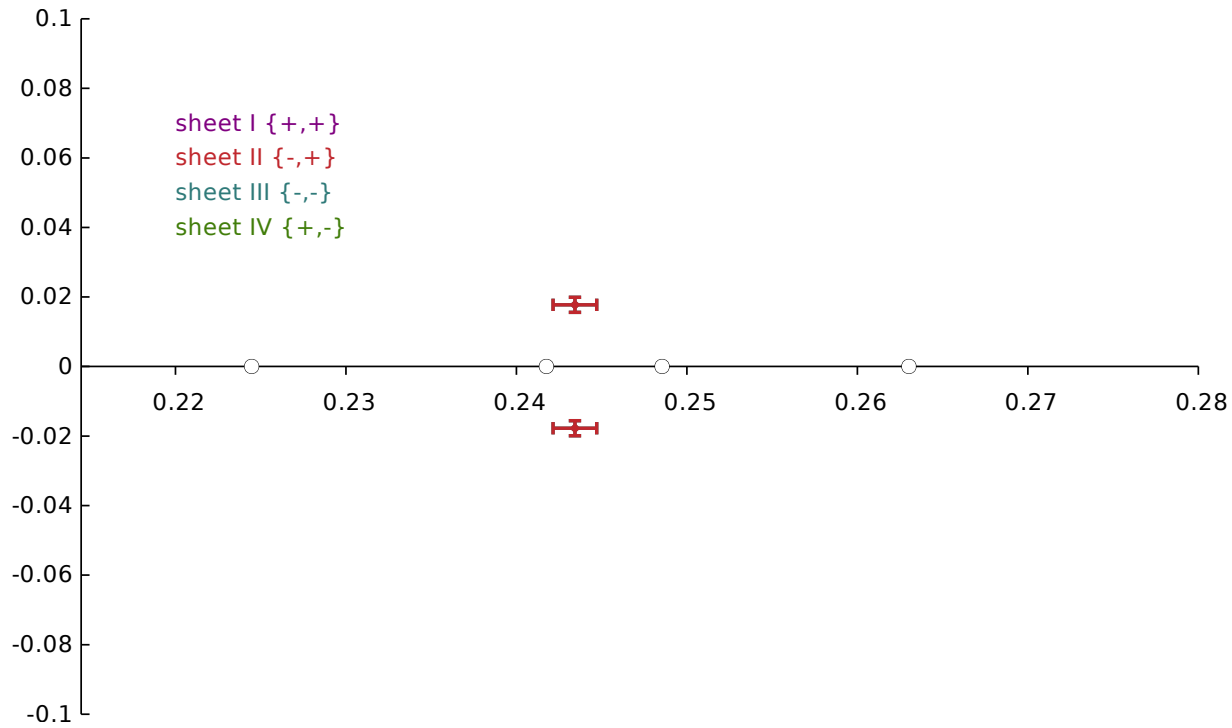

### parameter values

minimised with  $\text{chisq}/\text{nDoF} = 36.71 / (36 - 7) = 1.27$

|                                               |  |                        |  |      |      |       |      |       |       |       |
|-----------------------------------------------|--|------------------------|--|------|------|-------|------|-------|-------|-------|
| JP1+_g_pi:omega/3^D_1_pole0_order0            |  | 1.1813 +/- 0.57466     |  | 1.00 | 0.71 | 0.00  | 0.49 | -0.27 | -0.13 | -0.06 |
| JP1+_g_pi:omega/3^S_1_pole0_order0            |  | 0.11173 +/- 0.0083178  |  |      | 1.00 | -0.01 | 0.20 | -0.51 | -0.08 | -0.09 |
| JP1+_g_pi:phi/3^S_1_pole0_order0              |  | 1.4311e-05 +/- 0.01061 |  |      |      | 1.00  | 0.01 | -0.00 | 0.00  | -0.06 |
| JP1+_gamma_pi:omega/3^S_1 pi:omega/3^D_1_orde |  | 1.8245 +/- 13.11       |  |      |      |       | 1.00 | 0.15  | -0.17 | -0.19 |
| JP1+_gamma_pi:omega/3^S_1 pi:omega/3^S_1_orde |  | -0.39864 +/- 0.23104   |  |      |      |       |      | 1.00  | 0.18  | -0.04 |
| JP1+_gamma_pi:phi/3^S_1 pi:phi/3^S_1_order0   |  | 0.96384 +/- 0.29008    |  |      |      |       |      |       | 1.00  | -0.27 |
| JP1+_m_pole0                                  |  | 0.24645 +/- 0.00071639 |  |      |      |       |      |       |       | 1.00  |

### pole singularities

pi:omega[-] pi:phi[+] upper half-plane

$\text{sqrt}(s)_{\text{pole}} = (0.24343 \pm 0.0012845)$   
 $+ (i/2) * (0.017745 \pm 0.0021584) [-0.47]$

$s_{\text{pole}} = (0.05918 \pm 0.00063461)$   
 $+ i * (0.0043197 \pm 0.00051506) [-0.46]$

|                          |                         |
|--------------------------|-------------------------|
| pi:omega                 | pi:phi                  |
| ===== =====              | =====                   |
| k_re= -0.0450 +/- 0.0014 | k_re= 0.0153 +/- 0.0013 |
| k_im= -0.0107 +/- 0.0014 | k_im= 0.0277 +/- 0.0022 |



# 1 Successful Parameterizations

```

corr= [-0.50] | corr= [ 0.03] |

===== pi:omega/3^S_1(*) | pi:phi/3^S_1 | pi:omega/3^D_1 |
=====
|g|= 0.1064 +/- 0.0068 | |g|= 0.0003 +/- 0.0052 | |g|= 0.0103 +/- 0.0058 |
arg(g)/pi= 0.0776 +/- 0.0245 | arg(g)/pi= -0.4102 +/- 11.1563 | arg(g)/pi= 0.1623 +/- 0.1168 |
-----
g_re= 0.1033 +/- 0.0069 | g_re= 0.0000 +/- 0.0085 | g_re= 0.0090 +/- 0.0063 |
g_im= 0.0257 +/- 0.0081 | g_im= 0.0000 +/- 0.0018 | g_im= 0.0050 +/- 0.0028 |
corr= [-0.07] | corr= [ 1.00] | corr= [ 0.10] |
-----
Br = 0.9498 +/- 0.0253 | Br = 0.0000 +/- 0.0000 | Br = 0.0088 +/- 0.0093 |

--
pi:omega[-] pi:phi[+] lower half-plane

sqrt(s)_pole = (0.24343 +/- 0.0012845)
+ (i/2)*(-0.017745 +/- 0.0021584) [ 0.47]

s_pole = (0.05918 +/- 0.00063461)
+ i*(-0.0043197 +/- 0.00051506) [ 0.46]

===== pi:omega | pi:phi |
=====
k_re= 0.0450 +/- 0.0014 | k_re= -0.0153 +/- 0.0013 |
k_im= -0.0107 +/- 0.0014 | k_im= 0.0277 +/- 0.0022 |
corr= [ 0.50] | corr= [-0.03] |

===== pi:omega/3^S_1(*) | pi:phi/3^S_1 | pi:omega/3^D_1 |
=====
|g|= 0.1064 +/- 0.0068 | |g|= 0.0003 +/- 0.0052 | |g|= 0.0103 +/- 0.0058 |
arg(g)/pi= -0.0776 +/- 0.0245 | arg(g)/pi= 0.4102 +/- 11.1563 | arg(g)/pi= -0.1623 +/- 0.1168 |
-----
g_re= 0.1033 +/- 0.0069 | g_re= 0.0000 +/- 0.0085 | g_re= 0.0090 +/- 0.0063 |
g_im= -0.0257 +/- 0.0081 | g_im= -0.0000 +/- 0.0018 | g_im= -0.0050 +/- 0.0028 |
corr= [ 0.07] | corr= [-1.00] | corr= [-0.10] |
-----
Br = 0.9498 +/- 0.0253 | Br = 0.0000 +/- 0.0000 | Br = 0.0088 +/- 0.0093 |

--
pi:omega[-] pi:phi[-] upper half-plane

sqrt(s)_pole = (0.24343 +/- 0.0012841)
+ (i/2)*(+0.017745 +/- 0.0021581) [-0.47]

s_pole = (0.05918 +/- 0.00063443)
+ i*(+0.0043197 +/- 0.00051499) [-0.46]

===== pi:omega | pi:phi |
=====
k_re= -0.0450 +/- 0.0014 | k_re= -0.0153 +/- 0.0013 |
k_im= -0.0107 +/- 0.0014 | k_im= -0.0277 +/- 0.0022 |
corr= [-0.50] | corr= [ 0.03] |

===== pi:omega/3^S_1(*) | pi:phi/3^S_1 | pi:omega/3^D_1 |
=====
|g|= 0.1064 +/- 0.0068 | |g|= 0.0005 +/- 0.0080 | |g|= 0.0103 +/- 0.0058 |
arg(g)/pi= 0.0776 +/- 0.0245 | arg(g)/pi= 0.4562 +/- 11.1578 | arg(g)/pi= 0.1623 +/- 0.1168 |
-----
g_re= 0.1033 +/- 0.0069 | g_re= 0.0000 +/- 0.0133 | g_re= 0.0090 +/- 0.0063 |
g_im= 0.0257 +/- 0.0081 | g_im= -0.0000 +/- 0.0008 | g_im= 0.0050 +/- 0.0028 |
corr= [-0.07] | corr= [-1.00] | corr= [ 0.10] |

```



# 1 Successful Parameterizations

```

-----|-----|-----|
      Br =  0.9498 +/- 0.0253 |      Br =  0.0000 +/- 0.0000 |      Br =  0.0088 +/- 0.0093 |

--
pi:omega[-] pi:phi[-] lower half-plane

sqrt(s)_pole = (0.24343 +/- 0.0012841)
               + (i/2)*(-0.017745 +/- 0.0021581) [ 0.47]

s_pole = (0.05918 +/- 0.00063443)
         + i*(-0.0043197 +/- 0.00051499) [ 0.46]

=====|=====|
      pi:omega |      pi:phi |
=====|=====|
      k_re=  0.0450 +/- 0.0014 |      k_re=  0.0153 +/- 0.0013 |
      k_im= -0.0107 +/- 0.0014 |      k_im= -0.0277 +/- 0.0022 |
      corr= [ 0.50]           |      corr= [-0.03]           |

=====|=====|=====|
      pi:omega/3^S_1(*) |      pi:phi/3^S_1 |      pi:omega/3^D_1 |
=====|=====|=====|
      |g|=  0.1064 +/- 0.0068 |      |g|=  0.0005 +/- 0.0080 |      |g|=  0.0103 +/- 0.0058 |
arg(g)/pi= -0.0776 +/- 0.0245 | arg(g)/pi= -0.4562 +/- 11.1578 | arg(g)/pi= -0.1623 +/- 0.1168 |
-----|-----|-----|
      g_re=  0.1033 +/- 0.0069 |      g_re=  0.0000 +/- 0.0133 |      g_re=  0.0090 +/- 0.0063 |
      g_im= -0.0257 +/- 0.0081 |      g_im=  0.0000 +/- 0.0008 |      g_im= -0.0050 +/- 0.0028 |
      corr= [ 0.07]           |      corr= [ 1.00]           |      corr= [-0.10]           |
-----|-----|-----|
      Br =  0.9498 +/- 0.0253 |      Br =  0.0000 +/- 0.0000 |      Br =  0.0088 +/- 0.0093 |

```



## 1.12 coupled\_po\_pp.3s1\_3d1.pole+G0\_3s1\_3sd1\_3S1.gorder0\_3s1\_3d1\_3S1.pole0\_sub

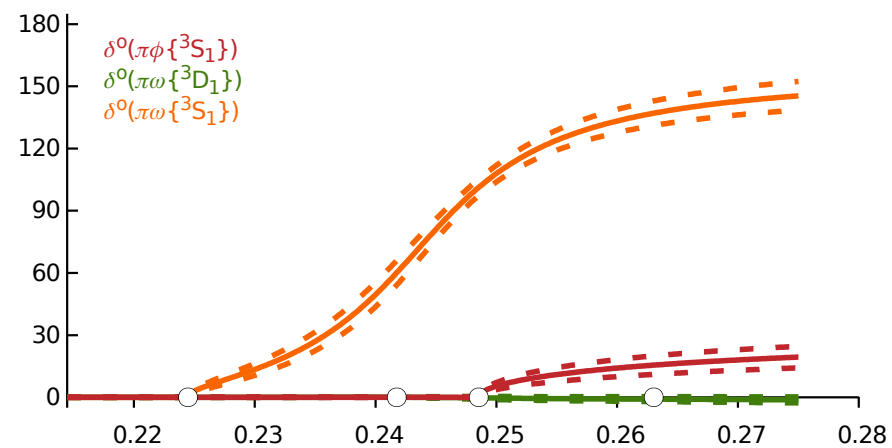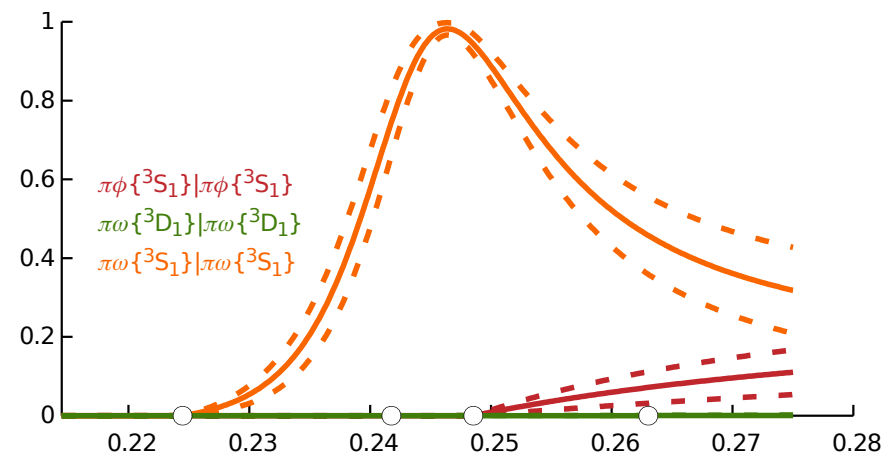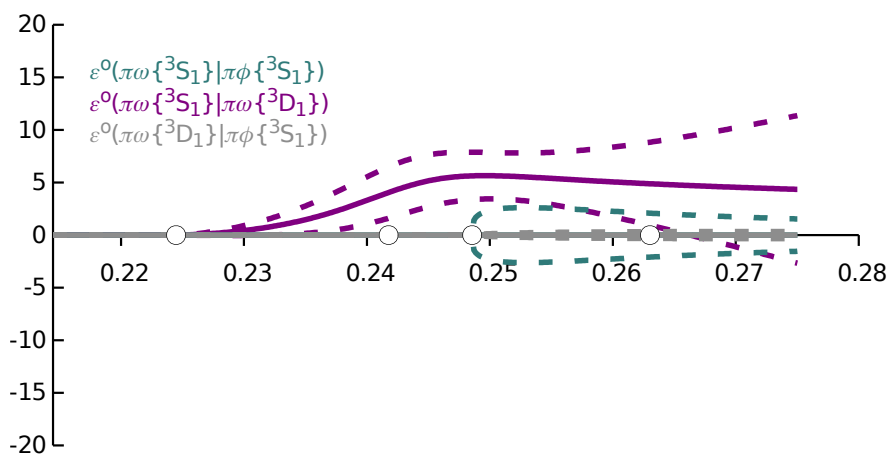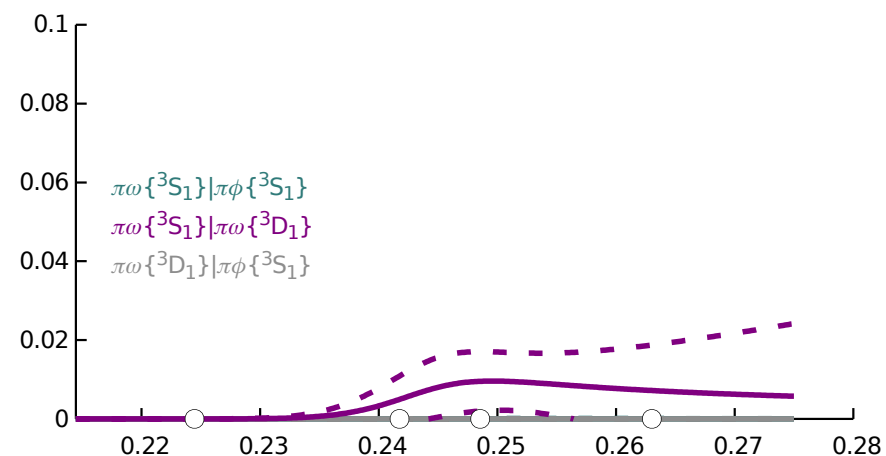



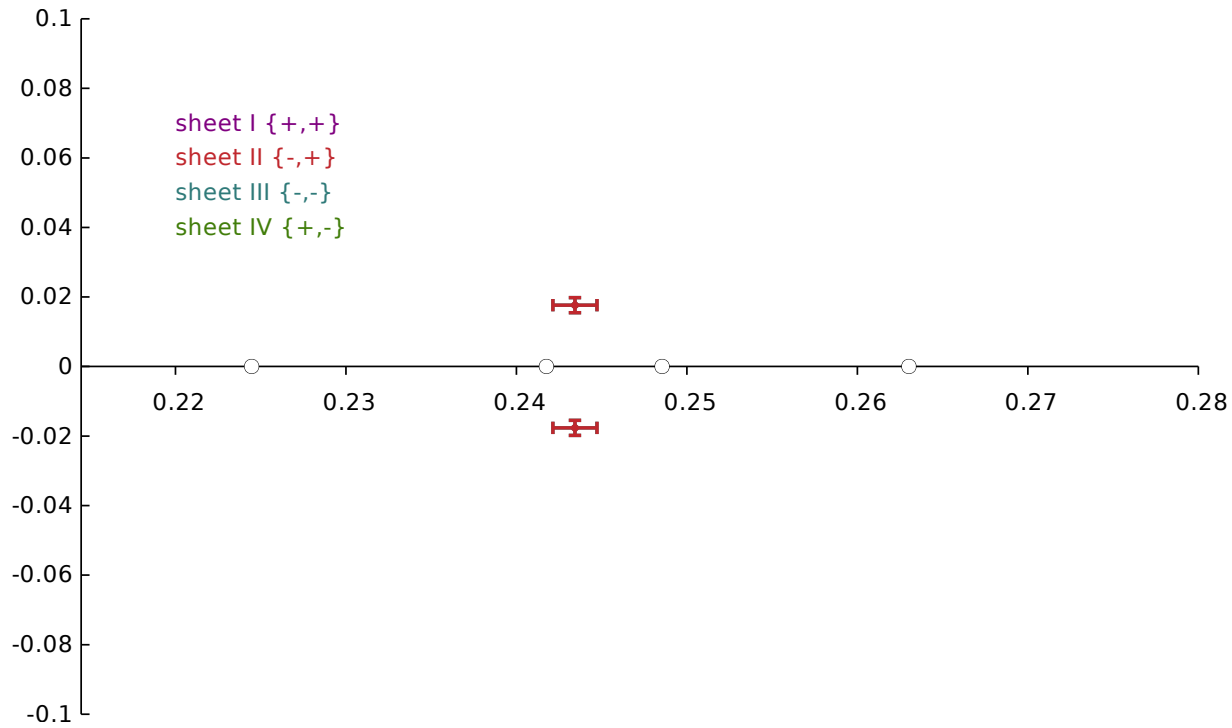

### parameter values

minimised with  $\text{chisq}/\text{nDoF} = 36.75 / (36 - 7) = 1.27$

|                                               |  |                           |  |      |      |       |      |       |       |       |
|-----------------------------------------------|--|---------------------------|--|------|------|-------|------|-------|-------|-------|
| JP1+_g_pi:omega/3^D_1_pole0_order0            |  | 1.1118 +/- 0.54329        |  | 1.00 | 0.70 | 0.00  | 0.50 | -0.25 | -0.14 | -0.06 |
| JP1+_g_pi:omega/3^S_1_pole0_order0            |  | 0.10595 +/- 0.0071609     |  |      | 1.00 | -0.01 | 0.20 | -0.49 | -0.09 | -0.09 |
| JP1+_g_pi:phi/3^S_1_pole0_order0              |  | -1.1354e-05 +/- 0.0090167 |  |      |      | 1.00  | 0.01 | -0.00 | -0.01 | -0.04 |
| JP1+_gamma_pi:omega/3^S_1 pi:omega/3^D_1_orde |  | 1.4667 +/- 12.163         |  |      |      |       | 1.00 | 0.16  | -0.18 | -0.20 |
| JP1+_gamma_pi:omega/3^S_1 pi:omega/3^S_1_orde |  | -0.34279 +/- 0.19569      |  |      |      |       |      | 1.00  | 0.19  | -0.04 |
| JP1+_gamma_pi:phi/3^S_1 pi:phi/3^S_1_order0   |  | 0.89334 +/- 0.24413       |  |      |      |       |      |       | 1.00  | -0.18 |
| JP1+_m_pole0                                  |  | 0.24645 +/- 0.00071224    |  |      |      |       |      |       |       | 1.00  |

### pole singularities

pi:omega[-] pi:phi[+] upper half-plane

$\text{sqrt}(s)_{\text{pole}} = (0.24343 \pm 0.0012951)$   
 $+ (i/2) * (0.017629 \pm 0.002161) [-0.46]$

$s_{\text{pole}} = (0.059182 \pm 0.00063942)$   
 $+ i * (0.0042914 \pm 0.00051605) [-0.44]$

|                          |                         |
|--------------------------|-------------------------|
| pi:omega                 | pi:phi                  |
| ===== =====              |                         |
| k_re= -0.0450 +/- 0.0014 | k_re= 0.0153 +/- 0.0013 |
| k_im= -0.0106 +/- 0.0014 | k_im= 0.0276 +/- 0.0022 |



# 1 Successful Parameterizations

```

corr= [-0.48]          |      corr= [ 0.02]          |
=====
pi:omega/3^S_1(*) |      pi:phi/3^S_1 |      pi:omega/3^D_1 |
=====
|g|= 0.1059 +/- 0.0069 |      |g|= 0.0003 +/- 0.0052 |      |g|= 0.0101 +/- 0.0058 |
arg(g)/pi= 0.0782 +/- 0.0250 | arg(g)/pi= -0.4352 +/- 11.1779 | arg(g)/pi= 0.1663 +/- 0.1217 |
-----
g_re= 0.1027 +/- 0.0071 |      g_re= -0.0000 +/- 0.0085 |      g_re= 0.0087 +/- 0.0064 |
g_im= 0.0258 +/- 0.0082 |      g_im= -0.0000 +/- 0.0016 |      g_im= 0.0050 +/- 0.0028 |
corr= [-0.12]          |      corr= [ 1.00]          |      corr= [ 0.08]          |
-----
Br = 0.9469 +/- 0.0266 |      Br = 0.0000 +/- 0.0000 |      Br = 0.0086 +/- 0.0092 |

--
pi:omega[-] pi:phi[+] lower half-plane

sqrt(s)_pole = (0.24343 +/- 0.0012951)
               + (i/2)*(-0.017629 +/- 0.002161) [ 0.46]

s_pole = (0.059182 +/- 0.00063942)
         + i*(-0.0042914 +/- 0.00051605) [ 0.44]

=====
pi:omega |      pi:phi |
=====
k_re= 0.0450 +/- 0.0014 |      k_re= -0.0153 +/- 0.0013 |
k_im= -0.0106 +/- 0.0014 |      k_im= 0.0276 +/- 0.0022 |
corr= [ 0.48]          |      corr= [-0.02]          |

=====
pi:omega/3^S_1(*) |      pi:phi/3^S_1 |      pi:omega/3^D_1 |
=====
|g|= 0.1059 +/- 0.0069 |      |g|= 0.0003 +/- 0.0052 |      |g|= 0.0101 +/- 0.0058 |
arg(g)/pi= -0.0782 +/- 0.0250 | arg(g)/pi= 0.4365 +/- 11.1576 | arg(g)/pi= -0.1663 +/- 0.1217 |
-----
g_re= 0.1027 +/- 0.0071 |      g_re= -0.0000 +/- 0.0085 |      g_re= 0.0087 +/- 0.0064 |
g_im= -0.0258 +/- 0.0082 |      g_im= 0.0000 +/- 0.0016 |      g_im= -0.0050 +/- 0.0028 |
corr= [ 0.12]          |      corr= [-1.00]          |      corr= [-0.08]          |
-----
Br = 0.9469 +/- 0.0266 |      Br = 0.0000 +/- 0.0000 |      Br = 0.0086 +/- 0.0092 |

--
pi:omega[-] pi:phi[-] upper half-plane

sqrt(s)_pole = (0.24343 +/- 0.0012948)
               + (i/2)*(+0.017629 +/- 0.0021606) [-0.46]

s_pole = (0.059182 +/- 0.00063926)
         + i*(+0.0042915 +/- 0.00051598) [-0.44]

=====
pi:omega |      pi:phi |
=====
k_re= -0.0450 +/- 0.0014 |      k_re= -0.0153 +/- 0.0013 |
k_im= -0.0106 +/- 0.0014 |      k_im= -0.0276 +/- 0.0022 |
corr= [-0.48]          |      corr= [ 0.02]          |

=====
pi:omega/3^S_1(*) |      pi:phi/3^S_1 |      pi:omega/3^D_1 |
=====
|g|= 0.1059 +/- 0.0069 |      |g|= 0.0005 +/- 0.0081 |      |g|= 0.0101 +/- 0.0058 |
arg(g)/pi= 0.0782 +/- 0.0250 | arg(g)/pi= 0.4622 +/- 11.1633 | arg(g)/pi= 0.1663 +/- 0.1217 |
-----
g_re= 0.1027 +/- 0.0071 |      g_re= -0.0000 +/- 0.0133 |      g_re= 0.0087 +/- 0.0064 |
g_im= 0.0258 +/- 0.0082 |      g_im= 0.0000 +/- 0.0014 |      g_im= 0.0050 +/- 0.0028 |
corr= [-0.12]          |      corr= [-1.00]          |      corr= [ 0.08]          |

```



# 1 Successful Parameterizations

```

-----|-----|-----|
      Br =  0.9469 +/- 0.0266 |      Br =  0.0000 +/- 0.0000 |      Br =  0.0086 +/- 0.0092 |

--
pi:omega[-] pi:phi[-]  lower half-plane

sqrt(s)_pole = (0.24343 +/- 0.0012948)
               + (i/2)*(-0.017629 +/- 0.0021606) [ 0.46]

s_pole = (0.059182 +/- 0.00063926)
         + i*(-0.0042915 +/- 0.00051598) [ 0.44]

=====|=====|
      pi:omega |      pi:phi |
=====|=====|
      k_re=  0.0450 +/- 0.0014 |      k_re=  0.0153 +/- 0.0013 |
      k_im= -0.0106 +/- 0.0014 |      k_im= -0.0276 +/- 0.0022 |
      corr= [ 0.48]           |      corr= [-0.02]           |

=====|=====|=====|
      pi:omega/3^S_1(*) |      pi:phi/3^S_1 |      pi:omega/3^D_1 |
=====|=====|=====|
      |g|=  0.1059 +/- 0.0069 |      |g|=  0.0005 +/- 0.0081 |      |g|=  0.0101 +/- 0.0058 |
arg(g)/pi= -0.0782 +/- 0.0250 | arg(g)/pi= -0.4613 +/- 11.1862 | arg(g)/pi= -0.1663 +/- 0.1217 |
-----|-----|-----|
      g_re=  0.1027 +/- 0.0071 |      g_re= -0.0000 +/- 0.0133 |      g_re=  0.0087 +/- 0.0064 |
      g_im= -0.0258 +/- 0.0082 |      g_im= -0.0000 +/- 0.0014 |      g_im= -0.0050 +/- 0.0028 |
      corr= [ 0.12]           |      corr= [ 1.00]           |      corr= [-0.08]           |
-----|-----|-----|
      Br =  0.9469 +/- 0.0266 |      Br =  0.0000 +/- 0.0000 |      Br =  0.0086 +/- 0.0092 |

```



## 1.13 coupled\_po\_pp.3s1\_3d1.pole+G0\_3s1\_3sd1\_3S1.gorder0\_3s1\_3d1\_3S1.threshold\_sub

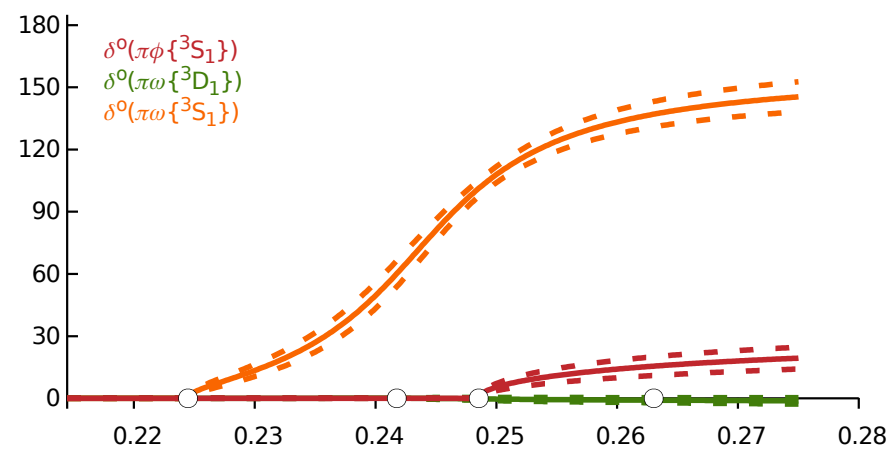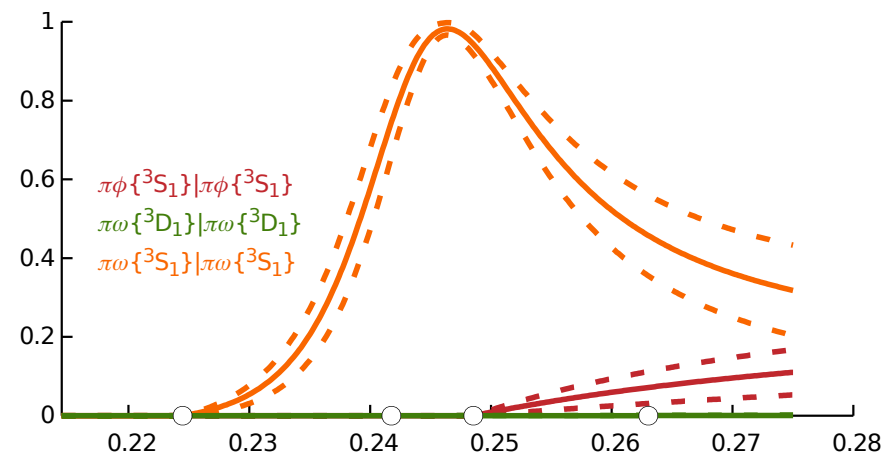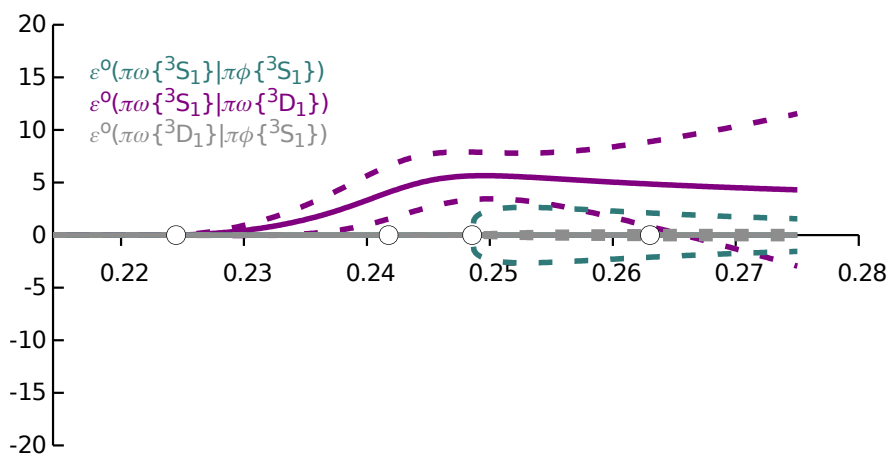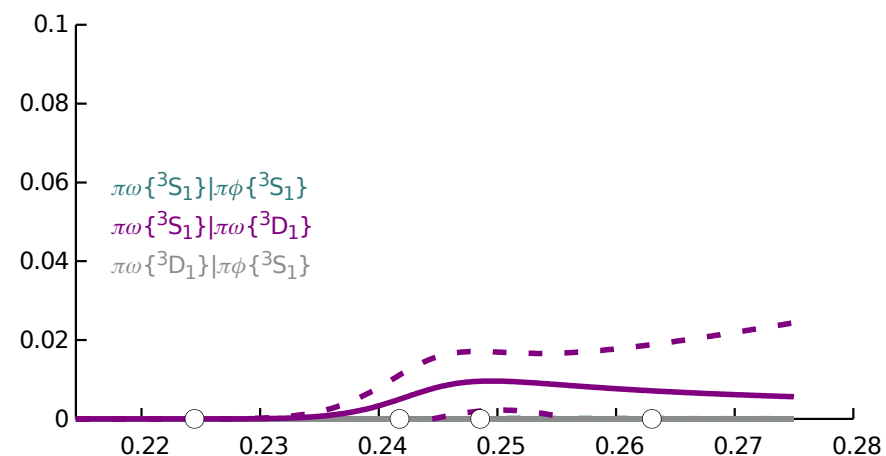



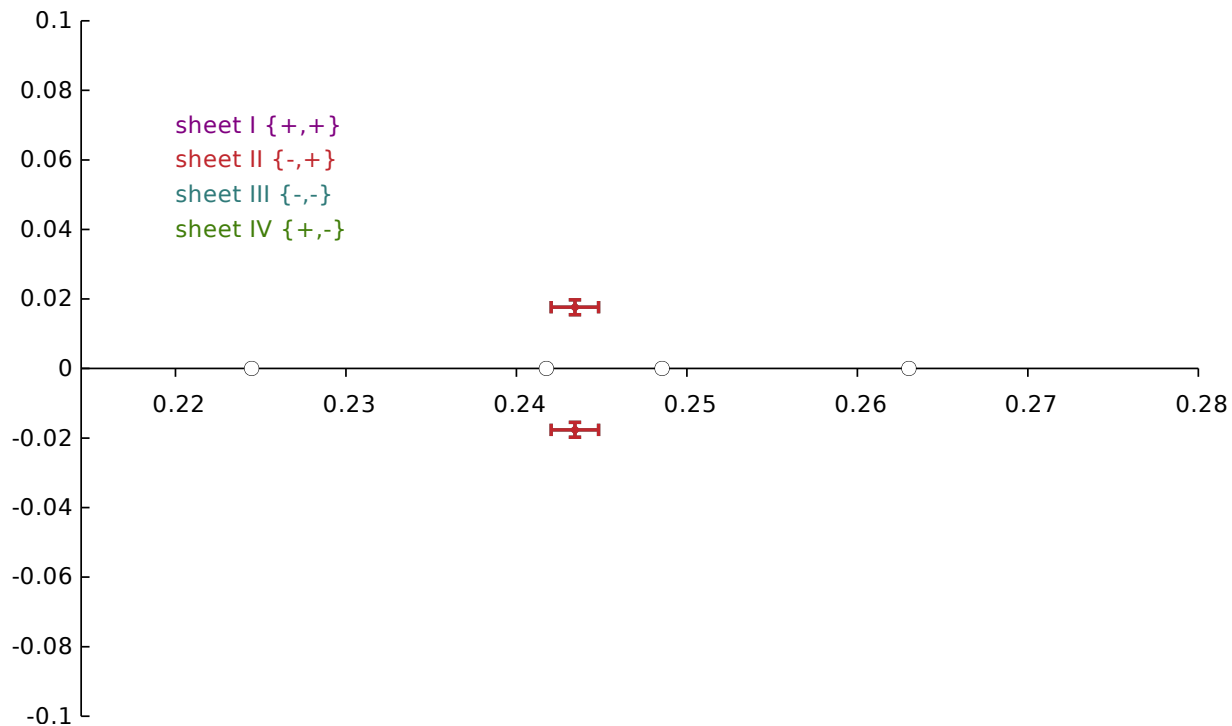

### parameter values

minimised with  $\text{chisq}/\text{nDoF} = 36.75 / (36 - 7) = 1.27$

|                                               |  |                          |  |      |      |       |      |       |       |       |
|-----------------------------------------------|--|--------------------------|--|------|------|-------|------|-------|-------|-------|
| JP1+_g_pi:omega/3^D_1_pole0_order0            |  | 1.1284 +/- 0.63356       |  | 1.00 | 0.70 | 0.00  | 0.66 | -0.22 | -0.13 | -0.45 |
| JP1+_g_pi:omega/3^S_1_pole0_order0            |  | 0.10237 +/- 0.0064041    |  |      | 1.00 | -0.00 | 0.32 | -0.27 | -0.01 | -0.58 |
| JP1+_g_pi:phi/3^S_1_pole0_order0              |  | -1.7035e-07 +/- 0.010042 |  |      |      | 1.00  | 0.00 | -0.00 | 0.00  | -0.02 |
| JP1+_gamma_pi:omega/3^S_1 pi:omega/3^D_1_orde |  | 1.5103 +/- 12.124        |  |      |      |       | 1.00 | 0.12  | -0.15 | -0.32 |
| JP1+_gamma_pi:omega/3^S_1 pi:omega/3^S_1_orde |  | -0.33091 +/- 0.18587     |  |      |      |       |      | 1.00  | 0.18  | 0.18  |
| JP1+_gamma_pi:phi/3^S_1 pi:phi/3^S_1_order0   |  | 0.98807 +/- 0.30528      |  |      |      |       |      |       | 1.00  | -0.20 |
| JP1+_m_pole0                                  |  | 0.24423 +/- 0.00079476   |  |      |      |       |      |       |       | 1.00  |

### pole singularities

pi:omega[-] pi:phi[+] upper half-plane

$\text{sqrt}(s)_{\text{pole}} = (0.24343 \pm 0.0013935)$   
 $+ (i/2) * (0.017633 \pm 0.0021476) [-0.48]$

$s_{\text{pole}} = (0.059181 \pm 0.00068779)$   
 $+ i * (0.0042923 \pm 0.00051137) [-0.47]$

|                          |                         |
|--------------------------|-------------------------|
| pi:omega                 | pi:phi                  |
| ===== =====              |                         |
| k_re= -0.0450 +/- 0.0015 | k_re= 0.0153 +/- 0.0013 |
| k_im= -0.0106 +/- 0.0014 | k_im= 0.0277 +/- 0.0023 |



# 1 Successful Parameterizations

```

corr= [-0.53]          |      corr= [-0.05]          |
=====
pi:omega/3^S_1(*) |      pi:phi/3^S_1 |      pi:omega/3^D_1 |
=====
|g|= 0.1059 +/- 0.0069 |      |g|= 0.0003 +/- 0.0052 |      |g|= 0.0101 +/- 0.0060 |
arg(g)/pi= 0.0782 +/- 0.0264 | arg(g)/pi= -0.4275 +/- 11.1657 | arg(g)/pi= 0.1654 +/- 0.1246 |
-----
g_re= 0.1028 +/- 0.0071 |      g_re= -0.0000 +/- 0.0086 |      g_re= 0.0088 +/- 0.0066 |
g_im= 0.0258 +/- 0.0086 |      g_im= -0.0000 +/- 0.0017 |      g_im= 0.0050 +/- 0.0028 |
corr= [-0.14]          |      corr= [ 1.00]          |      corr= [ 0.07]          |
-----
Br = 0.9467 +/- 0.0276 |      Br = 0.0000 +/- 0.0000 |      Br = 0.0086 +/- 0.0095 |

--
pi:omega[-] pi:phi[+] lower half-plane

sqrt(s)_pole = (0.24343 +/- 0.0013935)
               + (i/2)*(-0.017633 +/- 0.0021476) [ 0.48]

s_pole = (0.059181 +/- 0.00068779)
         + i*(-0.0042923 +/- 0.00051137) [ 0.47]

pi:omega |      pi:phi |
=====
k_re= 0.0450 +/- 0.0015 |      k_re= -0.0153 +/- 0.0013 |
k_im= -0.0106 +/- 0.0014 |      k_im= 0.0277 +/- 0.0023 |
corr= [ 0.53]          |      corr= [ 0.05]          |

pi:omega/3^S_1(*) |      pi:phi/3^S_1 |      pi:omega/3^D_1 |
=====
|g|= 0.1059 +/- 0.0069 |      |g|= 0.0003 +/- 0.0052 |      |g|= 0.0101 +/- 0.0060 |
arg(g)/pi= -0.0782 +/- 0.0264 | arg(g)/pi= 0.4275 +/- 11.1657 | arg(g)/pi= -0.1654 +/- 0.1246 |
-----
g_re= 0.1028 +/- 0.0071 |      g_re= -0.0000 +/- 0.0086 |      g_re= 0.0088 +/- 0.0066 |
g_im= -0.0258 +/- 0.0086 |      g_im= 0.0000 +/- 0.0017 |      g_im= -0.0050 +/- 0.0028 |
corr= [ 0.14]          |      corr= [-1.00]          |      corr= [-0.07]          |
-----
Br = 0.9467 +/- 0.0276 |      Br = 0.0000 +/- 0.0000 |      Br = 0.0086 +/- 0.0095 |

--
pi:omega[-] pi:phi[-] upper half-plane

sqrt(s)_pole = (0.24343 +/- 0.0013932)
               + (i/2)*(+0.017633 +/- 0.0021472) [-0.48]

s_pole = (0.059181 +/- 0.00068765)
         + i*(+0.0042924 +/- 0.00051128) [-0.47]

pi:omega |      pi:phi |
=====
k_re= -0.0450 +/- 0.0015 |      k_re= -0.0153 +/- 0.0013 |
k_im= -0.0106 +/- 0.0014 |      k_im= -0.0277 +/- 0.0023 |
corr= [-0.53]          |      corr= [-0.05]          |

pi:omega/3^S_1(*) |      pi:phi/3^S_1 |      pi:omega/3^D_1 |
=====
|g|= 0.1059 +/- 0.0069 |      |g|= 0.0005 +/- 0.0081 |      |g|= 0.0101 +/- 0.0060 |
arg(g)/pi= 0.0782 +/- 0.0264 | arg(g)/pi= 0.4541 +/- 11.1674 | arg(g)/pi= 0.1654 +/- 0.1246 |
-----
g_re= 0.1028 +/- 0.0071 |      g_re= -0.0000 +/- 0.0134 |      g_re= 0.0088 +/- 0.0066 |
g_im= 0.0258 +/- 0.0086 |      g_im= -0.0000 +/- 0.0014 |      g_im= 0.0050 +/- 0.0028 |
corr= [-0.14]          |      corr= [-1.00]          |      corr= [ 0.07]          |

```



## 1 Successful Parameterizations

```

-----|-----|-----|
      Br =  0.9467 +/- 0.0276 |      Br =  0.0000 +/- 0.0000 |      Br =  0.0086 +/- 0.0095 |

--
pi:omega[-] pi:phi[-]  lower half-plane

sqrt(s)_pole = (0.24343 +/- 0.0013932)
               + (i/2)*(-0.017633 +/- 0.0021472) [ 0.48]

s_pole = (0.059181 +/- 0.00068765)
         + i*(-0.0042924 +/- 0.00051128) [ 0.47]

=====|=====|
      pi:omega |      pi:phi |
=====|=====|
      k_re=  0.0450 +/- 0.0015 |      k_re=  0.0153 +/- 0.0013 |
      k_im= -0.0106 +/- 0.0014 |      k_im= -0.0277 +/- 0.0023 |
      corr= [ 0.53]           |      corr= [ 0.05]           |

=====|=====|=====|
      pi:omega/3^S_1(*) |      pi:phi/3^S_1 |      pi:omega/3^D_1 |
=====|=====|=====|
      |g|=  0.1059 +/- 0.0069 |      |g|=  0.0005 +/- 0.0081 |      |g|=  0.0101 +/- 0.0060 |
arg(g)/pi= -0.0782 +/- 0.0264 | arg(g)/pi= -0.4541 +/- 11.1674 | arg(g)/pi= -0.1654 +/- 0.1246 |
-----|-----|-----|
      g_re=  0.1028 +/- 0.0071 |      g_re= -0.0000 +/- 0.0134 |      g_re=  0.0088 +/- 0.0066 |
      g_im= -0.0258 +/- 0.0086 |      g_im=  0.0000 +/- 0.0014 |      g_im= -0.0050 +/- 0.0028 |
      corr= [ 0.14]           |      corr= [ 1.00]           |      corr= [-0.07]           |
-----|-----|-----|
      Br =  0.9467 +/- 0.0276 |      Br =  0.0000 +/- 0.0000 |      Br =  0.0086 +/- 0.0095 |

```



## 1.14 coupled\_po\_pp.3s1\_3d1.pole+G0\_3s1\_3sd1\_3S1.gorder0\_3s1\_3d1.irho

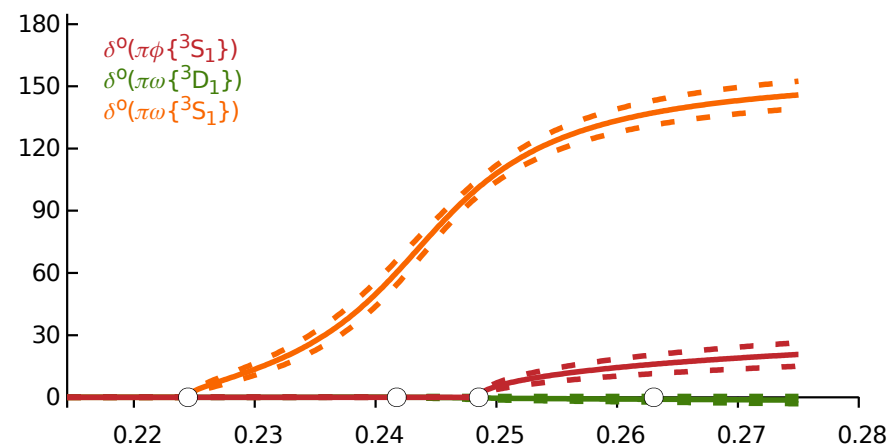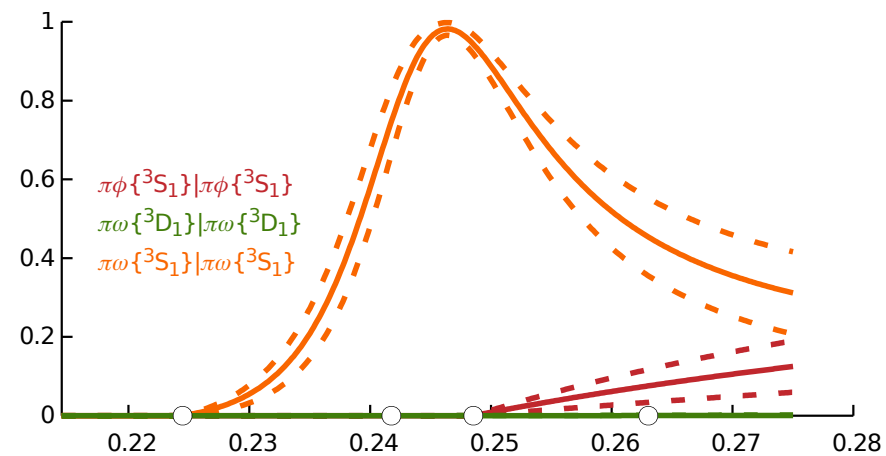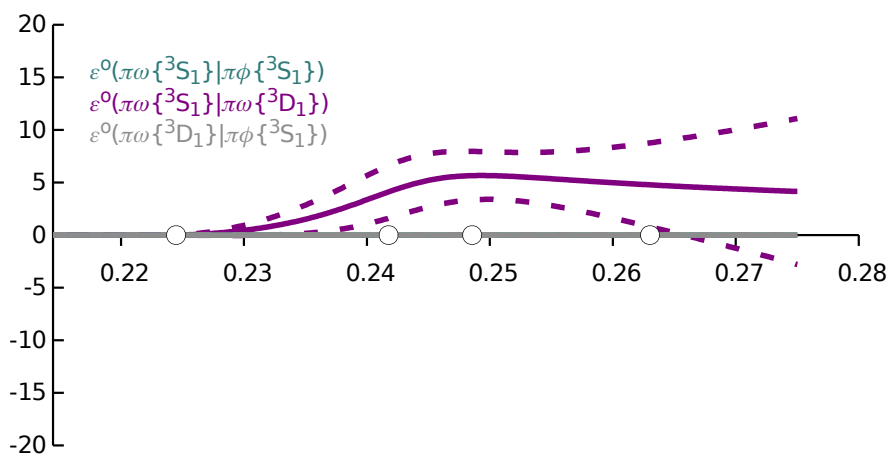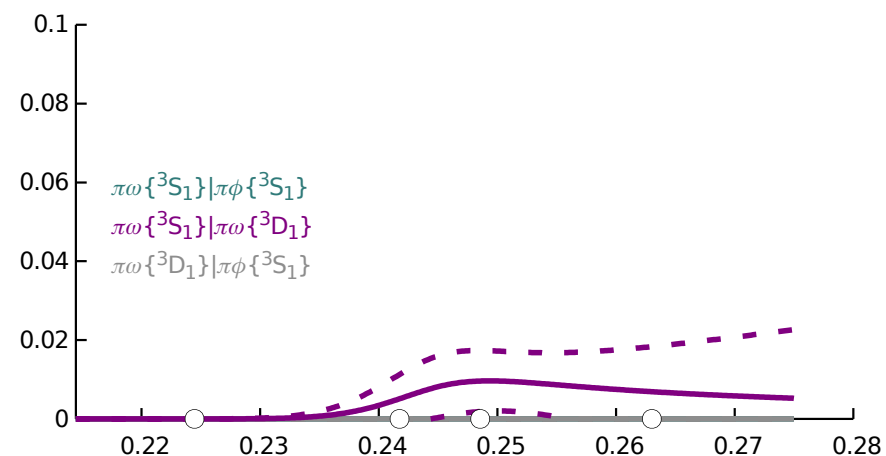



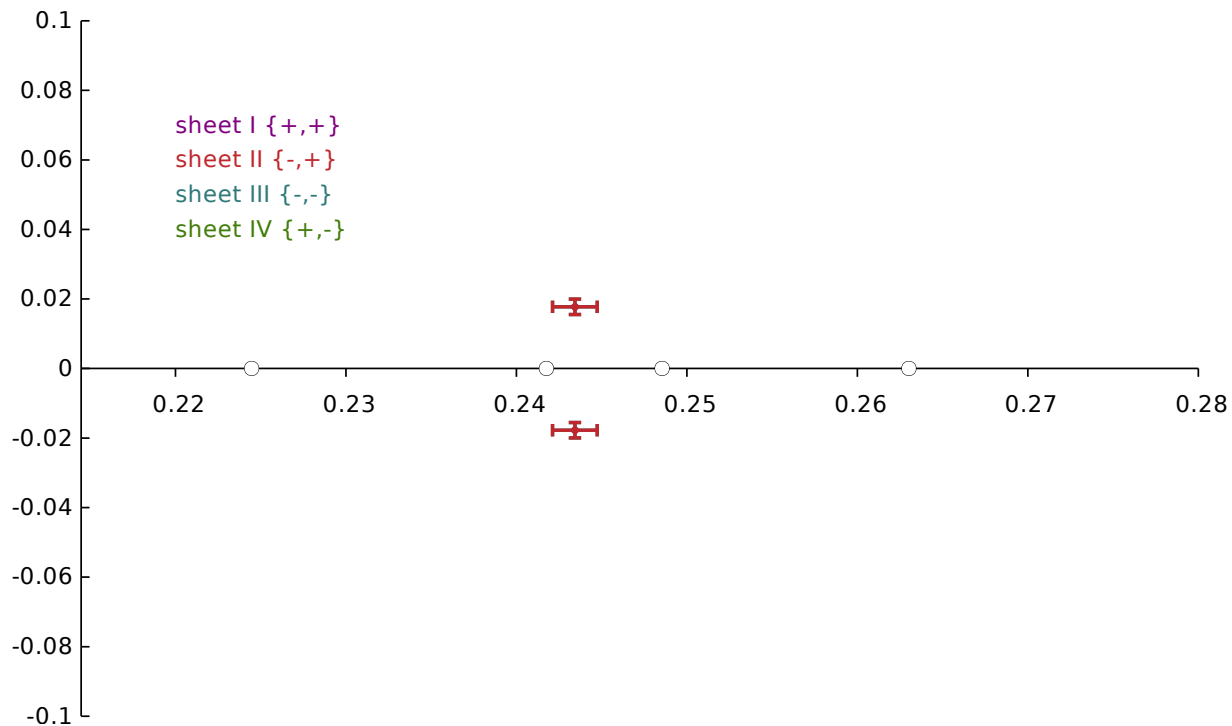

### parameter values

minimised with  $\text{chisq}/\text{nDoF} = 36.71 / (36 - 6) = 1.22$

|                                               |  |                        |  |      |      |      |       |       |       |
|-----------------------------------------------|--|------------------------|--|------|------|------|-------|-------|-------|
| JP1+_g_pi:omega/3^D_1_pole0_order0            |  | 1.1805 +/- 0.57462     |  | 1.00 | 0.71 | 0.49 | -0.27 | -0.13 | -0.06 |
| JP1+_g_pi:omega/3^S_1_pole0_order0            |  | 0.11171 +/- 0.0083153  |  |      | 1.00 | 0.21 | -0.51 | -0.08 | -0.09 |
| JP1+_gamma_pi:omega/3^S_1 pi:omega/3^D_1_orde |  | 1.8305 +/- 13.109      |  |      |      | 1.00 | 0.15  | -0.17 | -0.19 |
| JP1+_gamma_pi:omega/3^S_1 pi:omega/3^S_1_orde |  | -0.39831 +/- 0.23099   |  |      |      |      | 1.00  | 0.18  | -0.04 |
| JP1+_gamma_pi:phi/3^S_1 pi:phi/3^S_1_order0   |  | 0.96356 +/- 0.29003    |  |      |      |      |       | 1.00  | -0.27 |
| JP1+_m_pole0                                  |  | 0.24645 +/- 0.00071508 |  |      |      |      |       |       | 1.00  |

### pole singularities

pi:omega[-] pi:phi[+] upper half-plane

$\text{sqrt}(s)_{\text{pole}} = (0.24343 \pm 0.0013086)$   
 $+ (i/2)*(+0.017743 \pm 0.0022271) [-0.54]$

$s_{\text{pole}} = (0.059181 \pm 0.00064801)$   
 $+ i*(+0.0043193 \pm 0.00052998) [-0.53]$

|                          |                         |
|--------------------------|-------------------------|
| pi:omega                 | pi:phi                  |
| ===== =====              |                         |
| k_re= -0.0450 +/- 0.0014 | k_re= 0.0153 +/- 0.0012 |
| k_im= -0.0107 +/- 0.0015 | k_im= 0.0277 +/- 0.0023 |
| corr= [-0.56]            | corr= [ 0.08]           |



# 1 Successful Parameterizations

| pi:omega/3^S_1(*)                                                   | pi:phi/3^S_1                                                        | pi:omega/3^D_1                                                      |
|---------------------------------------------------------------------|---------------------------------------------------------------------|---------------------------------------------------------------------|
| g = 0.1064 +/- 0.0070<br>arg(g)/pi= 0.0775 +/- 0.0250               | g = 0.0000 +/- 0.0000<br>arg(g)/pi= 0.4225 +/- 0.0250               | g = 0.0103 +/- 0.0060<br>arg(g)/pi= 0.1622 +/- 0.1231               |
| g_re= 0.1033 +/- 0.0069<br>g_im= 0.0257 +/- 0.0084<br>corr= [-0.01] | g_re= 0.0000 +/- 0.0000<br>g_im= 0.0000 +/- 0.0000<br>corr= [-0.16] | g_re= 0.0090 +/- 0.0065<br>g_im= 0.0050 +/- 0.0030<br>corr= [ 0.08] |
| Br = 0.9489 +/- 0.0246                                              | Br = 0.0000 +/- 0.0000                                              | Br = 0.0088 +/- 0.0096                                              |

--  
pi:omega[-] pi:phi[+] lower half-plane

sqrt(s)\_pole = (0.24343 +/- 0.0013086)  
+ (i/2)\*(-0.017743 +/- 0.0022271) [ 0.54]

s\_pole = (0.059181 +/- 0.00064801)  
+ i\*(-0.0043193 +/- 0.00052998) [ 0.53]

| pi:omega                                                             | pi:phi                                                               |
|----------------------------------------------------------------------|----------------------------------------------------------------------|
| k_re= 0.0450 +/- 0.0014<br>k_im= -0.0107 +/- 0.0015<br>corr= [ 0.56] | k_re= -0.0153 +/- 0.0012<br>k_im= 0.0277 +/- 0.0023<br>corr= [-0.08] |

| pi:omega/3^S_1(*)                                                    | pi:phi/3^S_1                                                         | pi:omega/3^D_1                                                       |
|----------------------------------------------------------------------|----------------------------------------------------------------------|----------------------------------------------------------------------|
| g = 0.1064 +/- 0.0070<br>arg(g)/pi= -0.0775 +/- 0.0250               | g = 0.0000 +/- 0.0000<br>arg(g)/pi= 0.5775 +/- 0.0250                | g = 0.0103 +/- 0.0060<br>arg(g)/pi= -0.1622 +/- 0.1231               |
| g_re= 0.1033 +/- 0.0069<br>g_im= -0.0257 +/- 0.0084<br>corr= [ 0.01] | g_re= -0.0000 +/- 0.0000<br>g_im= 0.0000 +/- 0.0000<br>corr= [ 0.16] | g_re= 0.0090 +/- 0.0065<br>g_im= -0.0050 +/- 0.0030<br>corr= [-0.08] |
| Br = 0.9489 +/- 0.0246                                               | Br = 0.0000 +/- 0.0000                                               | Br = 0.0088 +/- 0.0096                                               |

--  
pi:omega[-] pi:phi[-] upper half-plane

sqrt(s)\_pole = (0.24343 +/- 0.0013086)  
+ (i/2)\*(+0.017743 +/- 0.0022271) [-0.54]

s\_pole = (0.059181 +/- 0.00064801)  
+ i\*(+0.0043193 +/- 0.00052998) [-0.53]

| pi:omega                                                              | pi:phi                                                                |
|-----------------------------------------------------------------------|-----------------------------------------------------------------------|
| k_re= -0.0450 +/- 0.0014<br>k_im= -0.0107 +/- 0.0015<br>corr= [-0.56] | k_re= -0.0153 +/- 0.0012<br>k_im= -0.0277 +/- 0.0023<br>corr= [ 0.08] |

| pi:omega/3^S_1(*)                                                   | pi:phi/3^S_1                                                        | pi:omega/3^D_1                                                      |
|---------------------------------------------------------------------|---------------------------------------------------------------------|---------------------------------------------------------------------|
| g = 0.1064 +/- 0.0070<br>arg(g)/pi= 0.0775 +/- 0.0250               | g = 0.0000 +/- 0.0000<br>arg(g)/pi= 0.4225 +/- 0.0250               | g = 0.0103 +/- 0.0060<br>arg(g)/pi= 0.1622 +/- 0.1231               |
| g_re= 0.1033 +/- 0.0069<br>g_im= 0.0257 +/- 0.0084<br>corr= [-0.01] | g_re= 0.0000 +/- 0.0000<br>g_im= 0.0000 +/- 0.0000<br>corr= [-0.16] | g_re= 0.0090 +/- 0.0065<br>g_im= 0.0050 +/- 0.0030<br>corr= [ 0.08] |



# 1 Successful Parameterizations

```

Br = 0.9489 +/- 0.0246 | Br = 0.0000 +/- 0.0000 | Br = 0.0088 +/- 0.0096 |

--
pi:omega[-] pi:phi[-] lower half-plane

sqrt(s)_pole = (0.24343 +/- 0.0013086)
               + (i/2)*(-0.017743 +/- 0.0022271) [ 0.54]

s_pole = (0.059181 +/- 0.00064801)
         + i*(-0.0043193 +/- 0.00052998) [ 0.53]

=====
pi:omega | pi:phi |
=====
k_re= 0.0450 +/- 0.0014 | k_re= 0.0153 +/- 0.0012 |
k_im= -0.0107 +/- 0.0015 | k_im= -0.0277 +/- 0.0023 |
corr= [ 0.56] | corr= [-0.08] |

=====
pi:omega/3^S_1(*) | pi:phi/3^S_1 | pi:omega/3^D_1 |
=====
|g|= 0.1064 +/- 0.0070 | |g|= 0.0000 +/- 0.0000 | |g|= 0.0103 +/- 0.0060 |
arg(g)/pi= -0.0775 +/- 0.0250 | arg(g)/pi= 0.5775 +/- 0.0250 | arg(g)/pi= -0.1622 +/- 0.1231 |
-----
g_re= 0.1033 +/- 0.0069 | g_re= -0.0000 +/- 0.0000 | g_re= 0.0090 +/- 0.0065 |
g_im= -0.0257 +/- 0.0084 | g_im= 0.0000 +/- 0.0000 | g_im= -0.0050 +/- 0.0030 |
corr= [ 0.01] | corr= [ 0.16] | corr= [-0.08] |
-----
Br = 0.9489 +/- 0.0246 | Br = 0.0000 +/- 0.0000 | Br = 0.0088 +/- 0.0096 |

```



## 1.15 coupled\_po\_pp.3s1\_3d1.pole+G0\_3s1\_3sd1\_3S1.gorder0\_3s1\_3d1.pole0\_sub

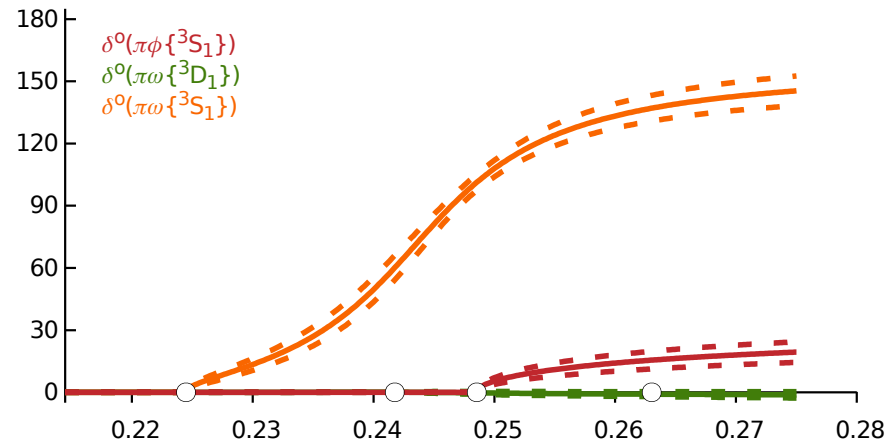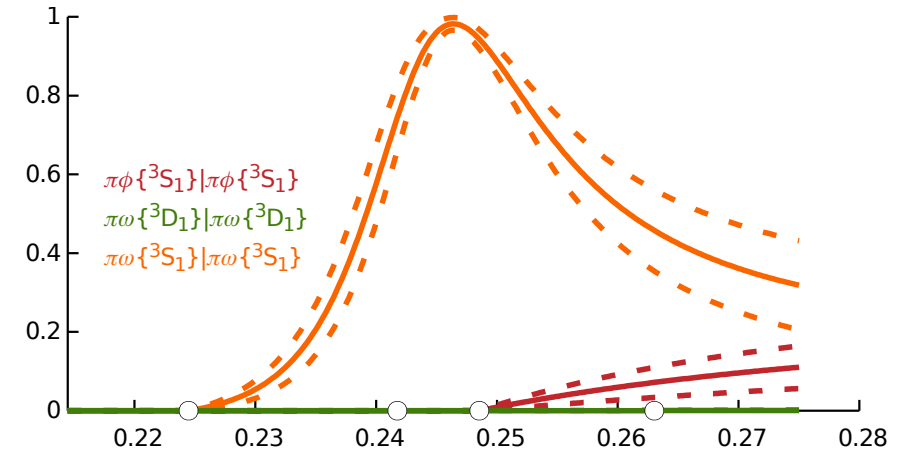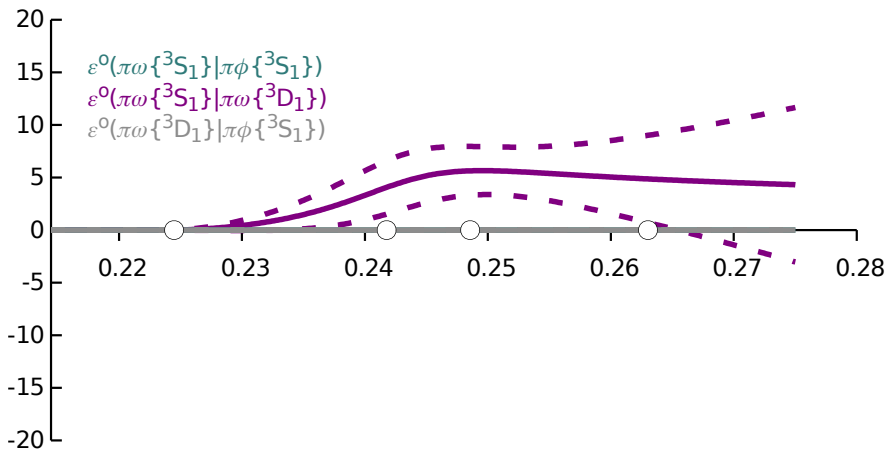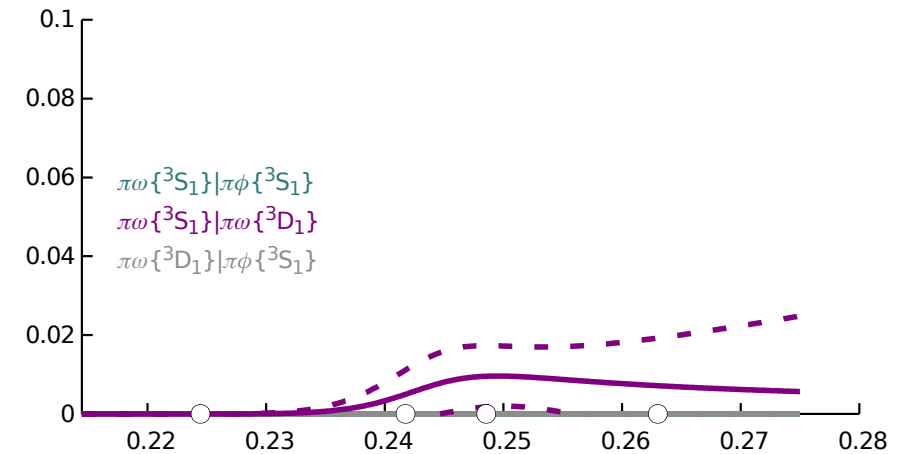



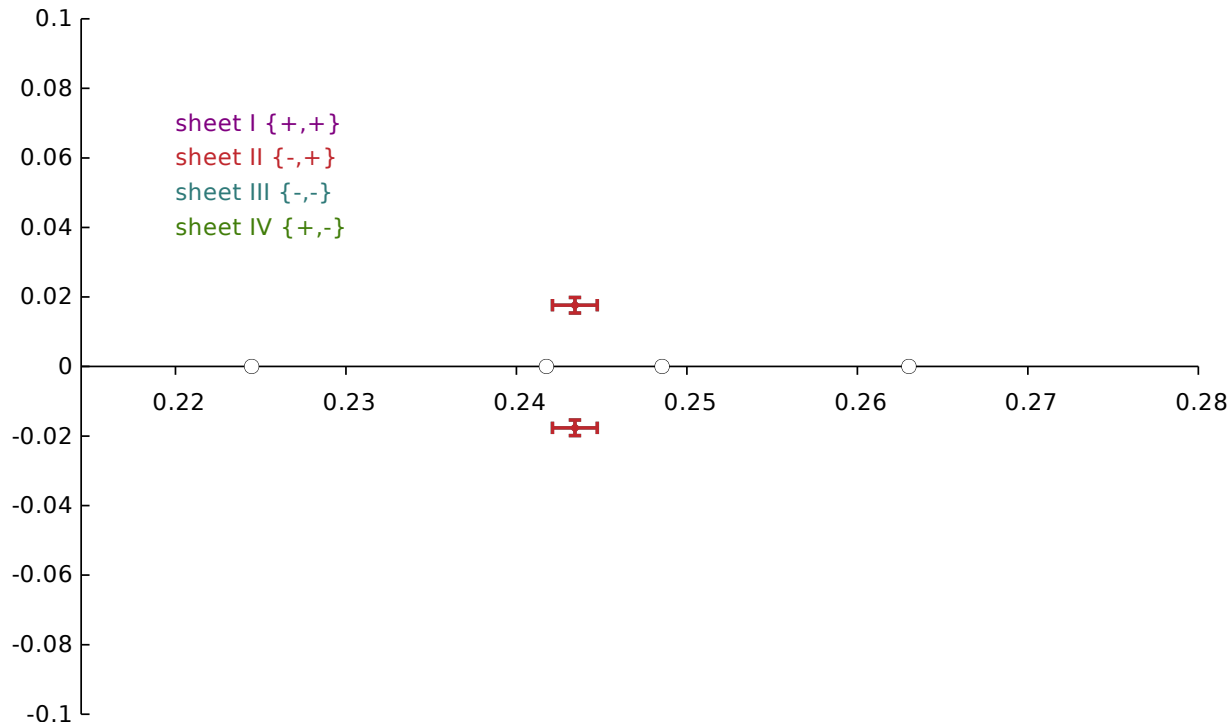

### parameter values

minimised with  $\text{chisq}/\text{nDoF} = 36.75 / (36 - 6) = 1.22$

|                                               |  |                        |  |      |      |      |       |       |       |
|-----------------------------------------------|--|------------------------|--|------|------|------|-------|-------|-------|
| JP1+_g_pi:omega/3^D_1_pole0_order0            |  | 1.1133 +/- 0.54313     |  | 1.00 | 0.70 | 0.50 | -0.25 | -0.14 | -0.06 |
| JP1+_g_pi:omega/3^S_1_pole0_order0            |  | 0.10595 +/- 0.0071587  |  |      | 1.00 | 0.20 | -0.49 | -0.09 | -0.09 |
| JP1+_gamma_pi:omega/3^S_1 pi:omega/3^D_1_orde |  | 1.5271 +/- 12.153      |  |      |      | 1.00 | 0.16  | -0.18 | -0.20 |
| JP1+_gamma_pi:omega/3^S_1 pi:omega/3^S_1_orde |  | -0.34290 +/- 0.19568   |  |      |      |      | 1.00  | 0.19  | -0.04 |
| JP1+_gamma_pi:phi/3^S_1 pi:phi/3^S_1_order0   |  | 0.89328 +/- 0.2441     |  |      |      |      |       | 1.00  | -0.19 |
| JP1+_m_pole0                                  |  | 0.24645 +/- 0.00071174 |  |      |      |      |       |       | 1.00  |

### pole singularities

pi:omega[-] pi:phi[+] upper half-plane

$\text{sqrt}(s)_{\text{pole}} = (0.24343 \pm 0.0013119)$   
 $+ (i/2)*(+0.017629 \pm 0.0022246) [-0.52]$

$s_{\text{pole}} = (0.059182 \pm 0.00064923)$   
 $+ i*(+0.0042915 \pm 0.00052978) [-0.51]$

|                          |                         |
|--------------------------|-------------------------|
| pi:omega                 | pi:phi                  |
| ===== =====              |                         |
| k_re= -0.0450 +/- 0.0014 | k_re= 0.0153 +/- 0.0013 |
| k_im= -0.0106 +/- 0.0015 | k_im= 0.0276 +/- 0.0023 |
| corr= [-0.54]            | corr= [ 0.07]           |



# 1 Successful Parameterizations

| pi:omega/3^S_1(*)            | pi:phi/3^S_1                 | pi:omega/3^D_1               |
|------------------------------|------------------------------|------------------------------|
| g = 0.1059 +/- 0.0070        | g = 0.0000 +/- 0.0000        | g = 0.0101 +/- 0.0060        |
| arg(g)/pi= 0.0782 +/- 0.0255 | arg(g)/pi= 0.4218 +/- 0.0255 | arg(g)/pi= 0.1656 +/- 0.1274 |
| g_re= 0.1027 +/- 0.0071      | g_re= 0.0000 +/- 0.0000      | g_re= 0.0088 +/- 0.0066      |
| g_im= 0.0258 +/- 0.0085      | g_im= 0.0000 +/- 0.0000      | g_im= 0.0050 +/- 0.0030      |
| corr= [-0.06]                | corr= [-0.12]                | corr= [ 0.07]                |
| Br = 0.9458 +/- 0.0261       | Br = 0.0000 +/- 0.0000       | Br = 0.0086 +/- 0.0095       |

--

pi:omega[-] pi:phi[+] lower half-plane

sqrt(s)\_pole = (0.24343 +/- 0.0013119)  
+ (i/2)\*(-0.017629 +/- 0.0022246) [ 0.52]

s\_pole = (0.059182 +/- 0.00064923)  
+ i\*(-0.0042915 +/- 0.00052978) [ 0.51]

| pi:omega                 | pi:phi                   |
|--------------------------|--------------------------|
| k_re= 0.0450 +/- 0.0014  | k_re= -0.0153 +/- 0.0013 |
| k_im= -0.0106 +/- 0.0015 | k_im= 0.0276 +/- 0.0023  |
| corr= [ 0.54]            | corr= [-0.07]            |

| pi:omega/3^S_1(*)             | pi:phi/3^S_1                 | pi:omega/3^D_1                |
|-------------------------------|------------------------------|-------------------------------|
| g = 0.1059 +/- 0.0070         | g = 0.0000 +/- 0.0000        | g = 0.0101 +/- 0.0060         |
| arg(g)/pi= -0.0782 +/- 0.0255 | arg(g)/pi= 0.5782 +/- 0.0255 | arg(g)/pi= -0.1656 +/- 0.1274 |
| g_re= 0.1027 +/- 0.0071       | g_re= -0.0000 +/- 0.0000     | g_re= 0.0088 +/- 0.0066       |
| g_im= -0.0258 +/- 0.0085      | g_im= 0.0000 +/- 0.0000      | g_im= -0.0050 +/- 0.0030      |
| corr= [ 0.06]                 | corr= [ 0.12]                | corr= [-0.07]                 |
| Br = 0.9458 +/- 0.0261        | Br = 0.0000 +/- 0.0000       | Br = 0.0086 +/- 0.0095        |

--

pi:omega[-] pi:phi[-] upper half-plane

sqrt(s)\_pole = (0.24343 +/- 0.0013185)  
+ (i/2)\*(+0.017629 +/- 0.002223) [-0.52]

s\_pole = (0.059182 +/- 0.00065243)  
+ i\*(+0.0042915 +/- 0.00052932) [-0.51]

| pi:omega                 | pi:phi                   |
|--------------------------|--------------------------|
| k_re= -0.0450 +/- 0.0014 | k_re= -0.0153 +/- 0.0013 |
| k_im= -0.0106 +/- 0.0015 | k_im= -0.0276 +/- 0.0023 |
| corr= [-0.54]            | corr= [ 0.06]            |

| pi:omega/3^S_1(*)            | pi:phi/3^S_1                 | pi:omega/3^D_1               |
|------------------------------|------------------------------|------------------------------|
| g = 0.1059 +/- 0.0070        | g = 0.0000 +/- 0.0000        | g = 0.0101 +/- 0.0060        |
| arg(g)/pi= 0.0782 +/- 0.0256 | arg(g)/pi= 0.4218 +/- 0.0256 | arg(g)/pi= 0.1657 +/- 0.1275 |
| g_re= 0.1027 +/- 0.0070      | g_re= 0.0000 +/- 0.0000      | g_re= 0.0088 +/- 0.0066      |
| g_im= 0.0258 +/- 0.0085      | g_im= 0.0000 +/- 0.0000      | g_im= 0.0050 +/- 0.0030      |
| corr= [-0.06]                | corr= [-0.12]                | corr= [ 0.07]                |



# 1 Successful Parameterizations

```

Br = 0.9458 +/- 0.0261 | Br = 0.0000 +/- 0.0000 | Br = 0.0086 +/- 0.0096 |

--
pi:omega[-] pi:phi[-] lower half-plane

sqrt(s)_pole = (0.24343 +/- 0.0013185)
               + (i/2)*(-0.017629 +/- 0.002223) [ 0.52]

s_pole = (0.059182 +/- 0.00065243)
          + i*(-0.0042915 +/- 0.00052932) [ 0.51]

=====
pi:omega | pi:phi |
=====
k_re= 0.0450 +/- 0.0014 | k_re= 0.0153 +/- 0.0013 |
k_im= -0.0106 +/- 0.0015 | k_im= -0.0276 +/- 0.0023 |
corr= [ 0.54] | corr= [-0.06] |

=====
pi:omega/3^S_1(*) | pi:phi/3^S_1 | pi:omega/3^D_1 |
=====
|g|= 0.1059 +/- 0.0070 | |g|= 0.0000 +/- 0.0000 | |g|= 0.0101 +/- 0.0060 |
arg(g)/pi= -0.0782 +/- 0.0256 | arg(g)/pi= 0.5782 +/- 0.0256 | arg(g)/pi= -0.1657 +/- 0.1275 |
-----
g_re= 0.1027 +/- 0.0070 | g_re= -0.0000 +/- 0.0000 | g_re= 0.0088 +/- 0.0066 |
g_im= -0.0258 +/- 0.0085 | g_im= 0.0000 +/- 0.0000 | g_im= -0.0050 +/- 0.0030 |
corr= [ 0.06] | corr= [ 0.12] | corr= [-0.07] |
-----
Br = 0.9458 +/- 0.0261 | Br = 0.0000 +/- 0.0000 | Br = 0.0086 +/- 0.0096 |

```



## 1.16 coupled\_po\_pp.3s1\_3d1.pole+G0\_3s1\_3sd1\_3S1.gorder0\_3s1\_3d1.threshold\_sub

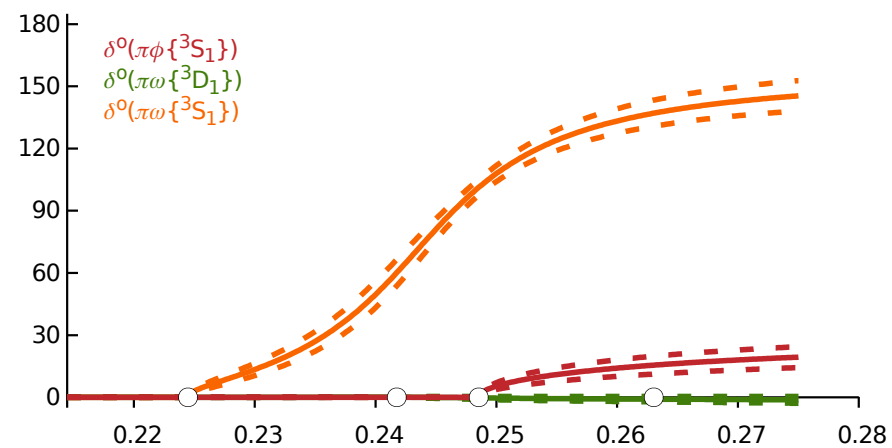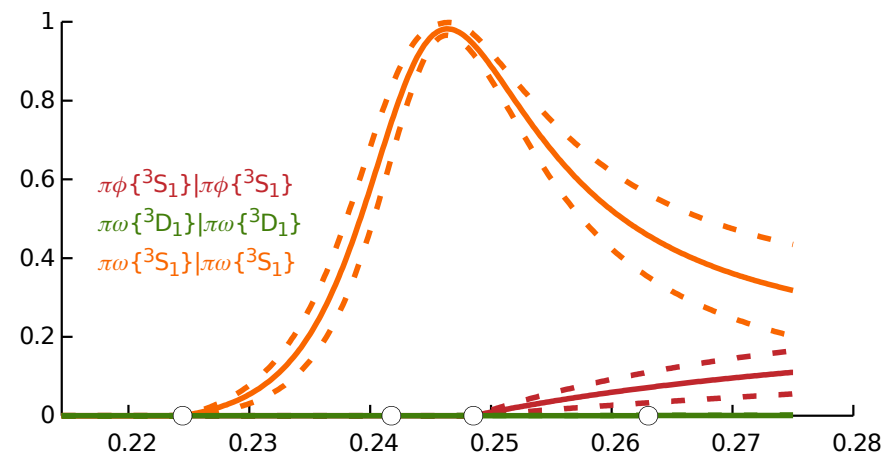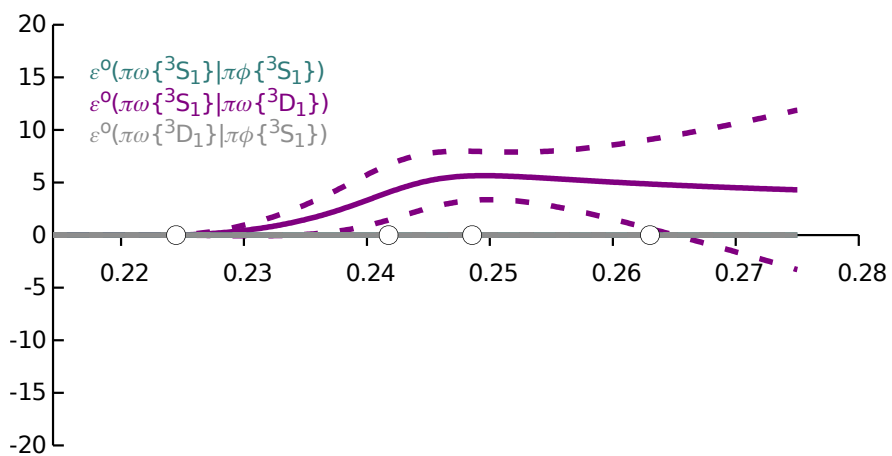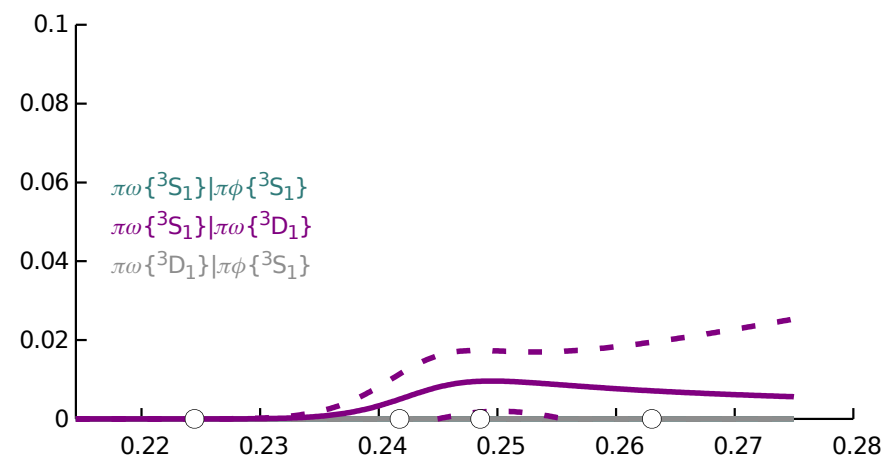



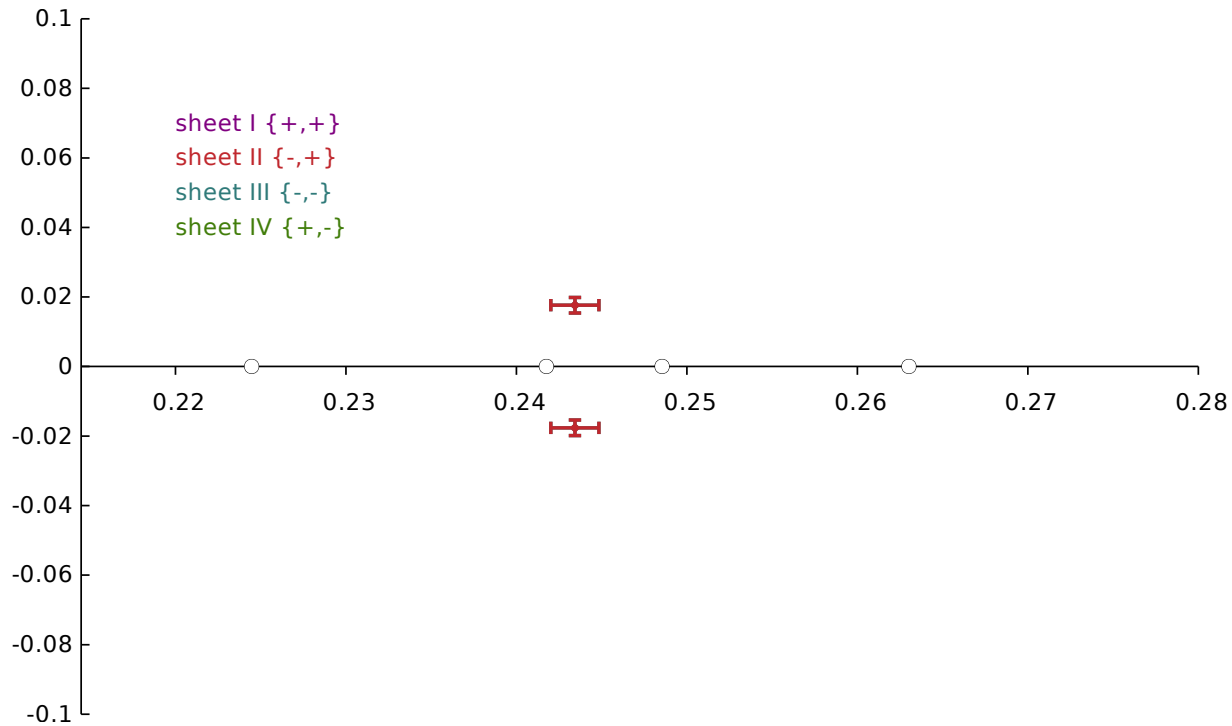

### parameter values

minimised with  $\text{chisq}/\text{nDoF} = 36.75 / (36 - 6) = 1.22$

|                                               |  |                        |  |      |      |      |       |       |       |
|-----------------------------------------------|--|------------------------|--|------|------|------|-------|-------|-------|
| JP1+_g_pi:omega/3^D_1_pole0_order0            |  | 1.1284 +/- 0.63356     |  | 1.00 | 0.70 | 0.66 | -0.22 | -0.13 | -0.45 |
| JP1+_g_pi:omega/3^S_1_pole0_order0            |  | 0.10237 +/- 0.0064041  |  |      | 1.00 | 0.32 | -0.27 | -0.01 | -0.58 |
| JP1+_gamma_pi:omega/3^S_1 pi:omega/3^D_1_orde |  | 1.5103 +/- 12.123      |  |      |      | 1.00 | 0.12  | -0.15 | -0.32 |
| JP1+_gamma_pi:omega/3^S_1 pi:omega/3^S_1_orde |  | -0.33091 +/- 0.18587   |  |      |      |      | 1.00  | 0.18  | 0.18  |
| JP1+_gamma_pi:phi/3^S_1 pi:phi/3^S_1_order0   |  | 0.98807 +/- 0.30528    |  |      |      |      |       | 1.00  | -0.20 |
| JP1+_m_pole0                                  |  | 0.24423 +/- 0.00079458 |  |      |      |      |       |       | 1.00  |

### pole singularities

pi:omega[-] pi:phi[+] upper half-plane

$\text{sqrt}(s)_{\text{pole}} = (0.24343 \pm 0.0014147)$   
 $+ (i/2)(+0.017633 \pm 0.0022466) [-0.55]$

$s_{\text{pole}} = (0.059181 \pm 0.00069996)$   
 $+ i(+0.0042923 \pm 0.00053347) [-0.54]$

|                          |                         |
|--------------------------|-------------------------|
| pi:omega                 | pi:phi                  |
| ===== =====              |                         |
| k_re= -0.0450 +/- 0.0015 | k_re= 0.0153 +/- 0.0013 |
| k_im= -0.0106 +/- 0.0015 | k_im= 0.0277 +/- 0.0024 |
| corr= [-0.59]            | corr= [ 0.01]           |



# 1 Successful Parameterizations

| pi:omega/3^S_1(*)                                                   | pi:phi/3^S_1                                                        | pi:omega/3^D_1                                                      |
|---------------------------------------------------------------------|---------------------------------------------------------------------|---------------------------------------------------------------------|
| g = 0.1059 +/- 0.0072<br>arg(g)/pi= 0.0782 +/- 0.0264               | g = 0.0000 +/- 0.0000<br>arg(g)/pi= 0.4218 +/- 0.0264               | g = 0.0101 +/- 0.0062<br>arg(g)/pi= 0.1654 +/- 0.1303               |
| g_re= 0.1028 +/- 0.0072<br>g_im= 0.0258 +/- 0.0088<br>corr= [-0.06] | g_re= 0.0000 +/- 0.0000<br>g_im= 0.0000 +/- 0.0000<br>corr= [-0.14] | g_re= 0.0088 +/- 0.0068<br>g_im= 0.0050 +/- 0.0030<br>corr= [ 0.07] |
| Br = 0.9454 +/- 0.0270                                              | Br = 0.0000 +/- 0.0000                                              | Br = 0.0086 +/- 0.0098                                              |

--  
pi:omega[-] pi:phi[+] lower half-plane

sqrt(s)\_pole = (0.24343 +/- 0.0014147)  
+ (i/2)\*(-0.017633 +/- 0.0022466) [ 0.55]

s\_pole = (0.059181 +/- 0.00069996)  
+ i\*(-0.0042923 +/- 0.00053347) [ 0.54]

| pi:omega                                                             | pi:phi                                                               |
|----------------------------------------------------------------------|----------------------------------------------------------------------|
| k_re= 0.0450 +/- 0.0015<br>k_im= -0.0106 +/- 0.0015<br>corr= [ 0.59] | k_re= -0.0153 +/- 0.0013<br>k_im= 0.0277 +/- 0.0024<br>corr= [-0.01] |

| pi:omega/3^S_1(*)                                                    | pi:phi/3^S_1                                                         | pi:omega/3^D_1                                                       |
|----------------------------------------------------------------------|----------------------------------------------------------------------|----------------------------------------------------------------------|
| g = 0.1059 +/- 0.0072<br>arg(g)/pi= -0.0782 +/- 0.0264               | g = 0.0000 +/- 0.0000<br>arg(g)/pi= 0.5782 +/- 0.0264                | g = 0.0101 +/- 0.0062<br>arg(g)/pi= -0.1654 +/- 0.1303               |
| g_re= 0.1028 +/- 0.0072<br>g_im= -0.0258 +/- 0.0088<br>corr= [ 0.06] | g_re= -0.0000 +/- 0.0000<br>g_im= 0.0000 +/- 0.0000<br>corr= [ 0.14] | g_re= 0.0088 +/- 0.0068<br>g_im= -0.0050 +/- 0.0030<br>corr= [-0.07] |
| Br = 0.9454 +/- 0.0270                                               | Br = 0.0000 +/- 0.0000                                               | Br = 0.0086 +/- 0.0098                                               |

--  
pi:omega[-] pi:phi[-] upper half-plane

sqrt(s)\_pole = (0.24343 +/- 0.0014147)  
+ (i/2)\*(+0.017633 +/- 0.0022466) [-0.55]

s\_pole = (0.059181 +/- 0.00069996)  
+ i\*(+0.0042923 +/- 0.00053347) [-0.54]

| pi:omega                                                              | pi:phi                                                                |
|-----------------------------------------------------------------------|-----------------------------------------------------------------------|
| k_re= -0.0450 +/- 0.0015<br>k_im= -0.0106 +/- 0.0015<br>corr= [-0.59] | k_re= -0.0153 +/- 0.0013<br>k_im= -0.0277 +/- 0.0024<br>corr= [ 0.01] |

| pi:omega/3^S_1(*)                                                   | pi:phi/3^S_1                                                        | pi:omega/3^D_1                                                      |
|---------------------------------------------------------------------|---------------------------------------------------------------------|---------------------------------------------------------------------|
| g = 0.1059 +/- 0.0072<br>arg(g)/pi= 0.0782 +/- 0.0264               | g = 0.0000 +/- 0.0000<br>arg(g)/pi= 0.4218 +/- 0.0264               | g = 0.0101 +/- 0.0062<br>arg(g)/pi= 0.1654 +/- 0.1303               |
| g_re= 0.1028 +/- 0.0072<br>g_im= 0.0258 +/- 0.0088<br>corr= [-0.06] | g_re= 0.0000 +/- 0.0000<br>g_im= 0.0000 +/- 0.0000<br>corr= [-0.14] | g_re= 0.0088 +/- 0.0068<br>g_im= 0.0050 +/- 0.0030<br>corr= [ 0.07] |



# 1 Successful Parameterizations

```

Br = 0.9454 +/- 0.0270 | Br = 0.0000 +/- 0.0000 | Br = 0.0086 +/- 0.0098 |

--
pi:omega[-] pi:phi[-] lower half-plane

sqrt(s)_pole = (0.24343 +/- 0.0014147)
               + (i/2)*(-0.017633 +/- 0.0022466) [ 0.55]

s_pole = (0.059181 +/- 0.00069996)
          + i*(-0.0042923 +/- 0.00053347) [ 0.54]

=====
pi:omega | pi:phi |
=====
k_re= 0.0450 +/- 0.0015 | k_re= 0.0153 +/- 0.0013 |
k_im= -0.0106 +/- 0.0015 | k_im= -0.0277 +/- 0.0024 |
corr= [ 0.59] | corr= [-0.01] |

=====
pi:omega/3^S_1(*) | pi:phi/3^S_1 | pi:omega/3^D_1 |
=====
|g|= 0.1059 +/- 0.0072 | |g|= 0.0000 +/- 0.0000 | |g|= 0.0101 +/- 0.0062 |
arg(g)/pi= -0.0782 +/- 0.0264 | arg(g)/pi= 0.5782 +/- 0.0264 | arg(g)/pi= -0.1654 +/- 0.1303 |
-----
g_re= 0.1028 +/- 0.0072 | g_re= -0.0000 +/- 0.0000 | g_re= 0.0088 +/- 0.0068 |
g_im= -0.0258 +/- 0.0088 | g_im= 0.0000 +/- 0.0000 | g_im= -0.0050 +/- 0.0030 |
corr= [ 0.06] | corr= [ 0.14] | corr= [-0.07] |
-----
Br = 0.9454 +/- 0.0270 | Br = 0.0000 +/- 0.0000 | Br = 0.0086 +/- 0.0098 |

```



## 1.17 coupled\_po\_pp.3s1\_3d1.pole+G0\_3s1\_3sd1\_3S1.gorder0\_3s1+gorder1\_3s1.irho

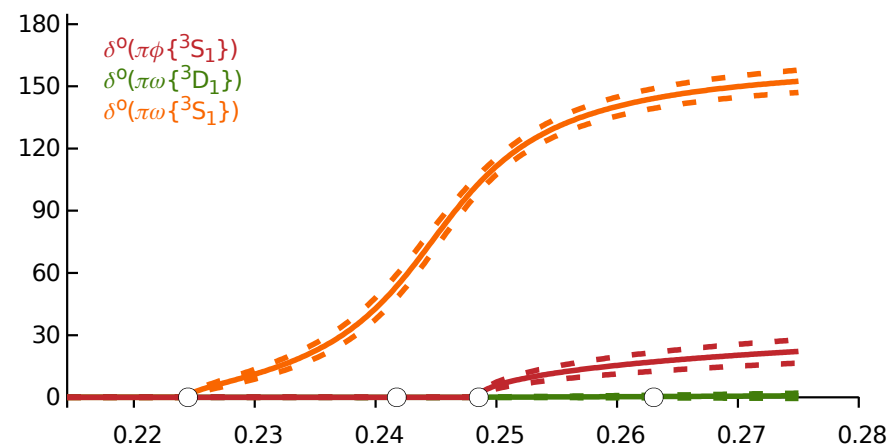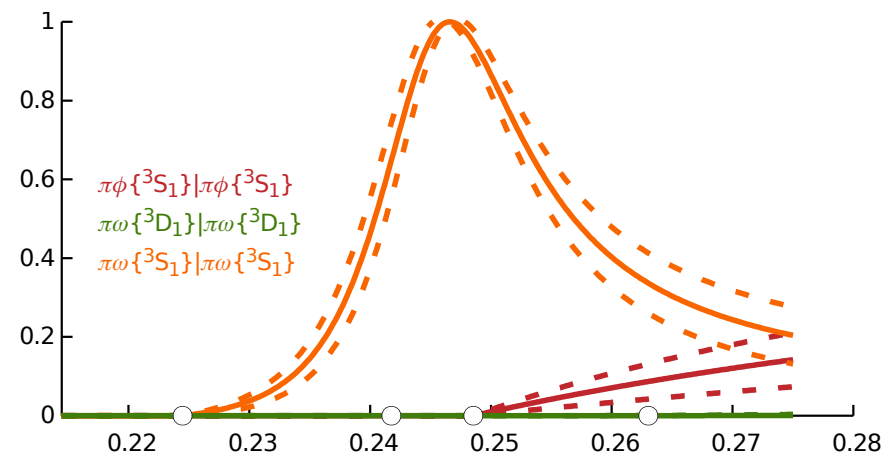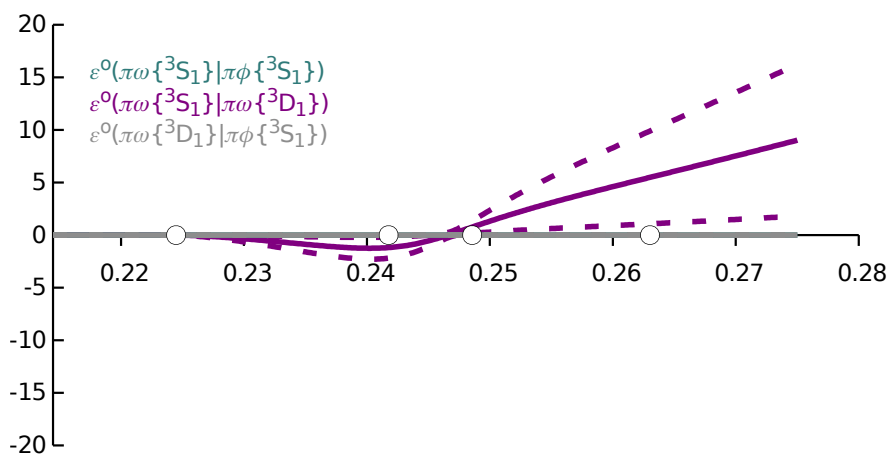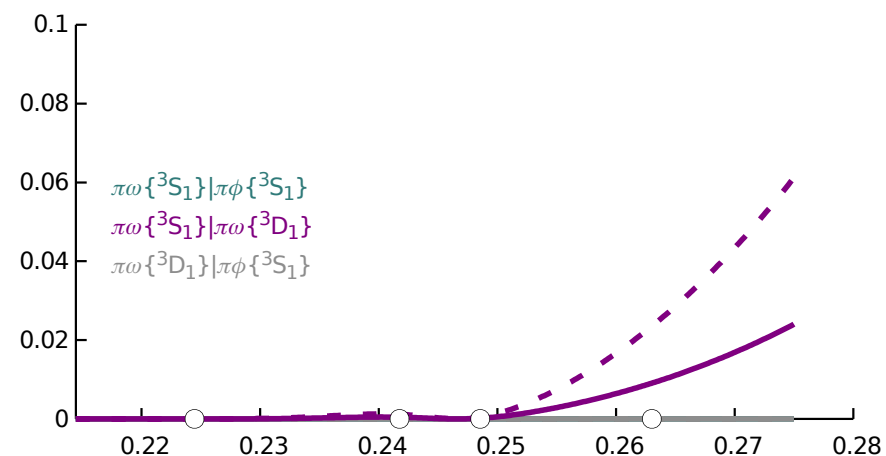



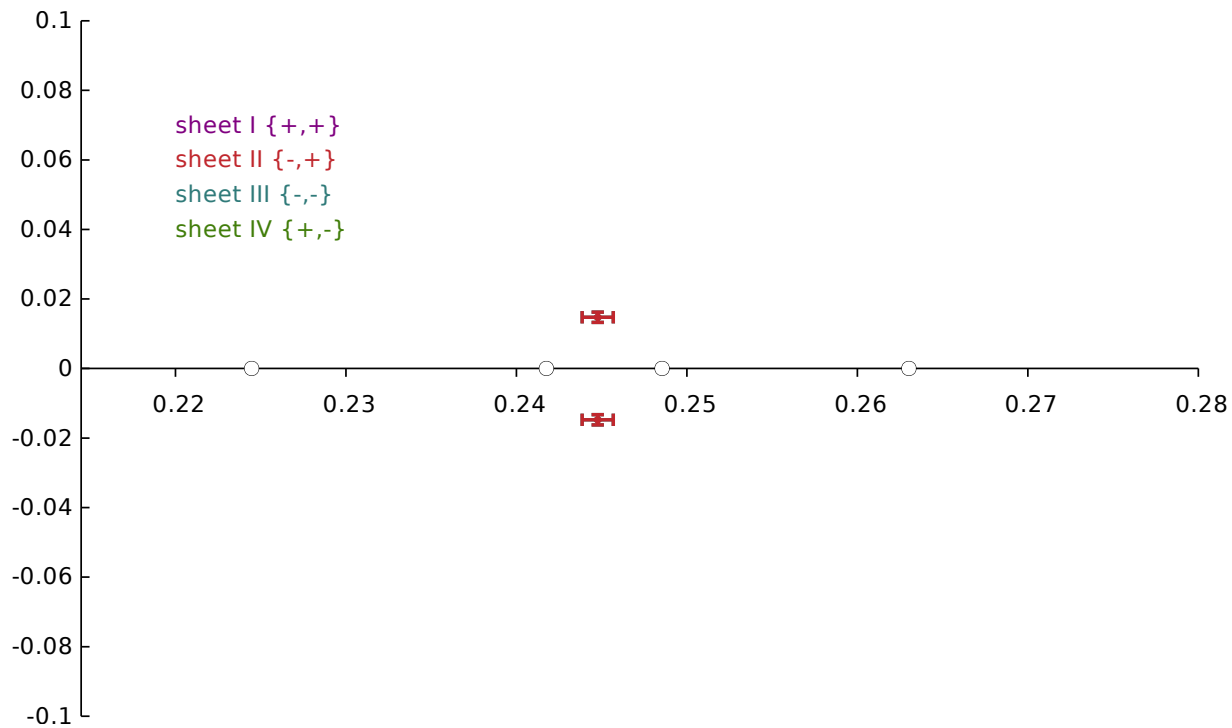

### parameter values

minimised with  $\text{chisq}/\text{nDoF} = 40.51 / (36 - 6) = 1.35$

|                                               |  |                        |  |      |       |       |       |       |       |
|-----------------------------------------------|--|------------------------|--|------|-------|-------|-------|-------|-------|
| JP1+_g_pi:omega/3^S_1_pole0_order0            |  | 0.097352 +/- 0.02161   |  | 1.00 | -0.97 | -0.01 | -0.37 | 0.01  | -0.01 |
| JP1+_g_pi:omega/3^S_1_pole0_order1            |  | 0.038015 +/- 0.35788   |  |      | 1.00  | -0.03 | 0.29  | 0.01  | -0.03 |
| JP1+_gamma_pi:omega/3^S_1 pi:omega/3^D_1_orde |  | -14.357 +/- 11.752     |  |      |       | 1.00  | 0.19  | -0.15 | -0.19 |
| JP1+_gamma_pi:omega/3^S_1 pi:omega/3^S_1_orde |  | -0.27232 +/- 0.19385   |  |      |       |       | 1.00  | 0.16  | -0.07 |
| JP1+_gamma_pi:phi/3^S_1 pi:phi/3^S_1_order0   |  | 1.0383 +/- 0.29546     |  |      |       |       |       | 1.00  | -0.28 |
| JP1+_m_pole0                                  |  | 0.24660 +/- 0.00066147 |  |      |       |       |       |       | 1.00  |

### pole singularities

pi:omega[-] pi:phi[+] upper half-plane

$\text{sqrt}(s)_{\text{pole}} = (0.24477 \pm 0.00091651)$   
 $+ (i/2)*(+0.014753 \pm 0.0014859) [-0.36]$

$s_{\text{pole}} = (0.059857 \pm 0.00045271)$   
 $+ i*(+0.003611 \pm 0.00035909) [-0.35]$

| pi:omega                 | pi:phi                  |
|--------------------------|-------------------------|
| k_re= -0.0463 +/- 0.0010 | k_re= 0.0145 +/- 0.0011 |
| k_im= -0.0087 +/- 0.0009 | k_im= 0.0246 +/- 0.0017 |
| corr= [-0.40]            | corr= [-0.07]           |



# 1 Successful Parameterizations

| pi:omega/3^S_1(*)                                                   | pi:phi/3^S_1                                                        | pi:omega/3^D_1                                                       |
|---------------------------------------------------------------------|---------------------------------------------------------------------|----------------------------------------------------------------------|
| g = 0.0973 +/- 0.0053<br>arg(g)/pi= 0.0571 +/- 0.0209               | g = 0.0000 +/- 0.0000<br>arg(g)/pi= 0.4429 +/- 0.0209               | g = 0.0048 +/- 0.0040<br>arg(g)/pi= 0.7255 +/- 0.0314                |
| g_re= 0.0958 +/- 0.0054<br>g_im= 0.0174 +/- 0.0063<br>corr= [-0.14] | g_re= 0.0000 +/- 0.0000<br>g_im= 0.0000 +/- 0.0000<br>corr= [ 0.01] | g_re= -0.0031 +/- 0.0027<br>g_im= 0.0036 +/- 0.0030<br>corr= [-0.97] |
| Br = 0.9785 +/- 0.0209                                              | Br = 0.0000 +/- 0.0000                                              | Br = 0.0024 +/- 0.0039                                               |

--

pi:omega[-] pi:phi[+] lower half-plane

sqrt(s)\_pole = (0.24477 +/- 0.00091651)  
+ (i/2)\*(-0.014753 +/- 0.0014859) [ 0.36]

s\_pole = (0.059857 +/- 0.00045271)  
+ i\*(-0.003611 +/- 0.00035909) [ 0.35]

| pi:omega                                                             | pi:phi                                                               |
|----------------------------------------------------------------------|----------------------------------------------------------------------|
| k_re= 0.0463 +/- 0.0010<br>k_im= -0.0087 +/- 0.0009<br>corr= [ 0.40] | k_re= -0.0145 +/- 0.0011<br>k_im= 0.0246 +/- 0.0017<br>corr= [ 0.07] |

| pi:omega/3^S_1(*)                                                    | pi:phi/3^S_1                                                         | pi:omega/3^D_1                                                        |
|----------------------------------------------------------------------|----------------------------------------------------------------------|-----------------------------------------------------------------------|
| g = 0.0973 +/- 0.0053<br>arg(g)/pi= -0.0571 +/- 0.0209               | g = 0.0000 +/- 0.0000<br>arg(g)/pi= 0.5571 +/- 0.0209                | g = 0.0048 +/- 0.0040<br>arg(g)/pi= -0.7255 +/- 0.0314                |
| g_re= 0.0958 +/- 0.0054<br>g_im= -0.0174 +/- 0.0063<br>corr= [ 0.14] | g_re= -0.0000 +/- 0.0000<br>g_im= 0.0000 +/- 0.0000<br>corr= [-0.01] | g_re= -0.0031 +/- 0.0027<br>g_im= -0.0036 +/- 0.0030<br>corr= [ 0.97] |
| Br = 0.9785 +/- 0.0209                                               | Br = 0.0000 +/- 0.0000                                               | Br = 0.0024 +/- 0.0039                                                |

--

pi:omega[-] pi:phi[-] upper half-plane

sqrt(s)\_pole = (0.24477 +/- 0.00091651)  
+ (i/2)\*(+0.014753 +/- 0.0014859) [-0.36]

s\_pole = (0.059857 +/- 0.00045271)  
+ i\*(+0.003611 +/- 0.00035909) [-0.35]

| pi:omega                                                              | pi:phi                                                                |
|-----------------------------------------------------------------------|-----------------------------------------------------------------------|
| k_re= -0.0463 +/- 0.0010<br>k_im= -0.0087 +/- 0.0009<br>corr= [-0.40] | k_re= -0.0145 +/- 0.0011<br>k_im= -0.0246 +/- 0.0017<br>corr= [-0.07] |

| pi:omega/3^S_1(*)                                                   | pi:phi/3^S_1                                                        | pi:omega/3^D_1                                                       |
|---------------------------------------------------------------------|---------------------------------------------------------------------|----------------------------------------------------------------------|
| g = 0.0973 +/- 0.0053<br>arg(g)/pi= 0.0571 +/- 0.0209               | g = 0.0000 +/- 0.0000<br>arg(g)/pi= 0.4429 +/- 0.0209               | g = 0.0048 +/- 0.0040<br>arg(g)/pi= 0.7255 +/- 0.0314                |
| g_re= 0.0958 +/- 0.0054<br>g_im= 0.0174 +/- 0.0063<br>corr= [-0.14] | g_re= 0.0000 +/- 0.0000<br>g_im= 0.0000 +/- 0.0000<br>corr= [ 0.01] | g_re= -0.0031 +/- 0.0027<br>g_im= 0.0036 +/- 0.0030<br>corr= [-0.97] |



# 1 Successful Parameterizations

```

Br = 0.9785 +/- 0.0209 | Br = 0.0000 +/- 0.0000 | Br = 0.0024 +/- 0.0039 |

--
pi:omega[-] pi:phi[-] lower half-plane

sqrt(s)_pole = (0.24477 +/- 0.00091651)
               + (i/2)*(-0.014753 +/- 0.0014859) [ 0.36]

s_pole = (0.059857 +/- 0.00045271)
          + i*(-0.003611 +/- 0.00035909) [ 0.35]

=====
pi:omega | pi:phi |
=====
k_re= 0.0463 +/- 0.0010 | k_re= 0.0145 +/- 0.0011 |
k_im= -0.0087 +/- 0.0009 | k_im= -0.0246 +/- 0.0017 |
corr= [ 0.40] | corr= [ 0.07] |

=====
pi:omega/3^S_1(*) | pi:phi/3^S_1 | pi:omega/3^D_1 |
=====
|g|= 0.0973 +/- 0.0053 | |g|= 0.0000 +/- 0.0000 | |g|= 0.0048 +/- 0.0040 |
arg(g)/pi= -0.0571 +/- 0.0209 | arg(g)/pi= 0.5571 +/- 0.0209 | arg(g)/pi= -0.7255 +/- 0.0314 |
-----
g_re= 0.0958 +/- 0.0054 | g_re= -0.0000 +/- 0.0000 | g_re= -0.0031 +/- 0.0027 |
g_im= -0.0174 +/- 0.0063 | g_im= 0.0000 +/- 0.0000 | g_im= -0.0036 +/- 0.0030 |
corr= [ 0.14] | corr= [-0.01] | corr= [ 0.97] |
-----
Br = 0.9785 +/- 0.0209 | Br = 0.0000 +/- 0.0000 | Br = 0.0024 +/- 0.0039 |

```



## 1.18 coupled\_po\_pp.3s1\_3d1.pole+G0\_3s1\_3sd1\_3S1.gorder0\_3s1+gorder1\_3s1.pole0\_sub

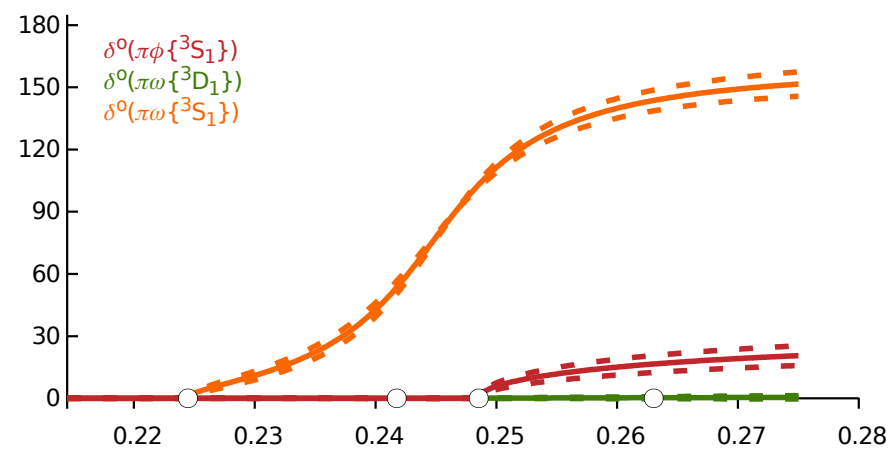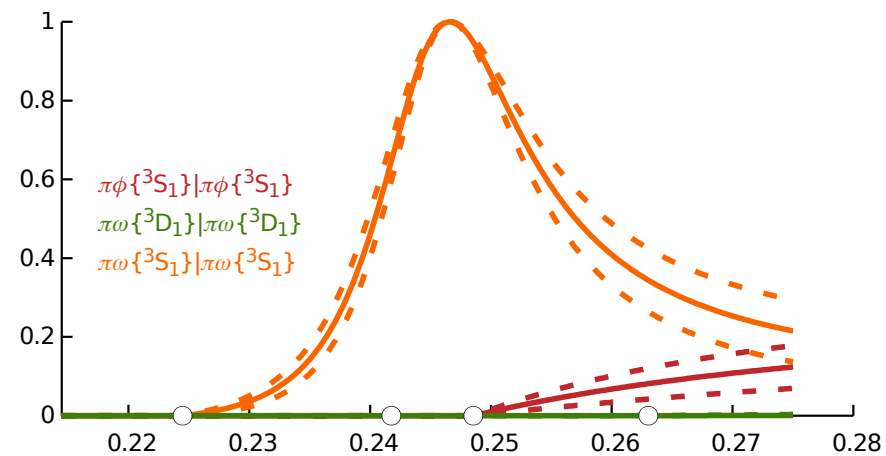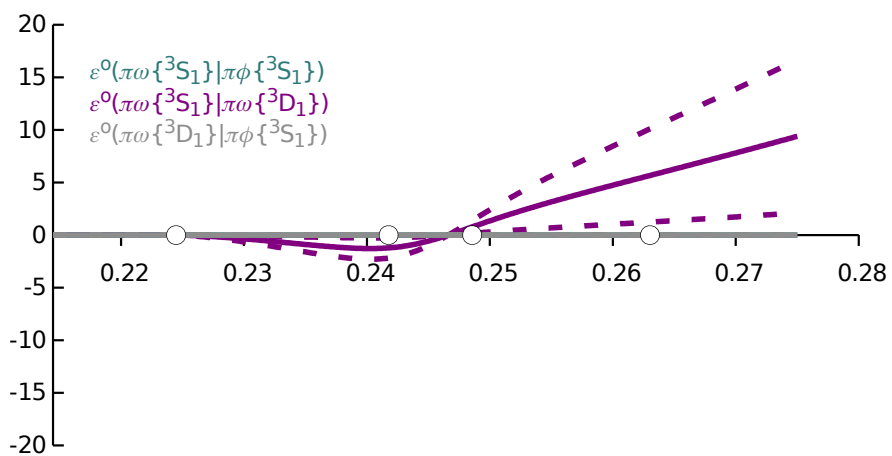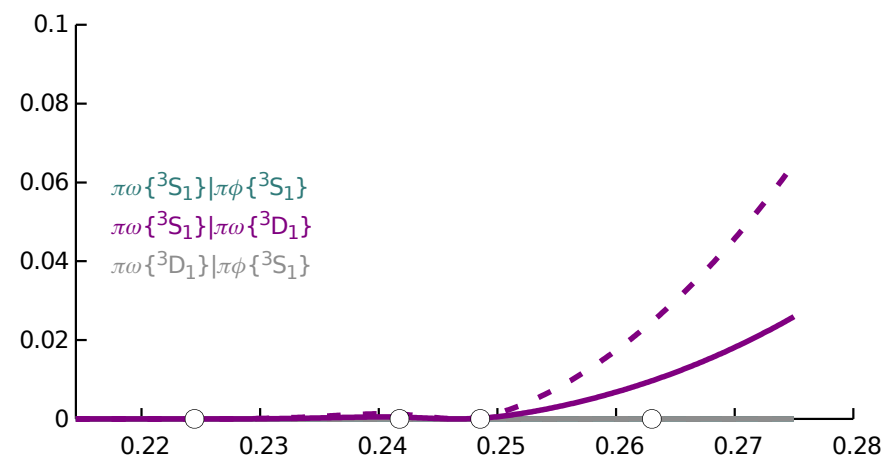



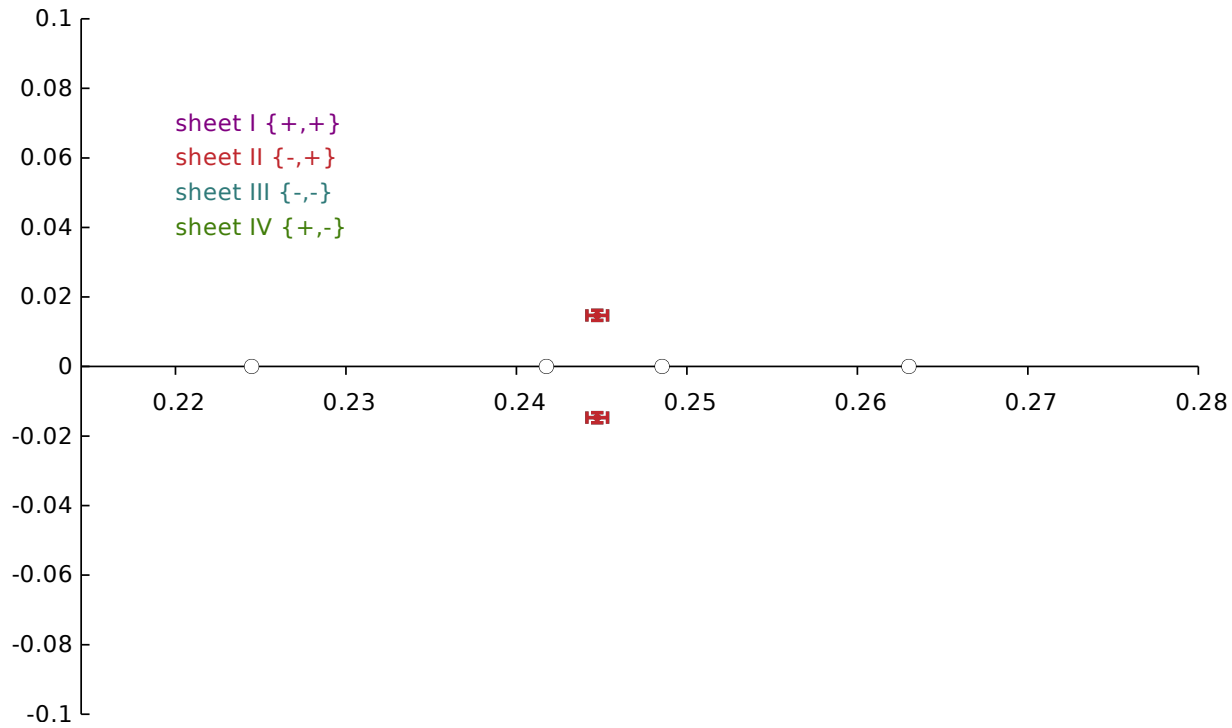

### parameter values

```

minimised with chisq/nDoF = 40.52 / (36 - 6) = 1.35
=====
JP1+_g_pi:omega/3^S_1_pole0_order0 | 0.095682 +/- 0.040029 | 1.00 -0.99 -0.00 -0.62 0.00 0.00
JP1+_g_pi:omega/3^S_1_pole0_order1 | 0.00023770 +/- 0.65955 | 1.00 -0.02 0.59 -0.00 -0.00
JP1+_gamma_pi:omega/3^S_1|pi:omega/3^D_1_orde | -13.559 +/- 10.747 | 1.00 0.16 -0.20 -0.01
JP1+_gamma_pi:omega/3^S_1|pi:omega/3^S_1_orde | -0.25801 +/- 0.20352 | 1.00 0.13 -0.00
JP1+_gamma_pi:phi/3^S_1|pi:phi/3^S_1_order0 | 0.95604 +/- 0.24245 | 1.00 -0.01
JP1+_m_pole0 | 0.24661 +/- 2.161e-05 | 1.00
=====

```

### pole singularities

pi:omega[+] pi:phi[-] lower half-plane

```

sqrt(s)_pole = (0.18996 +/- 0.023288)
               + (i/2)*(-1.478e-14 +/- 7.3905e-12) [ 0.00]

```

```

s_pole = (0.036087 +/- 0.0088419)
         + i*(-2.8062e-15 +/- 1.4032e-12) [ 0.00]

```

```

=====
pi:omega | pi:phi |
=====
k_re= -0.0000 +/- 0.0000 | k_re= 0.0000 +/- 0.0000 |
k_im= 0.0532 +/- 0.0147 | k_im= -0.0652 +/- 0.0071 |
corr= [ 0.00] | corr= [ 0.00] |
=====

```



# 1 Successful Parameterizations

| pi:omega/3^S_1               | pi:phi/3^S_1(*)              | pi:omega/3^D_1               |
|------------------------------|------------------------------|------------------------------|
| =====                        | =====                        | =====                        |
| g = 0.0000 +/- 0.0000        | g = 0.1837 +/- 0.0018        | g = 0.0000 +/- 0.0000        |
| arg(g)/pi= 0.0000 +/- 0.0000 | arg(g)/pi= 0.5000 +/- 0.0000 | arg(g)/pi= 0.0000 +/- 0.0000 |
| -----                        | -----                        | -----                        |
| g_re= 0.0000 +/- 0.0000      | g_re= 0.0000 +/- 0.0000      | g_re= 0.0000 +/- 0.0000      |
| g_im= 0.0000 +/- 0.0000      | g_im= 0.1837 +/- 0.0018      | g_im= 0.0000 +/- 0.0000      |
| corr= [ 0.00]                | corr= [-1.00]                | corr= [ 0.00]                |
| -----                        | -----                        | -----                        |
| Br = 0.0000 +/- 0.0000       | Br = 0.0000 +/- 0.0000       | Br = 0.0000 +/- 0.0000       |

--

pi:omega[-] pi:phi[+] upper half-plane

sqrt(s)\_pole = (0.24474 +/- 0.00060418)  
+ (i/2)\*(+0.014715 +/- 0.0014647) [-0.39]

s\_pole = (0.059843 +/- 0.00030013)  
+ i\*(+0.0036013 +/- 0.00035508) [-0.40]

| pi:omega                 | pi:phi                  |
|--------------------------|-------------------------|
| =====                    | =====                   |
| k_re= -0.0463 +/- 0.0007 | k_re= 0.0145 +/- 0.0010 |
| k_im= -0.0087 +/- 0.0009 | k_im= 0.0246 +/- 0.0013 |
| corr= [-0.33]            | corr= [ 0.33]           |

| pi:omega/3^S_1(*)            | pi:phi/3^S_1                 | pi:omega/3^D_1               |
|------------------------------|------------------------------|------------------------------|
| =====                        | =====                        | =====                        |
| g = 0.0971 +/- 0.0052        | g = 0.0000 +/- 0.0000        | g = 0.0049 +/- 0.0039        |
| arg(g)/pi= 0.0587 +/- 0.0215 | arg(g)/pi= 0.4413 +/- 0.0215 | arg(g)/pi= 0.7288 +/- 0.0323 |
| -----                        | -----                        | -----                        |
| g_re= 0.0955 +/- 0.0053      | g_re= 0.0000 +/- 0.0000      | g_re= -0.0032 +/- 0.0027     |
| g_im= 0.0178 +/- 0.0064      | g_im= 0.0000 +/- 0.0000      | g_im= 0.0037 +/- 0.0029      |
| corr= [-0.19]                | corr= [ 0.02]                | corr= [-0.97]                |
| -----                        | -----                        | -----                        |
| Br = 0.9758 +/- 0.0108       | Br = 0.0000 +/- 0.0000       | Br = 0.0025 +/- 0.0039       |

--

pi:omega[-] pi:phi[+] lower half-plane

sqrt(s)\_pole = (0.24474 +/- 0.00060418)  
+ (i/2)\*(-0.014715 +/- 0.0014647) [ 0.39]

s\_pole = (0.059843 +/- 0.00030013)  
+ i\*(-0.0036013 +/- 0.00035508) [ 0.40]

| pi:omega                 | pi:phi                   |
|--------------------------|--------------------------|
| =====                    | =====                    |
| k_re= 0.0463 +/- 0.0007  | k_re= -0.0145 +/- 0.0010 |
| k_im= -0.0087 +/- 0.0009 | k_im= 0.0246 +/- 0.0013  |
| corr= [ 0.33]            | corr= [-0.33]            |

| pi:omega/3^S_1(*)             | pi:phi/3^S_1                 | pi:omega/3^D_1                |
|-------------------------------|------------------------------|-------------------------------|
| =====                         | =====                        | =====                         |
| g = 0.0971 +/- 0.0052         | g = 0.0000 +/- 0.0000        | g = 0.0049 +/- 0.0039         |
| arg(g)/pi= -0.0587 +/- 0.0215 | arg(g)/pi= 0.5587 +/- 0.0215 | arg(g)/pi= -0.7288 +/- 0.0323 |
| -----                         | -----                        | -----                         |
| g_re= 0.0955 +/- 0.0053       | g_re= -0.0000 +/- 0.0000     | g_re= -0.0032 +/- 0.0027      |
| g_im= -0.0178 +/- 0.0064      | g_im= 0.0000 +/- 0.0000      | g_im= -0.0037 +/- 0.0029      |
| corr= [ 0.19]                 | corr= [-0.02]                | corr= [ 0.97]                 |
| -----                         | -----                        | -----                         |



## 1 Successful Parameterizations

```
Br = 0.9758 +/- 0.0108 | Br = 0.0000 +/- 0.0000 | Br = 0.0025 +/- 0.0039 |

--
pi:omega[-] pi:phi[-] upper half-plane

sqrt(s)_pole = (0.18996 +/- 0.023288)
+ (i/2)*(+2.3412e-12 +/- 1.1696e-09) [-0.00]

s_pole = (0.036087 +/- 0.0088419)
+ i*(+4.445e-13 +/- 2.2205e-10) [-0.00]

=====
pi:omega | pi:phi |
=====
k_re= -0.0000 +/- 0.0000 | k_re= -0.0000 +/- 0.0000 |
k_im= -0.0532 +/- 0.0147 | k_im= -0.0652 +/- 0.0071 |
corr= [ 0.01] | corr= [ 0.01] |

=====
pi:omega/3^S_1 | pi:phi/3^S_1(*) | pi:omega/3^D_1 |
=====
|g|= 0.0000 +/- 0.0000 | |g|= 0.1837 +/- 0.0018 | |g|= 0.0000 +/- 0.0000 |
arg(g)/pi= 0.0000 +/- 0.0000 | arg(g)/pi= 0.5000 +/- 0.0000 | arg(g)/pi= 0.0000 +/- 0.0000 |
-----
g_re= 0.0000 +/- 0.0000 | g_re= 0.0000 +/- 0.0000 | g_re= 0.0000 +/- 0.0000 |
g_im= 0.0000 +/- 0.0000 | g_im= 0.1837 +/- 0.0018 | g_im= 0.0000 +/- 0.0000 |
corr= [ 0.00] | corr= [-1.00] | corr= [ 0.00] |
-----
Br = 0.0000 +/- 0.0000 | Br = 0.0000 +/- 0.0000 | Br = 0.0000 +/- 0.0000 |

--
pi:omega[-] pi:phi[-] upper half-plane

sqrt(s)_pole = (0.24474 +/- 0.00060865)
+ (i/2)*(+0.014715 +/- 0.0014686) [-0.40]

s_pole = (0.059844 +/- 0.00030242)
+ i*(+0.0036013 +/- 0.00035592) [-0.41]

=====
pi:omega | pi:phi |
=====
k_re= -0.0463 +/- 0.0007 | k_re= -0.0145 +/- 0.0010 |
k_im= -0.0087 +/- 0.0009 | k_im= -0.0246 +/- 0.0013 |
corr= [-0.34] | corr= [ 0.33] |

=====
pi:omega/3^S_1(*) | pi:phi/3^S_1 | pi:omega/3^D_1 |
=====
|g|= 0.0971 +/- 0.0052 | |g|= 0.0000 +/- 0.0000 | |g|= 0.0049 +/- 0.0039 |
arg(g)/pi= 0.0587 +/- 0.0215 | arg(g)/pi= 0.4413 +/- 0.0215 | arg(g)/pi= 0.7287 +/- 0.0325 |
-----
g_re= 0.0955 +/- 0.0053 | g_re= 0.0000 +/- 0.0000 | g_re= -0.0032 +/- 0.0027 |
g_im= 0.0178 +/- 0.0064 | g_im= 0.0000 +/- 0.0000 | g_im= 0.0037 +/- 0.0029 |
corr= [-0.18] | corr= [ 0.01] | corr= [-0.97] |
-----
Br = 0.9758 +/- 0.0108 | Br = 0.0000 +/- 0.0000 | Br = 0.0025 +/- 0.0039 |

--
pi:omega[-] pi:phi[-] lower half-plane

sqrt(s)_pole = (0.24474 +/- 0.00060865)
+ (i/2)*(-0.014715 +/- 0.0014686) [ 0.40]

s_pole = (0.059844 +/- 0.00030242)
+ i*(-0.0036013 +/- 0.00035592) [ 0.41]
```



# 1 Successful Parameterizations

| pi:omega |                    | pi:phi |                    |
|----------|--------------------|--------|--------------------|
| =====    |                    | =====  |                    |
| k_re=    | 0.0463 +/- 0.0007  | k_re=  | 0.0145 +/- 0.0010  |
| k_im=    | -0.0087 +/- 0.0009 | k_im=  | -0.0246 +/- 0.0013 |
| corr=    | [ 0.34]            | corr=  | [-0.33]            |

  

| pi:omega/3^S_1(*) |                    | pi:phi/3^S_1 |                    | pi:omega/3^D_1 |                    |
|-------------------|--------------------|--------------|--------------------|----------------|--------------------|
| =====             |                    | =====        |                    | =====          |                    |
| g =               | 0.0971 +/- 0.0052  | g =          | 0.0000 +/- 0.0000  | g =            | 0.0049 +/- 0.0039  |
| arg(g)/pi=        | -0.0587 +/- 0.0215 | arg(g)/pi=   | 0.5587 +/- 0.0215  | arg(g)/pi=     | -0.7287 +/- 0.0325 |
| -----             |                    | -----        |                    | -----          |                    |
| g_re=             | 0.0955 +/- 0.0053  | g_re=        | -0.0000 +/- 0.0000 | g_re=          | -0.0032 +/- 0.0027 |
| g_im=             | -0.0178 +/- 0.0064 | g_im=        | 0.0000 +/- 0.0000  | g_im=          | -0.0037 +/- 0.0029 |
| corr=             | [ 0.18]            | corr=        | [-0.01]            | corr=          | [ 0.97]            |
| -----             |                    | -----        |                    | -----          |                    |
| Br =              | 0.9758 +/- 0.0108  | Br =         | 0.0000 +/- 0.0000  | Br =           | 0.0025 +/- 0.0039  |



## 1.19 coupled\_po\_pp.3s1\_3d1.pole+G0\_3s1\_3sd1\_3S1.gorder0\_3s1.irho

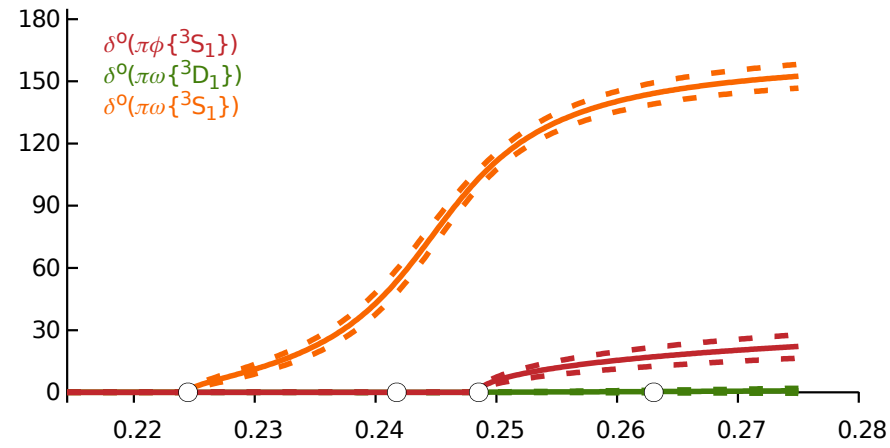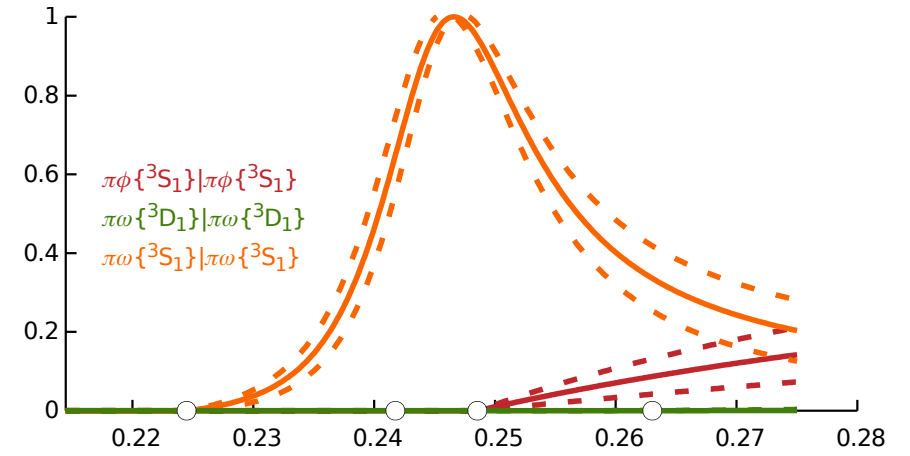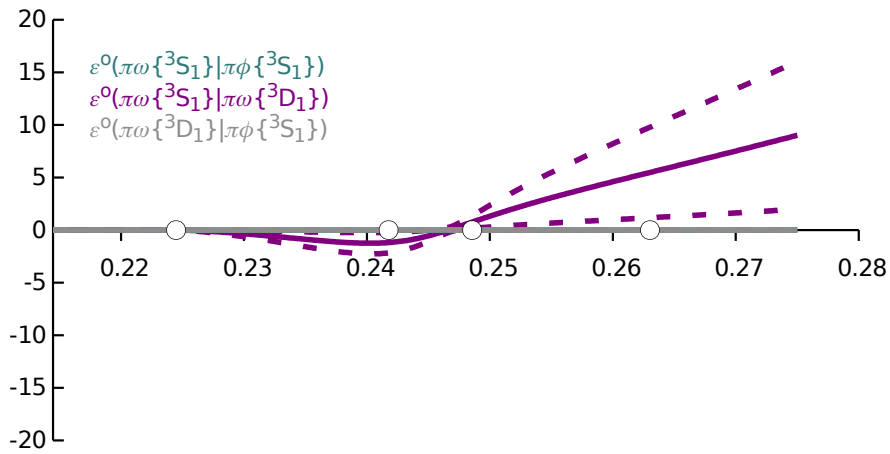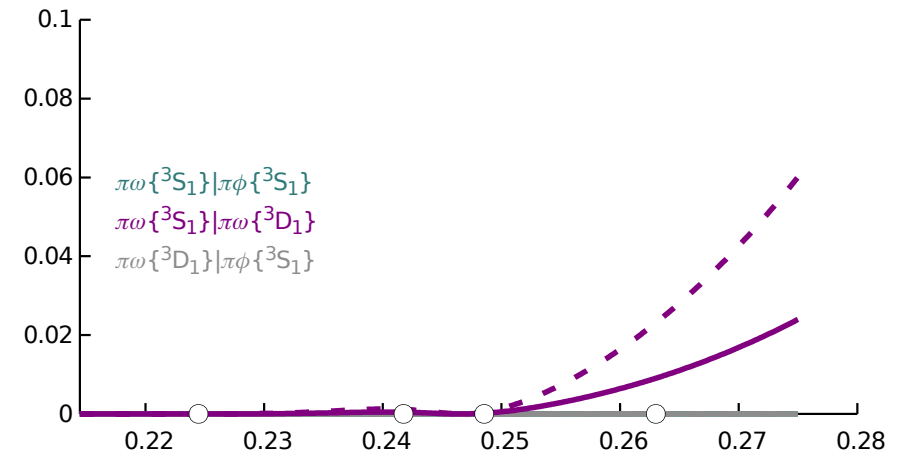



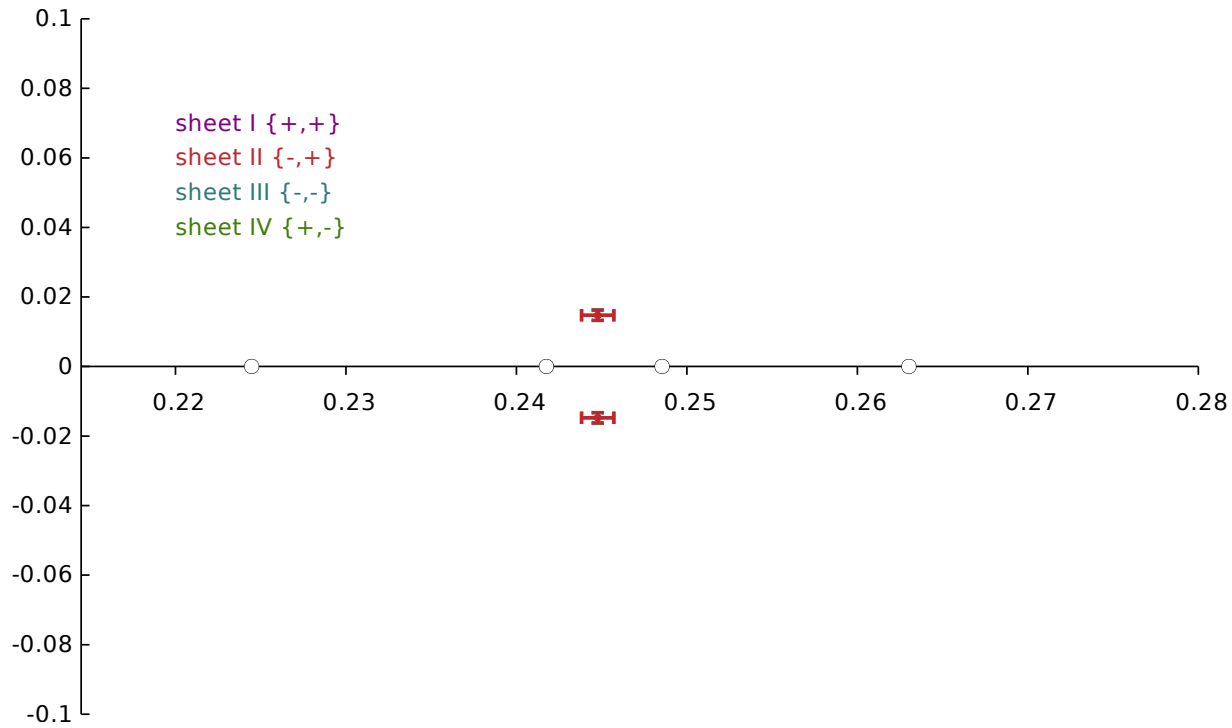

### parameter values

minimised with  $\text{chisq}/\text{nDoF} = 40.51 / (36 - 5) = 1.31$

|                                               |  |                        |  |      |       |       |       |       |
|-----------------------------------------------|--|------------------------|--|------|-------|-------|-------|-------|
| JP1+_g_pi:omega/3^S_1_pole0_order0            |  | 0.099630 +/- 0.005526  |  | 1.00 | -0.14 | -0.37 | 0.04  | -0.16 |
| JP1+_gamma_pi:omega/3^S_1 pi:omega/3^D_1_orde |  | -14.336 +/- 11.746     |  |      | 1.00  | 0.20  | -0.15 | -0.19 |
| JP1+_gamma_pi:omega/3^S_1 pi:omega/3^S_1_orde |  | -0.27893 +/- 0.1857    |  |      |       | 1.00  | 0.16  | -0.06 |
| JP1+_gamma_pi:phi/3^S_1 pi:phi/3^S_1_order0   |  | 1.0387 +/- 0.29552     |  |      |       |       | 1.00  | -0.28 |
| JP1+_m_pole0                                  |  | 0.24660 +/- 0.00066129 |  |      |       |       |       | 1.00  |

### pole singularities

pi:omega[-] pi:phi[+] upper half-plane

$\text{s\_pole} = (0.24477 \pm 0.00093997)$   
 $+ (i/2) * (0.014746 \pm 0.001489) [-0.37]$

$\text{s\_pole} = (0.059859 \pm 0.00046435)$   
 $+ i * (0.0036095 \pm 0.00035953) [-0.36]$

| pi:omega                 | pi:phi                  |
|--------------------------|-------------------------|
| ===== =====              |                         |
| k_re= -0.0463 +/- 0.0010 | k_re= 0.0145 +/- 0.0011 |
| k_im= -0.0087 +/- 0.0009 | k_im= 0.0246 +/- 0.0017 |
| corr= [-0.41]            | corr= [-0.09]           |



# 1 Successful Parameterizations

| pi:omega/3^S_1(*)            |                              | pi:phi/3^S_1                 |  | pi:omega/3^D_1 |  |
|------------------------------|------------------------------|------------------------------|--|----------------|--|
| g = 0.0973 +/- 0.0053        | g = 0.0000 +/- 0.0000        | g = 0.0048 +/- 0.0038        |  |                |  |
| arg(g)/pi= 0.0570 +/- 0.0220 | arg(g)/pi= 0.4430 +/- 0.0220 | arg(g)/pi= 0.7253 +/- 0.0332 |  |                |  |
| g_re= 0.0958 +/- 0.0054      | g_re= 0.0000 +/- 0.0000      | g_re= -0.0031 +/- 0.0025     |  |                |  |
| g_im= 0.0173 +/- 0.0066      | g_im= 0.0000 +/- 0.0000      | g_im= 0.0036 +/- 0.0029      |  |                |  |
| corr= [-0.11]                | corr= [-0.05]                | corr= [-0.97]                |  |                |  |
| Br = 0.9797 +/- 0.0208       | Br = 0.0000 +/- 0.0000       | Br = 0.0024 +/- 0.0038       |  |                |  |

--

pi:omega[-] pi:phi[+] lower half-plane

sqrt(s)\_pole = (0.24477 +/- 0.00093997)  
+ (i/2)\*(-0.014746 +/- 0.001489) [ 0.37]

s\_pole = (0.059859 +/- 0.00046435)  
+ i\*(-0.0036095 +/- 0.00035953) [ 0.36]

| pi:omega                 |                          | pi:phi |  |
|--------------------------|--------------------------|--------|--|
| k_re= 0.0463 +/- 0.0010  | k_re= -0.0145 +/- 0.0011 |        |  |
| k_im= -0.0087 +/- 0.0009 | k_im= 0.0246 +/- 0.0017  |        |  |
| corr= [ 0.41]            | corr= [ 0.09]            |        |  |

| pi:omega/3^S_1(*)             |                              | pi:phi/3^S_1                  |  | pi:omega/3^D_1 |  |
|-------------------------------|------------------------------|-------------------------------|--|----------------|--|
| g = 0.0973 +/- 0.0053         | g = 0.0000 +/- 0.0000        | g = 0.0048 +/- 0.0038         |  |                |  |
| arg(g)/pi= -0.0570 +/- 0.0220 | arg(g)/pi= 0.5570 +/- 0.0220 | arg(g)/pi= -0.7253 +/- 0.0332 |  |                |  |
| g_re= 0.0958 +/- 0.0054       | g_re= -0.0000 +/- 0.0000     | g_re= -0.0031 +/- 0.0025      |  |                |  |
| g_im= -0.0173 +/- 0.0066      | g_im= 0.0000 +/- 0.0000      | g_im= -0.0036 +/- 0.0029      |  |                |  |
| corr= [ 0.11]                 | corr= [ 0.05]                | corr= [ 0.97]                 |  |                |  |
| Br = 0.9797 +/- 0.0208        | Br = 0.0000 +/- 0.0000       | Br = 0.0024 +/- 0.0038        |  |                |  |

--

pi:omega[-] pi:phi[-] upper half-plane

sqrt(s)\_pole = (0.24477 +/- 0.00094871)  
+ (i/2)\*(+0.014746 +/- 0.001502) [-0.38]

s\_pole = (0.059859 +/- 0.00046877)  
+ i\*(+0.0036095 +/- 0.00036253) [-0.37]

| pi:omega                 |                          | pi:phi |  |
|--------------------------|--------------------------|--------|--|
| k_re= -0.0463 +/- 0.0011 | k_re= -0.0145 +/- 0.0011 |        |  |
| k_im= -0.0087 +/- 0.0009 | k_im= -0.0246 +/- 0.0017 |        |  |
| corr= [-0.42]            | corr= [-0.08]            |        |  |

| pi:omega/3^S_1(*)            |                              | pi:phi/3^S_1                 |  | pi:omega/3^D_1 |  |
|------------------------------|------------------------------|------------------------------|--|----------------|--|
| g = 0.0973 +/- 0.0053        | g = 0.0000 +/- 0.0000        | g = 0.0048 +/- 0.0039        |  |                |  |
| arg(g)/pi= 0.0570 +/- 0.0221 | arg(g)/pi= 0.4430 +/- 0.0221 | arg(g)/pi= 0.7253 +/- 0.0337 |  |                |  |
| g_re= 0.0958 +/- 0.0054      | g_re= 0.0000 +/- 0.0000      | g_re= -0.0031 +/- 0.0026     |  |                |  |
| g_im= 0.0173 +/- 0.0067      | g_im= 0.0000 +/- 0.0000      | g_im= 0.0036 +/- 0.0029      |  |                |  |
| corr= [-0.10]                | corr= [-0.07]                | corr= [-0.97]                |  |                |  |
| Br = 0.9797 +/- 0.0210       | Br = 0.0000 +/- 0.0000       | Br = 0.0024 +/- 0.0038       |  |                |  |



```
--
pi:omega[-] pi:phi[-] lower half-plane

sqrt(s)_pole = (0.24477 +/- 0.00094871)
               + (i/2)*(-0.014746 +/- 0.001502) [ 0.38]

s_pole = (0.059859 +/- 0.00046877)
         + i*(-0.0036095 +/- 0.00036253) [ 0.37]
```

| pi:omega                 | pi:phi                   |
|--------------------------|--------------------------|
| =====                    | =====                    |
| k_re= 0.0463 +/- 0.0011  | k_re= 0.0145 +/- 0.0011  |
| k_im= -0.0087 +/- 0.0009 | k_im= -0.0246 +/- 0.0017 |
| corr= [ 0.42]            | corr= [ 0.08]            |

  

| pi:omega/3^S_1(*)             | pi:phi/3^S_1                 | pi:omega/3^D_1                |
|-------------------------------|------------------------------|-------------------------------|
| =====                         | =====                        | =====                         |
| g = 0.0973 +/- 0.0053         | g = 0.0000 +/- 0.0000        | g = 0.0048 +/- 0.0039         |
| arg(g)/pi= -0.0570 +/- 0.0221 | arg(g)/pi= 0.5570 +/- 0.0221 | arg(g)/pi= -0.7253 +/- 0.0337 |
| -----                         | -----                        | -----                         |
| g_re= 0.0958 +/- 0.0054       | g_re= -0.0000 +/- 0.0000     | g_re= -0.0031 +/- 0.0026      |
| g_im= -0.0173 +/- 0.0067      | g_im= 0.0000 +/- 0.0000      | g_im= -0.0036 +/- 0.0029      |
| corr= [ 0.10]                 | corr= [ 0.07]                | corr= [ 0.97]                 |
| -----                         | -----                        | -----                         |
| Br = 0.9797 +/- 0.0210        | Br = 0.0000 +/- 0.0000       | Br = 0.0024 +/- 0.0038        |



## 1.20 coupled\_po\_pp.3s1\_3d1.pole+G0\_3s1\_3sd1\_3S1.gorder0\_3s1.pole0\_sub

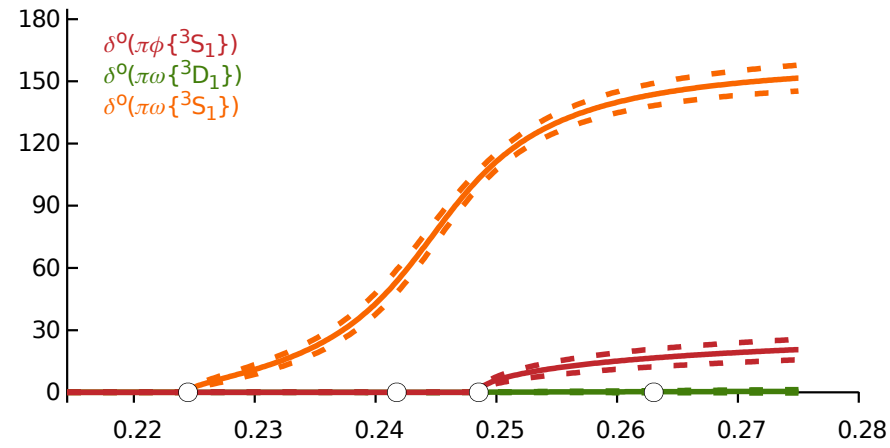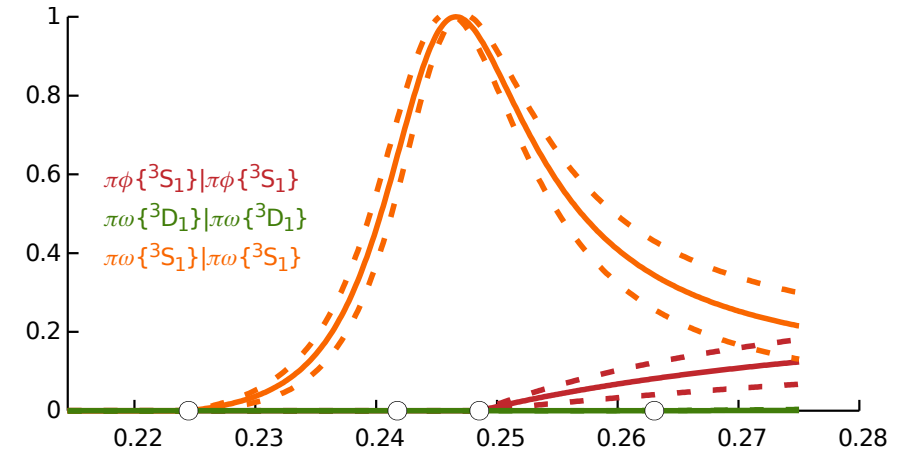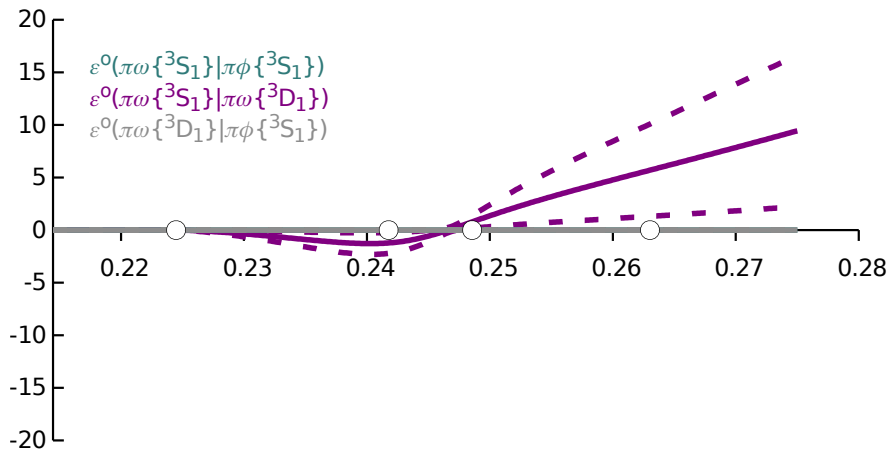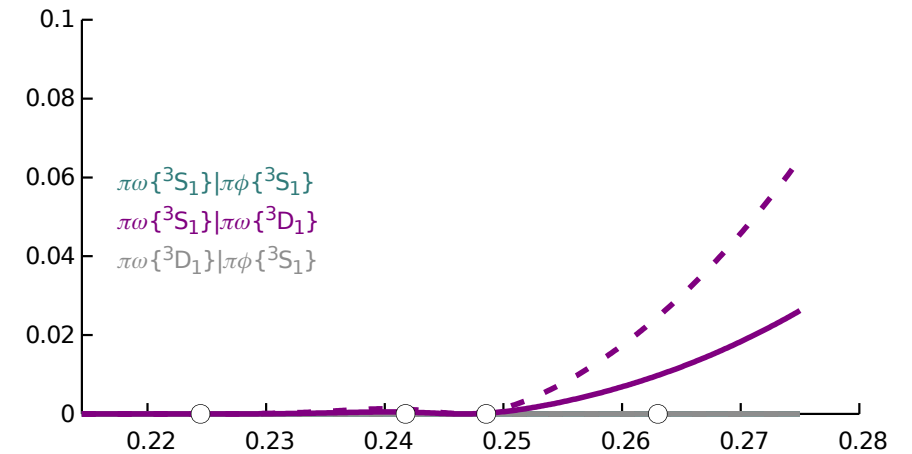



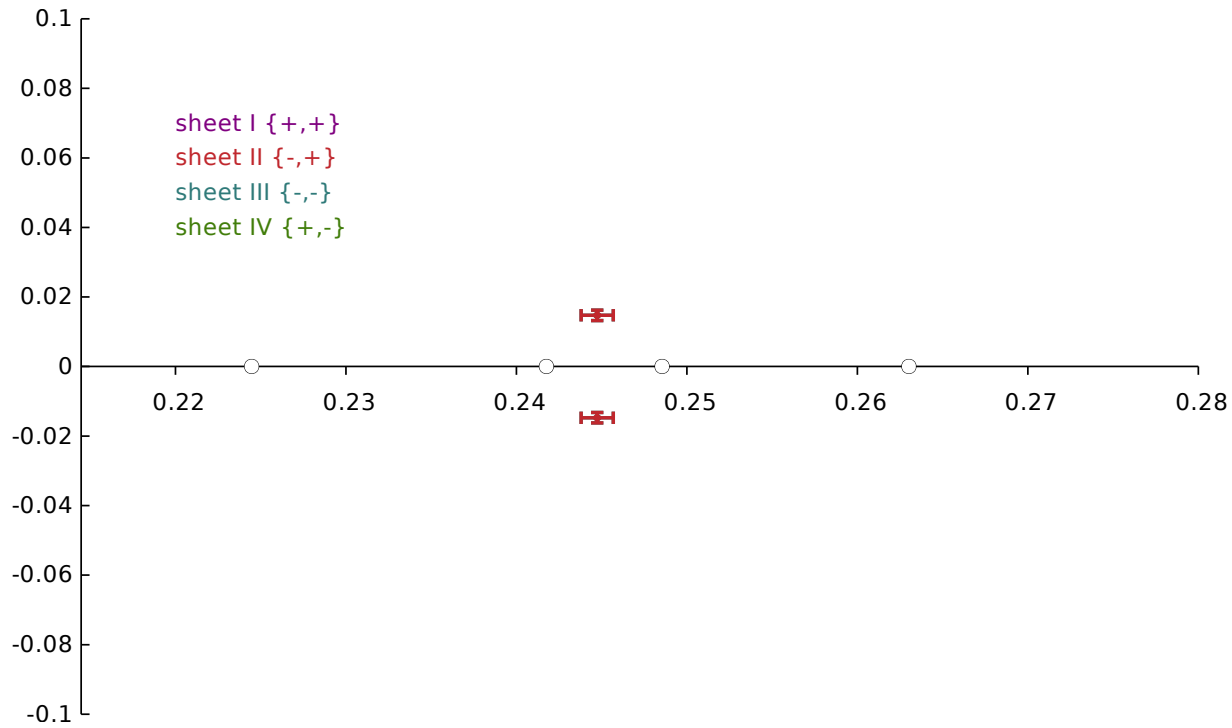

### parameter values

minimised with  $\text{chisq}/\text{nDoF} = 40.52 / (36 - 5) = 1.31$

|                                               |  |                        |  |      |       |       |       |       |
|-----------------------------------------------|--|------------------------|--|------|-------|-------|-------|-------|
| JP1+_g_pi:omega/3^S_1_pole0                   |  | 0.095712 +/- 0.0049231 |  | 1.00 | -0.14 | -0.38 | 0.02  | -0.14 |
| JP1+_gamma_pi:omega/3^S_1 pi:omega/3^D_1_orde |  | -13.632 +/- 10.973     |  |      | 1.00  | 0.22  | -0.16 | -0.20 |
| JP1+_gamma_pi:omega/3^S_1 pi:omega/3^S_1_orde |  | -0.25788 +/- 0.16449   |  |      |       | 1.00  | 0.17  | -0.06 |
| JP1+_gamma_pi:phi/3^S_1 pi:phi/3^S_1_order0   |  | 0.95710 +/- 0.24639    |  |      |       |       | 1.00  | -0.18 |
| JP1+_m_pole0                                  |  | 0.24661 +/- 0.00064059 |  |      |       |       |       | 1.00  |

### pole singularities

pi:omega[-] pi:phi[+] upper half-plane

$\text{s\_pole} = (0.24474 \pm 0.00094169) + (i/2) * (0.014719 \pm 0.0014873) [-0.37]$

$\text{s\_pole} = (0.059842 \pm 0.00046512) + i * (0.0036023 \pm 0.00035906) [-0.36]$

|                          |                         |
|--------------------------|-------------------------|
| pi:omega                 | pi:phi                  |
| ===== =====              | =====                   |
| k_re= -0.0463 +/- 0.0010 | k_re= 0.0145 +/- 0.0011 |
| k_im= -0.0087 +/- 0.0009 | k_im= 0.0246 +/- 0.0017 |
| corr= [-0.42]            | corr= [-0.09]           |



# 1 Successful Parameterizations

| pi:omega/3^S_1(*)            |                              | pi:phi/3^S_1                 |  | pi:omega/3^D_1 |  |
|------------------------------|------------------------------|------------------------------|--|----------------|--|
| g = 0.0971 +/- 0.0053        | g = 0.0000 +/- 0.0000        | g = 0.0049 +/- 0.0039        |  |                |  |
| arg(g)/pi= 0.0587 +/- 0.0228 | arg(g)/pi= 0.4413 +/- 0.0228 | arg(g)/pi= 0.7288 +/- 0.0355 |  |                |  |
| g_re= 0.0955 +/- 0.0054      | g_re= 0.0000 +/- 0.0000      | g_re= -0.0032 +/- 0.0026     |  |                |  |
| g_im= 0.0178 +/- 0.0069      | g_im= 0.0000 +/- 0.0000      | g_im= 0.0037 +/- 0.0029      |  |                |  |
| corr= [-0.14]                | corr= [-0.06]                | corr= [-0.96]                |  |                |  |
| Br = 0.9770 +/- 0.0208       | Br = 0.0000 +/- 0.0000       | Br = 0.0025 +/- 0.0039       |  |                |  |

--  
pi:omega[-] pi:phi[+] lower half-plane

sqrt(s)\_pole = (0.24474 +/- 0.00094169)  
+ (i/2)\*(-0.014719 +/- 0.0014873) [ 0.37]

s\_pole = (0.059842 +/- 0.00046512)  
+ i\*(-0.0036023 +/- 0.00035906) [ 0.36]

| pi:omega                 |                          | pi:phi |  |
|--------------------------|--------------------------|--------|--|
| k_re= 0.0463 +/- 0.0010  | k_re= -0.0145 +/- 0.0011 |        |  |
| k_im= -0.0087 +/- 0.0009 | k_im= 0.0246 +/- 0.0017  |        |  |
| corr= [ 0.42]            | corr= [ 0.09]            |        |  |

| pi:omega/3^S_1(*)             |                              | pi:phi/3^S_1                  |  | pi:omega/3^D_1 |  |
|-------------------------------|------------------------------|-------------------------------|--|----------------|--|
| g = 0.0971 +/- 0.0053         | g = 0.0000 +/- 0.0000        | g = 0.0049 +/- 0.0039         |  |                |  |
| arg(g)/pi= -0.0587 +/- 0.0228 | arg(g)/pi= 0.5587 +/- 0.0228 | arg(g)/pi= -0.7288 +/- 0.0355 |  |                |  |
| g_re= 0.0955 +/- 0.0054       | g_re= -0.0000 +/- 0.0000     | g_re= -0.0032 +/- 0.0026      |  |                |  |
| g_im= -0.0178 +/- 0.0069      | g_im= 0.0000 +/- 0.0000      | g_im= -0.0037 +/- 0.0029      |  |                |  |
| corr= [ 0.14]                 | corr= [ 0.06]                | corr= [ 0.96]                 |  |                |  |
| Br = 0.9770 +/- 0.0208        | Br = 0.0000 +/- 0.0000       | Br = 0.0025 +/- 0.0039        |  |                |  |

--  
pi:omega[-] pi:phi[-] upper half-plane

sqrt(s)\_pole = (0.24474 +/- 0.0009444)  
+ (i/2)\*(+0.014719 +/- 0.0014962) [-0.38]

s\_pole = (0.059842 +/- 0.00046651)  
+ i\*(+0.0036024 +/- 0.00036118) [-0.36]

| pi:omega                 |                          | pi:phi |  |
|--------------------------|--------------------------|--------|--|
| k_re= -0.0463 +/- 0.0010 | k_re= -0.0145 +/- 0.0011 |        |  |
| k_im= -0.0087 +/- 0.0009 | k_im= -0.0246 +/- 0.0017 |        |  |
| corr= [-0.42]            | corr= [-0.08]            |        |  |

| pi:omega/3^S_1(*)            |                              | pi:phi/3^S_1                 |  | pi:omega/3^D_1 |  |
|------------------------------|------------------------------|------------------------------|--|----------------|--|
| g = 0.0971 +/- 0.0053        | g = 0.0000 +/- 0.0000        | g = 0.0049 +/- 0.0039        |  |                |  |
| arg(g)/pi= 0.0587 +/- 0.0228 | arg(g)/pi= 0.4413 +/- 0.0228 | arg(g)/pi= 0.7288 +/- 0.0356 |  |                |  |
| g_re= 0.0955 +/- 0.0054      | g_re= 0.0000 +/- 0.0000      | g_re= -0.0032 +/- 0.0026     |  |                |  |
| g_im= 0.0178 +/- 0.0069      | g_im= 0.0000 +/- 0.0000      | g_im= 0.0037 +/- 0.0029      |  |                |  |
| corr= [-0.14]                | corr= [-0.05]                | corr= [-0.96]                |  |                |  |
| Br = 0.9771 +/- 0.0209       | Br = 0.0000 +/- 0.0000       | Br = 0.0025 +/- 0.0039       |  |                |  |



```
--
pi:omega[-] pi:phi[-] lower half-plane

sqrt(s)_pole = (0.24474 +/- 0.0009444)
               + (i/2)*(-0.014719 +/- 0.0014962) [ 0.38]

s_pole = (0.059842 +/- 0.00046651)
         + i*(-0.0036024 +/- 0.00036118) [ 0.36]

=====
               pi:omega |               pi:phi |
=====
k_re=  0.0463 +/- 0.0010 | k_re=  0.0145 +/- 0.0011 |
k_im= -0.0087 +/- 0.0009 | k_im= -0.0246 +/- 0.0017 |
corr= [ 0.42]           | corr= [ 0.08]           |

=====
pi:omega/3^S_1(*) | pi:phi/3^S_1 | pi:omega/3^D_1 |
=====
|g|=  0.0971 +/- 0.0053 | |g|=  0.0000 +/- 0.0000 | |g|=  0.0049 +/- 0.0039 |
arg(g)/pi= -0.0587 +/- 0.0228 | arg(g)/pi=  0.5587 +/- 0.0228 | arg(g)/pi= -0.7288 +/- 0.0356 |
-----
g_re=  0.0955 +/- 0.0054 | g_re= -0.0000 +/- 0.0000 | g_re= -0.0032 +/- 0.0026 |
g_im= -0.0178 +/- 0.0069 | g_im=  0.0000 +/- 0.0000 | g_im= -0.0037 +/- 0.0029 |
corr= [ 0.14]           | corr= [ 0.05]           | corr= [ 0.96]           |
-----
Br =  0.9771 +/- 0.0209 | Br =  0.0000 +/- 0.0000 | Br =  0.0025 +/- 0.0039 |
```



## 1.21 coupled\_po\_pp.3s1\_3d1.pole+G0\_3s1\_3sd1\_3S1.gorder0\_3s1.threshold\_sub

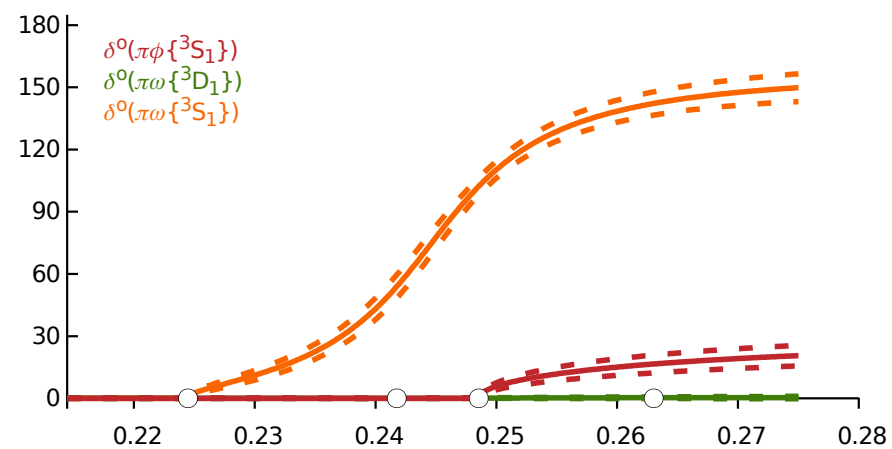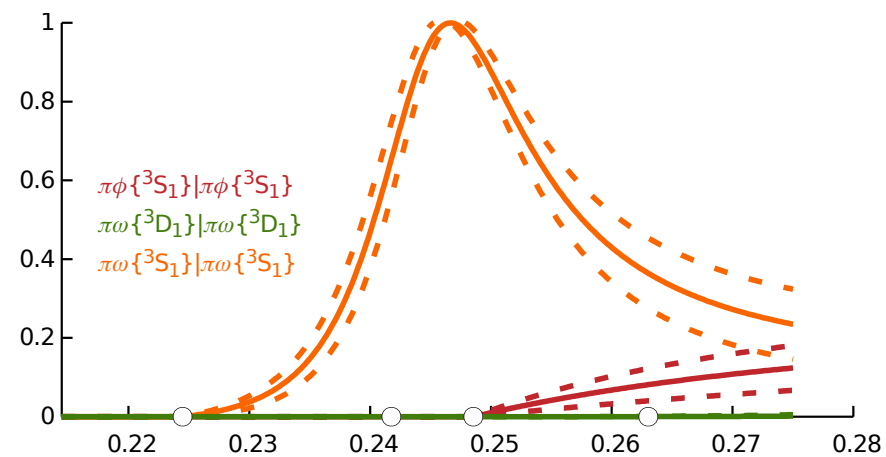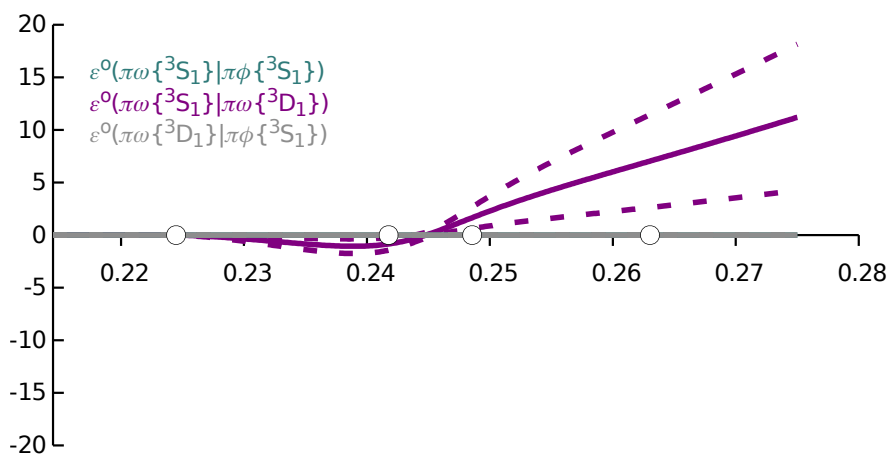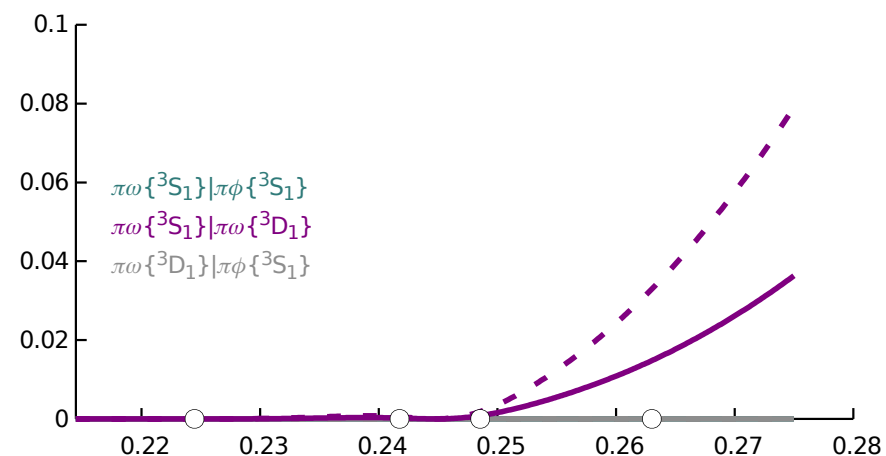



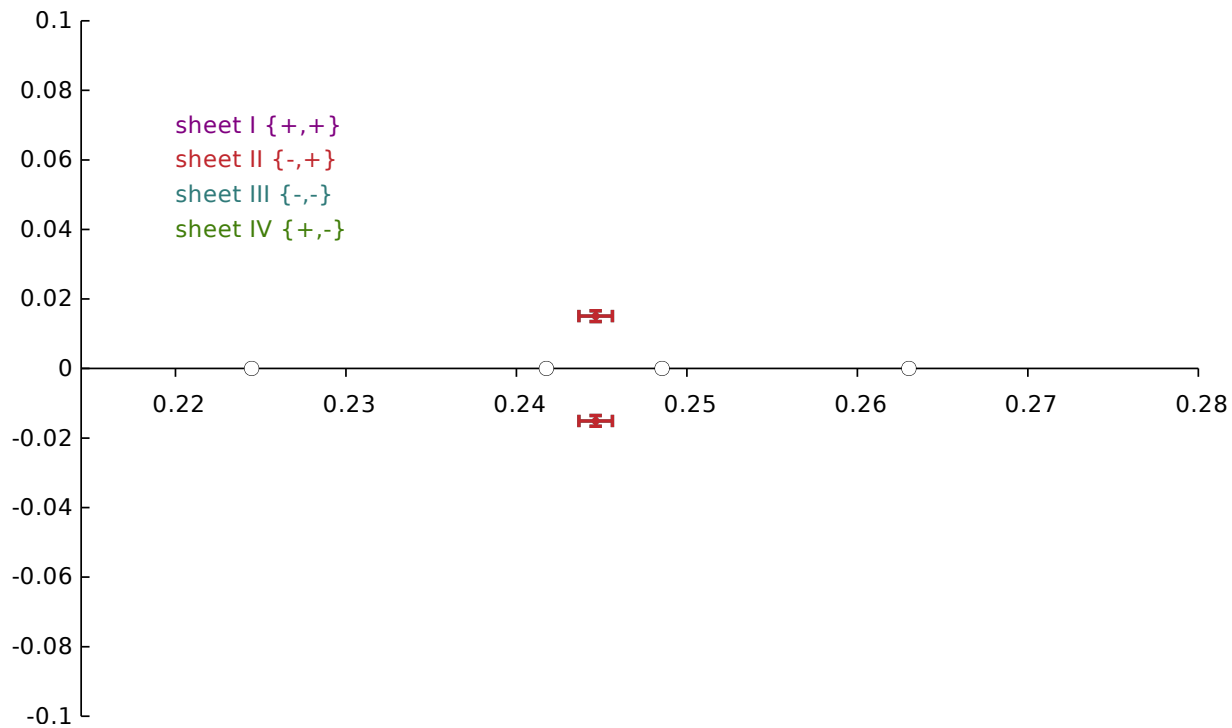

### parameter values

minimised with  $\text{chisq}/\text{nDoF} = 39.62 / (36 - 5) = 1.28$

|                                               |  |                        |  |      |       |       |       |       |
|-----------------------------------------------|--|------------------------|--|------|-------|-------|-------|-------|
| JP1+_g_pi:omega/3^S_1_pole0_order0            |  | 0.094485 +/- 0.0045903 |  | 1.00 | -0.20 | -0.11 | 0.11  | -0.43 |
| JP1+_gamma_pi:omega/3^S_1 pi:omega/3^D_1_orde |  | -14.970 +/- 9.8761     |  |      | 1.00  | 0.22  | -0.11 | -0.14 |
| JP1+_gamma_pi:omega/3^S_1 pi:omega/3^S_1_orde |  | -0.27034 +/- 0.16117   |  |      |       | 1.00  | 0.17  | 0.03  |
| JP1+_gamma_pi:phi/3^S_1 pi:phi/3^S_1_order0   |  | 1.0625 +/- 0.31038     |  |      |       |       | 1.00  | -0.28 |
| JP1+_m_pole0                                  |  | 0.24479 +/- 0.00066808 |  |      |       |       |       | 1.00  |

### pole singularities

pi:omega[-] pi:phi[+] upper half-plane

$\text{sqr}(s)_{\text{pole}} = (0.27238 \pm 0.016564)$   
 $+ (i/2) * (0.21117 \pm 0.083878) [0.89]$

$s_{\text{pole}} = (0.063037 \pm 0.0041536)$   
 $+ i * (0.057521 \pm 0.026021) [-0.14]$

|                          |                         |
|--------------------------|-------------------------|
| pi:omega                 | pi:phi                  |
| ===== =====              |                         |
| k_re= -0.0892 +/- 0.0167 | k_re= 0.0769 +/- 0.0187 |
| k_im= -0.0764 +/- 0.0224 | k_im= 0.0838 +/- 0.0219 |
| corr= [ 0.95]            | corr= [ 0.95]           |



# 1 Successful Parameterizations

| pi:omega/3^S_1(*)             | pi:phi/3^S_1                 | pi:omega/3^D_1               |
|-------------------------------|------------------------------|------------------------------|
| g = 0.1434 +/- 0.0181         | g = 0.0000 +/- 0.0000        | g = 0.1340 +/- 0.0181        |
| arg(g)/pi= -0.4372 +/- 0.0475 | arg(g)/pi= 0.9372 +/- 0.0475 | arg(g)/pi= 0.5050 +/- 0.0431 |
| g_re= 0.0281 +/- 0.0241       | g_re= -0.0000 +/- 0.0000     | g_re= -0.0021 +/- 0.0184     |
| g_im= -0.1406 +/- 0.0143      | g_im= 0.0000 +/- 0.0000      | g_im= 0.1340 +/- 0.0179      |
| corr= [-0.80]                 | corr= [ 0.84]                | corr= [-0.92]                |
| Br = 0.1915 +/- 0.0507        | Br = 0.0000 +/- 0.0000       | Br = 0.1672 +/- 0.0402       |

--  
pi:omega[-] pi:phi[+] upper half-plane

sqrts)\_pole = (0.24465 +/- 0.00098683)  
+ (i/2)\*(+0.015065 +/- 0.0015335) [-0.37]

s\_pole = (0.059796 +/- 0.00048728)  
+ i\*(+0.0036857 +/- 0.00036987) [-0.36]

| pi:omega                 | pi:phi                  |
|--------------------------|-------------------------|
| k_re= -0.0462 +/- 0.0011 | k_re= 0.0146 +/- 0.0011 |
| k_im= -0.0089 +/- 0.0010 | k_im= 0.0249 +/- 0.0018 |
| corr= [-0.42]            | corr= [-0.10]           |

| pi:omega/3^S_1(*)            | pi:phi/3^S_1                 | pi:omega/3^D_1               |
|------------------------------|------------------------------|------------------------------|
| g = 0.0981 +/- 0.0054        | g = 0.0000 +/- 0.0000        | g = 0.0054 +/- 0.0035        |
| arg(g)/pi= 0.0618 +/- 0.0234 | arg(g)/pi= 0.4382 +/- 0.0234 | arg(g)/pi= 0.6595 +/- 0.0368 |
| g_re= 0.0963 +/- 0.0055      | g_re= 0.0000 +/- 0.0000      | g_re= -0.0026 +/- 0.0018     |
| g_im= 0.0189 +/- 0.0071      | g_im= 0.0000 +/- 0.0000      | g_im= 0.0047 +/- 0.0031      |
| corr= [-0.16]                | corr= [-0.06]                | corr= [-0.92]                |
| Br = 0.9723 +/- 0.0219       | Br = 0.0000 +/- 0.0000       | Br = 0.0029 +/- 0.0038       |

--  
pi:omega[-] pi:phi[+] lower half-plane

sqrts)\_pole = (0.27238 +/- 0.016564)  
+ (i/2)\*(-0.21117 +/- 0.083878) [-0.89]

s\_pole = (0.063037 +/- 0.0041536)  
+ i\*(-0.057521 +/- 0.026021) [ 0.14]

| pi:omega                 | pi:phi                   |
|--------------------------|--------------------------|
| k_re= 0.0892 +/- 0.0167  | k_re= -0.0769 +/- 0.0187 |
| k_im= -0.0764 +/- 0.0224 | k_im= 0.0838 +/- 0.0219  |
| corr= [-0.95]            | corr= [-0.95]            |

| pi:omega/3^S_1(*)            | pi:phi/3^S_1                 | pi:omega/3^D_1                |
|------------------------------|------------------------------|-------------------------------|
| g = 0.1434 +/- 0.0181        | g = 0.0000 +/- 0.0000        | g = 0.1340 +/- 0.0181         |
| arg(g)/pi= 0.4372 +/- 0.0475 | arg(g)/pi= 0.0628 +/- 0.0475 | arg(g)/pi= -0.5050 +/- 0.0431 |
| g_re= 0.0281 +/- 0.0241      | g_re= 0.0000 +/- 0.0000      | g_re= -0.0021 +/- 0.0184      |
| g_im= 0.1406 +/- 0.0143      | g_im= 0.0000 +/- 0.0000      | g_im= -0.1340 +/- 0.0179      |
| corr= [ 0.80]                | corr= [-0.84]                | corr= [ 0.92]                 |
| Br = 0.1915 +/- 0.0507       | Br = 0.0000 +/- 0.0000       | Br = 0.1672 +/- 0.0402        |



## 1 Successful Parameterizations

```
--
pi:omega[-] pi:phi[+] lower half-plane

sqrt(s)_pole = (0.24465 +/- 0.00098683)
               + (i/2)*(-0.015065 +/- 0.0015335) [ 0.37]

s_pole = (0.059796 +/- 0.00048728)
         + i*(-0.0036857 +/- 0.00036987) [ 0.36]

=====
pi:omega | pi:phi |
=====
k_re= 0.0462 +/- 0.0011 | k_re= -0.0146 +/- 0.0011 |
k_im= -0.0089 +/- 0.0010 | k_im= 0.0249 +/- 0.0018 |
corr= [ 0.42] | corr= [ 0.10] |

=====
pi:omega/3^S_1(*) | pi:phi/3^S_1 | pi:omega/3^D_1 |
=====
|g|= 0.0981 +/- 0.0054 | |g|= 0.0000 +/- 0.0000 | |g|= 0.0054 +/- 0.0035 |
arg(g)/pi= -0.0618 +/- 0.0234 | arg(g)/pi= 0.5618 +/- 0.0234 | arg(g)/pi= -0.6595 +/- 0.0368 |
-----
g_re= 0.0963 +/- 0.0055 | g_re= -0.0000 +/- 0.0000 | g_re= -0.0026 +/- 0.0018 |
g_im= -0.0189 +/- 0.0071 | g_im= 0.0000 +/- 0.0000 | g_im= -0.0047 +/- 0.0031 |
corr= [ 0.16] | corr= [ 0.06] | corr= [ 0.92] |
-----
Br = 0.9723 +/- 0.0219 | Br = 0.0000 +/- 0.0000 | Br = 0.0029 +/- 0.0038 |

--
pi:omega[-] pi:phi[-] upper half-plane

sqrt(s)_pole = (0.27238 +/- 0.016564)
               + (i/2)*(+0.21117 +/- 0.083878) [ 0.89]

s_pole = (0.063037 +/- 0.0041536)
         + i*(+0.057521 +/- 0.026021) [-0.14]

=====
pi:omega | pi:phi |
=====
k_re= -0.0892 +/- 0.0167 | k_re= -0.0769 +/- 0.0187 |
k_im= -0.0764 +/- 0.0224 | k_im= -0.0838 +/- 0.0219 |
corr= [ 0.95] | corr= [ 0.95] |

=====
pi:omega/3^S_1(*) | pi:phi/3^S_1 | pi:omega/3^D_1 |
=====
|g|= 0.1434 +/- 0.0181 | |g|= 0.0000 +/- 0.0000 | |g|= 0.1340 +/- 0.0181 |
arg(g)/pi= -0.4372 +/- 0.0475 | arg(g)/pi= 0.9372 +/- 0.0475 | arg(g)/pi= 0.5050 +/- 0.0431 |
-----
g_re= 0.0281 +/- 0.0241 | g_re= -0.0000 +/- 0.0000 | g_re= -0.0021 +/- 0.0184 |
g_im= -0.1406 +/- 0.0143 | g_im= 0.0000 +/- 0.0000 | g_im= 0.1340 +/- 0.0179 |
corr= [-0.80] | corr= [ 0.84] | corr= [-0.92] |
-----
Br = 0.1915 +/- 0.0507 | Br = 0.0000 +/- 0.0000 | Br = 0.1672 +/- 0.0402 |

--
pi:omega[-] pi:phi[-] upper half-plane

sqrt(s)_pole = (0.24465 +/- 0.00098836)
               + (i/2)*(+0.015065 +/- 0.0015342) [-0.37]

s_pole = (0.059796 +/- 0.00048804)
         + i*(+0.0036857 +/- 0.00037002) [-0.36]

pi:omega | pi:phi |
```



# 1 Successful Parameterizations

```

=====|=====|
k_re= -0.0462 +/- 0.0011 | k_re= -0.0146 +/- 0.0011 |
k_im= -0.0089 +/- 0.0010 | k_im= -0.0249 +/- 0.0018 |
corr= [-0.42] | corr= [-0.10] |

pi:omega/3^S_1(*) | pi:phi/3^S_1 | pi:omega/3^D_1 |
=====|=====|=====|
|g|= 0.0981 +/- 0.0054 | |g|= 0.0000 +/- 0.0000 | |g|= 0.0054 +/- 0.0035 |
arg(g)/pi= 0.0618 +/- 0.0234 | arg(g)/pi= 0.4382 +/- 0.0234 | arg(g)/pi= 0.6595 +/- 0.0368 |
-----|-----|-----|
g_re= 0.0963 +/- 0.0055 | g_re= 0.0000 +/- 0.0000 | g_re= -0.0026 +/- 0.0018 |
g_im= 0.0189 +/- 0.0071 | g_im= 0.0000 +/- 0.0000 | g_im= 0.0047 +/- 0.0031 |
corr= [-0.16] | corr= [-0.06] | corr= [-0.92] |
-----|-----|-----|
Br = 0.9723 +/- 0.0220 | Br = 0.0000 +/- 0.0000 | Br = 0.0029 +/- 0.0038 |

--
pi:omega[-] pi:phi[-] lower half-plane

sqrt(s)_pole = (0.27238 +/- 0.016564)
+ (i/2)*(-0.21117 +/- 0.083878) [-0.89]

s_pole = (0.063037 +/- 0.0041536)
+ i*(-0.057521 +/- 0.026021) [ 0.14]

pi:omega | pi:phi |
=====|=====|
k_re= 0.0892 +/- 0.0167 | k_re= 0.0769 +/- 0.0187 |
k_im= -0.0764 +/- 0.0224 | k_im= -0.0838 +/- 0.0219 |
corr= [-0.95] | corr= [-0.95] |

pi:omega/3^S_1(*) | pi:phi/3^S_1 | pi:omega/3^D_1 |
=====|=====|=====|
|g|= 0.1434 +/- 0.0181 | |g|= 0.0000 +/- 0.0000 | |g|= 0.1340 +/- 0.0181 |
arg(g)/pi= 0.4372 +/- 0.0475 | arg(g)/pi= 0.0628 +/- 0.0475 | arg(g)/pi= -0.5050 +/- 0.0431 |
-----|-----|-----|
g_re= 0.0281 +/- 0.0241 | g_re= 0.0000 +/- 0.0000 | g_re= -0.0021 +/- 0.0184 |
g_im= 0.1406 +/- 0.0143 | g_im= 0.0000 +/- 0.0000 | g_im= -0.1340 +/- 0.0179 |
corr= [ 0.80] | corr= [-0.84] | corr= [ 0.92] |
-----|-----|-----|
Br = 0.1915 +/- 0.0507 | Br = 0.0000 +/- 0.0000 | Br = 0.1672 +/- 0.0402 |

--
pi:omega[-] pi:phi[-] lower half-plane

sqrt(s)_pole = (0.24465 +/- 0.00098836)
+ (i/2)*(-0.015065 +/- 0.0015342) [ 0.37]

s_pole = (0.059796 +/- 0.00048804)
+ i*(-0.0036857 +/- 0.00037002) [ 0.36]

pi:omega | pi:phi |
=====|=====|
k_re= 0.0462 +/- 0.0011 | k_re= 0.0146 +/- 0.0011 |
k_im= -0.0089 +/- 0.0010 | k_im= -0.0249 +/- 0.0018 |
corr= [ 0.42] | corr= [ 0.10] |

pi:omega/3^S_1(*) | pi:phi/3^S_1 | pi:omega/3^D_1 |
=====|=====|=====|
|g|= 0.0981 +/- 0.0054 | |g|= 0.0000 +/- 0.0000 | |g|= 0.0054 +/- 0.0035 |
arg(g)/pi= -0.0618 +/- 0.0234 | arg(g)/pi= 0.5618 +/- 0.0234 | arg(g)/pi= -0.6595 +/- 0.0368 |
-----|-----|-----|

```



# 1 Successful Parameterizations

|                          |                          |                          |
|--------------------------|--------------------------|--------------------------|
| g_re= 0.0963 +/- 0.0055  | g_re= -0.0000 +/- 0.0000 | g_re= -0.0026 +/- 0.0018 |
| g_im= -0.0189 +/- 0.0071 | g_im= 0.0000 +/- 0.0000  | g_im= -0.0047 +/- 0.0031 |
| corr= [ 0.16]            | corr= [ 0.06]            | corr= [ 0.92]            |
| -----                    | -----                    | -----                    |
| Br = 0.9723 +/- 0.0220   | Br = 0.0000 +/- 0.0000   | Br = 0.0029 +/- 0.0038   |



## 2 Unphysical Parameterizations



## 2.1 coupled\_po\_pp.3s1\_3d1.pole+G0\_3s1\_3S1+G1\_3s1.gorder0\_3s1\_3d1\_3S1.irho

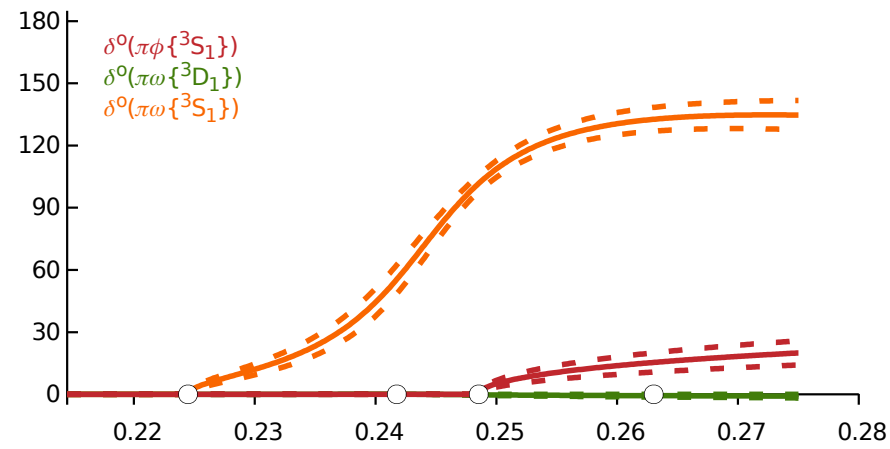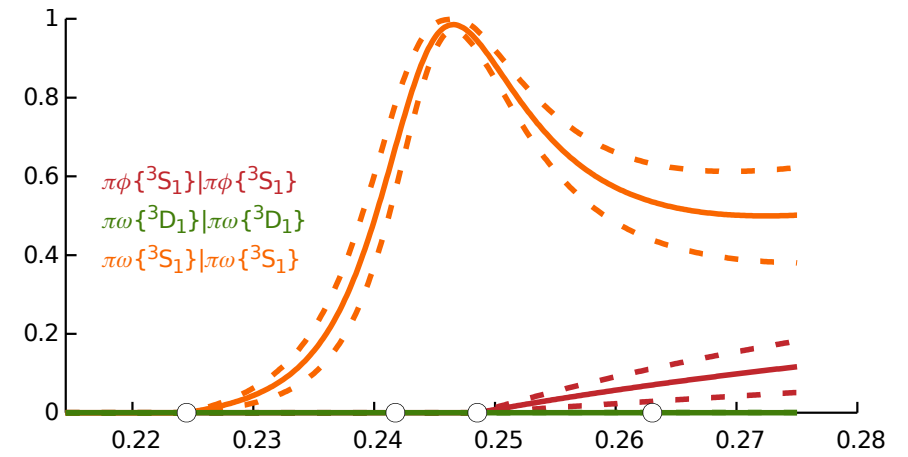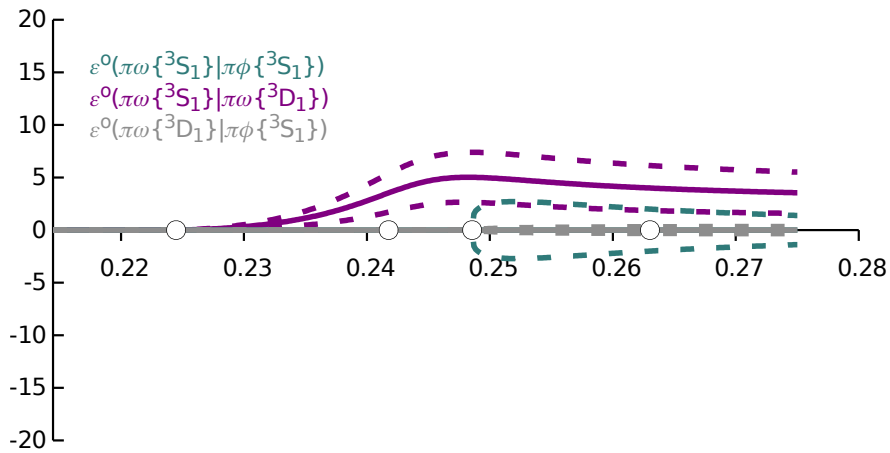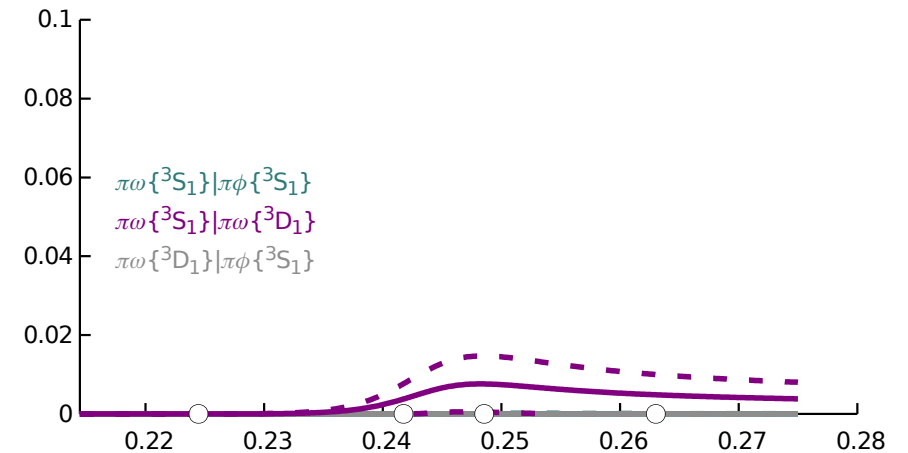



## 2 Unphysical Parameterizations

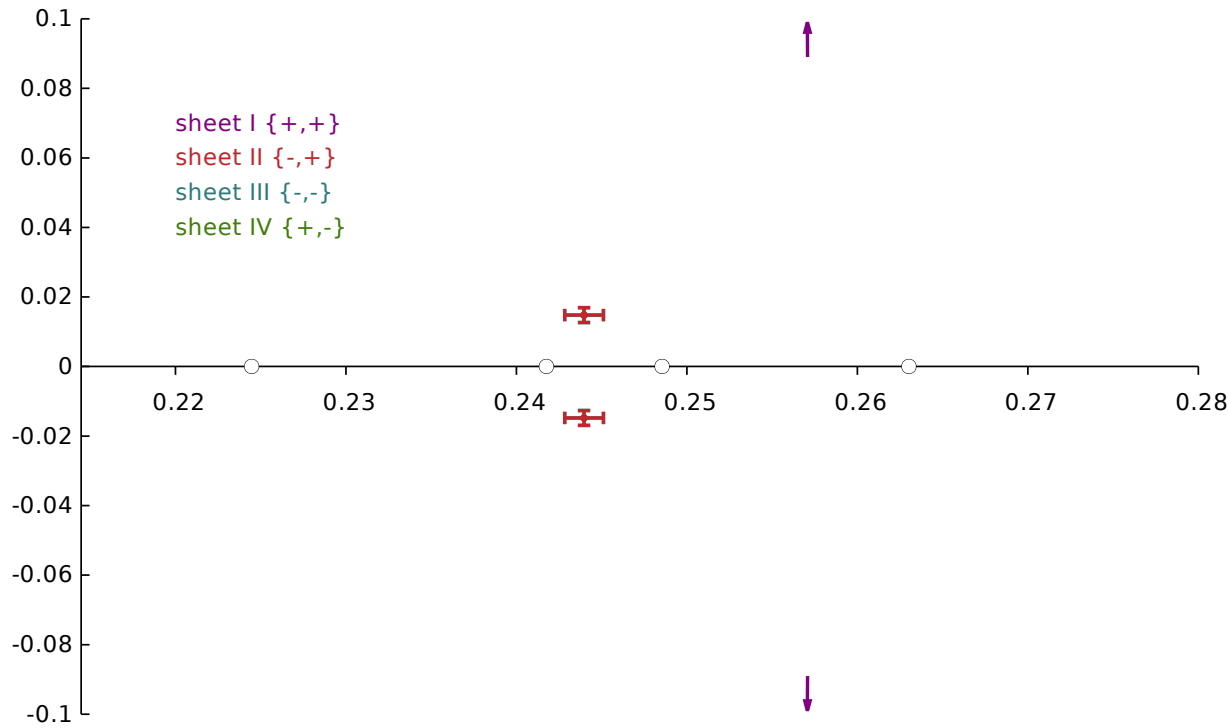

### parameter values

minimised with  $\text{chisq}/\text{nDoF} = 36.06 / (36 - 7) = 1.24$

|                                               |  |                         |  |      |      |       |       |       |       |       |
|-----------------------------------------------|--|-------------------------|--|------|------|-------|-------|-------|-------|-------|
| JP1+_g_pi:omega/3^D_1_pole0                   |  | 0.99610 +/- 0.53535     |  | 1.00 | 0.75 | -0.00 | -0.18 | 0.05  | -0.03 | -0.07 |
| JP1+_g_pi:omega/3^S_1_pole0                   |  | 0.10524 +/- 0.0091525   |  |      | 1.00 | -0.01 | -0.38 | 0.22  | -0.01 | -0.15 |
| JP1+_g_pi:phi/3^S_1_pole0                     |  | 1.5477e-06 +/- 0.011046 |  |      |      | 1.00  | 0.00  | -0.00 | 0.00  | -0.04 |
| JP1+_gamma_pi:omega/3^S_1 pi:omega/3^S_1_orde |  | 1.4004 +/- 0.8417       |  |      |      |       | 1.00  | -0.96 | -0.03 | 0.05  |
| JP1+_gamma_pi:omega/3^S_1 pi:omega/3^S_1_orde |  | -33.012 +/- 15.389      |  |      |      |       |       | 1.00  | 0.09  | -0.04 |
| JP1+_gamma_pi:phi/3^S_1 pi:phi/3^S_1_order0   |  | 0.92714 +/- 0.28285     |  |      |      |       |       |       | 1.00  | -0.30 |
| JP1+_m_pole0                                  |  | 0.24656 +/- 0.00067665  |  |      |      |       |       |       |       | 1.00  |

### pole singularities

pi:omega[+] pi:phi[+] upper half-plane

$\text{sqrt}(s)_{\text{pole}} = (0.25707 \pm 0.011603)$   
 $+ (i/2) * (0.17385 \pm 0.052196) \quad [0.59]$

$s_{\text{pole}} = (0.058527 \pm 0.0049009)$   
 $+ i * (0.044693 \pm 0.014711) \quad [-0.09]$

|                         |  |                         |  |
|-------------------------|--|-------------------------|--|
| pi:omega                |  | pi:phi                  |  |
| =====                   |  | =====                   |  |
| k_re= 0.0763 +/- 0.0114 |  | k_re= 0.0631 +/- 0.0126 |  |
| k_im= 0.0681 +/- 0.0147 |  | k_im= 0.0762 +/- 0.0143 |  |



## 2 Unphysical Parameterizations

```

corr= [ 0.79]          |      corr= [ 0.80]          |
=====
pi:omega/3^S_1(*) |      pi:phi/3^S_1 |      pi:omega/3^D_1 |
=====
|g|= 0.1943 +/- 0.0284 |      |g|= 0.0001 +/- 0.0016 |      |g|= 0.0148 +/- 0.0102 |
arg(g)/pi= -0.0990 +/- 0.0181 | arg(g)/pi= -0.3710 +/- 11.1949 | arg(g)/pi= -0.5219 +/- 0.0339 |
-----
g_re= 0.1850 +/- 0.0304 |      g_re= -0.0000 +/- 0.0024 |      g_re= -0.0010 +/- 0.0013 |
g_im= -0.0595 +/- 0.0021 |      g_im= -0.0000 +/- 0.0012 |      g_im= -0.0148 +/- 0.0102 |
corr= [ 0.89]          |      corr= [ 1.00]          |      corr= [-0.23]          |
-----
Br = 0.3923 +/- 0.0306 |      Br = 0.0000 +/- 0.0000 |      Br = 0.0023 +/- 0.0029 |

--
pi:omega[+] pi:phi[+] lower half-plane

sqrt(s)_pole = (0.25707 +/- 0.011603)
               + (i/2)*(-0.17385 +/- 0.052196) [-0.59]

s_pole = (0.058527 +/- 0.0049009)
         + i*(-0.044693 +/- 0.014711) [ 0.09]

pi:omega |      pi:phi |
=====
k_re= -0.0763 +/- 0.0114 |      k_re= -0.0631 +/- 0.0126 |
k_im= 0.0681 +/- 0.0147 |      k_im= 0.0762 +/- 0.0143 |
corr= [-0.79]          |      corr= [-0.80]          |

pi:omega/3^S_1(*) |      pi:phi/3^S_1 |      pi:omega/3^D_1 |
=====
|g|= 0.1943 +/- 0.0284 |      |g|= 0.0001 +/- 0.0016 |      |g|= 0.0148 +/- 0.0102 |
arg(g)/pi= 0.0990 +/- 0.0181 | arg(g)/pi= 0.3732 +/- 11.1486 | arg(g)/pi= 0.5219 +/- 0.0339 |
-----
g_re= 0.1850 +/- 0.0304 |      g_re= -0.0000 +/- 0.0024 |      g_re= -0.0010 +/- 0.0013 |
g_im= 0.0595 +/- 0.0021 |      g_im= 0.0000 +/- 0.0012 |      g_im= 0.0148 +/- 0.0102 |
corr= [-0.89]          |      corr= [-1.00]          |      corr= [ 0.23]          |
-----
Br = 0.3923 +/- 0.0306 |      Br = 0.0000 +/- 0.0000 |      Br = 0.0023 +/- 0.0029 |

--
pi:omega[+] pi:phi[-] upper half-plane

sqrt(s)_pole = (0.25707 +/- 0.011603)
               + (i/2)*(+0.17385 +/- 0.052196) [ 0.59]

s_pole = (0.058526 +/- 0.0049009)
         + i*(+0.044693 +/- 0.014711) [-0.09]

pi:omega |      pi:phi |
=====
k_re= 0.0763 +/- 0.0114 |      k_re= -0.0631 +/- 0.0126 |
k_im= 0.0681 +/- 0.0147 |      k_im= -0.0762 +/- 0.0143 |
corr= [ 0.79]          |      corr= [ 0.80]          |

pi:omega/3^S_1(*) |      pi:phi/3^S_1 |      pi:omega/3^D_1 |
=====
|g|= 0.1943 +/- 0.0284 |      |g|= 0.0002 +/- 0.0027 |      |g|= 0.0148 +/- 0.0102 |
arg(g)/pi= -0.0990 +/- 0.0181 | arg(g)/pi= 0.2981 +/- 11.1552 | arg(g)/pi= -0.5219 +/- 0.0339 |
-----
g_re= 0.1850 +/- 0.0304 |      g_re= -0.0000 +/- 0.0035 |      g_re= -0.0010 +/- 0.0013 |
g_im= -0.0595 +/- 0.0021 |      g_im= 0.0000 +/- 0.0029 |      g_im= -0.0148 +/- 0.0102 |
corr= [ 0.89]          |      corr= [-1.00]          |      corr= [-0.23]          |

```



## 2 Unphysical Parameterizations

```

-----|-----|-----|
Br = 0.3923 +/- 0.0306 | Br = 0.0000 +/- 0.0000 | Br = 0.0023 +/- 0.0029 |

--
pi:omega[+] pi:phi[-] lower half-plane

sqrt(s)_pole = (0.25707 +/- 0.011603)
+ (i/2)*(-0.17385 +/- 0.052196) [-0.59]

s_pole = (0.058526 +/- 0.0049009)
+ i*(-0.044693 +/- 0.014711) [ 0.09]

=====|=====|
pi:omega | pi:phi |
=====|=====|
k_re= -0.0763 +/- 0.0114 | k_re= 0.0631 +/- 0.0126 |
k_im= 0.0681 +/- 0.0147 | k_im= -0.0762 +/- 0.0143 |
corr= [-0.79] | corr= [-0.80] |

=====|=====|
pi:omega/3^S_1(*) | pi:phi/3^S_1 | pi:omega/3^D_1 |
=====|=====|
|g|= 0.1943 +/- 0.0284 | |g|= 0.0002 +/- 0.0027 | |g|= 0.0148 +/- 0.0102 |
arg(g)/pi= 0.0990 +/- 0.0181 | arg(g)/pi= -0.2959 +/- 11.1746 | arg(g)/pi= 0.5219 +/- 0.0339 |
-----|-----|
g_re= 0.1850 +/- 0.0304 | g_re= -0.0000 +/- 0.0035 | g_re= -0.0010 +/- 0.0013 |
g_im= 0.0595 +/- 0.0021 | g_im= -0.0000 +/- 0.0029 | g_im= 0.0148 +/- 0.0102 |
corr= [-0.89] | corr= [ 1.00] | corr= [ 0.23] |
-----|-----|
Br = 0.3923 +/- 0.0306 | Br = 0.0000 +/- 0.0000 | Br = 0.0023 +/- 0.0029 |

--
pi:omega[-] pi:phi[+] upper half-plane

sqrt(s)_pole = (0.24397 +/- 0.001135)
+ (i/2)*(+0.014784 +/- 0.0021108) [-0.51]

s_pole = (0.059466 +/- 0.00056198)
+ i*(+0.0036069 +/- 0.00050653) [-0.51]

=====|=====|
pi:omega | pi:phi |
=====|=====|
k_re= -0.0454 +/- 0.0012 | k_re= 0.0138 +/- 0.0013 |
k_im= -0.0089 +/- 0.0013 | k_im= 0.0257 +/- 0.0022 |
corr= [-0.51] | corr= [ 0.19] |

=====|=====|
pi:omega/3^S_1(*) | pi:phi/3^S_1 | pi:omega/3^D_1 |
=====|=====|
|g|= 0.0930 +/- 0.0073 | |g|= 0.0003 +/- 0.0054 | |g|= 0.0083 +/- 0.0041 |
arg(g)/pi= 0.0790 +/- 0.0219 | arg(g)/pi= -0.4301 +/- 11.1776 | arg(g)/pi= 0.1429 +/- 0.0246 |
-----|-----|
g_re= 0.0902 +/- 0.0072 | g_re= -0.0000 +/- 0.0088 | g_re= 0.0074 +/- 0.0036 |
g_im= 0.0228 +/- 0.0064 | g_im= -0.0000 +/- 0.0014 | g_im= 0.0036 +/- 0.0022 |
corr= [ 0.05] | corr= [ 1.00] | corr= [ 0.97] |
-----|-----|
Br = 0.8800 +/- 0.0337 | Br = 0.0000 +/- 0.0000 | Br = 0.0070 +/- 0.0064 |

--
pi:omega[-] pi:phi[+] lower half-plane

sqrt(s)_pole = (0.24397 +/- 0.001135)
+ (i/2)*(-0.014784 +/- 0.0021108) [ 0.51]

s_pole = (0.059466 +/- 0.00056198)
+ i*(-0.0036069 +/- 0.00050653) [ 0.51]

```



```

===== pi:omega | pi:phi |
k_re= 0.0454 +/- 0.0012 | k_re= -0.0138 +/- 0.0013 |
k_im= -0.0089 +/- 0.0013 | k_im= 0.0257 +/- 0.0022 |
corr= [ 0.51] | corr= [-0.19] |

===== pi:omega/3^S_1(*) | pi:phi/3^S_1 | pi:omega/3^D_1 |
|g|= 0.0930 +/- 0.0073 | |g|= 0.0003 +/- 0.0054 | |g|= 0.0083 +/- 0.0041 |
arg(g)/pi= -0.0790 +/- 0.0219 | arg(g)/pi= 0.4318 +/- 11.1508 | arg(g)/pi= -0.1429 +/- 0.0246 |
-----
g_re= 0.0902 +/- 0.0072 | g_re= -0.0000 +/- 0.0088 | g_re= 0.0074 +/- 0.0036 |
g_im= -0.0228 +/- 0.0064 | g_im= 0.0000 +/- 0.0014 | g_im= -0.0036 +/- 0.0022 |
corr= [-0.05] | corr= [-1.00] | corr= [-0.97] |
-----
Br = 0.8800 +/- 0.0337 | Br = 0.0000 +/- 0.0000 | Br = 0.0070 +/- 0.0064 |

--
pi:omega[-] pi:phi[-] upper half-plane

sqrt(s)_pole = (0.24397 +/- 0.0011398)
+ (i/2)*(+0.014784 +/- 0.0021632) [-0.52]

s_pole = (0.059465 +/- 0.00056461)
+ i*(+0.0036067 +/- 0.00051919) [-0.52]

===== pi:omega | pi:phi |
k_re= -0.0454 +/- 0.0012 | k_re= -0.0138 +/- 0.0013 |
k_im= -0.0089 +/- 0.0014 | k_im= -0.0257 +/- 0.0022 |
corr= [-0.51] | corr= [ 0.21] |

===== pi:omega/3^S_1(*) | pi:phi/3^S_1 | pi:omega/3^D_1 |
|g|= 0.0930 +/- 0.0074 | |g|= 0.0005 +/- 0.0080 | |g|= 0.0083 +/- 0.0042 |
arg(g)/pi= 0.0790 +/- 0.0221 | arg(g)/pi= 0.4591 +/- 11.1530 | arg(g)/pi= 0.1429 +/- 0.0251 |
-----
g_re= 0.0902 +/- 0.0074 | g_re= 0.0000 +/- 0.0132 | g_re= 0.0074 +/- 0.0036 |
g_im= 0.0228 +/- 0.0065 | g_im= -0.0000 +/- 0.0010 | g_im= 0.0036 +/- 0.0023 |
corr= [ 0.05] | corr= [-1.00] | corr= [ 0.97] |
-----
Br = 0.8800 +/- 0.0337 | Br = 0.0000 +/- 0.0000 | Br = 0.0069 +/- 0.0065 |

--
pi:omega[-] pi:phi[-] lower half-plane

sqrt(s)_pole = (0.24397 +/- 0.0011398)
+ (i/2)*(-0.014784 +/- 0.0021632) [ 0.52]

s_pole = (0.059465 +/- 0.00056461)
+ i*(-0.0036067 +/- 0.00051919) [ 0.52]

===== pi:omega | pi:phi |
k_re= 0.0454 +/- 0.0012 | k_re= 0.0138 +/- 0.0013 |
k_im= -0.0089 +/- 0.0014 | k_im= -0.0257 +/- 0.0022 |
corr= [ 0.51] | corr= [-0.21] |

===== pi:omega/3^S_1(*) | pi:phi/3^S_1 | pi:omega/3^D_1 |
|g|= 0.0930 +/- 0.0074 | |g|= 0.0005 +/- 0.0080 | |g|= 0.0083 +/- 0.0042 |

```



|                                      |                                     |                                      |
|--------------------------------------|-------------------------------------|--------------------------------------|
| $\arg(g)/\pi = -0.0790 \pm 0.0221$   | $\arg(g)/\pi = -0.4576 \pm 11.1899$ | $\arg(g)/\pi = -0.1429 \pm 0.0251$   |
| $g_{\text{re}} = 0.0902 \pm 0.0074$  | $g_{\text{re}} = 0.0000 \pm 0.0132$ | $g_{\text{re}} = 0.0074 \pm 0.0036$  |
| $g_{\text{im}} = -0.0228 \pm 0.0065$ | $g_{\text{im}} = 0.0000 \pm 0.0010$ | $g_{\text{im}} = -0.0036 \pm 0.0023$ |
| $\text{corr} = [-0.05]$              | $\text{corr} = [1.00]$              | $\text{corr} = [-0.97]$              |
| $\text{Br} = 0.8800 \pm 0.0337$      | $\text{Br} = 0.0000 \pm 0.0000$     | $\text{Br} = 0.0069 \pm 0.0065$      |

## 2.2 coupled\_po\_pp.3s1\_3d1.pole+G0\_3s1\_3S1+G1\_3s1.gorder0\_3s1\_3d1.irho

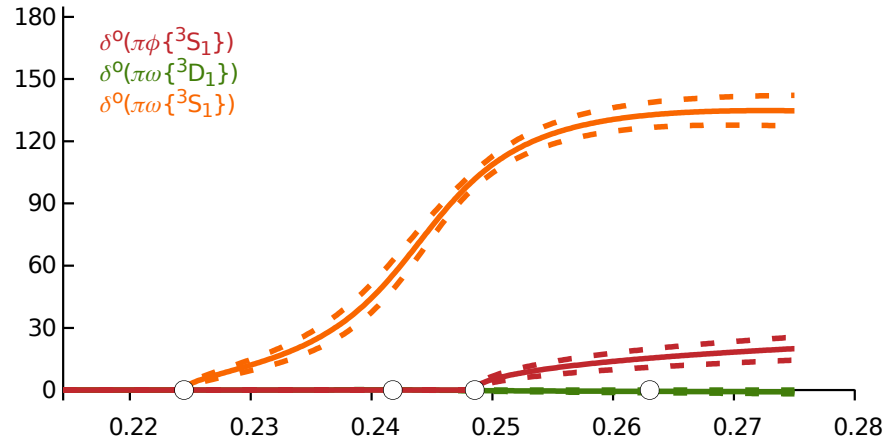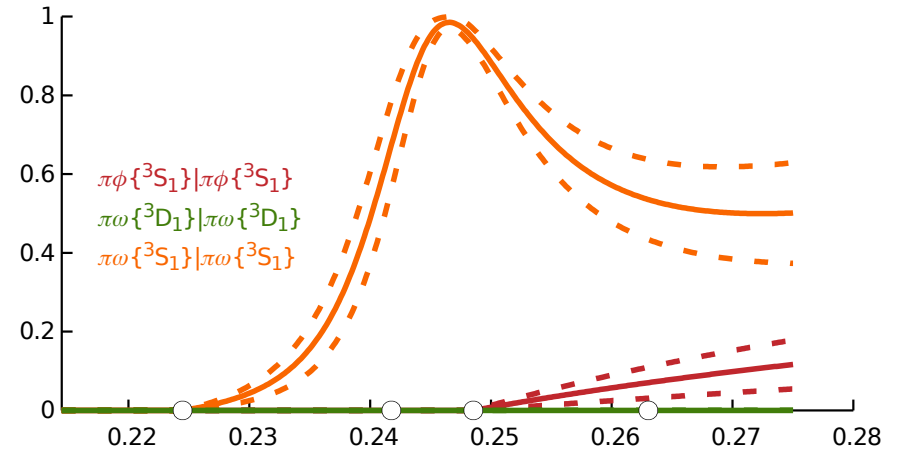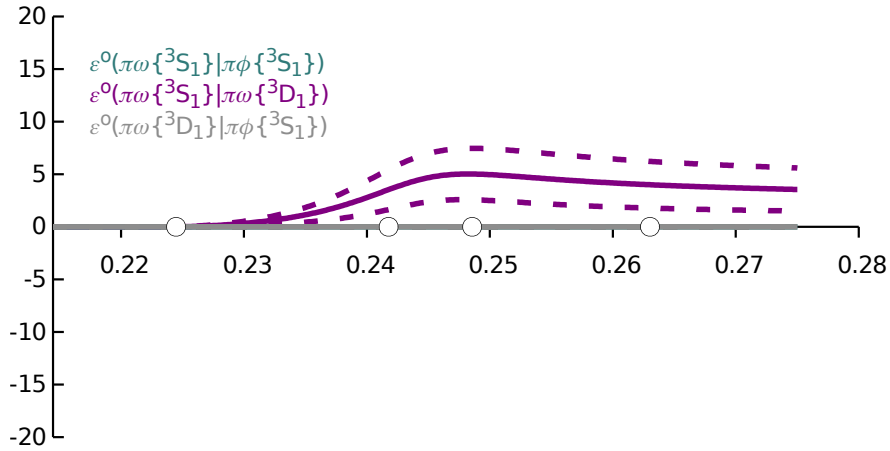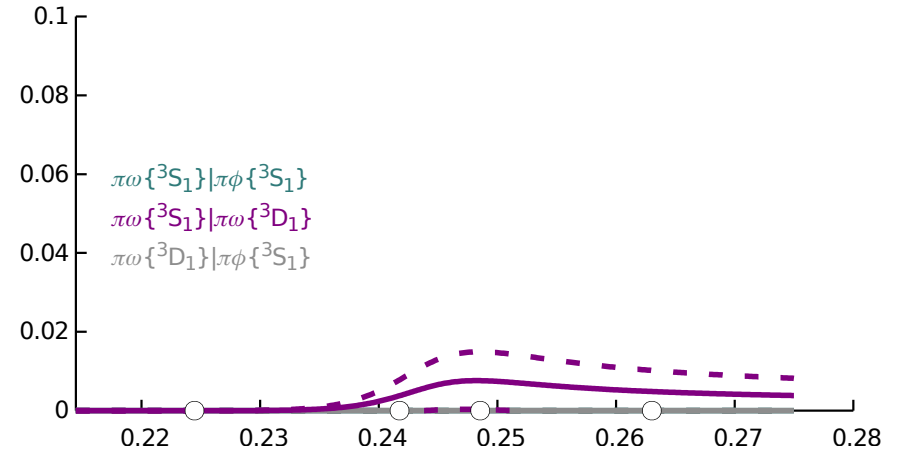



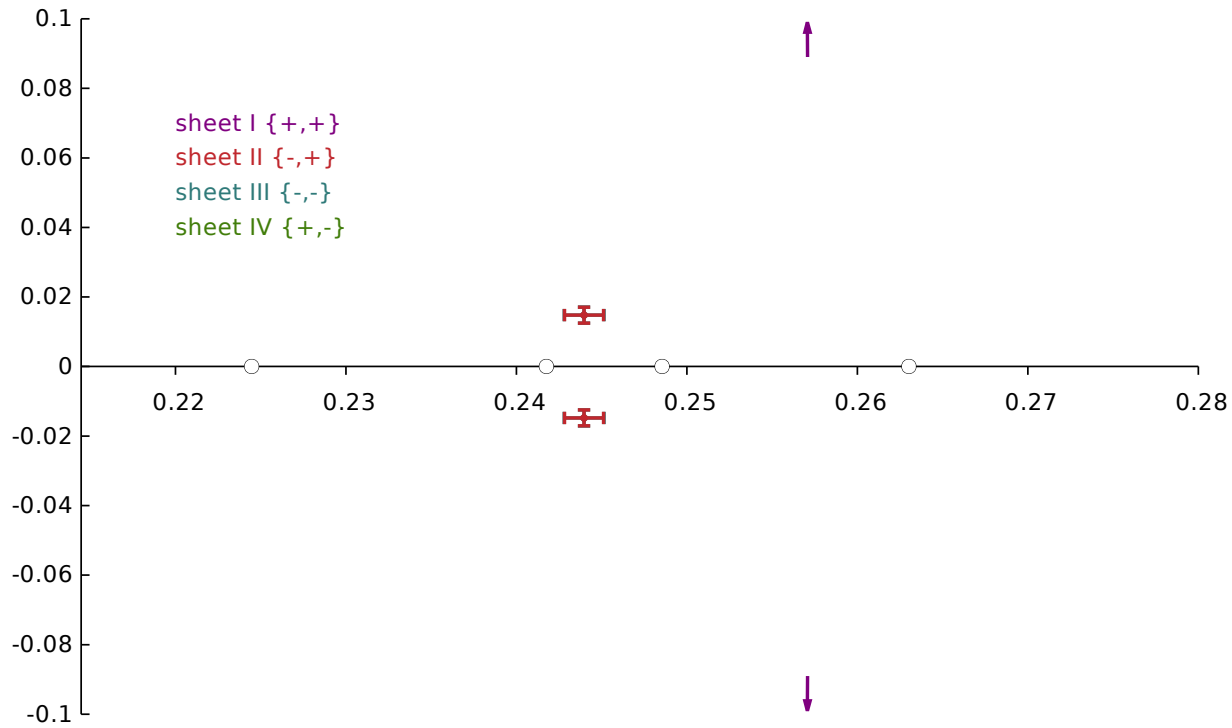

### parameter values

minimised with  $\text{chisq}/\text{nDoF} = 36.06 / (36 - 6) = 1.20$

|                                               |  |                        |  |      |      |       |       |       |       |
|-----------------------------------------------|--|------------------------|--|------|------|-------|-------|-------|-------|
| JP1+_g_pi:omega/3^D_1_pole0                   |  | 0.99621 +/- 0.53534    |  | 1.00 | 0.75 | -0.18 | 0.05  | -0.03 | -0.07 |
| JP1+_g_pi:omega/3^S_1_pole0                   |  | 0.10524 +/- 0.0091527  |  |      | 1.00 | -0.38 | 0.22  | -0.01 | -0.15 |
| JP1+_gamma_pi:omega/3^S_1 pi:omega/3^S_1_orde |  | 1.3995 +/- 0.84205     |  |      |      | 1.00  | -0.96 | -0.03 | 0.05  |
| JP1+_gamma_pi:omega/3^S_1 pi:omega/3^S_1_orde |  | -32.994 +/- 15.396     |  |      |      |       | 1.00  | 0.09  | -0.04 |
| JP1+_gamma_pi:phi/3^S_1 pi:phi/3^S_1_order0   |  | 0.92718 +/- 0.28285    |  |      |      |       |       | 1.00  | -0.30 |
| JP1+_m_pole0                                  |  | 0.24656 +/- 0.00067624 |  |      |      |       |       |       | 1.00  |

### pole singularities

pi:omega[+] pi:phi[+] upper half-plane

$\text{sqrt}(s)_{\text{pole}} = (0.25708 \pm 0.012193)$   
 $+ (i/2)*(0.17392 \pm 0.055717) [0.62]$

$s_{\text{pole}} = (0.058525 \pm 0.0050058)$   
 $+ i*(0.044712 \pm 0.015735) [-0.09]$

|                         |                         |
|-------------------------|-------------------------|
| pi:omega                | pi:phi                  |
| ===== =====             |                         |
| k_re= 0.0763 +/- 0.0121 | k_re= 0.0631 +/- 0.0134 |
| k_im= 0.0681 +/- 0.0157 | k_im= 0.0762 +/- 0.0152 |
| corr= [ 0.80]           | corr= [ 0.81]           |



| pi:omega/3^S_1(*)             | pi:phi/3^S_1                 | pi:omega/3^D_1                |
|-------------------------------|------------------------------|-------------------------------|
| g = 0.1943 +/- 0.0302         | g = 0.0000 +/- 0.0000        | g = 0.0148 +/- 0.0107         |
| arg(g)/pi= -0.0990 +/- 0.0194 | arg(g)/pi= 0.5990 +/- 0.0194 | arg(g)/pi= -0.5219 +/- 0.0358 |
| g_re= 0.1850 +/- 0.0324       | g_re= -0.0000 +/- 0.0000     | g_re= -0.0010 +/- 0.0013      |
| g_im= -0.0595 +/- 0.0022      | g_im= 0.0000 +/- 0.0000      | g_im= -0.0148 +/- 0.0108      |
| corr= [ 0.90]                 | corr= [-1.00]                | corr= [-0.27]                 |
| Br = 0.3835 +/- 0.0321        | Br = 0.0000 +/- 0.0000       | Br = 0.0022 +/- 0.0029        |

--

pi:omega[+] pi:phi[+] lower half-plane

sqrt(s)\_pole = (0.25708 +/- 0.012193)  
+ (i/2)\*(-0.17392 +/- 0.055717) [-0.62]

s\_pole = (0.058525 +/- 0.0050058)  
+ i\*(-0.044712 +/- 0.015735) [ 0.09]

| pi:omega                 | pi:phi                   |
|--------------------------|--------------------------|
| k_re= -0.0763 +/- 0.0121 | k_re= -0.0631 +/- 0.0134 |
| k_im= 0.0681 +/- 0.0157  | k_im= 0.0762 +/- 0.0152  |
| corr= [-0.80]            | corr= [-0.81]            |

| pi:omega/3^S_1(*)            | pi:phi/3^S_1                 | pi:omega/3^D_1               |
|------------------------------|------------------------------|------------------------------|
| g = 0.1943 +/- 0.0302        | g = 0.0000 +/- 0.0000        | g = 0.0148 +/- 0.0107        |
| arg(g)/pi= 0.0990 +/- 0.0194 | arg(g)/pi= 0.4010 +/- 0.0194 | arg(g)/pi= 0.5219 +/- 0.0358 |
| g_re= 0.1850 +/- 0.0324      | g_re= 0.0000 +/- 0.0000      | g_re= -0.0010 +/- 0.0013     |
| g_im= 0.0595 +/- 0.0022      | g_im= 0.0000 +/- 0.0000      | g_im= 0.0148 +/- 0.0108      |
| corr= [-0.90]                | corr= [ 1.00]                | corr= [ 0.27]                |
| Br = 0.3835 +/- 0.0321       | Br = 0.0000 +/- 0.0000       | Br = 0.0022 +/- 0.0029       |

--

pi:omega[+] pi:phi[-] upper half-plane

sqrt(s)\_pole = (0.25708 +/- 0.012193)  
+ (i/2)\*(+0.17392 +/- 0.055717) [ 0.62]

s\_pole = (0.058525 +/- 0.0050058)  
+ i\*(+0.044712 +/- 0.015735) [-0.09]

| pi:omega                | pi:phi                   |
|-------------------------|--------------------------|
| k_re= 0.0763 +/- 0.0121 | k_re= -0.0631 +/- 0.0134 |
| k_im= 0.0681 +/- 0.0157 | k_im= -0.0762 +/- 0.0152 |
| corr= [ 0.80]           | corr= [ 0.81]            |

| pi:omega/3^S_1(*)             | pi:phi/3^S_1                 | pi:omega/3^D_1                |
|-------------------------------|------------------------------|-------------------------------|
| g = 0.1943 +/- 0.0302         | g = 0.0000 +/- 0.0000        | g = 0.0148 +/- 0.0107         |
| arg(g)/pi= -0.0990 +/- 0.0194 | arg(g)/pi= 0.5990 +/- 0.0194 | arg(g)/pi= -0.5219 +/- 0.0358 |
| g_re= 0.1850 +/- 0.0324       | g_re= -0.0000 +/- 0.0000     | g_re= -0.0010 +/- 0.0013      |
| g_im= -0.0595 +/- 0.0022      | g_im= 0.0000 +/- 0.0000      | g_im= -0.0148 +/- 0.0108      |
| corr= [ 0.90]                 | corr= [-1.00]                | corr= [-0.27]                 |



## 2 Unphysical Parameterizations

```

Br = 0.3835 +/- 0.0321 | Br = 0.0000 +/- 0.0000 | Br = 0.0022 +/- 0.0029 |

--
pi:omega[+] pi:phi[-] lower half-plane

sqrt(s)_pole = (0.25708 +/- 0.012193)
+ (i/2)*(-0.17392 +/- 0.055717) [-0.62]

s_pole = (0.058525 +/- 0.0050058)
+ i*(-0.044712 +/- 0.015735) [ 0.09]

=====
pi:omega | pi:phi |
=====
k_re= -0.0763 +/- 0.0121 | k_re= 0.0631 +/- 0.0134 |
k_im= 0.0681 +/- 0.0157 | k_im= -0.0762 +/- 0.0152 |
corr= [-0.80] | corr= [-0.81] |

=====
pi:omega/3^S_1(*) | pi:phi/3^S_1 | pi:omega/3^D_1 |
=====
|g|= 0.1943 +/- 0.0302 | |g|= 0.0000 +/- 0.0000 | |g|= 0.0148 +/- 0.0107 |
arg(g)/pi= 0.0990 +/- 0.0194 | arg(g)/pi= 0.4010 +/- 0.0194 | arg(g)/pi= 0.5219 +/- 0.0358 |
-----
g_re= 0.1850 +/- 0.0324 | g_re= 0.0000 +/- 0.0000 | g_re= -0.0010 +/- 0.0013 |
g_im= 0.0595 +/- 0.0022 | g_im= 0.0000 +/- 0.0000 | g_im= 0.0148 +/- 0.0108 |
corr= [-0.90] | corr= [ 1.00] | corr= [ 0.27] |
-----
Br = 0.3835 +/- 0.0321 | Br = 0.0000 +/- 0.0000 | Br = 0.0022 +/- 0.0029 |

--
pi:omega[-] pi:phi[+] upper half-plane

sqrt(s)_pole = (0.24397 +/- 0.0011434)
+ (i/2)*(+0.014781 +/- 0.0022969) [-0.56]

s_pole = (0.059465 +/- 0.00056759)
+ i*(+0.003606 +/- 0.00055108) [-0.56]

=====
pi:omega | pi:phi |
=====
k_re= -0.0454 +/- 0.0012 | k_re= 0.0138 +/- 0.0013 |
k_im= -0.0089 +/- 0.0015 | k_im= 0.0257 +/- 0.0023 |
corr= [-0.54] | corr= [ 0.29] |

=====
pi:omega/3^S_1(*) | pi:phi/3^S_1 | pi:omega/3^D_1 |
=====
|g|= 0.0930 +/- 0.0080 | |g|= 0.0000 +/- 0.0000 | |g|= 0.0083 +/- 0.0043 |
arg(g)/pi= 0.0790 +/- 0.0230 | arg(g)/pi= 0.4210 +/- 0.0230 | arg(g)/pi= 0.1429 +/- 0.0268 |
-----
g_re= 0.0902 +/- 0.0080 | g_re= 0.0000 +/- 0.0000 | g_re= 0.0074 +/- 0.0037 |
g_im= 0.0229 +/- 0.0067 | g_im= 0.0000 +/- 0.0000 | g_im= 0.0036 +/- 0.0023 |
corr= [ 0.04] | corr= [ 0.12] | corr= [ 0.97] |
-----
Br = 0.8791 +/- 0.0349 | Br = 0.0000 +/- 0.0000 | Br = 0.0069 +/- 0.0066 |

--
pi:omega[-] pi:phi[+] lower half-plane

sqrt(s)_pole = (0.24397 +/- 0.0011434)
+ (i/2)*(-0.014781 +/- 0.0022969) [ 0.56]

s_pole = (0.059465 +/- 0.00056759)
+ i*(-0.003606 +/- 0.00055108) [ 0.56]

```



## 2 Unphysical Parameterizations

```

          pi:omega |          pi:phi |
=====|=====|
k_re=  0.0454 +/- 0.0012 | k_re= -0.0138 +/- 0.0013 |
k_im= -0.0089 +/- 0.0015 | k_im=  0.0257 +/- 0.0023 |
corr= [ 0.54] | corr= [-0.29] |

          pi:omega/3^S_1(*) |          pi:phi/3^S_1 |          pi:omega/3^D_1 |
=====|=====|=====|
|g|=  0.0930 +/- 0.0080 | |g|=  0.0000 +/- 0.0000 | |g|=  0.0083 +/- 0.0043 |
arg(g)/pi= -0.0790 +/- 0.0230 | arg(g)/pi=  0.5790 +/- 0.0230 | arg(g)/pi= -0.1429 +/- 0.0268 |
-----|-----|-----|
g_re=  0.0902 +/- 0.0080 | g_re= -0.0000 +/- 0.0000 | g_re=  0.0074 +/- 0.0037 |
g_im= -0.0229 +/- 0.0067 | g_im=  0.0000 +/- 0.0000 | g_im= -0.0036 +/- 0.0023 |
corr= [-0.04] | corr= [-0.12] | corr= [-0.97] |
-----|-----|-----|
Br =  0.8791 +/- 0.0349 | Br =  0.0000 +/- 0.0000 | Br =  0.0069 +/- 0.0066 |

--
pi:omega[-] pi:phi[-] upper half-plane

sqrt(s)_pole = (0.24397 +/- 0.0011696)
               + (i/2)*(+0.014785 +/- 0.0023058) [-0.56]

s_pole = (0.059465 +/- 0.0005805)
         + i*(+0.0036071 +/- 0.00055297) [-0.56]

          pi:omega |          pi:phi |
=====|=====|
k_re= -0.0454 +/- 0.0013 | k_re= -0.0138 +/- 0.0013 |
k_im= -0.0089 +/- 0.0015 | k_im= -0.0257 +/- 0.0024 |
corr= [-0.55] | corr= [ 0.28] |

          pi:omega/3^S_1(*) |          pi:phi/3^S_1 |          pi:omega/3^D_1 |
=====|=====|=====|
|g|=  0.0930 +/- 0.0080 | |g|=  0.0000 +/- 0.0000 | |g|=  0.0083 +/- 0.0044 |
arg(g)/pi=  0.0790 +/- 0.0228 | arg(g)/pi=  0.4210 +/- 0.0228 | arg(g)/pi=  0.1430 +/- 0.0269 |
-----|-----|-----|
g_re=  0.0902 +/- 0.0079 | g_re=  0.0000 +/- 0.0000 | g_re=  0.0074 +/- 0.0037 |
g_im=  0.0228 +/- 0.0068 | g_im=  0.0000 +/- 0.0000 | g_im=  0.0036 +/- 0.0024 |
corr= [ 0.09] | corr= [ 0.08] | corr= [ 0.97] |
-----|-----|-----|
Br =  0.8792 +/- 0.0349 | Br =  0.0000 +/- 0.0000 | Br =  0.0069 +/- 0.0067 |

--
pi:omega[-] pi:phi[-] lower half-plane

sqrt(s)_pole = (0.24397 +/- 0.0011696)
               + (i/2)*(-0.014785 +/- 0.0023058) [ 0.56]

s_pole = (0.059465 +/- 0.0005805)
         + i*(-0.0036071 +/- 0.00055297) [ 0.56]

          pi:omega |          pi:phi |
=====|=====|
k_re=  0.0454 +/- 0.0013 | k_re=  0.0138 +/- 0.0013 |
k_im= -0.0089 +/- 0.0015 | k_im= -0.0257 +/- 0.0024 |
corr= [ 0.55] | corr= [-0.28] |

          pi:omega/3^S_1(*) |          pi:phi/3^S_1 |          pi:omega/3^D_1 |
=====|=====|=====|
|g|=  0.0930 +/- 0.0080 | |g|=  0.0000 +/- 0.0000 | |g|=  0.0083 +/- 0.0044 |
arg(g)/pi= -0.0790 +/- 0.0228 | arg(g)/pi=  0.5790 +/- 0.0228 | arg(g)/pi= -0.1430 +/- 0.0269 |

```



|                               |                               |                               |
|-------------------------------|-------------------------------|-------------------------------|
| $g_{re} = 0.0902 \pm 0.0079$  | $g_{re} = -0.0000 \pm 0.0000$ | $g_{re} = 0.0074 \pm 0.0037$  |
| $g_{im} = -0.0228 \pm 0.0068$ | $g_{im} = 0.0000 \pm 0.0000$  | $g_{im} = -0.0036 \pm 0.0024$ |
| $corr = [-0.09]$              | $corr = [-0.08]$              | $corr = [-0.97]$              |
| $Br = 0.8792 \pm 0.0349$      | $Br = 0.0000 \pm 0.0000$      | $Br = 0.0069 \pm 0.0067$      |

### 2.3 coupled\_po\_pp.3s1\_3d1.pole+G0\_3s1\_3sd1\_3S1+G1\_3s1+G2\_3s1.gorder0\_3s1.irho

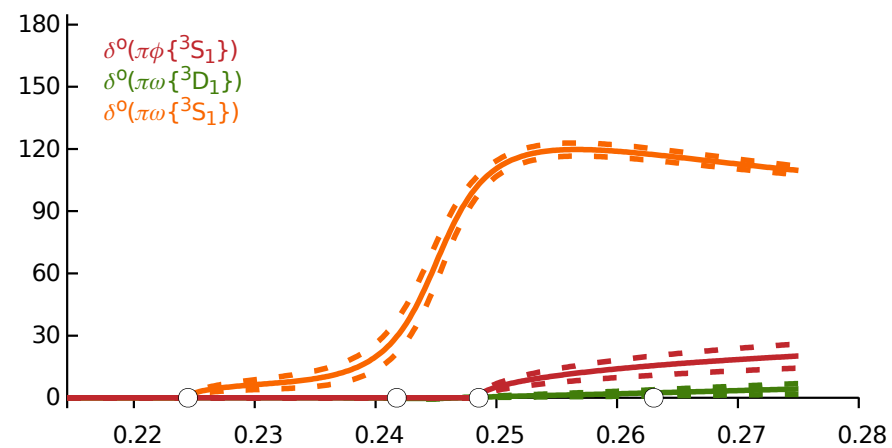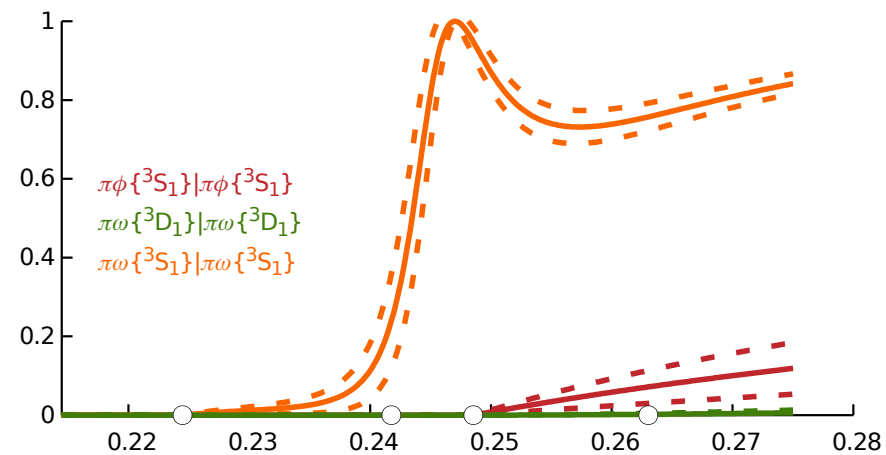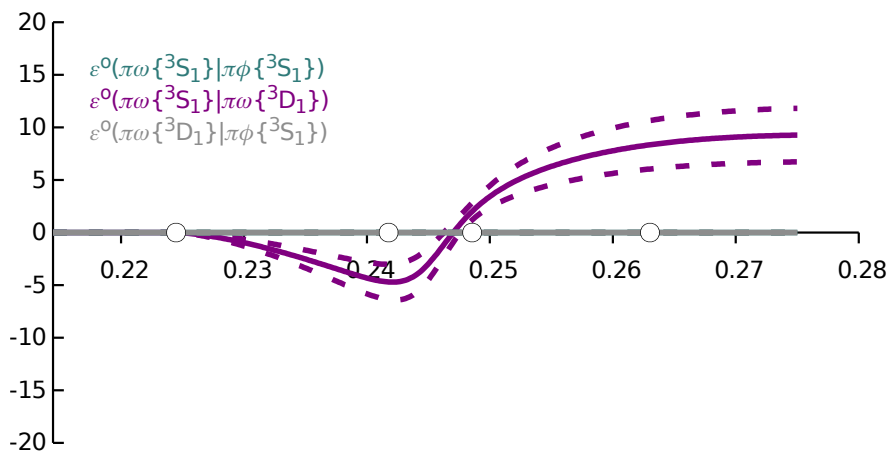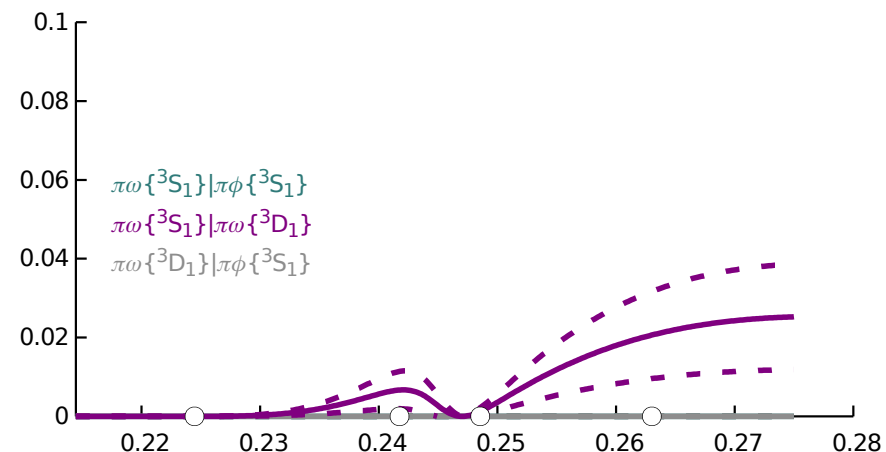



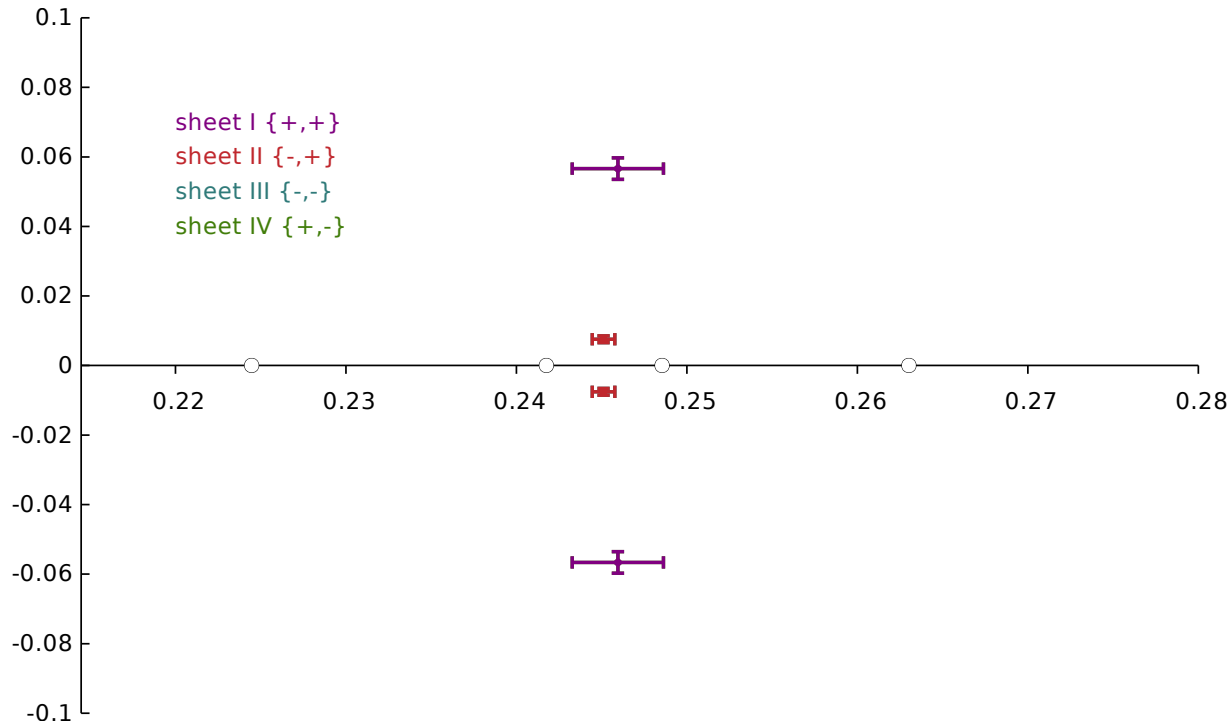

### parameter values

minimised with  $\text{chisq}/\text{nDoF} = 33.27 / (36 - 7) = 1.15$

|                                               |  |                        |  |      |       |       |       |       |       |       |
|-----------------------------------------------|--|------------------------|--|------|-------|-------|-------|-------|-------|-------|
| JP1+_g_pi:omega/3^S_1_pole0                   |  | 0.083497 +/- 0.0060229 |  | 1.00 | -0.25 | -0.19 | -0.10 | 0.03  | 0.00  | -0.05 |
| JP1+_gamma_pi:omega/3^S_1 pi:omega/3^D_1_orde |  | -38.749 +/- 13.045     |  |      | 1.00  | -0.21 | 0.06  | 0.39  | -0.08 | -0.15 |
| JP1+_gamma_pi:omega/3^S_1 pi:omega/3^S_1_orde |  | -1.8786 +/- 0.42699    |  |      |       | 1.00  | -0.44 | -0.47 | 0.01  | 0.01  |
| JP1+_gamma_pi:omega/3^S_1 pi:omega/3^S_1_orde |  | 182.15 +/- 8.4568      |  |      |       |       | 1.00  | -0.47 | 0.03  | -0.02 |
| JP1+_gamma_pi:omega/3^S_1 pi:omega/3^S_1_orde |  | -2883.3 +/- 170.62     |  |      |       |       |       | 1.00  | 0.04  | -0.04 |
| JP1+_gamma_pi:phi/3^S_1 pi:phi/3^S_1_order0   |  | 0.93625 +/- 0.28474    |  |      |       |       |       |       | 1.00  | -0.28 |
| JP1+_m_pole0                                  |  | 0.24702 +/- 0.00060479 |  |      |       |       |       |       |       | 1.00  |

### pole singularities

pi:omega[+] pi:phi[+] lower half-plane

$\sqrt{s}_{\text{pole}} = (0.24595 \pm 0.0026761)$   
 $+ (i/2) * (-0.056642 \pm 0.0031056) [-0.48]$

$s_{\text{pole}} = (0.05969 \pm 0.0012767)$   
 $+ i * (-0.013931 \pm 0.00084682) [-0.56]$

|                          |                          |
|--------------------------|--------------------------|
| pi:omega                 | pi:phi                   |
| ===== =====              | ===== =====              |
| k_re= -0.0531 +/- 0.0026 | k_re= -0.0337 +/- 0.0026 |
| k_im= 0.0295 +/- 0.0012  | k_im= 0.0414 +/- 0.0014  |



## 2 Unphysical Parameterizations

```

corr= [-0.01]          |      corr= [ 0.45]          |
=====
pi:omega/3^S_1(*) |      pi:phi/3^S_1 |      pi:omega/3^D_1 |
=====
|g|= 0.1215 +/- 0.0026 |      |g|= 0.0000 +/- 0.0000 |      |g|= 0.0341 +/- 0.0088 |
arg(g)/pi= 0.1647 +/- 0.0050 |      arg(g)/pi= 0.3353 +/- 0.0050 |      arg(g)/pi= 0.2174 +/- 0.0252 |
-----
g_re= 0.1056 +/- 0.0018 |      g_re= 0.0000 +/- 0.0000 |      g_re= 0.0265 +/- 0.0081 |
g_im= 0.0601 +/- 0.0027 |      g_im= 0.0000 +/- 0.0000 |      g_im= 0.0215 +/- 0.0044 |
corr= [ 0.59]          |      corr= [-0.06]          |      corr= [ 0.87]          |
-----
Br = 0.4056 +/- 0.0238 |      Br = 0.0000 +/- 0.0000 |      Br = 0.0320 +/- 0.0172 |

--
pi:omega[+] pi:phi[+] upper half-plane

sqrt(s)_pole = (0.24595 +/- 0.0026761)
               + (i/2)*(+0.056642 +/- 0.0031056) [ 0.48]

s_pole = (0.05969 +/- 0.0012767)
         + i*(+0.013931 +/- 0.00084682) [ 0.56]

pi:omega |      pi:phi |
=====
k_re= 0.0531 +/- 0.0026 |      k_re= 0.0337 +/- 0.0026 |
k_im= 0.0295 +/- 0.0012 |      k_im= 0.0414 +/- 0.0014 |
corr= [ 0.01]          |      corr= [-0.45]          |

pi:omega/3^S_1(*) |      pi:phi/3^S_1 |      pi:omega/3^D_1 |
=====
|g|= 0.1215 +/- 0.0026 |      |g|= 0.0000 +/- 0.0000 |      |g|= 0.0341 +/- 0.0088 |
arg(g)/pi= -0.1647 +/- 0.0050 |      arg(g)/pi= 0.6647 +/- 0.0050 |      arg(g)/pi= -0.2174 +/- 0.0252 |
-----
g_re= 0.1056 +/- 0.0018 |      g_re= -0.0000 +/- 0.0000 |      g_re= 0.0265 +/- 0.0081 |
g_im= -0.0601 +/- 0.0027 |      g_im= 0.0000 +/- 0.0000 |      g_im= -0.0215 +/- 0.0044 |
corr= [-0.59]          |      corr= [ 0.06]          |      corr= [-0.87]          |
-----
Br = 0.4056 +/- 0.0238 |      Br = 0.0000 +/- 0.0000 |      Br = 0.0320 +/- 0.0172 |

--
pi:omega[+] pi:phi[-] upper half-plane

sqrt(s)_pole = (0.24595 +/- 0.0026761)
               + (i/2)*(+0.056642 +/- 0.0031056) [ 0.48]

s_pole = (0.05969 +/- 0.0012767)
         + i*(+0.013931 +/- 0.00084682) [ 0.56]

pi:omega |      pi:phi |
=====
k_re= 0.0531 +/- 0.0026 |      k_re= -0.0337 +/- 0.0026 |
k_im= 0.0295 +/- 0.0012 |      k_im= -0.0414 +/- 0.0014 |
corr= [ 0.01]          |      corr= [-0.45]          |

pi:omega/3^S_1(*) |      pi:phi/3^S_1 |      pi:omega/3^D_1 |
=====
|g|= 0.1215 +/- 0.0026 |      |g|= 0.0000 +/- 0.0000 |      |g|= 0.0341 +/- 0.0088 |
arg(g)/pi= -0.1647 +/- 0.0050 |      arg(g)/pi= 0.6647 +/- 0.0050 |      arg(g)/pi= -0.2174 +/- 0.0252 |
-----
g_re= 0.1056 +/- 0.0018 |      g_re= -0.0000 +/- 0.0000 |      g_re= 0.0265 +/- 0.0081 |
g_im= -0.0601 +/- 0.0027 |      g_im= 0.0000 +/- 0.0000 |      g_im= -0.0215 +/- 0.0044 |
corr= [-0.59]          |      corr= [ 0.06]          |      corr= [-0.87]          |

```



## 2 Unphysical Parameterizations

```

-----|-----|-----|
      Br =  0.4056 +/- 0.0238 |      Br =  0.0000 +/- 0.0000 |      Br =  0.0320 +/- 0.0172 |

--
pi:omega[+] pi:phi[-] lower half-plane

sqrt(s)_pole = (0.24595 +/- 0.0026761)
               + (i/2)*(-0.056642 +/- 0.0031056) [-0.48]

s_pole = (0.05969 +/- 0.0012767)
         + i*(-0.013931 +/- 0.00084682) [-0.56]

=====|=====|
      pi:omega |      pi:phi |
=====|=====|
      k_re= -0.0531 +/- 0.0026 |      k_re=  0.0337 +/- 0.0026 |
      k_im=  0.0295 +/- 0.0012 |      k_im= -0.0414 +/- 0.0014 |
      corr= [-0.01]           |      corr= [ 0.45]           |

=====|=====|=====|
      pi:omega/3^S_1(*) |      pi:phi/3^S_1 |      pi:omega/3^D_1 |
=====|=====|=====|
      |g|=  0.1215 +/- 0.0026 |      |g|=  0.0000 +/- 0.0000 |      |g|=  0.0341 +/- 0.0088 |
arg(g)/pi= 0.1647 +/- 0.0050 | arg(g)/pi= 0.3353 +/- 0.0050 | arg(g)/pi= 0.2174 +/- 0.0252 |
-----|-----|-----|
      g_re=  0.1056 +/- 0.0018 |      g_re=  0.0000 +/- 0.0000 |      g_re=  0.0265 +/- 0.0081 |
      g_im=  0.0601 +/- 0.0027 |      g_im=  0.0000 +/- 0.0000 |      g_im=  0.0215 +/- 0.0044 |
      corr= [ 0.59]           |      corr= [-0.06]           |      corr= [ 0.87]           |
-----|-----|-----|
      Br =  0.4056 +/- 0.0238 |      Br =  0.0000 +/- 0.0000 |      Br =  0.0320 +/- 0.0172 |

--
pi:omega[-] pi:phi[+] upper half-plane

sqrt(s)_pole = (0.24511 +/- 0.00066447)
               + (i/2)*(+0.0075743 +/- 0.00098795) [-0.37]

s_pole = (0.060064 +/- 0.00032714)
         + i*(+0.0018565 +/- 0.00024033) [-0.36]

=====|=====|
      pi:omega |      pi:phi |
=====|=====|
      k_re= -0.0462 +/- 0.0008 |      k_re=  0.0089 +/- 0.0009 |
      k_im= -0.0045 +/- 0.0006 |      k_im=  0.0206 +/- 0.0015 |
      corr= [-0.40]           |      corr= [ 0.00]           |

=====|=====|=====|
      pi:omega/3^S_1(*) |      pi:phi/3^S_1 |      pi:omega/3^D_1 |
=====|=====|=====|
      |g|=  0.0631 +/- 0.0039 |      |g|=  0.0000 +/- 0.0000 |      |g|=  0.0080 +/- 0.0026 |
arg(g)/pi= 0.1203 +/- 0.0200 | arg(g)/pi= 0.3797 +/- 0.0200 | arg(g)/pi= 0.7080 +/- 0.0191 |
-----|-----|-----|
      g_re=  0.0586 +/- 0.0044 |      g_re=  0.0000 +/- 0.0000 |      g_re= -0.0049 +/- 0.0018 |
      g_im=  0.0233 +/- 0.0033 |      g_im=  0.0000 +/- 0.0000 |      g_im=  0.0064 +/- 0.0019 |
      corr= [-0.37]           |      corr= [ 0.33]           |      corr= [-0.95]           |
-----|-----|-----|
      Br =  0.8064 +/- 0.0169 |      Br =  0.0000 +/- 0.0000 |      Br =  0.0130 +/- 0.0085 |

--
pi:omega[-] pi:phi[+] lower half-plane

sqrt(s)_pole = (0.24511 +/- 0.00066447)
               + (i/2)*(-0.0075743 +/- 0.00098795) [ 0.37]

s_pole = (0.060064 +/- 0.00032714)
         + i*(-0.0018565 +/- 0.00024033) [ 0.36]

```



| pi:omega                 |                          | pi:phi |       |
|--------------------------|--------------------------|--------|-------|
| =====                    | =====                    | =====  | ===== |
| k_re= 0.0462 +/- 0.0008  | k_re= -0.0089 +/- 0.0009 |        |       |
| k_im= -0.0045 +/- 0.0006 | k_im= 0.0206 +/- 0.0015  |        |       |
| corr= [ 0.40]            | corr= [-0.00]            |        |       |

| pi:omega/3^S_1(*)             |                              | pi:phi/3^S_1                  |       | pi:omega/3^D_1 |       |
|-------------------------------|------------------------------|-------------------------------|-------|----------------|-------|
| =====                         | =====                        | =====                         | ===== | =====          | ===== |
| g = 0.0631 +/- 0.0039         | g = 0.0000 +/- 0.0000        | g = 0.0080 +/- 0.0026         |       |                |       |
| arg(g)/pi= -0.1203 +/- 0.0200 | arg(g)/pi= 0.6203 +/- 0.0200 | arg(g)/pi= -0.7080 +/- 0.0191 |       |                |       |
| -----                         | -----                        | -----                         |       |                |       |
| g_re= 0.0586 +/- 0.0044       | g_re= -0.0000 +/- 0.0000     | g_re= -0.0049 +/- 0.0018      |       |                |       |
| g_im= -0.0233 +/- 0.0033      | g_im= 0.0000 +/- 0.0000      | g_im= -0.0064 +/- 0.0019      |       |                |       |
| corr= [ 0.37]                 | corr= [-0.33]                | corr= [ 0.95]                 |       |                |       |
| -----                         | -----                        | -----                         |       |                |       |
| Br = 0.8064 +/- 0.0169        | Br = 0.0000 +/- 0.0000       | Br = 0.0130 +/- 0.0085        |       |                |       |

--

pi:omega[-] pi:phi[-] upper half-plane

sqrt(s)\_pole = (0.24511 +/- 0.00066447)  
+ (i/2)\*(+0.0075743 +/- 0.00098795) [-0.37]

s\_pole = (0.060064 +/- 0.00032714)  
+ i\*(+0.0018565 +/- 0.00024033) [-0.36]

| pi:omega                 |                          | pi:phi |       |
|--------------------------|--------------------------|--------|-------|
| =====                    | =====                    | =====  | ===== |
| k_re= -0.0462 +/- 0.0008 | k_re= -0.0089 +/- 0.0009 |        |       |
| k_im= -0.0045 +/- 0.0006 | k_im= -0.0206 +/- 0.0015 |        |       |
| corr= [-0.40]            | corr= [ 0.00]            |        |       |

| pi:omega/3^S_1(*)            |                              | pi:phi/3^S_1                 |       | pi:omega/3^D_1 |       |
|------------------------------|------------------------------|------------------------------|-------|----------------|-------|
| =====                        | =====                        | =====                        | ===== | =====          | ===== |
| g = 0.0631 +/- 0.0039        | g = 0.0000 +/- 0.0000        | g = 0.0080 +/- 0.0026        |       |                |       |
| arg(g)/pi= 0.1203 +/- 0.0200 | arg(g)/pi= 0.3797 +/- 0.0200 | arg(g)/pi= 0.7080 +/- 0.0191 |       |                |       |
| -----                        | -----                        | -----                        |       |                |       |
| g_re= 0.0586 +/- 0.0044      | g_re= 0.0000 +/- 0.0000      | g_re= -0.0049 +/- 0.0018     |       |                |       |
| g_im= 0.0233 +/- 0.0033      | g_im= 0.0000 +/- 0.0000      | g_im= 0.0064 +/- 0.0019      |       |                |       |
| corr= [-0.37]                | corr= [ 0.33]                | corr= [-0.95]                |       |                |       |
| -----                        | -----                        | -----                        |       |                |       |
| Br = 0.8064 +/- 0.0169       | Br = 0.0000 +/- 0.0000       | Br = 0.0130 +/- 0.0085       |       |                |       |

--

pi:omega[-] pi:phi[-] lower half-plane

sqrt(s)\_pole = (0.24511 +/- 0.00066447)  
+ (i/2)\*(-0.0075743 +/- 0.00098795) [ 0.37]

s\_pole = (0.060064 +/- 0.00032714)  
+ i\*(-0.0018565 +/- 0.00024033) [ 0.36]

| pi:omega                 |                          | pi:phi |       |
|--------------------------|--------------------------|--------|-------|
| =====                    | =====                    | =====  | ===== |
| k_re= 0.0462 +/- 0.0008  | k_re= 0.0089 +/- 0.0009  |        |       |
| k_im= -0.0045 +/- 0.0006 | k_im= -0.0206 +/- 0.0015 |        |       |
| corr= [ 0.40]            | corr= [-0.00]            |        |       |

| pi:omega/3^S_1(*)     |                       | pi:phi/3^S_1          |       | pi:omega/3^D_1 |       |
|-----------------------|-----------------------|-----------------------|-------|----------------|-------|
| =====                 | =====                 | =====                 | ===== | =====          | ===== |
| g = 0.0631 +/- 0.0039 | g = 0.0000 +/- 0.0000 | g = 0.0080 +/- 0.0026 |       |                |       |



|                                      |                                      |                                      |
|--------------------------------------|--------------------------------------|--------------------------------------|
| $\arg(g)/\pi = -0.1203 \pm 0.0200$   | $\arg(g)/\pi = 0.6203 \pm 0.0200$    | $\arg(g)/\pi = -0.7080 \pm 0.0191$   |
| $g_{\text{re}} = 0.0586 \pm 0.0044$  | $g_{\text{re}} = -0.0000 \pm 0.0000$ | $g_{\text{re}} = -0.0049 \pm 0.0018$ |
| $g_{\text{im}} = -0.0233 \pm 0.0033$ | $g_{\text{im}} = 0.0000 \pm 0.0000$  | $g_{\text{im}} = -0.0064 \pm 0.0019$ |
| $\text{corr} = [0.37]$               | $\text{corr} = [-0.33]$              | $\text{corr} = [0.95]$               |
| $\text{Br} = 0.8064 \pm 0.0169$      | $\text{Br} = 0.0000 \pm 0.0000$      | $\text{Br} = 0.0130 \pm 0.0085$      |

## 2.4 coupled\_po\_pp.3s1\_3d1.pole+G0\_3s1\_3sd1\_3S1+G1\_3s1+G2\_3s1.gorder0\_3s1.pole0\_sub

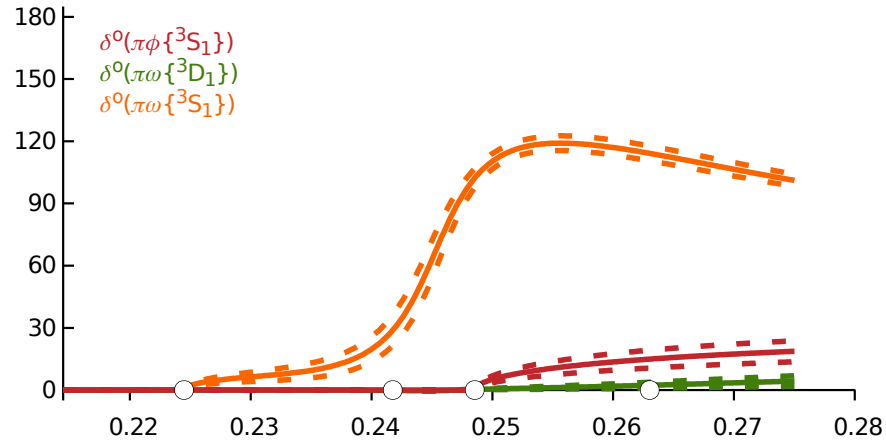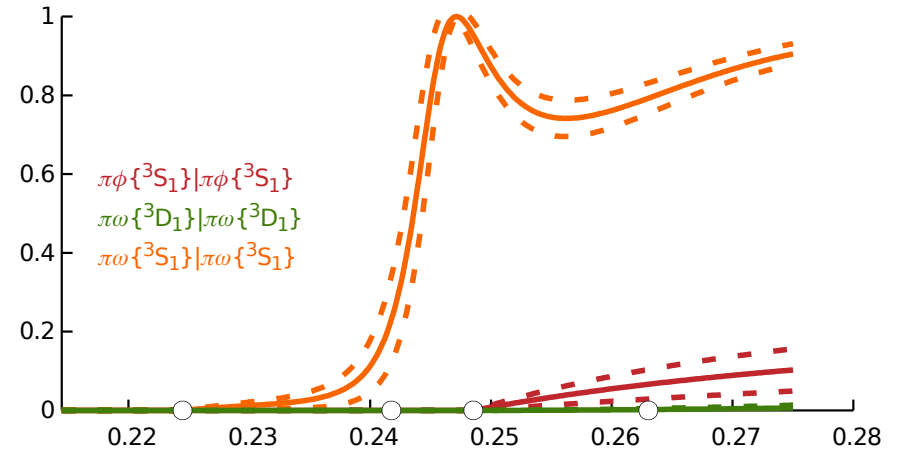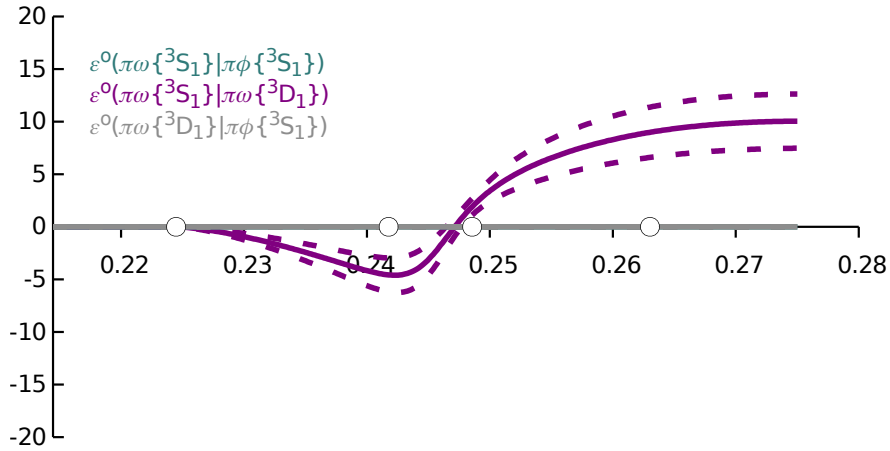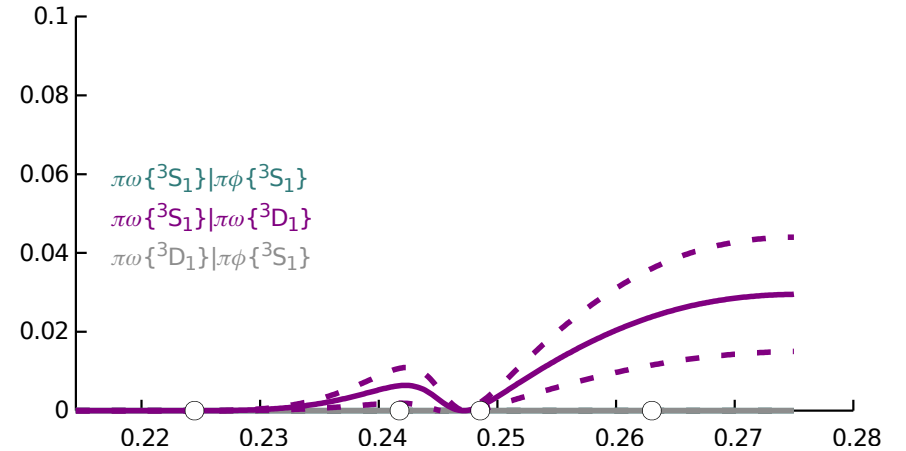



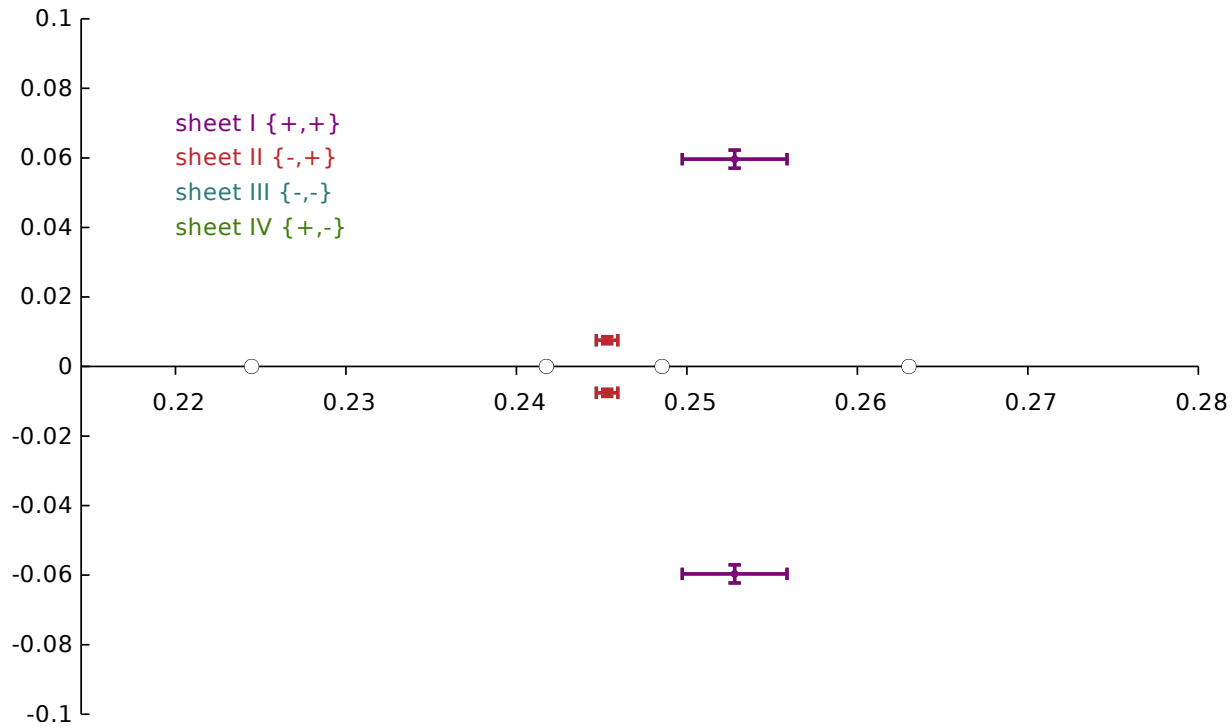

### parameter values

minimised with  $\text{chisq}/\text{nDoF} = 33.28 / (36 - 7) = 1.15$

|                                               |  |                        |  |      |       |       |       |       |       |       |
|-----------------------------------------------|--|------------------------|--|------|-------|-------|-------|-------|-------|-------|
| JP1+_g_pi:omega/3^S_1_pole0                   |  | 0.080358 +/- 0.0054111 |  | 1.00 | -0.24 | -0.22 | -0.07 | 0.09  | 0.00  | -0.04 |
| JP1+_gamma_pi:omega/3^S_1 pi:omega/3^D_1_orde |  | -36.122 +/- 12.164     |  |      | 1.00  | -0.29 | 0.05  | 0.44  | -0.09 | -0.14 |
| JP1+_gamma_pi:omega/3^S_1 pi:omega/3^S_1_orde |  | -2.3050 +/- 0.4453     |  |      |       | 1.00  | -0.47 | -0.50 | -0.00 | 0.03  |
| JP1+_gamma_pi:omega/3^S_1 pi:omega/3^S_1_orde |  | 181.29 +/- 8.5216      |  |      |       |       | 1.00  | -0.44 | 0.02  | -0.02 |
| JP1+_gamma_pi:omega/3^S_1 pi:omega/3^S_1_orde |  | -2696.5 +/- 171.85     |  |      |       |       |       | 1.00  | 0.04  | -0.05 |
| JP1+_gamma_pi:phi/3^S_1 pi:phi/3^S_1_order0   |  | 0.87190 +/- 0.2461     |  |      |       |       |       |       | 1.00  | -0.17 |
| JP1+_m_pole0                                  |  | 0.24714 +/- 0.00056675 |  |      |       |       |       |       |       | 1.00  |

### pole singularities

pi:omega[+] pi:phi[+] lower half-plane

$\text{sqrt}(s)_{\text{pole}} = (0.2528 \pm 0.0030699) + (i/2)(-0.059651 \pm 0.0026119) [-0.41]$

$s_{\text{pole}} = (0.063017 \pm 0.0015221) + i(-0.01508 \pm 0.00075364) [-0.56]$

|                          |  |                          |  |
|--------------------------|--|--------------------------|--|
| pi:omega                 |  | pi:phi                   |  |
| =====                    |  | =====                    |  |
| k_re= -0.0595 +/- 0.0028 |  | k_re= -0.0399 +/- 0.0029 |  |
| k_im= 0.0289 +/- 0.0011  |  | k_im= 0.0388 +/- 0.0015  |  |



## 2 Unphysical Parameterizations

```

corr= [ 0.20]          |      corr= [ 0.60]          |
=====|=====|=====
      pi:omega/3^S_1(*) |      pi:phi/3^S_1 |      pi:omega/3^D_1 |
=====|=====|=====
      |g|= 0.1422 +/- 0.0022 |      |g|= 0.0000 +/- 0.0000 |      |g|= 0.0377 +/- 0.0097 |
arg(g)/pi= 0.2315 +/- 0.0078 | arg(g)/pi= 0.2685 +/- 0.0078 | arg(g)/pi= 0.2829 +/- 0.0231 |
-----|-----|-----
      g_re= 0.1062 +/- 0.0019 |      g_re= 0.0000 +/- 0.0000 |      g_re= 0.0238 +/- 0.0078 |
      g_im= 0.0945 +/- 0.0036 |      g_im= 0.0000 +/- 0.0000 |      g_im= 0.0293 +/- 0.0065 |
      corr= [-0.44]          |      corr= [-0.55]          |      corr= [ 0.93]          |
-----|-----|-----
      Br = 0.5801 +/- 0.0298 |      Br = 0.0000 +/- 0.0000 |      Br = 0.0408 +/- 0.0215 |

--
pi:omega[+] pi:phi[+] upper half-plane

sqrt(s)_pole = ( 0.2528 +/- 0.0030699)
               + (i/2)*(+0.059651 +/- 0.0026119) [ 0.41]

s_pole = (0.063017 +/- 0.0015221)
         + i*(+0.01508 +/- 0.00075364) [ 0.56]

      pi:omega |      pi:phi |
=====|=====|
      k_re= 0.0595 +/- 0.0028 |      k_re= 0.0399 +/- 0.0029 |
      k_im= 0.0289 +/- 0.0011 |      k_im= 0.0388 +/- 0.0015 |
      corr= [-0.20]          |      corr= [-0.60]          |

      pi:omega/3^S_1(*) |      pi:phi/3^S_1 |      pi:omega/3^D_1 |
=====|=====|=====
      |g|= 0.1422 +/- 0.0022 |      |g|= 0.0000 +/- 0.0000 |      |g|= 0.0377 +/- 0.0097 |
arg(g)/pi= -0.2315 +/- 0.0078 | arg(g)/pi= 0.7315 +/- 0.0078 | arg(g)/pi= -0.2829 +/- 0.0231 |
-----|-----|-----
      g_re= 0.1062 +/- 0.0019 |      g_re= -0.0000 +/- 0.0000 |      g_re= 0.0238 +/- 0.0078 |
      g_im= -0.0945 +/- 0.0036 |      g_im= 0.0000 +/- 0.0000 |      g_im= -0.0293 +/- 0.0065 |
      corr= [ 0.44]          |      corr= [ 0.55]          |      corr= [-0.93]          |
-----|-----|-----
      Br = 0.5801 +/- 0.0298 |      Br = 0.0000 +/- 0.0000 |      Br = 0.0408 +/- 0.0215 |

--
pi:omega[+] pi:phi[-] upper half-plane

sqrt(s)_pole = ( 0.2528 +/- 0.0030699)
               + (i/2)*(+0.059651 +/- 0.0026119) [ 0.41]

s_pole = (0.063017 +/- 0.0015221)
         + i*(+0.01508 +/- 0.00075364) [ 0.56]

      pi:omega |      pi:phi |
=====|=====|
      k_re= 0.0595 +/- 0.0028 |      k_re= -0.0399 +/- 0.0029 |
      k_im= 0.0289 +/- 0.0011 |      k_im= -0.0388 +/- 0.0015 |
      corr= [-0.20]          |      corr= [-0.60]          |

      pi:omega/3^S_1(*) |      pi:phi/3^S_1 |      pi:omega/3^D_1 |
=====|=====|=====
      |g|= 0.1422 +/- 0.0022 |      |g|= 0.0000 +/- 0.0000 |      |g|= 0.0377 +/- 0.0097 |
arg(g)/pi= -0.2315 +/- 0.0078 | arg(g)/pi= 0.7315 +/- 0.0078 | arg(g)/pi= -0.2829 +/- 0.0231 |
-----|-----|-----
      g_re= 0.1062 +/- 0.0019 |      g_re= -0.0000 +/- 0.0000 |      g_re= 0.0238 +/- 0.0078 |
      g_im= -0.0945 +/- 0.0036 |      g_im= 0.0000 +/- 0.0000 |      g_im= -0.0293 +/- 0.0065 |
      corr= [ 0.44]          |      corr= [ 0.55]          |      corr= [-0.93]          |
-----|-----|-----

```



## 2 Unphysical Parameterizations

```

-----|-----|-----|
Br = 0.5801 +/- 0.0298 | Br = 0.0000 +/- 0.0000 | Br = 0.0408 +/- 0.0215 |

--
pi:omega[+] pi:phi[-] lower half-plane

sqrt(s)_pole = ( 0.2528 +/- 0.0030699)
               + (i/2)*(-0.059651 +/- 0.0026119) [-0.41]

s_pole = (0.063017 +/- 0.0015221)
          + i*(-0.01508 +/- 0.00075364) [-0.56]

=====|=====|
pi:omega | pi:phi |
=====|=====|
k_re= -0.0595 +/- 0.0028 | k_re= 0.0399 +/- 0.0029 |
k_im= 0.0289 +/- 0.0011 | k_im= -0.0388 +/- 0.0015 |
corr= [ 0.20] | corr= [ 0.60] |

=====|=====|=====|
pi:omega/3^S_1(*) | pi:phi/3^S_1 | pi:omega/3^D_1 |
=====|=====|=====|
|g|= 0.1422 +/- 0.0022 | |g|= 0.0000 +/- 0.0000 | |g|= 0.0377 +/- 0.0097 |
arg(g)/pi= 0.2315 +/- 0.0078 | arg(g)/pi= 0.2685 +/- 0.0078 | arg(g)/pi= 0.2829 +/- 0.0231 |
-----|-----|-----|
g_re= 0.1062 +/- 0.0019 | g_re= 0.0000 +/- 0.0000 | g_re= 0.0238 +/- 0.0078 |
g_im= 0.0945 +/- 0.0036 | g_im= 0.0000 +/- 0.0000 | g_im= 0.0293 +/- 0.0065 |
corr= [-0.44] | corr= [-0.55] | corr= [ 0.93] |
-----|-----|-----|
Br = 0.5801 +/- 0.0298 | Br = 0.0000 +/- 0.0000 | Br = 0.0408 +/- 0.0215 |

--
pi:omega[-] pi:phi[+] upper half-plane

sqrt(s)_pole = (0.24532 +/- 0.00062782)
               + (i/2)*(+0.0075705 +/- 0.00099665) [-0.34]

s_pole = (0.060169 +/- 0.00030934)
          + i*(+0.0018572 +/- 0.00024292) [-0.33]

=====|=====|
pi:omega | pi:phi |
=====|=====|
k_re= -0.0465 +/- 0.0007 | k_re= 0.0091 +/- 0.0010 |
k_im= -0.0045 +/- 0.0006 | k_im= 0.0202 +/- 0.0015 |
corr= [-0.37] | corr= [ 0.03] |

=====|=====|=====|
pi:omega/3^S_1(*) | pi:phi/3^S_1 | pi:omega/3^D_1 |
=====|=====|=====|
|g|= 0.0630 +/- 0.0039 | |g|= 0.0000 +/- 0.0000 | |g|= 0.0079 +/- 0.0025 |
arg(g)/pi= 0.1141 +/- 0.0194 | arg(g)/pi= 0.3859 +/- 0.0194 | arg(g)/pi= 0.7059 +/- 0.0191 |
-----|-----|-----|
g_re= 0.0590 +/- 0.0045 | g_re= 0.0000 +/- 0.0000 | g_re= -0.0048 +/- 0.0018 |
g_im= 0.0221 +/- 0.0031 | g_im= 0.0000 +/- 0.0000 | g_im= 0.0063 +/- 0.0019 |
corr= [-0.40] | corr= [ 0.43] | corr= [-0.95] |
-----|-----|-----|
Br = 0.8066 +/- 0.0168 | Br = 0.0000 +/- 0.0000 | Br = 0.0127 +/- 0.0082 |

--
pi:omega[-] pi:phi[+] lower half-plane

sqrt(s)_pole = (0.24532 +/- 0.00062782)
               + (i/2)*(-0.0075705 +/- 0.00099665) [ 0.34]

s_pole = (0.060169 +/- 0.00030934)
          + i*(-0.0018572 +/- 0.00024292) [ 0.33]

```



| pi:omega                 | pi:phi                   |
|--------------------------|--------------------------|
| =====                    | =====                    |
| k_re= 0.0465 +/- 0.0007  | k_re= -0.0091 +/- 0.0010 |
| k_im= -0.0045 +/- 0.0006 | k_im= 0.0202 +/- 0.0015  |
| corr= [ 0.37]            | corr= [-0.03]            |

| pi:omega/3^S_1(*)             | pi:phi/3^S_1                 | pi:omega/3^D_1                |
|-------------------------------|------------------------------|-------------------------------|
| =====                         | =====                        | =====                         |
| g = 0.0630 +/- 0.0039         | g = 0.0000 +/- 0.0000        | g = 0.0079 +/- 0.0025         |
| arg(g)/pi= -0.1141 +/- 0.0194 | arg(g)/pi= 0.6141 +/- 0.0194 | arg(g)/pi= -0.7059 +/- 0.0191 |
| -----                         | -----                        | -----                         |
| g_re= 0.0590 +/- 0.0045       | g_re= -0.0000 +/- 0.0000     | g_re= -0.0048 +/- 0.0018      |
| g_im= -0.0221 +/- 0.0031      | g_im= 0.0000 +/- 0.0000      | g_im= -0.0063 +/- 0.0019      |
| corr= [ 0.40]                 | corr= [-0.43]                | corr= [ 0.95]                 |
| -----                         | -----                        | -----                         |
| Br = 0.8066 +/- 0.0168        | Br = 0.0000 +/- 0.0000       | Br = 0.0127 +/- 0.0082        |

--

pi:omega[-] pi:phi[-] upper half-plane

sqrt(s)\_pole = (0.24532 +/- 0.00062782)  
+ (i/2)\*(+0.0075705 +/- 0.00099665) [-0.34]

s\_pole = (0.060169 +/- 0.00030934)  
+ i\*(+0.0018572 +/- 0.00024292) [-0.33]

| pi:omega                 | pi:phi                   |
|--------------------------|--------------------------|
| =====                    | =====                    |
| k_re= -0.0465 +/- 0.0007 | k_re= -0.0091 +/- 0.0010 |
| k_im= -0.0045 +/- 0.0006 | k_im= -0.0202 +/- 0.0015 |
| corr= [-0.37]            | corr= [ 0.03]            |

| pi:omega/3^S_1(*)            | pi:phi/3^S_1                 | pi:omega/3^D_1               |
|------------------------------|------------------------------|------------------------------|
| =====                        | =====                        | =====                        |
| g = 0.0630 +/- 0.0039        | g = 0.0000 +/- 0.0000        | g = 0.0079 +/- 0.0025        |
| arg(g)/pi= 0.1141 +/- 0.0194 | arg(g)/pi= 0.3859 +/- 0.0194 | arg(g)/pi= 0.7059 +/- 0.0191 |
| -----                        | -----                        | -----                        |
| g_re= 0.0590 +/- 0.0045      | g_re= 0.0000 +/- 0.0000      | g_re= -0.0048 +/- 0.0018     |
| g_im= 0.0221 +/- 0.0031      | g_im= 0.0000 +/- 0.0000      | g_im= 0.0063 +/- 0.0019      |
| corr= [-0.40]                | corr= [ 0.43]                | corr= [-0.95]                |
| -----                        | -----                        | -----                        |
| Br = 0.8066 +/- 0.0168       | Br = 0.0000 +/- 0.0000       | Br = 0.0127 +/- 0.0082       |

--

pi:omega[-] pi:phi[-] lower half-plane

sqrt(s)\_pole = (0.24532 +/- 0.00062782)  
+ (i/2)\*(-0.0075705 +/- 0.00099665) [ 0.34]

s\_pole = (0.060169 +/- 0.00030934)  
+ i\*(-0.0018572 +/- 0.00024292) [ 0.33]

| pi:omega                 | pi:phi                   |
|--------------------------|--------------------------|
| =====                    | =====                    |
| k_re= 0.0465 +/- 0.0007  | k_re= 0.0091 +/- 0.0010  |
| k_im= -0.0045 +/- 0.0006 | k_im= -0.0202 +/- 0.0015 |
| corr= [ 0.37]            | corr= [-0.03]            |

| pi:omega/3^S_1(*)     | pi:phi/3^S_1          | pi:omega/3^D_1        |
|-----------------------|-----------------------|-----------------------|
| =====                 | =====                 | =====                 |
| g = 0.0630 +/- 0.0039 | g = 0.0000 +/- 0.0000 | g = 0.0079 +/- 0.0025 |



|                                      |                                      |                                      |
|--------------------------------------|--------------------------------------|--------------------------------------|
| $\arg(g)/\pi = -0.1141 \pm 0.0194$   | $\arg(g)/\pi = 0.6141 \pm 0.0194$    | $\arg(g)/\pi = -0.7059 \pm 0.0191$   |
| $g_{\text{re}} = 0.0590 \pm 0.0045$  | $g_{\text{re}} = -0.0000 \pm 0.0000$ | $g_{\text{re}} = -0.0048 \pm 0.0018$ |
| $g_{\text{im}} = -0.0221 \pm 0.0031$ | $g_{\text{im}} = 0.0000 \pm 0.0000$  | $g_{\text{im}} = -0.0063 \pm 0.0019$ |
| $\text{corr} = [0.40]$               | $\text{corr} = [-0.43]$              | $\text{corr} = [0.95]$               |
| $\text{Br} = 0.8066 \pm 0.0168$      | $\text{Br} = 0.0000 \pm 0.0000$      | $\text{Br} = 0.0127 \pm 0.0082$      |

## 2.5 coupled\_po\_pp.3s1\_3d1.pole+G0\_3s1\_3sd1\_3S1+G1\_3s1+G2\_3s1.gorder0\_3s1.threshold\_sub

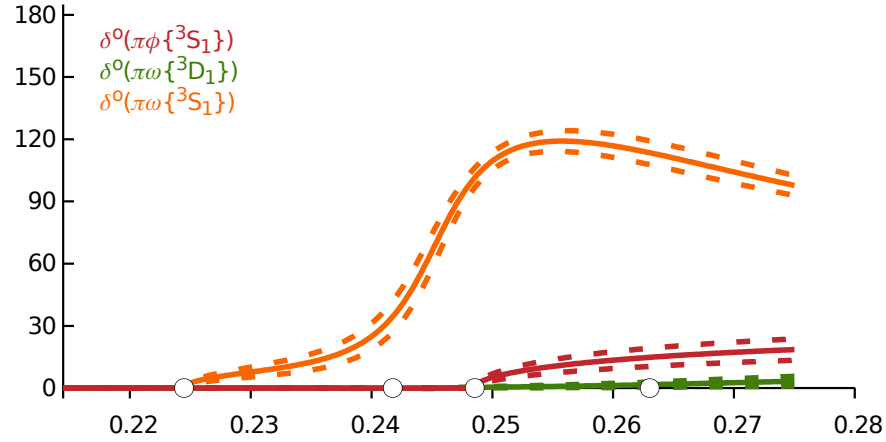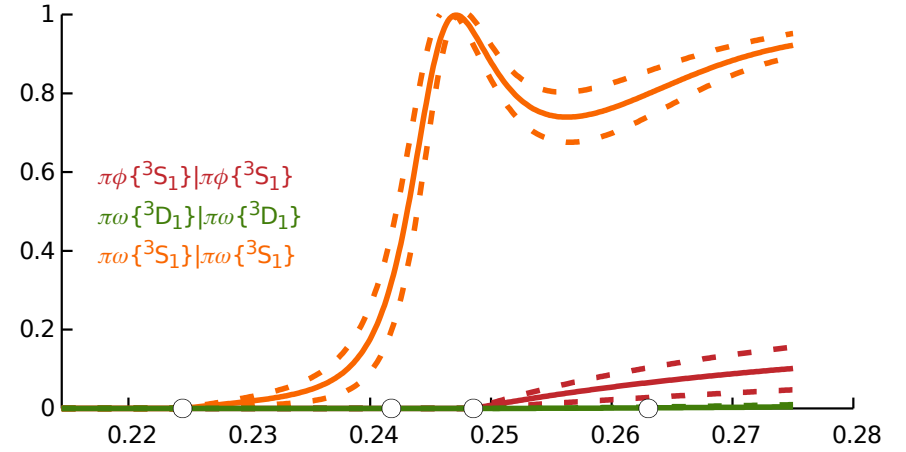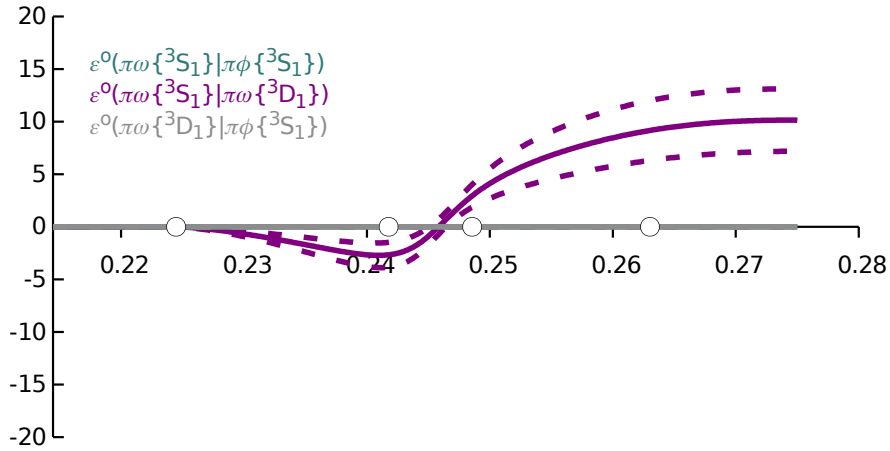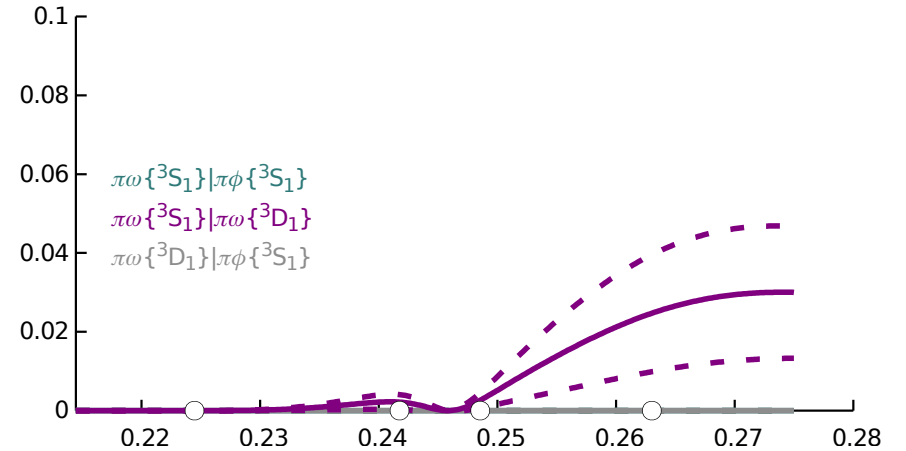



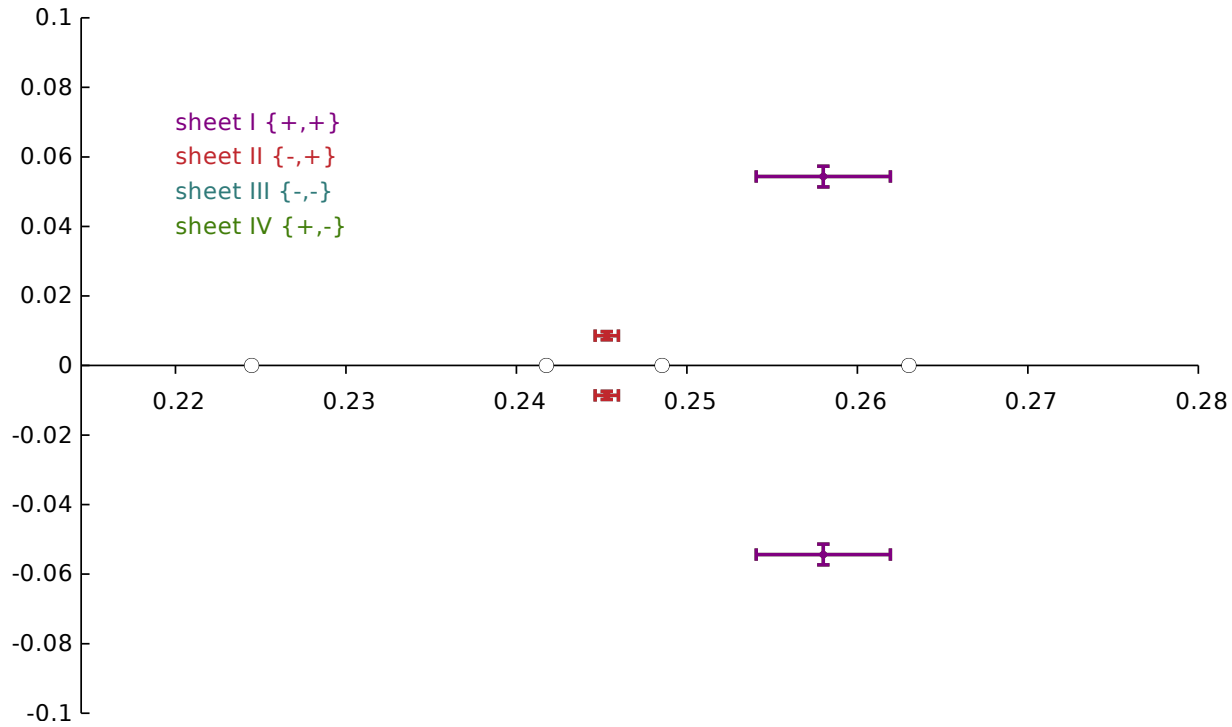

### parameter values

minimised with  $\text{chisq}/\text{nDoF} = 33.45 / (36 - 7) = 1.15$

|                                               |  |                        |  |      |       |       |       |       |       |       |
|-----------------------------------------------|--|------------------------|--|------|-------|-------|-------|-------|-------|-------|
| JP1+_g_pi:omega/3^S_1_pole0                   |  | 0.076185 +/- 0.0052365 |  | 1.00 | -0.05 | -0.39 | -0.04 | 0.39  | 0.13  | -0.46 |
| JP1+_gamma_pi:omega/3^S_1 pi:omega/3^D_1_orde |  | -27.465 +/- 10.958     |  |      | 1.00  | -0.29 | 0.02  | 0.45  | -0.03 | -0.08 |
| JP1+_gamma_pi:omega/3^S_1 pi:omega/3^S_1_orde |  | -2.8793 +/- 0.4829     |  |      |       | 1.00  | -0.46 | -0.46 | -0.01 | 0.13  |
| JP1+_gamma_pi:omega/3^S_1 pi:omega/3^S_1_orde |  | 179.07 +/- 9.5617      |  |      |       |       | 1.00  | -0.51 | 0.02  | 0.01  |
| JP1+_gamma_pi:omega/3^S_1 pi:omega/3^S_1_orde |  | -2387.3 +/- 180.34     |  |      |       |       |       | 1.00  | 0.05  | -0.15 |
| JP1+_gamma_pi:phi/3^S_1 pi:phi/3^S_1_order0   |  | 0.93893 +/- 0.29637    |  |      |       |       |       |       | 1.00  | -0.29 |
| JP1+_m_pole0                                  |  | 0.24583 +/- 0.00061697 |  |      |       |       |       |       |       | 1.00  |

### pole singularities

pi:omega[+] pi:phi[+] lower half-plane

$\text{sqrt}(s)_{\text{pole}} = (0.258 \pm 0.0039337) + (i/2)(-0.054362 \pm 0.0029824) [-0.39]$

$s_{\text{pole}} = (0.065827 \pm 0.0019996) + i(-0.014026 \pm 0.00087529) [-0.56]$

|                          |  |                          |  |
|--------------------------|--|--------------------------|--|
| pi:omega                 |  | pi:phi                   |  |
| k_re= -0.0633 +/- 0.0035 |  | k_re= -0.0431 +/- 0.0038 |  |
| k_im= 0.0254 +/- 0.0012  |  | k_im= 0.0340 +/- 0.0018  |  |



```

corr= [ 0.19]          |      corr= [ 0.61]          |
=====
pi:omega/3^S_1(*) |      pi:phi/3^S_1 |      pi:omega/3^D_1 |
=====
|g|= 0.1332 +/- 0.0029 |      |g|= 0.0000 +/- 0.0000 |      |g|= 0.0338 +/- 0.0101 |
arg(g)/pi= 0.2775 +/- 0.0082 |      arg(g)/pi= 0.2225 +/- 0.0082 |      arg(g)/pi= 0.3290 +/- 0.0254 |
-----
g_re= 0.0857 +/- 0.0018 |      g_re= 0.0000 +/- 0.0000 |      g_re= 0.0173 +/- 0.0070 |
g_im= 0.1020 +/- 0.0041 |      g_im= 0.0000 +/- 0.0000 |      g_im= 0.0290 +/- 0.0078 |
corr= [-0.40]          |      corr= [-0.06]          |      corr= [ 0.93]          |
-----
Br = 0.5882 +/- 0.0320 |      Br = 0.0000 +/- 0.0000 |      Br = 0.0378 +/- 0.0230 |

--
pi:omega[+] pi:phi[+] upper half-plane

sqrt(s)_pole = ( 0.258 +/- 0.0039337)
               + (i/2)*(+0.054362 +/- 0.0029824) [ 0.39]

s_pole = (0.065827 +/- 0.0019996)
         + i*(+0.014026 +/- 0.00087529) [ 0.56]

=====
pi:omega |      pi:phi |
=====
k_re= 0.0633 +/- 0.0035 |      k_re= 0.0431 +/- 0.0038 |
k_im= 0.0254 +/- 0.0012 |      k_im= 0.0340 +/- 0.0018 |
corr= [-0.19]          |      corr= [-0.61]          |

=====
pi:omega/3^S_1(*) |      pi:phi/3^S_1 |      pi:omega/3^D_1 |
=====
|g|= 0.1332 +/- 0.0029 |      |g|= 0.0000 +/- 0.0000 |      |g|= 0.0338 +/- 0.0101 |
arg(g)/pi= -0.2775 +/- 0.0082 |      arg(g)/pi= 0.7775 +/- 0.0082 |      arg(g)/pi= -0.3290 +/- 0.0254 |
-----
g_re= 0.0857 +/- 0.0018 |      g_re= -0.0000 +/- 0.0000 |      g_re= 0.0173 +/- 0.0070 |
g_im= -0.1020 +/- 0.0041 |      g_im= 0.0000 +/- 0.0000 |      g_im= -0.0290 +/- 0.0078 |
corr= [ 0.40]          |      corr= [ 0.06]          |      corr= [-0.93]          |
-----
Br = 0.5882 +/- 0.0320 |      Br = 0.0000 +/- 0.0000 |      Br = 0.0378 +/- 0.0230 |

--
pi:omega[+] pi:phi[-] upper half-plane

sqrt(s)_pole = ( 0.258 +/- 0.0039337)
               + (i/2)*(+0.054362 +/- 0.0029824) [ 0.39]

s_pole = (0.065827 +/- 0.0019996)
         + i*(+0.014026 +/- 0.00087529) [ 0.56]

=====
pi:omega |      pi:phi |
=====
k_re= 0.0633 +/- 0.0035 |      k_re= -0.0431 +/- 0.0038 |
k_im= 0.0254 +/- 0.0012 |      k_im= -0.0340 +/- 0.0018 |
corr= [-0.19]          |      corr= [-0.61]          |

=====
pi:omega/3^S_1(*) |      pi:phi/3^S_1 |      pi:omega/3^D_1 |
=====
|g|= 0.1332 +/- 0.0029 |      |g|= 0.0000 +/- 0.0000 |      |g|= 0.0338 +/- 0.0101 |
arg(g)/pi= -0.2775 +/- 0.0082 |      arg(g)/pi= 0.7775 +/- 0.0082 |      arg(g)/pi= -0.3290 +/- 0.0254 |
-----
g_re= 0.0857 +/- 0.0018 |      g_re= -0.0000 +/- 0.0000 |      g_re= 0.0173 +/- 0.0070 |
g_im= -0.1020 +/- 0.0041 |      g_im= 0.0000 +/- 0.0000 |      g_im= -0.0290 +/- 0.0078 |
corr= [ 0.40]          |      corr= [ 0.06]          |      corr= [-0.93]          |

```



## 2 Unphysical Parameterizations

```

-----|-----|-----|
      Br = 0.5882 +/- 0.0320 |      Br = 0.0000 +/- 0.0000 |      Br = 0.0378 +/- 0.0230 |

--
pi:omega[+] pi:phi[-] lower half-plane

sqrt(s)_pole = ( 0.258 +/- 0.0039337)
               + (i/2)*(-0.054362 +/- 0.0029824) [-0.39]

s_pole = (0.065827 +/- 0.0019996)
         + i*(-0.014026 +/- 0.00087529) [-0.56]

=====|=====|
      pi:omega |      pi:phi |
=====|=====|
      k_re= -0.0633 +/- 0.0035 |      k_re= 0.0431 +/- 0.0038 |
      k_im= 0.0254 +/- 0.0012 |      k_im= -0.0340 +/- 0.0018 |
      corr= [ 0.19] |      corr= [ 0.61] |

=====|=====|
      pi:omega/3^S_1(*) |      pi:phi/3^S_1 |      pi:omega/3^D_1 |
=====|=====|
      |g|= 0.1332 +/- 0.0029 |      |g|= 0.0000 +/- 0.0000 |      |g|= 0.0338 +/- 0.0101 |
arg(g)/pi= 0.2775 +/- 0.0082 | arg(g)/pi= 0.2225 +/- 0.0082 | arg(g)/pi= 0.3290 +/- 0.0254 |
-----|-----|-----|
      g_re= 0.0857 +/- 0.0018 |      g_re= 0.0000 +/- 0.0000 |      g_re= 0.0173 +/- 0.0070 |
      g_im= 0.1020 +/- 0.0041 |      g_im= 0.0000 +/- 0.0000 |      g_im= 0.0290 +/- 0.0078 |
      corr= [-0.40] |      corr= [-0.06] |      corr= [ 0.93] |
-----|-----|-----|
      Br = 0.5882 +/- 0.0320 |      Br = 0.0000 +/- 0.0000 |      Br = 0.0378 +/- 0.0230 |

--
pi:omega[-] pi:phi[+] upper half-plane

sqrt(s)_pole = ( 0.2453 +/- 0.00068214)
               + (i/2)*(+0.0085951 +/- 0.0011888) [-0.27]

s_pole = (0.060152 +/- 0.00033608)
         + i*(+0.0021084 +/- 0.00029008) [-0.27]

=====|=====|
      pi:omega |      pi:phi |
=====|=====|
      k_re= -0.0465 +/- 0.0008 |      k_re= 0.0101 +/- 0.0011 |
      k_im= -0.0051 +/- 0.0007 |      k_im= 0.0207 +/- 0.0015 |
      corr= [-0.29] |      corr= [ 0.04] |

=====|=====|
      pi:omega/3^S_1(*) |      pi:phi/3^S_1 |      pi:omega/3^D_1 |
=====|=====|
      |g|= 0.0669 +/- 0.0047 |      |g|= 0.0000 +/- 0.0000 |      |g|= 0.0065 +/- 0.0024 |
arg(g)/pi= 0.0984 +/- 0.0240 | arg(g)/pi= 0.4016 +/- 0.0240 | arg(g)/pi= 0.6200 +/- 0.0231 |
-----|-----|-----|
      g_re= 0.0637 +/- 0.0055 |      g_re= 0.0000 +/- 0.0000 |      g_re= -0.0024 +/- 0.0012 |
      g_im= 0.0203 +/- 0.0041 |      g_im= 0.0000 +/- 0.0000 |      g_im= 0.0060 +/- 0.0021 |
      corr= [-0.52] |      corr= [ 0.46] |      corr= [-0.94] |
-----|-----|-----|
      Br = 0.8005 +/- 0.0212 |      Br = 0.0000 +/- 0.0000 |      Br = 0.0075 +/- 0.0056 |

--
pi:omega[-] pi:phi[+] lower half-plane

sqrt(s)_pole = ( 0.2453 +/- 0.00068214)
               + (i/2)*(-0.0085951 +/- 0.0011888) [ 0.27]

s_pole = (0.060152 +/- 0.00033608)
         + i*(-0.0021084 +/- 0.00029008) [ 0.27]

```



| pi:omega                 | pi:phi                   |
|--------------------------|--------------------------|
| =====                    | =====                    |
| k_re= 0.0465 +/- 0.0008  | k_re= -0.0101 +/- 0.0011 |
| k_im= -0.0051 +/- 0.0007 | k_im= 0.0207 +/- 0.0015  |
| corr= [ 0.29]            | corr= [-0.04]            |

| pi:omega/3^S_1(*)             | pi:phi/3^S_1                 | pi:omega/3^D_1                |
|-------------------------------|------------------------------|-------------------------------|
| =====                         | =====                        | =====                         |
| g = 0.0669 +/- 0.0047         | g = 0.0000 +/- 0.0000        | g = 0.0065 +/- 0.0024         |
| arg(g)/pi= -0.0984 +/- 0.0240 | arg(g)/pi= 0.5984 +/- 0.0240 | arg(g)/pi= -0.6200 +/- 0.0231 |
| -----                         | -----                        | -----                         |
| g_re= 0.0637 +/- 0.0055       | g_re= -0.0000 +/- 0.0000     | g_re= -0.0024 +/- 0.0012      |
| g_im= -0.0203 +/- 0.0041      | g_im= 0.0000 +/- 0.0000      | g_im= -0.0060 +/- 0.0021      |
| corr= [ 0.52]                 | corr= [-0.46]                | corr= [ 0.94]                 |
| -----                         | -----                        | -----                         |
| Br = 0.8005 +/- 0.0212        | Br = 0.0000 +/- 0.0000       | Br = 0.0075 +/- 0.0056        |

--

pi:omega[-] pi:phi[-] upper half-plane

sqrt(s)\_pole = ( 0.2453 +/- 0.00068214)  
 + (i/2)\*(+0.0085951 +/- 0.0011888) [-0.27]

s\_pole = (0.060152 +/- 0.00033608)  
 + i\*(+0.0021084 +/- 0.00029008) [-0.27]

| pi:omega                 | pi:phi                   |
|--------------------------|--------------------------|
| =====                    | =====                    |
| k_re= -0.0465 +/- 0.0008 | k_re= -0.0101 +/- 0.0011 |
| k_im= -0.0051 +/- 0.0007 | k_im= -0.0207 +/- 0.0015 |
| corr= [-0.29]            | corr= [ 0.04]            |

| pi:omega/3^S_1(*)            | pi:phi/3^S_1                 | pi:omega/3^D_1               |
|------------------------------|------------------------------|------------------------------|
| =====                        | =====                        | =====                        |
| g = 0.0669 +/- 0.0047        | g = 0.0000 +/- 0.0000        | g = 0.0065 +/- 0.0024        |
| arg(g)/pi= 0.0984 +/- 0.0240 | arg(g)/pi= 0.4016 +/- 0.0240 | arg(g)/pi= 0.6200 +/- 0.0231 |
| -----                        | -----                        | -----                        |
| g_re= 0.0637 +/- 0.0055      | g_re= 0.0000 +/- 0.0000      | g_re= -0.0024 +/- 0.0012     |
| g_im= 0.0203 +/- 0.0041      | g_im= 0.0000 +/- 0.0000      | g_im= 0.0060 +/- 0.0021      |
| corr= [-0.52]                | corr= [ 0.46]                | corr= [-0.94]                |
| -----                        | -----                        | -----                        |
| Br = 0.8005 +/- 0.0212       | Br = 0.0000 +/- 0.0000       | Br = 0.0075 +/- 0.0056       |

--

pi:omega[-] pi:phi[-] lower half-plane

sqrt(s)\_pole = ( 0.2453 +/- 0.00068214)  
 + (i/2)\*(-0.0085951 +/- 0.0011888) [ 0.27]

s\_pole = (0.060152 +/- 0.00033608)  
 + i\*(-0.0021084 +/- 0.00029008) [ 0.27]

| pi:omega                 | pi:phi                   |
|--------------------------|--------------------------|
| =====                    | =====                    |
| k_re= 0.0465 +/- 0.0008  | k_re= 0.0101 +/- 0.0011  |
| k_im= -0.0051 +/- 0.0007 | k_im= -0.0207 +/- 0.0015 |
| corr= [ 0.29]            | corr= [-0.04]            |

| pi:omega/3^S_1(*)     | pi:phi/3^S_1          | pi:omega/3^D_1        |
|-----------------------|-----------------------|-----------------------|
| =====                 | =====                 | =====                 |
| g = 0.0669 +/- 0.0047 | g = 0.0000 +/- 0.0000 | g = 0.0065 +/- 0.0024 |



|                                      |                                      |                                      |
|--------------------------------------|--------------------------------------|--------------------------------------|
| $\arg(g)/\pi = -0.0984 \pm 0.0240$   | $\arg(g)/\pi = 0.5984 \pm 0.0240$    | $\arg(g)/\pi = -0.6200 \pm 0.0231$   |
| $g_{\text{re}} = 0.0637 \pm 0.0055$  | $g_{\text{re}} = -0.0000 \pm 0.0000$ | $g_{\text{re}} = -0.0024 \pm 0.0012$ |
| $g_{\text{im}} = -0.0203 \pm 0.0041$ | $g_{\text{im}} = 0.0000 \pm 0.0000$  | $g_{\text{im}} = -0.0060 \pm 0.0021$ |
| $\text{corr} = [0.52]$               | $\text{corr} = [-0.46]$              | $\text{corr} = [0.94]$               |
| $\text{Br} = 0.8005 \pm 0.0212$      | $\text{Br} = 0.0000 \pm 0.0000$      | $\text{Br} = 0.0075 \pm 0.0056$      |

## 2.6 coupled\_po\_pp.3s1\_3d1.pole+G0\_3s1\_3sd1\_3S1+G1\_3s1.gorder0\_3s1\_3d1\_3S1.irho

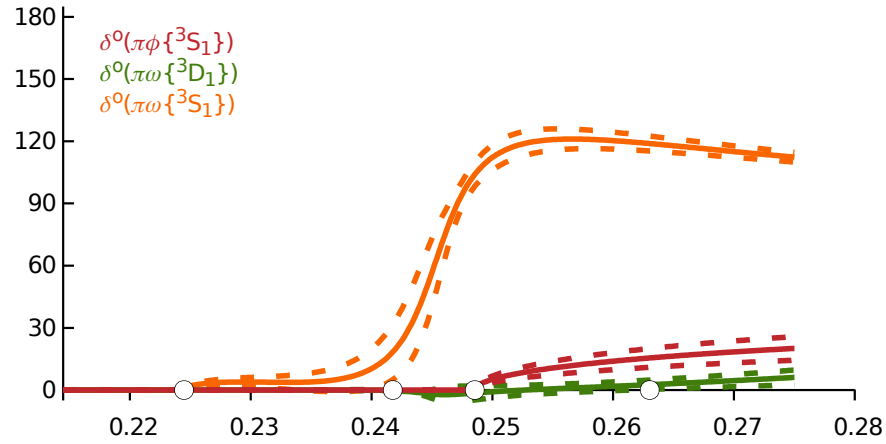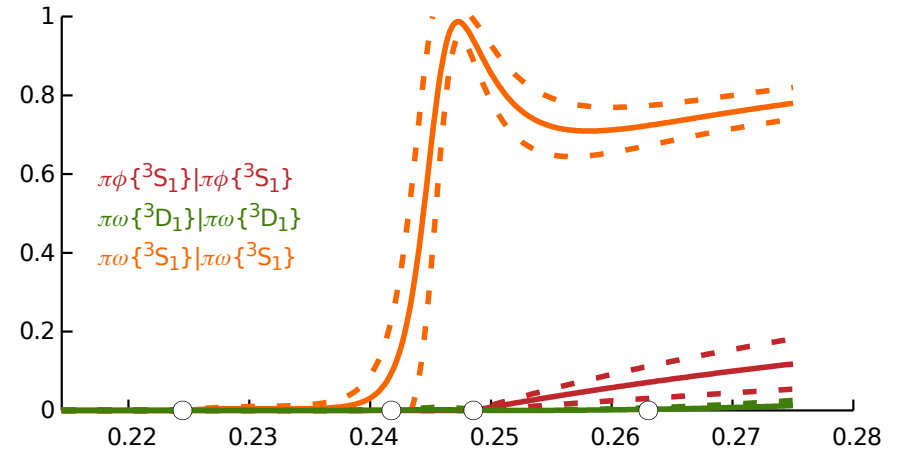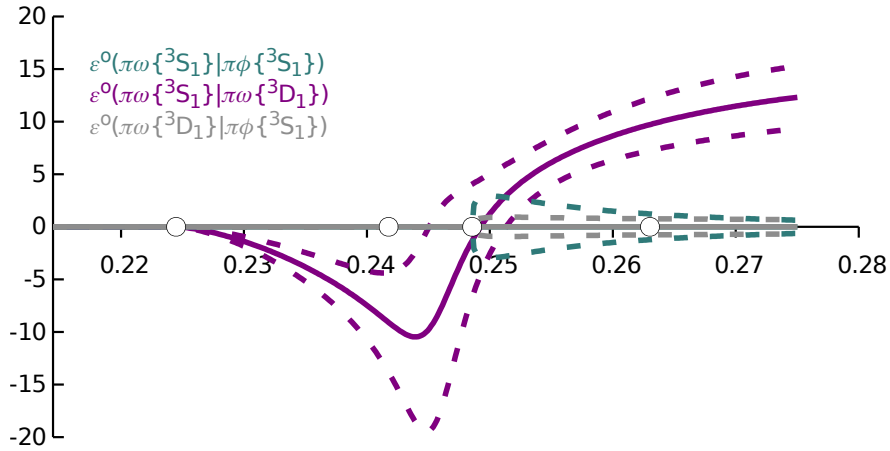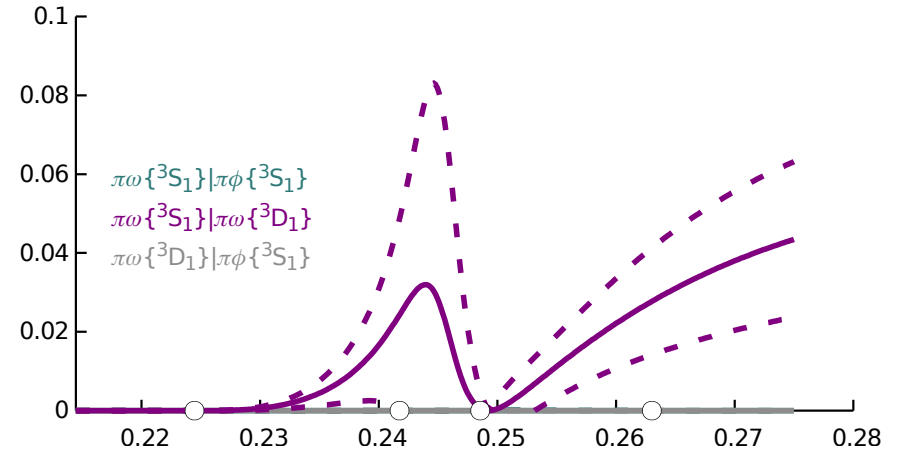



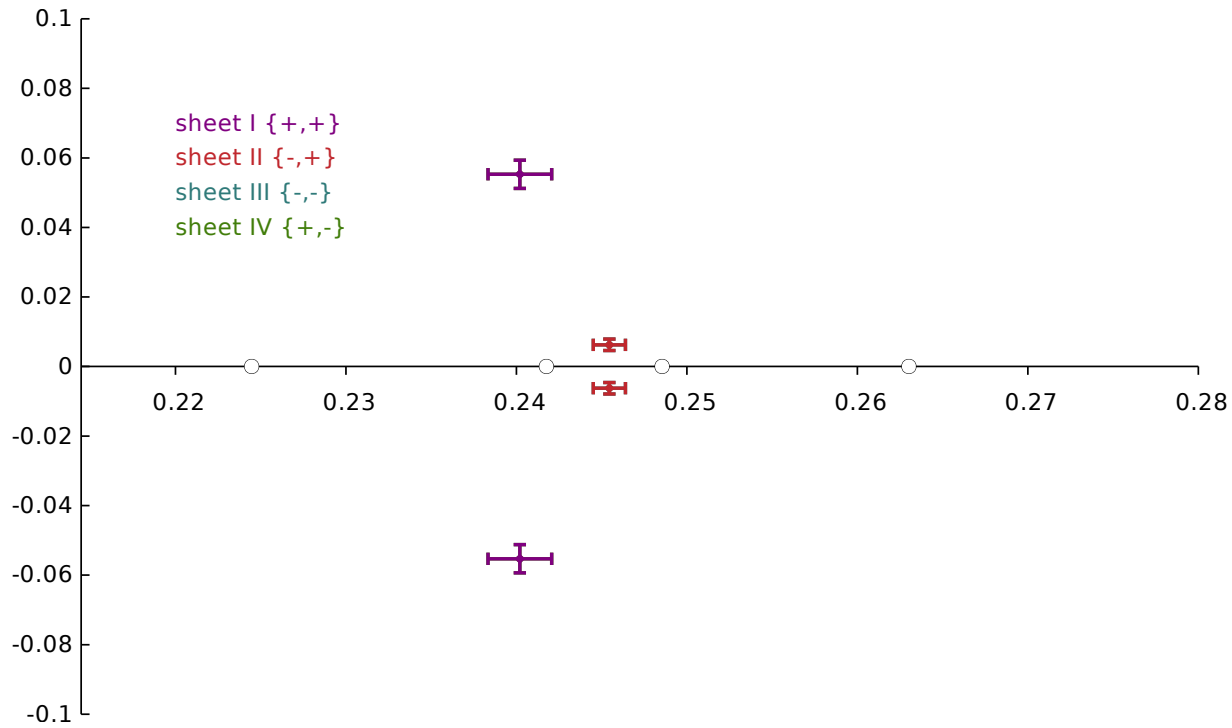

### parameter values

minimised with  $\text{chisq}/\text{nDoF} = 32.91 / (36 - 8) = 1.18$

|                                               |                          |      |      |       |      |       |       |       |       |
|-----------------------------------------------|--------------------------|------|------|-------|------|-------|-------|-------|-------|
| JP1+_g_pi:omega/3^D_1_pole0                   | -0.68305 +/- 0.96363     | 1.00 | 0.91 | -0.03 | 0.38 | -0.23 | -0.02 | -0.07 | -0.11 |
| JP1+_g_pi:omega/3^S_1_pole0                   | 0.076070 +/- 0.014463    |      | 1.00 | -0.03 | 0.24 | -0.27 | -0.04 | -0.06 | -0.15 |
| JP1+_g_pi:phi/3^S_1_pole0                     | -1.5893e-06 +/- 0.012991 |      |      | 1.00  | 0.00 | 0.01  | 0.00  | -0.01 | -0.06 |
| JP1+_gamma_pi:omega/3^S_1 pi:omega/3^D_1_orde | -49.282 +/- 13.536       |      |      |       | 1.00 | -0.24 | 0.30  | -0.12 | -0.16 |
| JP1+_gamma_pi:omega/3^S_1 pi:omega/3^S_1_orde | 8.0064 +/- 0.5651        |      |      |       |      | 1.00  | -0.91 | 0.02  | 0.04  |
| JP1+_gamma_pi:omega/3^S_1 pi:omega/3^S_1_orde | -158.42 +/- 10.981       |      |      |       |      |       | 1.00  | 0.04  | -0.02 |
| JP1+_gamma_pi:phi/3^S_1 pi:phi/3^S_1_order0   | 0.93319 +/- 0.28313      |      |      |       |      |       |       | 1.00  | -0.25 |
| JP1+_m_pole0                                  | 0.24712 +/- 0.00054717   |      |      |       |      |       |       |       | 1.00  |

### pole singularities

pi:omega[+] pi:phi[+] upper half-plane

$\text{sqrt}(s)_{\text{pole}} = (0.2402 \pm 0.0018646)$   
 $+ (i/2) * (+0.055298 \pm 0.0040575) [0.05]$

$s_{\text{pole}} = (0.056932 \pm 0.00089714)$   
 $+ i * (+0.013283 \pm 0.0009852) [0.03]$

|                         |                         |
|-------------------------|-------------------------|
| pi:omega                | pi:phi                  |
| =====                   | =====                   |
| k_re= 0.0479 +/- 0.0018 | k_re= 0.0291 +/- 0.0018 |



## 2 Unphysical Parameterizations

```

k_im= 0.0309 +/- 0.0019 | k_im= 0.0444 +/- 0.0018 |
corr= [ 0.10] | corr= [ 0.09] |

```

```

          pi:omega/3^S_1(*) |          pi:phi/3^S_1 |          pi:omega/3^D_1 |
=====|=====|=====|
|g|= 0.1272 +/- 0.0037 | |g|= 0.0001 +/- 0.0019 | |g|= 0.0394 +/- 0.0083 |
arg(g)/pi= -0.1319 +/- 0.0039 | arg(g)/pi= 0.4997 +/- 11.1461 | arg(g)/pi= -0.0993 +/- 0.0151 |
-----|-----|-----|
g_re= 0.1165 +/- 0.0037 | g_re= 0.0000 +/- 0.0031 | g_re= 0.0375 +/- 0.0080 |
g_im= -0.0512 +/- 0.0017 | g_im= 0.0000 +/- 0.0003 | g_im= -0.0121 +/- 0.0031 |
corr= [-0.49] | corr= [-1.00] | corr= [-0.77] |
-----|-----|-----|
Br = 0.4043 +/- 0.0333 | Br = 0.0000 +/- 0.0000 | Br = 0.0387 +/- 0.0183 |

```

```

--
pi:omega[+] pi:phi[+] lower half-plane

```

```

sqrt(s)_pole = ( 0.2402 +/- 0.0018646)
               + (i/2)*(-0.055298 +/- 0.0040575) [-0.05]

```

```

s_pole = (0.056932 +/- 0.00089714)
         + i*(-0.013283 +/- 0.0009852) [-0.03]

```

```

          pi:omega |          pi:phi |
=====|=====|
k_re= -0.0479 +/- 0.0018 | k_re= -0.0291 +/- 0.0018 |
k_im= 0.0309 +/- 0.0019 | k_im= 0.0444 +/- 0.0018 |
corr= [-0.10] | corr= [-0.09] |

```

```

          pi:omega/3^S_1(*) |          pi:phi/3^S_1 |          pi:omega/3^D_1 |
=====|=====|=====|
|g|= 0.1272 +/- 0.0037 | |g|= 0.0001 +/- 0.0019 | |g|= 0.0394 +/- 0.0083 |
arg(g)/pi= 0.1319 +/- 0.0039 | arg(g)/pi= -0.4997 +/- 11.1461 | arg(g)/pi= 0.0993 +/- 0.0151 |
-----|-----|-----|
g_re= 0.1165 +/- 0.0037 | g_re= 0.0000 +/- 0.0031 | g_re= 0.0375 +/- 0.0080 |
g_im= 0.0512 +/- 0.0017 | g_im= -0.0000 +/- 0.0003 | g_im= 0.0121 +/- 0.0031 |
corr= [ 0.49] | corr= [ 1.00] | corr= [ 0.77] |
-----|-----|-----|
Br = 0.4043 +/- 0.0333 | Br = 0.0000 +/- 0.0000 | Br = 0.0387 +/- 0.0183 |

```

```

--
pi:omega[+] pi:phi[-] upper half-plane

```

```

sqrt(s)_pole = ( 0.2402 +/- 0.0018646)
               + (i/2)*(+0.055298 +/- 0.0040575) [ 0.05]

```

```

s_pole = (0.056932 +/- 0.00089714)
         + i*(+0.013283 +/- 0.00098521) [ 0.03]

```

```

          pi:omega |          pi:phi |
=====|=====|
k_re= 0.0479 +/- 0.0018 | k_re= -0.0291 +/- 0.0018 |
k_im= 0.0309 +/- 0.0019 | k_im= -0.0444 +/- 0.0018 |
corr= [ 0.10] | corr= [ 0.09] |

```

```

          pi:omega/3^S_1(*) |          pi:phi/3^S_1 |          pi:omega/3^D_1 |
=====|=====|=====|
|g|= 0.1272 +/- 0.0037 | |g|= 0.0002 +/- 0.0035 | |g|= 0.0394 +/- 0.0083 |
arg(g)/pi= -0.1319 +/- 0.0039 | arg(g)/pi= 0.3203 +/- 11.1547 | arg(g)/pi= -0.0993 +/- 0.0151 |
-----|-----|-----|
g_re= 0.1165 +/- 0.0037 | g_re= 0.0000 +/- 0.0045 | g_re= 0.0375 +/- 0.0080 |
g_im= -0.0512 +/- 0.0017 | g_im= -0.0000 +/- 0.0035 | g_im= -0.0121 +/- 0.0031 |

```



## 2 Unphysical Parameterizations

```

corr= [-0.49] | corr= [-1.00] | corr= [-0.77] |
-----|-----|-----|
Br = 0.4043 +/- 0.0333 | Br = 0.0000 +/- 0.0000 | Br = 0.0387 +/- 0.0183 |

--
pi:omega[+] pi:phi[-] lower half-plane

sqrt(s)_pole = ( 0.2402 +/- 0.0018646)
               + (i/2)*(-0.055298 +/- 0.0040575) [-0.05]

s_pole = (0.056932 +/- 0.00089714)
         + i*(-0.013283 +/- 0.00098521) [-0.03]

=====|=====|
pi:omega | pi:phi |
=====|=====|
k_re= -0.0479 +/- 0.0018 | k_re= 0.0291 +/- 0.0018 |
k_im= 0.0309 +/- 0.0019 | k_im= -0.0444 +/- 0.0018 |
corr= [-0.10] | corr= [-0.09] |

=====|=====|
pi:omega/3^S_1(*) | pi:phi/3^S_1 | pi:omega/3^D_1 |
=====|=====|=====|
|g|= 0.1272 +/- 0.0037 | |g|= 0.0002 +/- 0.0035 | |g|= 0.0394 +/- 0.0083 |
arg(g)/pi= 0.1319 +/- 0.0039 | arg(g)/pi= -0.3203 +/- 11.1547 | arg(g)/pi= 0.0993 +/- 0.0151 |
-----|-----|-----|
g_re= 0.1165 +/- 0.0037 | g_re= 0.0000 +/- 0.0045 | g_re= 0.0375 +/- 0.0080 |
g_im= 0.0512 +/- 0.0017 | g_im= 0.0000 +/- 0.0035 | g_im= 0.0121 +/- 0.0031 |
corr= [ 0.49] | corr= [ 1.00] | corr= [ 0.77] |
-----|-----|-----|
Br = 0.4043 +/- 0.0333 | Br = 0.0000 +/- 0.0000 | Br = 0.0387 +/- 0.0183 |

--
pi:omega[-] pi:phi[+] lower half-plane

sqrt(s)_pole = (0.19876 +/- 0.001701)
               + (i/2)*(-3.3264e-15 +/- 1.6595e-12) [ 0.00]

s_pole = (0.039504 +/- 0.00067616)
         + i*(-6.6133e-16 +/- 3.2993e-13) [ 0.00]

=====|=====|
pi:omega | pi:phi |
=====|=====|
k_re= 0.0000 +/- 0.0000 | k_re= -0.0000 +/- 0.0000 |
k_im= -0.0470 +/- 0.0014 | k_im= 0.0620 +/- 0.0007 |
corr= [ 0.00] | corr= [ 0.00] |

=====|=====|
pi:omega/3^S_1(*) | pi:phi/3^S_1 | pi:omega/3^D_1 |
=====|=====|=====|
|g|= 0.1251 +/- 0.0040 | |g|= 0.0001 +/- 0.0010 | |g|= 0.0270 +/- 0.0071 |
arg(g)/pi= 0.5000 +/- 0.0000 | arg(g)/pi= 0.0301 +/- 11.1037 | arg(g)/pi= 0.5000 +/- 0.0000 |
-----|-----|-----|
g_re= 0.0000 +/- 0.0000 | g_re= 0.0000 +/- 0.0000 | g_re= 0.0000 +/- 0.0000 |
g_im= 0.1251 +/- 0.0040 | g_im= -0.0000 +/- 0.0017 | g_im= 0.0270 +/- 0.0071 |
corr= [-1.00] | corr= [-0.19] | corr= [-0.48] |
-----|-----|-----|
Br = 0.0000 +/- 0.0000 | Br = 0.0000 +/- 0.0000 | Br = 0.0000 +/- 0.0000 |

--
pi:omega[-] pi:phi[+] upper half-plane

sqrt(s)_pole = (0.24545 +/- 0.00094332)
               + (i/2)*(+0.0062427 +/- 0.0016376) [-0.81]

s_pole = (0.060236 +/- 0.00046723)

```



## 2 Unphysical Parameterizations

```

+ i*(+0.0015323 +/- 0.00039719) [-0.81]

=====
pi:omega | pi:phi |
=====
k_re= -0.0466 +/- 0.0011 | k_re= 0.0079 +/- 0.0012 |
k_im= -0.0037 +/- 0.0010 | k_im= 0.0193 +/- 0.0027 |
corr= [-0.81] | corr= [ 0.60] |

=====
pi:omega/3^S_1(*) | pi:phi/3^S_1 | pi:omega/3^D_1 |
=====
|g|= 0.0575 +/- 0.0080 | |g|= 0.0004 +/- 0.0066 | |g|= 0.0132 +/- 0.0070 |
arg(g)/pi= 0.1382 +/- 0.0156 | arg(g)/pi= -0.4558 +/- 11.1485 | arg(g)/pi= 0.8338 +/- 0.1066 |
-----
g_re= 0.0522 +/- 0.0071 | g_re= -0.0000 +/- 0.0108 | g_re= -0.0115 +/- 0.0081 |
g_im= 0.0242 +/- 0.0046 | g_im= -0.0000 +/- 0.0005 | g_im= 0.0066 +/- 0.0019 |
corr= [ 0.74] | corr= [ 1.00] | corr= [ 0.05] |
-----
Br = 0.8185 +/- 0.0283 | Br = 0.0000 +/- 0.0000 | Br = 0.0434 +/- 0.0553 |

--
pi:omega[-] pi:phi[+] lower half-plane

sqrt(s)_pole = (0.24545 +/- 0.00094332)
+ (i/2)*(-0.0062427 +/- 0.0016376) [ 0.81]

s_pole = (0.060236 +/- 0.00046723)
+ i*(-0.0015323 +/- 0.00039719) [ 0.81]

=====
pi:omega | pi:phi |
=====
k_re= 0.0466 +/- 0.0011 | k_re= -0.0079 +/- 0.0012 |
k_im= -0.0037 +/- 0.0010 | k_im= 0.0193 +/- 0.0027 |
corr= [ 0.81] | corr= [-0.60] |

=====
pi:omega/3^S_1(*) | pi:phi/3^S_1 | pi:omega/3^D_1 |
=====
|g|= 0.0575 +/- 0.0080 | |g|= 0.0004 +/- 0.0066 | |g|= 0.0132 +/- 0.0070 |
arg(g)/pi= -0.1382 +/- 0.0156 | arg(g)/pi= 0.4558 +/- 11.1485 | arg(g)/pi= -0.8338 +/- 0.1066 |
-----
g_re= 0.0522 +/- 0.0071 | g_re= -0.0000 +/- 0.0108 | g_re= -0.0115 +/- 0.0081 |
g_im= -0.0242 +/- 0.0046 | g_im= 0.0000 +/- 0.0005 | g_im= -0.0066 +/- 0.0019 |
corr= [-0.74] | corr= [-1.00] | corr= [-0.05] |
-----
Br = 0.8185 +/- 0.0283 | Br = 0.0000 +/- 0.0000 | Br = 0.0434 +/- 0.0553 |

--
pi:omega[-] pi:phi[-] lower half-plane

sqrt(s)_pole = (0.19876 +/- 0.001701)
+ (i/2)*(-1.1432e-15 +/- 5.6566e-13) [ 0.00]

s_pole = (0.039504 +/- 0.00067617)
+ i*(-2.2727e-16 +/- 1.1246e-13) [ 0.00]

=====
pi:omega | pi:phi |
=====
k_re= 0.0000 +/- 0.0000 | k_re= 0.0000 +/- 0.0000 |
k_im= -0.0470 +/- 0.0014 | k_im= -0.0620 +/- 0.0007 |
corr= [ 0.00] | corr= [ 0.00] |

=====
pi:omega/3^S_1(*) | pi:phi/3^S_1 | pi:omega/3^D_1 |
=====

```



## 2 Unphysical Parameterizations

|                                                                     |                                                                      |                                                                     |
|---------------------------------------------------------------------|----------------------------------------------------------------------|---------------------------------------------------------------------|
| g = 0.1251 +/- 0.0040<br>arg(g)/pi= 0.5000 +/- 0.0000               | g = 0.0002 +/- 0.0040<br>arg(g)/pi= 0.0300 +/- 11.1362               | g = 0.0270 +/- 0.0071<br>arg(g)/pi= 0.5000 +/- 0.0000               |
| g_re= 0.0000 +/- 0.0000<br>g_im= 0.1251 +/- 0.0040<br>corr= [-1.00] | g_re= 0.0000 +/- 0.0000<br>g_im= -0.0000 +/- 0.0065<br>corr= [-0.62] | g_re= 0.0000 +/- 0.0000<br>g_im= 0.0270 +/- 0.0071<br>corr= [-0.48] |
| Br = 0.0000 +/- 0.0000                                              | Br = 0.0000 +/- 0.0000                                               | Br = 0.0000 +/- 0.0000                                              |

--

pi:omega[-] pi:phi[-] upper half-plane

sqr(s)\_pole = (0.24545 +/- 0.00094351)  
+ (i/2)\*(+0.0062429 +/- 0.0016377) [-0.81]

s\_pole = (0.060236 +/- 0.00046733)  
+ i\*(+0.0015323 +/- 0.00039722) [-0.81]

| pi:omega                                                              | pi:phi                                                                |
|-----------------------------------------------------------------------|-----------------------------------------------------------------------|
| k_re= -0.0466 +/- 0.0011<br>k_im= -0.0037 +/- 0.0010<br>corr= [-0.81] | k_re= -0.0079 +/- 0.0012<br>k_im= -0.0193 +/- 0.0027<br>corr= [ 0.60] |

| pi:omega/3^S_1(*)                                                   | pi:phi/3^S_1                                                         | pi:omega/3^D_1                                                       |
|---------------------------------------------------------------------|----------------------------------------------------------------------|----------------------------------------------------------------------|
| g = 0.0575 +/- 0.0080<br>arg(g)/pi= 0.1382 +/- 0.0156               | g = 0.0005 +/- 0.0088<br>arg(g)/pi= 0.4441 +/- 11.1474               | g = 0.0132 +/- 0.0070<br>arg(g)/pi= 0.8338 +/- 0.1066                |
| g_re= 0.0522 +/- 0.0071<br>g_im= 0.0242 +/- 0.0046<br>corr= [ 0.74] | g_re= -0.0000 +/- 0.0145<br>g_im= 0.0000 +/- 0.0012<br>corr= [-1.00] | g_re= -0.0115 +/- 0.0081<br>g_im= 0.0066 +/- 0.0019<br>corr= [ 0.05] |
| Br = 0.8185 +/- 0.0283                                              | Br = 0.0000 +/- 0.0000                                               | Br = 0.0434 +/- 0.0553                                               |

--

pi:omega[-] pi:phi[-] lower half-plane

sqr(s)\_pole = (0.24545 +/- 0.00094351)  
+ (i/2)\*(-0.0062429 +/- 0.0016377) [ 0.81]

s\_pole = (0.060236 +/- 0.00046733)  
+ i\*(-0.0015323 +/- 0.00039722) [ 0.81]

| pi:omega                                                             | pi:phi                                                               |
|----------------------------------------------------------------------|----------------------------------------------------------------------|
| k_re= 0.0466 +/- 0.0011<br>k_im= -0.0037 +/- 0.0010<br>corr= [ 0.81] | k_re= 0.0079 +/- 0.0012<br>k_im= -0.0193 +/- 0.0027<br>corr= [-0.60] |

| pi:omega/3^S_1(*)                                                    | pi:phi/3^S_1                                                          | pi:omega/3^D_1                                                        |
|----------------------------------------------------------------------|-----------------------------------------------------------------------|-----------------------------------------------------------------------|
| g = 0.0575 +/- 0.0080<br>arg(g)/pi= -0.1382 +/- 0.0156               | g = 0.0005 +/- 0.0088<br>arg(g)/pi= -0.4441 +/- 11.1474               | g = 0.0132 +/- 0.0070<br>arg(g)/pi= -0.8338 +/- 0.1066                |
| g_re= 0.0522 +/- 0.0071<br>g_im= -0.0242 +/- 0.0046<br>corr= [-0.74] | g_re= -0.0000 +/- 0.0145<br>g_im= -0.0000 +/- 0.0012<br>corr= [ 1.00] | g_re= -0.0115 +/- 0.0081<br>g_im= -0.0066 +/- 0.0019<br>corr= [-0.05] |
| Br = 0.8185 +/- 0.0283                                               | Br = 0.0000 +/- 0.0000                                                | Br = 0.0434 +/- 0.0553                                                |



## 2.7 coupled\_po\_pp.3s1\_3d1.pole+G0\_3s1\_3sd1\_3S1+G1\_3s1.gorder0\_3s1\_3d1\_3S1.pole0\_sub

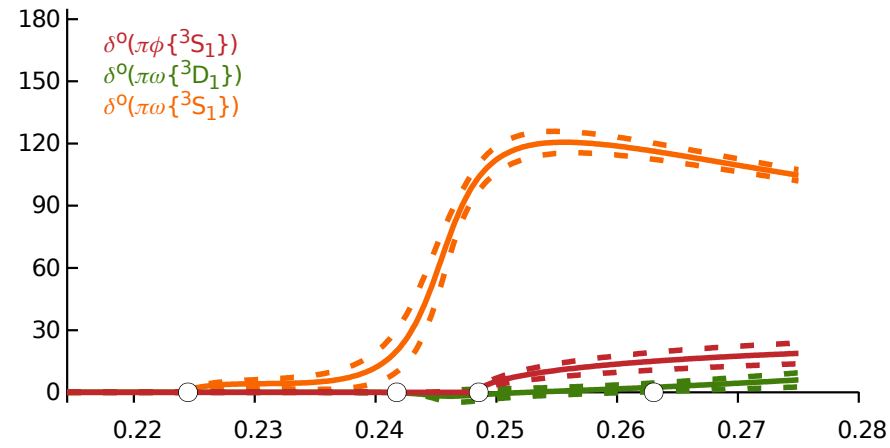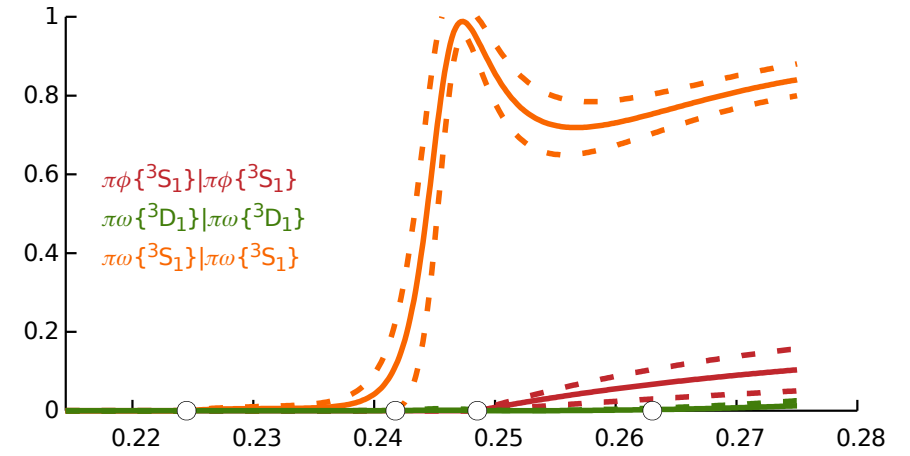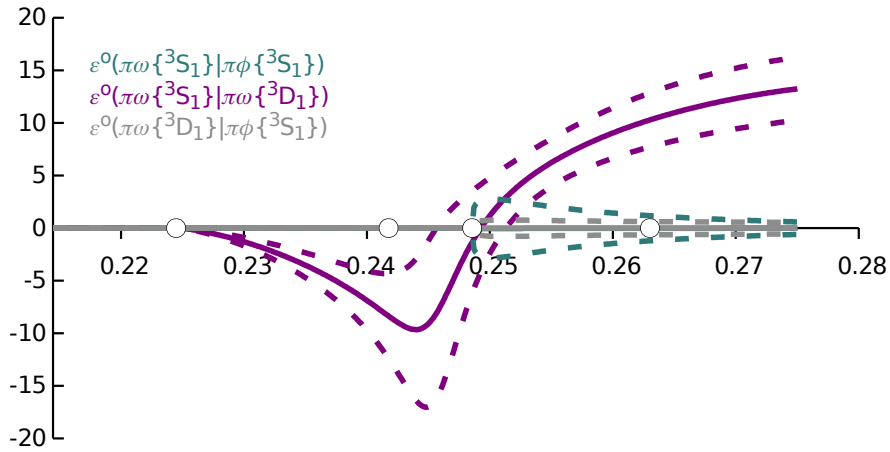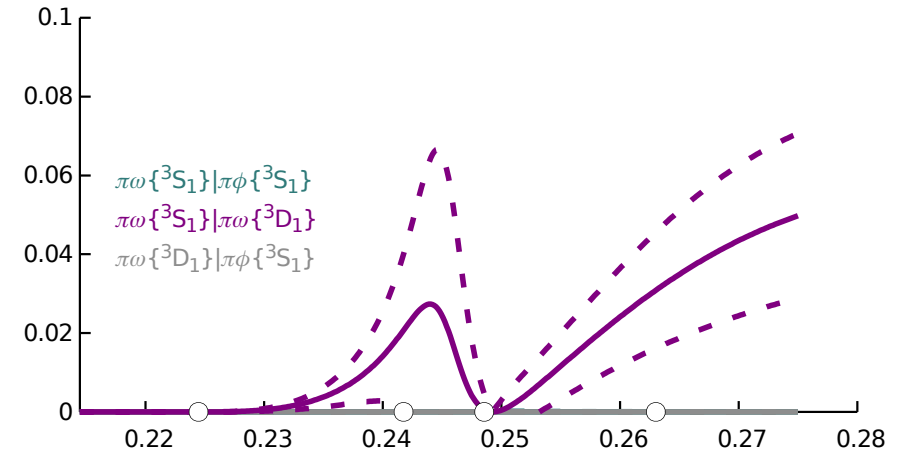



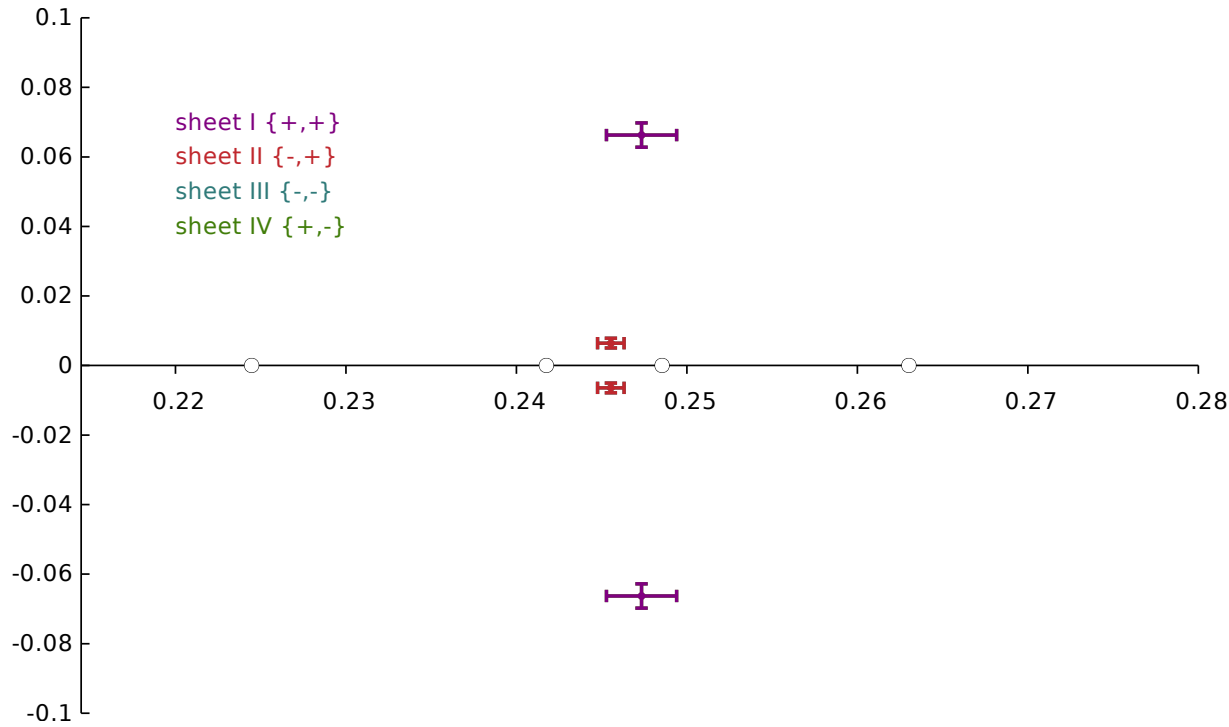

### parameter values

minimised with  $\text{chisq}/\text{nDoF} = 32.81 / (36 - 8) = 1.17$

|                                               |  |                          |  |      |      |       |      |       |       |       |       |
|-----------------------------------------------|--|--------------------------|--|------|------|-------|------|-------|-------|-------|-------|
| JP1+_g_pi:omega/3^D_1_pole0                   |  | -0.63114 +/- 0.85627     |  | 1.00 | 0.89 | -0.06 | 0.32 | -0.23 | -0.08 | -0.12 | 0.14  |
| JP1+_g_pi:omega/3^S_1_pole0                   |  | 0.074363 +/- 0.011753    |  |      | 1.00 | -0.07 | 0.15 | -0.29 | -0.10 | -0.11 | 0.11  |
| JP1+_g_pi:phi/3^S_1_pole0                     |  | -0.00013699 +/- 0.010827 |  |      |      | 1.00  | 0.00 | 0.02  | 0.01  | -0.04 | -0.08 |
| JP1+_gamma_pi:omega/3^S_1 pi:omega/3^D_1_orde |  | -44.862 +/- 11.88        |  |      |      |       | 1.00 | -0.14 | 0.25  | -0.15 | -0.11 |
| JP1+_gamma_pi:omega/3^S_1 pi:omega/3^S_1_orde |  | 6.8060 +/- 0.35295       |  |      |      |       |      | 1.00  | -0.85 | 0.05  | -0.04 |
| JP1+_gamma_pi:omega/3^S_1 pi:omega/3^S_1_orde |  | -134.83 +/- 6.8744       |  |      |      |       |      |       | 1.00  | 0.06  | -0.06 |
| JP1+_gamma_pi:phi/3^S_1 pi:phi/3^S_1_order0   |  | 0.87762 +/- 0.24824      |  |      |      |       |      |       |       | 1.00  | -0.18 |
| JP1+_m_pole0                                  |  | 0.24716 +/- 0.00056812   |  |      |      |       |      |       |       |       | 1.00  |

### pole singularities

pi:omega[+] pi:phi[+] upper half-plane

$\text{sqrt}(s)_{\text{pole}} = (0.24734 \pm 0.0020586)$   
 $+ (i/2)*(0.066284 \pm 0.0034993) [0.05]$

$s_{\text{pole}} = (0.060079 \pm 0.001019)$   
 $+ i*(0.016395 \pm 0.00088305) [0.09]$

|                         |                         |
|-------------------------|-------------------------|
| pi:omega                | pi:phi                  |
| =====                   | =====                   |
| k_re= 0.0558 +/- 0.0018 | k_re= 0.0374 +/- 0.0018 |



## 2 Unphysical Parameterizations

```

k_im= 0.0332 +/- 0.0015 | k_im= 0.0442 +/- 0.0016 |
corr= [-0.07] | corr= [-0.14] |

```

```

=====
pi:omega/3^S_1(*) | pi:phi/3^S_1 | pi:omega/3^D_1 |
=====
|g|= 0.1598 +/- 0.0040 | |g|= 0.0001 +/- 0.0016 | |g|= 0.0489 +/- 0.0098 |
arg(g)/pi= -0.1996 +/- 0.0031 | arg(g)/pi= 0.3774 +/- 11.2886 | arg(g)/pi= -0.1572 +/- 0.0133 |
-----
g_re= 0.1294 +/- 0.0032 | g_re= 0.0000 +/- 0.0025 | g_re= 0.0431 +/- 0.0088 |
g_im= -0.0938 +/- 0.0029 | g_im= -0.0000 +/- 0.0000 | g_im= -0.0232 +/- 0.0047 |
corr= [-0.76] | corr= [-0.88] | corr= [-0.88] |
-----
Br = 0.6120 +/- 0.0301 | Br = 0.0000 +/- 0.0000 | Br = 0.0574 +/- 0.0252 |

```

```

--
pi:omega[+] pi:phi[+] lower half-plane

```

```

sqrt(s)_pole = (0.24734 +/- 0.0020586)
+ (i/2)*(-0.066284 +/- 0.0034993) [-0.05]

```

```

s_pole = (0.060079 +/- 0.001019)
+ i*(-0.016395 +/- 0.00088305) [-0.09]

```

```

=====
pi:omega | pi:phi |
=====
k_re= -0.0558 +/- 0.0018 | k_re= -0.0374 +/- 0.0018 |
k_im= 0.0332 +/- 0.0015 | k_im= 0.0442 +/- 0.0016 |
corr= [ 0.07] | corr= [ 0.14] |

```

```

=====
pi:omega/3^S_1(*) | pi:phi/3^S_1 | pi:omega/3^D_1 |
=====
|g|= 0.1598 +/- 0.0040 | |g|= 0.0001 +/- 0.0016 | |g|= 0.0489 +/- 0.0098 |
arg(g)/pi= 0.1996 +/- 0.0031 | arg(g)/pi= -0.3774 +/- 11.2886 | arg(g)/pi= 0.1572 +/- 0.0133 |
-----
g_re= 0.1294 +/- 0.0032 | g_re= 0.0000 +/- 0.0025 | g_re= 0.0431 +/- 0.0088 |
g_im= 0.0938 +/- 0.0029 | g_im= 0.0000 +/- 0.0000 | g_im= 0.0232 +/- 0.0047 |
corr= [ 0.76] | corr= [ 0.88] | corr= [ 0.88] |
-----
Br = 0.6120 +/- 0.0301 | Br = 0.0000 +/- 0.0000 | Br = 0.0574 +/- 0.0252 |

```

```

--
pi:omega[+] pi:phi[-] lower half-plane

```

```

sqrt(s)_pole = (0.24734 +/- 0.0020586)
+ (i/2)*(-0.066284 +/- 0.0034994) [-0.05]

```

```

s_pole = (0.060079 +/- 0.001019)
+ i*(-0.016395 +/- 0.00088308) [-0.09]

```

```

=====
pi:omega | pi:phi |
=====
k_re= -0.0558 +/- 0.0018 | k_re= 0.0374 +/- 0.0018 |
k_im= 0.0332 +/- 0.0015 | k_im= -0.0442 +/- 0.0016 |
corr= [ 0.07] | corr= [ 0.14] |

```

```

=====
pi:omega/3^S_1(*) | pi:phi/3^S_1 | pi:omega/3^D_1 |
=====
|g|= 0.1598 +/- 0.0040 | |g|= 0.0001 +/- 0.0026 | |g|= 0.0489 +/- 0.0098 |
arg(g)/pi= 0.1996 +/- 0.0031 | arg(g)/pi= -0.1666 +/- 10.9516 | arg(g)/pi= 0.1572 +/- 0.0133 |
-----
g_re= 0.1294 +/- 0.0032 | g_re= 0.0000 +/- 0.0029 | g_re= 0.0431 +/- 0.0088 |
g_im= 0.0938 +/- 0.0029 | g_im= 0.0000 +/- 0.0027 | g_im= 0.0232 +/- 0.0047 |

```



## 2 Unphysical Parameterizations

```

corr= [ 0.76] | corr= [ 1.00] | corr= [ 0.88] |
-----|-----|-----|
Br = 0.6120 +/- 0.0302 | Br = 0.0000 +/- 0.0000 | Br = 0.0574 +/- 0.0252 |

--
pi:omega[+] pi:phi[-] upper half-plane

sqrt(s)_pole = (0.24734 +/- 0.0020586)
               + (i/2)*(+0.066284 +/- 0.0034994) [ 0.05]

s_pole = (0.060079 +/- 0.001019)
         + i*(+0.016395 +/- 0.00088308) [ 0.09]

=====|=====|
pi:omega | pi:phi |
=====|=====|
k_re= 0.0558 +/- 0.0018 | k_re= -0.0374 +/- 0.0018 |
k_im= 0.0332 +/- 0.0015 | k_im= -0.0442 +/- 0.0016 |
corr= [-0.07] | corr= [-0.14] |

=====|=====|
pi:omega/3^S_1(*) | pi:phi/3^S_1 | pi:omega/3^D_1 |
=====|=====|=====|
|g|= 0.1598 +/- 0.0040 | |g|= 0.0001 +/- 0.0026 | |g|= 0.0489 +/- 0.0098 |
arg(g)/pi= -0.1996 +/- 0.0031 | arg(g)/pi= 0.1666 +/- 10.9516 | arg(g)/pi= -0.1572 +/- 0.0133 |
-----|-----|-----|
g_re= 0.1294 +/- 0.0032 | g_re= 0.0000 +/- 0.0029 | g_re= 0.0431 +/- 0.0088 |
g_im= -0.0938 +/- 0.0029 | g_im= -0.0000 +/- 0.0027 | g_im= -0.0232 +/- 0.0047 |
corr= [-0.76] | corr= [-1.00] | corr= [-0.88] |
-----|-----|-----|
Br = 0.6120 +/- 0.0302 | Br = 0.0000 +/- 0.0000 | Br = 0.0574 +/- 0.0252 |

--
pi:omega[-] pi:phi[+] upper half-plane

sqrt(s)_pole = (0.27725 +/- 0.010217)
               + (i/2)*(+0.24382 +/- 0.071801) [ 0.96]

s_pole = (0.062003 +/- 0.0037425)
         + i*(+0.067602 +/- 0.022303) [-0.88]

=====|=====|
pi:omega | pi:phi |
=====|=====|
k_re= -0.0948 +/- 0.0115 | k_re= 0.0833 +/- 0.0131 |
k_im= -0.0852 +/- 0.0191 | k_im= 0.0924 +/- 0.0189 |
corr= [ 0.98] | corr= [ 0.99] |

=====|=====|
pi:omega/3^S_1 | pi:phi/3^S_1 | pi:omega/3^D_1(*) |
=====|=====|=====|
|g|= 0.0550 +/- 0.0053 | |g|= 0.0000 +/- 0.0008 | |g|= 0.1886 +/- 0.0230 |
arg(g)/pi= 0.5395 +/- 0.0342 | arg(g)/pi= 0.3172 +/- 10.9610 | arg(g)/pi= -0.4817 +/- 0.0359 |
-----|-----|-----|
g_re= -0.0068 +/- 0.0053 | g_re= 0.0000 +/- 0.0012 | g_re= 0.0109 +/- 0.0226 |
g_im= 0.0546 +/- 0.0059 | g_im= -0.0000 +/- 0.0003 | g_im= -0.1882 +/- 0.0217 |
corr= [ 0.82] | corr= [-0.99] | corr= [-1.00] |
-----|-----|-----|
Br = 0.0248 +/- 0.0133 | Br = 0.0000 +/- 0.0000 | Br = 0.2912 +/- 0.0354 |

--
pi:omega[-] pi:phi[+] lower half-plane

sqrt(s)_pole = (0.27725 +/- 0.010217)
               + (i/2)*(-0.24382 +/- 0.071801) [-0.96]

s_pole = (0.062003 +/- 0.0037425)

```



+ i\*(-0.067602 +/- 0.022303) [ 0.88]

| pi:omega          |                    | pi:phi          |                     |
|-------------------|--------------------|-----------------|---------------------|
| =====             |                    | =====           |                     |
| k_re=             | 0.0948 +/- 0.0115  | k_re=           | -0.0833 +/- 0.0131  |
| k_im=             | -0.0852 +/- 0.0191 | k_im=           | 0.0924 +/- 0.0189   |
| corr=             | [-0.98]            | corr=           | [-0.99]             |
| -----             |                    |                 |                     |
| pi:omega/3^S_1    |                    | pi:phi/3^S_1    |                     |
| =====             |                    | =====           |                     |
| g =               | 0.0550 +/- 0.0053  | g =             | 0.0000 +/- 0.0008   |
| arg(g)/pi=        | -0.5395 +/- 0.0342 | arg(g)/pi=      | -0.3172 +/- 10.9610 |
| -----             |                    | -----           |                     |
| g_re=             | -0.0068 +/- 0.0053 | g_re=           | 0.0000 +/- 0.0012   |
| g_im=             | -0.0546 +/- 0.0059 | g_im=           | 0.0000 +/- 0.0003   |
| corr=             | [-0.82]            | corr=           | [ 0.99]             |
| -----             |                    | -----           |                     |
| Br =              | 0.0248 +/- 0.0133  | Br =            | 0.0000 +/- 0.0000   |
| -----             |                    | -----           |                     |
| pi:omega/3^D_1(*) |                    | pi:phi/3^D_1(*) |                     |
| =====             |                    | =====           |                     |
| g =               | 0.1886 +/- 0.0230  | g =             | 0.1886 +/- 0.0230   |
| arg(g)/pi=        | -0.5395 +/- 0.0342 | arg(g)/pi=      | 0.4817 +/- 0.0359   |
| -----             |                    | -----           |                     |
| g_re=             | 0.0109 +/- 0.0226  | g_re=           | 0.0109 +/- 0.0226   |
| g_im=             | 0.1882 +/- 0.0217  | g_im=           | 0.1882 +/- 0.0217   |
| corr=             | [ 1.00]            | corr=           | [ 1.00]             |
| -----             |                    | -----           |                     |
| Br =              | 0.2912 +/- 0.0354  | Br =            | 0.2912 +/- 0.0354   |
| -----             |                    | -----           |                     |

--

pi:omega[-] pi:phi[+] lower half-plane

sqrt(s)\_pole = (0.20342 +/- 0.0013984)  
+ (i/2)\*(-3.2321e-15 +/- 1.6321e-12) [ 0.00]

s\_pole = (0.041381 +/- 0.00056894)  
+ i\*(-6.576e-16 +/- 3.3207e-13) [ 0.00]

| pi:omega          |                    | pi:phi       |                     |
|-------------------|--------------------|--------------|---------------------|
| =====             |                    | =====        |                     |
| k_re=             | 0.0000 +/- 0.0000  | k_re=        | -0.0000 +/- 0.0000  |
| k_im=             | -0.0430 +/- 0.0013 | k_im=        | 0.0600 +/- 0.0007   |
| corr=             | [ 0.00]            | corr=        | [ 0.00]             |
| -----             |                    |              |                     |
| pi:omega/3^S_1(*) |                    | pi:phi/3^S_1 |                     |
| =====             |                    | =====        |                     |
| g =               | 0.1016 +/- 0.0037  | g =          | 0.0001 +/- 0.0013   |
| arg(g)/pi=        | 0.5000 +/- 0.0000  | arg(g)/pi=   | -0.1003 +/- 10.8879 |
| -----             |                    | -----        |                     |
| g_re=             | 0.0000 +/- 0.0000  | g_re=        | 0.0000 +/- 0.0000   |
| g_im=             | 0.1016 +/- 0.0037  | g_im=        | -0.0000 +/- 0.0021  |
| corr=             | [-1.00]            | corr=        | [-0.24]             |
| -----             |                    | -----        |                     |
| Br =              | 0.0000 +/- 0.0000  | Br =         | 0.0000 +/- 0.0000   |
| -----             |                    | -----        |                     |
| pi:omega/3^D_1    |                    | pi:phi/3^D_1 |                     |
| =====             |                    | =====        |                     |
| g =               | 0.0224 +/- 0.0058  | g =          | 0.0224 +/- 0.0058   |
| arg(g)/pi=        | 0.5000 +/- 0.0000  | arg(g)/pi=   | 0.5000 +/- 0.0000   |
| -----             |                    | -----        |                     |
| g_re=             | 0.0000 +/- 0.0000  | g_re=        | 0.0000 +/- 0.0000   |
| g_im=             | 0.0224 +/- 0.0058  | g_im=        | 0.0224 +/- 0.0058   |
| corr=             | [-0.27]            | corr=        | [-0.27]             |
| -----             |                    | -----        |                     |
| Br =              | 0.0000 +/- 0.0000  | Br =         | 0.0000 +/- 0.0000   |
| -----             |                    | -----        |                     |

--

pi:omega[-] pi:phi[+] upper half-plane

sqrt(s)\_pole = (0.24554 +/- 0.00078055)  
+ (i/2)\*(+0.0064303 +/- 0.0014011) [-0.69]

s\_pole = (0.060278 +/- 0.00038644)  
+ i\*(+0.0015789 +/- 0.00034056) [-0.69]

| pi:omega          |                    | pi:phi       |                     |
|-------------------|--------------------|--------------|---------------------|
| =====             |                    | =====        |                     |
| k_re=             | -0.0467 +/- 0.0009 | k_re=        | 0.0082 +/- 0.0011   |
| k_im=             | -0.0038 +/- 0.0009 | k_im=        | 0.0192 +/- 0.0022   |
| corr=             | [-0.70]            | corr=        | [ 0.46]             |
| -----             |                    |              |                     |
| pi:omega/3^S_1(*) |                    | pi:phi/3^S_1 |                     |
| =====             |                    | =====        |                     |
| g =               | 0.0000 +/- 0.0000  | g =          | 0.0000 +/- 0.0000   |
| arg(g)/pi=        | 0.5000 +/- 0.0000  | arg(g)/pi=   | -0.1003 +/- 10.8879 |
| -----             |                    | -----        |                     |
| g_re=             | 0.0000 +/- 0.0000  | g_re=        | 0.0000 +/- 0.0000   |
| g_im=             | 0.1016 +/- 0.0037  | g_im=        | -0.0000 +/- 0.0021  |
| corr=             | [-1.00]            | corr=        | [-0.24]             |
| -----             |                    | -----        |                     |
| Br =              | 0.0000 +/- 0.0000  | Br =         | 0.0000 +/- 0.0000   |
| -----             |                    | -----        |                     |



## 2 Unphysical Parameterizations

| $ g $                               | $ g $                                | $ g $                                |
|-------------------------------------|--------------------------------------|--------------------------------------|
| $0.0584 \pm 0.0065$                 | $0.0004 \pm 0.0065$                  | $0.0126 \pm 0.0061$                  |
| $\arg(g)/\pi = 0.1295 \pm 0.0150$   | $\arg(g)/\pi = -0.5837 \pm 10.9431$  | $\arg(g)/\pi = 0.8320 \pm 0.1043$    |
| $g_{\text{re}} = 0.0536 \pm 0.0057$ | $g_{\text{re}} = -0.0001 \pm 0.0100$ | $g_{\text{re}} = -0.0109 \pm 0.0071$ |
| $g_{\text{im}} = 0.0231 \pm 0.0042$ | $g_{\text{im}} = -0.0000 \pm 0.0005$ | $g_{\text{im}} = 0.0063 \pm 0.0019$  |
| $\text{corr} = [0.71]$              | $\text{corr} = [1.00]$               | $\text{corr} = [0.11]$               |
| $\text{Br} = 0.8194 \pm 0.0214$     | $\text{Br} = 0.0000 \pm 0.0000$      | $\text{Br} = 0.0381 \pm 0.0434$      |

--

pi:omega[-] pi:phi[+] lower half-plane

$\text{sqrt}(s)_{\text{pole}} = (0.24554 \pm 0.00078055)$   
 $+ (i/2)*(-0.0064303 \pm 0.0014011) [0.69]$

$s_{\text{pole}} = (0.060278 \pm 0.00038644)$   
 $+ i*(-0.0015789 \pm 0.00034056) [0.69]$

| pi:omega                             | pi:phi                               |
|--------------------------------------|--------------------------------------|
| $k_{\text{re}} = 0.0467 \pm 0.0009$  | $k_{\text{re}} = -0.0082 \pm 0.0011$ |
| $k_{\text{im}} = -0.0038 \pm 0.0009$ | $k_{\text{im}} = 0.0192 \pm 0.0022$  |
| $\text{corr} = [0.70]$               | $\text{corr} = [-0.46]$              |

| pi:omega/3 <sup>S</sup> _1(*)        | pi:phi/3 <sup>S</sup> _1             | pi:omega/3 <sup>D</sup> _1           |
|--------------------------------------|--------------------------------------|--------------------------------------|
| $ g  = 0.0584 \pm 0.0065$            | $ g  = 0.0004 \pm 0.0065$            | $ g  = 0.0126 \pm 0.0061$            |
| $\arg(g)/\pi = -0.1295 \pm 0.0150$   | $\arg(g)/\pi = 0.5837 \pm 10.9431$   | $\arg(g)/\pi = -0.8320 \pm 0.1043$   |
| $g_{\text{re}} = 0.0536 \pm 0.0057$  | $g_{\text{re}} = -0.0001 \pm 0.0100$ | $g_{\text{re}} = -0.0109 \pm 0.0071$ |
| $g_{\text{im}} = -0.0231 \pm 0.0042$ | $g_{\text{im}} = 0.0000 \pm 0.0005$  | $g_{\text{im}} = -0.0063 \pm 0.0019$ |
| $\text{corr} = [-0.71]$              | $\text{corr} = [-1.00]$              | $\text{corr} = [-0.11]$              |
| $\text{Br} = 0.8194 \pm 0.0214$      | $\text{Br} = 0.0000 \pm 0.0000$      | $\text{Br} = 0.0381 \pm 0.0434$      |

--

pi:omega[-] pi:phi[-] upper half-plane

$\text{sqrt}(s)_{\text{pole}} = (0.27725 \pm 0.010217)$   
 $+ (i/2)*(+0.24382 \pm 0.071801) [0.96]$

$s_{\text{pole}} = (0.062003 \pm 0.0037425)$   
 $+ i*(+0.067602 \pm 0.022303) [-0.88]$

| pi:omega                             | pi:phi                               |
|--------------------------------------|--------------------------------------|
| $k_{\text{re}} = -0.0948 \pm 0.0115$ | $k_{\text{re}} = -0.0833 \pm 0.0131$ |
| $k_{\text{im}} = -0.0852 \pm 0.0191$ | $k_{\text{im}} = -0.0924 \pm 0.0189$ |
| $\text{corr} = [0.98]$               | $\text{corr} = [0.99]$               |

| pi:omega/3 <sup>S</sup> _1           | pi:phi/3 <sup>S</sup> _1             | pi:omega/3 <sup>D</sup> _1(*)        |
|--------------------------------------|--------------------------------------|--------------------------------------|
| $ g  = 0.0550 \pm 0.0053$            | $ g  = 0.0000 \pm 0.0009$            | $ g  = 0.1886 \pm 0.0230$            |
| $\arg(g)/\pi = 0.5395 \pm 0.0342$    | $\arg(g)/\pi = -0.0327 \pm 10.9784$  | $\arg(g)/\pi = -0.4817 \pm 0.0359$   |
| $g_{\text{re}} = -0.0068 \pm 0.0053$ | $g_{\text{re}} = 0.0000 \pm 0.0003$  | $g_{\text{re}} = 0.0109 \pm 0.0226$  |
| $g_{\text{im}} = 0.0546 \pm 0.0059$  | $g_{\text{im}} = -0.0000 \pm 0.0013$ | $g_{\text{im}} = -0.1882 \pm 0.0217$ |
| $\text{corr} = [0.82]$               | $\text{corr} = [-0.99]$              | $\text{corr} = [-1.00]$              |
| $\text{Br} = 0.0248 \pm 0.0133$      | $\text{Br} = 0.0000 \pm 0.0000$      | $\text{Br} = 0.2912 \pm 0.0354$      |

--

pi:omega[-] pi:phi[-] upper half-plane



## 2 Unphysical Parameterizations

```
sqrt(s)_pole = (0.20342 +/- 0.0013984)
               + (i/2)*(+2.3447e-16 +/- 6.0429e-14) [ 0.00]
```

```
s_pole = (0.041381 +/- 0.00056896)
          + i*(+4.7691e-17 +/- 1.2294e-14) [ 0.00]
```

| pi:omega                 | pi:phi                   |
|--------------------------|--------------------------|
| k_re= -0.0000 +/- 0.0000 | k_re= -0.0000 +/- 0.0000 |
| k_im= -0.0430 +/- 0.0013 | k_im= -0.0600 +/- 0.0007 |
| corr= [ 0.00]            | corr= [ 0.00]            |

| pi:omega/3^S_1(*)            | pi:phi/3^S_1                   | pi:omega/3^D_1               |
|------------------------------|--------------------------------|------------------------------|
| g = 0.1016 +/- 0.0037        | g = 0.0004 +/- 0.0075          | g = 0.0224 +/- 0.0058        |
| arg(g)/pi= 0.5000 +/- 0.0000 | arg(g)/pi= -0.1001 +/- 10.9322 | arg(g)/pi= 0.5000 +/- 0.0000 |
| g_re= 0.0000 +/- 0.0000      | g_re= 0.0000 +/- 0.0000        | g_re= 0.0000 +/- 0.0000      |
| g_im= 0.1016 +/- 0.0037      | g_im= -0.0001 +/- 0.0114       | g_im= 0.0224 +/- 0.0058      |
| corr= [-1.00]                | corr= [-0.83]                  | corr= [-0.27]                |
| Br = 0.0000 +/- 0.0000       | Br = 0.0000 +/- 0.0000         | Br = 0.0000 +/- 0.0000       |

```
--
pi:omega[-] pi:phi[-] lower half-plane
```

```
sqrt(s)_pole = (0.27725 +/- 0.010217)
               + (i/2)*(-0.24382 +/- 0.071801) [-0.96]
```

```
s_pole = (0.062003 +/- 0.0037425)
          + i*(-0.067602 +/- 0.022303) [ 0.88]
```

| pi:omega                 | pi:phi                   |
|--------------------------|--------------------------|
| k_re= 0.0948 +/- 0.0115  | k_re= 0.0833 +/- 0.0131  |
| k_im= -0.0852 +/- 0.0191 | k_im= -0.0924 +/- 0.0189 |
| corr= [-0.98]            | corr= [-0.99]            |

| pi:omega/3^S_1                | pi:phi/3^S_1                  | pi:omega/3^D_1(*)            |
|-------------------------------|-------------------------------|------------------------------|
| g = 0.0550 +/- 0.0053         | g = 0.0000 +/- 0.0009         | g = 0.1886 +/- 0.0230        |
| arg(g)/pi= -0.5395 +/- 0.0342 | arg(g)/pi= 0.0336 +/- 10.9575 | arg(g)/pi= 0.4817 +/- 0.0359 |
| g_re= -0.0068 +/- 0.0053      | g_re= 0.0000 +/- 0.0003       | g_re= 0.0109 +/- 0.0226      |
| g_im= -0.0546 +/- 0.0059      | g_im= 0.0000 +/- 0.0013       | g_im= 0.1882 +/- 0.0217      |
| corr= [-0.82]                 | corr= [ 0.99]                 | corr= [ 1.00]                |
| Br = 0.0248 +/- 0.0133        | Br = 0.0000 +/- 0.0000        | Br = 0.2912 +/- 0.0354       |

```
--
pi:omega[-] pi:phi[-] upper half-plane
```

```
sqrt(s)_pole = (0.24554 +/- 0.00078084)
               + (i/2)*(+0.0064305 +/- 0.0014015) [-0.69]
```

```
s_pole = (0.060278 +/- 0.00038659)
          + i*(+0.0015789 +/- 0.00034065) [-0.69]
```

| pi:omega                 | pi:phi                   |
|--------------------------|--------------------------|
| k_re= -0.0467 +/- 0.0009 | k_re= -0.0082 +/- 0.0011 |
| k_im= -0.0038 +/- 0.0009 | k_im= -0.0192 +/- 0.0022 |



## 2 Unphysical Parameterizations

```

corr= [-0.70] | corr= [ 0.46] |

===== pi:omega/3^S_1(*) | pi:phi/3^S_1 | pi:omega/3^D_1 |
=====
|g|= 0.0584 +/- 0.0065 | |g|= 0.0005 +/- 0.0088 | |g|= 0.0126 +/- 0.0061 |
arg(g)/pi= 0.1295 +/- 0.0150 | arg(g)/pi= 0.5722 +/- 10.9412 | arg(g)/pi= 0.8320 +/- 0.1043 |
-----
g_re= 0.0536 +/- 0.0057 | g_re= -0.0002 +/- 0.0134 | g_re= -0.0109 +/- 0.0071 |
g_im= 0.0231 +/- 0.0042 | g_im= 0.0000 +/- 0.0012 | g_im= 0.0063 +/- 0.0019 |
corr= [ 0.71] | corr= [-1.00] | corr= [ 0.11] |
-----
Br = 0.8194 +/- 0.0214 | Br = 0.0000 +/- 0.0000 | Br = 0.0381 +/- 0.0434 |

--
pi:omega[-] pi:phi[-] lower half-plane

sqrt(s)_pole = (0.24554 +/- 0.00078084)
+ (i/2)*(-0.0064305 +/- 0.0014015) [ 0.69]

s_pole = (0.060278 +/- 0.00038659)
+ i*(-0.0015789 +/- 0.00034065) [ 0.69]

===== pi:omega | pi:phi |
=====
k_re= 0.0467 +/- 0.0009 | k_re= 0.0082 +/- 0.0011 |
k_im= -0.0038 +/- 0.0009 | k_im= -0.0192 +/- 0.0022 |
corr= [ 0.70] | corr= [-0.46] |

===== pi:omega/3^S_1(*) | pi:phi/3^S_1 | pi:omega/3^D_1 |
=====
|g|= 0.0584 +/- 0.0065 | |g|= 0.0005 +/- 0.0088 | |g|= 0.0126 +/- 0.0061 |
arg(g)/pi= -0.1295 +/- 0.0150 | arg(g)/pi= -0.5722 +/- 10.9412 | arg(g)/pi= -0.8320 +/- 0.1043 |
-----
g_re= 0.0536 +/- 0.0057 | g_re= -0.0002 +/- 0.0134 | g_re= -0.0109 +/- 0.0071 |
g_im= -0.0231 +/- 0.0042 | g_im= -0.0000 +/- 0.0012 | g_im= -0.0063 +/- 0.0019 |
corr= [-0.71] | corr= [ 1.00] | corr= [-0.11] |
-----
Br = 0.8194 +/- 0.0214 | Br = 0.0000 +/- 0.0000 | Br = 0.0381 +/- 0.0434 |

```



## 2.8 coupled\_po\_pp.3s1\_3d1.pole+G0\_3s1\_3sd1\_3S1+G1\_3s1.gorder0\_3s1\_3d1\_3S1.threshold\_sub

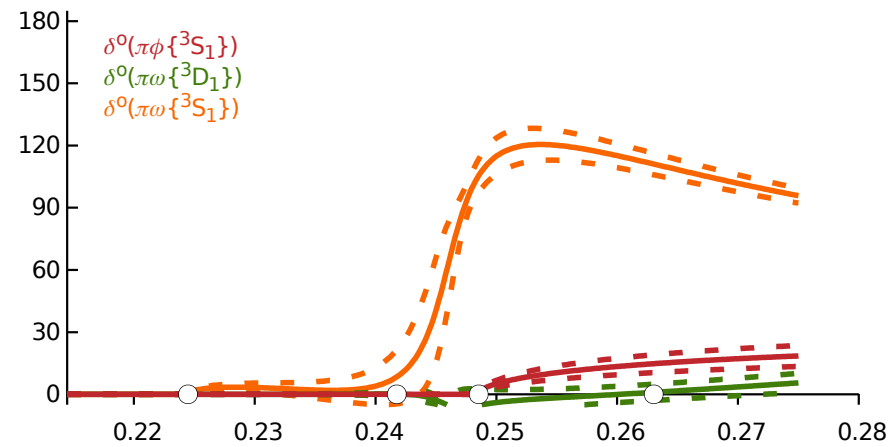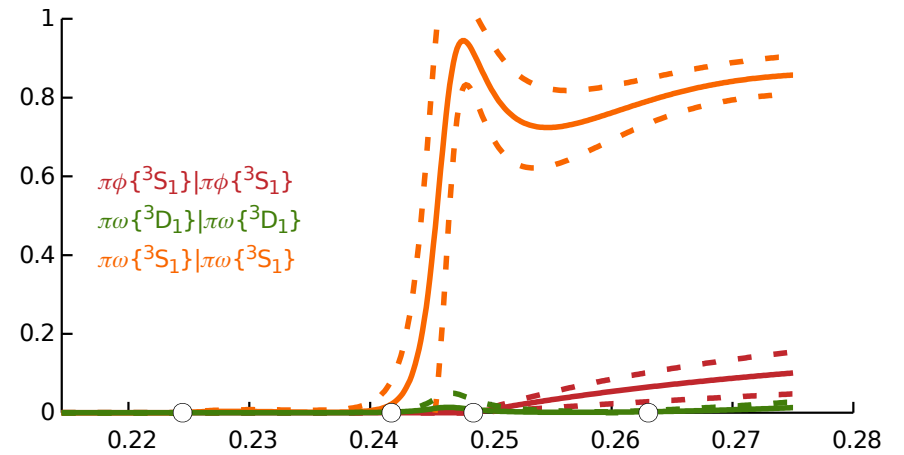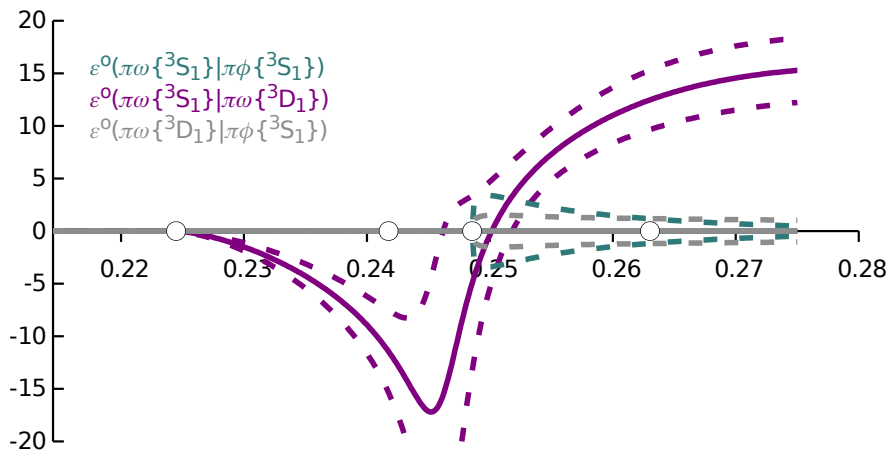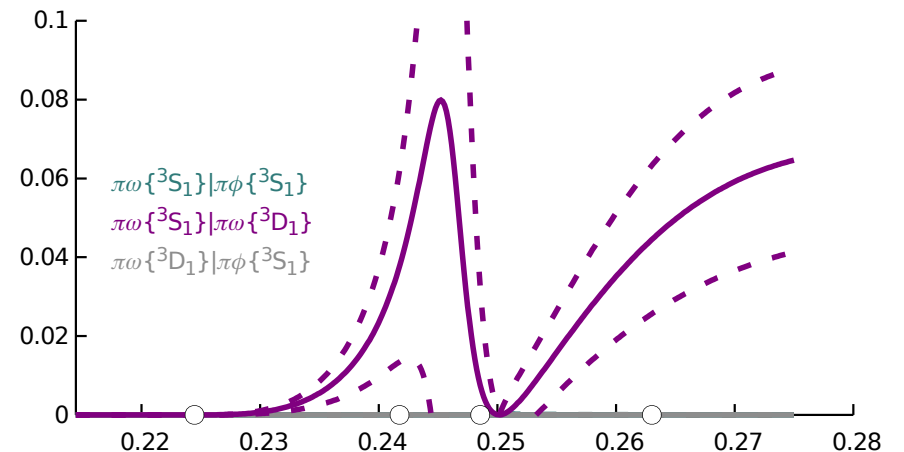



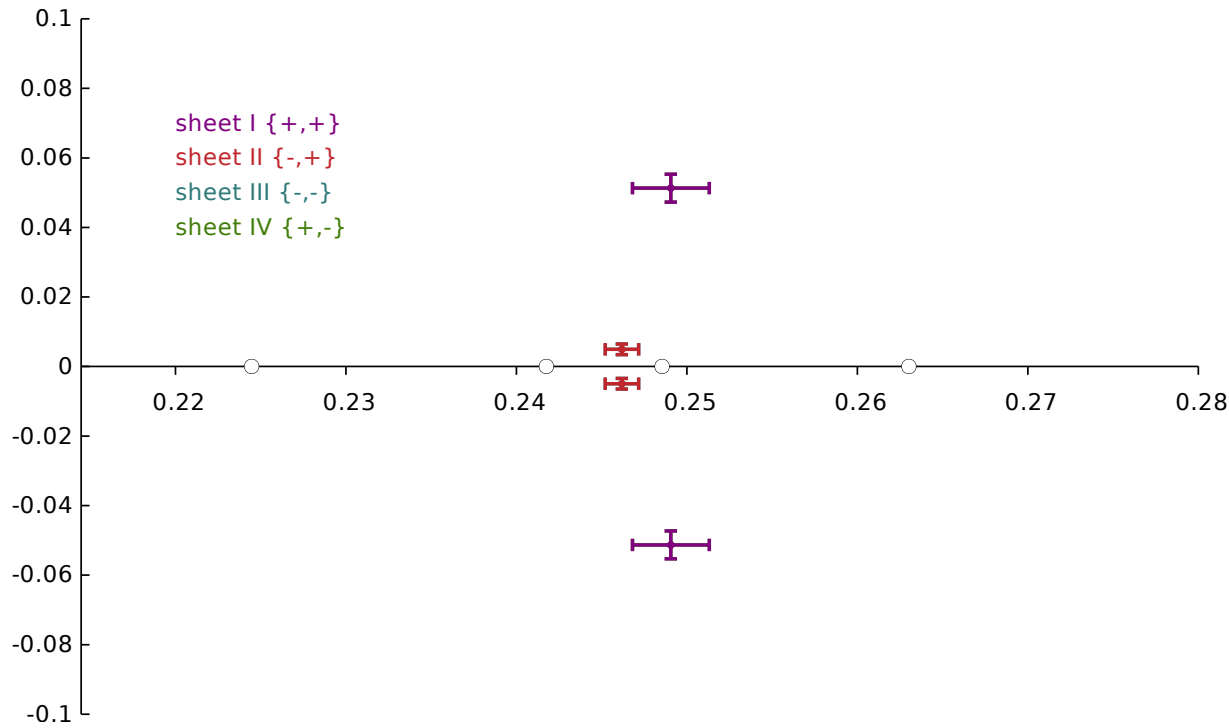

### parameter values

minimised with  $\text{chisq}/\text{nDoF} = 31.74 / (36 - 8) = 1.13$

|                                               |  |                          |  |      |      |       |      |       |       |       |       |
|-----------------------------------------------|--|--------------------------|--|------|------|-------|------|-------|-------|-------|-------|
| JP1+_g_pi:omega/3^D_1_pole0                   |  | -1.5754 +/- 1.1522       |  | 1.00 | 0.93 | -0.04 | 0.40 | -0.23 | 0.08  | -0.03 | -0.58 |
| JP1+_g_pi:omega/3^S_1_pole0                   |  | 0.056120 +/- 0.013546    |  |      | 1.00 | -0.05 | 0.26 | -0.31 | 0.13  | 0.01  | -0.67 |
| JP1+_g_pi:phi/3^S_1_pole0                     |  | -1.0156e-05 +/- 0.013765 |  |      |      | 1.00  | 0.00 | 0.01  | -0.00 | -0.02 | -0.03 |
| JP1+_gamma_pi:omega/3^S_1 pi:omega/3^D_1_orde |  | -49.510 +/- 11.958       |  |      |      |       | 1.00 | -0.29 | 0.37  | -0.08 | -0.23 |
| JP1+_gamma_pi:omega/3^S_1 pi:omega/3^S_1_orde |  | 7.1524 +/- 0.556         |  |      |      |       |      | 1.00  | -0.95 | -0.00 | 0.20  |
| JP1+_gamma_pi:omega/3^S_1 pi:omega/3^S_1_orde |  | -137.29 +/- 10.628       |  |      |      |       |      |       | 1.00  | 0.05  | -0.10 |
| JP1+_gamma_pi:phi/3^S_1 pi:phi/3^S_1_order0   |  | 0.93591 +/- 0.29484      |  |      |      |       |      |       |       | 1.00  | -0.20 |
| JP1+_m_pole0                                  |  | 0.24655 +/- 0.00064837   |  |      |      |       |      |       |       |       | 1.00  |

### pole singularities

pi:omega[+] pi:phi[+] upper half-plane

$\text{sqrt}(s)_{\text{pole}} = (0.24906 \pm 0.0022514)$   
 $+ (i/2) * (0.051312 \pm 0.0040097) [0.28]$

$s_{\text{pole}} = (0.061375 \pm 0.0010967)$   
 $+ i * (0.01278 \pm 0.0010375) [0.30]$

|                         |                         |
|-------------------------|-------------------------|
| pi:omega                | pi:phi                  |
| =====                   | =====                   |
| k_re= 0.0551 +/- 0.0022 | k_re= 0.0345 +/- 0.0025 |



## 2 Unphysical Parameterizations

```

k_im= 0.0262 +/- 0.0017 | k_im= 0.0374 +/- 0.0018 |
corr= [ 0.17] | corr= [-0.02] |

```

```

===== pi:omega/3^S_1(*) | pi:phi/3^S_1 | pi:omega/3^D_1 |
=====
|g|= 0.1424 +/- 0.0042 | |g|= 0.0001 +/- 0.0017 | |g|= 0.0482 +/- 0.0083 |
arg(g)/pi= -0.2299 +/- 0.0045 | arg(g)/pi= -0.5163 +/- 11.3389 | arg(g)/pi= -0.1920 +/- 0.0116 |
-----
g_re= 0.1069 +/- 0.0033 | g_re= 0.0000 +/- 0.0028 | g_re= 0.0397 +/- 0.0068 |
g_im= -0.0942 +/- 0.0033 | g_im= 0.0000 +/- 0.0001 | g_im= -0.0273 +/- 0.0052 |
corr= [-0.63] | corr= [ 0.93] | corr= [-0.91] |
-----
Br = 0.6437 +/- 0.0497 | Br = 0.0000 +/- 0.0000 | Br = 0.0736 +/- 0.0295 |

```

```

--
pi:omega[+] pi:phi[+] lower half-plane

```

```

sqrt(s)_pole = (0.24906 +/- 0.0022514)
+ (i/2)*(-0.051312 +/- 0.0040097) [-0.28]

```

```

s_pole = (0.061375 +/- 0.0010967)
+ i*(-0.01278 +/- 0.0010375) [-0.30]

```

```

===== pi:omega | pi:phi |
=====
k_re= -0.0551 +/- 0.0022 | k_re= -0.0345 +/- 0.0025 |
k_im= 0.0262 +/- 0.0017 | k_im= 0.0374 +/- 0.0018 |
corr= [-0.17] | corr= [ 0.02] |

```

```

===== pi:omega/3^S_1(*) | pi:phi/3^S_1 | pi:omega/3^D_1 |
=====
|g|= 0.1424 +/- 0.0042 | |g|= 0.0001 +/- 0.0017 | |g|= 0.0482 +/- 0.0083 |
arg(g)/pi= 0.2299 +/- 0.0045 | arg(g)/pi= 0.5163 +/- 11.3389 | arg(g)/pi= 0.1920 +/- 0.0116 |
-----
g_re= 0.1069 +/- 0.0033 | g_re= 0.0000 +/- 0.0028 | g_re= 0.0397 +/- 0.0068 |
g_im= 0.0942 +/- 0.0033 | g_im= -0.0000 +/- 0.0001 | g_im= 0.0273 +/- 0.0052 |
corr= [ 0.63] | corr= [-0.93] | corr= [ 0.91] |
-----
Br = 0.6437 +/- 0.0497 | Br = 0.0000 +/- 0.0000 | Br = 0.0736 +/- 0.0295 |

```

```

--
pi:omega[+] pi:phi[-] lower half-plane

```

```

sqrt(s)_pole = (0.24906 +/- 0.0022514)
+ (i/2)*(-0.051312 +/- 0.0040097) [-0.28]

```

```

s_pole = (0.061375 +/- 0.0010967)
+ i*(-0.01278 +/- 0.0010375) [-0.30]

```

```

===== pi:omega | pi:phi |
=====
k_re= -0.0551 +/- 0.0022 | k_re= 0.0345 +/- 0.0025 |
k_im= 0.0262 +/- 0.0017 | k_im= -0.0374 +/- 0.0018 |
corr= [-0.17] | corr= [ 0.02] |

```

```

===== pi:omega/3^S_1(*) | pi:phi/3^S_1 | pi:omega/3^D_1 |
=====
|g|= 0.1424 +/- 0.0042 | |g|= 0.0001 +/- 0.0026 | |g|= 0.0482 +/- 0.0083 |
arg(g)/pi= 0.2299 +/- 0.0045 | arg(g)/pi= -0.3391 +/- 11.1546 | arg(g)/pi= 0.1920 +/- 0.0116 |
-----
g_re= 0.1069 +/- 0.0033 | g_re= 0.0000 +/- 0.0035 | g_re= 0.0397 +/- 0.0068 |
g_im= 0.0942 +/- 0.0033 | g_im= 0.0000 +/- 0.0024 | g_im= 0.0273 +/- 0.0052 |

```



## 2 Unphysical Parameterizations

```

corr= [ 0.63] | corr= [ 1.00] | corr= [ 0.91] |
-----|-----|-----|
Br = 0.6437 +/- 0.0497 | Br = 0.0000 +/- 0.0000 | Br = 0.0736 +/- 0.0295 |

--
pi:omega[+] pi:phi[-] upper half-plane

sqrt(s)_pole = (0.24906 +/- 0.0022514)
               + (i/2)*(+0.051312 +/- 0.0040097) [ 0.28]

s_pole = (0.061375 +/- 0.0010967)
          + i*(+0.01278 +/- 0.0010375) [ 0.30]

=====|=====|
pi:omega | pi:phi |
=====|=====|
k_re= 0.0551 +/- 0.0022 | k_re= -0.0345 +/- 0.0025 |
k_im= 0.0262 +/- 0.0017 | k_im= -0.0374 +/- 0.0018 |
corr= [ 0.17] | corr= [-0.02] |

=====|=====|
pi:omega/3^S_1(*) | pi:phi/3^S_1 | pi:omega/3^D_1 |
=====|=====|=====|
|g|= 0.1424 +/- 0.0042 | |g|= 0.0001 +/- 0.0026 | |g|= 0.0482 +/- 0.0083 |
arg(g)/pi= -0.2299 +/- 0.0045 | arg(g)/pi= 0.3391 +/- 11.1546 | arg(g)/pi= -0.1920 +/- 0.0116 |
-----|-----|-----|
g_re= 0.1069 +/- 0.0033 | g_re= 0.0000 +/- 0.0035 | g_re= 0.0397 +/- 0.0068 |
g_im= -0.0942 +/- 0.0033 | g_im= -0.0000 +/- 0.0024 | g_im= -0.0273 +/- 0.0052 |
corr= [-0.63] | corr= [-1.00] | corr= [-0.91] |
-----|-----|-----|
Br = 0.6437 +/- 0.0497 | Br = 0.0000 +/- 0.0000 | Br = 0.0736 +/- 0.0295 |

--
pi:omega[-] pi:phi[+] upper half-plane

sqrt(s)_pole = (0.27188 +/- 0.010619)
               + (i/2)*(+0.23968 +/- 0.064676) [ 0.91]

s_pole = (0.059553 +/- 0.0035147)
          + i*(+0.065165 +/- 0.019921) [-0.68]

=====|=====|
pi:omega | pi:phi |
=====|=====|
k_re= -0.0914 +/- 0.0113 | k_re= 0.0797 +/- 0.0127 |
k_im= -0.0849 +/- 0.0170 | k_im= 0.0923 +/- 0.0168 |
corr= [ 0.96] | corr= [ 0.97] |

=====|=====|
pi:omega/3^S_1 | pi:phi/3^S_1 | pi:omega/3^D_1(*) |
=====|=====|=====|
|g|= 0.0573 +/- 0.0069 | |g|= 0.0001 +/- 0.0018 | |g|= 0.1817 +/- 0.0204 |
arg(g)/pi= 0.5491 +/- 0.0320 | arg(g)/pi= 0.4223 +/- 13.1689 | arg(g)/pi= -0.4684 +/- 0.0327 |
-----|-----|-----|
g_re= -0.0088 +/- 0.0055 | g_re= 0.0000 +/- 0.0030 | g_re= 0.0180 +/- 0.0206 |
g_im= 0.0566 +/- 0.0071 | g_im= -0.0000 +/- 0.0000 | g_im= -0.1808 +/- 0.0185 |
corr= [ 0.21] | corr= [-0.76] | corr= [-1.00] |
-----|-----|-----|
Br = 0.0268 +/- 0.0125 | Br = 0.0000 +/- 0.0000 | Br = 0.2692 +/- 0.0317 |

--
pi:omega[-] pi:phi[+] lower half-plane

sqrt(s)_pole = (0.27188 +/- 0.010619)
               + (i/2)*(-0.23968 +/- 0.064676) [-0.91]

s_pole = (0.059553 +/- 0.0035147)

```



## 2 Unphysical Parameterizations

+ i\*(-0.065165 +/- 0.019921) [ 0.68]

| pi:omega                      |                                | pi:phi          |  |
|-------------------------------|--------------------------------|-----------------|--|
| =====                         |                                | =====           |  |
| k_re= 0.0914 +/- 0.0113       | k_re= -0.0797 +/- 0.0127       |                 |  |
| k_im= -0.0849 +/- 0.0170      | k_im= 0.0923 +/- 0.0168        |                 |  |
| corr= [-0.96]                 | corr= [-0.97]                  |                 |  |
| -----                         |                                | -----           |  |
| pi:omega/3`S_1                |                                | pi:phi/3`S_1    |  |
| =====                         |                                | =====           |  |
| g = 0.0573 +/- 0.0069         | g = 0.0001 +/- 0.0018          |                 |  |
| arg(g)/pi= -0.5491 +/- 0.0320 | arg(g)/pi= -0.4223 +/- 13.1689 |                 |  |
| -----                         |                                | -----           |  |
| g_re= -0.0088 +/- 0.0055      | g_re= 0.0000 +/- 0.0030        |                 |  |
| g_im= -0.0566 +/- 0.0071      | g_im= 0.0000 +/- 0.0000        |                 |  |
| corr= [-0.21]                 | corr= [ 0.76]                  |                 |  |
| -----                         |                                | -----           |  |
| Br = 0.0268 +/- 0.0125        | Br = 0.0000 +/- 0.0000         |                 |  |
| -----                         |                                | -----           |  |
| pi:omega/3`D_1(*)             |                                | pi:phi/3`D_1(*) |  |
| =====                         |                                | =====           |  |
| g = 0.1817 +/- 0.0204         | g = 0.1817 +/- 0.0204          |                 |  |
| arg(g)/pi= 0.4684 +/- 0.0327  | arg(g)/pi= 0.4684 +/- 0.0327   |                 |  |
| -----                         |                                | -----           |  |
| g_re= 0.0180 +/- 0.0206       | g_re= 0.0180 +/- 0.0206        |                 |  |
| g_im= 0.1808 +/- 0.0185       | g_im= 0.1808 +/- 0.0185        |                 |  |
| corr= [ 1.00]                 | corr= [ 1.00]                  |                 |  |
| -----                         |                                | -----           |  |
| Br = 0.2692 +/- 0.0317        | Br = 0.2692 +/- 0.0317         |                 |  |
| -----                         |                                | -----           |  |

--

pi:omega[-] pi:phi[+] lower half-plane

sqrt(s)\_pole = (0.20196 +/- 0.0014676)  
+ (i/2)\*(-1.1041e-16 +/- 5.6455e-14) [ 0.00]

s\_pole = (0.040787 +/- 0.00059281)  
+ i\*(-2.2299e-17 +/- 1.1404e-14) [ 0.00]

| pi:omega                     |  | pi:phi                        |  |                              |  |
|------------------------------|--|-------------------------------|--|------------------------------|--|
| =====                        |  | =====                         |  |                              |  |
| k_re= 0.0000 +/- 0.0000      |  | k_re= -0.0000 +/- 0.0000      |  |                              |  |
| k_im= -0.0443 +/- 0.0013     |  | k_im= 0.0607 +/- 0.0007       |  |                              |  |
| corr= [ 0.00]                |  | corr= [ 0.00]                 |  |                              |  |
| -----                        |  | -----                         |  |                              |  |
| pi:omega/3`S_1(*)            |  | pi:phi/3`S_1                  |  | pi:omega/3`D_1               |  |
| =====                        |  | =====                         |  | =====                        |  |
| g = 0.1067 +/- 0.0037        |  | g = 0.0001 +/- 0.0011         |  | g = 0.0251 +/- 0.0056        |  |
| arg(g)/pi= 0.5000 +/- 0.0000 |  | arg(g)/pi= 0.0293 +/- 11.1046 |  | arg(g)/pi= 0.5000 +/- 0.0000 |  |
| -----                        |  | -----                         |  | -----                        |  |
| g_re= 0.0000 +/- 0.0000      |  | g_re= 0.0000 +/- 0.0000       |  | g_re= 0.0000 +/- 0.0000      |  |
| g_im= 0.1067 +/- 0.0037      |  | g_im= -0.0000 +/- 0.0017      |  | g_im= 0.0251 +/- 0.0056      |  |
| corr= [-1.00]                |  | corr= [-0.19]                 |  | corr= [-0.25]                |  |
| -----                        |  | -----                         |  | -----                        |  |
| Br = 0.0000 +/- 0.0000       |  | Br = 0.0000 +/- 0.0000        |  | Br = 0.0000 +/- 0.0000       |  |

--

pi:omega[-] pi:phi[+] upper half-plane

sqrt(s)\_pole = (0.24619 +/- 0.00097563)  
+ (i/2)\*(+0.0049355 +/- 0.0015193) [-0.84]

s\_pole = (0.060604 +/- 0.00048354)  
+ i\*(+0.0012151 +/- 0.00037003) [-0.84]

| pi:omega                 |                         | pi:phi       |  |
|--------------------------|-------------------------|--------------|--|
| =====                    |                         | =====        |  |
| k_re= -0.0474 +/- 0.0011 | k_re= 0.0071 +/- 0.0011 |              |  |
| k_im= -0.0029 +/- 0.0009 | k_im= 0.0169 +/- 0.0031 |              |  |
| corr= [-0.84]            | corr= [ 0.56]           |              |  |
| -----                    |                         | -----        |  |
| pi:omega/3`S_1(*)        |                         | pi:phi/3`S_1 |  |
| =====                    |                         | =====        |  |
| -----                    |                         | -----        |  |
| pi:omega/3`D_1           |                         | pi:phi/3`D_1 |  |
| =====                    |                         | =====        |  |
| -----                    |                         | -----        |  |



## 2 Unphysical Parameterizations

|                                     |                                      |                                      |
|-------------------------------------|--------------------------------------|--------------------------------------|
| $ g  = 0.0497 \pm 0.0099$           | $ g  = 0.0004 \pm 0.0073$            | $ g  = 0.0181 \pm 0.0091$            |
| $\arg(g)/\pi = 0.1332 \pm 0.0209$   | $\arg(g)/\pi = -0.4510 \pm 11.1485$  | $\arg(g)/\pi = 0.8829 \pm 0.0875$    |
| $g_{\text{re}} = 0.0454 \pm 0.0085$ | $g_{\text{re}} = -0.0000 \pm 0.0119$ | $g_{\text{re}} = -0.0169 \pm 0.0101$ |
| $g_{\text{im}} = 0.0202 \pm 0.0059$ | $g_{\text{im}} = -0.0000 \pm 0.0007$ | $g_{\text{im}} = 0.0065 \pm 0.0022$  |
| $\text{corr} = [0.82]$              | $\text{corr} = [1.00]$               | $\text{corr} = [0.47]$               |
| $\text{Br} = 0.7812 \pm 0.0852$     | $\text{Br} = 0.0000 \pm 0.0000$      | $\text{Br} = 0.1035 \pm 0.1310$      |

--

pi:omega[-] pi:phi[+] lower half-plane

$\text{sqrt}(s)_{\text{pole}} = (0.24619 \pm 0.00097563)$   
 $+ (i/2)*(-0.0049355 \pm 0.0015193) [0.84]$

$s_{\text{pole}} = (0.060604 \pm 0.00048354)$   
 $+ i*(-0.0012151 \pm 0.00037003) [0.84]$

| pi:omega                             | pi:phi                               |
|--------------------------------------|--------------------------------------|
| $k_{\text{re}} = 0.0474 \pm 0.0011$  | $k_{\text{re}} = -0.0071 \pm 0.0011$ |
| $k_{\text{im}} = -0.0029 \pm 0.0009$ | $k_{\text{im}} = 0.0169 \pm 0.0031$  |
| $\text{corr} = [0.84]$               | $\text{corr} = [-0.56]$              |

| pi:omega/3 <sup>S</sup> _1(*)        | pi:phi/3 <sup>S</sup> _1             | pi:omega/3 <sup>D</sup> _1           |
|--------------------------------------|--------------------------------------|--------------------------------------|
| $ g  = 0.0497 \pm 0.0099$            | $ g  = 0.0004 \pm 0.0073$            | $ g  = 0.0181 \pm 0.0091$            |
| $\arg(g)/\pi = -0.1332 \pm 0.0209$   | $\arg(g)/\pi = 0.4510 \pm 11.1485$   | $\arg(g)/\pi = -0.8829 \pm 0.0875$   |
| $g_{\text{re}} = 0.0454 \pm 0.0085$  | $g_{\text{re}} = -0.0000 \pm 0.0119$ | $g_{\text{re}} = -0.0169 \pm 0.0101$ |
| $g_{\text{im}} = -0.0202 \pm 0.0059$ | $g_{\text{im}} = 0.0000 \pm 0.0007$  | $g_{\text{im}} = -0.0065 \pm 0.0022$ |
| $\text{corr} = [-0.82]$              | $\text{corr} = [-1.00]$              | $\text{corr} = [-0.47]$              |
| $\text{Br} = 0.7812 \pm 0.0852$      | $\text{Br} = 0.0000 \pm 0.0000$      | $\text{Br} = 0.1035 \pm 0.1310$      |

--

pi:omega[-] pi:phi[-] upper half-plane

$\text{sqrt}(s)_{\text{pole}} = (0.27188 \pm 0.010619)$   
 $+ (i/2)*(+0.23968 \pm 0.064676) [0.91]$

$s_{\text{pole}} = (0.059553 \pm 0.0035147)$   
 $+ i*(+0.065165 \pm 0.019921) [-0.68]$

| pi:omega                             | pi:phi                               |
|--------------------------------------|--------------------------------------|
| $k_{\text{re}} = -0.0914 \pm 0.0113$ | $k_{\text{re}} = -0.0797 \pm 0.0127$ |
| $k_{\text{im}} = -0.0849 \pm 0.0170$ | $k_{\text{im}} = -0.0923 \pm 0.0168$ |
| $\text{corr} = [0.96]$               | $\text{corr} = [0.97]$               |

| pi:omega/3 <sup>S</sup> _1           | pi:phi/3 <sup>S</sup> _1             | pi:omega/3 <sup>D</sup> _1(*)        |
|--------------------------------------|--------------------------------------|--------------------------------------|
| $ g  = 0.0573 \pm 0.0069$            | $ g  = 0.0001 \pm 0.0021$            | $ g  = 0.1817 \pm 0.0204$            |
| $\arg(g)/\pi = 0.5491 \pm 0.0320$    | $\arg(g)/\pi = 0.1764 \pm 11.1605$   | $\arg(g)/\pi = -0.4684 \pm 0.0327$   |
| $g_{\text{re}} = -0.0088 \pm 0.0055$ | $g_{\text{re}} = 0.0000 \pm 0.0015$  | $g_{\text{re}} = 0.0180 \pm 0.0206$  |
| $g_{\text{im}} = 0.0566 \pm 0.0071$  | $g_{\text{im}} = -0.0000 \pm 0.0030$ | $g_{\text{im}} = -0.1808 \pm 0.0185$ |
| $\text{corr} = [0.21]$               | $\text{corr} = [-1.00]$              | $\text{corr} = [-1.00]$              |
| $\text{Br} = 0.0268 \pm 0.0125$      | $\text{Br} = 0.0000 \pm 0.0000$      | $\text{Br} = 0.2692 \pm 0.0317$      |

--

pi:omega[-] pi:phi[-] upper half-plane



## 2 Unphysical Parameterizations

```
sqrt(s)_pole = (0.24619 +/- 0.00097583)
               + (i/2)*(+0.0049357 +/- 0.0015195) [-0.84]
```

```
s_pole = (0.060604 +/- 0.00048363)
          + i*(+0.0012151 +/- 0.00037006) [-0.84]
```

| pi:omega                 | pi:phi                   |
|--------------------------|--------------------------|
| k_re= -0.0474 +/- 0.0011 | k_re= -0.0071 +/- 0.0011 |
| k_im= -0.0029 +/- 0.0009 | k_im= -0.0169 +/- 0.0031 |
| corr= [-0.84]            | corr= [ 0.56]            |

| pi:omega/3^S_1(*)            | pi:phi/3^S_1                  | pi:omega/3^D_1               |
|------------------------------|-------------------------------|------------------------------|
| g = 0.0497 +/- 0.0099        | g = 0.0005 +/- 0.0094         | g = 0.0181 +/- 0.0091        |
| arg(g)/pi= 0.1332 +/- 0.0209 | arg(g)/pi= 0.4519 +/- 11.1470 | arg(g)/pi= 0.8829 +/- 0.0875 |
| g_re= 0.0454 +/- 0.0085      | g_re= -0.0000 +/- 0.0154      | g_re= -0.0169 +/- 0.0101     |
| g_im= 0.0202 +/- 0.0059      | g_im= 0.0000 +/- 0.0009       | g_im= 0.0065 +/- 0.0022      |
| corr= [ 0.82]                | corr= [-1.00]                 | corr= [ 0.47]                |
| Br = 0.7812 +/- 0.0852       | Br = 0.0000 +/- 0.0000        | Br = 0.1035 +/- 0.1310       |

```
--
pi:omega[-] pi:phi[-] upper half-plane
```

```
sqrt(s)_pole = (0.20196 +/- 0.0014677)
               + (i/2)*(+2.1953e-14 +/- 1.087e-11) [ 0.00]
```

```
s_pole = (0.040787 +/- 0.00059283)
          + i*(+4.4345e-15 +/- 2.1958e-12) [ 0.00]
```

| pi:omega                 | pi:phi                   |
|--------------------------|--------------------------|
| k_re= -0.0000 +/- 0.0000 | k_re= -0.0000 +/- 0.0000 |
| k_im= -0.0443 +/- 0.0013 | k_im= -0.0607 +/- 0.0007 |
| corr= [ 0.00]            | corr= [ 0.00]            |

| pi:omega/3^S_1(*)            | pi:phi/3^S_1                  | pi:omega/3^D_1               |
|------------------------------|-------------------------------|------------------------------|
| g = 0.1067 +/- 0.0037        | g = 0.0003 +/- 0.0059         | g = 0.0251 +/- 0.0056        |
| arg(g)/pi= 0.5000 +/- 0.0000 | arg(g)/pi= 0.0299 +/- 11.1407 | arg(g)/pi= 0.5000 +/- 0.0000 |
| g_re= 0.0000 +/- 0.0000      | g_re= 0.0000 +/- 0.0000       | g_re= 0.0000 +/- 0.0000      |
| g_im= 0.1067 +/- 0.0037      | g_im= -0.0000 +/- 0.0096      | g_im= 0.0251 +/- 0.0056      |
| corr= [-1.00]                | corr= [-0.78]                 | corr= [-0.25]                |
| Br = 0.0000 +/- 0.0000       | Br = 0.0000 +/- 0.0000        | Br = 0.0000 +/- 0.0000       |

```
--
pi:omega[-] pi:phi[-] lower half-plane
```

```
sqrt(s)_pole = (0.27188 +/- 0.010619)
               + (i/2)*(-0.23968 +/- 0.064676) [-0.91]
```

```
s_pole = (0.059553 +/- 0.0035147)
          + i*(-0.065165 +/- 0.019921) [ 0.68]
```

| pi:omega                 | pi:phi                   |
|--------------------------|--------------------------|
| k_re= 0.0914 +/- 0.0113  | k_re= 0.0797 +/- 0.0127  |
| k_im= -0.0849 +/- 0.0170 | k_im= -0.0923 +/- 0.0168 |



## 2 Unphysical Parameterizations

```

corr= [-0.96] | corr= [-0.97] |

```

| pi:omega/3^S_1                                                        | pi:phi/3^S_1                                                        | pi:omega/3^D_1(*)                                                   |
|-----------------------------------------------------------------------|---------------------------------------------------------------------|---------------------------------------------------------------------|
| g = 0.0573 +/- 0.0069<br>arg(g)/pi= -0.5491 +/- 0.0320                | g = 0.0001 +/- 0.0021<br>arg(g)/pi= -0.1764 +/- 11.1605             | g = 0.1817 +/- 0.0204<br>arg(g)/pi= 0.4684 +/- 0.0327               |
| g_re= -0.0088 +/- 0.0055<br>g_im= -0.0566 +/- 0.0071<br>corr= [-0.21] | g_re= 0.0000 +/- 0.0015<br>g_im= 0.0000 +/- 0.0030<br>corr= [ 1.00] | g_re= 0.0180 +/- 0.0206<br>g_im= 0.1808 +/- 0.0185<br>corr= [ 1.00] |
| Br = 0.0268 +/- 0.0125                                                | Br = 0.0000 +/- 0.0000                                              | Br = 0.2692 +/- 0.0317                                              |

```

--
pi:omega[-] pi:phi[-] lower half-plane

sqrt(s)_pole = (0.24619 +/- 0.00097583)
               + (i/2)*(-0.0049357 +/- 0.0015195) [ 0.84]

s_pole = (0.060604 +/- 0.00048363)
         + i*(-0.0012151 +/- 0.00037006) [ 0.84]

```

| pi:omega                                                             | pi:phi                                                               |
|----------------------------------------------------------------------|----------------------------------------------------------------------|
| k_re= 0.0474 +/- 0.0011<br>k_im= -0.0029 +/- 0.0009<br>corr= [ 0.84] | k_re= 0.0071 +/- 0.0011<br>k_im= -0.0169 +/- 0.0031<br>corr= [-0.56] |

| pi:omega/3^S_1(*)                                                    | pi:phi/3^S_1                                                          | pi:omega/3^D_1                                                        |
|----------------------------------------------------------------------|-----------------------------------------------------------------------|-----------------------------------------------------------------------|
| g = 0.0497 +/- 0.0099<br>arg(g)/pi= -0.1332 +/- 0.0209               | g = 0.0005 +/- 0.0094<br>arg(g)/pi= -0.4519 +/- 11.1470               | g = 0.0181 +/- 0.0091<br>arg(g)/pi= -0.8829 +/- 0.0875                |
| g_re= 0.0454 +/- 0.0085<br>g_im= -0.0202 +/- 0.0059<br>corr= [-0.82] | g_re= -0.0000 +/- 0.0154<br>g_im= -0.0000 +/- 0.0009<br>corr= [ 1.00] | g_re= -0.0169 +/- 0.0101<br>g_im= -0.0065 +/- 0.0022<br>corr= [-0.47] |
| Br = 0.7812 +/- 0.0852                                               | Br = 0.0000 +/- 0.0000                                                | Br = 0.1035 +/- 0.1310                                                |



## 2.9 coupled\_po\_pp.3s1\_3d1.pole+G0\_3s1\_3sd1\_3S1+G1\_3s1.gorder0\_3s1\_3d1+gorder1\_3s1.irho

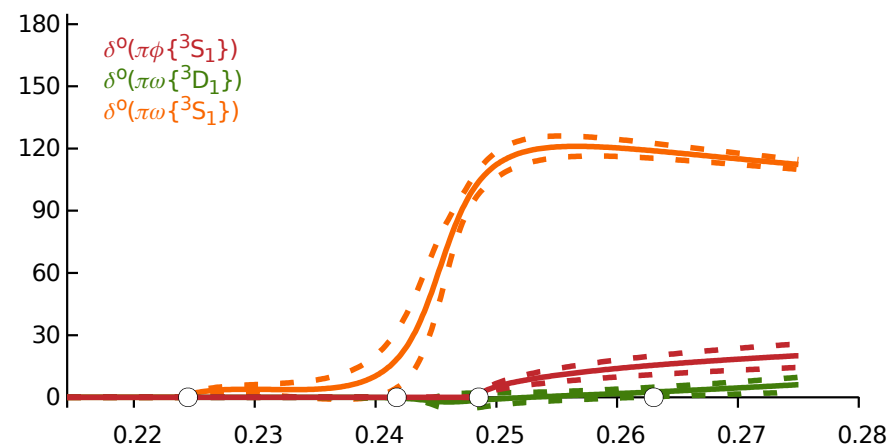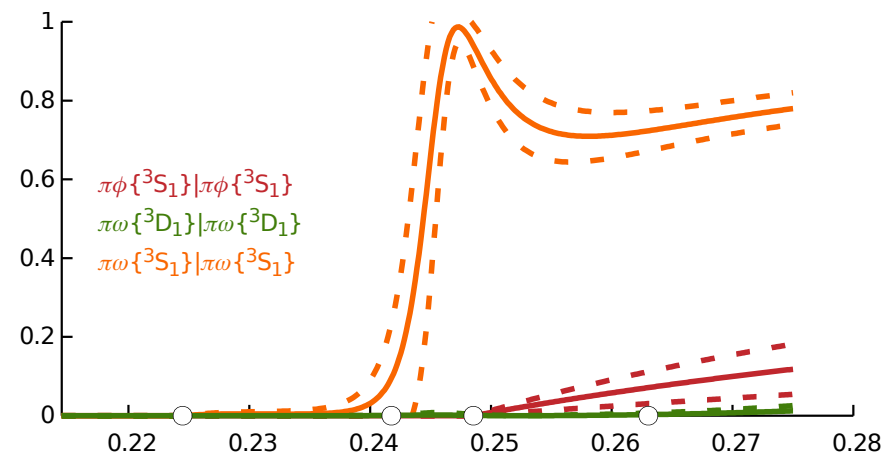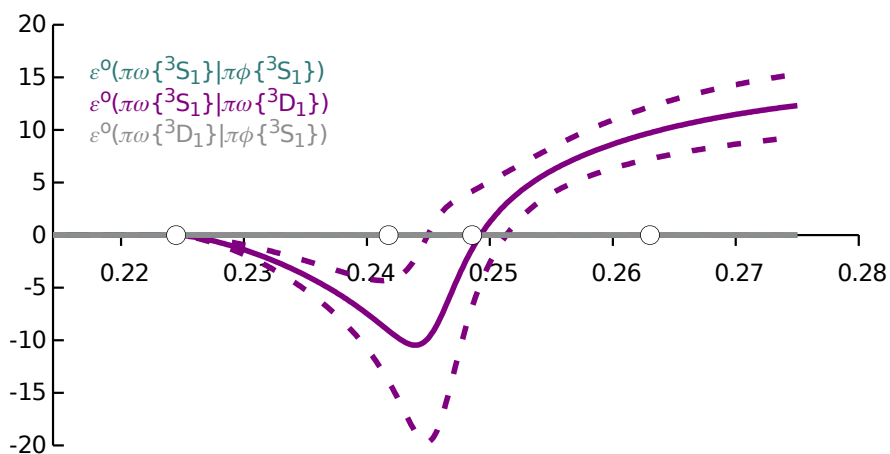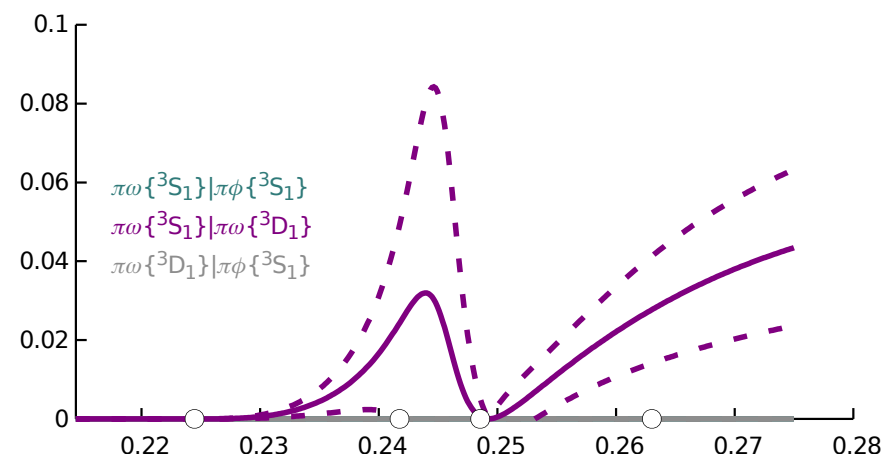



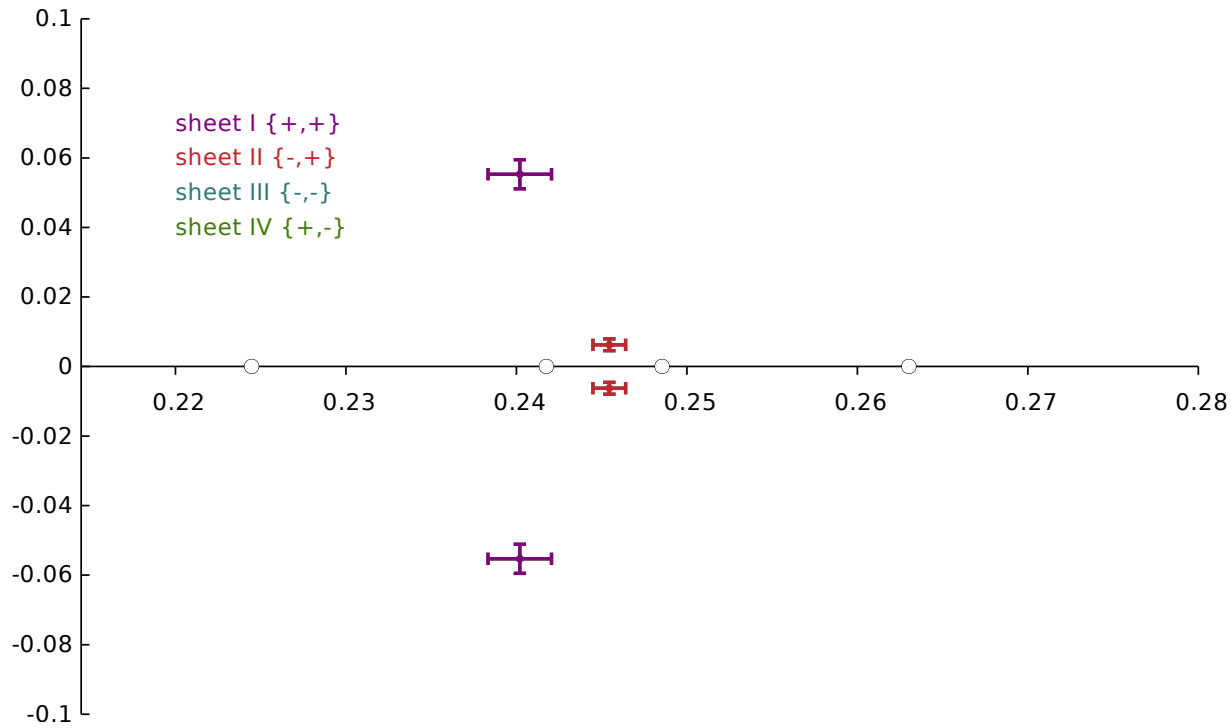

### parameter values

minimised with  $\text{chisq}/\text{nDoF} = 32.91 / (36 - 8) = 1.18$

|                                               |                        |      |      |       |      |       |       |       |       |
|-----------------------------------------------|------------------------|------|------|-------|------|-------|-------|-------|-------|
| JP1+_g_pi:omega/3^D_1_pole0_order0            | -0.68322 +/- 0.98264   | 1.00 | 0.14 | 0.24  | 0.33 | -0.23 | -0.02 | -0.07 | -0.12 |
| JP1+_g_pi:omega/3^S_1_pole0_order0            | 0.12065 +/- 0.034824   |      | 1.00 | -0.91 | 0.03 | -0.13 | -0.08 | -0.01 | -0.02 |
| JP1+_g_pi:omega/3^S_1_pole0_order1            | -0.73003 +/- 0.58369   |      |      | 1.00  | 0.06 | 0.02  | 0.06  | -0.01 | -0.04 |
| JP1+_gamma_pi:omega/3^S_1 pi:omega/3^D_1_orde | -48.781 +/- 13.294     |      |      |       | 1.00 | -0.23 | 0.31  | -0.12 | -0.16 |
| JP1+_gamma_pi:omega/3^S_1 pi:omega/3^S_1_orde | 7.8618 +/- 0.56821     |      |      |       |      | 1.00  | -0.90 | 0.02  | 0.04  |
| JP1+_gamma_pi:omega/3^S_1 pi:omega/3^S_1_orde | -157.86 +/- 11.022     |      |      |       |      |       | 1.00  | 0.04  | -0.02 |
| JP1+_gamma_pi:phi/3^S_1 pi:phi/3^S_1_order0   | 0.93320 +/- 0.28312    |      |      |       |      |       |       | 1.00  | -0.25 |
| JP1+_m_pole0                                  | 0.24712 +/- 0.00054685 |      |      |       |      |       |       |       | 1.00  |

### pole singularities

pi:omega[+] pi:phi[+] upper half-plane

$\text{sqrt}(s)_{\text{pole}} = (0.2402 \pm 0.0018612)$   
 $+ (i/2) * (0.055303 \pm 0.0042018) [0.03]$

$s_{\text{pole}} = (0.056932 \pm 0.00089839)$   
 $+ i * (0.013284 \pm 0.0010174) [-0.00]$

| pi:omega                | pi:phi                  |
|-------------------------|-------------------------|
| =====                   | =====                   |
| k_re= 0.0479 +/- 0.0018 | k_re= 0.0291 +/- 0.0018 |



## 2 Unphysical Parameterizations

```

k_im= 0.0309 +/- 0.0020 | k_im= 0.0444 +/- 0.0018 |
corr= [ 0.11] | corr= [ 0.12] |

```

```

          pi:omega/3^S_1(*) |          pi:phi/3^S_1 |          pi:omega/3^D_1 |
=====|=====|=====|
|g|= 0.1272 +/- 0.0037 | |g|= 0.0000 +/- 0.0000 | |g|= 0.0394 +/- 0.0084 |
arg(g)/pi= -0.1319 +/- 0.0039 | arg(g)/pi= 0.6319 +/- 0.0039 | arg(g)/pi= -0.0993 +/- 0.0148 |
-----|-----|-----|
g_re= 0.1165 +/- 0.0037 | g_re= -0.0000 +/- 0.0000 | g_re= 0.0375 +/- 0.0080 |
g_im= -0.0512 +/- 0.0017 | g_im= 0.0000 +/- 0.0000 | g_im= -0.0121 +/- 0.0031 |
corr= [-0.49] | corr= [-0.71] | corr= [-0.78] |
-----|-----|-----|
Br = 0.4041 +/- 0.0345 | Br = 0.0000 +/- 0.0000 | Br = 0.0387 +/- 0.0184 |

```

```

--
pi:omega[+] pi:phi[+] lower half-plane

```

```

sqrt(s)_pole = ( 0.2402 +/- 0.0018612)
               + (i/2)*(-0.055303 +/- 0.0042018) [-0.03]

```

```

s_pole = (0.056932 +/- 0.00089839)
         + i*(-0.013284 +/- 0.0010174) [ 0.00]

```

```

          pi:omega |          pi:phi |
=====|=====|
k_re= -0.0479 +/- 0.0018 | k_re= -0.0291 +/- 0.0018 |
k_im= 0.0309 +/- 0.0020 | k_im= 0.0444 +/- 0.0018 |
corr= [-0.11] | corr= [-0.12] |

```

```

          pi:omega/3^S_1(*) |          pi:phi/3^S_1 |          pi:omega/3^D_1 |
=====|=====|=====|
|g|= 0.1272 +/- 0.0037 | |g|= 0.0000 +/- 0.0000 | |g|= 0.0394 +/- 0.0084 |
arg(g)/pi= 0.1319 +/- 0.0039 | arg(g)/pi= 0.3681 +/- 0.0039 | arg(g)/pi= 0.0993 +/- 0.0148 |
-----|-----|-----|
g_re= 0.1165 +/- 0.0037 | g_re= 0.0000 +/- 0.0000 | g_re= 0.0375 +/- 0.0080 |
g_im= 0.0512 +/- 0.0017 | g_im= 0.0000 +/- 0.0000 | g_im= 0.0121 +/- 0.0031 |
corr= [ 0.49] | corr= [ 0.71] | corr= [ 0.78] |
-----|-----|-----|
Br = 0.4041 +/- 0.0345 | Br = 0.0000 +/- 0.0000 | Br = 0.0387 +/- 0.0184 |

```

```

--
pi:omega[+] pi:phi[-] upper half-plane

```

```

sqrt(s)_pole = ( 0.2402 +/- 0.0018612)
               + (i/2)*(+0.055303 +/- 0.0042018) [ 0.03]

```

```

s_pole = (0.056932 +/- 0.00089839)
         + i*(+0.013284 +/- 0.0010174) [-0.00]

```

```

          pi:omega |          pi:phi |
=====|=====|
k_re= 0.0479 +/- 0.0018 | k_re= -0.0291 +/- 0.0018 |
k_im= 0.0309 +/- 0.0020 | k_im= -0.0444 +/- 0.0018 |
corr= [ 0.11] | corr= [ 0.12] |

```

```

          pi:omega/3^S_1(*) |          pi:phi/3^S_1 |          pi:omega/3^D_1 |
=====|=====|=====|
|g|= 0.1272 +/- 0.0037 | |g|= 0.0000 +/- 0.0000 | |g|= 0.0394 +/- 0.0084 |
arg(g)/pi= -0.1319 +/- 0.0039 | arg(g)/pi= 0.6319 +/- 0.0039 | arg(g)/pi= -0.0993 +/- 0.0148 |
-----|-----|-----|
g_re= 0.1165 +/- 0.0037 | g_re= -0.0000 +/- 0.0000 | g_re= 0.0375 +/- 0.0080 |
g_im= -0.0512 +/- 0.0017 | g_im= 0.0000 +/- 0.0000 | g_im= -0.0121 +/- 0.0031 |

```



## 2 Unphysical Parameterizations

```

corr= [-0.49] | corr= [-0.71] | corr= [-0.78] |
-----|-----|-----|
Br = 0.4041 +/- 0.0345 | Br = 0.0000 +/- 0.0000 | Br = 0.0387 +/- 0.0184 |

--
pi:omega[+] pi:phi[-] lower half-plane

sqrt(s)_pole = ( 0.2402 +/- 0.0018612)
               + (i/2)*(-0.055303 +/- 0.0042018) [-0.03]

s_pole = (0.056932 +/- 0.00089839)
         + i*(-0.013284 +/- 0.0010174) [ 0.00]

=====|=====|
pi:omega | pi:phi |
=====|=====|
k_re= -0.0479 +/- 0.0018 | k_re= 0.0291 +/- 0.0018 |
k_im= 0.0309 +/- 0.0020 | k_im= -0.0444 +/- 0.0018 |
corr= [-0.11] | corr= [-0.12] |

=====|=====|
pi:omega/3^S_1(*) | pi:phi/3^S_1 | pi:omega/3^D_1 |
=====|=====|=====|
|g|= 0.1272 +/- 0.0037 | |g|= 0.0000 +/- 0.0000 | |g|= 0.0394 +/- 0.0084 |
arg(g)/pi= 0.1319 +/- 0.0039 | arg(g)/pi= 0.3681 +/- 0.0039 | arg(g)/pi= 0.0993 +/- 0.0148 |
-----|-----|-----|
g_re= 0.1165 +/- 0.0037 | g_re= 0.0000 +/- 0.0000 | g_re= 0.0375 +/- 0.0080 |
g_im= 0.0512 +/- 0.0017 | g_im= 0.0000 +/- 0.0000 | g_im= 0.0121 +/- 0.0031 |
corr= [ 0.49] | corr= [ 0.71] | corr= [ 0.78] |
-----|-----|-----|
Br = 0.4041 +/- 0.0345 | Br = 0.0000 +/- 0.0000 | Br = 0.0387 +/- 0.0184 |

--
pi:omega[-] pi:phi[+] lower half-plane

sqrt(s)_pole = (0.19875 +/- 0.0017434)
               + (i/2)*(-3.0966e-15 +/- 1.5467e-12) [ 0.00]

s_pole = (0.039503 +/- 0.00069304)
         + i*(-6.1558e-16 +/- 3.0748e-13) [ 0.00]

=====|=====|
pi:omega | pi:phi |
=====|=====|
k_re= 0.0000 +/- 0.0000 | k_re= -0.0000 +/- 0.0000 |
k_im= -0.0470 +/- 0.0014 | k_im= 0.0620 +/- 0.0007 |
corr= [ 0.00] | corr= [ 0.00] |

=====|=====|
pi:omega/3^S_1(*) | pi:phi/3^S_1 | pi:omega/3^D_1 |
=====|=====|=====|
|g|= 0.1251 +/- 0.0040 | |g|= 0.0000 +/- 0.0000 | |g|= 0.0270 +/- 0.0071 |
arg(g)/pi= 0.5000 +/- 0.0000 | arg(g)/pi= 0.0000 +/- 0.0000 | arg(g)/pi= 0.5000 +/- 0.0000 |
-----|-----|-----|
g_re= 0.0000 +/- 0.0000 | g_re= 0.0000 +/- 0.0000 | g_re= 0.0000 +/- 0.0000 |
g_im= 0.1251 +/- 0.0040 | g_im= 0.0000 +/- 0.0000 | g_im= 0.0270 +/- 0.0071 |
corr= [-1.00] | corr= [ 0.00] | corr= [-0.49] |
-----|-----|-----|
Br = 0.0000 +/- 0.0000 | Br = 0.0000 +/- 0.0000 | Br = 0.0000 +/- 0.0000 |

--
pi:omega[-] pi:phi[+] upper half-plane

sqrt(s)_pole = (0.24545 +/- 0.00096149)
               + (i/2)*(+0.0062435 +/- 0.0016873) [-0.82]

s_pole = (0.060236 +/- 0.00047631)

```



+ i\*(+0.0015325 +/- 0.00040926) [-0.82]

| pi:omega                     |  | pi:phi                       |  |
|------------------------------|--|------------------------------|--|
| =====                        |  | =====                        |  |
| k_re= -0.0466 +/- 0.0011     |  | k_re= 0.0079 +/- 0.0012      |  |
| k_im= -0.0037 +/- 0.0010     |  | k_im= 0.0193 +/- 0.0027      |  |
| corr= [-0.82]                |  | corr= [ 0.62]                |  |
| -----                        |  | -----                        |  |
| pi:omega/3^S_1(*)            |  | pi:phi/3^S_1                 |  |
| =====                        |  | =====                        |  |
| g = 0.0575 +/- 0.0083        |  | g = 0.0000 +/- 0.0000        |  |
| arg(g)/pi= 0.1382 +/- 0.0156 |  | arg(g)/pi= 0.3618 +/- 0.0156 |  |
| -----                        |  | -----                        |  |
| g_re= 0.0522 +/- 0.0073      |  | g_re= 0.0000 +/- 0.0000      |  |
| g_im= 0.0242 +/- 0.0047      |  | g_im= 0.0000 +/- 0.0000      |  |
| corr= [ 0.75]                |  | corr= [ 0.66]                |  |
| -----                        |  | -----                        |  |
| Br = 0.8184 +/- 0.0287       |  | Br = 0.0000 +/- 0.0000       |  |
| -----                        |  | -----                        |  |
| pi:omega/3^D_1               |  | pi:phi/3^D_1                 |  |
| =====                        |  | =====                        |  |
| g = 0.0575 +/- 0.0083        |  | g = 0.0132 +/- 0.0071        |  |
| arg(g)/pi= 0.1382 +/- 0.0156 |  | arg(g)/pi= 0.8338 +/- 0.1085 |  |
| -----                        |  | -----                        |  |
| g_re= 0.0522 +/- 0.0073      |  | g_re= -0.0115 +/- 0.0082     |  |
| g_im= 0.0242 +/- 0.0047      |  | g_im= 0.0066 +/- 0.0019      |  |
| corr= [ 0.75]                |  | corr= [ 0.06]                |  |
| -----                        |  | -----                        |  |
| Br = 0.8184 +/- 0.0287       |  | Br = 0.0434 +/- 0.0564       |  |
| -----                        |  | -----                        |  |

--

pi:omega[-] pi:phi[+] lower half-plane

sqrt(s)\_pole = (0.24545 +/- 0.00096149)  
+ (i/2)\*(-0.0062435 +/- 0.0016873) [ 0.82]

s\_pole = (0.060236 +/- 0.00047631)  
+ i\*(-0.0015325 +/- 0.00040926) [ 0.82]

| pi:omega                      |  | pi:phi                        |  |
|-------------------------------|--|-------------------------------|--|
| =====                         |  | =====                         |  |
| k_re= 0.0466 +/- 0.0011       |  | k_re= -0.0079 +/- 0.0012      |  |
| k_im= -0.0037 +/- 0.0010      |  | k_im= 0.0193 +/- 0.0027       |  |
| corr= [ 0.82]                 |  | corr= [-0.62]                 |  |
| -----                         |  | -----                         |  |
| pi:omega/3^S_1(*)             |  | pi:phi/3^S_1                  |  |
| =====                         |  | =====                         |  |
| g = 0.0575 +/- 0.0083         |  | g = 0.0000 +/- 0.0000         |  |
| arg(g)/pi= -0.1382 +/- 0.0156 |  | arg(g)/pi= 0.6382 +/- 0.0156  |  |
| -----                         |  | -----                         |  |
| g_re= 0.0522 +/- 0.0073       |  | g_re= -0.0000 +/- 0.0000      |  |
| g_im= -0.0242 +/- 0.0047      |  | g_im= 0.0000 +/- 0.0000       |  |
| corr= [-0.75]                 |  | corr= [-0.66]                 |  |
| -----                         |  | -----                         |  |
| Br = 0.8184 +/- 0.0287        |  | Br = 0.0000 +/- 0.0000        |  |
| -----                         |  | -----                         |  |
| pi:omega/3^D_1                |  | pi:phi/3^D_1                  |  |
| =====                         |  | =====                         |  |
| g = 0.0575 +/- 0.0083         |  | g = 0.0132 +/- 0.0071         |  |
| arg(g)/pi= -0.1382 +/- 0.0156 |  | arg(g)/pi= -0.8338 +/- 0.1085 |  |
| -----                         |  | -----                         |  |
| g_re= 0.0522 +/- 0.0073       |  | g_re= -0.0115 +/- 0.0082      |  |
| g_im= -0.0242 +/- 0.0047      |  | g_im= -0.0066 +/- 0.0019      |  |
| corr= [-0.75]                 |  | corr= [-0.06]                 |  |
| -----                         |  | -----                         |  |
| Br = 0.8184 +/- 0.0287        |  | Br = 0.0434 +/- 0.0564        |  |
| -----                         |  | -----                         |  |

--

pi:omega[-] pi:phi[-] lower half-plane

sqrt(s)\_pole = (0.19875 +/- 0.0017434)  
+ (i/2)\*(-1.6036e-12 +/- 8.0261e-10) [-0.02]

s\_pole = (0.039503 +/- 0.00069304)  
+ i\*(-3.1879e-13 +/- 1.5955e-10) [-0.02]

| pi:omega                      |  | pi:phi                        |  |
|-------------------------------|--|-------------------------------|--|
| =====                         |  | =====                         |  |
| k_re= 0.0000 +/- 0.0000       |  | k_re= 0.0000 +/- 0.0000       |  |
| k_im= -0.0470 +/- 0.0014      |  | k_im= -0.0620 +/- 0.0007      |  |
| corr= [ 0.02]                 |  | corr= [ 0.02]                 |  |
| -----                         |  | -----                         |  |
| pi:omega/3^S_1(*)             |  | pi:phi/3^S_1                  |  |
| =====                         |  | =====                         |  |
| g = 0.0575 +/- 0.0083         |  | g = 0.0000 +/- 0.0000         |  |
| arg(g)/pi= -0.1382 +/- 0.0156 |  | arg(g)/pi= 0.6382 +/- 0.0156  |  |
| -----                         |  | -----                         |  |
| g_re= 0.0522 +/- 0.0073       |  | g_re= -0.0000 +/- 0.0000      |  |
| g_im= -0.0242 +/- 0.0047      |  | g_im= 0.0000 +/- 0.0000       |  |
| corr= [-0.75]                 |  | corr= [-0.66]                 |  |
| -----                         |  | -----                         |  |
| Br = 0.8184 +/- 0.0287        |  | Br = 0.0000 +/- 0.0000        |  |
| -----                         |  | -----                         |  |
| pi:omega/3^D_1                |  | pi:phi/3^D_1                  |  |
| =====                         |  | =====                         |  |
| g = 0.0575 +/- 0.0083         |  | g = 0.0132 +/- 0.0071         |  |
| arg(g)/pi= -0.1382 +/- 0.0156 |  | arg(g)/pi= -0.8338 +/- 0.1085 |  |
| -----                         |  | -----                         |  |
| g_re= 0.0522 +/- 0.0073       |  | g_re= -0.0115 +/- 0.0082      |  |
| g_im= -0.0242 +/- 0.0047      |  | g_im= -0.0066 +/- 0.0019      |  |
| corr= [-0.75]                 |  | corr= [-0.06]                 |  |
| -----                         |  | -----                         |  |
| Br = 0.8184 +/- 0.0287        |  | Br = 0.0434 +/- 0.0564        |  |
| -----                         |  | -----                         |  |



## 2 Unphysical Parameterizations

|                                                                     |                                                                     |                                                                     |
|---------------------------------------------------------------------|---------------------------------------------------------------------|---------------------------------------------------------------------|
| g = 0.1251 +/- 0.0040<br>arg(g)/pi= 0.5000 +/- 0.0000               | g = 0.0000 +/- 0.0000<br>arg(g)/pi= 0.0000 +/- 0.0000               | g = 0.0270 +/- 0.0071<br>arg(g)/pi= 0.5000 +/- 0.0000               |
| g_re= 0.0000 +/- 0.0000<br>g_im= 0.1251 +/- 0.0040<br>corr= [-1.00] | g_re= 0.0000 +/- 0.0000<br>g_im= 0.0000 +/- 0.0000<br>corr= [ 0.00] | g_re= 0.0000 +/- 0.0000<br>g_im= 0.0270 +/- 0.0071<br>corr= [-0.49] |
| Br = 0.0000 +/- 0.0000                                              | Br = 0.0000 +/- 0.0000                                              | Br = 0.0000 +/- 0.0000                                              |

--

pi:omega[-] pi:phi[-] upper half-plane

sqr(s)\_pole = (0.24545 +/- 0.00096149)  
+ (i/2)\*(+0.0062435 +/- 0.0016873) [-0.82]

s\_pole = (0.060236 +/- 0.00047631)  
+ i\*(+0.0015325 +/- 0.00040926) [-0.82]

| pi:omega                                                              | pi:phi                                                                |
|-----------------------------------------------------------------------|-----------------------------------------------------------------------|
| k_re= -0.0466 +/- 0.0011<br>k_im= -0.0037 +/- 0.0010<br>corr= [-0.82] | k_re= -0.0079 +/- 0.0012<br>k_im= -0.0193 +/- 0.0027<br>corr= [ 0.62] |

| pi:omega/3^S_1(*)                                                   | pi:phi/3^S_1                                                        | pi:omega/3^D_1                                                       |
|---------------------------------------------------------------------|---------------------------------------------------------------------|----------------------------------------------------------------------|
| g = 0.0575 +/- 0.0083<br>arg(g)/pi= 0.1382 +/- 0.0156               | g = 0.0000 +/- 0.0000<br>arg(g)/pi= 0.3618 +/- 0.0156               | g = 0.0132 +/- 0.0071<br>arg(g)/pi= 0.8338 +/- 0.1085                |
| g_re= 0.0522 +/- 0.0073<br>g_im= 0.0242 +/- 0.0047<br>corr= [ 0.75] | g_re= 0.0000 +/- 0.0000<br>g_im= 0.0000 +/- 0.0000<br>corr= [ 0.66] | g_re= -0.0115 +/- 0.0082<br>g_im= 0.0066 +/- 0.0019<br>corr= [ 0.06] |
| Br = 0.8184 +/- 0.0287                                              | Br = 0.0000 +/- 0.0000                                              | Br = 0.0434 +/- 0.0564                                               |

--

pi:omega[-] pi:phi[-] lower half-plane

sqr(s)\_pole = (0.24545 +/- 0.00096149)  
+ (i/2)\*(-0.0062435 +/- 0.0016873) [ 0.82]

s\_pole = (0.060236 +/- 0.00047631)  
+ i\*(-0.0015325 +/- 0.00040926) [ 0.82]

| pi:omega                                                             | pi:phi                                                               |
|----------------------------------------------------------------------|----------------------------------------------------------------------|
| k_re= 0.0466 +/- 0.0011<br>k_im= -0.0037 +/- 0.0010<br>corr= [ 0.82] | k_re= 0.0079 +/- 0.0012<br>k_im= -0.0193 +/- 0.0027<br>corr= [-0.62] |

| pi:omega/3^S_1(*)                                                    | pi:phi/3^S_1                                                         | pi:omega/3^D_1                                                        |
|----------------------------------------------------------------------|----------------------------------------------------------------------|-----------------------------------------------------------------------|
| g = 0.0575 +/- 0.0083<br>arg(g)/pi= -0.1382 +/- 0.0156               | g = 0.0000 +/- 0.0000<br>arg(g)/pi= 0.6382 +/- 0.0156                | g = 0.0132 +/- 0.0071<br>arg(g)/pi= -0.8338 +/- 0.1085                |
| g_re= 0.0522 +/- 0.0073<br>g_im= -0.0242 +/- 0.0047<br>corr= [-0.75] | g_re= -0.0000 +/- 0.0000<br>g_im= 0.0000 +/- 0.0000<br>corr= [-0.66] | g_re= -0.0115 +/- 0.0082<br>g_im= -0.0066 +/- 0.0019<br>corr= [-0.06] |
| Br = 0.8184 +/- 0.0287                                               | Br = 0.0000 +/- 0.0000                                               | Br = 0.0434 +/- 0.0564                                                |



## 2.10 coupled\_po\_pp.3s1\_3d1.pole+G0\_3s1\_3sd1\_3S1+G1\_3s1.gorder0\_3s1\_3d1+gorder1\_3s1.pole0\_sub

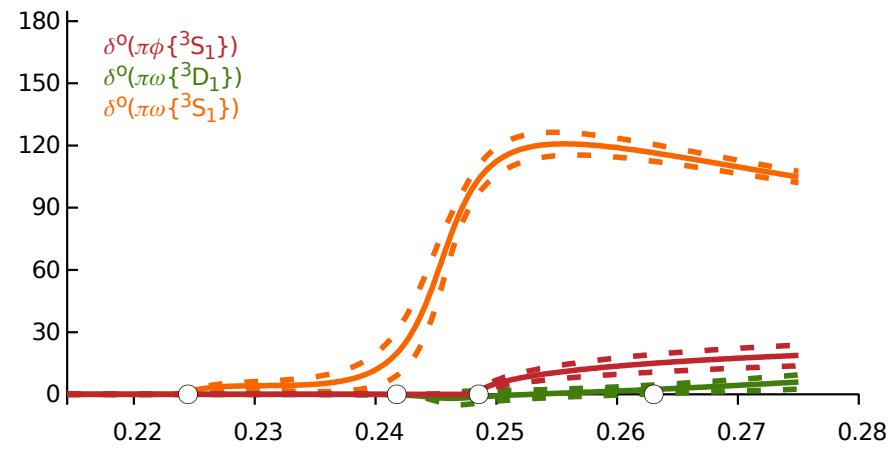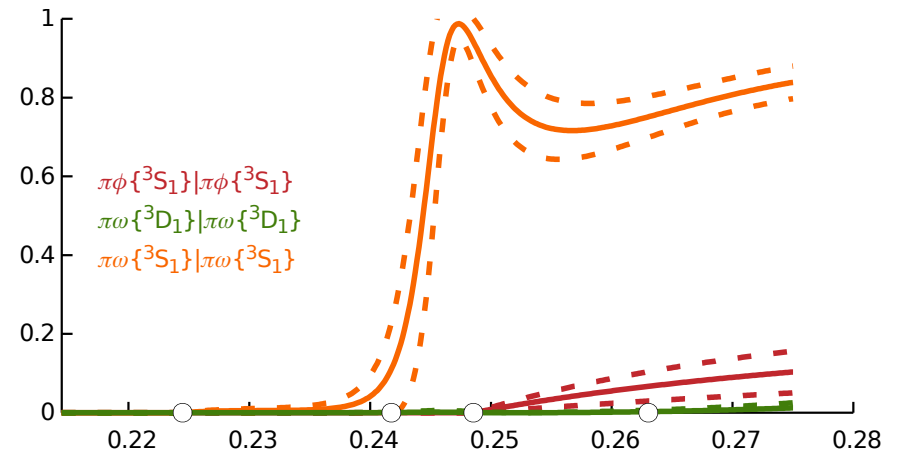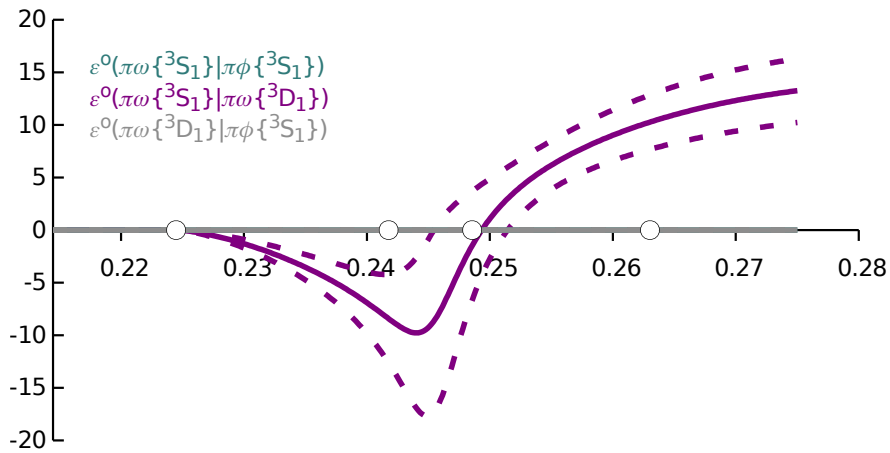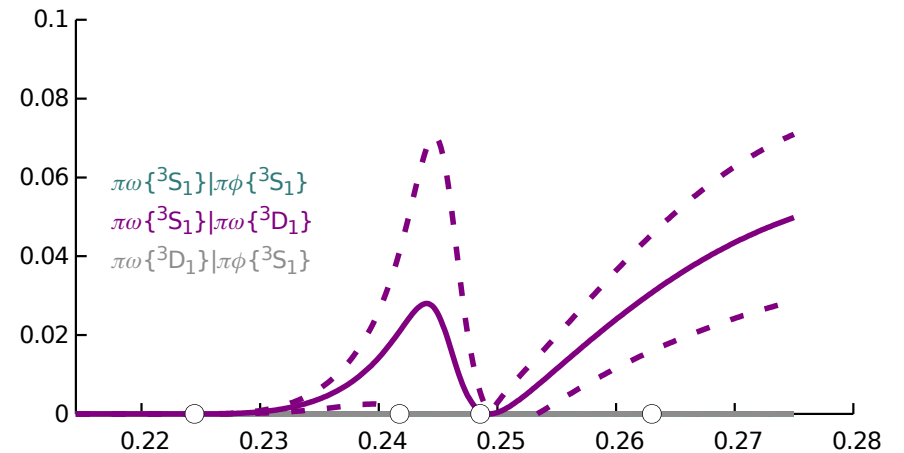



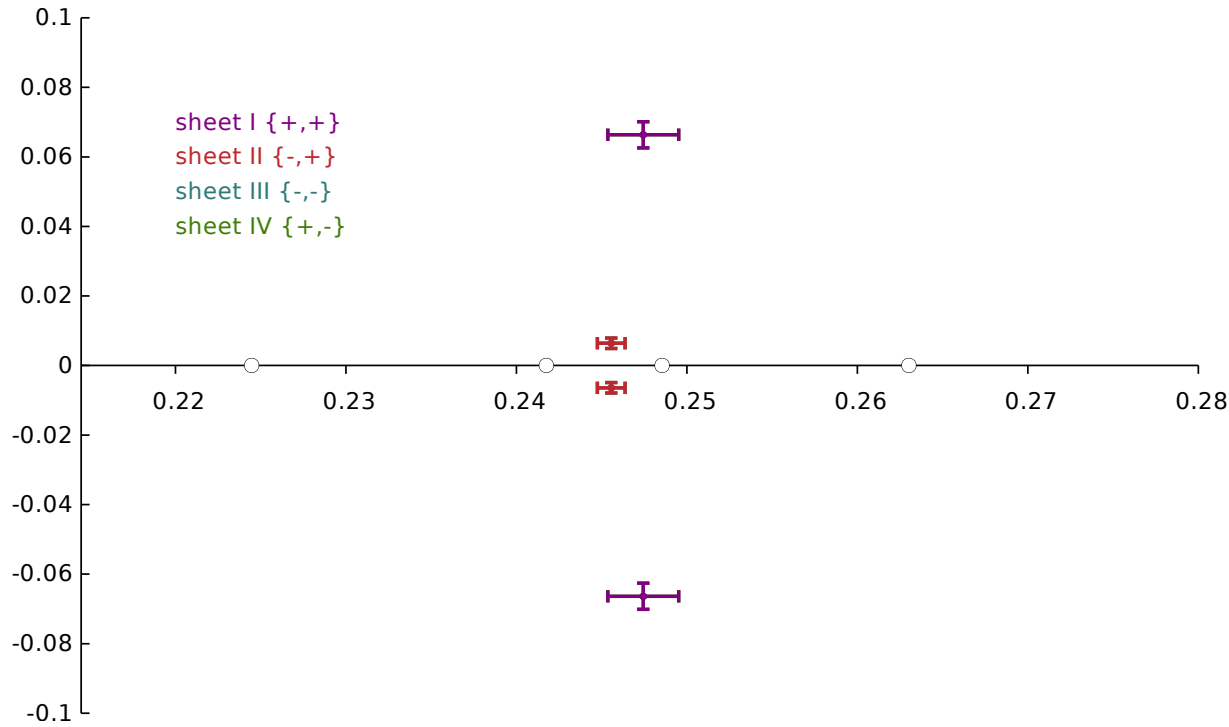

### parameter values

minimised with  $\text{chisq}/\text{nDoF} = 32.81 / (36 - 8) = 1.17$

|                                               |  |                        |  |      |      |       |      |       |       |       |       |
|-----------------------------------------------|--|------------------------|--|------|------|-------|------|-------|-------|-------|-------|
| JP1+_g_pi:omega/3^D_1_pole0_order0            |  | -0.64947 +/- 0.90553   |  | 1.00 | 0.08 | 0.22  | 0.29 | -0.24 | -0.07 | -0.13 | 0.13  |
| JP1+_g_pi:omega/3^S_1_pole0_order0            |  | 0.10805 +/- 0.036508   |  |      | 1.00 | -0.94 | 0.01 | -0.17 | -0.13 | -0.01 | 0.03  |
| JP1+_g_pi:omega/3^S_1_pole0_order1            |  | -0.55600 +/- 0.61415   |  |      |      | 1.00  | 0.04 | 0.07  | 0.10  | -0.03 | 0.01  |
| JP1+_gamma_pi:omega/3^S_1 pi:omega/3^D_1_orde |  | -44.396 +/- 11.735     |  |      |      |       | 1.00 | -0.13 | 0.25  | -0.15 | -0.11 |
| JP1+_gamma_pi:omega/3^S_1 pi:omega/3^S_1_orde |  | 6.6798 +/- 0.35871     |  |      |      |       |      | 1.00  | -0.82 | 0.05  | -0.04 |
| JP1+_gamma_pi:omega/3^S_1 pi:omega/3^S_1_orde |  | -133.94 +/- 6.9516     |  |      |      |       |      |       | 1.00  | 0.06  | -0.06 |
| JP1+_gamma_pi:phi/3^S_1 pi:phi/3^S_1_order0   |  | 0.87601 +/- 0.24811    |  |      |      |       |      |       |       | 1.00  | -0.19 |
| JP1+_m_pole0                                  |  | 0.24717 +/- 0.00056503 |  |      |      |       |      |       |       |       | 1.00  |

### pole singularities

pi:omega[+] pi:phi[+] upper half-plane

$\text{sqrt}(s)_{\text{pole}} = (0.24744 \pm 0.0020766)$   
 $+ (i/2)*(0.066366 \pm 0.0037648) [0.02]$

$s_{\text{pole}} = (0.060126 \pm 0.0010333)$   
 $+ i*(0.016422 \pm 0.0009438) [0.04]$

|                         |                         |
|-------------------------|-------------------------|
| pi:omega                | pi:phi                  |
| =====                   | =====                   |
| k_re= 0.0559 +/- 0.0018 | k_re= 0.0375 +/- 0.0018 |



## 2 Unphysical Parameterizations

```

k_im=  0.0332 +/- 0.0017 |    k_im=  0.0442 +/- 0.0017 |
corr= [-0.05]           |    corr= [-0.09]           |

```

```

          pi:omega/3^S_1(*) |          pi:phi/3^S_1 |          pi:omega/3^D_1 |
=====|=====|=====|
|g|=  0.1599 +/- 0.0040 | |g|=  0.0000 +/- 0.0000 | |g|=  0.0491 +/- 0.0099 |
arg(g)/pi= -0.1997 +/- 0.0033 | arg(g)/pi= 0.6997 +/- 0.0033 | arg(g)/pi= -0.1573 +/- 0.0130 |
-----|-----|-----|
g_re=  0.1295 +/- 0.0032 | g_re= -0.0000 +/- 0.0000 | g_re=  0.0432 +/- 0.0089 |
g_im= -0.0939 +/- 0.0030 | g_im=  0.0000 +/- 0.0000 | g_im= -0.0233 +/- 0.0048 |
corr= [-0.73]           | corr= [-0.68]           | corr= [-0.89]           |
-----|-----|-----|
Br =  0.6131 +/- 0.0322 | Br =  0.0000 +/- 0.0000 | Br =  0.0577 +/- 0.0257 |

```

```

--
pi:omega[+] pi:phi[+] lower half-plane

```

```

sqrt(s)_pole = (0.24744 +/- 0.0020766)
               + (i/2)*(-0.066366 +/- 0.0037648) [-0.02]

```

```

s_pole = (0.060126 +/- 0.0010333)
         + i*(-0.016422 +/- 0.0009438) [-0.04]

```

```

          pi:omega |          pi:phi |
=====|=====|
k_re= -0.0559 +/- 0.0018 | k_re= -0.0375 +/- 0.0018 |
k_im=  0.0332 +/- 0.0017 | k_im=  0.0442 +/- 0.0017 |
corr= [ 0.05]           | corr= [ 0.09]           |

```

```

          pi:omega/3^S_1(*) |          pi:phi/3^S_1 |          pi:omega/3^D_1 |
=====|=====|=====|
|g|=  0.1599 +/- 0.0040 | |g|=  0.0000 +/- 0.0000 | |g|=  0.0491 +/- 0.0099 |
arg(g)/pi= 0.1997 +/- 0.0033 | arg(g)/pi= 0.3003 +/- 0.0033 | arg(g)/pi= 0.1573 +/- 0.0130 |
-----|-----|-----|
g_re=  0.1295 +/- 0.0032 | g_re=  0.0000 +/- 0.0000 | g_re=  0.0432 +/- 0.0089 |
g_im=  0.0939 +/- 0.0030 | g_im=  0.0000 +/- 0.0000 | g_im=  0.0233 +/- 0.0048 |
corr= [ 0.73]           | corr= [ 0.68]           | corr= [ 0.89]           |
-----|-----|-----|
Br =  0.6131 +/- 0.0322 | Br =  0.0000 +/- 0.0000 | Br =  0.0577 +/- 0.0257 |

```

```

--
pi:omega[+] pi:phi[-] lower half-plane

```

```

sqrt(s)_pole = (0.24744 +/- 0.0020766)
               + (i/2)*(-0.066366 +/- 0.0037648) [-0.02]

```

```

s_pole = (0.060126 +/- 0.0010333)
         + i*(-0.016422 +/- 0.0009438) [-0.04]

```

```

          pi:omega |          pi:phi |
=====|=====|
k_re= -0.0559 +/- 0.0018 | k_re=  0.0375 +/- 0.0018 |
k_im=  0.0332 +/- 0.0017 | k_im= -0.0442 +/- 0.0017 |
corr= [ 0.05]           | corr= [ 0.09]           |

```

```

          pi:omega/3^S_1(*) |          pi:phi/3^S_1 |          pi:omega/3^D_1 |
=====|=====|=====|
|g|=  0.1599 +/- 0.0040 | |g|=  0.0000 +/- 0.0000 | |g|=  0.0491 +/- 0.0099 |
arg(g)/pi= 0.1997 +/- 0.0033 | arg(g)/pi= 0.3003 +/- 0.0033 | arg(g)/pi= 0.1573 +/- 0.0130 |
-----|-----|-----|
g_re=  0.1295 +/- 0.0032 | g_re=  0.0000 +/- 0.0000 | g_re=  0.0432 +/- 0.0089 |
g_im=  0.0939 +/- 0.0030 | g_im=  0.0000 +/- 0.0000 | g_im=  0.0233 +/- 0.0048 |

```



## 2 Unphysical Parameterizations

```

corr= [ 0.73] | corr= [ 0.68] | corr= [ 0.89] |
-----|-----|-----|
Br = 0.6131 +/- 0.0322 | Br = 0.0000 +/- 0.0000 | Br = 0.0577 +/- 0.0257 |

--
pi:omega[+] pi:phi[-] upper half-plane

sqrt(s)_pole = (0.24744 +/- 0.0020766)
               + (i/2)*(+0.066366 +/- 0.0037648) [ 0.02]

s_pole = (0.060126 +/- 0.0010333)
          + i*(+0.016422 +/- 0.0009438) [ 0.04]

=====|=====|
pi:omega | pi:phi |
=====|=====|
k_re= 0.0559 +/- 0.0018 | k_re= -0.0375 +/- 0.0018 |
k_im= 0.0332 +/- 0.0017 | k_im= -0.0442 +/- 0.0017 |
corr= [-0.05] | corr= [-0.09] |

=====|=====|
pi:omega/3^S_1(*) | pi:phi/3^S_1 | pi:omega/3^D_1 |
=====|=====|=====|
|g|= 0.1599 +/- 0.0040 | |g|= 0.0000 +/- 0.0000 | |g|= 0.0491 +/- 0.0099 |
arg(g)/pi= -0.1997 +/- 0.0033 | arg(g)/pi= 0.6997 +/- 0.0033 | arg(g)/pi= -0.1573 +/- 0.0130 |
-----|-----|-----|
g_re= 0.1295 +/- 0.0032 | g_re= -0.0000 +/- 0.0000 | g_re= 0.0432 +/- 0.0089 |
g_im= -0.0939 +/- 0.0030 | g_im= 0.0000 +/- 0.0000 | g_im= -0.0233 +/- 0.0048 |
corr= [-0.73] | corr= [-0.68] | corr= [-0.89] |
-----|-----|-----|
Br = 0.6131 +/- 0.0322 | Br = 0.0000 +/- 0.0000 | Br = 0.0577 +/- 0.0257 |

--
pi:omega[-] pi:phi[+] upper half-plane

sqrt(s)_pole = (0.27735 +/- 0.010309)
               + (i/2)*(+0.24413 +/- 0.072227) [ 0.95]

s_pole = (0.062021 +/- 0.0037939)
          + i*(+0.067711 +/- 0.022447) [-0.87]

=====|=====|
pi:omega | pi:phi |
=====|=====|
k_re= -0.0949 +/- 0.0116 | k_re= 0.0834 +/- 0.0131 |
k_im= -0.0852 +/- 0.0192 | k_im= 0.0925 +/- 0.0190 |
corr= [ 0.98] | corr= [ 0.99] |

=====|=====|
pi:omega/3^S_1 | pi:phi/3^S_1 | pi:omega/3^D_1(*) |
=====|=====|=====|
|g|= 0.0552 +/- 0.0054 | |g|= 0.0000 +/- 0.0000 | |g|= 0.1887 +/- 0.0232 |
arg(g)/pi= 0.5397 +/- 0.0344 | arg(g)/pi= 0.9815 +/- 0.0361 | arg(g)/pi= -0.4815 +/- 0.0361 |
-----|-----|-----|
g_re= -0.0069 +/- 0.0054 | g_re= -0.0000 +/- 0.0000 | g_re= 0.0110 +/- 0.0227 |
g_im= 0.0547 +/- 0.0060 | g_im= 0.0000 +/- 0.0000 | g_im= -0.1883 +/- 0.0219 |
corr= [ 0.81] | corr= [ 1.00] | corr= [-1.00] |
-----|-----|-----|
Br = 0.0249 +/- 0.0134 | Br = 0.0000 +/- 0.0000 | Br = 0.2910 +/- 0.0355 |

--
pi:omega[-] pi:phi[+] lower half-plane

sqrt(s)_pole = (0.27735 +/- 0.010309)
               + (i/2)*(-0.24413 +/- 0.072227) [-0.95]

s_pole = (0.062021 +/- 0.0037939)

```



## 2 Unphysical Parameterizations

+ i\*(-0.067711 +/- 0.022447) [ 0.87]

| pi:omega                      |                              | pi:phi          |  |
|-------------------------------|------------------------------|-----------------|--|
| =====                         |                              | =====           |  |
| k_re= 0.0949 +/- 0.0116       | k_re= -0.0834 +/- 0.0131     |                 |  |
| k_im= -0.0852 +/- 0.0192      | k_im= 0.0925 +/- 0.0190      |                 |  |
| corr= [-0.98]                 | corr= [-0.99]                |                 |  |
| -----                         |                              | -----           |  |
| pi:omega/3^S_1                |                              | pi:phi/3^S_1    |  |
| =====                         |                              | =====           |  |
| g = 0.0552 +/- 0.0054         | g = 0.0000 +/- 0.0000        |                 |  |
| arg(g)/pi= -0.5397 +/- 0.0344 | arg(g)/pi= 0.0185 +/- 0.0361 |                 |  |
| -----                         |                              | -----           |  |
| g_re= -0.0069 +/- 0.0054      | g_re= 0.0000 +/- 0.0000      |                 |  |
| g_im= -0.0547 +/- 0.0060      | g_im= 0.0000 +/- 0.0000      |                 |  |
| corr= [-0.81]                 | corr= [-1.00]                |                 |  |
| -----                         |                              | -----           |  |
| Br = 0.0249 +/- 0.0134        | Br = 0.0000 +/- 0.0000       |                 |  |
| -----                         |                              | -----           |  |
| pi:omega/3^D_1(*)             |                              | pi:phi/3^D_1(*) |  |
| =====                         |                              | =====           |  |
| g = 0.1887 +/- 0.0232         | g = 0.1887 +/- 0.0232        |                 |  |
| arg(g)/pi= 0.4815 +/- 0.0361  | arg(g)/pi= 0.4815 +/- 0.0361 |                 |  |
| -----                         |                              | -----           |  |
| g_re= 0.0110 +/- 0.0227       | g_re= 0.0110 +/- 0.0227      |                 |  |
| g_im= 0.1883 +/- 0.0219       | g_im= 0.1883 +/- 0.0219      |                 |  |
| corr= [ 1.00]                 | corr= [ 1.00]                |                 |  |
| -----                         |                              | -----           |  |
| Br = 0.2910 +/- 0.0355        | Br = 0.2910 +/- 0.0355       |                 |  |
| -----                         |                              | -----           |  |

--

pi:omega[-] pi:phi[+] lower half-plane

sqrt(s)\_pole = (0.20339 +/- 0.0014496)  
+ (i/2)\*(-1.9254e-15 +/- 9.3274e-13) [ 0.00]

s\_pole = (0.041368 +/- 0.00058969)  
+ i\*(-3.9166e-16 +/- 1.8973e-13) [ 0.00]

| pi:omega                     |                              | pi:phi                       |  |                |  |
|------------------------------|------------------------------|------------------------------|--|----------------|--|
| =====                        |                              | =====                        |  |                |  |
| k_re= 0.0000 +/- 0.0000      | k_re= -0.0000 +/- 0.0000     |                              |  |                |  |
| k_im= -0.0430 +/- 0.0013     | k_im= 0.0600 +/- 0.0007      |                              |  |                |  |
| corr= [ 0.00]                | corr= [ 0.00]                |                              |  |                |  |
| -----                        |                              | -----                        |  |                |  |
| pi:omega/3^S_1(*)            |                              | pi:phi/3^S_1                 |  | pi:omega/3^D_1 |  |
| =====                        |                              | =====                        |  | =====          |  |
| g = 0.1017 +/- 0.0037        | g = 0.0000 +/- 0.0000        | g = 0.0224 +/- 0.0058        |  |                |  |
| arg(g)/pi= 0.5000 +/- 0.0000 | arg(g)/pi= 0.0000 +/- 0.0000 | arg(g)/pi= 0.5000 +/- 0.0000 |  |                |  |
| -----                        |                              | -----                        |  | -----          |  |
| g_re= 0.0000 +/- 0.0000      | g_re= 0.0000 +/- 0.0000      | g_re= 0.0000 +/- 0.0000      |  |                |  |
| g_im= 0.1017 +/- 0.0037      | g_im= 0.0000 +/- 0.0000      | g_im= 0.0224 +/- 0.0058      |  |                |  |
| corr= [-1.00]                | corr= [ 0.00]                | corr= [-0.28]                |  |                |  |
| -----                        |                              | -----                        |  | -----          |  |
| Br = 0.0000 +/- 0.0000       | Br = 0.0000 +/- 0.0000       | Br = 0.0000 +/- 0.0000       |  |                |  |
| -----                        |                              | -----                        |  | -----          |  |

--

pi:omega[-] pi:phi[+] upper half-plane

sqrt(s)\_pole = (0.24556 +/- 0.00081333)  
+ (i/2)\*(+0.0064084 +/- 0.0014939) [-0.72]

s\_pole = (0.060291 +/- 0.00040292)  
+ i\*(+0.0015737 +/- 0.00036311) [-0.72]

| pi:omega                     |                         | pi:phi                       |  |                              |  |
|------------------------------|-------------------------|------------------------------|--|------------------------------|--|
| =====                        |                         | =====                        |  |                              |  |
| k_re= -0.0467 +/- 0.0009     | k_re= 0.0082 +/- 0.0012 |                              |  |                              |  |
| k_im= -0.0038 +/- 0.0009     | k_im= 0.0191 +/- 0.0023 |                              |  |                              |  |
| corr= [-0.72]                | corr= [ 0.51]           |                              |  |                              |  |
| -----                        |                         | -----                        |  |                              |  |
| pi:omega/3^S_1(*)            |                         | pi:phi/3^S_1                 |  | pi:omega/3^D_1               |  |
| =====                        |                         | =====                        |  | =====                        |  |
| g = 0.0000 +/- 0.0000        |                         | g = 0.0000 +/- 0.0000        |  | g = 0.0000 +/- 0.0000        |  |
| arg(g)/pi= 0.5000 +/- 0.0000 |                         | arg(g)/pi= 0.5000 +/- 0.0000 |  | arg(g)/pi= 0.5000 +/- 0.0000 |  |
| -----                        |                         | -----                        |  | -----                        |  |
| g_re= 0.0000 +/- 0.0000      |                         | g_re= 0.0000 +/- 0.0000      |  | g_re= 0.0000 +/- 0.0000      |  |
| g_im= 0.0000 +/- 0.0000      |                         | g_im= 0.0000 +/- 0.0000      |  | g_im= 0.0000 +/- 0.0000      |  |
| corr= [ 0.00]                |                         | corr= [ 0.00]                |  | corr= [ 0.00]                |  |
| -----                        |                         | -----                        |  | -----                        |  |
| Br = 0.0000 +/- 0.0000       |                         | Br = 0.0000 +/- 0.0000       |  | Br = 0.0000 +/- 0.0000       |  |
| -----                        |                         | -----                        |  | -----                        |  |



## 2 Unphysical Parameterizations

|                                     |                                     |                                      |
|-------------------------------------|-------------------------------------|--------------------------------------|
| $ g  = 0.0583 \pm 0.0070$           | $ g  = 0.0000 \pm 0.0000$           | $ g  = 0.0127 \pm 0.0065$            |
| $\arg(g)/\pi = 0.1289 \pm 0.0153$   | $\arg(g)/\pi = 0.3711 \pm 0.0153$   | $\arg(g)/\pi = 0.8342 \pm 0.1083$    |
| $g_{\text{re}} = 0.0536 \pm 0.0061$ | $g_{\text{re}} = 0.0000 \pm 0.0000$ | $g_{\text{re}} = -0.0110 \pm 0.0075$ |
| $g_{\text{im}} = 0.0230 \pm 0.0044$ | $g_{\text{im}} = 0.0000 \pm 0.0000$ | $g_{\text{im}} = 0.0063 \pm 0.0019$  |
| $\text{corr} = [0.74]$              | $\text{corr} = [0.47]$              | $\text{corr} = [0.14]$               |
| $\text{Br} = 0.8196 \pm 0.0222$     | $\text{Br} = 0.0000 \pm 0.0000$     | $\text{Br} = 0.0389 \pm 0.0466$      |

--

pi:omega[-] pi:phi[+] lower half-plane

$\text{sqrt}(s)_{\text{pole}} = (0.24556 \pm 0.00081333)$   
 $+ (i/2)*(-0.0064084 \pm 0.0014939) [0.72]$

$s_{\text{pole}} = (0.060291 \pm 0.00040292)$   
 $+ i*(-0.0015737 \pm 0.00036311) [0.72]$

| pi:omega                             | pi:phi                               |
|--------------------------------------|--------------------------------------|
| $k_{\text{re}} = 0.0467 \pm 0.0009$  | $k_{\text{re}} = -0.0082 \pm 0.0012$ |
| $k_{\text{im}} = -0.0038 \pm 0.0009$ | $k_{\text{im}} = 0.0191 \pm 0.0023$  |
| $\text{corr} = [0.72]$               | $\text{corr} = [-0.51]$              |

| pi:omega/3 <sup>S</sup> _1(*)        | pi:phi/3 <sup>S</sup> _1             | pi:omega/3 <sup>D</sup> _1           |
|--------------------------------------|--------------------------------------|--------------------------------------|
| $ g  = 0.0583 \pm 0.0070$            | $ g  = 0.0000 \pm 0.0000$            | $ g  = 0.0127 \pm 0.0065$            |
| $\arg(g)/\pi = -0.1289 \pm 0.0153$   | $\arg(g)/\pi = 0.6289 \pm 0.0153$    | $\arg(g)/\pi = -0.8342 \pm 0.1083$   |
| $g_{\text{re}} = 0.0536 \pm 0.0061$  | $g_{\text{re}} = -0.0000 \pm 0.0000$ | $g_{\text{re}} = -0.0110 \pm 0.0075$ |
| $g_{\text{im}} = -0.0230 \pm 0.0044$ | $g_{\text{im}} = 0.0000 \pm 0.0000$  | $g_{\text{im}} = -0.0063 \pm 0.0019$ |
| $\text{corr} = [-0.74]$              | $\text{corr} = [-0.47]$              | $\text{corr} = [-0.14]$              |
| $\text{Br} = 0.8196 \pm 0.0222$      | $\text{Br} = 0.0000 \pm 0.0000$      | $\text{Br} = 0.0389 \pm 0.0466$      |

--

pi:omega[-] pi:phi[-] upper half-plane

$\text{sqrt}(s)_{\text{pole}} = (0.27735 \pm 0.010309)$   
 $+ (i/2)*(+0.24413 \pm 0.072227) [0.95]$

$s_{\text{pole}} = (0.062021 \pm 0.0037939)$   
 $+ i*(+0.067711 \pm 0.022447) [-0.87]$

| pi:omega                             | pi:phi                               |
|--------------------------------------|--------------------------------------|
| $k_{\text{re}} = -0.0949 \pm 0.0116$ | $k_{\text{re}} = -0.0834 \pm 0.0131$ |
| $k_{\text{im}} = -0.0852 \pm 0.0192$ | $k_{\text{im}} = -0.0925 \pm 0.0190$ |
| $\text{corr} = [0.98]$               | $\text{corr} = [0.99]$               |

| pi:omega/3 <sup>S</sup> _1           | pi:phi/3 <sup>S</sup> _1             | pi:omega/3 <sup>D</sup> _1(*)        |
|--------------------------------------|--------------------------------------|--------------------------------------|
| $ g  = 0.0552 \pm 0.0054$            | $ g  = 0.0000 \pm 0.0000$            | $ g  = 0.1887 \pm 0.0232$            |
| $\arg(g)/\pi = 0.5397 \pm 0.0344$    | $\arg(g)/\pi = 0.9815 \pm 0.0361$    | $\arg(g)/\pi = -0.4815 \pm 0.0361$   |
| $g_{\text{re}} = -0.0069 \pm 0.0054$ | $g_{\text{re}} = -0.0000 \pm 0.0000$ | $g_{\text{re}} = 0.0110 \pm 0.0227$  |
| $g_{\text{im}} = 0.0547 \pm 0.0060$  | $g_{\text{im}} = 0.0000 \pm 0.0000$  | $g_{\text{im}} = -0.1883 \pm 0.0219$ |
| $\text{corr} = [0.81]$               | $\text{corr} = [1.00]$               | $\text{corr} = [-1.00]$              |
| $\text{Br} = 0.0249 \pm 0.0134$      | $\text{Br} = 0.0000 \pm 0.0000$      | $\text{Br} = 0.2910 \pm 0.0355$      |

--

pi:omega[-] pi:phi[-] upper half-plane



## 2 Unphysical Parameterizations

```
sqrt(s)_pole = (0.24556 +/- 0.00081333)
               + (i/2)*(+0.0064084 +/- 0.0014939) [-0.72]
```

```
s_pole = (0.060291 +/- 0.00040292)
          + i*(+0.0015737 +/- 0.00036311) [-0.72]
```

| pi:omega                 | pi:phi                   |
|--------------------------|--------------------------|
| =====                    | =====                    |
| k_re= -0.0467 +/- 0.0009 | k_re= -0.0082 +/- 0.0012 |
| k_im= -0.0038 +/- 0.0009 | k_im= -0.0191 +/- 0.0023 |
| corr= [-0.72]            | corr= [ 0.51]            |

| pi:omega/3^S_1(*)            | pi:phi/3^S_1                 | pi:omega/3^D_1               |
|------------------------------|------------------------------|------------------------------|
| =====                        | =====                        | =====                        |
| g = 0.0583 +/- 0.0070        | g = 0.0000 +/- 0.0000        | g = 0.0127 +/- 0.0065        |
| arg(g)/pi= 0.1289 +/- 0.0153 | arg(g)/pi= 0.3711 +/- 0.0153 | arg(g)/pi= 0.8342 +/- 0.1083 |
| -----                        | -----                        | -----                        |
| g_re= 0.0536 +/- 0.0061      | g_re= 0.0000 +/- 0.0000      | g_re= -0.0110 +/- 0.0075     |
| g_im= 0.0230 +/- 0.0044      | g_im= 0.0000 +/- 0.0000      | g_im= 0.0063 +/- 0.0019      |
| corr= [ 0.74]                | corr= [ 0.47]                | corr= [ 0.14]                |
| -----                        | -----                        | -----                        |
| Br = 0.8196 +/- 0.0222       | Br = 0.0000 +/- 0.0000       | Br = 0.0389 +/- 0.0466       |

```
--
pi:omega[-] pi:phi[-] upper half-plane
```

```
sqrt(s)_pole = (0.20339 +/- 0.0014496)
               + (i/2)*(+6.8462e-15 +/- 3.4335e-12) [ 0.00]
```

```
s_pole = (0.041368 +/- 0.00058969)
          + i*(+1.3926e-15 +/- 6.9843e-13) [ 0.00]
```

| pi:omega                 | pi:phi                   |
|--------------------------|--------------------------|
| =====                    | =====                    |
| k_re= -0.0000 +/- 0.0000 | k_re= -0.0000 +/- 0.0000 |
| k_im= -0.0430 +/- 0.0013 | k_im= -0.0600 +/- 0.0007 |
| corr= [ 0.00]            | corr= [ 0.00]            |

| pi:omega/3^S_1(*)            | pi:phi/3^S_1                 | pi:omega/3^D_1               |
|------------------------------|------------------------------|------------------------------|
| =====                        | =====                        | =====                        |
| g = 0.1017 +/- 0.0037        | g = 0.0000 +/- 0.0000        | g = 0.0224 +/- 0.0058        |
| arg(g)/pi= 0.5000 +/- 0.0000 | arg(g)/pi= 0.0000 +/- 0.0000 | arg(g)/pi= 0.5000 +/- 0.0000 |
| -----                        | -----                        | -----                        |
| g_re= 0.0000 +/- 0.0000      | g_re= 0.0000 +/- 0.0000      | g_re= 0.0000 +/- 0.0000      |
| g_im= 0.1017 +/- 0.0037      | g_im= 0.0000 +/- 0.0000      | g_im= 0.0224 +/- 0.0058      |
| corr= [-1.00]                | corr= [ 0.00]                | corr= [-0.28]                |
| -----                        | -----                        | -----                        |
| Br = 0.0000 +/- 0.0000       | Br = 0.0000 +/- 0.0000       | Br = 0.0000 +/- 0.0000       |

```
--
pi:omega[-] pi:phi[-] lower half-plane
```

```
sqrt(s)_pole = (0.27735 +/- 0.010309)
               + (i/2)*(-0.24413 +/- 0.072227) [-0.95]
```

```
s_pole = (0.062021 +/- 0.0037939)
          + i*(-0.067711 +/- 0.022447) [ 0.87]
```

| pi:omega                 | pi:phi                   |
|--------------------------|--------------------------|
| =====                    | =====                    |
| k_re= 0.0949 +/- 0.0116  | k_re= 0.0834 +/- 0.0131  |
| k_im= -0.0852 +/- 0.0192 | k_im= -0.0925 +/- 0.0190 |



## 2 Unphysical Parameterizations

```

corr= [-0.98] | corr= [-0.99] |

```

| pi:omega/3^S_1                | pi:phi/3^S_1                 | pi:omega/3^D_1(*)            |
|-------------------------------|------------------------------|------------------------------|
| g = 0.0552 +/- 0.0054         | g = 0.0000 +/- 0.0000        | g = 0.1887 +/- 0.0232        |
| arg(g)/pi= -0.5397 +/- 0.0344 | arg(g)/pi= 0.0185 +/- 0.0361 | arg(g)/pi= 0.4815 +/- 0.0361 |
| g_re= -0.0069 +/- 0.0054      | g_re= 0.0000 +/- 0.0000      | g_re= 0.0110 +/- 0.0227      |
| g_im= -0.0547 +/- 0.0060      | g_im= 0.0000 +/- 0.0000      | g_im= 0.1883 +/- 0.0219      |
| corr= [-0.81]                 | corr= [-1.00]                | corr= [ 1.00]                |
| Br = 0.0249 +/- 0.0134        | Br = 0.0000 +/- 0.0000       | Br = 0.2910 +/- 0.0355       |

```

--
pi:omega[-] pi:phi[-] lower half-plane

sqrt(s)_pole = (0.24556 +/- 0.00081333)
               + (i/2)*(-0.0064084 +/- 0.0014939) [ 0.72]

s_pole = (0.060291 +/- 0.00040292)
         + i*(-0.0015737 +/- 0.00036311) [ 0.72]

```

| pi:omega                 | pi:phi                   |
|--------------------------|--------------------------|
| k_re= 0.0467 +/- 0.0009  | k_re= 0.0082 +/- 0.0012  |
| k_im= -0.0038 +/- 0.0009 | k_im= -0.0191 +/- 0.0023 |
| corr= [ 0.72]            | corr= [-0.51]            |

| pi:omega/3^S_1(*)             | pi:phi/3^S_1                 | pi:omega/3^D_1                |
|-------------------------------|------------------------------|-------------------------------|
| g = 0.0583 +/- 0.0070         | g = 0.0000 +/- 0.0000        | g = 0.0127 +/- 0.0065         |
| arg(g)/pi= -0.1289 +/- 0.0153 | arg(g)/pi= 0.6289 +/- 0.0153 | arg(g)/pi= -0.8342 +/- 0.1083 |
| g_re= 0.0536 +/- 0.0061       | g_re= -0.0000 +/- 0.0000     | g_re= -0.0110 +/- 0.0075      |
| g_im= -0.0230 +/- 0.0044      | g_im= 0.0000 +/- 0.0000      | g_im= -0.0063 +/- 0.0019      |
| corr= [-0.74]                 | corr= [-0.47]                | corr= [-0.14]                 |
| Br = 0.8196 +/- 0.0222        | Br = 0.0000 +/- 0.0000       | Br = 0.0389 +/- 0.0466        |



## 2.11 coupled\_po\_pp.3s1\_3d1.pole+G0\_3s1\_3sd1\_3S1+G1\_3s1.gorder0\_3s1\_3d1+gorder1\_3s1.threshold\_sub

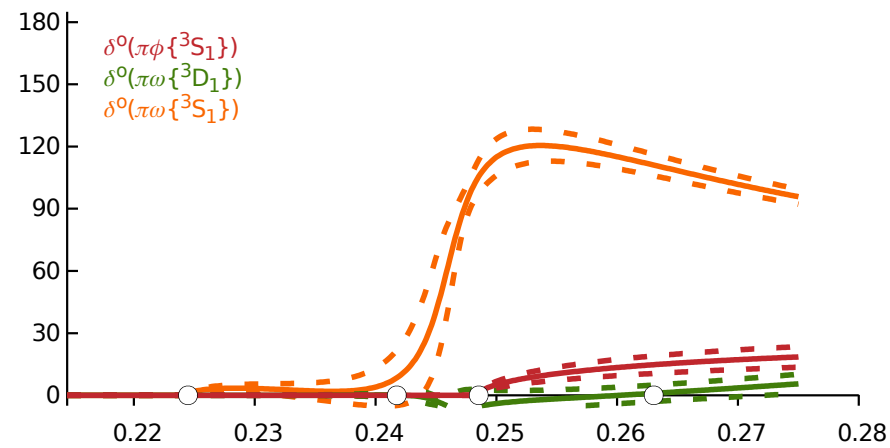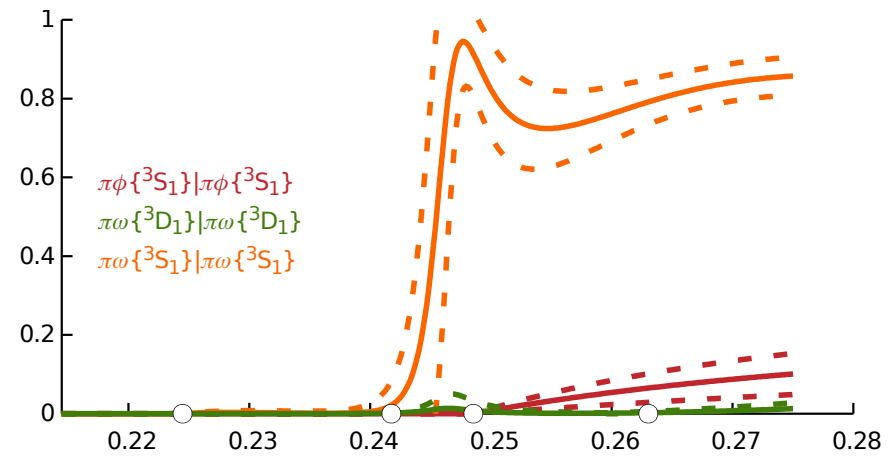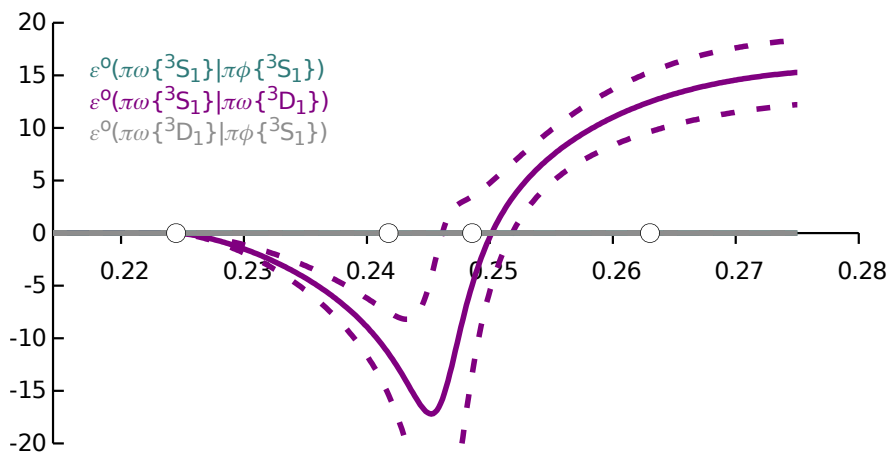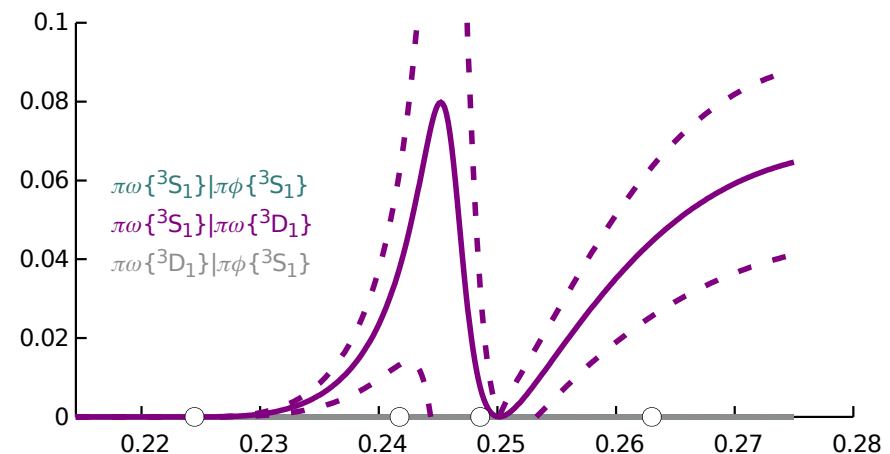



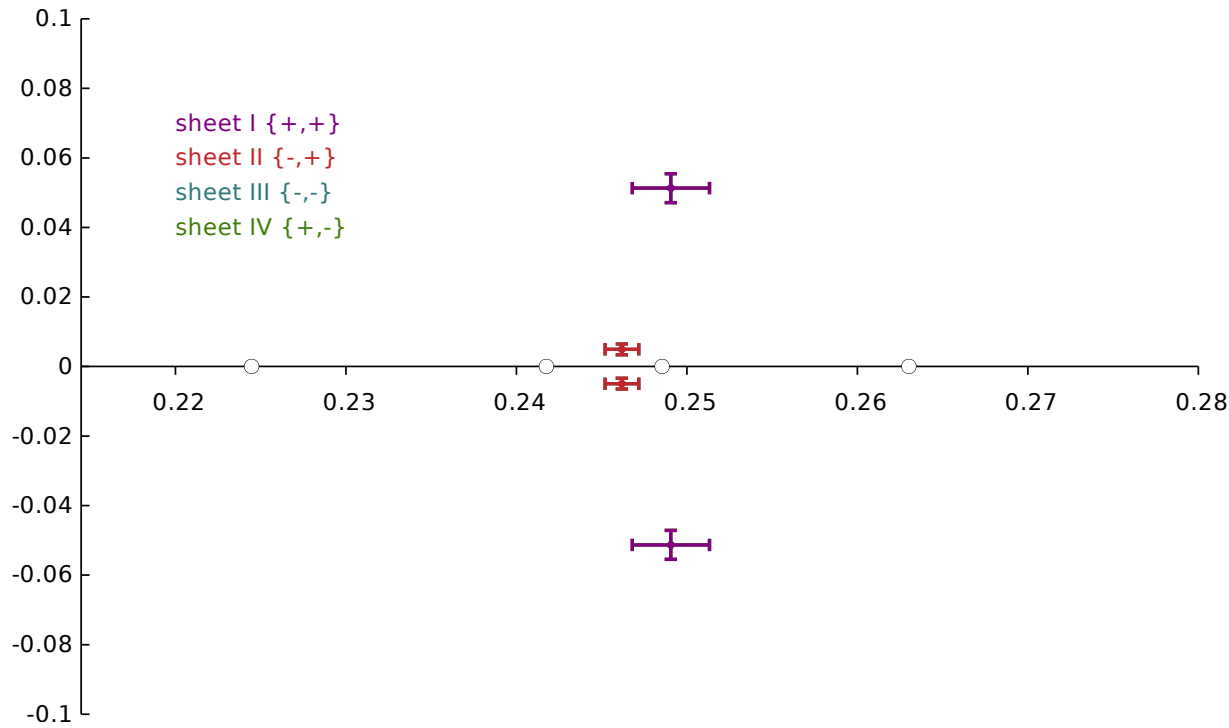

### parameter values

```

minimised with chisq/nDoF = 31.74 / (36 - 8) = 1.13
=====
JP1+_g_pi:omega/3^D_1_pole0_order0 | -1.5750 +/- 1.166 | 1.00 0.06 0.19 0.32 -0.23 0.08 -0.03 -0.59
JP1+_g_pi:omega/3^S_1_pole0_order0 | 0.10273 +/- 0.050521 | 1.00 -0.96 0.07 -0.13 -0.07 -0.01 -0.03
JP1+_g_pi:omega/3^S_1_pole0_order1 | -0.76670 +/- 0.84953 | 1.00 -0.02 0.05 0.10 0.01 -0.15
JP1+_gamma_pi:omega/3^S_1|pi:omega/3^D_1_orde | -48.310 +/- 11.622 | 1.00 -0.28 0.37 -0.08 -0.19
JP1+_gamma_pi:omega/3^S_1|pi:omega/3^S_1_orde | 7.0316 +/- 0.55986 | 1.00 -0.93 -0.00 0.20
JP1+_gamma_pi:omega/3^S_1|pi:omega/3^S_1_orde | -136.73 +/- 10.661 | 1.00 0.05 -0.10
JP1+_gamma_pi:phi/3^S_1|pi:phi/3^S_1_order0 | 0.93586 +/- 0.29477 | 1.00 -0.20
JP1+_m_pole0 | 0.24655 +/- 0.00065445 | 1.00
=====

```

### pole singularities

pi:omega[+] pi:phi[+] upper half-plane

```

sqrt(s)_pole = (0.24906 +/- 0.0022615)
               + (i/2)*(+0.051308 +/- 0.0041576) [ 0.30]

```

```

s_pole = (0.061373 +/- 0.0010996)
          + i*(+0.012779 +/- 0.0010756) [ 0.31]

```

```

=====
pi:omega | pi:phi |
=====|=====|
k_re= 0.0551 +/- 0.0023 | k_re= 0.0345 +/- 0.0025 |

```



## 2 Unphysical Parameterizations

```

k_im= 0.0262 +/- 0.0018 | k_im= 0.0374 +/- 0.0018 |
corr= [ 0.20] | corr= [ 0.01] |

```

```

===== pi:omega/3^S_1(*) | pi:phi/3^S_1 | pi:omega/3^D_1 |
=====
|g|= 0.1424 +/- 0.0042 | |g|= 0.0000 +/- 0.0000 | |g|= 0.0481 +/- 0.0084 |
arg(g)/pi= -0.2299 +/- 0.0047 | arg(g)/pi= 0.7299 +/- 0.0047 | arg(g)/pi= -0.1920 +/- 0.0114 |
-----
g_re= 0.1069 +/- 0.0033 | g_re= -0.0000 +/- 0.0000 | g_re= 0.0397 +/- 0.0068 |
g_im= -0.0942 +/- 0.0034 | g_im= 0.0000 +/- 0.0000 | g_im= -0.0273 +/- 0.0052 |
corr= [-0.61] | corr= [-0.59] | corr= [-0.92] |
-----
Br = 0.6436 +/- 0.0512 | Br = 0.0000 +/- 0.0000 | Br = 0.0736 +/- 0.0297 |

```

```

--
pi:omega[+] pi:phi[+] lower half-plane

```

```

sqrt(s)_pole = (0.24906 +/- 0.0022615)
+ (i/2)*(-0.051308 +/- 0.0041576) [-0.30]

```

```

s_pole = (0.061373 +/- 0.0010996)
+ i*(-0.012779 +/- 0.0010756) [-0.31]

```

```

===== pi:omega | pi:phi |
=====
k_re= -0.0551 +/- 0.0023 | k_re= -0.0345 +/- 0.0025 |
k_im= 0.0262 +/- 0.0018 | k_im= 0.0374 +/- 0.0018 |
corr= [-0.20] | corr= [-0.01] |

```

```

===== pi:omega/3^S_1(*) | pi:phi/3^S_1 | pi:omega/3^D_1 |
=====
|g|= 0.1424 +/- 0.0042 | |g|= 0.0000 +/- 0.0000 | |g|= 0.0481 +/- 0.0084 |
arg(g)/pi= 0.2299 +/- 0.0047 | arg(g)/pi= 0.2701 +/- 0.0047 | arg(g)/pi= 0.1920 +/- 0.0114 |
-----
g_re= 0.1069 +/- 0.0033 | g_re= 0.0000 +/- 0.0000 | g_re= 0.0397 +/- 0.0068 |
g_im= 0.0942 +/- 0.0034 | g_im= 0.0000 +/- 0.0000 | g_im= 0.0273 +/- 0.0052 |
corr= [ 0.61] | corr= [ 0.59] | corr= [ 0.92] |
-----
Br = 0.6436 +/- 0.0512 | Br = 0.0000 +/- 0.0000 | Br = 0.0736 +/- 0.0297 |

```

```

--
pi:omega[+] pi:phi[-] lower half-plane

```

```

sqrt(s)_pole = (0.24906 +/- 0.0022615)
+ (i/2)*(-0.051308 +/- 0.0041577) [-0.30]

```

```

s_pole = (0.061373 +/- 0.0010996)
+ i*(-0.012779 +/- 0.0010756) [-0.31]

```

```

===== pi:omega | pi:phi |
=====
k_re= -0.0551 +/- 0.0023 | k_re= 0.0345 +/- 0.0025 |
k_im= 0.0262 +/- 0.0018 | k_im= -0.0374 +/- 0.0018 |
corr= [-0.20] | corr= [-0.01] |

```

```

===== pi:omega/3^S_1(*) | pi:phi/3^S_1 | pi:omega/3^D_1 |
=====
|g|= 0.1424 +/- 0.0042 | |g|= 0.0000 +/- 0.0000 | |g|= 0.0481 +/- 0.0084 |
arg(g)/pi= 0.2299 +/- 0.0047 | arg(g)/pi= 0.2701 +/- 0.0047 | arg(g)/pi= 0.1920 +/- 0.0114 |
-----
g_re= 0.1069 +/- 0.0033 | g_re= 0.0000 +/- 0.0000 | g_re= 0.0397 +/- 0.0068 |
g_im= 0.0942 +/- 0.0034 | g_im= 0.0000 +/- 0.0000 | g_im= 0.0273 +/- 0.0052 |

```



## 2 Unphysical Parameterizations

```

corr= [ 0.61] | corr= [ 0.59] | corr= [ 0.92] |
-----|-----|-----|
Br = 0.6436 +/- 0.0512 | Br = 0.0000 +/- 0.0000 | Br = 0.0736 +/- 0.0297 |

--
pi:omega[+] pi:phi[-] upper half-plane

sqrt(s)_pole = (0.24906 +/- 0.0022615)
               + (i/2)*(+0.051308 +/- 0.0041577) [ 0.30]

s_pole = (0.061373 +/- 0.0010996)
          + i*(+0.012779 +/- 0.0010756) [ 0.31]

=====|=====|
pi:omega | pi:phi |
=====|=====|
k_re= 0.0551 +/- 0.0023 | k_re= -0.0345 +/- 0.0025 |
k_im= 0.0262 +/- 0.0018 | k_im= -0.0374 +/- 0.0018 |
corr= [ 0.20] | corr= [ 0.01] |

=====|=====|
pi:omega/3^S_1(*) | pi:phi/3^S_1 | pi:omega/3^D_1 |
=====|=====|=====|
|g|= 0.1424 +/- 0.0042 | |g|= 0.0000 +/- 0.0000 | |g|= 0.0481 +/- 0.0084 |
arg(g)/pi= -0.2299 +/- 0.0047 | arg(g)/pi= 0.7299 +/- 0.0047 | arg(g)/pi= -0.1920 +/- 0.0114 |
-----|-----|-----|
g_re= 0.1069 +/- 0.0033 | g_re= -0.0000 +/- 0.0000 | g_re= 0.0397 +/- 0.0068 |
g_im= -0.0942 +/- 0.0034 | g_im= 0.0000 +/- 0.0000 | g_im= -0.0273 +/- 0.0052 |
corr= [-0.61] | corr= [-0.59] | corr= [-0.92] |
-----|-----|-----|
Br = 0.6436 +/- 0.0512 | Br = 0.0000 +/- 0.0000 | Br = 0.0736 +/- 0.0297 |

--
pi:omega[-] pi:phi[+] upper half-plane

sqrt(s)_pole = (0.27187 +/- 0.010718)
               + (i/2)*(+0.23965 +/- 0.065039) [ 0.91]

s_pole = (0.059554 +/- 0.0035152)
          + i*(+0.065154 +/- 0.020045) [-0.68]

=====|=====|
pi:omega | pi:phi |
=====|=====|
k_re= -0.0914 +/- 0.0114 | k_re= 0.0797 +/- 0.0128 |
k_im= -0.0848 +/- 0.0171 | k_im= 0.0923 +/- 0.0168 |
corr= [ 0.96] | corr= [ 0.97] |

=====|=====|
pi:omega/3^S_1 | pi:phi/3^S_1 | pi:omega/3^D_1(*) |
=====|=====|=====|
|g|= 0.0573 +/- 0.0069 | |g|= 0.0000 +/- 0.0000 | |g|= 0.1817 +/- 0.0206 |
arg(g)/pi= 0.5491 +/- 0.0322 | arg(g)/pi= 0.9684 +/- 0.0329 | arg(g)/pi= -0.4684 +/- 0.0329 |
-----|-----|-----|
g_re= -0.0088 +/- 0.0055 | g_re= -0.0000 +/- 0.0000 | g_re= 0.0180 +/- 0.0207 |
g_im= 0.0566 +/- 0.0071 | g_im= 0.0000 +/- 0.0000 | g_im= -0.1808 +/- 0.0186 |
corr= [ 0.21] | corr= [ 1.00] | corr= [-1.00] |
-----|-----|-----|
Br = 0.0267 +/- 0.0125 | Br = 0.0000 +/- 0.0000 | Br = 0.2689 +/- 0.0318 |

--
pi:omega[-] pi:phi[+] lower half-plane

sqrt(s)_pole = (0.27187 +/- 0.010718)
               + (i/2)*(-0.23965 +/- 0.065039) [-0.91]

s_pole = (0.059554 +/- 0.0035152)

```



## 2 Unphysical Parameterizations

+ i\*(-0.065154 +/- 0.020045) [ 0.68]

| pi:omega                      |                              | pi:phi          |  |
|-------------------------------|------------------------------|-----------------|--|
| =====                         |                              | =====           |  |
| k_re= 0.0914 +/- 0.0114       | k_re= -0.0797 +/- 0.0128     |                 |  |
| k_im= -0.0848 +/- 0.0171      | k_im= 0.0923 +/- 0.0168      |                 |  |
| corr= [-0.96]                 | corr= [-0.97]                |                 |  |
| -----                         |                              | -----           |  |
| pi:omega/3^S_1                |                              | pi:phi/3^S_1    |  |
| =====                         |                              | =====           |  |
| g = 0.0573 +/- 0.0069         | g = 0.0000 +/- 0.0000        |                 |  |
| arg(g)/pi= -0.5491 +/- 0.0322 | arg(g)/pi= 0.0316 +/- 0.0329 |                 |  |
| -----                         |                              | -----           |  |
| g_re= -0.0088 +/- 0.0055      | g_re= 0.0000 +/- 0.0000      |                 |  |
| g_im= -0.0566 +/- 0.0071      | g_im= 0.0000 +/- 0.0000      |                 |  |
| corr= [-0.21]                 | corr= [-1.00]                |                 |  |
| -----                         |                              | -----           |  |
| Br = 0.0267 +/- 0.0125        | Br = 0.0000 +/- 0.0000       |                 |  |
| -----                         |                              | -----           |  |
| pi:omega/3^D_1(*)             |                              | pi:phi/3^D_1(*) |  |
| =====                         |                              | =====           |  |
| g = 0.1817 +/- 0.0206         | g = 0.1817 +/- 0.0206        |                 |  |
| arg(g)/pi= 0.4684 +/- 0.0329  | arg(g)/pi= 0.4684 +/- 0.0329 |                 |  |
| -----                         |                              | -----           |  |
| g_re= 0.0180 +/- 0.0207       | g_re= 0.0180 +/- 0.0207      |                 |  |
| g_im= 0.1808 +/- 0.0186       | g_im= 0.1808 +/- 0.0186      |                 |  |
| corr= [ 1.00]                 | corr= [ 1.00]                |                 |  |
| -----                         |                              | -----           |  |
| Br = 0.2689 +/- 0.0318        | Br = 0.2689 +/- 0.0318       |                 |  |
| -----                         |                              | -----           |  |

--

pi:omega[-] pi:phi[+] lower half-plane

sqrt(s)\_pole = (0.20196 +/- 0.0015008)  
+ (i/2)\*(-8.0085e-17 +/- 4.9859e-14) [ 0.00]

s\_pole = (0.040788 +/- 0.00060621)  
+ i\*(-1.6183e-17 +/- 1.0071e-14) [ 0.00]

| pi:omega                     |                              | pi:phi                       |  |                |  |
|------------------------------|------------------------------|------------------------------|--|----------------|--|
| =====                        |                              | =====                        |  |                |  |
| k_re= 0.0000 +/- 0.0000      | k_re= -0.0000 +/- 0.0000     |                              |  |                |  |
| k_im= -0.0443 +/- 0.0013     | k_im= 0.0607 +/- 0.0007      |                              |  |                |  |
| corr= [ 0.00]                | corr= [ 0.00]                |                              |  |                |  |
| -----                        |                              |                              |  |                |  |
| pi:omega/3^S_1(*)            |                              | pi:phi/3^S_1                 |  | pi:omega/3^D_1 |  |
| =====                        |                              | =====                        |  | =====          |  |
| g = 0.1067 +/- 0.0037        | g = 0.0000 +/- 0.0000        | g = 0.0251 +/- 0.0056        |  |                |  |
| arg(g)/pi= 0.5000 +/- 0.0000 | arg(g)/pi= 0.0000 +/- 0.0000 | arg(g)/pi= 0.5000 +/- 0.0000 |  |                |  |
| -----                        |                              | -----                        |  | -----          |  |
| g_re= 0.0000 +/- 0.0000      | g_re= 0.0000 +/- 0.0000      | g_re= 0.0000 +/- 0.0000      |  |                |  |
| g_im= 0.1067 +/- 0.0037      | g_im= 0.0000 +/- 0.0000      | g_im= 0.0251 +/- 0.0056      |  |                |  |
| corr= [-1.00]                | corr= [ 0.00]                | corr= [-0.25]                |  |                |  |
| -----                        |                              | -----                        |  | -----          |  |
| Br = 0.0000 +/- 0.0000       | Br = 0.0000 +/- 0.0000       | Br = 0.0000 +/- 0.0000       |  |                |  |
| -----                        |                              | -----                        |  | -----          |  |

--

pi:omega[-] pi:phi[+] upper half-plane

sqrt(s)\_pole = (0.24619 +/- 0.00099068)  
+ (i/2)\*(+0.0049357 +/- 0.0015516) [-0.84]

s\_pole = (0.060604 +/- 0.00049103)  
+ i\*(+0.0012151 +/- 0.00037787) [-0.84]

| pi:omega                 |                         | pi:phi       |  |
|--------------------------|-------------------------|--------------|--|
| =====                    |                         | =====        |  |
| k_re= -0.0474 +/- 0.0011 | k_re= 0.0071 +/- 0.0011 |              |  |
| k_im= -0.0029 +/- 0.0009 | k_im= 0.0169 +/- 0.0032 |              |  |
| corr= [-0.85]            | corr= [ 0.58]           |              |  |
| -----                    |                         | -----        |  |
| pi:omega/3^S_1(*)        |                         | pi:phi/3^S_1 |  |
| =====                    |                         | =====        |  |
| -----                    |                         | -----        |  |
| pi:omega/3^D_1           |                         | pi:phi/3^D_1 |  |
| =====                    |                         | =====        |  |
| -----                    |                         | -----        |  |



## 2 Unphysical Parameterizations

|                                     |                                     |                                      |
|-------------------------------------|-------------------------------------|--------------------------------------|
| $ g  = 0.0497 \pm 0.0101$           | $ g  = 0.0000 \pm 0.0000$           | $ g  = 0.0181 \pm 0.0092$            |
| $\arg(g)/\pi = 0.1332 \pm 0.0210$   | $\arg(g)/\pi = 0.3668 \pm 0.0210$   | $\arg(g)/\pi = 0.8829 \pm 0.0886$    |
| $g_{\text{re}} = 0.0454 \pm 0.0088$ | $g_{\text{re}} = 0.0000 \pm 0.0000$ | $g_{\text{re}} = -0.0169 \pm 0.0102$ |
| $g_{\text{im}} = 0.0202 \pm 0.0060$ | $g_{\text{im}} = 0.0000 \pm 0.0000$ | $g_{\text{im}} = 0.0065 \pm 0.0023$  |
| $\text{corr} = [0.82]$              | $\text{corr} = [0.64]$              | $\text{corr} = [0.48]$               |
| $\text{Br} = 0.7811 \pm 0.0866$     | $\text{Br} = 0.0000 \pm 0.0000$     | $\text{Br} = 0.1035 \pm 0.1330$      |

--

pi:omega[-] pi:phi[+] lower half-plane

$\text{sqrt}(s)_{\text{pole}} = (0.24619 \pm 0.00099068)$   
 $+ (i/2)*(-0.0049357 \pm 0.0015516) [0.84]$

$s_{\text{pole}} = (0.060604 \pm 0.00049103)$   
 $+ i*(-0.0012151 \pm 0.00037787) [0.84]$

| pi:omega                             | pi:phi                               |
|--------------------------------------|--------------------------------------|
| $k_{\text{re}} = 0.0474 \pm 0.0011$  | $k_{\text{re}} = -0.0071 \pm 0.0011$ |
| $k_{\text{im}} = -0.0029 \pm 0.0009$ | $k_{\text{im}} = 0.0169 \pm 0.0032$  |
| $\text{corr} = [0.85]$               | $\text{corr} = [-0.58]$              |

| pi:omega/3 <sup>S</sup> _1(*)        | pi:phi/3 <sup>S</sup> _1             | pi:omega/3 <sup>D</sup> _1           |
|--------------------------------------|--------------------------------------|--------------------------------------|
| $ g  = 0.0497 \pm 0.0101$            | $ g  = 0.0000 \pm 0.0000$            | $ g  = 0.0181 \pm 0.0092$            |
| $\arg(g)/\pi = -0.1332 \pm 0.0210$   | $\arg(g)/\pi = 0.6332 \pm 0.0210$    | $\arg(g)/\pi = -0.8829 \pm 0.0886$   |
| $g_{\text{re}} = 0.0454 \pm 0.0088$  | $g_{\text{re}} = -0.0000 \pm 0.0000$ | $g_{\text{re}} = -0.0169 \pm 0.0102$ |
| $g_{\text{im}} = -0.0202 \pm 0.0060$ | $g_{\text{im}} = 0.0000 \pm 0.0000$  | $g_{\text{im}} = -0.0065 \pm 0.0023$ |
| $\text{corr} = [-0.82]$              | $\text{corr} = [-0.64]$              | $\text{corr} = [-0.48]$              |
| $\text{Br} = 0.7811 \pm 0.0866$      | $\text{Br} = 0.0000 \pm 0.0000$      | $\text{Br} = 0.1035 \pm 0.1330$      |

--

pi:omega[-] pi:phi[-] upper half-plane

$\text{sqrt}(s)_{\text{pole}} = (0.27187 \pm 0.010718)$   
 $+ (i/2)*(+0.23965 \pm 0.065039) [0.91]$

$s_{\text{pole}} = (0.059554 \pm 0.0035152)$   
 $+ i*(+0.065154 \pm 0.020045) [-0.68]$

| pi:omega                             | pi:phi                               |
|--------------------------------------|--------------------------------------|
| $k_{\text{re}} = -0.0914 \pm 0.0114$ | $k_{\text{re}} = -0.0797 \pm 0.0128$ |
| $k_{\text{im}} = -0.0848 \pm 0.0171$ | $k_{\text{im}} = -0.0923 \pm 0.0168$ |
| $\text{corr} = [0.96]$               | $\text{corr} = [0.97]$               |

| pi:omega/3 <sup>S</sup> _1           | pi:phi/3 <sup>S</sup> _1             | pi:omega/3 <sup>D</sup> _1(*)        |
|--------------------------------------|--------------------------------------|--------------------------------------|
| $ g  = 0.0573 \pm 0.0069$            | $ g  = 0.0000 \pm 0.0000$            | $ g  = 0.1817 \pm 0.0206$            |
| $\arg(g)/\pi = 0.5491 \pm 0.0322$    | $\arg(g)/\pi = 0.9684 \pm 0.0329$    | $\arg(g)/\pi = -0.4684 \pm 0.0329$   |
| $g_{\text{re}} = -0.0088 \pm 0.0055$ | $g_{\text{re}} = -0.0000 \pm 0.0000$ | $g_{\text{re}} = 0.0180 \pm 0.0207$  |
| $g_{\text{im}} = 0.0566 \pm 0.0071$  | $g_{\text{im}} = 0.0000 \pm 0.0000$  | $g_{\text{im}} = -0.1808 \pm 0.0186$ |
| $\text{corr} = [0.21]$               | $\text{corr} = [1.00]$               | $\text{corr} = [-1.00]$              |
| $\text{Br} = 0.0267 \pm 0.0125$      | $\text{Br} = 0.0000 \pm 0.0000$      | $\text{Br} = 0.2689 \pm 0.0318$      |

--

pi:omega[-] pi:phi[-] upper half-plane



## 2 Unphysical Parameterizations

```
sqrt(s)_pole = (0.24619 +/- 0.00099068)
               + (i/2)*(+0.0049357 +/- 0.0015516) [-0.84]
```

```
s_pole = (0.060604 +/- 0.00049103)
          + i*(+0.0012151 +/- 0.00037787) [-0.84]
```

| pi:omega                 | pi:phi                   |
|--------------------------|--------------------------|
| k_re= -0.0474 +/- 0.0011 | k_re= -0.0071 +/- 0.0011 |
| k_im= -0.0029 +/- 0.0009 | k_im= -0.0169 +/- 0.0032 |
| corr= [-0.85]            | corr= [ 0.58]            |

| pi:omega/3^S_1(*)            | pi:phi/3^S_1                 | pi:omega/3^D_1               |
|------------------------------|------------------------------|------------------------------|
| g = 0.0497 +/- 0.0101        | g = 0.0000 +/- 0.0000        | g = 0.0181 +/- 0.0092        |
| arg(g)/pi= 0.1332 +/- 0.0210 | arg(g)/pi= 0.3668 +/- 0.0210 | arg(g)/pi= 0.8829 +/- 0.0886 |
| g_re= 0.0454 +/- 0.0088      | g_re= 0.0000 +/- 0.0000      | g_re= -0.0169 +/- 0.0102     |
| g_im= 0.0202 +/- 0.0060      | g_im= 0.0000 +/- 0.0000      | g_im= 0.0065 +/- 0.0023      |
| corr= [ 0.82]                | corr= [ 0.64]                | corr= [ 0.48]                |
| Br = 0.7811 +/- 0.0866       | Br = 0.0000 +/- 0.0000       | Br = 0.1035 +/- 0.1330       |

```
--
pi:omega[-] pi:phi[-] upper half-plane
```

```
sqrt(s)_pole = (0.20196 +/- 0.0015008)
               + (i/2)*(+4.3632e-15 +/- 2.1641e-12) [ 0.00]
```

```
s_pole = (0.040788 +/- 0.00060621)
          + i*(+8.8134e-16 +/- 4.3713e-13) [ 0.00]
```

| pi:omega                 | pi:phi                   |
|--------------------------|--------------------------|
| k_re= -0.0000 +/- 0.0000 | k_re= -0.0000 +/- 0.0000 |
| k_im= -0.0443 +/- 0.0013 | k_im= -0.0607 +/- 0.0007 |
| corr= [ 0.00]            | corr= [ 0.00]            |

| pi:omega/3^S_1(*)            | pi:phi/3^S_1                 | pi:omega/3^D_1               |
|------------------------------|------------------------------|------------------------------|
| g = 0.1067 +/- 0.0037        | g = 0.0000 +/- 0.0000        | g = 0.0251 +/- 0.0056        |
| arg(g)/pi= 0.5000 +/- 0.0000 | arg(g)/pi= 0.0000 +/- 0.0000 | arg(g)/pi= 0.5000 +/- 0.0000 |
| g_re= 0.0000 +/- 0.0000      | g_re= 0.0000 +/- 0.0000      | g_re= 0.0000 +/- 0.0000      |
| g_im= 0.1067 +/- 0.0037      | g_im= 0.0000 +/- 0.0000      | g_im= 0.0251 +/- 0.0056      |
| corr= [-1.00]                | corr= [ 0.00]                | corr= [-0.25]                |
| Br = 0.0000 +/- 0.0000       | Br = 0.0000 +/- 0.0000       | Br = 0.0000 +/- 0.0000       |

```
--
pi:omega[-] pi:phi[-] lower half-plane
```

```
sqrt(s)_pole = (0.27187 +/- 0.010718)
               + (i/2)*(-0.23965 +/- 0.065039) [-0.91]
```

```
s_pole = (0.059554 +/- 0.0035152)
          + i*(-0.065154 +/- 0.020045) [ 0.68]
```

| pi:omega                 | pi:phi                   |
|--------------------------|--------------------------|
| k_re= 0.0914 +/- 0.0114  | k_re= 0.0797 +/- 0.0128  |
| k_im= -0.0848 +/- 0.0171 | k_im= -0.0923 +/- 0.0168 |



## 2 Unphysical Parameterizations

```

corr= [-0.96] | corr= [-0.97] |

===== pi:omega/3^S_1 | pi:phi/3^S_1 | pi:omega/3^D_1(*) |
=====
|g|= 0.0573 +/- 0.0069 | |g|= 0.0000 +/- 0.0000 | |g|= 0.1817 +/- 0.0206 |
arg(g)/pi= -0.5491 +/- 0.0322 | arg(g)/pi= 0.0316 +/- 0.0329 | arg(g)/pi= 0.4684 +/- 0.0329 |
-----
g_re= -0.0088 +/- 0.0055 | g_re= 0.0000 +/- 0.0000 | g_re= 0.0180 +/- 0.0207 |
g_im= -0.0566 +/- 0.0071 | g_im= 0.0000 +/- 0.0000 | g_im= 0.1808 +/- 0.0186 |
corr= [-0.21] | corr= [-1.00] | corr= [ 1.00] |
-----
Br = 0.0267 +/- 0.0125 | Br = 0.0000 +/- 0.0000 | Br = 0.2689 +/- 0.0318 |

--
pi:omega[-] pi:phi[-] lower half-plane

sqrt(s)_pole = (0.24619 +/- 0.00099068)
+ (i/2)*(-0.0049357 +/- 0.0015516) [ 0.84]

s_pole = (0.060604 +/- 0.00049103)
+ i*(-0.0012151 +/- 0.00037787) [ 0.84]

===== pi:omega | pi:phi |
=====
k_re= 0.0474 +/- 0.0011 | k_re= 0.0071 +/- 0.0011 |
k_im= -0.0029 +/- 0.0009 | k_im= -0.0169 +/- 0.0032 |
corr= [ 0.85] | corr= [-0.58] |

===== pi:omega/3^S_1(*) | pi:phi/3^S_1 | pi:omega/3^D_1 |
=====
|g|= 0.0497 +/- 0.0101 | |g|= 0.0000 +/- 0.0000 | |g|= 0.0181 +/- 0.0092 |
arg(g)/pi= -0.1332 +/- 0.0210 | arg(g)/pi= 0.6332 +/- 0.0210 | arg(g)/pi= -0.8829 +/- 0.0886 |
-----
g_re= 0.0454 +/- 0.0088 | g_re= -0.0000 +/- 0.0000 | g_re= -0.0169 +/- 0.0102 |
g_im= -0.0202 +/- 0.0060 | g_im= 0.0000 +/- 0.0000 | g_im= -0.0065 +/- 0.0023 |
corr= [-0.82] | corr= [-0.64] | corr= [-0.48] |
-----
Br = 0.7811 +/- 0.0866 | Br = 0.0000 +/- 0.0000 | Br = 0.1035 +/- 0.1330 |

```



## 2.12 coupled\_po\_pp.3s1\_3d1.pole+G0\_3s1\_3sd1\_3S1+G1\_3s1.gorder0\_3s1\_3S1.irho

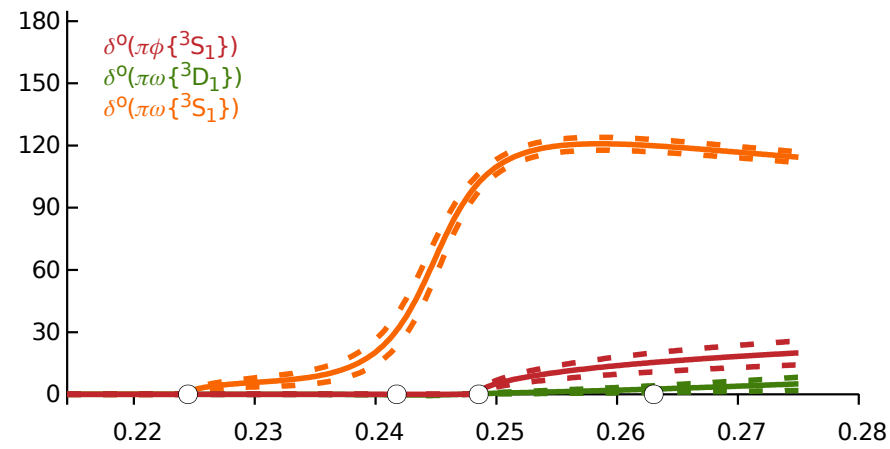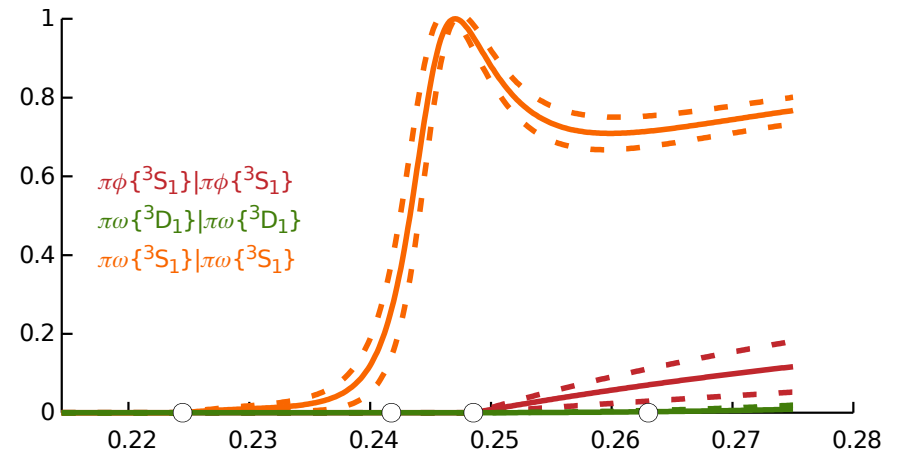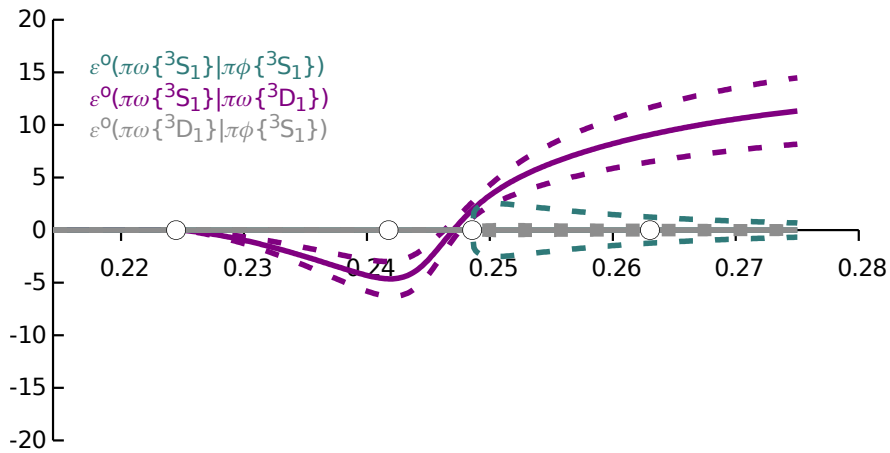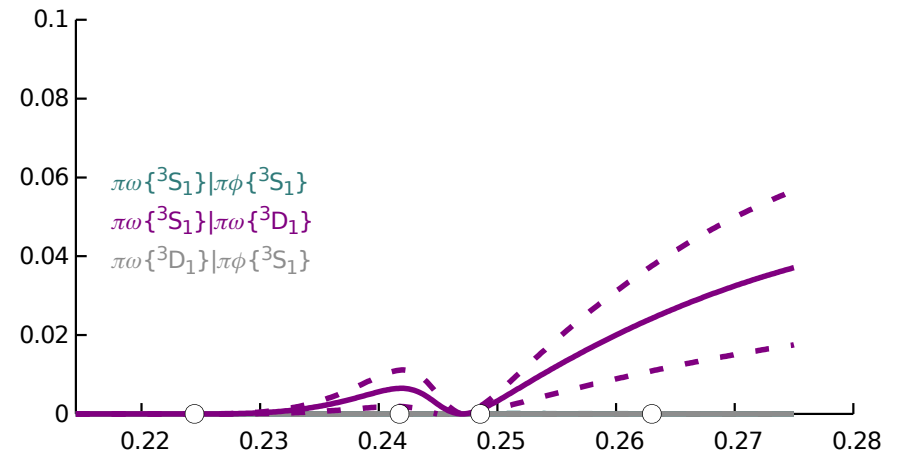



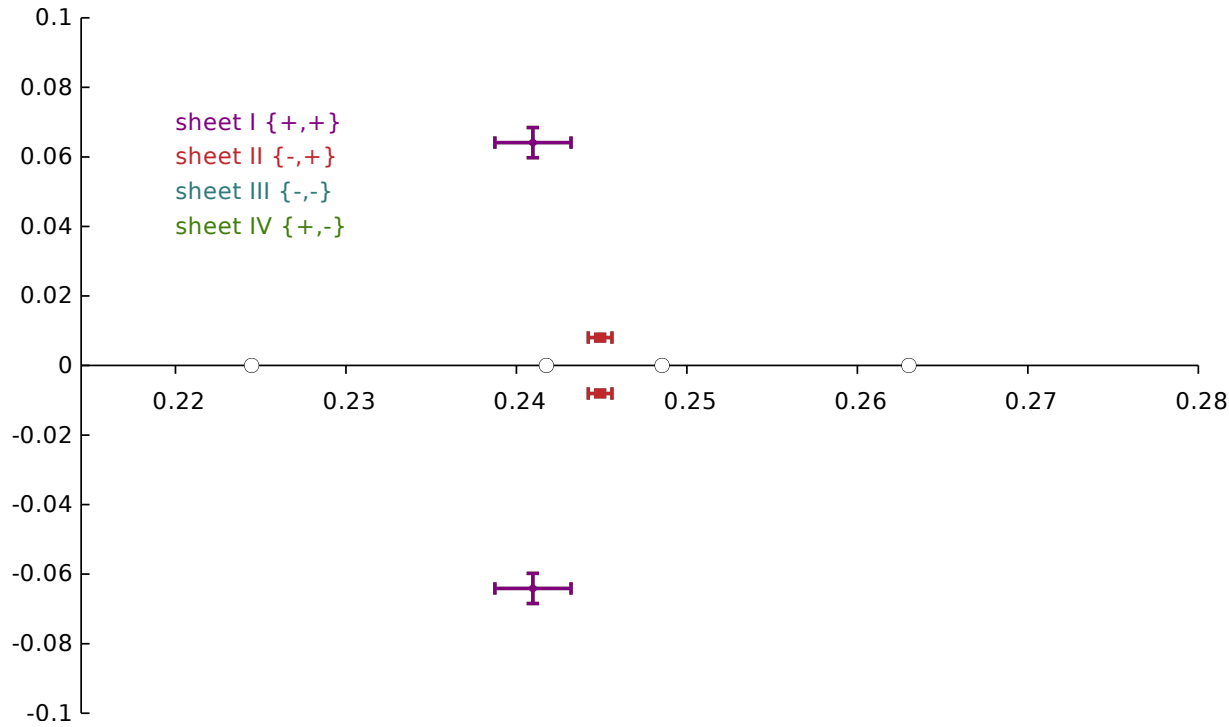

### parameter values

minimised with  $\text{chisq}/\text{nDoF} = 33.27 / (36 - 7) = 1.15$

|                                               |  |                         |  |      |       |       |       |       |       |       |
|-----------------------------------------------|--|-------------------------|--|------|-------|-------|-------|-------|-------|-------|
| JP1+_g_pi:omega/3^S_1_pole0                   |  | 0.086324 +/- 0.0061901  |  | 1.00 | -0.01 | -0.25 | -0.17 | -0.02 | 0.01  | -0.11 |
| JP1+_g_pi:phi/3^S_1_pole0                     |  | 2.7768e-06 +/- 0.011352 |  |      | 1.00  | 0.01  | 0.00  | 0.00  | -0.00 | -0.04 |
| JP1+_gamma_pi:omega/3^S_1 pi:omega/3^D_1_orde |  | -38.748 +/- 12.701      |  |      |       | 1.00  | -0.20 | 0.34  | -0.11 | -0.14 |
| JP1+_gamma_pi:omega/3^S_1 pi:omega/3^S_1_orde |  | 6.6946 +/- 0.6193       |  |      |       |       | 1.00  | -0.95 | 0.00  | 0.02  |
| JP1+_gamma_pi:omega/3^S_1 pi:omega/3^S_1_orde |  | -134.47 +/- 12.322      |  |      |       |       |       | 1.00  | 0.04  | -0.03 |
| JP1+_gamma_pi:phi/3^S_1 pi:phi/3^S_1_order0   |  | 0.92768 +/- 0.28228     |  |      |       |       |       |       | 1.00  | -0.26 |
| JP1+_m_pole0                                  |  | 0.24703 +/- 0.00058788  |  |      |       |       |       |       |       | 1.00  |

### pole singularities

pi:omega[+] pi:phi[+] upper half-plane

$\text{sqrt}(s)_{\text{pole}} = (0.24097 \pm 0.0022381) + (i/2) * (0.06412 \pm 0.0043147) [0.60]$

$s_{\text{pole}} = (0.05704 \pm 0.0010018) + i * (0.015451 \pm 0.0011316) [0.59]$

| pi:omega                |  | pi:phi                  |  |
|-------------------------|--|-------------------------|--|
| k_re= 0.0501 +/- 0.0024 |  | k_re= 0.0323 +/- 0.0024 |  |
| k_im= 0.0344 +/- 0.0015 |  | k_im= 0.0469 +/- 0.0012 |  |



## 2 Unphysical Parameterizations

```

corr= [ 0.43]          |      corr= [ 0.08]          |
=====|=====|=====
      pi:omega/3^S_1(*) |      pi:phi/3^S_1 |      pi:omega/3^D_1 |
=====|=====|=====
      |g|= 0.1302 +/- 0.0045 |      |g|= 0.0001 +/- 0.0017 |      |g|= 0.0373 +/- 0.0089 |
arg(g)/pi= -0.1313 +/- 0.0041 | arg(g)/pi= -0.4801 +/- 11.2960 | arg(g)/pi= -0.0997 +/- 0.0178 |
-----|-----|-----
      g_re= 0.1193 +/- 0.0045 |      g_re= -0.0000 +/- 0.0029 |      g_re= 0.0355 +/- 0.0087 |
      g_im= -0.0522 +/- 0.0015 |      g_im= -0.0000 +/- 0.0001 |      g_im= -0.0115 +/- 0.0029 |
      corr= [-0.47]          |      corr= [ 0.97]          |      corr= [-0.71]          |
-----|-----|-----
      Br = 0.3733 +/- 0.0185 |      Br = 0.0000 +/- 0.0000 |      Br = 0.0306 +/- 0.0158 |

--
pi:omega[+] pi:phi[+] lower half-plane

sqrt(s)_pole = (0.24097 +/- 0.0022381)
               + (i/2)*(-0.06412 +/- 0.0043147) [-0.60]

s_pole = (0.05704 +/- 0.0010018)
         + i*(-0.015451 +/- 0.0011316) [-0.59]

      pi:omega |      pi:phi |
=====|=====|
      k_re= -0.0501 +/- 0.0024 |      k_re= -0.0323 +/- 0.0024 |
      k_im= 0.0344 +/- 0.0015 |      k_im= 0.0469 +/- 0.0012 |
      corr= [-0.43]          |      corr= [-0.08]          |

      pi:omega/3^S_1(*) |      pi:phi/3^S_1 |      pi:omega/3^D_1 |
=====|=====|=====
      |g|= 0.1302 +/- 0.0045 |      |g|= 0.0001 +/- 0.0017 |      |g|= 0.0373 +/- 0.0089 |
arg(g)/pi= 0.1313 +/- 0.0041 | arg(g)/pi= 0.4857 +/- 11.1438 | arg(g)/pi= 0.0997 +/- 0.0178 |
-----|-----|-----
      g_re= 0.1193 +/- 0.0045 |      g_re= -0.0000 +/- 0.0029 |      g_re= 0.0355 +/- 0.0087 |
      g_im= 0.0522 +/- 0.0015 |      g_im= 0.0000 +/- 0.0001 |      g_im= 0.0115 +/- 0.0029 |
      corr= [ 0.47]          |      corr= [-0.97]          |      corr= [ 0.71]          |
-----|-----|-----
      Br = 0.3733 +/- 0.0185 |      Br = 0.0000 +/- 0.0000 |      Br = 0.0306 +/- 0.0158 |

--
pi:omega[+] pi:phi[-] upper half-plane

sqrt(s)_pole = (0.24097 +/- 0.0022381)
               + (i/2)*(+0.06412 +/- 0.0043148) [ 0.60]

s_pole = (0.05704 +/- 0.0010018)
         + i*(+0.015451 +/- 0.0011316) [ 0.59]

      pi:omega |      pi:phi |
=====|=====|
      k_re= 0.0501 +/- 0.0024 |      k_re= -0.0323 +/- 0.0024 |
      k_im= 0.0344 +/- 0.0015 |      k_im= -0.0469 +/- 0.0012 |
      corr= [ 0.43]          |      corr= [ 0.08]          |

      pi:omega/3^S_1(*) |      pi:phi/3^S_1 |      pi:omega/3^D_1 |
=====|=====|=====
      |g|= 0.1302 +/- 0.0045 |      |g|= 0.0002 +/- 0.0032 |      |g|= 0.0373 +/- 0.0089 |
arg(g)/pi= -0.1313 +/- 0.0041 | arg(g)/pi= 0.3022 +/- 11.1691 | arg(g)/pi= -0.0997 +/- 0.0178 |
-----|-----|-----
      g_re= 0.1193 +/- 0.0045 |      g_re= -0.0000 +/- 0.0044 |      g_re= 0.0355 +/- 0.0087 |
      g_im= -0.0522 +/- 0.0015 |      g_im= 0.0000 +/- 0.0030 |      g_im= -0.0115 +/- 0.0029 |
      corr= [-0.47]          |      corr= [-1.00]          |      corr= [-0.71]          |

```



## 2 Unphysical Parameterizations

```

-----|-----|-----|
      Br =  0.3733 +/- 0.0186 |      Br =  0.0000 +/- 0.0000 |      Br =  0.0306 +/- 0.0158 |

--
pi:omega[+] pi:phi[-] lower half-plane

sqrt(s)_pole = (0.24097 +/- 0.0022381)
               + (i/2)*(-0.06412 +/- 0.0043148) [-0.60]

s_pole = (0.05704 +/- 0.0010018)
         + i*(-0.015451 +/- 0.0011316) [-0.59]

=====|=====|
      pi:omega |      pi:phi |
=====|=====|
      k_re= -0.0501 +/- 0.0024 |      k_re=  0.0323 +/- 0.0024 |
      k_im=  0.0344 +/- 0.0015 |      k_im= -0.0469 +/- 0.0012 |
      corr= [-0.43]           |      corr= [-0.08]           |

=====|=====|=====|
      pi:omega/3^S_1(*) |      pi:phi/3^S_1 |      pi:omega/3^D_1 |
=====|=====|=====|
      |g|=  0.1302 +/- 0.0045 |      |g|=  0.0002 +/- 0.0032 |      |g|=  0.0373 +/- 0.0089 |
arg(g)/pi= 0.1313 +/- 0.0041 | arg(g)/pi= -0.3022 +/- 11.1691 | arg(g)/pi= 0.0997 +/- 0.0178 |
-----|-----|-----|
      g_re=  0.1193 +/- 0.0045 |      g_re= -0.0000 +/- 0.0044 |      g_re=  0.0355 +/- 0.0087 |
      g_im=  0.0522 +/- 0.0015 |      g_im= -0.0000 +/- 0.0030 |      g_im=  0.0115 +/- 0.0029 |
      corr= [ 0.47]           |      corr= [ 1.00]           |      corr= [ 0.71]           |
-----|-----|-----|
      Br =  0.3733 +/- 0.0186 |      Br =  0.0000 +/- 0.0000 |      Br =  0.0306 +/- 0.0158 |

--
pi:omega[-] pi:phi[+] upper half-plane

sqrt(s)_pole = (0.19527 +/- 0.0022414)
               + (i/2)*(+1.8478e-18 +/- 9.2366e-16) [ 0.00]

s_pole = (0.038131 +/- 0.00087534)
         + i*(+3.6061e-19 +/- 1.8026e-16) [ 0.00]

=====|=====|
      pi:omega |      pi:phi |
=====|=====|
      k_re= -0.0000 +/- 0.0000 |      k_re=  0.0000 +/- 0.0000 |
      k_im= -0.0496 +/- 0.0016 |      k_im=  0.0634 +/- 0.0008 |
      corr= [ 0.00]           |      corr= [ 0.00]           |

=====|=====|=====|
      pi:omega/3^S_1(*) |      pi:phi/3^S_1 |      pi:omega/3^D_1 |
=====|=====|=====|
      |g|=  0.1283 +/- 0.0047 |      |g|=  0.0001 +/- 0.0010 |      |g|=  0.0249 +/- 0.0079 |
arg(g)/pi= 0.5000 +/- 0.0000 | arg(g)/pi= -0.0073 +/- 11.0928 | arg(g)/pi= 0.5000 +/- 0.0000 |
-----|-----|-----|
      g_re=  0.0000 +/- 0.0000 |      g_re=  0.0000 +/- 0.0000 |      g_re=  0.0000 +/- 0.0000 |
      g_im=  0.1283 +/- 0.0047 |      g_im=  0.0000 +/- 0.0017 |      g_im=  0.0249 +/- 0.0079 |
      corr= [-1.00]           |      corr= [-0.26]           |      corr= [-0.35]           |
-----|-----|-----|
      Br =  0.0000 +/- 0.0000 |      Br =  0.0000 +/- 0.0000 |      Br =  0.0000 +/- 0.0000 |

--
pi:omega[-] pi:phi[+] upper half-plane

sqrt(s)_pole = (0.24491 +/- 0.00068982)
               + (i/2)*(+0.0080338 +/- 0.00094559) [-0.46]

s_pole = (0.059965 +/- 0.00033965)
         + i*(+0.0019676 +/- 0.0002291) [-0.45]

```



## 2 Unphysical Parameterizations

```

===== pi:omega | pi:phi |
k_re= -0.0460 +/- 0.0008 | k_re= 0.0092 +/- 0.0008 |
k_im= -0.0048 +/- 0.0006 | k_im= 0.0212 +/- 0.0016 |
corr= [-0.50] | corr= [-0.01] |

===== pi:omega/3^S_1(*) | pi:phi/3^S_1 | pi:omega/3^D_1 |
|g|= 0.0656 +/- 0.0036 | |g|= 0.0003 +/- 0.0055 | |g|= 0.0082 +/- 0.0027 |
arg(g)/pi= 0.1270 +/- 0.0172 | arg(g)/pi= -0.4881 +/- 11.1776 | arg(g)/pi= 0.7207 +/- 0.0189 |
-----
g_re= 0.0604 +/- 0.0040 | g_re= 0.0000 +/- 0.0092 | g_re= -0.0053 +/- 0.0020 |
g_im= 0.0255 +/- 0.0031 | g_im= 0.0000 +/- 0.0005 | g_im= 0.0063 +/- 0.0020 |
corr= [-0.21] | corr= [ 1.00] | corr= [-0.95] |
-----
Br = 0.8181 +/- 0.0155 | Br = 0.0000 +/- 0.0000 | Br = 0.0129 +/- 0.0086 |

--
pi:omega[-] pi:phi[+] lower half-plane

sqrt(s)_pole = (0.24491 +/- 0.00068982)
+ (i/2)*(-0.0080338 +/- 0.00094559) [ 0.46]

s_pole = (0.059965 +/- 0.00033965)
+ i*(-0.0019676 +/- 0.0002291) [ 0.45]

===== pi:omega | pi:phi |
k_re= 0.0460 +/- 0.0008 | k_re= -0.0092 +/- 0.0008 |
k_im= -0.0048 +/- 0.0006 | k_im= 0.0212 +/- 0.0016 |
corr= [ 0.50] | corr= [ 0.01] |

===== pi:omega/3^S_1(*) | pi:phi/3^S_1 | pi:omega/3^D_1 |
|g|= 0.0656 +/- 0.0036 | |g|= 0.0003 +/- 0.0055 | |g|= 0.0082 +/- 0.0027 |
arg(g)/pi= -0.1270 +/- 0.0172 | arg(g)/pi= 0.4900 +/- 11.1471 | arg(g)/pi= -0.7207 +/- 0.0189 |
-----
g_re= 0.0604 +/- 0.0040 | g_re= 0.0000 +/- 0.0092 | g_re= -0.0053 +/- 0.0020 |
g_im= -0.0255 +/- 0.0031 | g_im= -0.0000 +/- 0.0005 | g_im= -0.0063 +/- 0.0020 |
corr= [ 0.21] | corr= [-1.00] | corr= [ 0.95] |
-----
Br = 0.8181 +/- 0.0155 | Br = 0.0000 +/- 0.0000 | Br = 0.0129 +/- 0.0086 |

--
pi:omega[-] pi:phi[-] lower half-plane

sqrt(s)_pole = (0.19527 +/- 0.0022414)
+ (i/2)*(-2.1031e-15 +/- 1.0511e-12) [ 0.00]

s_pole = (0.038131 +/- 0.00087533)
+ i*(-4.1043e-16 +/- 2.0513e-13) [ 0.00]

===== pi:omega | pi:phi |
k_re= 0.0000 +/- 0.0000 | k_re= 0.0000 +/- 0.0000 |
k_im= -0.0496 +/- 0.0016 | k_im= -0.0634 +/- 0.0008 |
corr= [ 0.00] | corr= [ 0.00] |

===== pi:omega/3^S_1(*) | pi:phi/3^S_1 | pi:omega/3^D_1 |
|g|= 0.1283 +/- 0.0047 | |g|= 0.0002 +/- 0.0042 | |g|= 0.0249 +/- 0.0079 |

```



## 2 Unphysical Parameterizations

| arg(g)/pi= | 0.5000 +/- 0.0000 | arg(g)/pi= | -0.0066 +/- 11.1417 | arg(g)/pi= | 0.5000 +/- 0.0000 |
|------------|-------------------|------------|---------------------|------------|-------------------|
| g_re=      | 0.0000 +/- 0.0000 | g_re=      | 0.0000 +/- 0.0000   | g_re=      | 0.0000 +/- 0.0000 |
| g_im=      | 0.1283 +/- 0.0047 | g_im=      | 0.0000 +/- 0.0069   | g_im=      | 0.0249 +/- 0.0079 |
| corr=      | [-1.00]           | corr=      | [-0.64]             | corr=      | [-0.35]           |
| Br =       | 0.0000 +/- 0.0000 | Br =       | 0.0000 +/- 0.0000   | Br =       | 0.0000 +/- 0.0000 |

--

pi:omega[-] pi:phi[-] upper half-plane

sqrt(s)\_pole = (0.24491 +/- 0.00069007)  
+ (i/2)\*(+0.008034 +/- 0.00094594) [-0.46]

s\_pole = (0.059965 +/- 0.00033977)  
+ i\*(+0.0019676 +/- 0.00022918) [-0.45]

| pi:omega                 | pi:phi                   |
|--------------------------|--------------------------|
| k_re= -0.0460 +/- 0.0008 | k_re= -0.0092 +/- 0.0008 |
| k_im= -0.0048 +/- 0.0006 | k_im= -0.0212 +/- 0.0016 |
| corr= [-0.50]            | corr= [-0.01]            |

| pi:omega/3^S_1(*)            | pi:phi/3^S_1                  | pi:omega/3^D_1               |
|------------------------------|-------------------------------|------------------------------|
| g = 0.0656 +/- 0.0036        | g = 0.0005 +/- 0.0076         | g = 0.0082 +/- 0.0027        |
| arg(g)/pi= 0.1270 +/- 0.0172 | arg(g)/pi= 0.4768 +/- 11.1617 | arg(g)/pi= 0.7207 +/- 0.0189 |
| g_re= 0.0604 +/- 0.0040      | g_re= 0.0000 +/- 0.0126       | g_re= -0.0053 +/- 0.0020     |
| g_im= 0.0255 +/- 0.0031      | g_im= -0.0000 +/- 0.0012      | g_im= 0.0063 +/- 0.0020      |
| corr= [-0.21]                | corr= [-1.00]                 | corr= [-0.95]                |
| Br = 0.8181 +/- 0.0155       | Br = 0.0000 +/- 0.0000        | Br = 0.0129 +/- 0.0086       |

--

pi:omega[-] pi:phi[-] lower half-plane

sqrt(s)\_pole = (0.24491 +/- 0.00069007)  
+ (i/2)\*(-0.008034 +/- 0.00094594) [ 0.46]

s\_pole = (0.059965 +/- 0.00033977)  
+ i\*(-0.0019676 +/- 0.00022918) [ 0.45]

| pi:omega                 | pi:phi                   |
|--------------------------|--------------------------|
| k_re= 0.0460 +/- 0.0008  | k_re= 0.0092 +/- 0.0008  |
| k_im= -0.0048 +/- 0.0006 | k_im= -0.0212 +/- 0.0016 |
| corr= [ 0.50]            | corr= [ 0.01]            |

| pi:omega/3^S_1(*)             | pi:phi/3^S_1                   | pi:omega/3^D_1                |
|-------------------------------|--------------------------------|-------------------------------|
| g = 0.0656 +/- 0.0036         | g = 0.0005 +/- 0.0076          | g = 0.0082 +/- 0.0027         |
| arg(g)/pi= -0.1270 +/- 0.0172 | arg(g)/pi= -0.4753 +/- 11.2004 | arg(g)/pi= -0.7207 +/- 0.0189 |
| g_re= 0.0604 +/- 0.0040       | g_re= 0.0000 +/- 0.0126        | g_re= -0.0053 +/- 0.0020      |
| g_im= -0.0255 +/- 0.0031      | g_im= 0.0000 +/- 0.0012        | g_im= -0.0063 +/- 0.0020      |
| corr= [ 0.21]                 | corr= [ 1.00]                  | corr= [ 0.95]                 |
| Br = 0.8181 +/- 0.0155        | Br = 0.0000 +/- 0.0000         | Br = 0.0129 +/- 0.0086        |



## 2.13 coupled\_po\_pp.3s1\_3d1.pole+G0\_3s1\_3sd1\_3S1+G1\_3s1.gorder0\_3s1\_3S1.pole0\_sub

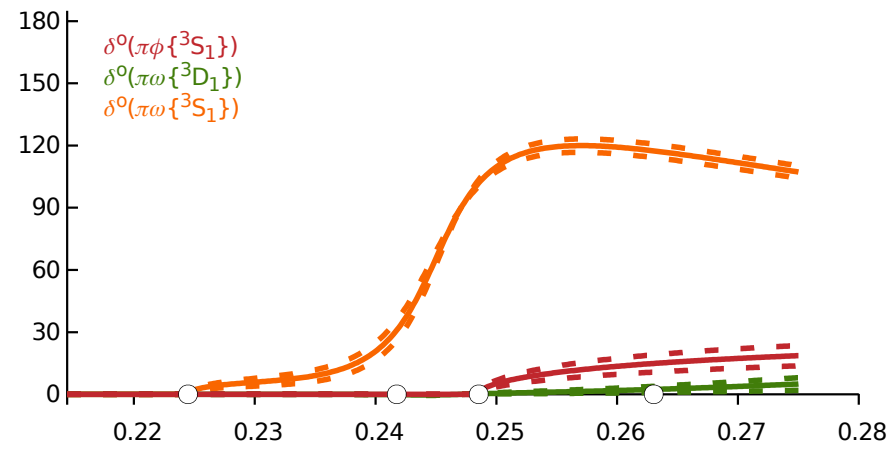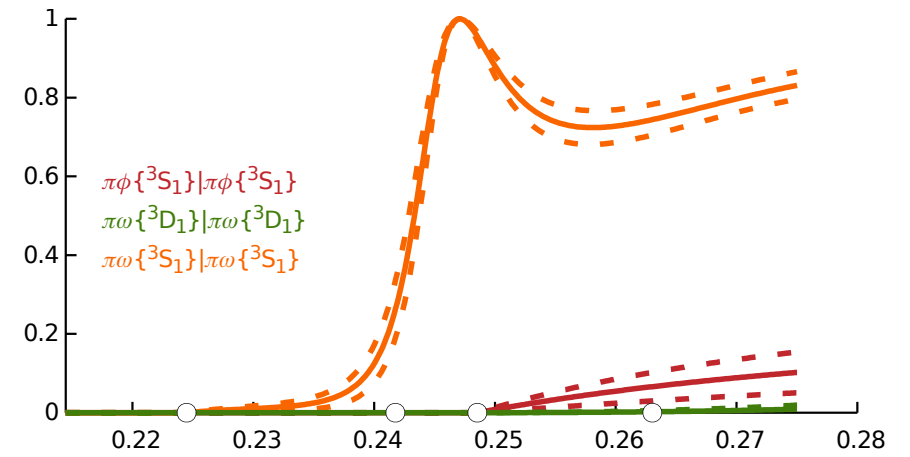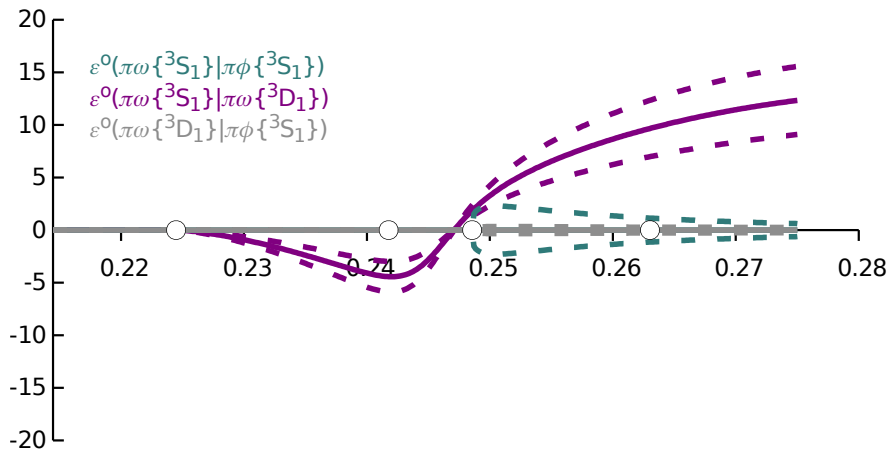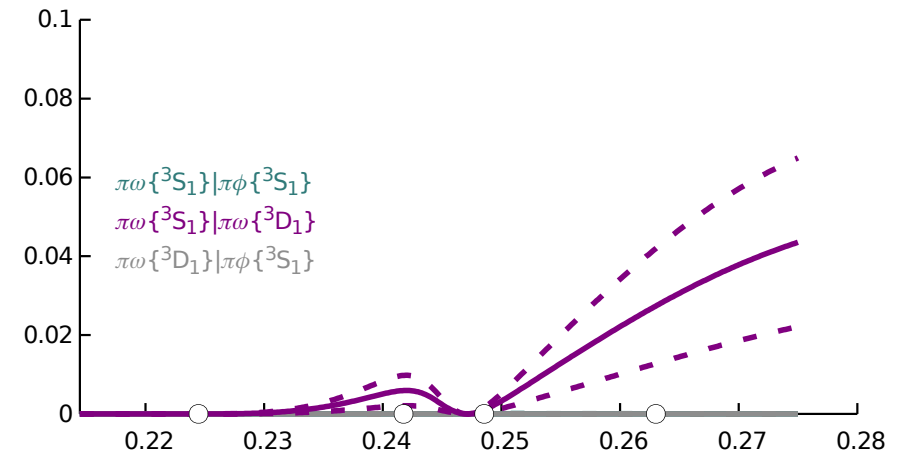



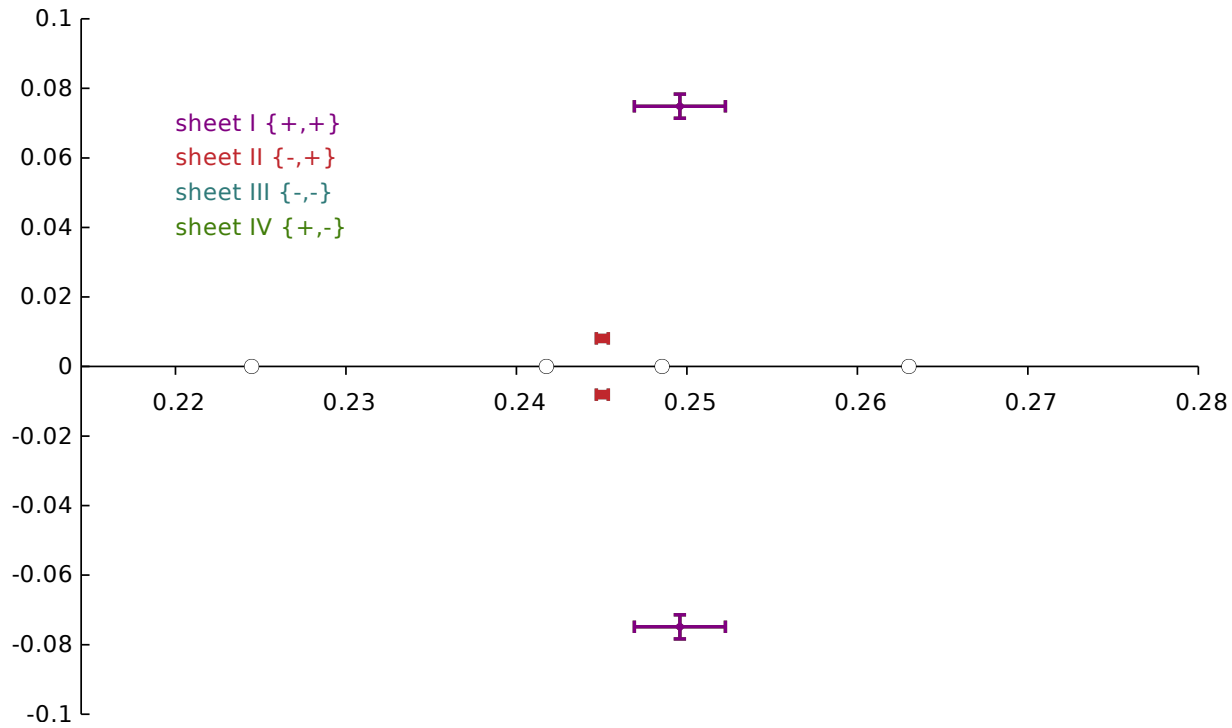

### parameter values

minimised with  $\text{chisq}/\text{nDoF} = 33.21 / (36 - 7) = 1.15$

|                                               |  |                          |  |      |       |       |       |       |       |       |
|-----------------------------------------------|--|--------------------------|--|------|-------|-------|-------|-------|-------|-------|
| JP1+_g_pi:omega/3^S_1_pole0                   |  | 0.083218 +/- 0.0054395   |  | 1.00 | -0.09 | -0.29 | -0.19 | -0.03 | -0.01 | -0.00 |
| JP1+_g_pi:phi/3^S_1_pole0                     |  | 6.9465e-07 +/- 0.0089728 |  |      | 1.00  | -0.00 | 0.01  | -0.01 | -0.05 | -0.00 |
| JP1+_gamma_pi:omega/3^S_1 pi:omega/3^D_1_orde |  | -35.607 +/- 11.282       |  |      |       | 1.00  | -0.12 | 0.30  | -0.15 | -0.00 |
| JP1+_gamma_pi:omega/3^S_1 pi:omega/3^S_1_orde |  | 5.7152 +/- 0.42929       |  |      |       |       | 1.00  | -0.92 | 0.01  | 0.00  |
| JP1+_gamma_pi:omega/3^S_1 pi:omega/3^S_1_orde |  | -114.88 +/- 8.5207       |  |      |       |       |       | 1.00  | 0.04  | -0.00 |
| JP1+_gamma_pi:phi/3^S_1 pi:phi/3^S_1_order0   |  | 0.86859 +/- 0.24167      |  |      |       |       |       |       | 1.00  | -0.01 |
| JP1+_m_pole0                                  |  | 0.24708 +/- 1.7509e-05   |  |      |       |       |       |       |       | 1.00  |

### pole singularities

pi:omega[+] pi:phi[+] upper half-plane

$\text{sqrt}(s)_{\text{pole}} = (0.24959 \pm 0.0026708) + (i/2) * (0.074858 \pm 0.0034639) [0.63]$

$s_{\text{pole}} = (0.060896 \pm 0.001255) + i * (0.018684 \pm 0.0010033) [0.69]$

|                         |  |                         |  |
|-------------------------|--|-------------------------|--|
| pi:omega                |  | pi:phi                  |  |
| =====                   |  | =====                   |  |
| k_re= 0.0589 +/- 0.0025 |  | k_re= 0.0412 +/- 0.0025 |  |
| k_im= 0.0360 +/- 0.0011 |  | k_im= 0.0462 +/- 0.0011 |  |



## 2 Unphysical Parameterizations

```

corr= [ 0.26]          |      corr= [-0.18]          |
=====|=====|=====
      pi:omega/3^S_1(*) |      pi:phi/3^S_1 |      pi:omega/3^D_1 |
=====|=====|=====
      |g|= 0.1651 +/- 0.0053 |      |g|= 0.0001 +/- 0.0013 |      |g|= 0.0472 +/- 0.0109 |
arg(g)/pi= -0.2075 +/- 0.0033 | arg(g)/pi= -0.4642 +/- 11.2075 | arg(g)/pi= -0.1669 +/- 0.0149 |
-----|-----|-----
      g_re= 0.1312 +/- 0.0040 |      g_re= -0.0000 +/- 0.0022 |      g_re= 0.0408 +/- 0.0098 |
      g_im= -0.1002 +/- 0.0039 |      g_im= -0.0000 +/- 0.0002 |      g_im= -0.0236 +/- 0.0052 |
      corr= [-0.84]          |      corr= [ 1.00]          |      corr= [-0.89]          |
-----|-----|-----
      Br = 0.5997 +/- 0.0229 |      Br = 0.0000 +/- 0.0000 |      Br = 0.0490 +/- 0.0243 |

--
pi:omega[+] pi:phi[+] lower half-plane

sqrt(s)_pole = (0.24959 +/- 0.0026708)
               + (i/2)*(-0.074858 +/- 0.0034639) [-0.63]

s_pole = (0.060896 +/- 0.001255)
         + i*(-0.018684 +/- 0.0010033) [-0.69]

      pi:omega |      pi:phi |
=====|=====|
      k_re= -0.0589 +/- 0.0025 |      k_re= -0.0412 +/- 0.0025 |
      k_im= 0.0360 +/- 0.0011 |      k_im= 0.0462 +/- 0.0011 |
      corr= [-0.26]          |      corr= [ 0.18]          |

      pi:omega/3^S_1(*) |      pi:phi/3^S_1 |      pi:omega/3^D_1 |
=====|=====|=====
      |g|= 0.1651 +/- 0.0053 |      |g|= 0.0001 +/- 0.0013 |      |g|= 0.0472 +/- 0.0109 |
arg(g)/pi= 0.2075 +/- 0.0033 | arg(g)/pi= 0.4658 +/- 11.1602 | arg(g)/pi= 0.1669 +/- 0.0149 |
-----|-----|-----
      g_re= 0.1312 +/- 0.0040 |      g_re= -0.0000 +/- 0.0022 |      g_re= 0.0408 +/- 0.0098 |
      g_im= 0.1002 +/- 0.0039 |      g_im= 0.0000 +/- 0.0002 |      g_im= 0.0236 +/- 0.0052 |
      corr= [ 0.84]          |      corr= [-1.00]          |      corr= [ 0.89]          |
-----|-----|-----
      Br = 0.5997 +/- 0.0229 |      Br = 0.0000 +/- 0.0000 |      Br = 0.0490 +/- 0.0243 |

--
pi:omega[+] pi:phi[-] lower half-plane

sqrt(s)_pole = (0.24959 +/- 0.0026708)
               + (i/2)*(-0.074858 +/- 0.0034639) [-0.63]

s_pole = (0.060896 +/- 0.001255)
         + i*(-0.018684 +/- 0.0010033) [-0.69]

      pi:omega |      pi:phi |
=====|=====|
      k_re= -0.0589 +/- 0.0025 |      k_re= 0.0412 +/- 0.0025 |
      k_im= 0.0360 +/- 0.0011 |      k_im= -0.0462 +/- 0.0011 |
      corr= [-0.26]          |      corr= [ 0.18]          |

      pi:omega/3^S_1(*) |      pi:phi/3^S_1 |      pi:omega/3^D_1 |
=====|=====|=====
      |g|= 0.1651 +/- 0.0053 |      |g|= 0.0001 +/- 0.0020 |      |g|= 0.0472 +/- 0.0109 |
arg(g)/pi= 0.2075 +/- 0.0033 | arg(g)/pi= -0.2861 +/- 11.1741 | arg(g)/pi= 0.1669 +/- 0.0149 |
-----|-----|-----
      g_re= 0.1312 +/- 0.0040 |      g_re= -0.0000 +/- 0.0027 |      g_re= 0.0408 +/- 0.0098 |
      g_im= 0.1002 +/- 0.0039 |      g_im= -0.0000 +/- 0.0021 |      g_im= 0.0236 +/- 0.0052 |
      corr= [ 0.84]          |      corr= [ 1.00]          |      corr= [ 0.89]          |

```



## 2 Unphysical Parameterizations

```

-----|-----|-----|
      Br = 0.5997 +/- 0.0229 |      Br = 0.0000 +/- 0.0000 |      Br = 0.0490 +/- 0.0243 |

--
pi:omega[+] pi:phi[-] upper half-plane

sqrt(s)_pole = (0.24959 +/- 0.0026708)
               + (i/2)*(+0.074858 +/- 0.0034639) [ 0.63]

s_pole = (0.060896 +/- 0.001255)
         + i*(+0.018684 +/- 0.0010033) [ 0.69]

=====|=====|
      pi:omega |      pi:phi |
=====|=====|
      k_re= 0.0589 +/- 0.0025 |      k_re= -0.0412 +/- 0.0025 |
      k_im= 0.0360 +/- 0.0011 |      k_im= -0.0462 +/- 0.0011 |
      corr= [ 0.26] |      corr= [-0.18] |

=====|=====|
      pi:omega/3^S_1(*) |      pi:phi/3^S_1 |      pi:omega/3^D_1 |
=====|=====|
      |g|= 0.1651 +/- 0.0053 |      |g|= 0.0001 +/- 0.0020 |      |g|= 0.0472 +/- 0.0109 |
arg(g)/pi= -0.2075 +/- 0.0033 | arg(g)/pi= 0.2880 +/- 11.1677 | arg(g)/pi= -0.1669 +/- 0.0149 |
-----|-----|-----|
      g_re= 0.1312 +/- 0.0040 |      g_re= -0.0000 +/- 0.0027 |      g_re= 0.0408 +/- 0.0098 |
      g_im= -0.1002 +/- 0.0039 |      g_im= 0.0000 +/- 0.0021 |      g_im= -0.0236 +/- 0.0052 |
      corr= [-0.84] |      corr= [-1.00] |      corr= [-0.89] |
-----|-----|-----|
      Br = 0.5997 +/- 0.0229 |      Br = 0.0000 +/- 0.0000 |      Br = 0.0490 +/- 0.0243 |

--
pi:omega[-] pi:phi[+] lower half-plane

sqrt(s)_pole = (0.20068 +/- 0.0018421)
               + (i/2)*(-5.5937e-16 +/- 2.9218e-13) [ 0.00]

s_pole = (0.040274 +/- 0.00073934)
         + i*(-1.1221e-16 +/- 5.8613e-14) [ 0.00]

=====|=====|
      pi:omega |      pi:phi |
=====|=====|
      k_re= 0.0000 +/- 0.0000 |      k_re= -0.0000 +/- 0.0000 |
      k_im= -0.0454 +/- 0.0016 |      k_im= 0.0612 +/- 0.0008 |
      corr= [ 0.00] |      corr= [ 0.00] |

=====|=====|
      pi:omega/3^S_1(*) |      pi:phi/3^S_1 |      pi:omega/3^D_1 |
=====|=====|
      |g|= 0.1044 +/- 0.0043 |      |g|= 0.0001 +/- 0.0012 |      |g|= 0.0207 +/- 0.0065 |
arg(g)/pi= 0.5000 +/- 0.0000 | arg(g)/pi= -0.0015 +/- 11.1209 | arg(g)/pi= 0.5000 +/- 0.0000 |
-----|-----|-----|
      g_re= 0.0000 +/- 0.0000 |      g_re= 0.0000 +/- 0.0000 |      g_re= 0.0000 +/- 0.0000 |
      g_im= 0.1044 +/- 0.0043 |      g_im= 0.0000 +/- 0.0020 |      g_im= 0.0207 +/- 0.0065 |
      corr= [-1.00] |      corr= [-0.29] |      corr= [-0.19] |
-----|-----|-----|
      Br = 0.0000 +/- 0.0000 |      Br = 0.0000 +/- 0.0000 |      Br = 0.0000 +/- 0.0000 |

--
pi:omega[-] pi:phi[+] upper half-plane

sqrt(s)_pole = (0.24504 +/- 0.00034832)
               + (i/2)*(+0.0080754 +/- 0.00087325) [-0.63]

s_pole = (0.060029 +/- 0.00017295)
         + i*(+0.0019788 +/- 0.00021222) [-0.63]

```



## 2 Unphysical Parameterizations

```

===== pi:omega | pi:phi |
k_re= -0.0462 +/- 0.0004 | k_re= 0.0093 +/- 0.0007 |
k_im= -0.0048 +/- 0.0005 | k_im= 0.0210 +/- 0.0010 |
corr= [-0.60] | corr= [ 0.59] |

===== pi:omega/3^S_1(*) | pi:phi/3^S_1 | pi:omega/3^D_1 |
|g|= 0.0656 +/- 0.0032 | |g|= 0.0003 +/- 0.0049 | |g|= 0.0080 +/- 0.0026 |
arg(g)/pi= 0.1210 +/- 0.0147 | arg(g)/pi= -0.4798 +/- 11.2037 | arg(g)/pi= 0.7202 +/- 0.0186 |
-----
g_re= 0.0610 +/- 0.0034 | g_re= 0.0000 +/- 0.0081 | g_re= -0.0051 +/- 0.0018 |
g_im= 0.0244 +/- 0.0028 | g_im= 0.0000 +/- 0.0005 | g_im= 0.0062 +/- 0.0019 |
corr= [-0.12] | corr= [ 1.00] | corr= [-0.95] |
-----
Br = 0.8175 +/- 0.0101 | Br = 0.0000 +/- 0.0000 | Br = 0.0121 +/- 0.0077 |

--
pi:omega[-] pi:phi[+] lower half-plane

sqrt(s)_pole = (0.24504 +/- 0.00034832)
+ (i/2)*(-0.0080754 +/- 0.00087325) [ 0.63]

s_pole = (0.060029 +/- 0.00017295)
+ i*(-0.0019788 +/- 0.00021222) [ 0.63]

===== pi:omega | pi:phi |
k_re= 0.0462 +/- 0.0004 | k_re= -0.0093 +/- 0.0007 |
k_im= -0.0048 +/- 0.0005 | k_im= 0.0210 +/- 0.0010 |
corr= [ 0.60] | corr= [-0.59] |

===== pi:omega/3^S_1(*) | pi:phi/3^S_1 | pi:omega/3^D_1 |
|g|= 0.0656 +/- 0.0032 | |g|= 0.0003 +/- 0.0049 | |g|= 0.0080 +/- 0.0026 |
arg(g)/pi= -0.1210 +/- 0.0147 | arg(g)/pi= 0.4824 +/- 11.1617 | arg(g)/pi= -0.7202 +/- 0.0186 |
-----
g_re= 0.0610 +/- 0.0034 | g_re= 0.0000 +/- 0.0081 | g_re= -0.0051 +/- 0.0018 |
g_im= -0.0244 +/- 0.0028 | g_im= -0.0000 +/- 0.0005 | g_im= -0.0062 +/- 0.0019 |
corr= [ 0.12] | corr= [-1.00] | corr= [ 0.95] |
-----
Br = 0.8175 +/- 0.0101 | Br = 0.0000 +/- 0.0000 | Br = 0.0121 +/- 0.0077 |

--
pi:omega[-] pi:phi[-] lower half-plane

sqrt(s)_pole = (0.20068 +/- 0.0018421)
+ (i/2)*(-1.0073e-16 +/- 3.6747e-14) [ 0.00]

s_pole = (0.040274 +/- 0.00073933)
+ i*(-2.0226e-17 +/- 7.3776e-15) [ 0.00]

===== pi:omega | pi:phi |
k_re= 0.0000 +/- 0.0000 | k_re= 0.0000 +/- 0.0000 |
k_im= -0.0454 +/- 0.0016 | k_im= -0.0612 +/- 0.0008 |
corr= [ 0.00] | corr= [ 0.00] |

===== pi:omega/3^S_1(*) | pi:phi/3^S_1 | pi:omega/3^D_1 |
|g|= 0.1044 +/- 0.0043 | |g|= 0.0004 +/- 0.0071 | |g|= 0.0207 +/- 0.0065 |

```



## 2 Unphysical Parameterizations

| arg(g)/pi= 0.5000 +/- 0.0000 | arg(g)/pi= -0.0017 +/- 11.1555 | arg(g)/pi= 0.5000 +/- 0.0000 |
|------------------------------|--------------------------------|------------------------------|
| g_re= 0.0000 +/- 0.0000      | g_re= 0.0000 +/- 0.0000        | g_re= 0.0000 +/- 0.0000      |
| g_im= 0.1044 +/- 0.0043      | g_im= 0.0000 +/- 0.0119        | g_im= 0.0207 +/- 0.0065      |
| corr= [-1.00]                | corr= [-0.82]                  | corr= [-0.19]                |
| Br = 0.0000 +/- 0.0000       | Br = 0.0000 +/- 0.0000         | Br = 0.0000 +/- 0.0000       |

--

pi:omega[-] pi:phi[-] upper half-plane

sqrt(s)\_pole = (0.24504 +/- 0.00034856)  
+ (i/2)\*(+0.0080756 +/- 0.00087354) [-0.63]

s\_pole = (0.060029 +/- 0.00017307)  
+ i\*(+0.0019788 +/- 0.00021229) [-0.64]

| pi:omega                 | pi:phi                   |
|--------------------------|--------------------------|
| k_re= -0.0462 +/- 0.0004 | k_re= -0.0093 +/- 0.0007 |
| k_im= -0.0048 +/- 0.0005 | k_im= -0.0210 +/- 0.0010 |
| corr= [-0.60]            | corr= [ 0.59]            |

| pi:omega/3~S_1(*)            | pi:phi/3~S_1                  | pi:omega/3~D_1               |
|------------------------------|-------------------------------|------------------------------|
| g = 0.0656 +/- 0.0032        | g = 0.0004 +/- 0.0067         | g = 0.0080 +/- 0.0026        |
| arg(g)/pi= 0.1210 +/- 0.0147 | arg(g)/pi= 0.4695 +/- 11.1579 | arg(g)/pi= 0.7202 +/- 0.0186 |
| g_re= 0.0610 +/- 0.0034      | g_re= 0.0000 +/- 0.0112       | g_re= -0.0051 +/- 0.0018     |
| g_im= 0.0244 +/- 0.0028      | g_im= -0.0000 +/- 0.0011      | g_im= 0.0062 +/- 0.0019      |
| corr= [-0.12]                | corr= [-1.00]                 | corr= [-0.95]                |
| Br = 0.8175 +/- 0.0101       | Br = 0.0000 +/- 0.0000        | Br = 0.0121 +/- 0.0077       |

--

pi:omega[-] pi:phi[-] lower half-plane

sqrt(s)\_pole = (0.24504 +/- 0.00034856)  
+ (i/2)\*(-0.0080756 +/- 0.00087354) [ 0.63]

s\_pole = (0.060029 +/- 0.00017307)  
+ i\*(-0.0019788 +/- 0.00021229) [ 0.64]

| pi:omega                 | pi:phi                   |
|--------------------------|--------------------------|
| k_re= 0.0462 +/- 0.0004  | k_re= 0.0093 +/- 0.0007  |
| k_im= -0.0048 +/- 0.0005 | k_im= -0.0210 +/- 0.0010 |
| corr= [ 0.60]            | corr= [-0.59]            |

| pi:omega/3~S_1(*)             | pi:phi/3~S_1                   | pi:omega/3~D_1                |
|-------------------------------|--------------------------------|-------------------------------|
| g = 0.0656 +/- 0.0032         | g = 0.0004 +/- 0.0067          | g = 0.0080 +/- 0.0026         |
| arg(g)/pi= -0.1210 +/- 0.0147 | arg(g)/pi= -0.4666 +/- 11.2324 | arg(g)/pi= -0.7202 +/- 0.0186 |
| g_re= 0.0610 +/- 0.0034       | g_re= 0.0000 +/- 0.0112        | g_re= -0.0051 +/- 0.0018      |
| g_im= -0.0244 +/- 0.0028      | g_im= 0.0000 +/- 0.0011        | g_im= -0.0062 +/- 0.0019      |
| corr= [ 0.12]                 | corr= [ 1.00]                  | corr= [ 0.95]                 |
| Br = 0.8175 +/- 0.0101        | Br = 0.0000 +/- 0.0000         | Br = 0.0121 +/- 0.0077        |



## 2.14 coupled\_po\_pp.3s1\_3d1.pole+G0\_3s1\_3sd1\_3S1+G1\_3s1.gorder0\_3s1\_3S1.threshold\_sub

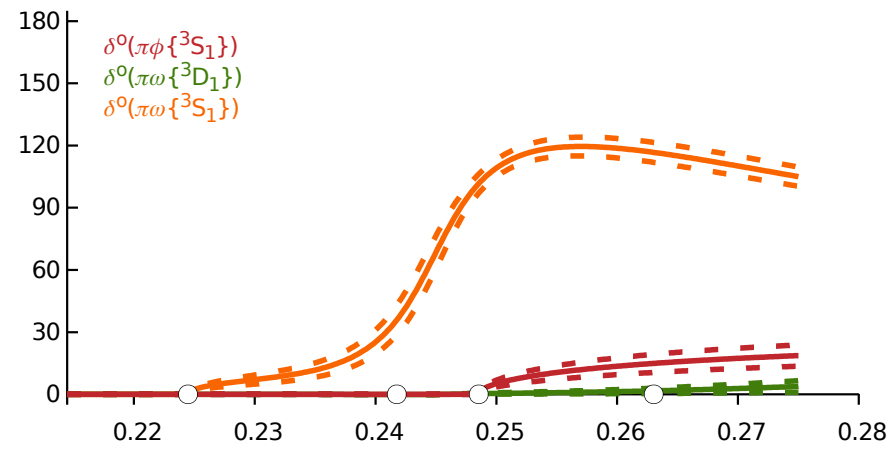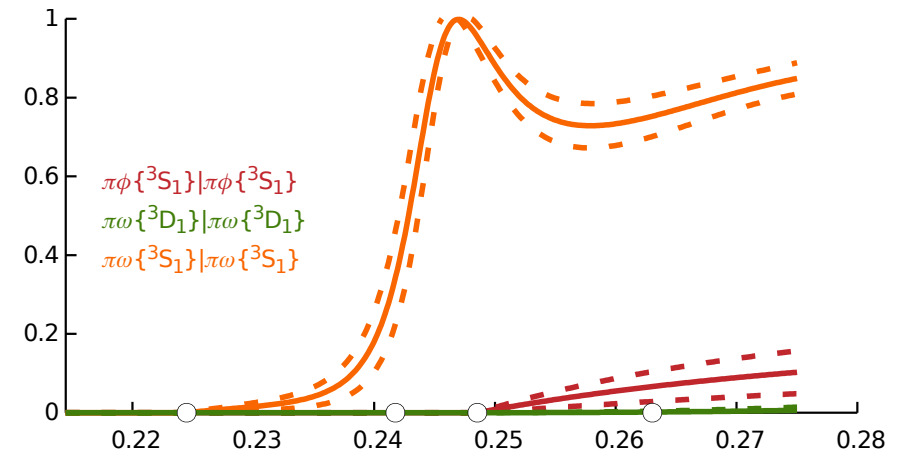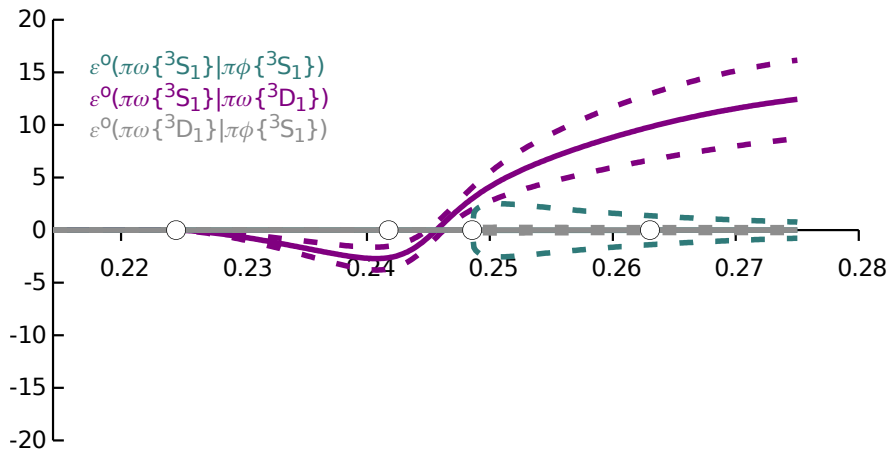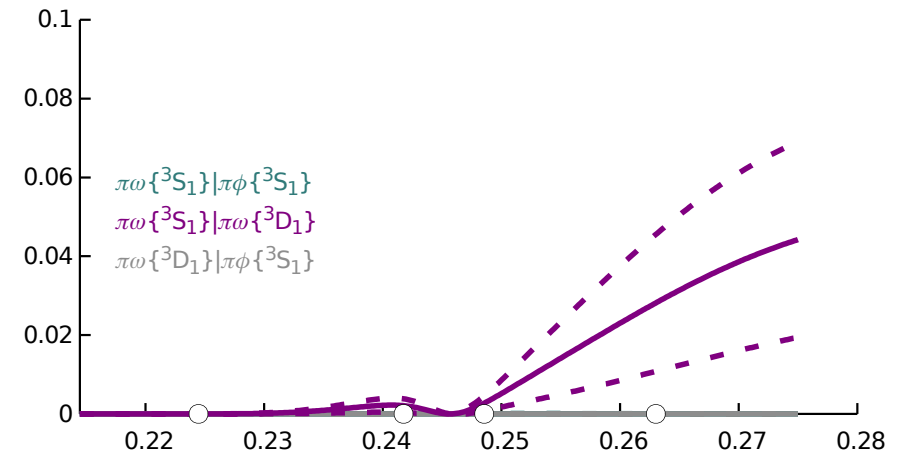



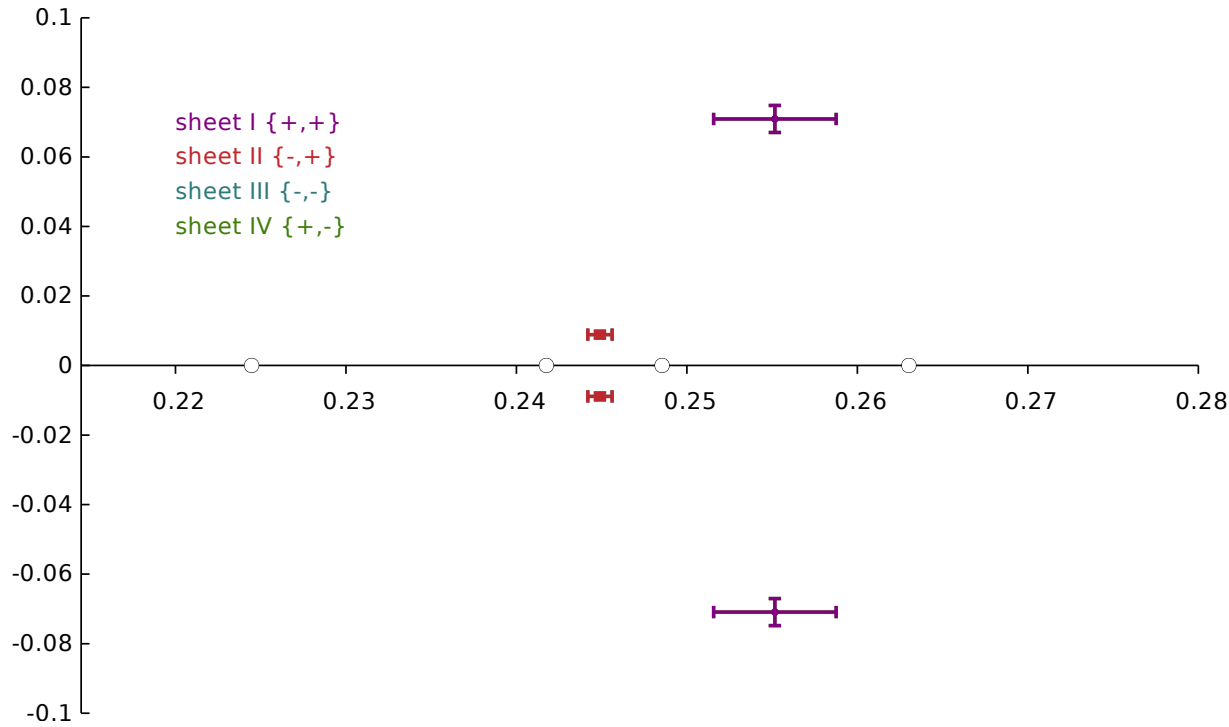

### parameter values

minimised with  $\text{chisq}/\text{nDoF} = 33.27 / (36 - 7) = 1.15$

|                                               |  |                          |  |      |       |       |       |       |       |       |
|-----------------------------------------------|--|--------------------------|--|------|-------|-------|-------|-------|-------|-------|
| JP1+_g_pi:omega/3^S_1_pole0                   |  | 0.077770 +/- 0.004756    |  | 1.00 | -0.05 | -0.26 | -0.26 | 0.18  | 0.10  | -0.42 |
| JP1+_g_pi:phi/3^S_1_pole0                     |  | -7.9299e-05 +/- 0.010548 |  |      | 1.00  | 0.02  | 0.00  | 0.00  | -0.01 | -0.04 |
| JP1+_gamma_pi:omega/3^S_1 pi:omega/3^D_1_orde |  | -27.774 +/- 10.309       |  |      |       | 1.00  | -0.09 | 0.31  | -0.06 | -0.05 |
| JP1+_gamma_pi:omega/3^S_1 pi:omega/3^S_1_orde |  | 4.6885 +/- 0.42072       |  |      |       |       | 1.00  | -0.91 | 0.01  | 0.07  |
| JP1+_gamma_pi:omega/3^S_1 pi:omega/3^S_1_orde |  | -92.121 +/- 8.0762       |  |      |       |       |       | 1.00  | 0.06  | -0.07 |
| JP1+_gamma_pi:phi/3^S_1 pi:phi/3^S_1_order0   |  | 0.94613 +/- 0.29679      |  |      |       |       |       |       | 1.00  | -0.28 |
| JP1+_m_pole0                                  |  | 0.24564 +/- 0.00062583   |  |      |       |       |       |       |       | 1.00  |

### pole singularities

pi:omega[+] pi:phi[+] upper half-plane

$\text{sqrt}(s)_{\text{pole}} = (0.25516 \pm 0.0035961) + (i/2) * (0.070919 \pm 0.0038913) [0.67]$

$s_{\text{pole}} = (0.063852 \pm 0.0017463) + i * (0.018096 \pm 0.0011783) [0.74]$

|                         |  |                         |  |
|-------------------------|--|-------------------------|--|
| pi:omega                |  | pi:phi                  |  |
| =====                   |  | =====                   |  |
| k_re= 0.0628 +/- 0.0032 |  | k_re= 0.0445 +/- 0.0035 |  |
| k_im= 0.0329 +/- 0.0012 |  | k_im= 0.0422 +/- 0.0013 |  |



## 2 Unphysical Parameterizations

```

corr= [ 0.24]          |      corr= [-0.28]          |
=====
pi:omega/3^S_1(*) |      pi:phi/3^S_1 |      pi:omega/3^D_1 |
=====
|g|= 0.1567 +/- 0.0065 |      |g|= 0.0001 +/- 0.0016 |      |g|= 0.0440 +/- 0.0117 |
arg(g)/pi= -0.2478 +/- 0.0032 |      arg(g)/pi= -0.2954 +/- 10.9312 |      arg(g)/pi= -0.2080 +/- 0.0172 |
-----
g_re= 0.1116 +/- 0.0046 |      g_re= 0.0000 +/- 0.0025 |      g_re= 0.0349 +/- 0.0099 |
g_im= -0.1101 +/- 0.0049 |      g_im= 0.0000 +/- 0.0008 |      g_im= -0.0267 +/- 0.0066 |
corr= [-0.89]          |      corr= [ 1.00]          |      corr= [-0.92]          |
-----
Br = 0.6086 +/- 0.0274 |      Br = 0.0000 +/- 0.0000 |      Br = 0.0479 +/- 0.0273 |

--
pi:omega[+] pi:phi[+] lower half-plane

sqrt(s)_pole = (0.25516 +/- 0.0035961)
               + (i/2)*(-0.070919 +/- 0.0038913) [-0.67]

s_pole = (0.063852 +/- 0.0017463)
         + i*(-0.018096 +/- 0.0011783) [-0.74]

pi:omega |      pi:phi |
=====
k_re= -0.0628 +/- 0.0032 |      k_re= -0.0445 +/- 0.0035 |
k_im= 0.0329 +/- 0.0012 |      k_im= 0.0422 +/- 0.0013 |
corr= [-0.24]          |      corr= [ 0.28]          |

pi:omega/3^S_1(*) |      pi:phi/3^S_1 |      pi:omega/3^D_1 |
=====
|g|= 0.1567 +/- 0.0065 |      |g|= 0.0001 +/- 0.0016 |      |g|= 0.0440 +/- 0.0117 |
arg(g)/pi= 0.2478 +/- 0.0032 |      arg(g)/pi= 0.2954 +/- 10.9312 |      arg(g)/pi= 0.2080 +/- 0.0172 |
-----
g_re= 0.1116 +/- 0.0046 |      g_re= 0.0000 +/- 0.0025 |      g_re= 0.0349 +/- 0.0099 |
g_im= 0.1101 +/- 0.0049 |      g_im= -0.0000 +/- 0.0008 |      g_im= 0.0267 +/- 0.0066 |
corr= [ 0.89]          |      corr= [-1.00]          |      corr= [ 0.92]          |
-----
Br = 0.6086 +/- 0.0274 |      Br = 0.0000 +/- 0.0000 |      Br = 0.0479 +/- 0.0273 |

--
pi:omega[+] pi:phi[-] lower half-plane

sqrt(s)_pole = (0.25516 +/- 0.0035961)
               + (i/2)*(-0.070919 +/- 0.0038913) [-0.67]

s_pole = (0.063852 +/- 0.0017463)
         + i*(-0.018096 +/- 0.0011783) [-0.74]

pi:omega |      pi:phi |
=====
k_re= -0.0628 +/- 0.0032 |      k_re= 0.0445 +/- 0.0035 |
k_im= 0.0329 +/- 0.0012 |      k_im= -0.0422 +/- 0.0013 |
corr= [-0.24]          |      corr= [ 0.28]          |

pi:omega/3^S_1(*) |      pi:phi/3^S_1 |      pi:omega/3^D_1 |
=====
|g|= 0.1567 +/- 0.0065 |      |g|= 0.0001 +/- 0.0022 |      |g|= 0.0440 +/- 0.0117 |
arg(g)/pi= 0.2478 +/- 0.0032 |      arg(g)/pi= -0.2612 +/- 10.9326 |      arg(g)/pi= 0.2080 +/- 0.0172 |
-----
g_re= 0.1116 +/- 0.0046 |      g_re= 0.0000 +/- 0.0034 |      g_re= 0.0349 +/- 0.0099 |
g_im= 0.1101 +/- 0.0049 |      g_im= 0.0000 +/- 0.0016 |      g_im= 0.0267 +/- 0.0066 |
corr= [ 0.89]          |      corr= [ 1.00]          |      corr= [ 0.92]          |

```



```

-----|-----|-----|
      Br =  0.6086 +/- 0.0274 |      Br =  0.0000 +/- 0.0000 |      Br =  0.0479 +/- 0.0273 |

--
pi:omega[+] pi:phi[-] upper half-plane

sqrt(s)_pole = (0.25516 +/- 0.0035961)
               + (i/2)*(+0.070919 +/- 0.0038913) [ 0.67]

s_pole = (0.063852 +/- 0.0017463)
         + i*(+0.018096 +/- 0.0011783) [ 0.74]

=====|=====|
      pi:omega |      pi:phi |
=====|=====|
      k_re=  0.0628 +/- 0.0032 |      k_re= -0.0445 +/- 0.0035 |
      k_im=  0.0329 +/- 0.0012 |      k_im= -0.0422 +/- 0.0013 |
      corr= [ 0.24]           |      corr= [-0.28]           |

=====|=====|=====|
      pi:omega/3^S_1(*) |      pi:phi/3^S_1 |      pi:omega/3^D_1 |
=====|=====|=====|
      |g|=  0.1567 +/- 0.0065 |      |g|=  0.0001 +/- 0.0022 |      |g|=  0.0440 +/- 0.0117 |
arg(g)/pi= -0.2478 +/- 0.0032 | arg(g)/pi=  0.2612 +/- 10.9326 | arg(g)/pi= -0.2080 +/- 0.0172 |
-----|-----|-----|
      g_re=  0.1116 +/- 0.0046 |      g_re=  0.0000 +/- 0.0034 |      g_re=  0.0349 +/- 0.0099 |
      g_im= -0.1101 +/- 0.0049 |      g_im= -0.0000 +/- 0.0016 |      g_im= -0.0267 +/- 0.0066 |
      corr= [-0.89]           |      corr= [-1.00]           |      corr= [-0.92]           |
-----|-----|-----|
      Br =  0.6086 +/- 0.0274 |      Br =  0.0000 +/- 0.0000 |      Br =  0.0479 +/- 0.0273 |

--
pi:omega[-] pi:phi[+] lower half-plane

sqrt(s)_pole = (0.19499 +/- 0.0024408)
               + (i/2)*(-7.9964e-17 +/- 3.1845e-14) [ 0.00]

s_pole = (0.038023 +/- 0.00095185)
         + i*(-1.5606e-17 +/- 6.213e-15) [ 0.00]

=====|=====|
      pi:omega |      pi:phi |
=====|=====|
      k_re=  0.0000 +/- 0.0000 |      k_re= -0.0000 +/- 0.0000 |
      k_im= -0.0498 +/- 0.0018 |      k_im=  0.0635 +/- 0.0009 |
      corr= [ 0.00]           |      corr= [ 0.00]           |

=====|=====|=====|
      pi:omega/3^S_1(*) |      pi:phi/3^S_1 |      pi:omega/3^D_1 |
=====|=====|=====|
      |g|=  0.1119 +/- 0.0051 |      |g|=  0.0001 +/- 0.0012 |      |g|=  0.0205 +/- 0.0077 |
arg(g)/pi=  0.5000 +/- 0.0000 | arg(g)/pi= -0.1016 +/- 10.9000 | arg(g)/pi=  0.5000 +/- 0.0000 |
-----|-----|-----|
      g_re=  0.0000 +/- 0.0000 |      g_re=  0.0000 +/- 0.0000 |      g_re=  0.0000 +/- 0.0000 |
      g_im=  0.1119 +/- 0.0051 |      g_im= -0.0000 +/- 0.0019 |      g_im=  0.0205 +/- 0.0077 |
      corr= [-1.00]           |      corr= [-0.28]           |      corr= [-0.20]           |
-----|-----|-----|
      Br =  0.0000 +/- 0.0000 |      Br =  0.0000 +/- 0.0000 |      Br =  0.0000 +/- 0.0000 |

--
pi:omega[-] pi:phi[+] upper half-plane

sqrt(s)_pole = ( 0.2449 +/- 0.00071073)
               + (i/2)*(+0.0088836 +/- 0.00097498) [-0.38]

s_pole = (0.059957 +/- 0.00034977)
         + i*(+0.0021756 +/- 0.00023647) [-0.36]
    
```



```

===== pi:omega | pi:phi |
k_re= -0.0461 +/- 0.0008 | k_re= 0.0100 +/- 0.0009 |
k_im= -0.0053 +/- 0.0006 | k_im= 0.0216 +/- 0.0015 |
corr= [-0.43] | corr= [-0.10] |

===== pi:omega/3^S_1(*) | pi:phi/3^S_1 | pi:omega/3^D_1 |
=====
|g|= 0.0686 +/- 0.0035 | |g|= 0.0003 +/- 0.0052 | |g|= 0.0065 +/- 0.0025 |
arg(g)/pi= 0.1109 +/- 0.0197 | arg(g)/pi= -0.5743 +/- 10.9347 | arg(g)/pi= 0.6384 +/- 0.0224 |
-----
g_re= 0.0645 +/- 0.0041 | g_re= -0.0001 +/- 0.0086 | g_re= -0.0028 +/- 0.0013 |
g_im= 0.0234 +/- 0.0037 | g_im= -0.0000 +/- 0.0008 | g_im= 0.0059 +/- 0.0021 |
corr= [-0.39] | corr= [ 1.00] | corr= [-0.95] |
-----
Br = 0.8097 +/- 0.0184 | Br = 0.0000 +/- 0.0000 | Br = 0.0074 +/- 0.0055 |

--
pi:omega[-] pi:phi[+] lower half-plane

sqrt(s)_pole = ( 0.2449 +/- 0.00071073)
+ (i/2)*(-0.0088836 +/- 0.00097498) [ 0.38]

s_pole = (0.059957 +/- 0.00034977)
+ i*(-0.0021756 +/- 0.00023647) [ 0.36]

===== pi:omega | pi:phi |
k_re= 0.0461 +/- 0.0008 | k_re= -0.0100 +/- 0.0009 |
k_im= -0.0053 +/- 0.0006 | k_im= 0.0216 +/- 0.0015 |
corr= [ 0.43] | corr= [ 0.10] |

===== pi:omega/3^S_1(*) | pi:phi/3^S_1 | pi:omega/3^D_1 |
=====
|g|= 0.0686 +/- 0.0035 | |g|= 0.0003 +/- 0.0052 | |g|= 0.0065 +/- 0.0025 |
arg(g)/pi= -0.1109 +/- 0.0197 | arg(g)/pi= 0.5743 +/- 10.9347 | arg(g)/pi= -0.6384 +/- 0.0224 |
-----
g_re= 0.0645 +/- 0.0041 | g_re= -0.0001 +/- 0.0086 | g_re= -0.0028 +/- 0.0013 |
g_im= -0.0234 +/- 0.0037 | g_im= 0.0000 +/- 0.0008 | g_im= -0.0059 +/- 0.0021 |
corr= [ 0.39] | corr= [-1.00] | corr= [ 0.95] |
-----
Br = 0.8097 +/- 0.0184 | Br = 0.0000 +/- 0.0000 | Br = 0.0074 +/- 0.0055 |

--
pi:omega[-] pi:phi[-] upper half-plane

sqrt(s)_pole = (0.19499 +/- 0.0024408)
+ (i/2)*(+3.487e-14 +/- 1.7624e-11) [ 0.00]

s_pole = (0.038023 +/- 0.00095182)
+ i*(+6.7949e-15 +/- 3.4344e-12) [ 0.00]

===== pi:omega | pi:phi |
k_re= -0.0000 +/- 0.0000 | k_re= -0.0000 +/- 0.0000 |
k_im= -0.0498 +/- 0.0018 | k_im= -0.0635 +/- 0.0009 |
corr= [ 0.00] | corr= [ 0.00] |

===== pi:omega/3^S_1(*) | pi:phi/3^S_1 | pi:omega/3^D_1 |
=====
|g|= 0.1119 +/- 0.0051 | |g|= 0.0006 +/- 0.0101 | |g|= 0.0205 +/- 0.0077 |

```



## 2 Unphysical Parameterizations

| arg(g)/pi= 0.5000 +/- 0.0000 | arg(g)/pi= -0.1019 +/- 10.9302 | arg(g)/pi= 0.5000 +/- 0.0000 |
|------------------------------|--------------------------------|------------------------------|
| g_re= 0.0000 +/- 0.0000      | g_re= 0.0000 +/- 0.0000        | g_re= 0.0000 +/- 0.0000      |
| g_im= 0.1119 +/- 0.0051      | g_im= -0.0001 +/- 0.0166       | g_im= 0.0205 +/- 0.0077      |
| corr= [-1.00]                | corr= [-0.87]                  | corr= [-0.20]                |
| Br = 0.0000 +/- 0.0000       | Br = 0.0000 +/- 0.0000         | Br = 0.0000 +/- 0.0000       |

--

pi:omega[-] pi:phi[-] upper half-plane

sqrt(s)\_pole = ( 0.2449 +/- 0.00071093)  
+ (i/2)\*(+0.0088838 +/- 0.00097538) [-0.38]

s\_pole = (0.059957 +/- 0.00034987)  
+ i\*(+0.0021757 +/- 0.00023656) [-0.37]

| pi:omega                 | pi:phi                   |
|--------------------------|--------------------------|
| k_re= -0.0461 +/- 0.0008 | k_re= -0.0100 +/- 0.0009 |
| k_im= -0.0053 +/- 0.0006 | k_im= -0.0216 +/- 0.0015 |
| corr= [-0.43]            | corr= [-0.10]            |

| pi:omega/3~S_1(*)            | pi:phi/3~S_1                  | pi:omega/3~D_1               |
|------------------------------|-------------------------------|------------------------------|
| g = 0.0686 +/- 0.0035        | g = 0.0004 +/- 0.0073         | g = 0.0065 +/- 0.0025        |
| arg(g)/pi= 0.1109 +/- 0.0197 | arg(g)/pi= 0.5749 +/- 10.9349 | arg(g)/pi= 0.6384 +/- 0.0224 |
| g_re= 0.0645 +/- 0.0041      | g_re= -0.0001 +/- 0.0121      | g_re= -0.0028 +/- 0.0013     |
| g_im= 0.0234 +/- 0.0037      | g_im= 0.0000 +/- 0.0010       | g_im= 0.0059 +/- 0.0021      |
| corr= [-0.39]                | corr= [-1.00]                 | corr= [-0.95]                |
| Br = 0.8097 +/- 0.0184       | Br = 0.0000 +/- 0.0000        | Br = 0.0074 +/- 0.0055       |

--

pi:omega[-] pi:phi[-] lower half-plane

sqrt(s)\_pole = ( 0.2449 +/- 0.00071093)  
+ (i/2)\*(-0.0088838 +/- 0.00097538) [ 0.38]

s\_pole = (0.059957 +/- 0.00034987)  
+ i\*(-0.0021757 +/- 0.00023656) [ 0.37]

| pi:omega                 | pi:phi                   |
|--------------------------|--------------------------|
| k_re= 0.0461 +/- 0.0008  | k_re= 0.0100 +/- 0.0009  |
| k_im= -0.0053 +/- 0.0006 | k_im= -0.0216 +/- 0.0015 |
| corr= [ 0.43]            | corr= [ 0.10]            |

| pi:omega/3~S_1(*)             | pi:phi/3~S_1                   | pi:omega/3~D_1                |
|-------------------------------|--------------------------------|-------------------------------|
| g = 0.0686 +/- 0.0035         | g = 0.0004 +/- 0.0073          | g = 0.0065 +/- 0.0025         |
| arg(g)/pi= -0.1109 +/- 0.0197 | arg(g)/pi= -0.5749 +/- 10.9349 | arg(g)/pi= -0.6384 +/- 0.0224 |
| g_re= 0.0645 +/- 0.0041       | g_re= -0.0001 +/- 0.0121       | g_re= -0.0028 +/- 0.0013      |
| g_im= -0.0234 +/- 0.0037      | g_im= -0.0000 +/- 0.0010       | g_im= -0.0059 +/- 0.0021      |
| corr= [ 0.39]                 | corr= [ 1.00]                  | corr= [ 0.95]                 |
| Br = 0.8097 +/- 0.0184        | Br = 0.0000 +/- 0.0000         | Br = 0.0074 +/- 0.0055        |



## 2.15 coupled\_po\_pp.3s1\_3d1.pole+G0\_3s1\_3sd1\_3S1+G1\_3s1.gorder0\_3s1.irho

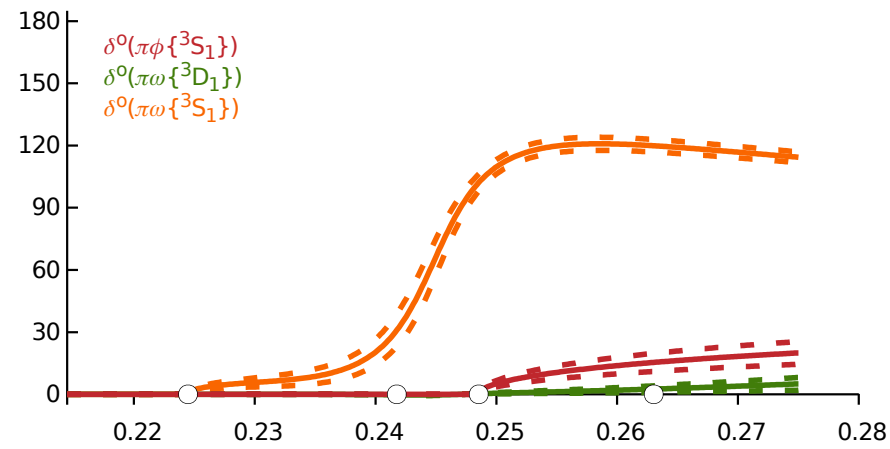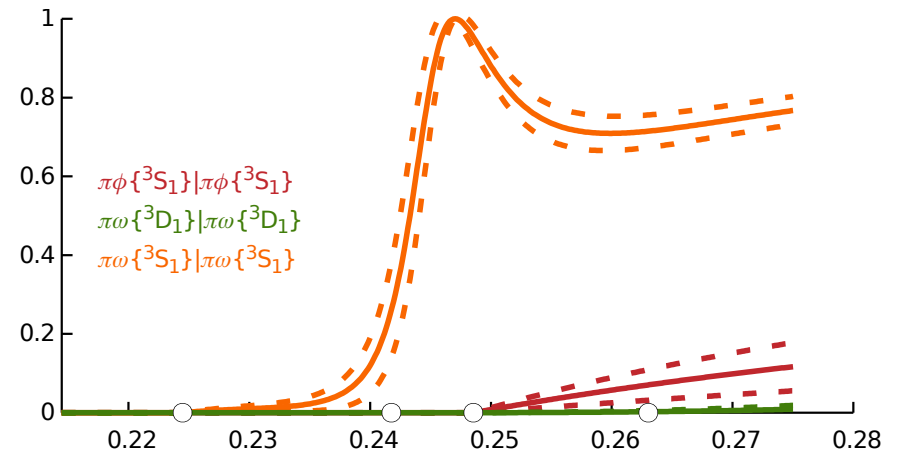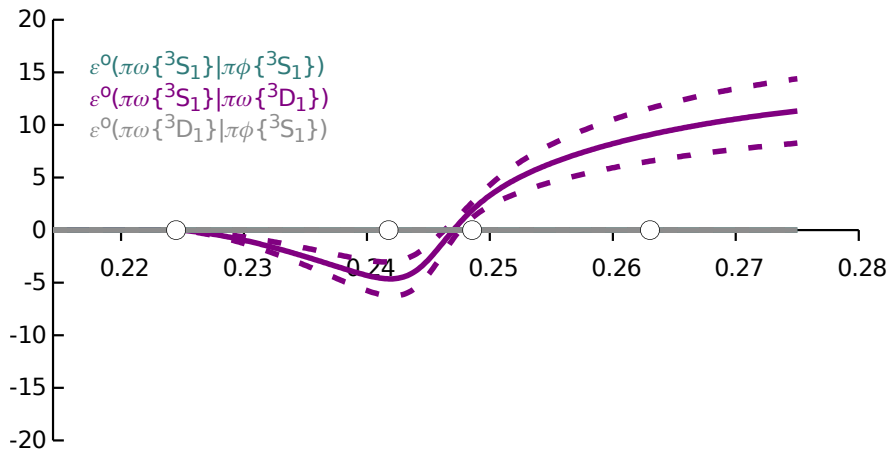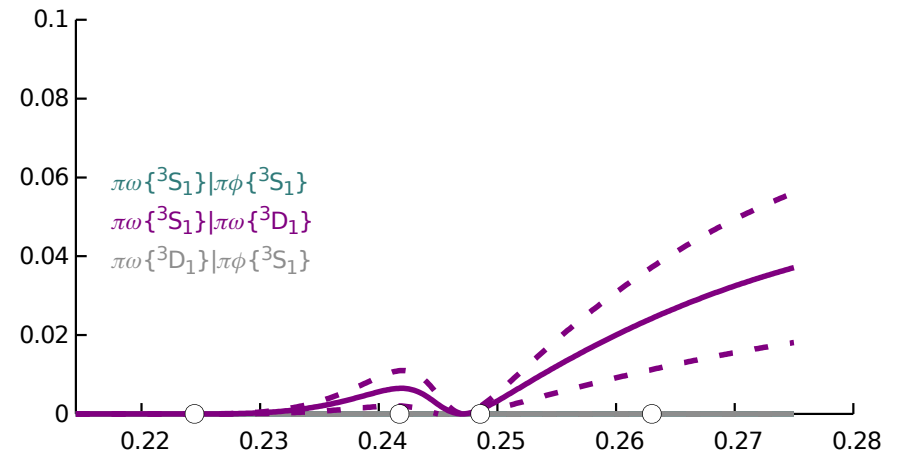



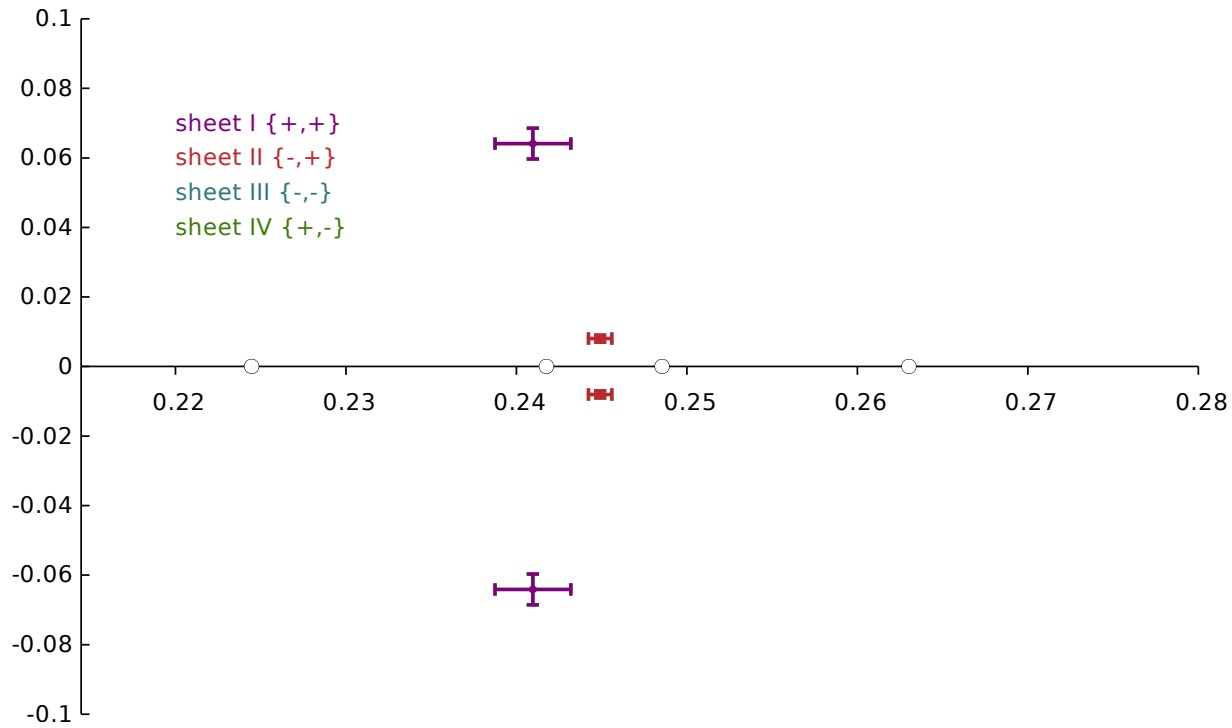

### parameter values

minimised with  $\text{chisq}/\text{nDoF} = 33.27 / (36 - 6) = 1.11$

|                                               |  |                        |  |      |       |       |       |       |       |
|-----------------------------------------------|--|------------------------|--|------|-------|-------|-------|-------|-------|
| JP1+_g_pi:omega/3~S_1 pole0                   |  | 0.086326 +/- 0.0061901 |  | 1.00 | -0.25 | -0.17 | -0.02 | 0.01  | -0.11 |
| JP1+_gamma_pi:omega/3~S_1 pi:omega/3~D_1_orde |  | -38.753 +/- 12.701     |  |      | 1.00  | -0.20 | 0.34  | -0.11 | -0.14 |
| JP1+_gamma_pi:omega/3~S_1 pi:omega/3~S_1_orde |  | 6.6946 +/- 0.61919     |  |      |       | 1.00  | -0.95 | 0.00  | 0.02  |
| JP1+_gamma_pi:omega/3~S_1 pi:omega/3~S_1_orde |  | -134.48 +/- 12.32      |  |      |       |       | 1.00  | 0.04  | -0.03 |
| JP1+_gamma_pi:phi/3~S_1 pi:phi/3~S_1_order0   |  | 0.92773 +/- 0.28229    |  |      |       |       |       | 1.00  | -0.26 |
| JP1+_m_pole0                                  |  | 0.24703 +/- 0.00058739 |  |      |       |       |       |       | 1.00  |

### pole singularities

pi:omega[+] pi:phi[+] upper half-plane

$\text{sqrt}(s)_{\text{pole}} = (0.24097 \pm 0.0022232)$   
 $+ (i/2)*(+0.064119 \pm 0.0044446)$  [ 0.60]

$s_{\text{pole}} = (0.05704 \pm 0.00099292)$   
 $+ i*(+0.015451 \pm 0.0011618)$  [ 0.58]

|                         |                         |
|-------------------------|-------------------------|
| pi:omega                | pi:phi                  |
| ===== =====             | ===== =====             |
| k_re= 0.0501 +/- 0.0024 | k_re= 0.0323 +/- 0.0025 |
| k_im= 0.0344 +/- 0.0015 | k_im= 0.0469 +/- 0.0012 |
| corr= [ 0.45]           | corr= [ 0.12]           |



| pi:omega/3^S_1(*)                                                    | pi:phi/3^S_1                                                         | pi:omega/3^D_1                                                       |
|----------------------------------------------------------------------|----------------------------------------------------------------------|----------------------------------------------------------------------|
| g = 0.1302 +/- 0.0043<br>arg(g)/pi= -0.1313 +/- 0.0040               | g = 0.0000 +/- 0.0000<br>arg(g)/pi= 0.6313 +/- 0.0040                | g = 0.0373 +/- 0.0086<br>arg(g)/pi= -0.0996 +/- 0.0178               |
| g_re= 0.1193 +/- 0.0043<br>g_im= -0.0522 +/- 0.0015<br>corr= [-0.47] | g_re= -0.0000 +/- 0.0000<br>g_im= 0.0000 +/- 0.0000<br>corr= [-0.84] | g_re= 0.0355 +/- 0.0083<br>g_im= -0.0115 +/- 0.0030<br>corr= [-0.70] |
| Br = 0.3710 +/- 0.0191                                               | Br = 0.0000 +/- 0.0000                                               | Br = 0.0305 +/- 0.0151                                               |

--

pi:omega[+] pi:phi[+] lower half-plane

sqrt(s)\_pole = (0.24097 +/- 0.0022232)  
+ (i/2)\*(-0.064119 +/- 0.0044446) [-0.60]

s\_pole = (0.05704 +/- 0.00099292)  
+ i\*(-0.015451 +/- 0.0011618) [-0.58]

| pi:omega                                                             | pi:phi                                                               |
|----------------------------------------------------------------------|----------------------------------------------------------------------|
| k_re= -0.0501 +/- 0.0024<br>k_im= 0.0344 +/- 0.0015<br>corr= [-0.45] | k_re= -0.0323 +/- 0.0025<br>k_im= 0.0469 +/- 0.0012<br>corr= [-0.12] |

| pi:omega/3^S_1(*)                                                   | pi:phi/3^S_1                                                        | pi:omega/3^D_1                                                      |
|---------------------------------------------------------------------|---------------------------------------------------------------------|---------------------------------------------------------------------|
| g = 0.1302 +/- 0.0043<br>arg(g)/pi= 0.1313 +/- 0.0040               | g = 0.0000 +/- 0.0000<br>arg(g)/pi= 0.3687 +/- 0.0040               | g = 0.0373 +/- 0.0086<br>arg(g)/pi= 0.0996 +/- 0.0178               |
| g_re= 0.1193 +/- 0.0043<br>g_im= 0.0522 +/- 0.0015<br>corr= [ 0.47] | g_re= 0.0000 +/- 0.0000<br>g_im= 0.0000 +/- 0.0000<br>corr= [ 0.84] | g_re= 0.0355 +/- 0.0083<br>g_im= 0.0115 +/- 0.0030<br>corr= [ 0.70] |
| Br = 0.3710 +/- 0.0191                                              | Br = 0.0000 +/- 0.0000                                              | Br = 0.0305 +/- 0.0151                                              |

--

pi:omega[+] pi:phi[-] upper half-plane

sqrt(s)\_pole = (0.24097 +/- 0.0022232)  
+ (i/2)\*(+0.064119 +/- 0.0044446) [ 0.60]

s\_pole = (0.05704 +/- 0.00099292)  
+ i\*(+0.015451 +/- 0.0011618) [ 0.58]

| pi:omega                                                            | pi:phi                                                                |
|---------------------------------------------------------------------|-----------------------------------------------------------------------|
| k_re= 0.0501 +/- 0.0024<br>k_im= 0.0344 +/- 0.0015<br>corr= [ 0.45] | k_re= -0.0323 +/- 0.0025<br>k_im= -0.0469 +/- 0.0012<br>corr= [ 0.12] |

| pi:omega/3^S_1(*)                                                    | pi:phi/3^S_1                                                         | pi:omega/3^D_1                                                       |
|----------------------------------------------------------------------|----------------------------------------------------------------------|----------------------------------------------------------------------|
| g = 0.1302 +/- 0.0043<br>arg(g)/pi= -0.1313 +/- 0.0040               | g = 0.0000 +/- 0.0000<br>arg(g)/pi= 0.6313 +/- 0.0040                | g = 0.0373 +/- 0.0086<br>arg(g)/pi= -0.0996 +/- 0.0178               |
| g_re= 0.1193 +/- 0.0043<br>g_im= -0.0522 +/- 0.0015<br>corr= [-0.47] | g_re= -0.0000 +/- 0.0000<br>g_im= 0.0000 +/- 0.0000<br>corr= [-0.84] | g_re= 0.0355 +/- 0.0083<br>g_im= -0.0115 +/- 0.0030<br>corr= [-0.70] |



## 2 Unphysical Parameterizations

```

Br = 0.3710 +/- 0.0191 | Br = 0.0000 +/- 0.0000 | Br = 0.0305 +/- 0.0151 |

--
pi:omega[+] pi:phi[-] lower half-plane

sqrt(s)_pole = (0.24097 +/- 0.0022232)
+ (i/2)*(-0.064119 +/- 0.0044446) [-0.60]

s_pole = (0.05704 +/- 0.00099292)
+ i*(-0.015451 +/- 0.0011618) [-0.58]

=====
pi:omega | pi:phi |
=====
k_re= -0.0501 +/- 0.0024 | k_re= 0.0323 +/- 0.0025 |
k_im= 0.0344 +/- 0.0015 | k_im= -0.0469 +/- 0.0012 |
corr= [-0.45] | corr= [-0.12] |

=====
pi:omega/3^S_1(*) | pi:phi/3^S_1 | pi:omega/3^D_1 |
=====
|g|= 0.1302 +/- 0.0043 | |g|= 0.0000 +/- 0.0000 | |g|= 0.0373 +/- 0.0086 |
arg(g)/pi= 0.1313 +/- 0.0040 | arg(g)/pi= 0.3687 +/- 0.0040 | arg(g)/pi= 0.0996 +/- 0.0178 |
-----
g_re= 0.1193 +/- 0.0043 | g_re= 0.0000 +/- 0.0000 | g_re= 0.0355 +/- 0.0083 |
g_im= 0.0522 +/- 0.0015 | g_im= 0.0000 +/- 0.0000 | g_im= 0.0115 +/- 0.0030 |
corr= [ 0.47] | corr= [ 0.84] | corr= [ 0.70] |
-----
Br = 0.3710 +/- 0.0191 | Br = 0.0000 +/- 0.0000 | Br = 0.0305 +/- 0.0151 |

--
pi:omega[-] pi:phi[+] upper half-plane

sqrt(s)_pole = (0.19527 +/- 0.0022187)
+ (i/2)*(+1.1421e-18 +/- 5.7126e-16) [ 0.00]

s_pole = (0.038131 +/- 0.00086647)
+ i*(+2.2294e-19 +/- 1.1151e-16) [ 0.00]

=====
pi:omega | pi:phi |
=====
k_re= -0.0000 +/- 0.0000 | k_re= 0.0000 +/- 0.0000 |
k_im= -0.0496 +/- 0.0016 | k_im= 0.0634 +/- 0.0008 |
corr= [ 0.00] | corr= [ 0.00] |

=====
pi:omega/3^S_1(*) | pi:phi/3^S_1 | pi:omega/3^D_1 |
=====
|g|= 0.1283 +/- 0.0046 | |g|= 0.0000 +/- 0.0000 | |g|= 0.0249 +/- 0.0075 |
arg(g)/pi= 0.5000 +/- 0.0000 | arg(g)/pi= 0.0000 +/- 0.0000 | arg(g)/pi= 0.5000 +/- 0.0000 |
-----
g_re= 0.0000 +/- 0.0000 | g_re= 0.0000 +/- 0.0000 | g_re= 0.0000 +/- 0.0000 |
g_im= 0.1283 +/- 0.0046 | g_im= 0.0000 +/- 0.0000 | g_im= 0.0249 +/- 0.0075 |
corr= [-1.00] | corr= [ 0.00] | corr= [-0.33] |
-----
Br = 0.0000 +/- 0.0000 | Br = 0.0000 +/- 0.0000 | Br = 0.0000 +/- 0.0000 |

--
pi:omega[-] pi:phi[+] upper half-plane

sqrt(s)_pole = (0.24491 +/- 0.00068209)
+ (i/2)*(+0.008034 +/- 0.00099896) [-0.49]

s_pole = (0.059965 +/- 0.0003361)
+ i*(+0.0019676 +/- 0.000242) [-0.49]

```



| pi:omega                 | pi:phi                  |
|--------------------------|-------------------------|
| ===== =====              | ===== =====             |
| k_re= -0.0460 +/- 0.0008 | k_re= 0.0092 +/- 0.0008 |
| k_im= -0.0048 +/- 0.0006 | k_im= 0.0212 +/- 0.0016 |
| corr= [-0.53]            | corr= [ 0.08]           |

| pi:omega/3^S_1(*)            | pi:phi/3^S_1                 | pi:omega/3^D_1               |
|------------------------------|------------------------------|------------------------------|
| ===== ===== =====            | ===== ===== =====            | ===== ===== =====            |
| g = 0.0656 +/- 0.0038        | g = 0.0000 +/- 0.0000        | g = 0.0082 +/- 0.0026        |
| arg(g)/pi= 0.1270 +/- 0.0174 | arg(g)/pi= 0.3730 +/- 0.0174 | arg(g)/pi= 0.7207 +/- 0.0193 |
| ----- ----- -----            | ----- ----- -----            | ----- ----- -----            |
| g_re= 0.0604 +/- 0.0042      | g_re= 0.0000 +/- 0.0000      | g_re= -0.0053 +/- 0.0019     |
| g_im= 0.0255 +/- 0.0032      | g_im= 0.0000 +/- 0.0000      | g_im= 0.0063 +/- 0.0019      |
| corr= [-0.18]                | corr= [ 0.27]                | corr= [-0.94]                |
| ----- ----- -----            | ----- ----- -----            | ----- ----- -----            |
| Br = 0.8178 +/- 0.0146       | Br = 0.0000 +/- 0.0000       | Br = 0.0129 +/- 0.0082       |

--

pi:omega[-] pi:phi[+] lower half-plane

```
sqrt(s)_pole = (0.24491 +/- 0.00068209)
               + (i/2)*(-0.008034 +/- 0.00099896) [ 0.49]
```

```
s_pole = (0.059965 +/- 0.0003361)
          + i*(-0.0019676 +/- 0.000242) [ 0.49]
```

| pi:omega                 | pi:phi                   |
|--------------------------|--------------------------|
| ===== =====              | ===== =====              |
| k_re= 0.0460 +/- 0.0008  | k_re= -0.0092 +/- 0.0008 |
| k_im= -0.0048 +/- 0.0006 | k_im= 0.0212 +/- 0.0016  |
| corr= [ 0.53]            | corr= [-0.08]            |

| pi:omega/3^S_1(*)             | pi:phi/3^S_1                 | pi:omega/3^D_1                |
|-------------------------------|------------------------------|-------------------------------|
| ===== ===== =====             | ===== ===== =====            | ===== ===== =====             |
| g = 0.0656 +/- 0.0038         | g = 0.0000 +/- 0.0000        | g = 0.0082 +/- 0.0026         |
| arg(g)/pi= -0.1270 +/- 0.0174 | arg(g)/pi= 0.6270 +/- 0.0174 | arg(g)/pi= -0.7207 +/- 0.0193 |
| ----- ----- -----             | ----- ----- -----            | ----- ----- -----             |
| g_re= 0.0604 +/- 0.0042       | g_re= -0.0000 +/- 0.0000     | g_re= -0.0053 +/- 0.0019      |
| g_im= -0.0255 +/- 0.0032      | g_im= 0.0000 +/- 0.0000      | g_im= -0.0063 +/- 0.0019      |
| corr= [ 0.18]                 | corr= [-0.27]                | corr= [ 0.94]                 |
| ----- ----- -----             | ----- ----- -----            | ----- ----- -----             |
| Br = 0.8178 +/- 0.0146        | Br = 0.0000 +/- 0.0000       | Br = 0.0129 +/- 0.0082        |

--

pi:omega[-] pi:phi[-] lower half-plane

```
sqrt(s)_pole = (0.19527 +/- 0.0022187)
               + (i/2)*(-1.6902e-15 +/- 8.4839e-13) [ 0.00]
```

```
s_pole = (0.038131 +/- 0.00086647)
          + i*(-3.2993e-16 +/- 1.6561e-13) [ 0.00]
```

| pi:omega                 | pi:phi                   |
|--------------------------|--------------------------|
| ===== =====              | ===== =====              |
| k_re= 0.0000 +/- 0.0000  | k_re= 0.0000 +/- 0.0000  |
| k_im= -0.0496 +/- 0.0016 | k_im= -0.0634 +/- 0.0008 |
| corr= [ 0.00]            | corr= [ 0.00]            |

| pi:omega/3^S_1(*)            | pi:phi/3^S_1                 | pi:omega/3^D_1               |
|------------------------------|------------------------------|------------------------------|
| ===== ===== =====            | ===== ===== =====            | ===== ===== =====            |
| g = 0.1283 +/- 0.0046        | g = 0.0000 +/- 0.0000        | g = 0.0249 +/- 0.0075        |
| arg(g)/pi= 0.5000 +/- 0.0000 | arg(g)/pi= 0.0000 +/- 0.0000 | arg(g)/pi= 0.5000 +/- 0.0000 |



## 2 Unphysical Parameterizations

```

-----|-----|-----|
g_re= 0.0000 +/- 0.0000 | g_re= 0.0000 +/- 0.0000 | g_re= 0.0000 +/- 0.0000 |
g_im= 0.1283 +/- 0.0046 | g_im= 0.0000 +/- 0.0000 | g_im= 0.0249 +/- 0.0075 |
corr= [-1.00] | corr= [ 0.00] | corr= [-0.33] |
-----|-----|-----|
Br = 0.0000 +/- 0.0000 | Br = 0.0000 +/- 0.0000 | Br = 0.0000 +/- 0.0000 |

--
pi:omega[-] pi:phi[-] upper half-plane

sqrt(s)_pole = (0.24491 +/- 0.00068209)
               + (i/2)*(+0.008034 +/- 0.00099896) [-0.49]

s_pole = (0.059965 +/- 0.0003361)
         + i*(+0.0019676 +/- 0.000242) [-0.49]

=====|=====|
pi:omega | pi:phi |
=====|=====|
k_re= -0.0460 +/- 0.0008 | k_re= -0.0092 +/- 0.0008 |
k_im= -0.0048 +/- 0.0006 | k_im= -0.0212 +/- 0.0016 |
corr= [-0.53] | corr= [ 0.08] |

=====|=====|
pi:omega/3^S_1(*) | pi:phi/3^S_1 | pi:omega/3^D_1 |
=====|=====|
|g|= 0.0656 +/- 0.0038 | |g|= 0.0000 +/- 0.0000 | |g|= 0.0082 +/- 0.0026 |
arg(g)/pi= 0.1270 +/- 0.0174 | arg(g)/pi= 0.3730 +/- 0.0174 | arg(g)/pi= 0.7207 +/- 0.0193 |
-----|-----|-----|
g_re= 0.0604 +/- 0.0042 | g_re= 0.0000 +/- 0.0000 | g_re= -0.0053 +/- 0.0019 |
g_im= 0.0255 +/- 0.0032 | g_im= 0.0000 +/- 0.0000 | g_im= 0.0063 +/- 0.0019 |
corr= [-0.18] | corr= [ 0.27] | corr= [-0.94] |
-----|-----|-----|
Br = 0.8178 +/- 0.0146 | Br = 0.0000 +/- 0.0000 | Br = 0.0129 +/- 0.0082 |

--
pi:omega[-] pi:phi[-] lower half-plane

sqrt(s)_pole = (0.24491 +/- 0.00068209)
               + (i/2)*(-0.008034 +/- 0.00099896) [ 0.49]

s_pole = (0.059965 +/- 0.0003361)
         + i*(-0.0019676 +/- 0.000242) [ 0.49]

=====|=====|
pi:omega | pi:phi |
=====|=====|
k_re= 0.0460 +/- 0.0008 | k_re= 0.0092 +/- 0.0008 |
k_im= -0.0048 +/- 0.0006 | k_im= -0.0212 +/- 0.0016 |
corr= [ 0.53] | corr= [-0.08] |

=====|=====|
pi:omega/3^S_1(*) | pi:phi/3^S_1 | pi:omega/3^D_1 |
=====|=====|
|g|= 0.0656 +/- 0.0038 | |g|= 0.0000 +/- 0.0000 | |g|= 0.0082 +/- 0.0026 |
arg(g)/pi= -0.1270 +/- 0.0174 | arg(g)/pi= 0.6270 +/- 0.0174 | arg(g)/pi= -0.7207 +/- 0.0193 |
-----|-----|-----|
g_re= 0.0604 +/- 0.0042 | g_re= -0.0000 +/- 0.0000 | g_re= -0.0053 +/- 0.0019 |
g_im= -0.0255 +/- 0.0032 | g_im= 0.0000 +/- 0.0000 | g_im= -0.0063 +/- 0.0019 |
corr= [ 0.18] | corr= [-0.27] | corr= [ 0.94] |
-----|-----|-----|
Br = 0.8178 +/- 0.0146 | Br = 0.0000 +/- 0.0000 | Br = 0.0129 +/- 0.0082 |

```



## 2.16 coupled\_po\_pp.3s1\_3d1.pole+G0\_3s1\_3sd1\_3S1+G1\_3s1.gorder0\_3s1.pole0\_sub

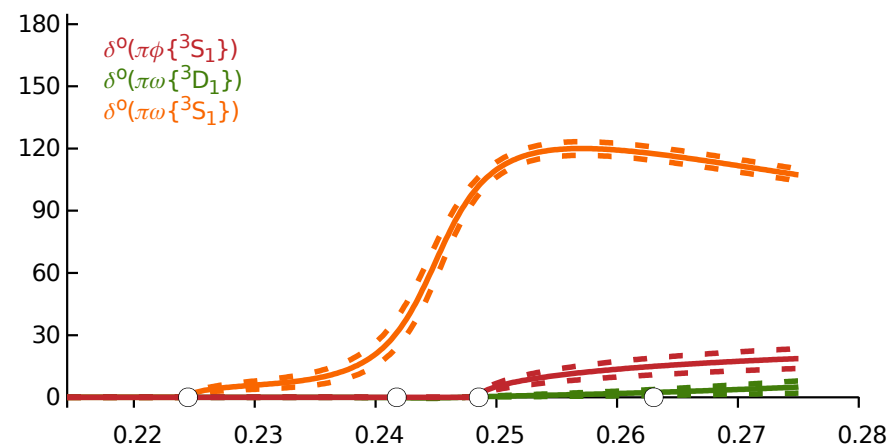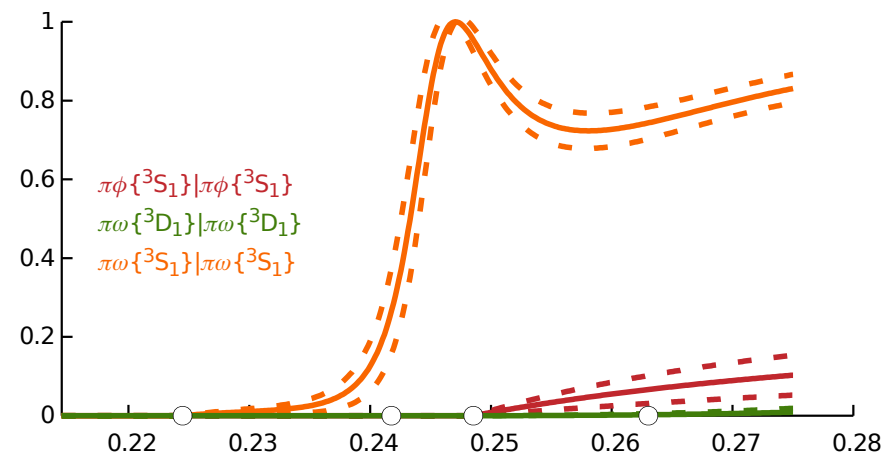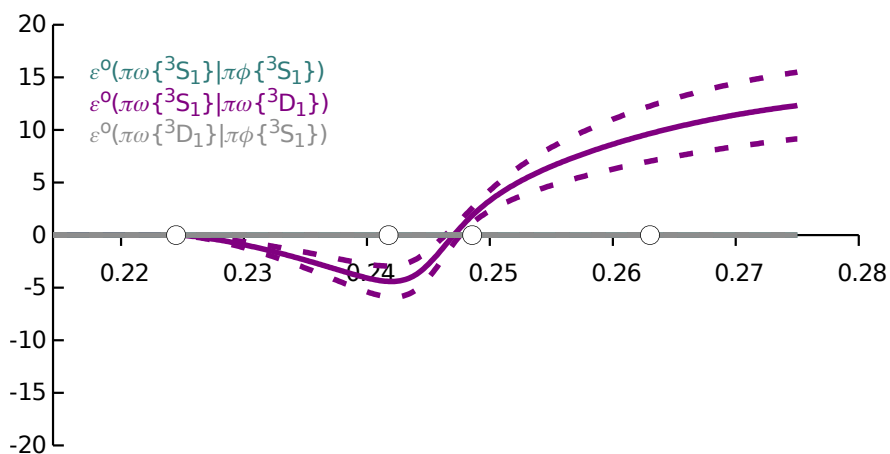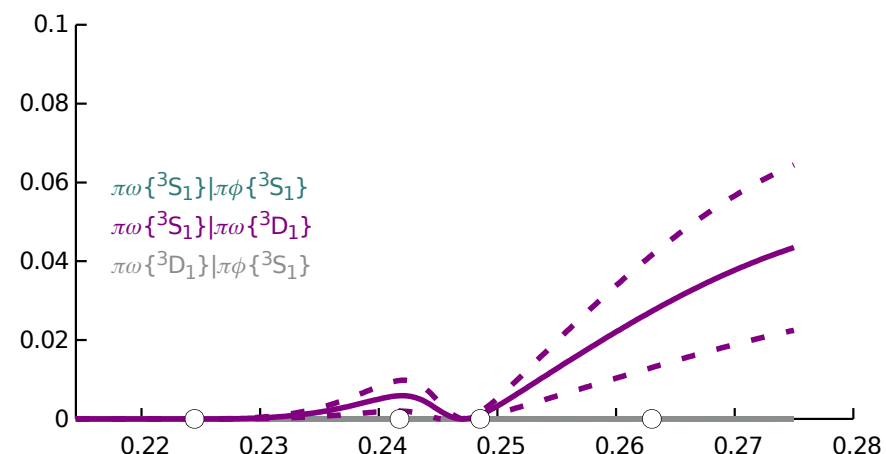



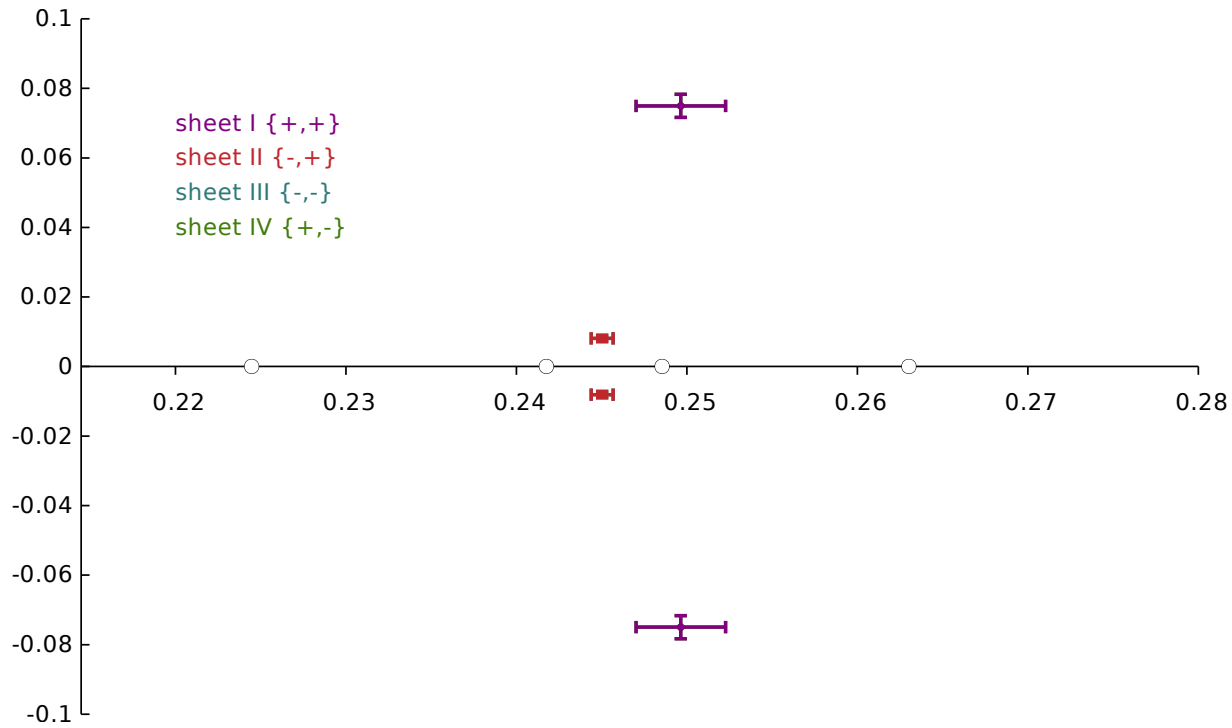

### parameter values

minimised with  $\text{chisq}/\text{nDoF} = 33.21 / (36 - 6) = 1.11$

|                                               |  |                        |  |      |       |       |       |       |       |
|-----------------------------------------------|--|------------------------|--|------|-------|-------|-------|-------|-------|
| JP1+_g_pi:omega/3~S_1 pole0                   |  | 0.083242 +/- 0.005384  |  | 1.00 | -0.29 | -0.19 | -0.05 | -0.01 | -0.03 |
| JP1+_gamma_pi:omega/3~S_1 pi:omega/3~D_1_orde |  | -35.507 +/- 11.415     |  |      | 1.00  | -0.10 | 0.30  | -0.12 | -0.16 |
| JP1+_gamma_pi:omega/3~S_1 pi:omega/3~S_1_orde |  | 5.7021 +/- 0.38676     |  |      |       | 1.00  | -0.90 | 0.02  | 0.00  |
| JP1+_gamma_pi:omega/3~S_1 pi:omega/3~S_1_orde |  | -114.60 +/- 7.7        |  |      |       |       | 1.00  | 0.04  | -0.04 |
| JP1+_gamma_pi:phi/3~S_1 pi:phi/3~S_1_order0   |  | 0.87101 +/- 0.24492    |  |      |       |       |       | 1.00  | -0.17 |
| JP1+_m_pole0                                  |  | 0.24707 +/- 0.00057888 |  |      |       |       |       |       | 1.00  |

### pole singularities

pi:omega[+] pi:phi[+] upper half-plane

$\sqrt{s}_{\text{pole}} = (0.24964 \pm 0.0026251)$   
 $+ (i/2)*(+0.074951 \pm 0.0033179) [0.61]$

$s_{\text{pole}} = (0.060917 \pm 0.001239)$   
 $+ i*(+0.018711 \pm 0.00096071) [0.67]$

| pi:omega                | pi:phi                  |
|-------------------------|-------------------------|
| ===== =====             |                         |
| k_re= 0.0589 +/- 0.0024 | k_re= 0.0412 +/- 0.0025 |
| k_im= 0.0360 +/- 0.0010 | k_im= 0.0462 +/- 0.0011 |
| corr= [0.21]            | corr= [-0.22]           |



| pi:omega/3^S_1(*)                                                    | pi:phi/3^S_1                                                         | pi:omega/3^D_1                                                       |
|----------------------------------------------------------------------|----------------------------------------------------------------------|----------------------------------------------------------------------|
| g = 0.1651 +/- 0.0050<br>arg(g)/pi= -0.2077 +/- 0.0033               | g = 0.0000 +/- 0.0000<br>arg(g)/pi= 0.7077 +/- 0.0033                | g = 0.0472 +/- 0.0107<br>arg(g)/pi= -0.1671 +/- 0.0151               |
| g_re= 0.1312 +/- 0.0038<br>g_im= -0.1003 +/- 0.0037<br>corr= [-0.81] | g_re= -0.0000 +/- 0.0000<br>g_im= 0.0000 +/- 0.0000<br>corr= [-0.77] | g_re= 0.0408 +/- 0.0096<br>g_im= -0.0236 +/- 0.0052<br>corr= [-0.89] |
| Br = 0.5968 +/- 0.0224                                               | Br = 0.0000 +/- 0.0000                                               | Br = 0.0487 +/- 0.0236                                               |

--

pi:omega[+] pi:phi[+] lower half-plane

sqrt(s)\_pole = (0.24964 +/- 0.0026251)  
+ (i/2)\*(-0.074951 +/- 0.0033179) [-0.61]

s\_pole = (0.060917 +/- 0.001239)  
+ i\*(-0.018711 +/- 0.00096071) [-0.67]

| pi:omega                                                             | pi:phi                                                               |
|----------------------------------------------------------------------|----------------------------------------------------------------------|
| k_re= -0.0589 +/- 0.0024<br>k_im= 0.0360 +/- 0.0010<br>corr= [-0.21] | k_re= -0.0412 +/- 0.0025<br>k_im= 0.0462 +/- 0.0011<br>corr= [ 0.22] |

| pi:omega/3^S_1(*)                                                   | pi:phi/3^S_1                                                        | pi:omega/3^D_1                                                      |
|---------------------------------------------------------------------|---------------------------------------------------------------------|---------------------------------------------------------------------|
| g = 0.1651 +/- 0.0050<br>arg(g)/pi= 0.2077 +/- 0.0033               | g = 0.0000 +/- 0.0000<br>arg(g)/pi= 0.2923 +/- 0.0033               | g = 0.0472 +/- 0.0107<br>arg(g)/pi= 0.1671 +/- 0.0151               |
| g_re= 0.1312 +/- 0.0038<br>g_im= 0.1003 +/- 0.0037<br>corr= [ 0.81] | g_re= 0.0000 +/- 0.0000<br>g_im= 0.0000 +/- 0.0000<br>corr= [ 0.77] | g_re= 0.0408 +/- 0.0096<br>g_im= 0.0236 +/- 0.0052<br>corr= [ 0.89] |
| Br = 0.5968 +/- 0.0224                                              | Br = 0.0000 +/- 0.0000                                              | Br = 0.0487 +/- 0.0236                                              |

--

pi:omega[+] pi:phi[-] upper half-plane

sqrt(s)\_pole = (0.24964 +/- 0.0026251)  
+ (i/2)\*(+0.074951 +/- 0.0033179) [ 0.61]

s\_pole = (0.060917 +/- 0.001239)  
+ i\*(+0.018711 +/- 0.00096071) [ 0.67]

| pi:omega                                                            | pi:phi                                                                |
|---------------------------------------------------------------------|-----------------------------------------------------------------------|
| k_re= 0.0589 +/- 0.0024<br>k_im= 0.0360 +/- 0.0010<br>corr= [ 0.21] | k_re= -0.0412 +/- 0.0025<br>k_im= -0.0462 +/- 0.0011<br>corr= [-0.22] |

| pi:omega/3^S_1(*)                                                    | pi:phi/3^S_1                                                         | pi:omega/3^D_1                                                       |
|----------------------------------------------------------------------|----------------------------------------------------------------------|----------------------------------------------------------------------|
| g = 0.1651 +/- 0.0050<br>arg(g)/pi= -0.2077 +/- 0.0033               | g = 0.0000 +/- 0.0000<br>arg(g)/pi= 0.7077 +/- 0.0033                | g = 0.0472 +/- 0.0107<br>arg(g)/pi= -0.1671 +/- 0.0151               |
| g_re= 0.1312 +/- 0.0038<br>g_im= -0.1003 +/- 0.0037<br>corr= [-0.81] | g_re= -0.0000 +/- 0.0000<br>g_im= 0.0000 +/- 0.0000<br>corr= [-0.77] | g_re= 0.0408 +/- 0.0096<br>g_im= -0.0236 +/- 0.0052<br>corr= [-0.89] |



## 2 Unphysical Parameterizations

```

Br = 0.5968 +/- 0.0224 | Br = 0.0000 +/- 0.0000 | Br = 0.0487 +/- 0.0236 |

--
pi:omega[+] pi:phi[-] lower half-plane

sqrt(s)_pole = (0.24964 +/- 0.0026251)
+ (i/2)*(-0.074951 +/- 0.0033179) [-0.61]

s_pole = (0.060917 +/- 0.001239)
+ i*(-0.018711 +/- 0.00096071) [-0.67]

=====
pi:omega | pi:phi |
=====
k_re= -0.0589 +/- 0.0024 | k_re= 0.0412 +/- 0.0025 |
k_im= 0.0360 +/- 0.0010 | k_im= -0.0462 +/- 0.0011 |
corr= [-0.21] | corr= [ 0.22] |

=====
pi:omega/3^S_1(*) | pi:phi/3^S_1 | pi:omega/3^D_1 |
=====
|g|= 0.1651 +/- 0.0050 | |g|= 0.0000 +/- 0.0000 | |g|= 0.0472 +/- 0.0107 |
arg(g)/pi= 0.2077 +/- 0.0033 | arg(g)/pi= 0.2923 +/- 0.0033 | arg(g)/pi= 0.1671 +/- 0.0151 |
-----
g_re= 0.1312 +/- 0.0038 | g_re= 0.0000 +/- 0.0000 | g_re= 0.0408 +/- 0.0096 |
g_im= 0.1003 +/- 0.0037 | g_im= 0.0000 +/- 0.0000 | g_im= 0.0236 +/- 0.0052 |
corr= [ 0.81] | corr= [ 0.77] | corr= [ 0.89] |
-----
Br = 0.5968 +/- 0.0224 | Br = 0.0000 +/- 0.0000 | Br = 0.0487 +/- 0.0236 |

--
pi:omega[-] pi:phi[+] lower half-plane

sqrt(s)_pole = (0.20065 +/- 0.0017539)
+ (i/2)*(-3.9663e-16 +/- 2.2217e-13) [ 0.00]

s_pole = (0.040262 +/- 0.00070385)
+ i*(-7.9551e-17 +/- 4.4562e-14) [ 0.00]

=====
pi:omega | pi:phi |
=====
k_re= 0.0000 +/- 0.0000 | k_re= -0.0000 +/- 0.0000 |
k_im= -0.0454 +/- 0.0015 | k_im= 0.0612 +/- 0.0008 |
corr= [ 0.00] | corr= [ 0.00] |

=====
pi:omega/3^S_1(*) | pi:phi/3^S_1 | pi:omega/3^D_1 |
=====
|g|= 0.1044 +/- 0.0044 | |g|= 0.0000 +/- 0.0000 | |g|= 0.0207 +/- 0.0063 |
arg(g)/pi= 0.5000 +/- 0.0000 | arg(g)/pi= 0.0000 +/- 0.0000 | arg(g)/pi= 0.5000 +/- 0.0000 |
-----
g_re= 0.0000 +/- 0.0000 | g_re= 0.0000 +/- 0.0000 | g_re= 0.0000 +/- 0.0000 |
g_im= 0.1044 +/- 0.0044 | g_im= 0.0000 +/- 0.0000 | g_im= 0.0207 +/- 0.0063 |
corr= [-1.00] | corr= [ 0.00] | corr= [-0.14] |
-----
Br = 0.0000 +/- 0.0000 | Br = 0.0000 +/- 0.0000 | Br = 0.0000 +/- 0.0000 |

--
pi:omega[-] pi:phi[+] upper half-plane

sqrt(s)_pole = (0.24503 +/- 0.00064036)
+ (i/2)*(+0.0080887 +/- 0.00091058) [-0.46]

s_pole = (0.060022 +/- 0.00031553)
+ i*(+0.0019819 +/- 0.00022076) [-0.45]

```



| pi:omega                 | pi:phi                  |
|--------------------------|-------------------------|
| =====                    | =====                   |
| k_re= -0.0462 +/- 0.0007 | k_re= 0.0093 +/- 0.0008 |
| k_im= -0.0048 +/- 0.0006 | k_im= 0.0210 +/- 0.0015 |
| corr= [-0.50]            | corr= [ 0.01]           |

| pi:omega/3^S_1(*)            | pi:phi/3^S_1                 | pi:omega/3^D_1               |
|------------------------------|------------------------------|------------------------------|
| =====                        | =====                        | =====                        |
| g = 0.0657 +/- 0.0034        | g = 0.0000 +/- 0.0000        | g = 0.0080 +/- 0.0025        |
| arg(g)/pi= 0.1207 +/- 0.0155 | arg(g)/pi= 0.3793 +/- 0.0155 | arg(g)/pi= 0.7201 +/- 0.0190 |
| -----                        | -----                        | -----                        |
| g_re= 0.0610 +/- 0.0036      | g_re= 0.0000 +/- 0.0000      | g_re= -0.0051 +/- 0.0018     |
| g_im= 0.0243 +/- 0.0029      | g_im= 0.0000 +/- 0.0000      | g_im= 0.0061 +/- 0.0018      |
| corr= [-0.15]                | corr= [ 0.23]                | corr= [-0.94]                |
| -----                        | -----                        | -----                        |
| Br = 0.8176 +/- 0.0150       | Br = 0.0000 +/- 0.0000       | Br = 0.0121 +/- 0.0076       |

--

pi:omega[-] pi:phi[+] lower half-plane

sqrt(s)\_pole = (0.24503 +/- 0.00064036)  
+ (i/2)\*(-0.0080887 +/- 0.00091058) [ 0.46]

s\_pole = (0.060022 +/- 0.00031553)  
+ i\*(-0.0019819 +/- 0.00022076) [ 0.45]

| pi:omega                 | pi:phi                   |
|--------------------------|--------------------------|
| =====                    | =====                    |
| k_re= 0.0462 +/- 0.0007  | k_re= -0.0093 +/- 0.0008 |
| k_im= -0.0048 +/- 0.0006 | k_im= 0.0210 +/- 0.0015  |
| corr= [ 0.50]            | corr= [-0.01]            |

| pi:omega/3^S_1(*)             | pi:phi/3^S_1                 | pi:omega/3^D_1                |
|-------------------------------|------------------------------|-------------------------------|
| =====                         | =====                        | =====                         |
| g = 0.0657 +/- 0.0034         | g = 0.0000 +/- 0.0000        | g = 0.0080 +/- 0.0025         |
| arg(g)/pi= -0.1207 +/- 0.0155 | arg(g)/pi= 0.6207 +/- 0.0155 | arg(g)/pi= -0.7201 +/- 0.0190 |
| -----                         | -----                        | -----                         |
| g_re= 0.0610 +/- 0.0036       | g_re= -0.0000 +/- 0.0000     | g_re= -0.0051 +/- 0.0018      |
| g_im= -0.0243 +/- 0.0029      | g_im= 0.0000 +/- 0.0000      | g_im= -0.0061 +/- 0.0018      |
| corr= [ 0.15]                 | corr= [-0.23]                | corr= [ 0.94]                 |
| -----                         | -----                        | -----                         |
| Br = 0.8176 +/- 0.0150        | Br = 0.0000 +/- 0.0000       | Br = 0.0121 +/- 0.0076        |

--

pi:omega[-] pi:phi[-] lower half-plane

sqrt(s)\_pole = (0.20065 +/- 0.0017539)  
+ (i/2)\*(-1.4992e-17 +/- 3.7668e-14) [ 0.00]

s\_pole = (0.040262 +/- 0.00070385)  
+ i\*(-3.0056e-18 +/- 7.5616e-15) [ 0.00]

| pi:omega                 | pi:phi                   |
|--------------------------|--------------------------|
| =====                    | =====                    |
| k_re= 0.0000 +/- 0.0000  | k_re= 0.0000 +/- 0.0000  |
| k_im= -0.0454 +/- 0.0015 | k_im= -0.0612 +/- 0.0008 |
| corr= [ 0.00]            | corr= [ 0.00]            |

| pi:omega/3^S_1(*)            | pi:phi/3^S_1                 | pi:omega/3^D_1               |
|------------------------------|------------------------------|------------------------------|
| =====                        | =====                        | =====                        |
| g = 0.1044 +/- 0.0044        | g = 0.0000 +/- 0.0000        | g = 0.0207 +/- 0.0063        |
| arg(g)/pi= 0.5000 +/- 0.0000 | arg(g)/pi= 0.0000 +/- 0.0000 | arg(g)/pi= 0.5000 +/- 0.0000 |



## 2 Unphysical Parameterizations

```

-----|-----|-----|
g_re=  0.0000 +/- 0.0000 | g_re=  0.0000 +/- 0.0000 | g_re=  0.0000 +/- 0.0000 |
g_im=  0.1044 +/- 0.0044 | g_im=  0.0000 +/- 0.0000 | g_im=  0.0207 +/- 0.0063 |
corr= [-1.00]           | corr= [ 0.00]           | corr= [-0.14]           |
-----|-----|-----|
Br =  0.0000 +/- 0.0000 | Br =  0.0000 +/- 0.0000 | Br =  0.0000 +/- 0.0000 |

--
pi:omega[-] pi:phi[-] upper half-plane

sqrt(s)_pole = (0.24503 +/- 0.00064036)
               + (i/2)*(+0.0080887 +/- 0.00091058) [-0.46]

s_pole = (0.060022 +/- 0.00031553)
         + i*(+0.0019819 +/- 0.00022076) [-0.45]

=====|=====|
pi:omega | pi:phi |
=====|=====|
k_re= -0.0462 +/- 0.0007 | k_re= -0.0093 +/- 0.0008 |
k_im= -0.0048 +/- 0.0006 | k_im= -0.0210 +/- 0.0015 |
corr= [-0.50]           | corr= [ 0.01]           |

=====|=====|
pi:omega/3^S_1(*) | pi:phi/3^S_1 | pi:omega/3^D_1 |
=====|=====|=====|
|g|=  0.0657 +/- 0.0034 | |g|=  0.0000 +/- 0.0000 | |g|=  0.0080 +/- 0.0025 |
arg(g)/pi= 0.1207 +/- 0.0155 | arg(g)/pi= 0.3793 +/- 0.0155 | arg(g)/pi= 0.7201 +/- 0.0190 |
-----|-----|-----|
g_re=  0.0610 +/- 0.0036 | g_re=  0.0000 +/- 0.0000 | g_re= -0.0051 +/- 0.0018 |
g_im=  0.0243 +/- 0.0029 | g_im=  0.0000 +/- 0.0000 | g_im=  0.0061 +/- 0.0018 |
corr= [-0.15]           | corr= [ 0.23]           | corr= [-0.94]           |
-----|-----|-----|
Br =  0.8176 +/- 0.0150 | Br =  0.0000 +/- 0.0000 | Br =  0.0121 +/- 0.0076 |

--
pi:omega[-] pi:phi[-] lower half-plane

sqrt(s)_pole = (0.24503 +/- 0.00064036)
               + (i/2)*(-0.0080887 +/- 0.00091058) [ 0.46]

s_pole = (0.060022 +/- 0.00031553)
         + i*(-0.0019819 +/- 0.00022076) [ 0.45]

=====|=====|
pi:omega | pi:phi |
=====|=====|
k_re=  0.0462 +/- 0.0007 | k_re=  0.0093 +/- 0.0008 |
k_im= -0.0048 +/- 0.0006 | k_im= -0.0210 +/- 0.0015 |
corr= [ 0.50]           | corr= [-0.01]           |

=====|=====|
pi:omega/3^S_1(*) | pi:phi/3^S_1 | pi:omega/3^D_1 |
=====|=====|=====|
|g|=  0.0657 +/- 0.0034 | |g|=  0.0000 +/- 0.0000 | |g|=  0.0080 +/- 0.0025 |
arg(g)/pi= -0.1207 +/- 0.0155 | arg(g)/pi= 0.6207 +/- 0.0155 | arg(g)/pi= -0.7201 +/- 0.0190 |
-----|-----|-----|
g_re=  0.0610 +/- 0.0036 | g_re= -0.0000 +/- 0.0000 | g_re= -0.0051 +/- 0.0018 |
g_im= -0.0243 +/- 0.0029 | g_im=  0.0000 +/- 0.0000 | g_im= -0.0061 +/- 0.0018 |
corr= [ 0.15]           | corr= [-0.23]           | corr= [ 0.94]           |
-----|-----|-----|
Br =  0.8176 +/- 0.0150 | Br =  0.0000 +/- 0.0000 | Br =  0.0121 +/- 0.0076 |

```



## 2.17 coupled\_po\_pp.3s1\_3d1.pole+G0\_3s1\_3sd1\_3S1+G1\_3s1.gorder0\_3s1.threshold\_sub

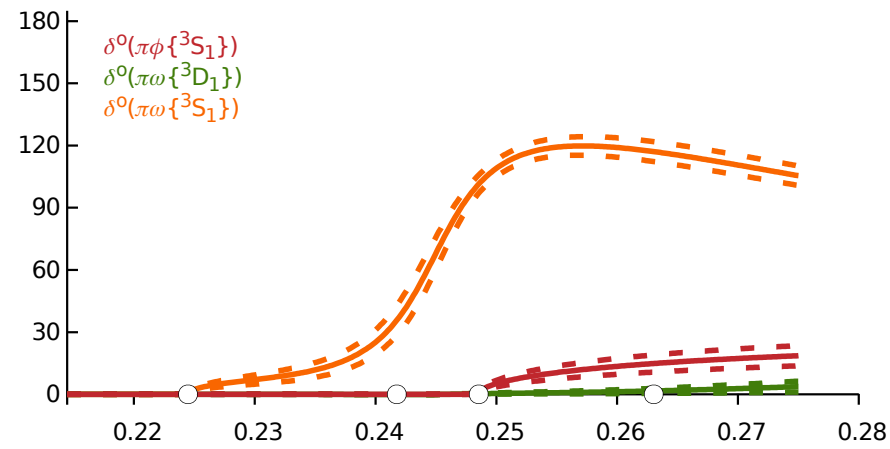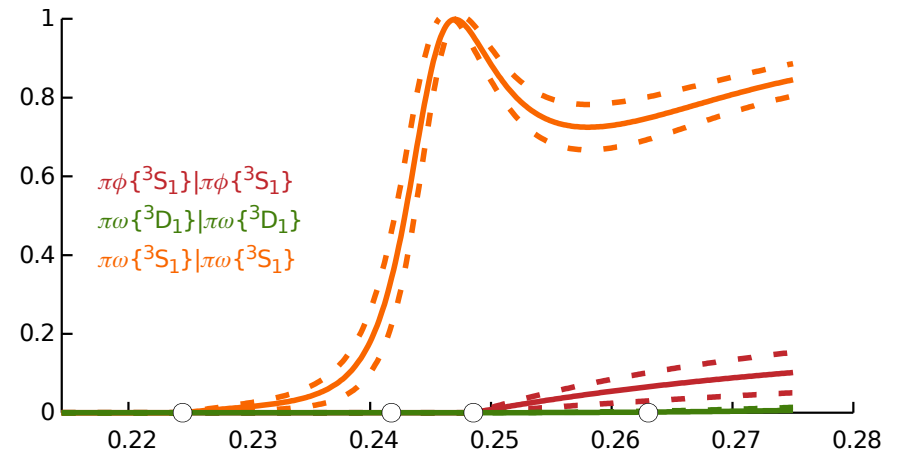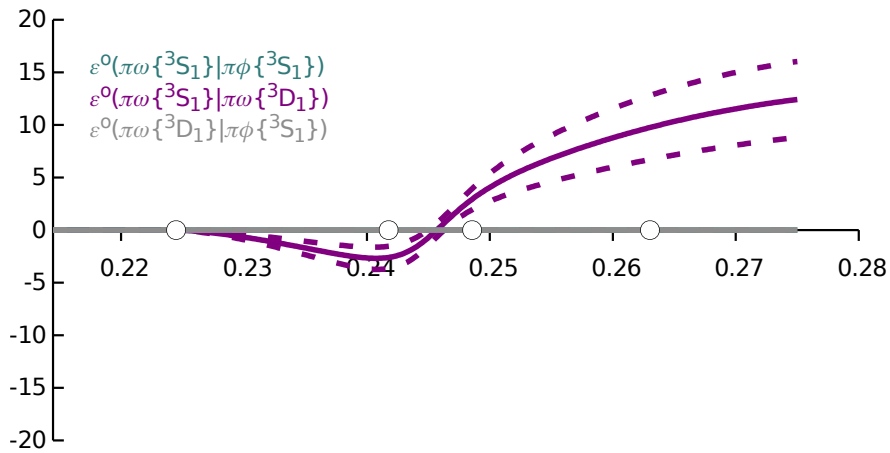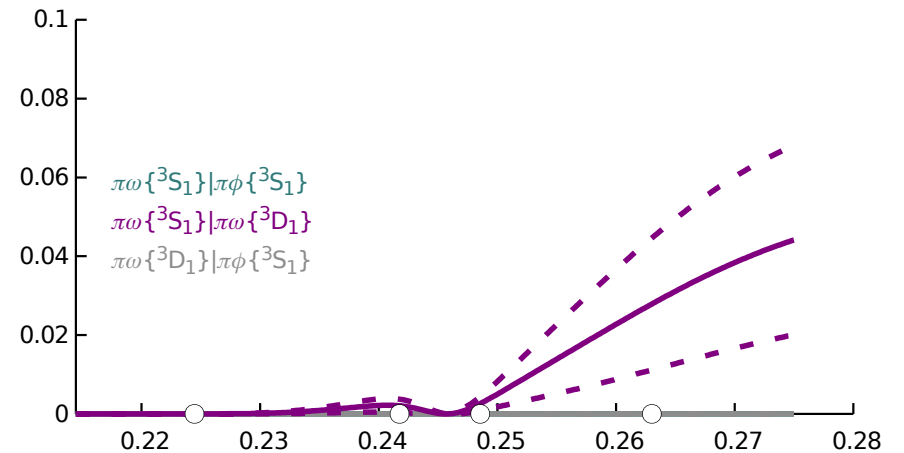



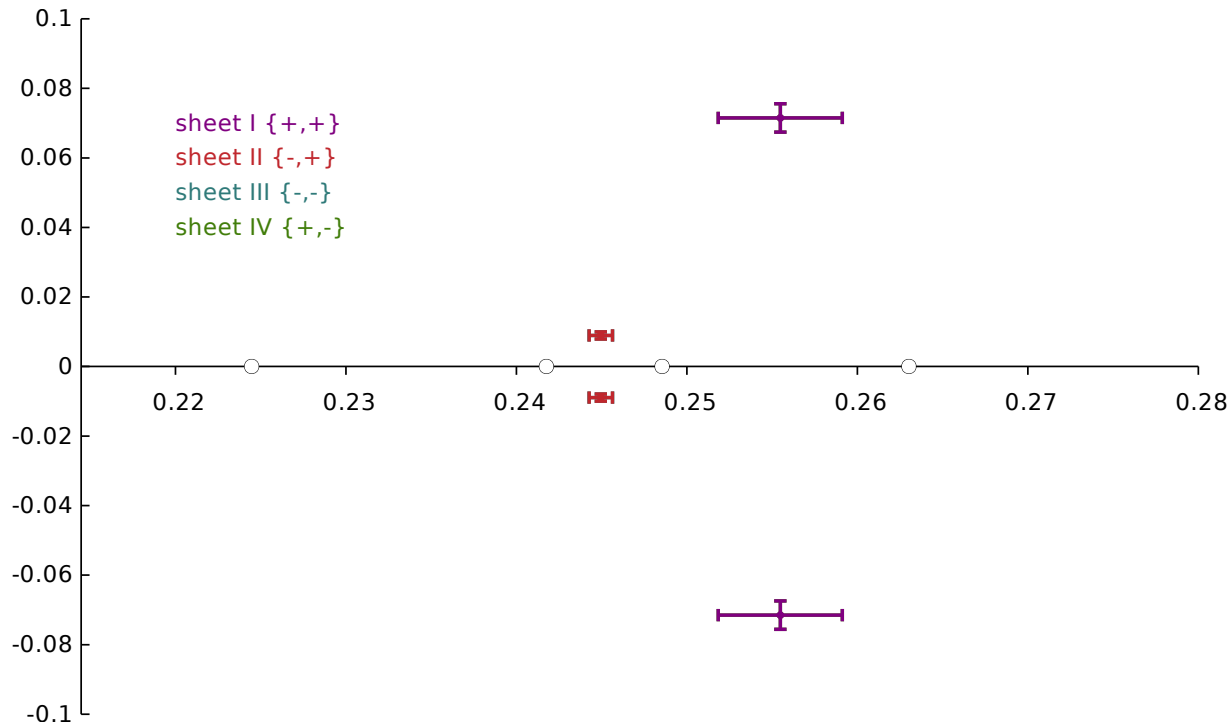

### parameter values

minimised with  $\text{chisq}/\text{nDoF} = 33.27 / (36 - 6) = 1.11$

|                                               |  |                        |  |      |       |       |       |       |       |
|-----------------------------------------------|--|------------------------|--|------|-------|-------|-------|-------|-------|
| JP1+_g_pi:omega/3~S_1_pole0                   |  | 0.077806 +/- 0.004737  |  | 1.00 | -0.26 | -0.26 | 0.18  | 0.10  | -0.42 |
| JP1+_gamma_pi:omega/3~S_1 pi:omega/3~D_1_orde |  | -27.448 +/- 10.267     |  |      | 1.00  | -0.09 | 0.31  | -0.06 | -0.06 |
| JP1+_gamma_pi:omega/3~S_1 pi:omega/3~S_1_orde |  | 4.6168 +/- 0.42057     |  |      |       | 1.00  | -0.92 | 0.01  | 0.07  |
| JP1+_gamma_pi:omega/3~S_1 pi:omega/3~S_1_orde |  | -90.723 +/- 8.0628     |  |      |       |       | 1.00  | 0.06  | -0.07 |
| JP1+_gamma_pi:phi/3~S_1 pi:phi/3~S_1_order0   |  | 0.94195 +/- 0.29608    |  |      |       |       |       | 1.00  | -0.28 |
| JP1+_m_pole0                                  |  | 0.24568 +/- 0.00061896 |  |      |       |       |       |       | 1.00  |

### pole singularities

pi:omega[+] pi:phi[+] upper half-plane

$\sqrt{s}_{\text{pole}} = (0.25548 \pm 0.0036387)$   
 $+ (i/2)*(+0.071494 \pm 0.0041044)$  [ 0.69]

$s_{\text{pole}} = (0.063991 \pm 0.0017611)$   
 $+ i*(+0.018265 \pm 0.0012426)$  [ 0.75]

| pi:omega                | pi:phi                  |
|-------------------------|-------------------------|
| ===== =====             | ===== =====             |
| k_re= 0.0632 +/- 0.0033 | k_re= 0.0448 +/- 0.0035 |
| k_im= 0.0331 +/- 0.0012 | k_im= 0.0422 +/- 0.0013 |
| corr= [ 0.31]           | corr= [-0.21]           |



| pi:omega/3^S_1(*)                                                    | pi:phi/3^S_1                                                         | pi:omega/3^D_1                                                       |
|----------------------------------------------------------------------|----------------------------------------------------------------------|----------------------------------------------------------------------|
| g = 0.1573 +/- 0.0064<br>arg(g)/pi= -0.2482 +/- 0.0033               | g = 0.0000 +/- 0.0000<br>arg(g)/pi= 0.7482 +/- 0.0033                | g = 0.0442 +/- 0.0113<br>arg(g)/pi= -0.2083 +/- 0.0168               |
| g_re= 0.1119 +/- 0.0044<br>g_im= -0.1106 +/- 0.0049<br>corr= [-0.88] | g_re= -0.0000 +/- 0.0000<br>g_im= 0.0000 +/- 0.0000<br>corr= [-0.88] | g_re= 0.0351 +/- 0.0095<br>g_im= -0.0269 +/- 0.0065<br>corr= [-0.92] |
| Br = 0.6069 +/- 0.0273                                               | Br = 0.0000 +/- 0.0000                                               | Br = 0.0480 +/- 0.0264                                               |

--

pi:omega[+] pi:phi[+] lower half-plane

sqrt(s)\_pole = (0.25548 +/- 0.0036387)  
+ (i/2)\*(-0.071494 +/- 0.0041044) [-0.69]

s\_pole = (0.063991 +/- 0.0017611)  
+ i\*(-0.018265 +/- 0.0012426) [-0.75]

| pi:omega                                                             | pi:phi                                                               |
|----------------------------------------------------------------------|----------------------------------------------------------------------|
| k_re= -0.0632 +/- 0.0033<br>k_im= 0.0331 +/- 0.0012<br>corr= [-0.31] | k_re= -0.0448 +/- 0.0035<br>k_im= 0.0422 +/- 0.0013<br>corr= [ 0.21] |

| pi:omega/3^S_1(*)                                                   | pi:phi/3^S_1                                                        | pi:omega/3^D_1                                                      |
|---------------------------------------------------------------------|---------------------------------------------------------------------|---------------------------------------------------------------------|
| g = 0.1573 +/- 0.0064<br>arg(g)/pi= 0.2482 +/- 0.0033               | g = 0.0000 +/- 0.0000<br>arg(g)/pi= 0.2518 +/- 0.0033               | g = 0.0442 +/- 0.0113<br>arg(g)/pi= 0.2083 +/- 0.0168               |
| g_re= 0.1119 +/- 0.0044<br>g_im= 0.1106 +/- 0.0049<br>corr= [ 0.88] | g_re= 0.0000 +/- 0.0000<br>g_im= 0.0000 +/- 0.0000<br>corr= [ 0.88] | g_re= 0.0351 +/- 0.0095<br>g_im= 0.0269 +/- 0.0065<br>corr= [ 0.92] |
| Br = 0.6069 +/- 0.0273                                              | Br = 0.0000 +/- 0.0000                                              | Br = 0.0480 +/- 0.0264                                              |

--

pi:omega[+] pi:phi[-] lower half-plane

sqrt(s)\_pole = (0.25548 +/- 0.0036387)  
+ (i/2)\*(-0.071494 +/- 0.0041044) [-0.69]

s\_pole = (0.063991 +/- 0.0017611)  
+ i\*(-0.018265 +/- 0.0012426) [-0.75]

| pi:omega                                                             | pi:phi                                                               |
|----------------------------------------------------------------------|----------------------------------------------------------------------|
| k_re= -0.0632 +/- 0.0033<br>k_im= 0.0331 +/- 0.0012<br>corr= [-0.31] | k_re= 0.0448 +/- 0.0035<br>k_im= -0.0422 +/- 0.0013<br>corr= [ 0.21] |

| pi:omega/3^S_1(*)                                                   | pi:phi/3^S_1                                                        | pi:omega/3^D_1                                                      |
|---------------------------------------------------------------------|---------------------------------------------------------------------|---------------------------------------------------------------------|
| g = 0.1573 +/- 0.0064<br>arg(g)/pi= 0.2482 +/- 0.0033               | g = 0.0000 +/- 0.0000<br>arg(g)/pi= 0.2518 +/- 0.0033               | g = 0.0442 +/- 0.0113<br>arg(g)/pi= 0.2083 +/- 0.0168               |
| g_re= 0.1119 +/- 0.0044<br>g_im= 0.1106 +/- 0.0049<br>corr= [ 0.88] | g_re= 0.0000 +/- 0.0000<br>g_im= 0.0000 +/- 0.0000<br>corr= [ 0.88] | g_re= 0.0351 +/- 0.0095<br>g_im= 0.0269 +/- 0.0065<br>corr= [ 0.92] |



## 2 Unphysical Parameterizations

```

Br = 0.6069 +/- 0.0273 | Br = 0.0000 +/- 0.0000 | Br = 0.0480 +/- 0.0264 |

--
pi:omega[+] pi:phi[-] upper half-plane

sqrt(s)_pole = (0.25548 +/- 0.0036387)
+ (i/2)*(+0.071494 +/- 0.0041044) [ 0.69]

s_pole = (0.063991 +/- 0.0017611)
+ i*(+0.018265 +/- 0.0012426) [ 0.75]

=====
pi:omega | pi:phi |
=====
k_re= 0.0632 +/- 0.0033 | k_re= -0.0448 +/- 0.0035 |
k_im= 0.0331 +/- 0.0012 | k_im= -0.0422 +/- 0.0013 |
corr= [ 0.31] | corr= [-0.21] |

=====
pi:omega/3^S_1(*) | pi:phi/3^S_1 | pi:omega/3^D_1 |
=====
|g|= 0.1573 +/- 0.0064 | |g|= 0.0000 +/- 0.0000 | |g|= 0.0442 +/- 0.0113 |
arg(g)/pi= -0.2482 +/- 0.0033 | arg(g)/pi= 0.7482 +/- 0.0033 | arg(g)/pi= -0.2083 +/- 0.0168 |
-----
g_re= 0.1119 +/- 0.0044 | g_re= -0.0000 +/- 0.0000 | g_re= 0.0351 +/- 0.0095 |
g_im= -0.1106 +/- 0.0049 | g_im= 0.0000 +/- 0.0000 | g_im= -0.0269 +/- 0.0065 |
corr= [-0.88] | corr= [-0.88] | corr= [-0.92] |
-----
Br = 0.6069 +/- 0.0273 | Br = 0.0000 +/- 0.0000 | Br = 0.0480 +/- 0.0264 |

--
pi:omega[-] pi:phi[+] upper half-plane

sqrt(s)_pole = (0.19471 +/- 0.0024271)
+ (i/2)*(+2.55e-17 +/- 3.1976e-14) [ 0.00]

s_pole = (0.037913 +/- 0.00094514)
+ i*(+4.9585e-18 +/- 6.2303e-15) [ 0.00]

=====
pi:omega | pi:phi |
=====
k_re= -0.0000 +/- 0.0000 | k_re= 0.0000 +/- 0.0000 |
k_im= -0.0501 +/- 0.0017 | k_im= 0.0636 +/- 0.0009 |
corr= [ 0.00] | corr= [ 0.00] |

=====
pi:omega/3^S_1(*) | pi:phi/3^S_1 | pi:omega/3^D_1 |
=====
|g|= 0.1120 +/- 0.0050 | |g|= 0.0000 +/- 0.0000 | |g|= 0.0206 +/- 0.0074 |
arg(g)/pi= 0.5000 +/- 0.0000 | arg(g)/pi= 0.0000 +/- 0.0000 | arg(g)/pi= 0.5000 +/- 0.0000 |
-----
g_re= 0.0000 +/- 0.0000 | g_re= 0.0000 +/- 0.0000 | g_re= 0.0000 +/- 0.0000 |
g_im= 0.1120 +/- 0.0050 | g_im= 0.0000 +/- 0.0000 | g_im= 0.0206 +/- 0.0074 |
corr= [-1.00] | corr= [ 0.00] | corr= [-0.17] |
-----
Br = 0.0000 +/- 0.0000 | Br = 0.0000 +/- 0.0000 | Br = 0.0000 +/- 0.0000 |

--
pi:omega[-] pi:phi[+] upper half-plane

sqrt(s)_pole = (0.24495 +/- 0.00068521)
+ (i/2)*(+0.008919 +/- 0.0010286) [-0.41]

s_pole = (0.059981 +/- 0.00033757)
+ i*(+0.0021847 +/- 0.00024954) [-0.40]

```



| pi:omega                 | pi:phi                  |
|--------------------------|-------------------------|
| =====                    | =====                   |
| k_re= -0.0461 +/- 0.0008 | k_re= 0.0100 +/- 0.0009 |
| k_im= -0.0053 +/- 0.0006 | k_im= 0.0215 +/- 0.0015 |
| corr= [-0.44]            | corr= [ 0.00]           |

| pi:omega/3^S_1(*)            | pi:phi/3^S_1                 | pi:omega/3^D_1               |
|------------------------------|------------------------------|------------------------------|
| =====                        | =====                        | =====                        |
| g = 0.0688 +/- 0.0037        | g = 0.0000 +/- 0.0000        | g = 0.0065 +/- 0.0024        |
| arg(g)/pi= 0.1101 +/- 0.0197 | arg(g)/pi= 0.3899 +/- 0.0197 | arg(g)/pi= 0.6377 +/- 0.0221 |
| -----                        | -----                        | -----                        |
| g_re= 0.0647 +/- 0.0043      | g_re= 0.0000 +/- 0.0000      | g_re= -0.0027 +/- 0.0013     |
| g_im= 0.0233 +/- 0.0037      | g_im= 0.0000 +/- 0.0000      | g_im= 0.0059 +/- 0.0020      |
| corr= [-0.38]                | corr= [ 0.23]                | corr= [-0.94]                |
| -----                        | -----                        | -----                        |
| Br = 0.8104 +/- 0.0175       | Br = 0.0000 +/- 0.0000       | Br = 0.0073 +/- 0.0052       |

--

pi:omega[-] pi:phi[+] lower half-plane

```
sqrt(s)_pole = (0.24495 +/- 0.00068521)
               + (i/2)*(-0.008919 +/- 0.0010286) [ 0.41]
```

```
s_pole = (0.059981 +/- 0.00033757)
          + i*(-0.0021847 +/- 0.00024954) [ 0.40]
```

| pi:omega                 | pi:phi                   |
|--------------------------|--------------------------|
| =====                    | =====                    |
| k_re= 0.0461 +/- 0.0008  | k_re= -0.0100 +/- 0.0009 |
| k_im= -0.0053 +/- 0.0006 | k_im= 0.0215 +/- 0.0015  |
| corr= [ 0.44]            | corr= [-0.00]            |

| pi:omega/3^S_1(*)             | pi:phi/3^S_1                 | pi:omega/3^D_1                |
|-------------------------------|------------------------------|-------------------------------|
| =====                         | =====                        | =====                         |
| g = 0.0688 +/- 0.0037         | g = 0.0000 +/- 0.0000        | g = 0.0065 +/- 0.0024         |
| arg(g)/pi= -0.1101 +/- 0.0197 | arg(g)/pi= 0.6101 +/- 0.0197 | arg(g)/pi= -0.6377 +/- 0.0221 |
| -----                         | -----                        | -----                         |
| g_re= 0.0647 +/- 0.0043       | g_re= -0.0000 +/- 0.0000     | g_re= -0.0027 +/- 0.0013      |
| g_im= -0.0233 +/- 0.0037      | g_im= 0.0000 +/- 0.0000      | g_im= -0.0059 +/- 0.0020      |
| corr= [ 0.38]                 | corr= [-0.23]                | corr= [ 0.94]                 |
| -----                         | -----                        | -----                         |
| Br = 0.8104 +/- 0.0175        | Br = 0.0000 +/- 0.0000       | Br = 0.0073 +/- 0.0052        |

--

pi:omega[-] pi:phi[-] upper half-plane

```
sqrt(s)_pole = (0.19471 +/- 0.0024271)
               + (i/2)*(+4.6886e-14 +/- 2.3685e-11) [ 0.00]
```

```
s_pole = (0.037913 +/- 0.00094514)
          + i*(+9.1247e-15 +/- 4.6095e-12) [ 0.00]
```

| pi:omega                 | pi:phi                   |
|--------------------------|--------------------------|
| =====                    | =====                    |
| k_re= -0.0000 +/- 0.0000 | k_re= -0.0000 +/- 0.0000 |
| k_im= -0.0501 +/- 0.0017 | k_im= -0.0636 +/- 0.0009 |
| corr= [ 0.00]            | corr= [ 0.00]            |

| pi:omega/3^S_1(*)            | pi:phi/3^S_1                 | pi:omega/3^D_1               |
|------------------------------|------------------------------|------------------------------|
| =====                        | =====                        | =====                        |
| g = 0.1120 +/- 0.0050        | g = 0.0000 +/- 0.0000        | g = 0.0206 +/- 0.0074        |
| arg(g)/pi= 0.5000 +/- 0.0000 | arg(g)/pi= 0.0000 +/- 0.0000 | arg(g)/pi= 0.5000 +/- 0.0000 |



## 2 Unphysical Parameterizations

```

-----|-----|-----|
g_re=  0.0000 +/- 0.0000 | g_re=  0.0000 +/- 0.0000 | g_re=  0.0000 +/- 0.0000 |
g_im=  0.1120 +/- 0.0050 | g_im=  0.0000 +/- 0.0000 | g_im=  0.0206 +/- 0.0074 |
corr= [-1.00]           | corr= [ 0.00]           | corr= [-0.17]           |
-----|-----|-----|
Br =  0.0000 +/- 0.0000 | Br =  0.0000 +/- 0.0000 | Br =  0.0000 +/- 0.0000 |

--
pi:omega[-] pi:phi[-] upper half-plane

sqrt(s)_pole = (0.24495 +/- 0.00069035)
               + (i/2)*(+0.008919 +/- 0.00103) [-0.41]

s_pole = (0.059981 +/- 0.00034011)
         + i*(+0.0021847 +/- 0.00024984) [-0.40]

=====|=====|
pi:omega | pi:phi |
=====|=====|
k_re= -0.0461 +/- 0.0008 | k_re= -0.0100 +/- 0.0009 |
k_im= -0.0053 +/- 0.0006 | k_im= -0.0215 +/- 0.0015 |
corr= [-0.45]           | corr= [-0.00]           |

=====|=====|
pi:omega/3^S_1(*) | pi:phi/3^S_1 | pi:omega/3^D_1 |
=====|=====|
|g|=  0.0688 +/- 0.0037 | |g|=  0.0000 +/- 0.0000 | |g|=  0.0065 +/- 0.0024 |
arg(g)/pi= 0.1101 +/- 0.0196 | arg(g)/pi= 0.3899 +/- 0.0196 | arg(g)/pi= 0.6377 +/- 0.0222 |
-----|-----|-----|
g_re=  0.0647 +/- 0.0043 | g_re=  0.0000 +/- 0.0000 | g_re= -0.0027 +/- 0.0013 |
g_im=  0.0233 +/- 0.0037 | g_im=  0.0000 +/- 0.0000 | g_im=  0.0059 +/- 0.0020 |
corr= [-0.38]           | corr= [ 0.23]           | corr= [-0.93]           |
-----|-----|-----|
Br =  0.8104 +/- 0.0175 | Br =  0.0000 +/- 0.0000 | Br =  0.0073 +/- 0.0052 |

--
pi:omega[-] pi:phi[-] lower half-plane

sqrt(s)_pole = (0.24495 +/- 0.00069035)
               + (i/2)*(-0.008919 +/- 0.00103) [ 0.41]

s_pole = (0.059981 +/- 0.00034011)
         + i*(-0.0021847 +/- 0.00024984) [ 0.40]

=====|=====|
pi:omega | pi:phi |
=====|=====|
k_re=  0.0461 +/- 0.0008 | k_re=  0.0100 +/- 0.0009 |
k_im= -0.0053 +/- 0.0006 | k_im= -0.0215 +/- 0.0015 |
corr= [ 0.45]           | corr= [ 0.00]           |

=====|=====|
pi:omega/3^S_1(*) | pi:phi/3^S_1 | pi:omega/3^D_1 |
=====|=====|
|g|=  0.0688 +/- 0.0037 | |g|=  0.0000 +/- 0.0000 | |g|=  0.0065 +/- 0.0024 |
arg(g)/pi= -0.1101 +/- 0.0196 | arg(g)/pi= 0.6101 +/- 0.0196 | arg(g)/pi= -0.6377 +/- 0.0222 |
-----|-----|-----|
g_re=  0.0647 +/- 0.0043 | g_re= -0.0000 +/- 0.0000 | g_re= -0.0027 +/- 0.0013 |
g_im= -0.0233 +/- 0.0037 | g_im=  0.0000 +/- 0.0000 | g_im= -0.0059 +/- 0.0020 |
corr= [ 0.38]           | corr= [-0.23]           | corr= [ 0.93]           |
-----|-----|-----|
Br =  0.8104 +/- 0.0175 | Br =  0.0000 +/- 0.0000 | Br =  0.0073 +/- 0.0052 |

```



## 2.18 coupled\_po\_pp.3s1\_3d1.pole+G0\_3s1\_3sd1\_3S1.gorder0\_3s1+gorder1\_3s1.threshold\_sub

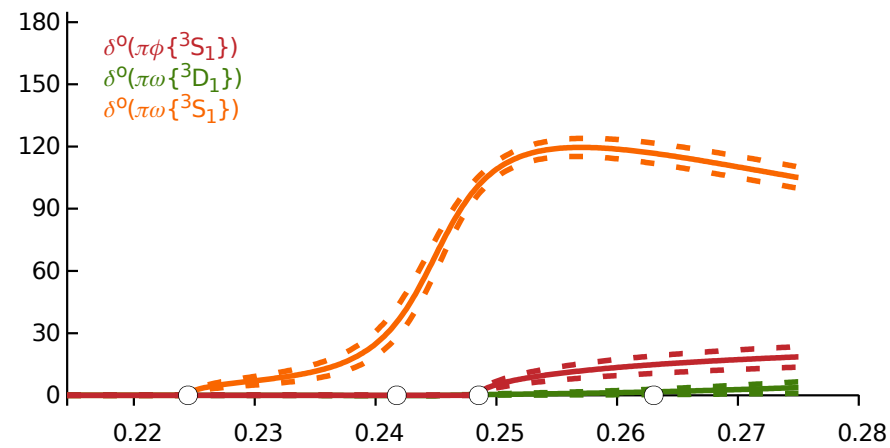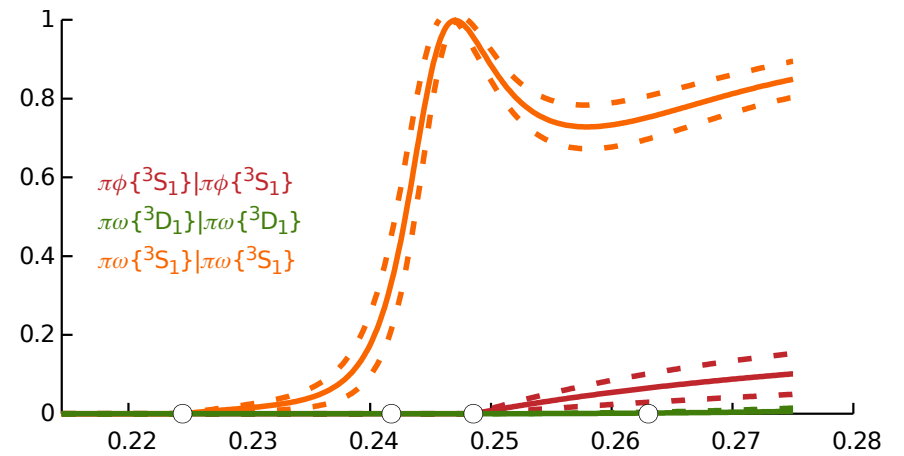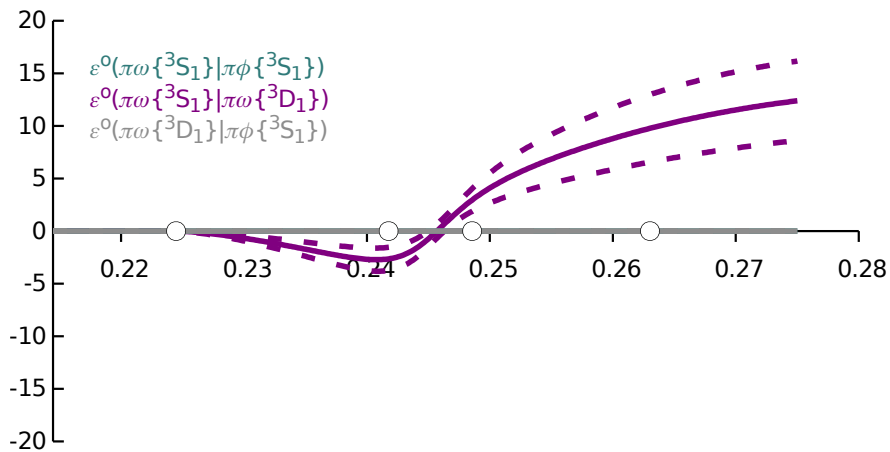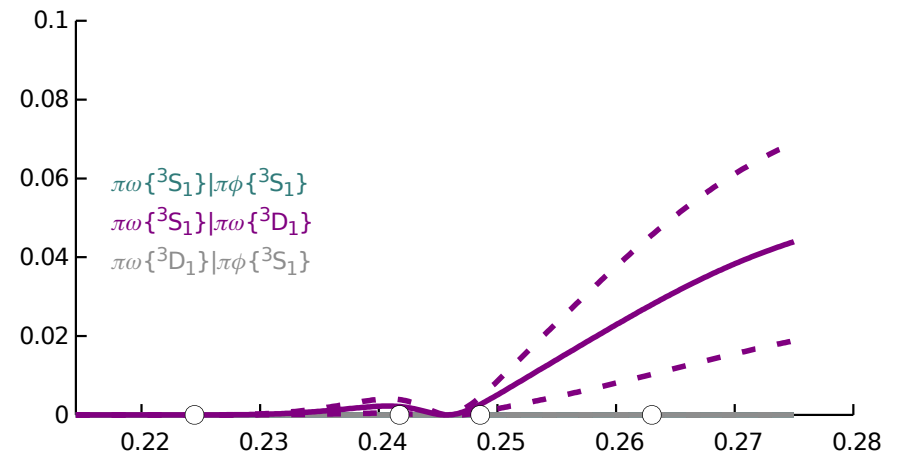



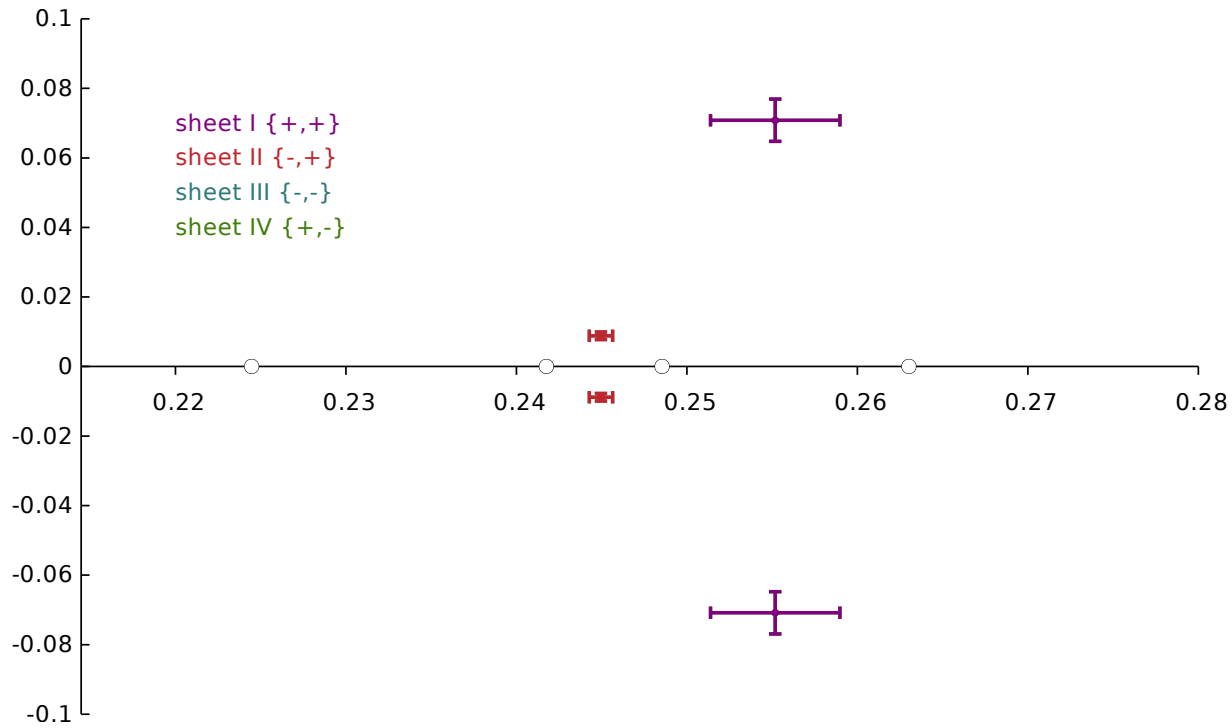

### parameter values

minimised with  $\text{chisq}/\text{nDoF} = 33.27 / (36 - 6) = 1.11$

|                                               |  |                        |  |      |       |       |       |       |       |
|-----------------------------------------------|--|------------------------|--|------|-------|-------|-------|-------|-------|
| JP1+_g_pi:omega/3^S_1_pole0_order0            |  | -0.50230 +/- 0.042477  |  | 1.00 | -0.99 | 0.31  | 0.24  | 0.05  | -0.17 |
| JP1+_g_pi:omega/3^S_1_pole0_order1            |  | 9.6054 +/- 0.66904     |  |      | 1.00  | -0.35 | -0.19 | -0.02 | 0.06  |
| JP1+_gamma_pi:omega/3^S_1 pi:omega/3^D_1_orde |  | -27.655 +/- 10.455     |  |      |       | 1.00  | 0.35  | -0.08 | -0.02 |
| JP1+_gamma_pi:omega/3^S_1 pi:omega/3^S_1_orde |  | 0.61835 +/- 0.17825    |  |      |       |       | 1.00  | 0.24  | -0.31 |
| JP1+_gamma_pi:phi/3^S_1 pi:phi/3^S_1_order0   |  | 0.93747 +/- 0.29453    |  |      |       |       |       | 1.00  | -0.27 |
| JP1+_m_pole0                                  |  | 0.24569 +/- 0.00060499 |  |      |       |       |       |       | 1.00  |

### pole singularities

pi:omega[+] pi:phi[+] upper half-plane

$\sqrt{s}_{\text{pole}} = (0.25518 \pm 0.003796)$   
 $+ (i/2)*(+0.070831 \pm 0.0060893)$  [ 0.75]

$s_{\text{pole}} = (0.063864 \pm 0.0017809)$   
 $+ i*(+0.018075 \pm 0.0017647)$  [ 0.76]

| pi:omega                | pi:phi                  |
|-------------------------|-------------------------|
| ===== =====             |                         |
| k_re= 0.0628 +/- 0.0037 | k_re= 0.0445 +/- 0.0041 |
| k_im= 0.0329 +/- 0.0019 | k_im= 0.0421 +/- 0.0016 |
| corr= [ 0.60]           | corr= [ 0.28]           |



| pi:omega/3^S_1(*)                                                    | pi:phi/3^S_1                                                         | pi:omega/3^D_1                                                       |
|----------------------------------------------------------------------|----------------------------------------------------------------------|----------------------------------------------------------------------|
| g = 0.1568 +/- 0.0079<br>arg(g)/pi= -0.2476 +/- 0.0051               | g = 0.0000 +/- 0.0000<br>arg(g)/pi= 0.7476 +/- 0.0051                | g = 0.0438 +/- 0.0119<br>arg(g)/pi= -0.2083 +/- 0.0157               |
| g_re= 0.1117 +/- 0.0049<br>g_im= -0.1100 +/- 0.0067<br>corr= [-0.86] | g_re= -0.0000 +/- 0.0000<br>g_im= 0.0000 +/- 0.0000<br>corr= [-0.86] | g_re= 0.0347 +/- 0.0099<br>g_im= -0.0267 +/- 0.0069<br>corr= [-0.93] |
| Br = 0.6072 +/- 0.0316                                               | Br = 0.0000 +/- 0.0000                                               | Br = 0.0474 +/- 0.0272                                               |

--

pi:omega[+] pi:phi[+] lower half-plane

$$\text{sqrt}(s)_{\text{pole}} = (0.25518 \pm 0.003796) + (i/2)(-0.070831 \pm 0.0060893) [-0.75]$$

$$s_{\text{pole}} = (0.063864 \pm 0.0017809) + i(-0.018075 \pm 0.0017647) [-0.76]$$

| pi:omega                                                             | pi:phi                                                               |
|----------------------------------------------------------------------|----------------------------------------------------------------------|
| k_re= -0.0628 +/- 0.0037<br>k_im= 0.0329 +/- 0.0019<br>corr= [-0.60] | k_re= -0.0445 +/- 0.0041<br>k_im= 0.0421 +/- 0.0016<br>corr= [-0.28] |

| pi:omega/3^S_1(*)                                                   | pi:phi/3^S_1                                                        | pi:omega/3^D_1                                                      |
|---------------------------------------------------------------------|---------------------------------------------------------------------|---------------------------------------------------------------------|
| g = 0.1568 +/- 0.0079<br>arg(g)/pi= 0.2476 +/- 0.0051               | g = 0.0000 +/- 0.0000<br>arg(g)/pi= 0.2524 +/- 0.0051               | g = 0.0438 +/- 0.0119<br>arg(g)/pi= 0.2083 +/- 0.0157               |
| g_re= 0.1117 +/- 0.0049<br>g_im= 0.1100 +/- 0.0067<br>corr= [ 0.86] | g_re= 0.0000 +/- 0.0000<br>g_im= 0.0000 +/- 0.0000<br>corr= [ 0.86] | g_re= 0.0347 +/- 0.0099<br>g_im= 0.0267 +/- 0.0069<br>corr= [ 0.93] |
| Br = 0.6072 +/- 0.0316                                              | Br = 0.0000 +/- 0.0000                                              | Br = 0.0474 +/- 0.0272                                              |

--

pi:omega[+] pi:phi[-] lower half-plane

$$\text{sqrt}(s)_{\text{pole}} = (0.25518 \pm 0.003796) + (i/2)(-0.070831 \pm 0.0060893) [-0.75]$$

$$s_{\text{pole}} = (0.063864 \pm 0.0017809) + i(-0.018075 \pm 0.0017647) [-0.76]$$

| pi:omega                                                             | pi:phi                                                               |
|----------------------------------------------------------------------|----------------------------------------------------------------------|
| k_re= -0.0628 +/- 0.0037<br>k_im= 0.0329 +/- 0.0019<br>corr= [-0.60] | k_re= 0.0445 +/- 0.0041<br>k_im= -0.0421 +/- 0.0016<br>corr= [-0.28] |

| pi:omega/3^S_1(*)                                                   | pi:phi/3^S_1                                                        | pi:omega/3^D_1                                                      |
|---------------------------------------------------------------------|---------------------------------------------------------------------|---------------------------------------------------------------------|
| g = 0.1568 +/- 0.0079<br>arg(g)/pi= 0.2476 +/- 0.0051               | g = 0.0000 +/- 0.0000<br>arg(g)/pi= 0.2524 +/- 0.0051               | g = 0.0438 +/- 0.0119<br>arg(g)/pi= 0.2083 +/- 0.0157               |
| g_re= 0.1117 +/- 0.0049<br>g_im= 0.1100 +/- 0.0067<br>corr= [ 0.86] | g_re= 0.0000 +/- 0.0000<br>g_im= 0.0000 +/- 0.0000<br>corr= [ 0.86] | g_re= 0.0347 +/- 0.0099<br>g_im= 0.0267 +/- 0.0069<br>corr= [ 0.93] |



## 2 Unphysical Parameterizations

```

Br = 0.6072 +/- 0.0316 | Br = 0.0000 +/- 0.0000 | Br = 0.0474 +/- 0.0272 |

--
pi:omega[+] pi:phi[-] upper half-plane

sqrt(s)_pole = (0.25518 +/- 0.003796)
+ (i/2)*(+0.070831 +/- 0.0060893) [ 0.75]

s_pole = (0.063864 +/- 0.0017809)
+ i*(+0.018075 +/- 0.0017647) [ 0.76]

=====
pi:omega | pi:phi |
=====
k_re= 0.0628 +/- 0.0037 | k_re= -0.0445 +/- 0.0041 |
k_im= 0.0329 +/- 0.0019 | k_im= -0.0421 +/- 0.0016 |
corr= [ 0.60] | corr= [ 0.28] |

=====
pi:omega/3^S_1(*) | pi:phi/3^S_1 | pi:omega/3^D_1 |
=====
|g|= 0.1568 +/- 0.0079 | |g|= 0.0000 +/- 0.0000 | |g|= 0.0438 +/- 0.0119 |
arg(g)/pi= -0.2476 +/- 0.0051 | arg(g)/pi= 0.7476 +/- 0.0051 | arg(g)/pi= -0.2083 +/- 0.0157 |
-----
g_re= 0.1117 +/- 0.0049 | g_re= -0.0000 +/- 0.0000 | g_re= 0.0347 +/- 0.0099 |
g_im= -0.1100 +/- 0.0067 | g_im= 0.0000 +/- 0.0000 | g_im= -0.0267 +/- 0.0069 |
corr= [-0.86] | corr= [-0.86] | corr= [-0.93] |
-----
Br = 0.6072 +/- 0.0316 | Br = 0.0000 +/- 0.0000 | Br = 0.0474 +/- 0.0272 |

--
pi:omega[-] pi:phi[+] lower half-plane

sqrt(s)_pole = (0.19502 +/- 0.0033682)
+ (i/2)*(-7.97e-17 +/- 3.9309e-14) [ 0.00]

s_pole = (0.038034 +/- 0.0013137)
+ i*(-1.555e-17 +/- 7.6706e-15) [ 0.00]

=====
pi:omega | pi:phi |
=====
k_re= 0.0000 +/- 0.0000 | k_re= -0.0000 +/- 0.0000 |
k_im= -0.0498 +/- 0.0024 | k_im= 0.0635 +/- 0.0012 |
corr= [ 0.00] | corr= [ 0.00] |

=====
pi:omega/3^S_1(*) | pi:phi/3^S_1 | pi:omega/3^D_1 |
=====
|g|= 0.1119 +/- 0.0045 | |g|= 0.0000 +/- 0.0000 | |g|= 0.0204 +/- 0.0073 |
arg(g)/pi= 0.5000 +/- 0.0000 | arg(g)/pi= 0.0000 +/- 0.0000 | arg(g)/pi= 0.5000 +/- 0.0000 |
-----
g_re= 0.0000 +/- 0.0000 | g_re= 0.0000 +/- 0.0000 | g_re= 0.0000 +/- 0.0000 |
g_im= 0.1119 +/- 0.0045 | g_im= 0.0000 +/- 0.0000 | g_im= 0.0204 +/- 0.0073 |
corr= [-1.00] | corr= [ 0.00] | corr= [-0.34] |
-----
Br = 0.0000 +/- 0.0000 | Br = 0.0000 +/- 0.0000 | Br = 0.0000 +/- 0.0000 |

--
pi:omega[-] pi:phi[+] upper half-plane

sqrt(s)_pole = (0.24496 +/- 0.00068038)
+ (i/2)*(+0.0088386 +/- 0.001092) [-0.40]

s_pole = (0.059986 +/- 0.00033531)
+ i*(+0.0021651 +/- 0.00026512) [-0.40]

```



| pi:omega                 | pi:phi                  |
|--------------------------|-------------------------|
| =====                    | =====                   |
| k_re= -0.0461 +/- 0.0008 | k_re= 0.0100 +/- 0.0009 |
| k_im= -0.0053 +/- 0.0007 | k_im= 0.0215 +/- 0.0015 |
| corr= [-0.43]            | corr= [ 0.06]           |

| pi:omega/3^S_1(*)            | pi:phi/3^S_1                 | pi:omega/3^D_1               |
|------------------------------|------------------------------|------------------------------|
| =====                        | =====                        | =====                        |
| g = 0.0684 +/- 0.0041        | g = 0.0000 +/- 0.0000        | g = 0.0065 +/- 0.0025        |
| arg(g)/pi= 0.1112 +/- 0.0186 | arg(g)/pi= 0.3888 +/- 0.0186 | arg(g)/pi= 0.6377 +/- 0.0209 |
| -----                        | -----                        | -----                        |
| g_re= 0.0643 +/- 0.0046      | g_re= 0.0000 +/- 0.0000      | g_re= -0.0027 +/- 0.0013     |
| g_im= 0.0234 +/- 0.0034      | g_im= 0.0000 +/- 0.0000      | g_im= 0.0059 +/- 0.0022      |
| corr= [-0.32]                | corr= [ 0.36]                | corr= [-0.94]                |
| -----                        | -----                        | -----                        |
| Br = 0.8095 +/- 0.0188       | Br = 0.0000 +/- 0.0000       | Br = 0.0074 +/- 0.0055       |

--

pi:omega[-] pi:phi[+] lower half-plane

```
sqrt(s)_pole = (0.24496 +/- 0.00068038)
               + (i/2)*(-0.0088386 +/- 0.001092) [ 0.40]
```

```
s_pole = (0.059986 +/- 0.00033531)
          + i*(-0.0021651 +/- 0.00026512) [ 0.40]
```

| pi:omega                 | pi:phi                   |
|--------------------------|--------------------------|
| =====                    | =====                    |
| k_re= 0.0461 +/- 0.0008  | k_re= -0.0100 +/- 0.0009 |
| k_im= -0.0053 +/- 0.0007 | k_im= 0.0215 +/- 0.0015  |
| corr= [ 0.43]            | corr= [-0.06]            |

| pi:omega/3^S_1(*)             | pi:phi/3^S_1                 | pi:omega/3^D_1                |
|-------------------------------|------------------------------|-------------------------------|
| =====                         | =====                        | =====                         |
| g = 0.0684 +/- 0.0041         | g = 0.0000 +/- 0.0000        | g = 0.0065 +/- 0.0025         |
| arg(g)/pi= -0.1112 +/- 0.0186 | arg(g)/pi= 0.6112 +/- 0.0186 | arg(g)/pi= -0.6377 +/- 0.0209 |
| -----                         | -----                        | -----                         |
| g_re= 0.0643 +/- 0.0046       | g_re= -0.0000 +/- 0.0000     | g_re= -0.0027 +/- 0.0013      |
| g_im= -0.0234 +/- 0.0034      | g_im= 0.0000 +/- 0.0000      | g_im= -0.0059 +/- 0.0022      |
| corr= [ 0.32]                 | corr= [-0.36]                | corr= [ 0.94]                 |
| -----                         | -----                        | -----                         |
| Br = 0.8095 +/- 0.0188        | Br = 0.0000 +/- 0.0000       | Br = 0.0074 +/- 0.0055        |

--

pi:omega[-] pi:phi[-] upper half-plane

```
sqrt(s)_pole = (0.19502 +/- 0.0033682)
               + (i/2)*(+1.9533e-14 +/- 9.7189e-12) [ 0.00]
```

```
s_pole = (0.038034 +/- 0.0013137)
          + i*(+3.8068e-15 +/- 1.8941e-12) [ 0.00]
```

| pi:omega                 | pi:phi                   |
|--------------------------|--------------------------|
| =====                    | =====                    |
| k_re= -0.0000 +/- 0.0000 | k_re= -0.0000 +/- 0.0000 |
| k_im= -0.0498 +/- 0.0024 | k_im= -0.0635 +/- 0.0012 |
| corr= [ 0.00]            | corr= [ 0.00]            |

| pi:omega/3^S_1(*)            | pi:phi/3^S_1                 | pi:omega/3^D_1               |
|------------------------------|------------------------------|------------------------------|
| =====                        | =====                        | =====                        |
| g = 0.1119 +/- 0.0045        | g = 0.0000 +/- 0.0000        | g = 0.0204 +/- 0.0073        |
| arg(g)/pi= 0.5000 +/- 0.0000 | arg(g)/pi= 0.0000 +/- 0.0000 | arg(g)/pi= 0.5000 +/- 0.0000 |



## 2 Unphysical Parameterizations

```

-----|-----|-----|
g_re=  0.0000 +/- 0.0000 | g_re=  0.0000 +/- 0.0000 | g_re=  0.0000 +/- 0.0000 |
g_im=  0.1119 +/- 0.0045 | g_im=  0.0000 +/- 0.0000 | g_im=  0.0204 +/- 0.0073 |
corr= [-1.00]           | corr= [ 0.00]           | corr= [-0.34]           |
-----|-----|-----|
Br =  0.0000 +/- 0.0000 | Br =  0.0000 +/- 0.0000 | Br =  0.0000 +/- 0.0000 |

--
pi:omega[-] pi:phi[-] upper half-plane

sqrt(s)_pole = (0.24496 +/- 0.00068038)
               + (i/2)*(+0.0088386 +/- 0.001092) [-0.40]

s_pole = (0.059986 +/- 0.00033531)
         + i*(+0.0021651 +/- 0.00026512) [-0.40]

=====|=====|
pi:omega | pi:phi |
=====|=====|
k_re= -0.0461 +/- 0.0008 | k_re= -0.0100 +/- 0.0009 |
k_im= -0.0053 +/- 0.0007 | k_im= -0.0215 +/- 0.0015 |
corr= [-0.43]           | corr= [ 0.06]           |

=====|=====|
pi:omega/3^S_1(*) | pi:phi/3^S_1 | pi:omega/3^D_1 |
=====|=====|=====|
|g|=  0.0684 +/- 0.0041 | |g|=  0.0000 +/- 0.0000 | |g|=  0.0065 +/- 0.0025 |
arg(g)/pi= 0.1112 +/- 0.0186 | arg(g)/pi= 0.3888 +/- 0.0186 | arg(g)/pi= 0.6377 +/- 0.0209 |
-----|-----|-----|
g_re=  0.0643 +/- 0.0046 | g_re=  0.0000 +/- 0.0000 | g_re= -0.0027 +/- 0.0013 |
g_im=  0.0234 +/- 0.0034 | g_im=  0.0000 +/- 0.0000 | g_im=  0.0059 +/- 0.0022 |
corr= [-0.32]           | corr= [ 0.36]           | corr= [-0.94]           |
-----|-----|-----|
Br =  0.8095 +/- 0.0188 | Br =  0.0000 +/- 0.0000 | Br =  0.0074 +/- 0.0055 |

--
pi:omega[-] pi:phi[-] lower half-plane

sqrt(s)_pole = (0.24496 +/- 0.00068038)
               + (i/2)*(-0.0088386 +/- 0.001092) [ 0.40]

s_pole = (0.059986 +/- 0.00033531)
         + i*(-0.0021651 +/- 0.00026512) [ 0.40]

=====|=====|
pi:omega | pi:phi |
=====|=====|
k_re=  0.0461 +/- 0.0008 | k_re=  0.0100 +/- 0.0009 |
k_im= -0.0053 +/- 0.0007 | k_im= -0.0215 +/- 0.0015 |
corr= [ 0.43]           | corr= [-0.06]           |

=====|=====|
pi:omega/3^S_1(*) | pi:phi/3^S_1 | pi:omega/3^D_1 |
=====|=====|=====|
|g|=  0.0684 +/- 0.0041 | |g|=  0.0000 +/- 0.0000 | |g|=  0.0065 +/- 0.0025 |
arg(g)/pi= -0.1112 +/- 0.0186 | arg(g)/pi= 0.6112 +/- 0.0186 | arg(g)/pi= -0.6377 +/- 0.0209 |
-----|-----|-----|
g_re=  0.0643 +/- 0.0046 | g_re= -0.0000 +/- 0.0000 | g_re= -0.0027 +/- 0.0013 |
g_im= -0.0234 +/- 0.0034 | g_im=  0.0000 +/- 0.0000 | g_im= -0.0059 +/- 0.0022 |
corr= [ 0.32]           | corr= [-0.36]           | corr= [ 0.94]           |
-----|-----|-----|
Br =  0.8095 +/- 0.0188 | Br =  0.0000 +/- 0.0000 | Br =  0.0074 +/- 0.0055 |

```
